# Supplementary material for: Non-freeness of groups generated by two parabolic elements with small rational parameters
Source: arXiv:1901.06375 ancillary file (2020-04-14)
Supplement: Supplementary file 1 [file relnum-v2.pdf]

**ANCILLARY DOCUMENT FOR**  
**NON-FREENESS OF GROUPS GENERATED BY TWO PARABOLIC**  
**ELEMENTS WITH SMALL RATIONAL PARAMETERS**

SANG-HYUN KIM AND THOMAS KOBERDA

1. MATHEMATICA (VERSION 11) CODE

Our computational heuristics can be summarized to definitions of five functions

$SR(x, y)$ ,  $RELNUM(s, r, M)$ ,  $MIN_3(a, b, c)$ ,  $RELNUMMIN(s, r, M)$ ,  $VERIFYLIST(s, T)$ .

The first four functions are introduced in Appendix of the paper “Non-freeness of groups generated by two parabolic elements with small rational parameters” (referred to as the Main Paper in this ancillary document). The detailed definitions and/or pseudo-code summaries of these functions can also be found in the Main Paper. We will explain the definition of  $VERIFYLIST(s, T)$  later in this document.

The following Mathematica code determines the above functions.

```
SR[x_Integer, y_Integer] := Module[{t}, t = x - y Floor[x/y];
Return[
  If[t == x + y || (t != x && Abs[t] <= Abs[y]/2), t, t - y]]];

RelNum[s_Integer, r_Integer, M_Integer] :=

Module[{flag, i, d, sg, S, x, y, Stemp},
  If[s/r >= 4 || IntegerQ[s/r] || GCD[r, s] != 1,
    Print["known cases"]; Return[]];
  x = r; y = (r - SR[r, s])/s; S = {{x, s y}}; i = 1; flag = False;
  While[i < M && ! flag, x = S[[i, 1]]; y = S[[i, 2]]/s;
    x = SR[x, s y];
    y = SR[r y, x]; x = r x;
    d = GCD[x, y]; sg = If[x >= 0, 1, -1];
    If[d != 0, x = x sg/d; y = y sg/d, x = x sg; y = y sg];
    Stemp = S;
    S = Append[S, {x, s y}];
    If[x y (Abs[x] - 1) == 0 || MemberQ[Stemp, {x, s y}]
      || MemberQ[Stemp, {x, -s y}],
```

---

2010 *Mathematics Subject Classification*. Primary: 30F35, 30F40; Secondary: 20E05, 11J70.

*Key words and phrases*. Fuchsian groups, Kleinian groups.

```

    Print[s/r, " is a relation number with a list ", S];
    flag = True]; i++;];
If[! flag,
    Print["No answers up to ", M, " iterations for ", s/r]];
Return[flag];];

```

Min3[a\_Integer, b\_Integer, c\_Integer] :=

```

Module[{ybound, y, t, x, xr, yr, min, minTemp},
    If[a b c == 0 || a < 0 || c < 0, Return[False]];
    If[Mod[b, a] == 0, Return[{-b/a, 1, c}]];
    ybound = Min[a - 2, c + Abs[c - Abs[a - Abs[b]]]];
    xr = 1; yr = 1; min = Abs[a + b + c];
    For[y = -ybound, y <= ybound, y++, If[y == 0, Continue[]];
        t = -(c/y + b)/a; x = Floor[t];
        If[x == 0 || (x != -1 && t - x > 1/2), x += 1];
        minTemp = Abs[(a x + b) y + c];
        If[minTemp < min, xr = x; yr = y; min = minTemp];];
    Return[{xr, yr, (a xr + b) yr + c}];];

```

RelNumMin[s\_Integer, r\_Integer, M\_Integer] :=

```

Module[{flag, i, d, sg, S, x, y, temp, u, v, xp, yp, Stemp},
    If[s/r >= 4 || IntegerQ[s/r] || GCD[r, s] != 1, Return[]];
    x = SR[r, s]; y = (r - SR[r, s])/s; sg = If[x >= 0, 1, -1];
    x = sg x; y = sg y; S = {{x, s y}}; i = 1; flag = False;
    If[y == 0, flag = True];
    While[i < M && ! flag, x = S[[i, 1]]; y = S[[i, 2]]/s;
        temp = Min3[s x, s r y, r x];
        u = temp[[1]]; v = temp[[2]]; xp = temp[[3]];
        yp = r y + u x;
        d = GCD[xp, yp]; sg = If[xp >= 0, 1, -1];
        If[d != 0, x = xp sg/d; y = yp sg/d, x = xp sg; y = yp sg];
        Stemp = S; S = Append[S, {x, s y}];
        If[x y (Abs[x] - 1) == 0 || MemberQ[Stemp, {x, s y}]
            || MemberQ[Stemp, {x, -s y}],
            Print[s/r, " is a relation number with a list ", S];
            flag = True]; i++;];
    If[! flag,
        Print["No answers up to ", M, " iterations for ", s/r]];
    Return[flag];];

```

VerifyList[s\_Integer, M\_Integer] :=

```

Module[{mList, mList2, lt, i, j, j2, lp, ltmp, w, flag, m, wp, d,
  DD, y, result, exc},
  exc = {}; result = {}; lp = {}; mList = Divisors[M];
  For[i = 2, i <= s - 2, i++,
    If[GCD[s, i] != 1, Continue[]];
    If[Mod[s + 1, i] == 0 || Mod[s - 1, i] == 0 ||
      Mod[s + 1, s - i] == 0 || Mod[s - 1, s - i] == 0, Continue[]];
    lp = Append[lp, i];];
  lt = lp; ltmp = {};
  For[i = 1, i < M, i++, lt = Union[lt, lp + s i];];
  For[i = 1, i <= Length[lt], i++,
    w = lt[[i]]; flag = False;
    If[Mod[w, s] == 0, flag = True;
      result = Append[result, {w, 1, 1}]; Continue[]];
  For[j = 1, j <= Length[mList] && ! flag, j++,
    m = mList[[j]];
    wp = Mod[w, s m]; d = GCD[s, wp]; DD = GCD[s m, wp];
    mList2 = Divisors[m d / DD];
    For[j2 = 1, j2 <= Length[mList2] && ! flag, j2++,
      y = mList2[[j2]];
      If[Mod[s m y + DD, wp] == 0 || Mod[s m y - DD, wp] == 0 ||
        Mod[s m y + DD, s m - wp] == 0 ||
        Mod[s m y - DD, s m - wp] == 0, flag = True;
        result = Append[result, {w, m, y}];
        exc = Union[
          exc, {{s, wp}, {s, s m - wp}, {s, DD}, {s, -DD}}]]];
    If[! flag, ltmp = Append[ltmp, i];];
  lt = Mod[lt[[ltmp]], s M];
  If[Length[lt] == 0,
    Return[{True, result, exc}];];
  Print["For s = ", s,
    ", the following remainders are not eliminated: ", lt,
    " modulo ", M, " * s "];
  Return[{False, lt}];];

```

## 2. INDIVIDUAL COMPUTER INPUTS AND OUTPUTS

Following the indexing in the Main Paper, let us include relevant computer inputs and outputs that are required for the proofs of results in Appendix of the Main Paper.

**2.1. Proof of Proposition A.2 (1).** The input (full) and the output (excerpt) below conclude that every rational number  $s/r \in (0, 4)$  satisfying  $2 \leq r \leq 10$  is a relation number, possibly except for  $s/r \in \{35/9, 39, 10\}$ . We also note that only  $M = 5000$

iterations suffice for the algorithm to terminate in this case. Only Algorithm 1 is used in this computation.

Here is the input.

```
excp={};
For[r = 2, r <= 10, r++, For[s = 2, s <= 4 r - 1, s++,
  If[!RelNum[s, r, 5000], excp=Append[excp, {s, r}]]];];
Print["Unresolved cases are :", excp, ": END"];
```

The relevant output for us is as below.

Unresolved cases are :{{35,9},{39,10}}: END

**2.2. Proof of Proposition A.2 (2).** Similarly to the previous subsection, we verify that every rational number  $s/r \in (0, 4)$  satisfying  $2 \leq s \leq 30$  and  $s/r \geq 1/10$  is a relation number, possibly except for  $s/r \in \{28/17, 29/17\}$ . Up to this point, only Algorithm 1 is used with at most 5000 iterations. Then, we feed the unresolved rational numbers  $\{28/17, 29/17\}$  to Algorithm 2 and see that these two numbers are also relation numbers.

Here is the input.

```
excp={};
For[s = 2, s <= 30, s++, For[r = 2, r <= 10 s, r++,
  If[GCD[s, r] == 1 && !RelNum[s, r, 5000],
    excp=Append[excp, {s, r}]]];];
Print["Unresolved cases are :", excp, ": END"];
```

The relevant output for us is as below.

Unresolved cases are :{{28,17},{29,17}}: END

Then we make another input as below.

```
RelNumMin[28, 17, 10];
RelNumMin[29, 17, 10];
```

We have the output

```
28/17 is a relation number with a list {{11,-28},{19,-168},
{13,-336},{3,-112},{5,-28},{1,84}}
29/17 is a relation number with a list {{12,-29},{1,203}}
```

This completes the proof.

**2.3. Proof of Proposition B.1.** Let us first explain the function  $\text{VERIFYLIST}(s, T)$ . Fix positive integers  $s$  and  $T$ . Then for each choice of  $w \in [1, sT]$  with  $\gcd(w, s) = 1$ , this function tries to find a triple  $(w', m, y)$  satisfying the conditions (i) through (iii) of Claim 1 in Appendix of the Main Paper. If this trial succeeds for all choices of  $w$ , then the function outputs a list of  $(w, m, y)$  that certifies each  $(w; sm)$  is a  $s$ -good residue class, and also certifies the union of all such residue classes cover  $\mathbb{Z}$ .

After running  $\text{VERIFYLIST}(s, t_s)$  for the range  $12 \leq s \leq 27$  and for specific choices  $t_s$  given in the Main Paper, then we verify Part (iv) of Claim 1.

This whole process is done by the following Mathematica input.

```
listgood = {};
excp = {}; excp2 = {}; T = {2, 2, 2, 2, 2, 3, 6, 2, 4, 6, 12, 12,
    1680, 6, 60, 60};
For[s = 12, s <= 27, s++,
    l0 = VerifyList[s, T[[s - 11]]]; l = l0[[2]]; flag = l0[[1]];
    If[flag, listgood = Append[listgood, s];
        Print[s, "/r is a relation number for almost all r;"];
        Print["this is certified by the list of s-good cosets ", l];
        excp = Union[excp, l0[[3]]];];
Print["The list of s such that s/r is a relation number
    for almost all r:"];
Print[listgood];
Print["Pairs of (s,r) that require individual verifications:", excp];
For[i = 1, i <= Length[excp], i++, s = excp[[i, 1]];
    r = excp[[i, 2]];
    If[! RelNum[s, Abs[r], 5000],
        Print["No answer found for s/r = ", s/r];
        excp2 = Append[excp2, {s, r}]]];
If[excp2 == {}, Print["Individual verification is complete."]];
```

The relevant output for us is as below.

The list of s such that s/r is a relation number  
for almost all r:  
{12,13,14,15,16,17,18,19,20,21,22,23,25,26,27}

This completes the proof of Parts (i) through (iv) of Claim.

### 3. THE FULL OUTPUT OF THE CODE

For completeness, let us include the full outputs of the inputs from the previous section below.

```

ln[19]:= excp = {};
For[r = 2, r ≤ 10, r++, For[s = 2, s ≤ 4 r - 1, s++,
    If[! RelNum[s, r, 5000], excp = Append[excp, {s, r}]]]];
Print["Unresolved cases are :", excp, ": END"];

known cases
 $\frac{3}{2}$  is a relation number with a list {{2, 3}, {1, 0}}

known cases
 $\frac{5}{2}$  is a relation number with a list {{2, 5}, {6, 5}, {1, 0}}

known cases
 $\frac{7}{2}$  is a relation number with a list
{{2, 7}, {10, 21}, {22, 35}, {26, 21}, {10, 7}, {6, -7}, {1, 0}}

 $\frac{2}{3}$  is a relation number with a list {{3, 2}, {1, 0}}

known cases
 $\frac{4}{3}$  is a relation number with a list {{3, 4}, {1, 0}}

 $\frac{5}{3}$  is a relation number with a list {{3, 5}, {6, 5}, {1, 0}}

known cases
 $\frac{7}{3}$  is a relation number with a list {{3, 7}, {12, 7}, {6, 7}, {1, 0}}

 $\frac{8}{3}$  is a relation number with a list {{3, 8}, {15, 16}, {1, 0}}

known cases
 $\frac{10}{3}$  is a relation number with a list
{{3, 10}, {21, 40}, {57, 70}, {39, 50}, {33, -40}, {21, -20}, {1, 0}}

 $\frac{11}{3}$  is a relation number with a list {{3, 11}, {24, 55}, {93, 176}, {249, 385},
{408, 341}, {201, 286}, {255, 77}, {24, -11}, {6, 11}, {15, 22}, {21, 11}, {1, 0}}

known cases
 $\frac{3}{4}$  is a relation number with a list {{4, 3}, {1, 0}}

known cases
 $\frac{5}{4}$  is a relation number with a list {{4, 5}, {1, 0}}

known cases
 $\frac{7}{4}$  is a relation number with a list {{4, 7}, {12, -7}, {1, 0}}

known cases

```

$\frac{9}{4}$  is a relation number with a list  $\{\{4, 9\}, \{20, 9\}, \{1, 0\}\}$

known cases

$\frac{11}{4}$  is a relation number with a list  $\{\{4, 11\}, \{28, 33\}, \{10, -11\}, \{1, 0\}\}$

known cases

$\frac{13}{4}$  is a relation number with a list  $\{\{4, 13\}, \{36, 65\}, \{116, 117\}, \{1, 0\}\}$

known cases

$\frac{15}{4}$  is a relation number with a list

$\{\{4, 15\}, \{44, 105\}, \{244, 495\}, \{1004, 1785\}, \{3124, 4575\},$   
 $\{5804, 3465\}, \{2252, 1515\}, \{2948, -4995\}, \{8188, -10725\}, \{10148, 4845\},$   
 $\{916, -615\}, \{1204, 2055\}, \{3404, 4545\}, \{4564, -1065\}, \{304, 75\}, \{1, 0\}\}$

$\frac{2}{5}$  is a relation number with a list  $\{\{5, 4\}, \{1, 0\}\}$

$\frac{3}{5}$  is a relation number with a list  $\{\{5, 6\}, \{1, 0\}\}$

$\frac{4}{5}$  is a relation number with a list  $\{\{5, 4\}, \{1, 0\}\}$

known cases

$\frac{6}{5}$  is a relation number with a list  $\{\{5, 6\}, \{1, 0\}\}$

$\frac{7}{5}$  is a relation number with a list  $\{\{5, 7\}, \{10, 7\}, \{15, -7\}, \{1, 0\}\}$

$\frac{8}{5}$  is a relation number with a list  $\{\{5, 8\}, \{15, 8\}, \{1, 0\}\}$

$\frac{9}{5}$  is a relation number with a list  $\{\{5, 9\}, \{20, -9\}, \{10, 9\}, \{1, 0\}\}$

known cases

$\frac{11}{5}$  is a relation number with a list

$\{\{5, 11\}, \{30, 11\}, \{15, 11\}, \{20, 11\}, \{10, 11\}, \{1, 0\}\}$

$\frac{12}{5}$  is a relation number with a list  $\{\{5, 12\}, \{35, 24\}, \{55, -12\}, \{1, 0\}\}$

$\frac{13}{5}$  is a relation number with a list  $\{\{5, 13\}, \{40, 39\}, \{1, 0\}\}$

$\frac{14}{5}$  is a relation number with a list  $\{\{5, 14\}, \{45, 56\}, \{55, 28\}, \{1, 0\}\}$

known cases

$\frac{16}{5}$  is a relation number with a list  $\{\{5, 16\}, \{55, 96\}, \{205, 176\}, \{145, -48\}, \{1, 0\}\}$

$\frac{17}{5}$  is a relation number with a list  $\{\{5, 17\}, \{60, 119\}, \{295, 408\},$   
 $\{565, -119\}, \{30, 17\}, \{20, -17\}, \{15, 17\}, \{10, 17\}, \{35, 34\}, \{1, 0\}\}$

$\frac{18}{5}$  is a relation number with a list  $\{\{5, 18\}, \{65, 144\}, \{395, 702\}, \{1535, 2016\}, \{2405, -1422\}, \{2195, -792\}, \{905, 702\}, \{1015, -144\}, \{35, 36\}, \{1, 0\}\}$

$\frac{19}{5}$  is a relation number with a list  $\{\{5, 19\}, \{70, 171\}, \{505, 1064\}, \{2795, 5301\}, \{12\,530, 21\,109\}, \{42\,895, 57\,456\}, \{72\,805, -10\,621\}, \{7710, -5491\}, \{11\,095, 14\,706\}, \{18\,055, -4921\}, \{8145, -6346\}, \{8995, 2451\}, \{4045, 3116\}, \{4645, -2071\}, \{2515, -798\}, \{605, 608\}, \{15, -19\}, \{20, 19\}, \{1, 0\}\}$

known cases

known cases

known cases

$\frac{5}{6}$  is a relation number with a list  $\{\{6, 5\}, \{1, 0\}\}$

known cases

$\frac{7}{6}$  is a relation number with a list  $\{\{6, 7\}, \{1, 0\}\}$

known cases

known cases

known cases

$\frac{11}{6}$  is a relation number with a list  $\{\{6, 11\}, \{30, -11\}, \{1, 0\}\}$

known cases

$\frac{13}{6}$  is a relation number with a list  $\{\{6, 13\}, \{42, 13\}, \{1, 0\}\}$

known cases

known cases

known cases

$\frac{17}{6}$  is a relation number with a list  $\{\{6, 17\}, \{66, 85\}, \{57, 68\}, \{33, -17\}, \{1, 0\}\}$

known cases

$\frac{19}{6}$  is a relation number with a list  $\{\{6, 19\}, \{78, 133\}, \{330, 247\}, \{498, -95\}, \{138, -133\}, \{15, -19\}, \{12, 19\}, \{42, 19\}, \{12, 19\}\}$

known cases

known cases

known cases



```

23
— is a relation number with a list
6
{{6, 23}, {102, 253}, {906, 1955}, {6294, 12397}, {36618, 65987}, {176214, 279565},
{620106, 699683}, {238731, -268778}, {90141, 115253}, {75336, -56971},
{110190, 80569}, {177726, -197869}, {40286, -67551}, {163590, -221789},
{349194, -7843}, {7482, -12995}, {33078, -48829}, {94506, -69299},
{151242, 163967}, {25450, -35259}, {58854, -14053}, {3963, -5888}, {11550, -8947},
{15618, 6187}, {5886, 10189}, {25818, 37835}, {72102, 49381}, {136326, -226297},
{539826, -711551}, {1030350, 319631}, {47638, 30475}, {39936, 61663},
{130362, 129743}, {3714, -4577}, {5178, 7613}, {14610, 10327}, {25698, -36547},
{65094, -30245}, {13812, 15157}, {2690, 621}, {309, -253}, {168, -115}, {318, 529},
{1266, 1679}, {2478, -575}, {267, 161}, {330, 299}, {62, -115}, {318, -529}}

2
— is a relation number with a list {{7, 6}, {1, 0}}
7

3
— is a relation number with a list {{7, 6}, {1, 0}}
7

4
— is a relation number with a list {{7, 8}, {1, 0}}
7

5
— is a relation number with a list {{7, 5}, {14, 5}, {1, 0}}
7

6
— is a relation number with a list {{7, 6}, {1, 0}}
7

known cases

8
— is a relation number with a list {{7, 8}, {1, 0}}
7

9
— is a relation number with a list {{7, 9}, {14, 9}, {28, 9}, {1, 0}}
7

10
— is a relation number with a list {{7, 10}, {21, -10}, {1, 0}}
7

11
— is a relation number with a list
7
{{7, 11}, {28, 11}, {35, -22}, {63, -44}, {133, -99}, {238, 55}, {126, -11}, {35, -22}}

12
— is a relation number with a list {{7, 12}, {35, -24}, {77, -36}, {35, -12}, {1, 0}}
7

13
— is a relation number with a list
7
{{7, 13}, {42, -13}, {21, -13}, {35, 26}, {63, -52}, {77, 65}, {84, -13}, {42, -13}}

known cases

15
— is a relation number with a list {{7, 15}, {56, 15}, {28, 15}, {14, 15}, {1, 0}}
7

16
— is a relation number with a list {{7, 16}, {63, 32}, {1, 0}}
7

17
— is a relation number with a list
7
{{7, 17}, {70, 51}, {133, 34}, {21, 17}, {28, -17}, {42, 17}, {56, -17}, {35, -34}, {1, 0}}

```

$\frac{18}{7}$  is a relation number with a list  $\{\{7, 18\}, \{77, 72\}, \{35, -36\}, \{1, 0\}\}$

$\frac{19}{7}$  is a relation number with a list  $\{\{7, 19\}, \{84, 95\}, \{77, -38\}, \{1, 0\}\}$

$\frac{20}{7}$  is a relation number with a list

$\{\{7, 20\}, \{91, 120\}, \{203, -260\}, \{399, -460\}, \{427, -440\}, \{91, -40\}, \{77, -60\},$   
 $\{119, -80\}, \{273, 220\}, \{371, 480\}, \{763, 1000\}, \{1659, -2260\}, \{4207, 3800\},$   
 $\{2849, 2180\}, \{4683, 1880\}, \{6461, -5300\}, \{8127, 9340\}, \{8491, 7400\},$   
 $\{7637, 8160\}, \{3661, -4820\}, \{8113, 10560\}, \{17129, 23960\}, \{47817, -31100\},$   
 $\{100681, -69960\}, \{215047, 124700\}, \{240471, -185840\}, \{382417, -208260\},$   
 $\{238721, 93700\}, \{296653, 191680\}, \{606949, 392380\}, \{1244677, 809560\},$   
 $\{2621101, 1821940\}, \{5594127, -3229640\}, \{6056071, 5304420\}, \{5261557, 7064900\},$   
 $\{12623401, -13387440\}, \{5348273, 2027400\}, \{5137489, 486740\}, \{1516557, 925840\},$   
 $\{2345861, 221580\}, \{640633, 279320\}, \{573951, 315380\}, \{397663, 64700\},$   
 $\{66241, 74380\}, \{56973, -32320\}, \{53669, 72900\}, \{134617, -125680\},$   
 $\{62559, 13940\}, \{47593, -38400\}, \{64351, -84940\}, \{144123, 182800\},$   
 $\{270739, 267480\}, \{22813, -17860\}, \{34671, -25960\}, \{60977, -7500\},$   
 $\{6839, 6120\}, \{5033, -300\}, \{469, -580\}, \{777, -380\}, \{119, 60\}, \{1, 0\}\}$

known cases

$\frac{22}{7}$  is a relation number with a list

$\{\{7, 22\}, \{105, 176\}, \{497, 330\}, \{1141, 1276\}, \{945, -22\}, \{1, 0\}\}$

$\frac{23}{7}$  is a relation number with a list

$\{\{7, 23\}, \{112, 207\}, \{665, 736\}, \{497, -253\}, \{63, -92\}, \{203, -23\}, \{28, -23\},$   
 $\{35, -46\}, \{77, 69\}, \{56, -69\}, \{91, -115\}, \{168, 253\}, \{595, 184\}, \{301, 299\}, \{14, 23\},$   
 $\{63, 46\}, \{119, -69\}, \{133, 46\}, \{35, 23\}, \{77, 92\}, \{105, 46\}, \{91, 23\}, \{1, 0\}\}$

$\frac{24}{7}$  is a relation number with a list  $\{\{7, 24\}, \{119, 240\},$

$\{847, 1224\}, \{2639, 480\}, \{1673, -2376\}, \{4921, -240\}, \{17, -24\}, \{1, 0\}\}$

$\frac{25}{7}$  is a relation number with a list

```
{ {7, 25}, {126, 275}, {1043, 1800}, {5299, 6325}, {7182, 7025}, {1099, -1850},
  {5257, -5825}, {3976, -1825}, {2282, 3525}, {8701, 6400}, {16107, -12725},
  {23674, -4525}, {7343, -5450}, {13251, 9175}, {28532, -37675},
  {64001, 35150}, {44093, 68900}, {173649, 137875}, {250418, 70775},
  {228774, 321625}, {649957, 69900}, {145999, -32125}, {102382, -140775},
  {268751, 25600}, {89257, -139575}, {352226, -280925}, {499107, -183950},
  {369201, -30925}, {13293, -20900}, {53249, -43875}, {65618, -72775},
  {50099, -27350}, {32207, -38600}, {44751, -49450}, {32893, -6275},
  {10626, -5975}, {9268, 8725}, {3801, 6775}, {20818, 26925}, {42749, -35800},
  {48643, -76875}, {197624, -167675}, {209643, 323725}, {798574, 585975},
  {1488193, -1213150}, {1925301, -1615975}, {2165282, -3578675},
  {9893751, -10284100}, {390349, 525375}, {945182, -301975}, {274799, -150975},
  {190057, -300725}, {774676, -661625}, {791357, 1021175}, {1608726, -1402775},
  {1441657, 478125}, {50974, 69975}, {133007, -14800}, {193, 325}, {924, 1025},
  {707, 400}, {651, -475}, {1232, 1075}, {1099, -325}, {868, 825}, {301, 400},
  {693, -325}, {301, -125}, {357, 400}, {301, 425}, {868, 125}, {1, 0}}
```

$\frac{26}{7}$  is a relation number with a list

```
{ {7, 26}, {133, 312}, {1253, 2470}, {8519, 14352}, {40831, 51194},
  {72541, -88920}, {114653, 196586}, {573531, 754156}, {1264375, -582842},
  {690837, 1052038}, {2528407, 2026960}, {3510129, 1151098}, {397845, 669136},
  {1899037, 2369614}, {3294039, -4352296}, {7407799, 2951390},
  {10124597, 16945916}, {47749233, 58732882}, {76885543, -125555300},
  {340688299, -386526582}, {320867981, 322095358}, {8591639, 11070436},
  {17351579, -13044330}, {30150743, 20678164}, {66308053, -101539906},
  {246622971, -205248836}, {289618945, -361014342}, {499767779, 670820072},
  {1197366051, -248380886}, {311768653, -577329506}, {1858925971, -2863275636},
  {7030447655, -6070161838}, {6722000719, 7443729618}, {5052102293, 4188746796},
  {6043488479, 6873984650}, {5813473197, -4932091658}, {6169670773, 11307198422},
  {35962693543, 54425329920}, {129238454639, 99051236362},
  {211310527939, -91509020668}, {198047406221, 95041507002},
  {55750745519, 44067956088}, {81779526017, 4723167410},
  {10399760329, -5565509352}, {5118808625, 933129964}, {3172111635, -5250219182},
  {14546752829, -17279261948}, {19127563833, -21135640552},
  {14056537033, -8680500218}, {23131243821, -25152546952},
  {14149121917, 18406184446}, {29799437703, -18159665368},
  {45639251231, -42399561282}, {22677829643, 40130825722},
  {122170972553, 172862118000}, {354838018129, 107934955622},
  {217232058841, -51317243484}, {83741594335, -48180496858},
  {88335795667, 9159094100}, {22786017331, 20520119958},
  {15861281611, 25814176310}, {69670262893, 78076028004},
  {58840355777, 109117482630}, {351939887971, 543382919768},
  {1340101222579, 117383838346}, {1163839839631, -428798661694},
  {857893018157, -184869149868}, {465169118281, -433686961682},
  {220375096193, 238335554522}, {125723208303, 199538784562},
  {516709033813, 522433490800}, {40071198909, 63862605950},
  {166539849287, 171538341416}, {34989444903, -31121231726},
  {27077492239, -16701536878}, {44279070619, -47554361296},
  {22927034739, -7749701336}, {2254484883, 4005103388},
```

{12 254 329 535, 17 480 357 414}, {36 582 195 153, 13 514 222 956},  
 {27 723 316 005, 8 372 755 898}, {18 235 338 177, -9 121 964 800}, {60 139 961, -32 067 828},  
 {27 969 865, 16 698 656}, {37 992 129, 24 223 030}, {73 177 517, 102 240 996},  
 {203 444 353, 39 963 482}, {25 388 601, -3 157 180}, {918 127, -1 639 144},  
 {5 047 119, -7 272 434}, {15 577 205, -6 951 152}, {11 724 307, -5 110 638},  
 {10 521 217, 3 304 340}, {4 257 379, 7 317 258}, {21 419 153, 28 336 048},  
 {48 418 265, -18 513 066}, {49 846 531, -55 552 796}, {39 943 855, -56 219 098},  
 {113 926 701, -29 622 632}, {31 946 789, -29 960 580}, {13 903 463, -3 158 324},  
 {8 891 169, 10 916 074}, {14 174 335, -23 764 988}, {67 134 571, -83 002 062},  
 {111 072 437, 168 459 668}, {401 710 617, 312 850 330}, {622 022 009, -120 415 152},  
 {139 623 743, 194 298 884}, {382 725 987, 61 461 478}, {97 699 833, 67 345 252},  
 {212 482 067, -317 802 342}, {737 241 925, -513 710 756}, {1 564 718 183, 2 215 835 102},  
 {4 557 818 433, 1 418 194 180}, {2 122 651 251, 2 043 226 042}, {79 425 209, -21 829 392},  
 {55 246 513, -52 395 590}, {19 956 461, 3 850 860}, {4 915 127, 8 699 834},  
 {26 492 949, 37 503 544}, {77 074 165, 23 750 662}, {40 755 253, 14 877 980},  
 {27 150 809, -3 299 998}, {5 255 775, -3 578 536}, {11 740 673, 18 558 462},  
 {47 724 523, 47 353 280}, {2 598 701, 3 294 148}, {4 868 129, -4 977 414}, {764 995, 744 978},  
 {140 119, 10 426}, {32 067, -46 124}, {98 399, -42 614}, {92 197, 44 148}, {27 307, 47 58},  
 {8687, -1040}, {2569, 2262}, {2149, -130}, {427, -676}, {1743, -1742}, {1, 0}

27  
 — is a relation number with a list  
 7

{{7, 27}, {140, 351}, {1477, 3240}, {12 341, 24 921}, {88 060, 165 213}, {540 071, 926 640},  
 {2 705 983, 3 950 883}, {8 714 300, 5 956 119}, {19 307 267, -32 778 054},  
 {94 295 509, -134 264 871}, {279 785 534, -139 318 677}, {8 037 260, -14 204 079},  
 {43 167 733, -67 075 560}, {167 354 789, -175 982 409}, {60 393 340, 67 148 163},  
 {47 283 761, 77 103 522}, {208 738 327, 265 408 893}, {396 693 962, -327 756 969},  
 {482 558 951, -432 999 972}, {346 912 853, -354 814 938}, {55 314 595, -76 570 974},  
 {148 794 653, -37 925 415}, {20 349 049, 30 010 338}, {67 629 023, 50 782 437},  
 {117 926 102, -99 380 763}, {129 817 373, -194 941 188}, {455 866 705, -393 754 689},  
 {434 784 112, 597 766 041}, {1 140 873 503, 216 149 796}, {420 871 661, -110 313 549},  
 {142 677 745, 221 866 398}, {554 320 571, 585 028 845}, {214 957 918, 50 415 075},  
 {93 083 326, -6 130 161}, {7 916 377, -12 376 530}, {31 221 071, -33 788 421},  
 {17 971 450, 28 563 597}, {74 145 029, 86 042 790}, {83 284 327, 40 179 564},  
 {20 476 393, -34 664 544}, {99 317 057, -140 428 269}, {287 778 484, -127 004 841},  
 {236 381 614, 22 723 767}, {64 007 608, -87 820 119}, {166 687 577, -28 196 964},  
 {17 459 449, -4 652 019}, {8 040 389, 1 551 204}, {1 990 583, 3 180 465},  
 {8 329 174, 9 863 559}, {10 740 695, 13 811 877}, {21 498 274, -13 761 225},  
 {42 169 232, -66 324 177}, {169 084 615, -187 914 276}, {131 807 627, -209 802 609},  
 {545 964 874, -637 246 251}, {638 969 639, -468 470 601}, {1 193 493 266, 1 324 179 819},  
 {914 805 871, 1 316 352 060}, {2 810 823 323, 1 627 282 683}, {3 106 194 301, 590 056 380},  
 {1 091 386 807, -79 240 167}, {17 975 531, 9 905 976}, {12 854 947, -19 758 465},  
 {48 324 626, -48 085 731}, {1 672 265, -1 191 537}, {3 365 096, 4 638 897},  
 {8 916 607, 1 920 348}, {4 795 931, 5 056 155}, {1 821 568, -262 845}, {2621, -2889},  
 {1876, -1485}, {2737, 162}, {119, -216}, {679, -1107}, {2996, -3807}, {5677, 4752},  
 {6475, 8289}, {12 698, -9045}, {25 571, 35 316}, {68 215, 15 903}, {32 221, -12 960},  
 {44 107, 79 407}, {247 100, 397 251}, {1 051 057, 1 273 320}, {1 555 841, -2 912 139},  
 {9 494 086, -16 235 073}, {47 186 909, -68 361 138}, {148 219 603, -93 176 217},  
 {266 929 817, -377 352 918}, {772 961 707, -339 953 301}, {651 385 735, 132 814 728},  
 {88 815 335, 98 017 209}, {64 413 118, 59 231 331}, {36 272 509, -5 105 430},  
 {534 499, -982 152}, {3 133 571, -5 211 567}, {14 545 972, -19 624 923},  
 {35 552 657, 242 784}, {743 351, -1 167 723}, {2 970 604, -3 283 983}, {2 193 653, -2 395 818},

```
{1415155, 395361}, {1164023, 1722276}, {3907771, 3016899}, {6236104, -2935251},
{2559214, -804249}, {1025269, -1675134}, {4549055, -5820417},
{8899534, 6416145}, {17383723, -22138488}, {33283355, 26590761},
{46848158, 5435289}, {14486101, 17827938}, {23392859, -34565967},
{78211756, -59712147}, {129497263, 81504414}, {234580955, 334281357},
{697902814, 351941355}, {41859272, -41731605}, {893669, 874530},
{133973, -79326}, {172753, -111051}, {345443, -555066}, {1467361, -1774359},
{2148986, 4131567}, {13878067, 24608718}, {75114557, 117466551},
{296463958, 321237981}, {173418161, -241970004}, {479862901, -157109733},
{59735914, 52281639}, {52179925, -36559377}, {109343836, 165839157},
{395467247, 364499568}, {216773753, 43114977}, {8392076, 10479915},
{14614873, -16987752}, {16610153, -9221202}, {12825757, 15077637},
{15763160, 16058061}, {294901, -133407}, {196609, -175500}, {147763, -88614},
{206255, -175257}, {216986, -389853}, {1210069, -1938438}, {5098583, -6096897},
{6988198, -11230677}, {29697353, -35932194}, {43643887, 83184651},
{276785348, 485308071}, {1459659061, 2232957024}, {5413085741, 5248345833},
{1153179356, 1154600703}, {9949429, 15208938}, {36816563, 35544177},
{1272386, 1189755}, {578417, -595863}, {122122, -68337}, {101864, 85455},
{114863, 155142}, {281953, 1539}, {2212, 2241}, {203, -27}, {91, -162}, {497, -783},
{2002, -2241}, {1673, 2781}, {7756, 10449}, {18851, -432}, {1099, -1215},
{812, -891}, {553, -162}, {469, 675}, {1442, 837}, {1624, 405}, {28, 27}, {1, 0}
```

known cases

```
3
- is a relation number with a list {{8, 9}, {1, 0}}
8
```

known cases

```
5
- is a relation number with a list {{8, 10}, {1, 0}}
8
```

known cases

```
7
- is a relation number with a list {{8, 7}, {1, 0}}
8
```

known cases

```
9
- is a relation number with a list {{8, 9}, {1, 0}}
8
```

known cases

```
11
- is a relation number with a list {{8, 11}, {24, 11}, {1, 0}}
8
```

known cases

```
13
- is a relation number with a list {{8, 13}, {20, 13}, {24, -13}, {1, 0}}
8
```

known cases

```
15
- is a relation number with a list {{8, 15}, {56, -15}, {1, 0}}
8
```

known cases

```
17
- is a relation number with a list {{8, 17}, {72, 17}, {1, 0}}
8
```

known cases

$\frac{19}{8}$  is a relation number with a list  $\{\{8, 19\}, \{88, 57\}, \{104, 19\}, \{72, -19\}, \{1, 0\}\}$

known cases

$\frac{21}{8}$  is a relation number with a list  $\{\{8, 21\}, \{104, 105\}, \{1, 0\}\}$

known cases

$\frac{23}{8}$  is a relation number with a list  
 $\{\{8, 23\}, \{120, 161\}, \{328, -345\}, \{136, 23\}, \{1, 0\}\}$

known cases

$\frac{25}{8}$  is a relation number with a list  $\{\{8, 25\}, \{136, 225\}, \{712, 425\}, \{552, 25\}, \{1, 0\}\}$

known cases

$\frac{27}{8}$  is a relation number with a list  
 $\{\{8, 27\}, \{152, 297\}, \{1160, 1539\}, \{3032, -2079\}, \{7624, 9099\}, \{5900, 3429\},$   
 $\{3832, -783\}, \{664, -459\}, \{1640, 1863\}, \{892, -1431\}, \{4312, -3105\},$   
 $\{9656, 7749\}, \{15256, 10503\}, \{38024, -44307\}, \{25132, 7587\},$   
 $\{18968, -3321\}, \{3832, 351\}, \{58, 81\}, \{184, -27\}, \{20, -27\}, \{56, 27\}, \{1, 0\}\}$

known cases

$\frac{29}{8}$  is a relation number with a list  
 $\{\{8, 29\}, \{168, 377\}, \{1672, 3045\}, \{10984, 15457\}, \{35784, 6061\}, \{2328, 1073\},$   
 $\{364, -493\}, \{1032, 203\}, \{136, 145\}, \{18, -29\}, \{88, -87\}, \{1, 0\}\}$

known cases

$\frac{31}{8}$  is a relation number with a list  
 $\{\{8, 31\}, \{184, 465\}, \{2248, 4991\}, \{21944, 45105\}, \{185288, 357151\},$   
 $\{1374904, 2470545\}, \{8765128, 14200511\}, \{43483064, 54892785\},$   
 $\{91277768, -85440929\}, \{11673678, 10060151\}, \{6454108, -9778733\},$   
 $\{26597000, -24833511\}, \{3526978, 5001137\}, \{11793272, 5689833\},$   
 $\{206803, -360530\}, \{1229816, -1881297\}, \{5211848, -5145535\}, \{132626, -12555\},$   
 $\{43832, -69409\}, \{204616, -237615\}, \{131996, -72509\}, \{52088, 88195\},$   
 $\{288856, 413757\}, \{999208, 561875\}, \{498168, -317099\}, \{544120, -840069\},$   
 $\{2367592, -2453867\}, \{690200, 909261\}, \{1752488, -483197\}, \{360600, -430931\},$   
 $\{281324, -456537\}, \{1401704, -1779307\}, \{3020824, 2528763\}, \{3936488, 4976213\},$   
 $\{8317800, -7578229\}, \{5916568, 8154271\}, \{17901624, 4134625\},$   
 $\{2726248, -2294961\}, \{3450296, -4989791\}, \{12315960, -7806017\},$   
 $\{13184296, -19865079\}, \{53446264, -48183641\}, \{21050492, -29593251\},$   
 $\{68342072, -28079521\}, \{48732120, 76518881\}, \{222294088, 249238543\},$   
 $\{107777820, -161676067\}, \{431185976, -377437121\}, \{214995420, 156466021\},$   
 $\{468235192, -562683201\}, \{377792036, -677155475\}, \{2394907512, -3863022809\},$   
 $\{11744922376, -14607391735\}, \{22899754872, 28122583751\},$   
 $\{41782631032, -63072974759\}, \{170322749816, -155416857465\},$   
 $\{119247138808, 142913128923\}, \{94663960460, 161993177873\},$   
 $\{538633739304, 791260316819\}, \{2021012620120, 1501341368413\},$   
 $\{4157370013656, -4099077855613\}, \{233168632172, -132799328455\},$

```

{129 720 098 952, 28 531 930 381}, {103 516 423 624, 172 870 698 495},
{554 834 198 968, 767 016 933 041}, {1 697 461 872 584, 441 529 291 935},
{17 163 823 789, 22 637 311 381}, {2 736 743 796, -713 773 481}, {118 350 128, -203 440 011},
{680 719 064, -1 010 266 285}, {2 636 377 768, -2 133 833 571}, {4 020 353 576, -1 491 798 461},
{3 640 334 456, -2 171 908 329}, {2 813 928 808, -2 216 340 815}, {4 780 703 944, 794 501 263},
{54 785 464, -6 400 043}, {22 519 384, -36 062 269}, {108 343 080, -131 331 283},
{183 905 624, 338 015 971}, {1 232 882 776, 2 073 292 989}, {6 723 281 704, 9 466 372 691},
{21 944 727 896, 9 304 839 069}, {13 340 199 032, -14 473 914 973},
{9 069 727 528, 10 355 737 271}, {5 144 038 972, -1 556 647 051},
{3 792 782 552, 2 243 855 981}, {2 779 717 640, 1 795 981 931}, {3 248 984 888, 5 405 888 717},
{17 255 230 632, 23 616 908 963}, {50 893 426 648, 8 276 756 557},
{2 465 774 612, -2 556 240 129}, {723 724 136, 818 903 843}, {380 718 828, -325 044 455},
{222 697 492, 425 727 743}, {1 624 242 008, 2 888 115 837}, {10 110 990 632, 16 075 162 003},
{47 713 370 968, 56 288 016 477}, {34 298 582 036, 40 661 944 871},
{25 453 451 340, 34 616 468 401}, {73 304 136 488, 7 121 781 683},
{8 345 278 632, -3 850 827 967}, {1 287 245 396, 2 274 495 885}, {7 898 003 912, 12 408 798 079},
{36 086 353 336, 40 564 234 545}, {17 911 524 836, -23 442 620 701},
{44 248 766 920, 16 076 993 793}, {31 857 715 672, -5 167 302 115},
{1 707 805 964, 2 900 891 991}, {9 544 688 216, 13 778 530 909}, {33 870 741 544, 21 020 876 211},
{32 684 043 512, 42 567 163 765}, {79 064 962 024, -34 160 582 277},
{42 975 189 880, 29 886 531 677}, {104 709 265 624, -166 656 150 877},
{495 575 082 024, -587 104 235 827}, {366 116 615 212, -488 986 824 585},
{982 961 674 984, 102 918 106 117}, {184 877 544 744, 304 728 061 415},
{958 804 133 368, 1 277 541 525 481}, {2 549 899 136 904, -339 473 048 345},
{165 885 249 856, -303 332 294 847}, {1 099 576 359 928, -1 834 200 035 945},
{5 876 989 408 136, -8 099 733 668 967}, {17 781 954 086 648, -4 107 202 734 025},
{2 706 286 301 096, 2 272 453 948 697}, {3 470 658 819 192, 4 730 828 665 207},
{10 081 358 768 120, 1 218 635 904 809}, {332 271 529 648, -68 916 272 577},
{98 478 665 896, 169 725 350 269}, {569 973 474 984, 850 844 413 411},
{2 246 967 507 416, 1 900 243 783 949}, {2 773 789 787 736, 4 453 514 844 115},
{13 437 800 451 032, 16 443 357 994 829}, {24 044 460 350 376, -38 374 580 100 925},
{114 640 958 004 392, -137 237 071 459 619}, {90 384 453 820 908, -151 531 231 273 561},
{489 174 219 621 224, -683 300 250 843 755}, {1 553 008 249 780 248, -551 504 961 148 421},
{812 053 069 320 120, 1 265 334 045 571 903}, {3 626 247 810 014 264, 3 929 037 899 230 049},
{2 422 320 713 726 280, -3 272 824 896 772 387}, {6 804 033 464 368 856, -183 030 500 250 221},
{255 239 640 885 432, -475 190 393 570 719}, {1 759 606 021 482 296, -3 016 950 184 678 145},
{10 058 753 305 566 792, -14 842 067 581 646 159}, {38 266 514 208 634 936,
-29 546 201 905 291 105}, {69 762 498 426 750 648, 33 960 066 161 329 921},
{7 369 464 416 363 224, -6 943 108 421 717 781}, {852 711 989 290 886, -669 181 009 426 829},
{1 468 247 838 912 456, 336 012 300 371 135}, {248 397 274 855 832, -290 514 839 324 079},
{168 470 257 872 988, -143 585 141 219 341}, {199 080 933 229 176, -377 242 513 491 671},
{1 425 292 642 099 960, -2 505 068 880 203 977}, {8 638 209 904 832 136, -13 432 512 339 592 711},
{38 354 419 478 084 600, -41 163 276 760 836 137},
{5 617 714 565 503 074, -4 748 022 243 625 373}, {6 957 538 575 021 608, -11 023 715 970 794 253},
{32 529 419 166 181 160, -37 861 771 502 597 971}, {21 329 409 345 667 244,
-13 855 836 418 529 257}, {25 529 053 965 565 080, -43 501 738 442 447 657},
{143 781 475 815 060 616, -209 139 311 243 778 631}, {522 862 683 429 744 120,
-352 978 408 340 029 417}, {1 359 074 200 717 717 624, 2 442 585 261 060 920 457},
{8 668 088 482 745 622 664, 14 048 160 782 151 924 167}, {43 040 578 395 250 412 024,
54 396 955 024 379 953 257}, {90 851 013 033 036 329 864, -83 127 964 692 023 847 833},
{61 784 386 728 099 856 248, 53 219 778 177 970 046 219}, {34 258 434 200 519 240 116,

```

```

-52 623 752 342 143 926 023}, {146 922 545 132 997 487 256, -148 334 843 653 213 854 933},
{11 298 388 161 730 941 416, 4 584 887 804 611 093 815}, {8 514 450 210 035 015 144,
-14 653 943 345 441 308 423}, {49 115 945 083 250 346 232, -73 092 740 434 064 624 265},
{191 814 362 806 514 224 264, -158 538 732 402 725 624 903},
{266 205 043 230 308 794 888, -236 765 316 704 358 419 033},
{117 758 906 103 801 503 420, -34 429 744 512 972 024 627},
{115 757 380 519 083 436 312, 173 121 893 407 672 118 693},
{458 916 103 108 709 459 048, 393 324 752 284 872 204 267},
{262 365 403 295 349 019 124, -460 032 866 399 466 081 143},
{1 581 339 704 832 936 496 152, -2 447 428 425 031 900 273 445},
{6 928 709 761 591 710 218 344, -7 269 322 925 912 674 908 523},
{1 362 452 657 283 858 760 716, -2 599 732 578 199 016 552 555},
{9 898 239 367 321 262 334 712, -17 557 816 922 777 759 126 569},
{61 276 620 443 651 974 334 856, -96 984 368 836 929 327 535 015},
{285 661 987 146 218 825 601 272, -331 065 249 496 163 328 924 809},
{181 613 049 399 778 013 294 148, -83 240 134 863 626 287 330 411},
{60 531 118 690 101 754 533 304, -98 402 454 530 360 850 505 091},
{302 970 686 722 072 767 774 296, -386 791 774 805 145 171 084 669},
{670 568 704 664 579 226 482 984, 495 880 467 865 916 866 055 789},
{1 397 505 894 389 298 883 417 560, -1 448 291 597 831 198 244 796 733},
{406 285 627 535 194 891 033 384, 565 835 135 757 424 539 093 323},
{1 276 396 065 777 837 184 479 512, 419 353 668 829 722 777 111 525},
{73 340 237 154 675 412 579 748, -27 745 838 527 312 234 033 041},
{79 178 227 418 090 316 155 000, -84 848 923 026 602 102 836 297},
{11 341 391 217 023 573 362 594, -6 093 717 810 661 181 447 613},
{846 044 404 298 789 532 632, -463 126 322 654 437 430 285},
{320 832 964 040 341 311 752, 609 277 554 961 427 138 101},
{2 307 556 727 368 686 610 792, 4 067 561 878 862 243 512 011},
{14 080 041 211 948 455 209 752, 22 019 664 665 402 315 841 701},
{63 516 987 627 630 885 055 592, 69 971 009 733 851 152 856 811},
{51 632 176 849 762 142 409 752, 40 455 978 007 675 682 658 879},
{89 409 590 736 691 678 006 984, -22 814 340 043 274 791 006 031},
{3 695 538 872 814 972 034 280, 2 668 040 690 075 532 113 557},
{8 219 985 461 915 519 365 784, -10 508 118 144 318 380 633 957},
{18 305 061 459 222 890 145 384, 13 132 832 000 058 345 758 293},
{41 377 835 673 316 355 096 728, -55 276 457 233 634 109 933 477},
{111 188 972 482 542 038 693 992, 11 354 389 499 222 479 528 597},
{9 419 690 038 731 026 367 912, -8 916 259 096 807 190 938 729},
{4 027 447 535 390 683 433 464, 6 701 723 223 736 964 013 533},
{21 394 205 506 770 244 640 552, 29 288 760 548 838 985 873 875},
{63 156 440 336 549 929 866 584, 10 421 121 913 419 091 242 013},
{314 854 428 017 691 207 253, 330 317 322 435 331 908 585},
{3 865 723 604 410 175 333, 7 298 743 193 703 599 346},
{27 464 156 714 347 392 104, 48 033 661 718 467 349 635},
{164 556 040 032 959 660 248, 253 385 361 379 979 886 381},
{710 634 570 776 161 809 064, 726 626 070 717 787 919 075},
{31 982 999 883 252 220 022, 33 957 353 135 652 392 873},
{3 948 706 504 800 345 702, -6 709 755 446 899 427 365},
{22 088 391 536 792 653 304, -31 914 473 629 876 112 633},
{78 608 656 744 667 674 632, -49 292 755 846 578 338 135},
{79 907 419 793 956 006 552, -112 470 228 315 266 172 849},

```



```

{260 502 468 170 481 330 376, -109 685 237 638 485 772 415},
{164 527 971 574 039 142 184, 198 804 939 295 458 586 303},
{274 215 741 771 355 552 952, -527 853 514 999 665 922 735},
{2 029 102 185 826 482 958 264, -3 639 942 850 080 294 081 393},
{12 886 725 314 030 488 985 032, -20 816 517 791 225 792 165 855},
{63 438 339 817 562 425 446 584, -79 291 424 463 248 061 278 673},
{126 824 677 165 485 086 656 712, 142 885 771 689 729 779 434 625},
{64 244 378 096 978 771 111 652, -73 649 156 507 333 641 623 197},
{37 619 113 641 419 482 046 180, 3 048 495 308 333 580 634 893},
{518 584 970 708 257 213 732, -485 269 107 327 706 385 765},
{66 631 726 761 101 655 934, 62 253 550 141 662 895 447},
{8 756 353 238 877 520 974, -11 216 374 919 275 784 203},
{19 680 173 443 186 105 832, 13 470 327 261 860 113 525},
{49 678 769 450 607 938 456, -84 742 613 526 224 853 317},
{280 510 752 604 935 318 888, -409 038 258 134 325 534 155},
{1 028 220 044 235 121 722 136, -712 046 606 336 492 400 037},
{2 529 387 503 189 034 576 792, 4 105 003 724 165 569 784 773},
{12 604 929 767 812 281 663 848, 16 004 073 056 948 033 169 227},
{27 193 146 313 086 012 043 032, -22 659 142 492 375 968 687 067},
{36 272 030 565 680 346 847 720, -40 719 021 496 996 405 461 621},
{17 787 963 725 264 234 455 604, 25 019 367 117 187 804 815 553},
{57 851 227 135 388 562 879 592, 24 018 568 212 128 242 633 995},
{39 256 362 844 528 310 446 408, -56 044 133 174 034 232 443 851},
{134 302 162 636 047 375 979 544, -72 067 814 822 409 722 369 925},
{19 666 934 017 544 137 520 612, -8 283 108 991 147 621 044 893},
{12 402 864 140 995 581 723 304, 14 928 662 581 767 394 998 231},
{10 103 193 763 087 253 099 708, 18 585 101 336 856 631 529 813},
{67 855 260 590 155 027 440 840, 114 258 324 091 997 679 094 751},
{371 224 508 014 741 213 231 288, 524 428 375 821 140 768 513 233},
{1 225 630 942 451 196 442 255 560, 553 892 895 429 260 065 634 431},
{471 380 606 370 705 243 946 792, 388 971 732 030 557 442 243 905},
{659 270 994 721 182 413 623 096, 557 098 751 699 877 685 161 743},
{817 377 944 170 437 827 690 824, 1 289 450 479 938 574 898 992 001},
{3 776 580 286 145 096 570 409 416, 4 318 644 769 303 650 018 400 479},
{2 168 257 932 634 213 791 964 252, -470 580 099 299 443 185 878 963},
{1 477 140 510 904 017 099 444 504, -1 959 278 685 357 520 773 315 749},
{3 857 105 395 628 029 390 969 960, 727 946 074 801 552 296 517 397},
{1 739 000 172 962 143 267 063 800, -915 057 071 815 886 787 733 049},
{364 455 882 678 521 233 609 192, -576 571 348 874 262 189 774 661},
{1 696 923 729 565 927 649 323 752, -1 963 008 661 073 872 122 932 251},
{1 064 339 726 031 777 894 433 996, -396 598 232 450 790 190 134 465},
{1 003 639 770 564 741 407 755 192, -716 318 251 332 051 433 975 649},
{2 298 572 153 861 519 790 236 344, 3 176 421 085 556 977 715 360 641},
{7 022 791 453 563 663 400 994 376, 1 801 948 198 103 373 955 968 079},
{370 002 677 699 664 845 755 880, 697 384 732 051 855 919 975 947},
{2 619 056 434 817 528 593 760 536, 4 569 765 828 503 075 941 014 501},
{15 605 675 149 484 378 778 031 720, 23 913 864 576 227 360 236 756 907},
{66 465 515 413 943 851 669 801 496, 66 242 955 619 213 543 326 425 541},
{1 780 478 357 842 466 747 007 640, -1 306 585 067 537 669 027 000 257},
{3 791 146 322 438 381 760 059 064, 4 238 011 459 147 377 104 226 817},
{1 787 460 546 835 981 376 671 012, -3 099 226 598 610 652 747 706 925},

```

```

{10 494 128 414 197 370 968 287 304, -15 870 934 816 129 590 520 457 903},
{43 014 451 215 457 756 417 364 792, -39 713 519 930 862 081 953 625 345},
{26 407 450 276 765 395 709 915 576, -10 721 549 979 498 930 501 234 189},
{19 857 401 271 070 138 829 788 792, 34 061 230 007 401 065 960 494 813},
{113 630 629 890 647 417 045 648 168, 167 828 850 767 050 213 367 928 147},
{433 585 767 011 222 370 578 239 832, 337 514 041 032 084 979 047 254 173},
{768 573 807 833 099 132 247 885 272, -278 111 177 096 579 305 082 522 045},
{526 077 787 653 110 263 997 446 904, 186 337 989 616 832 167 670 069 607},
{263 489 449 579 089 912 102 095 336, -469 682 299 815 683 931 964 937 429},
{1 649 542 801 892 752 158 902 736 744, -2 634 519 958 808 943 160 028 605 451},
{7 879 817 255 329 528 009 006 949 656, -9 458 132 193 930 375 754 673 086 309},
{6 313 259 754 403 390 982 664 546 612, -11 095 234 320 904 777 096 957 891 007},
{38 255 796 532 011 088 914 346 755 160, -59 479 336 994 304 752 767 430 548 189},
{169 788 323 698 349 310 824 670 344 232, -182 095 058 376 665 557 306 153 198 387},
{24 613 469 356 632 492 962 965 708 310, -17 318 658 274 472 526 313 662 082 031},
{58 358 488 657 279 733 194 429 010 232, 87 589 877 351 178 755 619 115 758 401},
{233 851 109 551 192 179 397 493 985 352, 205 454 030 701 439 650 212 363 126 031},
{113 588 315 399 010 116 740 523 437 284, -58 493 321 536 569 803 889 604 134 827},
{1 699 163 837 064 745 519 342 416 185, 2 909 621 293 781 346 394 994 616 546},
{9 683 659 653 732 807 005 217 602 888, 14 247 210 807 963 855 985 261 278 823},
{36 508 409 233 848 391 840 349 407 480, 27 492 399 317 451 670 499 263 723 401},
{72 128 079 331 173 770 728 685 472 632, -59 557 112 868 684 997 579 546 419 241},
{100 567 731 699 910 185 193 112 427 128, -86 756 942 612 328 013 013 060 698 807},
{55 243 156 350 328 688 720 206 913 284, 81 106 691 265 735 285 529 360 782 723},
{206 908 279 323 252 774 473 230 955 512, 152 916 052 251 722 216 848 883 690 825},
{431 937 816 572 244 460 994 778 117 496, -450 430 621 203 669 551 563 695 678 697},
{73 971 218 525 700 362 275 670 244 804, 81 891 654 092 144 783 345 449 523 095},
{63 363 484 531 555 368 558 234 226 328, 81 467 274 942 172 892 725 876 696 303},
{144 830 323 284 940 193 341 139 759 800, -90 520 696 808 239 892 610 097 001 199},
{144 844 281 326 158 367 516 216 970 392, -199 188 802 905 904 103 684 952 755 473},
{434 756 172 637 965 889 349 886 280 648, -91 169 745 724 884 991 751 187 293 727},
{168 740 447 891 672 555 248 401 503 896, 75 488 730 218 848 782 421 942 522 219},
{71 051 949 815 899 961 618 065 837 832, 26 628 615 338 782 778 417 764 967 277},
{70 671 169 603 586 989 081 832 511 992, 60 821 859 503 637 355 349 981 245 753},
{39 397 240 399 798 534 927 405 064 956, -62 041 175 083 889 224 287 464 270 397},
{181 151 477 472 725 514 880 473 643 528, -205 632 574 535 697 575 862 121 205 495},
{97 924 388 251 888 243 926 590 247 868, 63 616 289 190 656 413 017 410 401 003},
{117 232 760 517 698 328 432 922 216 552, 199 811 790 243 455 370 607 931 985 127},
{660 632 237 806 056 337 400 078 148 600, 961 455 599 550 825 342 561 846 944 809},
{2 406 586 893 958 152 041 294 150 369 672, 1 633 879 417 681 236 419 520 057 124 007},
{6 181 659 810 215 324 974 192 745 965 320, -10 882 896 423 134 492 918 836 433 623 559},
{37 609 892 903 353 343 557 149 501 265 912, -58 675 163 615 418 262 933 262 848 416 937},
{168 522 165 696 519 355 008 906 777 208 200, -183 622 083 150 666 397 193 410 974 346 279},
{120 799 339 633 176 337 476 033 577 104 632, 64 684 341 969 656 254 388 397 460 928 885},
{17 138 688 612 272 342 601 522 689 506 276, 3 456 152 805 798 146 385 005 921 815 869},
{568 301 666 873 557 294 027 678 292 276, -611 597 468 382 378 453 880 166 968 059},
{86 591 603 017 642 319 704 977 351 566, -118 974 910 008 699 047 666 815 013 155},
{259 066 455 928 453 823 694 701 292 712, -52 083 236 653 166 185 482 447 404 019},
{5 398 909 349 508 414 870 142 909 532, -874 790 680 786 334 288 248 128 289},
{300 330 529 580 818 281 308 279 596, 577 980 242 678 673 103 642 910 291},
{2 221 197 704 782 838 578 677 045 560, 3 983 299 164 604 114 663 230 269 217},

```

```

{14 096 811 678 570 208 676 425 789 256, 22 758 751 937 626 641 315 307 779 631},
{69 295 522 072 451 461 111 055 923 000, 86 450 132 529 736 281 282 879 464 577},
{137 236 883 658 278 561 374 588 332 616, -159 808 136 062 060 824 936 505 927 729},
{90 285 009 615 129 054 247 670 380 452, -60 476 280 269 006 870 673 421 737 587},
{238 469 834 768 977 468 593 989 142 920, 440 260 367 577 732 725 414 334 028 119},
{1 614 324 262 470 042 054 562 759 081 592, 2 733 423 576 449 551 158 116 019 216 217},
{8 952 794 511 836 072 828 426 081 077 000, 12 824 690 121 768 372 945 222 910 443 639},
{30 975 164 879 458 400 934 374 634 933 112, 17 431 242 933 754 320 058 918 426 816 697},
{15 549 283 952 200 956 733 848 874 801 128, -9 471 496 420 238 572 892 009 317 412 417},
{13 574 835 553 104 756 200 679 040 094 824, -14 716 502 087 326 638 709 594 010 717 775},
{9 133 332 273 775 060 071 319 764 983 608, 11 557 029 015 978 036 347 659 817 807 757},
{19 389 573 937 623 810 210 720 422 593 192, -17 321 633 119 532 026 214 736 904 913 437},
{8 271 763 272 367 135 983 934 070 719 020, -5 180 367 117 282 800 983 458 571 581 343},
{8 355 883 848 793 863 931 932 289 774 664, -11 657 581 444 945 018 802 403 336 551 451},
{26 413 580 769 209 238 963 768 374 214 296, -9 091 973 921 125 650 565 375 757 668 789},
{6 898 727 953 341 701 858 871 190 336 568, -7 461 921 088 592 079 586 371 526 312 291},
{4 505 545 082 003 021 820 002 687 805 784, 7 318 407 130 451 508 033 440 964 756 089},
{22 502 896 387 587 889 707 506 215 602 440, 28 651 466 458 291 008 349 058 867 410 743},
{49 188 560 565 624 949 132 421 214 466 424, -38 606 059 474 531 388 904 338 733 228 551},
{84 660 008 728 748 481 824 659 849 902 984, 19 209 058 027 649 255 835 847 052 545 655},
{15 647 553 236 302 916 962 543 279 440 728, -22 216 152 735 375 291 558 161 102 741 511},
{52 548 795 992 578 996 764 942 586 406 264, -25 897 362 588 241 279 998 863 700 392 185},
{3 016 283 264 385 747 068 860 742 487 576, 1 603 428 492 487 809 031 063 592 685 473},
{381 147 441 179 741 986 532 885 766 740, -252 964 315 832 617 666 497 320 678 711},
{499 124 761 941 973 385 847 022 362 728, -922 251 189 194 676 204 167 928 940 727},
{3 385 011 418 021 622 546 567 252 623 992, -5 738 909 731 276 377 734 604 672 392 153},
{18 831 186 506 038 041 504 299 358 145 288, -27 059 569 860 686 388 952 322 633 675 767},
{65 827 066 837 186 779 584 186 204 243 832, -38 603 325 108 607 659 270 140 472 038 713},
{45 518 333 520 114 155 824 378 959 334 376, -21 970 241 956 011 716 738 906 579 265 855},
{788 924 804 045 361 173 282 900 401 333, 1 243 213 484 697 239 816 431 666 587 734},
{3 634 309 445 215 029 145 190 129 491 208, 4 137 241 222 630 319 406 158 419 076 559},
{2 011 727 109 661 161 043 873 158 341 404, -958 079 790 647 279 534 616 699 160 355},
{382 270 113 466 407 898 559 040 082 776, 611 570 906 457 873 682 282 044 320 851},
{1 834 406 343 931 726 269 784 033 904 600, 2 215 757 331 072 449 837 156 776 813 517},
{3 050 807 897 125 788 538 981 943 271 336, -5 904 178 047 217 168 108 699 184 331 709},
{22 826 961 200 731 036 557 737 928 482 984, -41 221 050 275 095 421 791 640 998 217 891},
{147 152 712 594 915 081 871 224 557 879 256, -240 448 359 104 532 567 917 867 176 038 989},
{746 365 172 076 939 888 373 140 945 277 864, -968 578 168 961 881 524 102 983 754 639 811},
{1 777 703 975 079 533 085 838 742 474 895 576, 860 022 448 261 861 485 198 742 946 898 131},
{28 829 539 277 905 057 720 628 290 549 657, -16 846 634 676 597 652 070 367 030 070 618},
{38 909 840 602 321 971 360 846 156 732 632, -16 002 554 921 216 422 460 342 616 774 005},
{27 618 923 039 556 505 760 643 692 738 488, 43 013 107 093 415 769 981 123 842 265 621},
{123 153 472 430 874 113 763 841 196 217 064, 133 114 848 922 311 030 985 893 897 216 155},
{79 691 011 931 495 337 776 421 607 992 728, -138 510 777 674 854 946 236 249 984 813 777},
{470 558 125 946 876 867 678 627 014 568 392, -715 326 516 645 308 292 364 679 802 942 303},
{1 958 147 125 587 451 397 488 422 306 991 288, -1 865 207 978 488 907 826 350 198 016 052 817},
{743 513 176 788 348 569 105 794 327 507 768, -516 096 027 637 009 084 376 819 032 959 531},
{1 819 337 193 210 715 877 831 802 356 385 896, 2 921 163 402 595 451 351 583 681 867 319 099},
{8 814 609 675 077 883 790 015 036 087 465 624, 10 787 305 270 163 188 873 638 809 900 376 501},
{15 781 564 760 682 440 668 990 190 503 287 016, -25 144 878 713 661 053 396 773 491 002 774 821},
{74 906 511 623 828 901 822 266 403 995 902 440, -89 103 702 833 048 567 387 094 387 461 923 387},

```

```

{56 788 764 836 878 662 259 311 933 864 083 788, - 83 698 116 153 615 362 961 289 937 598 955 809},
{215 274 810 533 893 605 615 824 029 878 976 168,
- 164 604 961 589 914 818 070 998 614 989 386 179},
{405 358 791 551 830 300 358 603 319 116 719 912, 253 925 624 544 023 869 321 598 941 662 200 227},
{409 969 830 144 869 753 138 378 256 830 722 168, 572 930 593 635 274 816 124 819 978 570 247 493},
{1 303 686 107 923 240 503 891 533 773 916 202 600,
468 338 919 120 358 423 581 133 545 363 305 131},
{810 645 195 502 678 134 814 934 897 389 702 344,
- 605 461 220 389 989 616 241 195 635 521 344 465},
{1 641 471 800 901 508 148 589 914 094 946 863 032,
1 517 013 465 373 427 145 856 352 033 748 338 529},
{995 666 684 224 648 021 868 496 489 588 196 024, 561 482 518 875 883 912 629 544 578 523 929 453},
{509 193 414 108 479 213 562 370 669 838 651 528,
- 272 805 595 833 178 697 963 991 968 470 943 141},
{72 835 555 115 756 364 731 226 534 206 469 508, - 18 864 360 480 754 430 739 021 703 158 252 405},
{2 621 886 807 261 358 224 860 278 426 540 112, - 1 455 262 275 521 095 503 645 454 647 433 463},
{1 154 550 975 123 331 129 722 523 473 307 256, 1 347 164 073 481 473 886 907 040 130 668 235},
{770 452 393 432 571 028 738 066 629 443 916, 582 349 755 176 529 925 091 855 855 517 409},
{1 504 821 106 048 328 829 169 686 191 412 056, - 1 172 383 744 525 034 812 297 687 147 582 445},
{2 659 498 892 186 352 134 975 992 350 636 888, 926 488 251 021 836 024 650 473 178 058 381},
{479 863 443 516 623 755 901 708 734 153 020, 12 988 683 166 490 009 636 349 977 452 381},
{5 742 669 148 052 805 145 923 452 680 616, 7 354 749 411 603 022 611 467 076 067 887},
{12 896 642 108 401 739 724 348 987 098 168, - 8 863 507 122 767 439 459 884 283 537 695},
{32 265 079 885 074 402 115 717 628 483 784, 54 119 127 572 523 792 519 331 542 073 103},
{174 832 381 499 595 123 228 911 308 714 552, 244 522 457 730 740 762 357 378 984 684 065},
{557 520 609 849 165 113 027 741 407 756 104, 204 212 701 319 588 714 123 466 077 582 383},
{440 939 952 876 808 234 741 254 599 928 360, 74 940 706 840 922 196 634 632 954 063 331},
{17 408 576 337 449 890 133 086 248 903 252, - 14 964 947 066 607 744 737 847 479 126 459},
{9 774 517 083 368 581 580 955 079 107 172, 15 892 719 129 675 528 301 011 946 574 747},
{48 945 616 370 455 573 760 454 939 740 600, 62 522 510 398 111 121 913 667 318 896 849},
{108 615 152 221 244 385 225 699 033 249 992, - 79 296 368 327 566 982 559 754 797 331 073},
{234 550 271 149 419 221 327 553 887 351 352, 274 511 354 083 463 622 166 232 934 837 905},
{159 844 331 736 177 603 354 716 189 946 212, 140 748 154 621 521 937 334 118 732 731 523},
{76 384 708 458 622 664 082 389 828 858 756, - 28 988 872 068 237 897 302 046 242 729 267},
{84 655 261 968 728 222 589 991 194 632 360, - 96 128 163 582 918 684 119 845 937 366 259},
{45 891 606 456 761 846 119 418 970 935 596, 28 852 704 291 770 429 053 886 724 714 167},
{47 255 208 507 116 047 953 417 913 970 952, 67 703 115 797 992 969 603 947 517 780 771},
{163 583 258 327 015 373 204 236 830 478 552, 92 260 199 633 240 814 334 837 575 858 221},
{83 748 563 757 865 021 861 753 284 951 560, - 44 515 113 971 236 297 625 056 324 245 589},
{10 563 328 369 215 146 776 718 727 079 236, 7 164 433 081 055 207 730 542 513 627 099},
{27 191 162 305 279 512 369 409 707 617 096, - 48 050 289 284 516 448 587 122 507 999 455},
{166 873 015 833 895 489 741 702 403 058 872, - 262 230 622 080 213 434 052 116 747 857 489},
{762 860 849 970 543 554 483 314 758 388 936, - 858 240 816 994 148 801 205 910 705 897 215},
{381 519 868 094 420 986 890 383 790 033 116, 476 184 290 244 832 556 423 168 450 832 211},
{757 315 377 203 292 556 262 277 286 392 760, - 874 877 235 295 901 795 869 023 121 885 743},
{470 247 432 370 436 958 426 983 341 971 932, - 144 908 659 687 279 244 333 028 412 739 501},
{284 171 626 468 793 803 423 184 830 027 432, - 58 104 224 931 657 966 399 386 085 559 709},
{25 397 992 757 984 114 294 982 391 084 452, 35 582 455 852 254 979 811 430 811 334 333},
{81 475 704 754 166 924 131 587 361 999 048, 31 058 709 104 356 992 518 454 537 071 647},
{93 603 380 471 232 427 390 209 993 727 144, 114 243 426 491 169 715 989 427 429 119 507},
{165 120 368 159 498 308 793 739 483 138 904, - 274 105 985 311 301 781 339 678 935 792 803},

```

```

{871 884 937 214 427 780 367 515 621 231 192, -1 185 706 249 215 493 398 206 691 545 928 445},
{2 510 570 496 008 524 942 713 407 397 578 024, -242 810 678 309 086 967 360 921 298 187 283},
{329 854 851 670 621 076 416 777 662 820 776, 306 944 836 987 308 801 671 328 250 681 375},
{183 280 117 466 498 197 963 595 297 115 208, 324 927 330 350 428 862 043 830 676 486 707},
{1 133 177 703 071 445 312 641 883 034 971 992, 1 791 644 956 598 419 690 136 651 348 622 813},
{5 267 738 028 215 795 019 958 146 509 206 568, 6 079 325 206 548 848 181 244 606 934 192 947},
{3 246 348 713 332 212 645 145 841 699 945 516, 841 901 702 129 255 274 901 845 437 805 961},
{121 258 095 184 808 454 461 540 051 278 328, 97 848 535 553 010 247 175 089 959 601 081},
{187 276 477 054 385 658 291 600 733 417 976, 57 091 935 838 337 551 520 766 834 813 991},
{128 005 356 314 984 029 834 401 831 808 024, -39 285 269 013 862 703 442 172 419 744 165},
{81 196 394 187 167 356 063 076 580 604 232, 353 875 364 371 877 207 042 391 888 079},
{1 271 485 968 059 805 202 950 705 873 128, -2 096 005 211 256 727 505 094 850 153 739},
{6 596 153 945 575 378 417 153 154 244 888, -8 792 054 849 050 771 325 709 671 469 029},
{17 567 207 227 803 143 268 452 137 793 128, 2 263 510 784 668 990 440 425 337 803 861},
{540 879 049 548 780 254 950 564 637 760, -167 604 467 667 466 952 491 899 832 541},
{304 525 172 371 035 179 798 921 121 096, -160 800 698 401 974 298 214 379 316 081},
{34 152 448 865 826 833 259 675 022 132, 56 919 918 093 790 638 666 277 210 639},
{182 139 753 823 710 443 252 817 508 056, 250 432 201 316 552 858 274 450 158 605},
{546 339 579 942 739 320 173 061 204 392, 113 608 261 745 691 999 475 010 898 179},
{173 613 830 285 765 417 615 946 292 024, -236 112 501 608 195 002 538 295 303 839},
{499 989 370 579 436 679 378 792 094 520, -48 558 798 129 757 112 286 456 935 553},
{57 605 557 127 462 226 056 890 955 960, 28 986 341 349 887 676 824 624 712 133},
{183 562 786 156 563 796 179 234 153, -267 054 747 810 144 208 421 709 209},
{83 491 961 653 580 412 242 475 056, -56 476 603 597 479 889 017 881 633},
{216 122 864 448 804 185 796 747 384, 385 663 270 959 277 107 819 343 049},
{1 356 323 252 083 783 376 180 765 320, 2 170 446 434 150 443 720 145 721 223},
{6 512 985 456 533 282 751 719 647 224, 7 874 247 170 862 920 901 747 863 209},
{10 890 093 714 637 105 200 225 727 880, -20 794 864 222 684 584 563 108 210 137},
{79 238 164 064 379 834 903 059 858 056, -140 688 971 967 995 183 744 491 268 871},
{491 606 463 228 922 790 731 451 286 520, -779 463 269 268 114 344 128 443 584 297},
{2 302 854 448 313 532 427 175 938 382 216, -2 687 854 833 070 023 402 279 212 556 711},
{1 540 001 539 025 963 900 413 096 697 980, -1 183 592 595 171 126 619 084 649 182 501},
{2 851 271 550 838 698 250 627 580 123 832, 1 579 936 498 130 942 768 504 679 519 841},
{1 234 405 781 692 749 145 527 115 663 400, -1 536 423 588 464 368 135 101 144 883 689},
{2 416 142 454 172 951 916 592 233 762 312, 2 928 836 697 794 756 404 014 253 240 553},
{4 101 553 948 974 435 899 376 155 825 928, -7 537 172 030 082 112 122 031 422 098 953},
{27 484 944 648 861 409 781 242 130 184 200, -46 206 784 273 681 065 926 061 877 672 151},
{149 774 716 998 557 249 158 557 979 903 608, -210 722 754 179 960 813 080 917 150 749 273},
{487 584 297 451 228 511 378 873 366 765 320, -203 607 119 183 823 976 945 797 090 221 431},
{321 480 236 334 322 229 949 116 745 289 832, 431 307 439 060 202 733 269 639 027 112 375},
{878 617 621 807 044 026 564 178 254 580 344, -45 816 227 979 326 263 220 921 480 400 167},
{64 874 321 598 760 202 933 361 015 817 368, -115 141 827 639 414 319 400 597 906 909 035},
{402 140 048 325 232 931 737 895 128 733 336, -637 158 066 144 963 055 279 560 368 569 397},
{1 880 144 142 557 840 988 333 321 918 688 488, -2 188 294 023 251 929 387 555 139 486 362 715},
{1 232 599 522 776 353 596 887 270 270 696 908, -799 470 208 509 022 825 655 786 652 450 177},
{1 465 363 576 966 768 217 697 212 136 813 784, -2 480 403 026 710 135 540 953 550 420 352 705},
{8 120 315 597 946 938 586 050 706 268 311 368, -11 622 998 728 363 302 693 318 083 426 884 911},
{28 021 465 043 330 912 858 139 017 268 588 344, -15 599 187 216 000 865 778 744 024 500 700 545},
{12 707 637 554 683 274 797 396 126 931 250 984, 13 154 653 339 605 773 275 066 106 144 204 617},
{447 015 784 922 498 477 669 979 212 953 633, 702 835 992 991 679 532 703 249 457 358 006},
{2 046 561 664 553 448 440 266 161 955 234 984, 2 307 738 506 211 176 444 405 381 917 671 515},

```

```

{1 044 707 366 630 912 016 556 879 849 746 124, - 1 134 471 933 455 137 649 305 708 835 153 599},
{718 116 534 593 805 061 990 631 883 259 800, 727 670 752 988 117 348 804 575 038 333 617},
{19 108 436 788 624 573 627 886 310 147 634, 25 562 345 142 169 758 552 038 959 774 401},
{51 631 266 828 361 479 393 221 197 014 136, - 4 427 602 177 457 335 767 579 539 765 431},
{2 999 918 602 253 099 635 466 560 342 072, - 2 769 480 228 816 089 552 273 841 794 667},
{1 843 506 987 496 080 665 541 748 379 240, - 725 073 100 886 778 681 267 909 448 671},
{2 653 698 521 314 043 026 095 839 734 184, - 4 482 496 962 997 687 275 978 103 380 595},
{14 630 387 533 469 153 999 058 109 171 288, - 20 832 775 988 211 473 538 525 345 993 981},
{49 619 107 637 938 556 315 737 894 581 544, - 25 611 834 191 320 117 415 281 573 551 635},
{802 280 372 350 839 257 412 626 260 863, 370 571 324 222 050 217 745 079 732 441},
{244 550 895 626 955 287 689 867 183 924, - 412 984 144 220 702 608 616 151 745 647},
{1 347 465 988 749 978 567 410 276 493 784, - 1 917 557 552 640 546 079 785 607 448 237},
{4 560 732 511 124 540 099 002 647 635 624, - 2 332 378 059 483 224 245 350 400 002 147},
{208 047 215 683 816 783 396 304 737 340, - 172 341 645 682 291 723 263 285 138 861},
{285 644 560 012 200 481 064 156 787 832, - 271 860 495 411 056 921 982 673 558 039},
{110 272 516 809 148 472 651 865 838 344, - 38 353 950 111 203 718 231 487 846 397},
{19 157 334 097 850 728 170 390 803 388, 4 946 461 186 471 729 605 422 659 331},
{628 510 648 036 190 251 299 833 936, - 75 503 664 191 255 157 848 946 327},
{12 240 667 253 074 494 254 131 660, 9 680 753 510 036 086 310 287 019},
{20 479 309 944 307 263 550 757 128, - 1 911 297 953 901 955 776 887 719},
{4 359 740 388 913 999 960 062 248, - 1 603 610 375 826 103 630 139 459},
{3 608 725 908 514 487 442 849 032, - 1 154 929 888 884 809 799 924 327},
{575 744 967 440 232 172 304 204, - 157 696 057 877 439 864 339 727},
{55 039 264 069 527 285 054 704, - 55 581 090 391 978 365 247 251},
{2 167 305 289 804 320 770 188, 3 968 353 620 128 143 392 563},
{14 408 386 642 590 580 979 000, 24 085 669 279 013 354 153 121},
{77 418 261 091 382 185 392 968, 107 310 407 496 999 135 172 783},
{239 137 171 244 935 598 238 520, 68 173 278 598 132 361 792 001},
{67 111 886 295 187 697 858 968, 123 712 002 197 587 605 619 499},
{452 800 927 219 199 262 084 248, 764 907 575 393 696 295 620 469},
{2 496 853 185 395 976 268 289 768, 3 556 045 490 259 837 674 659 099},
{8 473 538 438 910 891 250 954 648, 4 386 597 528 701 002 200 176 469},
{149 828 309 245 556 574 699 145, 129 040 028 955 625 807 748 513},
{20 788 280 289 930 766 950 632, - 32 069 143 291 337 636 118 885},
{90 246 904 011 254 953 346 024, - 93 153 606 712 911 855 264 763},
{2 906 702 701 656 901 918 739, 3 045 822 961 547 895 783 854},
{556 481 039 563 975 460 460, 754 892 323 670 846 320 279},
{1 587 290 272 854 966 878 552, 111 611 217 946 226 092 157},
{98 932 886 431 206 353 416, 63 079 936 863 979 749 141},
{108 907 949 187 012 579 464, 169 698 555 643 754 748 859},
{486 324 851 653 937 355 160, 526 920 355 008 969 260 373},
{324 764 026 840 255 241 704, - 439 981 028 053 786 898 175},
{921 736 009 708 253 251 768, - 51 878 813 189 186 165 201},
{48 330 510 788 390 887 400, 20 234 523 451 729 972 129},
{31 445 855 539 723 772 568, - 40 914 596 409 509 730 185},
{75 749 926 958 287 660 936, 33 785 804 312 713 155 353},
{32 713 273 331 445 400 920, 8 379 283 091 501 692 847},
{1 607 718 069 122 740 936, 1 931 156 370 548 477 687},
{1 293 753 205 702 947 004, 2 301 961 862 003 928 533},
{8 065 669 250 407 852 232, 12 838 773 449 298 999 135},
{38 184 833 591 129 175 224, 45 256 042 571 233 560 913},

```

```

{28 284 835 920 417 542 756, 38 183 308 098 301 712 707},
{79 187 777 423 073 359 608, 1 386 172 727 995 566 825},
{703 727 709 304 202 332, 90 801 164 874 699 227},
{45 363 219 386 782 968, -5 819 854 625 614 453}, {1 195 617 618 132 656, 1 186 836 355 350 411},
{70 250 102 257 960, -32 979 275 932 537}, {8 583 100 785 772, 560 479 224 659},
{1 407 299 327 096, -969 451 095 225}, {3 502 785 854 968, 5 817 686 426 201},
{18 519 204 569 864, 25 220 426 298 615}, {53 609 773 830 008, 5 974 463 202 361},
{641 579 964 964, 963 370 832 911}, {2 574 326 943 576, 2 268 550 243 069},
{1 223 106 802 028, -404 876 743 441}, {16 953 143 410, -21 432 318 317},
{35 833 399 256, 32 604 124 419}, {25 834 198 696, -39 489 564 489},
{109 242 926 344, -107 399 823 671}, {14 744 821 384, -2 155 846 423},
{1 384 414 308, -2 105 825 195}, {5 771 287 096, -5 517 135 937},
{1 016 604 636, 1 567 514 039}, {4 407 275 224, 4 538 079 181}, {1 046 431 656, 189 670 555},
{366 366 696, 660 988 727}, {2 356 976 248, 3 845 373 145}, {11 907 175 176, 15 377 318 647},
{27 761 147 768, -15 444 101 575}, {12 508 221 528, 13 307 047 879},
{1 597 652 702, -1 850 478 877}, {1 011 304 700, -435 695 917},
{559 651 464, 425 865 755}, {1 070 285 672, -740 430 939}, {2 638 837 864, 4 302 049 211},
{13 305 690 776, 17 143 158 069}, {30 699 738 344, -18 183 778 469},
{22 671 274 376, -15 116 074 331}, {60 441 600 360, 113 282 606 747},
{422 728 051 096, 731 810 344 021}, {2 472 658 343 400, 3 727 068 328 507},
{10 035 279 880 856, 9 070 162 910 261}, {3 860 467 882 380, 6 362 025 552 599},
{20 012 461 361 752, 26 652 083 355 997}, {53 116 975 953 960, -7 388 385 026 381},
{11 186 246 154 344, -15 760 376 362 965}, {36 593 041 668 968, -15 715 025 563 531},
{20 651 962 167 624, 17 166 251 145 419}, {27 885 688 177 640, 29 272 967 474 997},
{11 098 234 378 856, -19 155 448 709 641}, {64 457 714 646 280, -96 530 054 577 207},
{256 578 719 447 416, -222 002 101 241 081}, {138 306 472 825 340, 183 866 759 432 061},
{364 482 292 853 768, -58 565 190 648 137}, {52 364 595 859 784, -31 347 953 635 885},
{41 325 245 647 944, -34 743 512 342 243}, {52 653 866 445 608, -73 914 366 261 213},
{170 083 998 524 840, -67 760 564 194 051}, {265 581 552 458 504, -487 044 002 224 295},
{1 771 699 598 126 328, -2 968 983 924 945 161}, {9 578 274 614 550 664, -13 363 942 731 822 535},
{30 285 344 938 174 968, -10 444 169 780 847 721},
{8 377 315 234 945 560, -13 832 931 359 460 367},
{43 644 928 996 118 456, -58 460 648 984 276 081},
{118 525 759 905 261 000, 8 397 872 241 322 273}, {1 911 097 053 498 356, 1 984 742 318 032 287},
{589 162 116 271 448, 103 083 859 604 731}, {117 364 165 427 752, 42 450 702 613 615},
{79 903 539 304 744, -29 979 406 103 037}, {80 277 432 034 936, -71 239 800 311 081},
{36 150 526 895 420, -4 792 617 804 819}, {4 380 831 086 264, -7 390 484 849 635},
{24 077 230 106 968, -34 175 387 867 421}, {80 785 262 083 624, -39 639 787 634 675},
{6 022 747 257 096, 4 807 868 810 029}, {9 719 027 576 536, 801 718 621 155},
{24 601 030 669, 9 771 667 604}, {37 711 777 144, 67 959 795 601},
{241 984 147 656, 394 010 207 359}, {1 216 208 477 624, 1 560 726 191 921},
{2 756 141 714 376, -1 805 760 392 161}, {3 421 516 279 784, -6 035 334 015 519},
{20 910 541 885 880, -32 745 677 683 633}, {94 681 086 382 024, -104 923 788 261 279},
{81 941 615 034 040, -113 180 968 680 483}, {249 914 829 171 544, -62 972 213 595 869},
{1 974 025 211 932, 1 777 432 025 977}, {786 372 743 820, 1 015 339 339 303},
{1 831 732 763 864, -1 024 750 254 451}, {871 070 980 152, 723 600 969 715},
{1 179 760 083 496, 1 217 237 434 173}, {37 477 350 677, -55 439 563 186},
{143 697 700 072, -113 312 082 291}, {243 084 942 248, 35 457 492 883},
{20 470 031 732, 16 812 774 391}, {29 258 058 728, 21 127 217 557},
{65 046 729 368, -83 038 335 845}, {143 932 851 816, 106 566 885 973},
{298 927 726 744, -305 809 853 349}, {55 057 012 840, 99 673 654 487},

```

```

{356933133176, 585726655161}, {1830348175880, 2406785940247},
{4611502114936, -1384716826599}, {3658813081112, 3100166076517},
{4469176036760, 7483271469691}, {24112763463448, 3357078666333},
{75664185599080, 24632425889771}, {3533815859534, -5509294043235},
{15803825469608, -17165471348851}, {10893167033944, 10690704021209},
{809852050940, -1171657678659}, {2894445021752, -1842713030017},
{3163924153128, -4889353973303}, {13803438561400, -14373492639001},
{4560432620808, -8713793727409}, {33226888852808, -59043844485359},
{206535645060408, -327974868726209}, {971513789326408, -1140816983830159},
{677212778015004, -685131094295645}, {31673265122564, 40378525483999},
{69642082891480, -53165132667507}, {131815601791784, 85464395603107},
{156452757657720, 264396853511237}, {863552766828136, 1231092143369131},
{2940315012327960, 1544983525817797}, {598608157230536, 778885724533793},
{1442220538426056, -642481209869377}, {629032474749208, -132423999824327},
{264700194979416, 33678743049379}, {4729749415616, 2976814921645},
{4895521710696, 7062886942367}, {17338921853368, 10685226642865},
{16126125729448, 19747830630151}, {28973639205624, -45709793119415},
{133889231310328, -153142426372201}, {77012780247492, 15720658570741},
{12724100849704, 22152403811881}, {75426423697416, 115058161332439},
{317053901080184, 308118576026201}, {71482600431864, -28007081851649},
{100309160984664, -164641344002381}, {514657464141736, -677166921530179},
{1300075659107544, 379542193199699}, {1291592636067576, -1968583919164265},
{5415930264773512, -5238058422683239}, {177871842090273, 275968682115224},
{784774720199608, 833252583851689}, {96955727304162, -163691394488867},
{533885337477640, -759274526814919}, {1803113514698232, -912868654936297},
{45247590348724, 72393183859539}, {217164748086520, 262367927958953},
{361625438979464, -697644847626201}, {2688155269173896, -4835442887039239},
{17178300942922744, -27882373057511721},
{85632576916711816, -108767251092164519},
{185077393403621624, 152963109298282359},
{256914272842714120, 228162067120741657},
{115008822887889852, 21329891101820275},
{66874939030307816, -88501259927880587},
{173010567180582168, 37594131598288795},
{119680726486894456, 163009762350405657},
{346632286908089608, 39122012965601975},
{21863319129312668, 12952671389765277}, {16168094600871544, 10840681019316125},
{42619308652443352, -78424372873688989},
{286440513769965096, -482562007869102835},
{1568971952793101912, -2219270254120447229},
{5202386410618762536, -2405085308184126995},
{784431588501017092, 1269174194514628473},
{3877940848108891048, 4873627230304925027},
{7965491057568271832, -8122739994362346867},
{1257991494352600280, 1610598426886535831},
{2820855460271484408, -1953972506540284567},
{6935063629849598728, 1124159151344918535},
{34452223067962558456, 43569632281595565737},
{72939273709064058248, -65917372630141300185},
{28087604315691032252, -45990557073959700787},
{143223622066149348280, -187067078914651118289},

```



```

{350 747 654 788 014 160 072, 137 389 469 013 654 076 033},
{491 366 018 023 584 544 216, 804 927 567 732 157 500 573},
{2 508 492 397 668 583 650 856, 3 280 987 499 108 501 642 483},
{6 179 960 811 519 343 933 016, -2 300 551 848 230 555 399 427},
{5 773 557 865 378 578 122 120, -3 968 121 942 497 547 027 799},
{14 443 487 383 048 248 754 568, 24 223 538 069 331 587 701 559},
{78 240 405 490 266 711 575 928, 109 393 266 720 130 805 744 249},
{249 222 889 838 912 753 346 568, 90 592 564 364 740 473 263 959},
{180 438 426 042 469 331 562 472, -25 541 614 003 355 126 307 093},
{3 294 256 037 966 894 825 642, -22 259 418 223 382 816 735},
{275 718 187 524 102 276, -354 298 572 782 011 949},
{628 643 082 063 277 384, 398 396 639 260 895 729},
{672 600 785 834 056 296, 1 012 741 488 063 385 231},
{2 721 125 617 834 631 480, 2 442 429 864 602 115 137},
{1 114 783 012 930 065 372, 1 130 151 108 200 453 915},
{122 944 762 163 108 344, 10 599 248 655 220 507}, {8 492 443 399 075 480, 11 709 720 860 976 471},
{25 738 219 695 207 928, 6 057 834 431 118 953}, {3 013 763 941 464 232, 437 333 589 064 007},
{190 284 727 935 268, -274 627 714 757 701}, {674 743 894 579 464, -417 610 873 433 815},
{641 911 409 152 664, -816 963 216 731 313}, {1 400 414 460 629 192, 1 109 099 698 912 385},
{2 330 518 093 734 456, -157 960 021 921 937}, {311 057 880 756 792, 58 330 887 442 927},
{155 227 548 337 256, -134 859 650 263 451}, {81 471 592 295 220, 91 966 239 234 151},
{41 978 587 755 724, -42 530 901 829 743}, {1 104 628 148 038, -546 877 813 459},
{10 872 521 120, 825 437 961}, {567 310 508, -1 094 904 593}, {4 220 752 680, -7 596 179 891},
{27 003 417 688, -43 868 804 413}, {134 923 093 800, -171 876 553 171},
{295 627 674 968, 229 455 184 867}, {529 379 920 808, -215 705 714 195},
{391 873 969 672, 655 688 775 699}, {2 110 518 448 216, 2 932 748 781 245},
{6 577 842 664 232, 2 027 150 073 939}, {3 971 139 539 320, 829 034 876 647},
{1 392 278 751 320, -1 237 198 851 811}, {620 319 598 036, -141 318 522 465},
{55 045 508 176, 71 982 821 717}, {135 498 508 328, -50 805 853 965},
{135 352 428 536, -118 043 828 857}, {69 234 398 716, 64 391 274 621},
{38 744 992 760, 64 719 656 133}, {207 797 306 984, 287 457 315 499},
{637 280 068 120, 169 801 739 973}, {83 853 783 544, -14 670 068 713},
{16 666 514 936, -5 902 470 525}, {8 327 173 112, 14 951 968 391},
{52 998 362 232, 85 752 906 521}, {262 036 354 312, 329 367 620 791},
{538 650 131 832, -547 671 705 479}, {9 021 573 647, -11 665 860 635},
{5 288 573 976, 2 838 497 113}, {776 840 500, 343 519 649}, {359 204 808, -17 840 035},
{1 202 054, 395 901}, {114 808, 53 041}, {17 452, -29 171}, {93 752, -129 921},
{289 352, -81 871}, {76 264, -131 781}, {444 136, -666 779}, {1 781 144, -1 567 701},
{853 772, 345 929}, {647 656, -1 125 951}, {3 826 360, -5 819 537},
{15 945 416, -15 232 191}, {2 852 900, 5 401 161}, {20 386 088, 35 786 803},
{123 205 720, 191 127 741}, {543 376 168, 576 560 723}, {66 369 110, -124 400 241},
{464 249 048, -803 763 133}, {2 716 112 680, -4 094 831 571}, {11 029 751 128, -9 981 633 053},
{4 192 472 300, -7 434 871 887}, {25 939 196 696, -41 035 412 101},
{120 769 723 240, -139 699 380 747}, {75 718 630 028, -28 021 859 729},
{66 775 593 272, -34 580 546 097}, {1 192 749 461, -1 197 343 597}, {2 297 068, 2 295 519},
{6196, 10 447}, {34 008, 48 205}, {113 576, 54 467}, {18 568, 2015}, {3464, 2697},
{6136, -2201}, {3736, 3131}, {4840, 6293}, {11 624, -5301}, {4088, -5363},
{10 200, 3379}, {252, -155}, {232, -279}, {188, -341}, {1224, -2015},
{6328, -8401}, {16 584, 2945}, {4344, 5053}, {2836, 1767}, {2792, 3751},
{7672, -279}, {1112, 2077}, {7720, 13 299}, {44 632, 66 557}, {175 400, 147 219},
{225 448, 304 141}, {629 544, 6355}, {798, 341}, {232, -217}, {30, 31}, {1, 0}

```

$\frac{2}{9}$  is a relation number with a list  $\{\{9, 8\}, \{1, 0\}\}$

known cases

$\frac{4}{9}$  is a relation number with a list  $\{\{9, 8\}, \{1, 0\}\}$

$\frac{5}{9}$  is a relation number with a list  $\{\{9, 10\}, \{1, 0\}\}$

known cases

$\frac{7}{9}$  is a relation number with a list  $\{\{9, 7\}, \{18, 7\}, \{1, 0\}\}$

$\frac{8}{9}$  is a relation number with a list  $\{\{9, 8\}, \{1, 0\}\}$

known cases

$\frac{10}{9}$  is a relation number with a list  $\{\{9, 10\}, \{1, 0\}\}$

$\frac{11}{9}$  is a relation number with a list  $\{\{9, 11\}, \{18, 11\}, \{36, -11\}, \{1, 0\}\}$

known cases

$\frac{13}{9}$  is a relation number with a list  $\{\{9, 13\}, \{36, -13\}, \{1, 0\}\}$

$\frac{14}{9}$  is a relation number with a list  $\{\{9, 14\}, \{45, 14\}, \{1, 0\}\}$

known cases

$\frac{16}{9}$  is a relation number with a list  $\{\{9, 16\}, \{63, -32\}, \{1, 0\}\}$

$\frac{17}{9}$  is a relation number with a list  $\{\{9, 17\}, \{72, -17\}, \{36, -17\}, \{18, 17\}, \{1, 0\}\}$

known cases

$\frac{19}{9}$  is a relation number with a list  $\{\{9, 19\}, \{90, 19\}, \{45, 19\}, \{63, 38\}, \{117, -95\}, \{198, -19\}, \{72, -19\}, \{36, 19\}, \{18, 19\}, \{1, 0\}\}$

$\frac{20}{9}$  is a relation number with a list  $\{\{9, 20\}, \{99, 40\}, \{171, -20\}, \{1, 0\}\}$

known cases

$\frac{22}{9}$  is a relation number with a list  $\{\{9, 22\}, \{117, 88\}, \{261, 154\}, \{423, -352\}, \{639, -44\}, \{63, -22\}, \{1, 0\}\}$

$\frac{23}{9}$  is a relation number with a list  $\{\{9, 23\}, \{126, 115\}, \{99, 23\}, \{63, 46\}, \{153, 23\}, \{72, -23\}, \{1, 0\}\}$

known cases

$\frac{25}{9}$  is a relation number with a list  $\{\{9, 25\}, \{144, 175\}, \{279, -25\}, \{36, -25\}, \{99, 50\}, \{1, 0\}\}$

$\frac{26}{9}$  is a relation number with a list  
 $\{\{9, 26\}, \{153, 208\}, \{495, -442\}, \{159, 52\}, \{1, 0\}\}$

known cases

$\frac{28}{9}$  is a relation number with a list  $\{\{9, 28\}, \{171, 280\}, \{981, 532\}, \{747, -140\},$   
 $\{423, 56\}, \{225, 196\}, \{261, 140\}, \{171, -196\}, \{75, -112\}, \{333, -28\}, \{1, 0\}\}$

$\frac{29}{9}$  is a relation number with a list  
 $\{\{9, 29\}, \{180, 319\}, \{1251, 1160\}, \{819, -116\}, \{63, -29\}, \{45, 29\}, \{117, 116\}, \{1, 0\}\}$

known cases

$\frac{31}{9}$  is a relation number with a list  
 $\{\{9, 31\}, \{198, 403\}, \{1845, 2728\}, \{7947, 2821\}, \{1548, 2201\}, \{5877, 434\},$   
 $\{1791, 2263\}, \{4248, -5735\}, \{13383, 5518\}, \{21123, -23095\}, \{5916, 8153\},$   
 $\{20133, -4030\}, \{51, -31\}, \{99, -62\}, \{225, -217\}, \{72, 31\}, \{90, -31\}, \{1, 0\}\}$

$\frac{32}{9}$  is a relation number with a list  
 $\{\{9, 32\}, \{207, 448\}, \{2169, 3680\}, \{13599, 15232\}, \{4899, 6560\},$   
 $\{14949, -5888\}, \{8145, -11296\}, \{28359, 832\}, \{213, 224\}, \{33, 32\}, \{1, 0\}\}$

known cases

$\frac{34}{9}$  is a relation number with a list  
 $\{\{9, 34\}, \{225, 544\}, \{2871, 5950\}, \{27711, 51136\}, \{210825, 336226\},$   
 $\{1128609, 1237600\}, \{326973, -7106\}, \{873, -1292\}, \{3771, -2618\},$   
 $\{10377, 15640\}, \{47367, 38182\}, \{82665, 31348\}, \{34137, 34918\}, \{2343, 1462\},$   
 $\{5229, 6596\}, \{12303, -12886\}, \{1749, -986\}, \{2007, 1292\}, \{5193, 7990\},$   
 $\{25173, 23188\}, \{5955, 2074\}, \{801, -170\}, \{441, -136\}, \{99, -34\}, \{1, 0\}\}$

No answers up to 5000 iterations for  $\frac{35}{9}$

known cases

$\frac{3}{10}$  is a relation number with a list  $\{\{10, 9\}, \{1, 0\}\}$

known cases

known cases

known cases

$\frac{7}{10}$  is a relation number with a list  $\{\{10, 7\}, \{30, 7\}, \{1, 0\}\}$

known cases

$\frac{9}{10}$  is a relation number with a list  $\{\{10, 9\}, \{1, 0\}\}$

known cases

$\frac{11}{10}$  is a relation number with a list  $\{\{10, 11\}, \{1, 0\}\}$

known cases

$\frac{13}{10}$  is a relation number with a list  $\{\{10, 13\}, \{30, -13\}, \{20, 13\}, \{30, 13\}\}$

known cases

known cases

known cases

$\frac{17}{10}$  is a relation number with a list

$\{\{10, 17\}, \{70, -51\}, \{95, 68\}, \{270, 221\}, \{490, -289\}, \{440, -51\}, \{95, -68\}\}$

known cases

$\frac{19}{10}$  is a relation number with a list  $\{\{10, 19\}, \{90, -19\}, \{1, 0\}\}$

known cases

$\frac{21}{10}$  is a relation number with a list  $\{\{10, 21\}, \{110, 21\}, \{1, 0\}\}$

known cases

$\frac{23}{10}$  is a relation number with a list

$\{\{10, 23\}, \{130, 69\}, \{40, 23\}, \{30, 23\}, \{70, 69\}, \{1, 0\}\}$

known cases

known cases

known cases

$\frac{27}{10}$  is a relation number with a list

$\{\{10, 27\}, \{170, 189\}, \{95, 81\}, \{70, 27\}, \{110, 27\}, \{1, 0\}\}$

known cases

$\frac{29}{10}$  is a relation number with a list  $\{\{10, 29\}, \{190, 261\}, \{710, -551\},$

$\{1590, -899\}, \{1040, 1479\}, \{4390, -2059\}, \{1360, 1537\}, \{1770, 29\}, \{1, 0\}\}$

known cases

$\frac{31}{10}$  is a relation number with a list

$\{\{10, 31\}, \{210, 341\}, \{1310, 651\}, \{40, 31\}, \{90, 31\}, \{30, -31\}, \{1, 0\}\}$

known cases

$\frac{33}{10}$  is a relation number with a list  $\{\{10, 33\}, \{230, 429\}, \{1990, 2277\},$

$\{1435, -1914\}, \{4790, 3333\}, \{14570, -14751\}, \{362, -363\}, \{1, 0\}\}$

known cases

known cases

known cases

```

37
10 is a relation number with a list
10
{{10, 37}, {270, 629}, {3590, 6993}, {34030, 55981}, {219510, 252377},
{164335, -45806}, {188890, -240833}, {519430, 486439}, {164955, -9139},
{906, -1517}, {6110, -7437}, {6635, -11914}, {52790, -76183},
{233930, -103711}, {132540, -28157}, {16490, -4699}, {5765, -9583},
{9545, -11359}, {9070, -10323}, {6265, 5254}, {10110, 15133},
{50230, 34521}, {157090, -236023}, {789330, -560291}, {2290390, 2871533},
{5811430, -7213039}, {14016090, 20270857}, {62547670, 28717809},
{25560260, -45556879}, {199966190, -284306113}, {843399230, -277516021},
{108511670, 35292043}, {13177705, -18569819}, {13480285, -3452507},
{3297430, -2076403}, {4276880, -5442441}, {11655610, 11298653},
{3569570, -5880151}, {23105810, -26689987}, {17920885, 835386},
{3777790, -5623963}, {18461730, -12068771}, {28379060, -44658667},
{162796070, -155758789}, {35186405, 2344246}, {22715, -9028},
{43690, -71373}, {276830, -310541}, {168555, 305398}, {1368430, 2009211},
{6407810, 3616787}, {4128820, -2807301}, {13215190, 20823193},
{76080030, 73264181}, {28158490, 3336919}, {3657845, -5191729},
{7669420, -2418209}, {2073965, 3256296}, {11823310, 11183287},
{1280046, -1314277}, {34231, 47730}, {134990, 22163}, {10060, -851}, {760, -1369},
{6090, -8843}, {27530, -13431}, {668, -1073}, {810, -851}, {205, -296},
{910, -407}, {480, -259}, {190, -111}, {160, -37}, {60, 37}, {35, 37}, {1, 0}}

```

known cases

No answers up to 5000 iterations for  $\frac{39}{10}$

Unresolved cases are :{{35, 9}, {39, 10}}: END

```

ln[16]:= excp = {};
For[s = 2, s ≤ 30, s++, For[r = 2, r ≤ 10 s, r++,
  If[GCD[s, r] == 1 && ! ReNum[s, r, 5000], excp = Append[excp, {s, r}]]];];
Print["Unresolved cases are :", excp, ": END"];

2
3 is a relation number with a list {{3, 2}, {1, 0}}

2
5 is a relation number with a list {{5, 4}, {1, 0}}

2
7 is a relation number with a list {{7, 6}, {1, 0}}

2
9 is a relation number with a list {{9, 8}, {1, 0}}

2
11 is a relation number with a list {{11, 10}, {1, 0}}

2
13 is a relation number with a list {{13, 12}, {1, 0}}

2
15 is a relation number with a list {{15, 14}, {1, 0}}

2
17 is a relation number with a list {{17, 16}, {1, 0}}

```

```

2
— is a relation number with a list {{19, 18}, {1, 0}}
19
3
— is a relation number with a list {{2, 3}, {1, 0}}
2
3
— is a relation number with a list {{4, 3}, {1, 0}}
4
3
— is a relation number with a list {{5, 6}, {1, 0}}
5
3
— is a relation number with a list {{7, 6}, {1, 0}}
7
3
— is a relation number with a list {{8, 9}, {1, 0}}
8
3
— is a relation number with a list {{10, 9}, {1, 0}}
10
3
— is a relation number with a list {{11, 12}, {1, 0}}
11
3
— is a relation number with a list {{13, 12}, {1, 0}}
13
3
— is a relation number with a list {{14, 15}, {1, 0}}
14
3
— is a relation number with a list {{16, 15}, {1, 0}}
16
3
— is a relation number with a list {{17, 18}, {1, 0}}
17
3
— is a relation number with a list {{19, 18}, {1, 0}}
19
3
— is a relation number with a list {{20, 21}, {1, 0}}
20
3
— is a relation number with a list {{22, 21}, {1, 0}}
22
3
— is a relation number with a list {{23, 24}, {1, 0}}
23
3
— is a relation number with a list {{25, 24}, {1, 0}}
25
3
— is a relation number with a list {{26, 27}, {1, 0}}
26
3
— is a relation number with a list {{28, 27}, {1, 0}}
28
3
— is a relation number with a list {{29, 30}, {1, 0}}
29
4
— is a relation number with a list {{3, 4}, {1, 0}}
3
4
— is a relation number with a list {{5, 4}, {1, 0}}
5
4
— is a relation number with a list {{7, 8}, {1, 0}}
7

```

```

4
— is a relation number with a list {{9, 8}, {1, 0}}
9

4
— is a relation number with a list {{11, 12}, {1, 0}}
11

4
— is a relation number with a list {{13, 12}, {1, 0}}
13

4
— is a relation number with a list {{15, 16}, {1, 0}}
15

4
— is a relation number with a list {{17, 16}, {1, 0}}
17

4
— is a relation number with a list {{19, 20}, {1, 0}}
19

4
— is a relation number with a list {{21, 20}, {1, 0}}
21

4
— is a relation number with a list {{23, 24}, {1, 0}}
23

4
— is a relation number with a list {{25, 24}, {1, 0}}
25

4
— is a relation number with a list {{27, 28}, {1, 0}}
27

4
— is a relation number with a list {{29, 28}, {1, 0}}
29

4
— is a relation number with a list {{31, 32}, {1, 0}}
31

4
— is a relation number with a list {{33, 32}, {1, 0}}
33

4
— is a relation number with a list {{35, 36}, {1, 0}}
35

4
— is a relation number with a list {{37, 36}, {1, 0}}
37

4
— is a relation number with a list {{39, 40}, {1, 0}}
39

5
— is a relation number with a list {{2, 5}, {6, 5}, {1, 0}}
2

5
— is a relation number with a list {{3, 5}, {6, 5}, {1, 0}}
3

5
— is a relation number with a list {{4, 5}, {1, 0}}
4

5
— is a relation number with a list {{6, 5}, {1, 0}}
6

5
— is a relation number with a list {{7, 5}, {14, 5}, {1, 0}}
7

5
— is a relation number with a list {{8, 10}, {1, 0}}
8

5
— is a relation number with a list {{9, 10}, {1, 0}}
9

```

```

5
— 11 is a relation number with a list {{11, 10}, {1, 0}}
5
— 12 is a relation number with a list {{12, 10}, {1, 0}}
5
— 13 is a relation number with a list {{13, 15}, {26, 5}, {1, 0}}
5
— 14 is a relation number with a list {{14, 15}, {1, 0}}
5
— 16 is a relation number with a list {{16, 15}, {1, 0}}
5
— 17 is a relation number with a list {{17, 15}, {34, 5}, {1, 0}}
5
— 18 is a relation number with a list {{18, 20}, {1, 0}}
5
— 19 is a relation number with a list {{19, 20}, {1, 0}}
5
— 21 is a relation number with a list {{21, 20}, {1, 0}}
5
— 22 is a relation number with a list {{22, 20}, {1, 0}}
5
— 23 is a relation number with a list {{23, 25}, {46, 5}, {1, 0}}
5
— 24 is a relation number with a list {{24, 25}, {1, 0}}
5
— 26 is a relation number with a list {{26, 25}, {1, 0}}
5
— 27 is a relation number with a list {{27, 25}, {54, 5}, {1, 0}}
5
— 28 is a relation number with a list {{28, 30}, {1, 0}}
5
— 29 is a relation number with a list {{29, 30}, {1, 0}}
5
— 31 is a relation number with a list {{31, 30}, {1, 0}}
5
— 32 is a relation number with a list {{32, 30}, {1, 0}}
5
— 33 is a relation number with a list {{33, 35}, {66, 5}, {1, 0}}
5
— 34 is a relation number with a list {{34, 35}, {1, 0}}
5
— 36 is a relation number with a list {{36, 35}, {1, 0}}
5
— 37 is a relation number with a list {{37, 35}, {74, 5}, {1, 0}}
5
— 38 is a relation number with a list {{38, 40}, {1, 0}}

```



```

5
— is a relation number with a list {{39, 40}, {1, 0}}
39

5
— is a relation number with a list {{41, 40}, {1, 0}}
41

5
— is a relation number with a list {{42, 40}, {1, 0}}
42

5
— is a relation number with a list {{43, 45}, {86, 5}, {1, 0}}
43

5
— is a relation number with a list {{44, 45}, {1, 0}}
44

5
— is a relation number with a list {{46, 45}, {1, 0}}
46

5
— is a relation number with a list {{47, 45}, {94, 5}, {1, 0}}
47

5
— is a relation number with a list {{48, 50}, {1, 0}}
48

5
— is a relation number with a list {{49, 50}, {1, 0}}
49

6
— is a relation number with a list {{5, 6}, {1, 0}}
5

6
— is a relation number with a list {{7, 6}, {1, 0}}
7

6
— is a relation number with a list {{11, 12}, {1, 0}}
11

6
— is a relation number with a list {{13, 12}, {1, 0}}
13

6
— is a relation number with a list {{17, 18}, {1, 0}}
17

6
— is a relation number with a list {{19, 18}, {1, 0}}
19

6
— is a relation number with a list {{23, 24}, {1, 0}}
23

6
— is a relation number with a list {{25, 24}, {1, 0}}
25

6
— is a relation number with a list {{29, 30}, {1, 0}}
29

6
— is a relation number with a list {{31, 30}, {1, 0}}
31

6
— is a relation number with a list {{35, 36}, {1, 0}}
35

6
— is a relation number with a list {{37, 36}, {1, 0}}
37

6
— is a relation number with a list {{41, 42}, {1, 0}}
41

6
— is a relation number with a list {{43, 42}, {1, 0}}
43

```

```

6
— is a relation number with a list {{47, 48}, {1, 0}}
47

6
— is a relation number with a list {{49, 48}, {1, 0}}
49

6
— is a relation number with a list {{53, 54}, {1, 0}}
53

6
— is a relation number with a list {{55, 54}, {1, 0}}
55

6
— is a relation number with a list {{59, 60}, {1, 0}}
59

7
— is a relation number with a list
2
  {{2, 7}, {10, 21}, {22, 35}, {26, 21}, {10, 7}, {6, -7}, {1, 0}}

7
— is a relation number with a list {{3, 7}, {12, 7}, {6, 7}, {1, 0}}
3

7
— is a relation number with a list {{4, 7}, {12, -7}, {1, 0}}
4

7
— is a relation number with a list {{5, 7}, {10, 7}, {15, -7}, {1, 0}}
5

7
— is a relation number with a list {{6, 7}, {1, 0}}
6

7
— is a relation number with a list {{8, 7}, {1, 0}}
8

7
— is a relation number with a list {{9, 7}, {18, 7}, {1, 0}}
9

7
— is a relation number with a list {{10, 7}, {30, 7}, {1, 0}}
10

7
— is a relation number with a list {{11, 14}, {33, -7}, {22, 7}, {1, 0}}
11

7
— is a relation number with a list {{12, 14}, {1, 0}}
12

7
— is a relation number with a list {{13, 14}, {1, 0}}
13

7
— is a relation number with a list {{15, 14}, {1, 0}}
15

7
— is a relation number with a list {{16, 14}, {1, 0}}
16

7
— is a relation number with a list {{17, 14}, {51, 7}, {34, 7}, {1, 0}}
17

7
— is a relation number with a list {{18, 21}, {1, 0}}
18

7
— is a relation number with a list {{19, 21}, {38, 7}, {57, 7}, {1, 0}}
19

7
— is a relation number with a list {{20, 21}, {1, 0}}
20

```

```

7
— is a relation number with a list {{22, 21}, {1, 0}}
22

7
— is a relation number with a list {{23, 21}, {46, 7}, {69, 7}, {1, 0}}
23

7
— is a relation number with a list {{24, 21}, {1, 0}}
24

7
— is a relation number with a list {{25, 28}, {75, -7}, {50, 7}, {1, 0}}
25

7
— is a relation number with a list {{26, 28}, {1, 0}}
26

7
— is a relation number with a list {{27, 28}, {1, 0}}
27

7
— is a relation number with a list {{29, 28}, {1, 0}}
29

7
— is a relation number with a list {{30, 28}, {1, 0}}
30

7
— is a relation number with a list {{31, 28}, {93, 7}, {62, 7}, {1, 0}}
31

7
— is a relation number with a list {{32, 35}, {96, -7}, {1, 0}}
32

7
— is a relation number with a list {{33, 35}, {66, 7}, {1, 0}}
33

7
— is a relation number with a list {{34, 35}, {1, 0}}
34

7
— is a relation number with a list {{36, 35}, {1, 0}}
36

7
— is a relation number with a list {{37, 35}, {74, 7}, {111, -7}, {1, 0}}
37

7
— is a relation number with a list {{38, 35}, {114, 7}, {1, 0}}
38

7
— is a relation number with a list {{39, 42}, {1, 0}}
39

7
— is a relation number with a list {{40, 42}, {1, 0}}
40

7
— is a relation number with a list {{41, 42}, {1, 0}}
41

7
— is a relation number with a list {{43, 42}, {1, 0}}
43

7
— is a relation number with a list {{44, 42}, {1, 0}}
44

7
— is a relation number with a list {{45, 42}, {1, 0}}
45

7
— is a relation number with a list {{46, 49}, {138, -7}, {1, 0}}
46

7
— is a relation number with a list {{47, 49}, {94, 7}, {141, -7}, {1, 0}}
47

```

```

7
— 48 is a relation number with a list {{48, 49}, {1, 0}}
7
— 50 is a relation number with a list {{50, 49}, {1, 0}}
7
— 51 is a relation number with a list {{51, 49}, {102, 7}, {1, 0}}
7
— 52 is a relation number with a list {{52, 49}, {156, 7}, {1, 0}}
7
— 53 is a relation number with a list {{53, 56}, {159, -7}, {106, 7}, {1, 0}}
7
— 54 is a relation number with a list {{54, 56}, {1, 0}}
7
— 55 is a relation number with a list {{55, 56}, {1, 0}}
7
— 57 is a relation number with a list {{57, 56}, {1, 0}}
7
— 58 is a relation number with a list {{58, 56}, {1, 0}}
7
— 59 is a relation number with a list {{59, 56}, {177, 7}, {118, 7}, {1, 0}}
7
— 60 is a relation number with a list {{60, 63}, {1, 0}}
7
— 61 is a relation number with a list {{61, 63}, {122, 7}, {183, 7}, {1, 0}}
7
— 62 is a relation number with a list {{62, 63}, {1, 0}}
7
— 64 is a relation number with a list {{64, 63}, {1, 0}}
7
— 65 is a relation number with a list {{65, 63}, {130, 7}, {195, 7}, {1, 0}}
7
— 66 is a relation number with a list {{66, 63}, {1, 0}}
7
— 67 is a relation number with a list {{67, 70}, {201, -7}, {134, 7}, {1, 0}}
7
— 68 is a relation number with a list {{68, 70}, {1, 0}}
7
— 69 is a relation number with a list {{69, 70}, {1, 0}}
8
— 3 is a relation number with a list {{3, 8}, {15, 16}, {1, 0}}
8
— 5 is a relation number with a list {{5, 8}, {15, 8}, {1, 0}}
8
— 7 is a relation number with a list {{7, 8}, {1, 0}}
8
— 9 is a relation number with a list {{9, 8}, {1, 0}}

```

```

8
— is a relation number with a list {{11, 8}, {33, -8}, {1, 0}}
11

8
— is a relation number with a list {{13, 16}, {39, 8}, {1, 0}}
13

8
— is a relation number with a list {{15, 16}, {1, 0}}
15

8
— is a relation number with a list {{17, 16}, {1, 0}}
17

8
— is a relation number with a list {{19, 16}, {57, -8}, {1, 0}}
19

8
— is a relation number with a list {{21, 24}, {1, 0}}
21

8
— is a relation number with a list {{23, 24}, {1, 0}}
23

8
— is a relation number with a list {{25, 24}, {1, 0}}
25

8
— is a relation number with a list {{27, 24}, {1, 0}}
27

8
— is a relation number with a list {{29, 32}, {87, 8}, {1, 0}}
29

8
— is a relation number with a list {{31, 32}, {1, 0}}
31

8
— is a relation number with a list {{33, 32}, {1, 0}}
33

8
— is a relation number with a list {{35, 32}, {105, -8}, {1, 0}}
35

8
— is a relation number with a list {{37, 40}, {111, 8}, {1, 0}}
37

8
— is a relation number with a list {{39, 40}, {1, 0}}
39

8
— is a relation number with a list {{41, 40}, {1, 0}}
41

8
— is a relation number with a list {{43, 40}, {129, -8}, {1, 0}}
43

8
— is a relation number with a list {{45, 48}, {1, 0}}
45

8
— is a relation number with a list {{47, 48}, {1, 0}}
47

8
— is a relation number with a list {{49, 48}, {1, 0}}
49

8
— is a relation number with a list {{51, 48}, {1, 0}}
51

8
— is a relation number with a list {{53, 56}, {159, 8}, {1, 0}}
53

8
— is a relation number with a list {{55, 56}, {1, 0}}
55

```

$\frac{8}{57}$  is a relation number with a list  $\{\{57, 56\}, \{1, 0\}\}$   
 $\frac{8}{59}$  is a relation number with a list  $\{\{59, 56\}, \{177, -8\}, \{1, 0\}\}$   
 $\frac{8}{61}$  is a relation number with a list  $\{\{61, 64\}, \{183, 8\}, \{1, 0\}\}$   
 $\frac{8}{63}$  is a relation number with a list  $\{\{63, 64\}, \{1, 0\}\}$   
 $\frac{8}{65}$  is a relation number with a list  $\{\{65, 64\}, \{1, 0\}\}$   
 $\frac{8}{67}$  is a relation number with a list  $\{\{67, 64\}, \{201, -8\}, \{1, 0\}\}$   
 $\frac{8}{69}$  is a relation number with a list  $\{\{69, 72\}, \{1, 0\}\}$   
 $\frac{8}{71}$  is a relation number with a list  $\{\{71, 72\}, \{1, 0\}\}$   
 $\frac{8}{73}$  is a relation number with a list  $\{\{73, 72\}, \{1, 0\}\}$   
 $\frac{8}{75}$  is a relation number with a list  $\{\{75, 72\}, \{1, 0\}\}$   
 $\frac{8}{77}$  is a relation number with a list  $\{\{77, 80\}, \{231, 8\}, \{1, 0\}\}$   
 $\frac{8}{79}$  is a relation number with a list  $\{\{79, 80\}, \{1, 0\}\}$

known cases

$\frac{9}{4}$  is a relation number with a list  $\{\{4, 9\}, \{20, 9\}, \{1, 0\}\}$   
 $\frac{9}{5}$  is a relation number with a list  $\{\{5, 9\}, \{20, -9\}, \{10, 9\}, \{1, 0\}\}$   
 $\frac{9}{7}$  is a relation number with a list  $\{\{7, 9\}, \{14, 9\}, \{28, 9\}, \{1, 0\}\}$   
 $\frac{9}{8}$  is a relation number with a list  $\{\{8, 9\}, \{1, 0\}\}$   
 $\frac{9}{10}$  is a relation number with a list  $\{\{10, 9\}, \{1, 0\}\}$   
 $\frac{9}{11}$  is a relation number with a list  $\{\{11, 9\}, \{22, 9\}, \{44, -9\}, \{1, 0\}\}$   
 $\frac{9}{13}$  is a relation number with a list  $\{\{13, 9\}, \{52, 9\}, \{26, 9\}, \{1, 0\}\}$   
 $\frac{9}{14}$  is a relation number with a list  $\{\{14, 18\}, \{1, 0\}\}$   
 $\frac{9}{16}$  is a relation number with a list  $\{\{16, 18\}, \{1, 0\}\}$   
 $\frac{9}{17}$  is a relation number with a list  $\{\{17, 18\}, \{1, 0\}\}$

```

9
— is a relation number with a list {{19, 18}, {1, 0}}
19
9
— is a relation number with a list {{20, 18}, {1, 0}}
20
9
— is a relation number with a list {{22, 18}, {1, 0}}
22
9
— is a relation number with a list {{23, 27}, {92, -9}, {46, 9}, {1, 0}}
23
9
— is a relation number with a list {{25, 27}, {50, 9}, {100, -9}, {1, 0}}
25
9
— is a relation number with a list {{26, 27}, {1, 0}}
26
9
— is a relation number with a list {{28, 27}, {1, 0}}
28
9
— is a relation number with a list {{29, 27}, {58, 9}, {116, 9}, {1, 0}}
29
9
— is a relation number with a list {{31, 27}, {124, 9}, {62, 9}, {1, 0}}
31
9
— is a relation number with a list {{32, 36}, {1, 0}}
32
9
— is a relation number with a list {{34, 36}, {1, 0}}
34
9
— is a relation number with a list {{35, 36}, {1, 0}}
35
9
— is a relation number with a list {{37, 36}, {1, 0}}
37
9
— is a relation number with a list {{38, 36}, {1, 0}}
38
9
— is a relation number with a list {{40, 36}, {1, 0}}
40
9
— is a relation number with a list {{41, 45}, {164, -9}, {82, 9}, {1, 0}}
41
9
— is a relation number with a list {{43, 45}, {86, 9}, {172, 9}, {1, 0}}
43
9
— is a relation number with a list {{44, 45}, {1, 0}}
44
9
— is a relation number with a list {{46, 45}, {1, 0}}
46
9
— is a relation number with a list {{47, 45}, {94, 9}, {188, -9}, {1, 0}}
47
9
— is a relation number with a list {{49, 45}, {196, 9}, {98, 9}, {1, 0}}
49
9
— is a relation number with a list {{50, 54}, {1, 0}}
50
9
— is a relation number with a list {{52, 54}, {1, 0}}
52

```

```

9
— is a relation number with a list {{53, 54}, {1, 0}}
53
9
— is a relation number with a list {{55, 54}, {1, 0}}
55
9
— is a relation number with a list {{56, 54}, {1, 0}}
56
9
— is a relation number with a list {{58, 54}, {1, 0}}
58
9
— is a relation number with a list {{59, 63}, {236, -9}, {118, 9}, {1, 0}}
59
9
— is a relation number with a list {{61, 63}, {122, 9}, {244, -9}, {1, 0}}
61
9
— is a relation number with a list {{62, 63}, {1, 0}}
62
9
— is a relation number with a list {{64, 63}, {1, 0}}
64
9
— is a relation number with a list {{65, 63}, {130, 9}, {260, 9}, {1, 0}}
65
9
— is a relation number with a list {{67, 63}, {268, 9}, {134, 9}, {1, 0}}
67
9
— is a relation number with a list {{68, 72}, {1, 0}}
68
9
— is a relation number with a list {{70, 72}, {1, 0}}
70
9
— is a relation number with a list {{71, 72}, {1, 0}}
71
9
— is a relation number with a list {{73, 72}, {1, 0}}
73
9
— is a relation number with a list {{74, 72}, {1, 0}}
74
9
— is a relation number with a list {{76, 72}, {1, 0}}
76
9
— is a relation number with a list {{77, 81}, {308, -9}, {154, 9}, {1, 0}}
77
9
— is a relation number with a list {{79, 81}, {158, 9}, {316, 9}, {1, 0}}
79
9
— is a relation number with a list {{80, 81}, {1, 0}}
80
9
— is a relation number with a list {{82, 81}, {1, 0}}
82
9
— is a relation number with a list {{83, 81}, {166, 9}, {332, -9}, {1, 0}}
83
9
— is a relation number with a list {{85, 81}, {340, 9}, {170, 9}, {1, 0}}
85
9
— is a relation number with a list {{86, 90}, {1, 0}}
86

```



```

9
— is a relation number with a list {{88, 90}, {1, 0}}
88
9
— is a relation number with a list {{89, 90}, {1, 0}}
89
10
— is a relation number with a list
3
  {{3, 10}, {21, 40}, {57, 70}, {39, 50}, {33, -40}, {21, -20}, {1, 0}}
10
— is a relation number with a list {{7, 10}, {21, -10}, {1, 0}}
7
10
— is a relation number with a list {{9, 10}, {1, 0}}
9
10
— is a relation number with a list {{11, 10}, {1, 0}}
11
10
— is a relation number with a list {{13, 10}, {39, 10}, {1, 0}}
13
10
— is a relation number with a list {{17, 20}, {51, -10}, {1, 0}}
17
10
— is a relation number with a list {{19, 20}, {1, 0}}
19
10
— is a relation number with a list {{21, 20}, {1, 0}}
21
10
— is a relation number with a list {{23, 20}, {69, 10}, {1, 0}}
23
10
— is a relation number with a list {{27, 30}, {1, 0}}
27
10
— is a relation number with a list {{29, 30}, {1, 0}}
29
10
— is a relation number with a list {{31, 30}, {1, 0}}
31
10
— is a relation number with a list {{33, 30}, {1, 0}}
33
10
— is a relation number with a list {{37, 40}, {111, -10}, {1, 0}}
37
10
— is a relation number with a list {{39, 40}, {1, 0}}
39
10
— is a relation number with a list {{41, 40}, {1, 0}}
41
10
— is a relation number with a list {{43, 40}, {129, 10}, {1, 0}}
43
10
— is a relation number with a list {{47, 50}, {141, -10}, {1, 0}}
47
10
— is a relation number with a list {{49, 50}, {1, 0}}
49
10
— is a relation number with a list {{51, 50}, {1, 0}}
51

```

```

10
— is a relation number with a list {{53, 50}, {159, 10}, {1, 0}}
53
10
— is a relation number with a list {{57, 60}, {1, 0}}
57
10
— is a relation number with a list {{59, 60}, {1, 0}}
59
10
— is a relation number with a list {{61, 60}, {1, 0}}
61
10
— is a relation number with a list {{63, 60}, {1, 0}}
63
10
— is a relation number with a list {{67, 70}, {201, -10}, {1, 0}}
67
10
— is a relation number with a list {{69, 70}, {1, 0}}
69
10
— is a relation number with a list {{71, 70}, {1, 0}}
71
10
— is a relation number with a list {{73, 70}, {219, 10}, {1, 0}}
73
10
— is a relation number with a list {{77, 80}, {231, -10}, {1, 0}}
77
10
— is a relation number with a list {{79, 80}, {1, 0}}
79
10
— is a relation number with a list {{81, 80}, {1, 0}}
81
10
— is a relation number with a list {{83, 80}, {249, 10}, {1, 0}}
83
10
— is a relation number with a list {{87, 90}, {1, 0}}
87
10
— is a relation number with a list {{89, 90}, {1, 0}}
89
10
— is a relation number with a list {{91, 90}, {1, 0}}
91
10
— is a relation number with a list {{93, 90}, {1, 0}}
93
10
— is a relation number with a list {{97, 100}, {291, -10}, {1, 0}}
97
10
— is a relation number with a list {{99, 100}, {1, 0}}
99

```

known cases

```

11
— is a relation number with a list {{3, 11}, {24, 55}, {93, 176}, {249, 385},
3
  {408, 341}, {201, 286}, {255, 77}, {24, -11}, {6, 11}, {15, 22}, {21, 11}, {1, 0}}
11
— is a relation number with a list {{4, 11}, {28, 33}, {10, -11}, {1, 0}}
4

```

```

11
5 is a relation number with a list
  {{5, 11}, {30, 11}, {15, 11}, {20, 11}, {10, 11}, {1, 0}}

11
6 is a relation number with a list {{6, 11}, {30, -11}, {1, 0}}

11
7 is a relation number with a list
  {{7, 11}, {28, 11}, {35, -22}, {63, -44}, {133, -99}, {238, 55}, {126, -11}, {35, -22}}

11
8 is a relation number with a list {{8, 11}, {24, 11}, {1, 0}}

11
9 is a relation number with a list {{9, 11}, {18, 11}, {36, -11}, {1, 0}}

11
10 is a relation number with a list {{10, 11}, {1, 0}}

11
12 is a relation number with a list {{12, 11}, {1, 0}}

11
13 is a relation number with a list
  {{13, 11}, {26, 11}, {52, 11}, {39, -11}, {65, -22}, {1, 0}}

11
14 is a relation number with a list {{14, 11}, {42, -11}, {1, 0}}

11
15 is a relation number with a list {{15, 11}, {60, -11}, {1, 0}}

11
16 is a relation number with a list {{16, 11}, {80, 11}, {48, 11}, {1, 0}}

11
17 is a relation number with a list
  {{17, 22}, {85, 11}, {51, 11}, {68, -11}, {34, 11}, {1, 0}}

11
18 is a relation number with a list {{18, 22}, {1, 0}}

11
19 is a relation number with a list
  {{19, 22}, {57, 11}, {38, 11}, {95, -11}, {76, -11}, {1, 0}}

11
20 is a relation number with a list {{20, 22}, {1, 0}}

11
21 is a relation number with a list {{21, 22}, {1, 0}}

11
23 is a relation number with a list {{23, 22}, {1, 0}}

11
24 is a relation number with a list {{24, 22}, {1, 0}}

11
25 is a relation number with a list {{25, 22}, {75, -11}, {50, 11}, {1, 0}}

11
26 is a relation number with a list {{26, 22}, {1, 0}}

```

```

11
— is a relation number with a list {{27, 22}, {135, -11}, {1, 0}}
27

11
— is a relation number with a list {{28, 33}, {140, 11}, {84, -11}, {1, 0}}
28

11
— is a relation number with a list
29
  {{29, 33}, {116, 11}, {145, 11}, {58, 11}, {87, -11}, {1, 0}}

11
— is a relation number with a list {{30, 33}, {1, 0}}
30

11
— is a relation number with a list
31
  {{31, 33}, {62, 11}, {124, 11}, {93, 11}, {155, 11}, {1, 0}}

11
— is a relation number with a list {{32, 33}, {1, 0}}
32

11
— is a relation number with a list {{34, 33}, {1, 0}}
34

11
— is a relation number with a list {{35, 33}, {70, 11}, {140, -11}, {105, -11}, {1, 0}}
35

11
— is a relation number with a list {{36, 33}, {1, 0}}
36

11
— is a relation number with a list
37
  {{37, 33}, {148, -11}, {185, -22}, {333, -22}, {111, 11}, {1, 0}}

11
— is a relation number with a list {{38, 33}, {190, -11}, {114, 11}, {76, 11}, {1, 0}}
38

11
— is a relation number with a list {{39, 44}, {195, -11}, {1, 0}}
39

11
— is a relation number with a list {{40, 44}, {1, 0}}
40

11
— is a relation number with a list
41
  {{41, 44}, {123, 11}, {82, 11}, {205, 11}, {164, -11}, {1, 0}}

11
— is a relation number with a list {{42, 44}, {1, 0}}
42

11
— is a relation number with a list {{43, 44}, {1, 0}}
43

11
— is a relation number with a list {{45, 44}, {1, 0}}
45

11
— is a relation number with a list {{46, 44}, {1, 0}}
46

11
— is a relation number with a list
47
  {{47, 44}, {141, -11}, {94, 11}, {235, -22}, {329, 33}, {1, 0}}

11
— is a relation number with a list {{48, 44}, {1, 0}}
48

```

```

11
— is a relation number with a list
49
  {{49, 44}, {245, 11}, {147, 11}, {196, 11}, {98, 11}, {1, 0}}

11
— is a relation number with a list {{50, 55}, {1, 0}}
50

11
— is a relation number with a list {{51, 55}, {204, 11}, {255, -11}, {102, 11}, {1, 0}}
51

11
— is a relation number with a list {{52, 55}, {156, 11}, {1, 0}}
52

11
— is a relation number with a list
53
  {{53, 55}, {106, 11}, {212, -11}, {159, 11}, {265, -22}, {1, 0}}

11
— is a relation number with a list {{54, 55}, {1, 0}}
54

11
— is a relation number with a list {{56, 55}, {1, 0}}
56

11
— is a relation number with a list {{57, 55}, {114, 11}, {228, 11}, {1, 0}}
57

11
— is a relation number with a list {{58, 55}, {174, -11}, {1, 0}}
58

11
— is a relation number with a list
59
  {{59, 55}, {236, -11}, {295, 11}, {118, 11}, {177, 11}, {1, 0}}

11
— is a relation number with a list {{60, 55}, {1, 0}}
60

11
— is a relation number with a list
61
  {{61, 66}, {305, -11}, {183, 11}, {244, -11}, {122, 11}, {1, 0}}

11
— is a relation number with a list {{62, 66}, {1, 0}}
62

11
— is a relation number with a list {{63, 66}, {1, 0}}
63

11
— is a relation number with a list {{64, 66}, {1, 0}}
64

11
— is a relation number with a list {{65, 66}, {1, 0}}
65

11
— is a relation number with a list {{67, 66}, {1, 0}}
67

11
— is a relation number with a list {{68, 66}, {1, 0}}
68

11
— is a relation number with a list {{69, 66}, {1, 0}}
69

11
— is a relation number with a list {{70, 66}, {1, 0}}
70

```

```

11
— is a relation number with a list
71
  {{71, 66}, {355, 11}, {213, -11}, {284, 11}, {142, 11}, {1, 0}}

11
— is a relation number with a list {{72, 77}, {360, 11}, {1, 0}}
72

11
— is a relation number with a list
73
  {{73, 77}, {292, 11}, {365, 22}, {657, -22}, {219, -11}, {1, 0}}

11
— is a relation number with a list {{74, 77}, {222, 11}, {1, 0}}
74

11
— is a relation number with a list {{75, 77}, {150, 11}, {300, 11}, {1, 0}}
75

11
— is a relation number with a list {{76, 77}, {1, 0}}
76

11
— is a relation number with a list {{78, 77}, {1, 0}}
78

11
— is a relation number with a list
79
  {{79, 77}, {158, 11}, {316, -11}, {237, 11}, {395, 11}, {1, 0}}

11
— is a relation number with a list {{80, 77}, {240, -11}, {1, 0}}
80

11
— is a relation number with a list
81
  {{81, 77}, {324, -11}, {405, -11}, {162, 11}, {1, 0}}

11
— is a relation number with a list
82
  {{82, 77}, {410, -11}, {246, -11}, {164, 11}, {1, 0}}

11
— is a relation number with a list
83
  {{83, 88}, {415, 11}, {249, 11}, {332, 11}, {166, 11}, {1, 0}}

11
— is a relation number with a list {{84, 88}, {1, 0}}
84

11
— is a relation number with a list {{85, 88}, {255, 11}, {170, 11}, {1, 0}}
85

11
— is a relation number with a list {{86, 88}, {1, 0}}
86

11
— is a relation number with a list {{87, 88}, {1, 0}}
87

11
— is a relation number with a list {{89, 88}, {1, 0}}
89

11
— is a relation number with a list {{90, 88}, {1, 0}}
90

11
— is a relation number with a list
91
  {{91, 88}, {273, -11}, {182, 11}, {455, -11}, {364, 11}, {1, 0}}

```

```

11
— is a relation number with a list {{92, 88}, {1, 0}}
92
11
— is a relation number with a list {{93, 88}, {465, -11}, {1, 0}}
93
11
— is a relation number with a list {{94, 99}, {470, -11}, {282, 11}, {188, 11}, {1, 0}}
94
11
— is a relation number with a list {{95, 99}, {380, 11}, {1, 0}}
95
11
— is a relation number with a list {{96, 99}, {1, 0}}
96
11
— is a relation number with a list
97
  {{97, 99}, {194, 11}, {388, -11}, {291, -11}, {485, -22}, {1, 0}}
11
— is a relation number with a list {{98, 99}, {1, 0}}
98
11
— is a relation number with a list {{100, 99}, {1, 0}}
100
11
— is a relation number with a list
101
  {{101, 99}, {202, 11}, {404, 11}, {303, 11}, {505, -11}, {1, 0}}
11
— is a relation number with a list {{102, 99}, {1, 0}}
102
11
— is a relation number with a list
103
  {{103, 99}, {412, -11}, {515, 22}, {927, -11}, {309, -11}, {1, 0}}
11
— is a relation number with a list {{104, 99}, {520, 11}, {312, -11}, {1, 0}}
104
11
— is a relation number with a list {{105, 110}, {1, 0}}
105
11
— is a relation number with a list {{106, 110}, {1, 0}}
106
11
— is a relation number with a list
107
  {{107, 110}, {321, 11}, {214, 11}, {535, 22}, {749, -33}, {1070, 11}, {321, -11}}
11
— is a relation number with a list {{108, 110}, {1, 0}}
108
11
— is a relation number with a list {{109, 110}, {1, 0}}
109
12
— is a relation number with a list {{5, 12}, {35, 24}, {55, -12}, {1, 0}}
5
12
— is a relation number with a list {{7, 12}, {35, -24}, {77, -36}, {35, -12}, {1, 0}}
7
12
— is a relation number with a list {{11, 12}, {1, 0}}
11
12
— is a relation number with a list {{13, 12}, {1, 0}}
13

```

```

12
— is a relation number with a list {{17, 12}, {85, 24}, {187, -12}, {85, 24}}
17

12
— is a relation number with a list {{19, 24}, {95, 24}, {1, 0}}
19

12
— is a relation number with a list {{23, 24}, {1, 0}}
23

12
— is a relation number with a list {{25, 24}, {1, 0}}
25

12
— is a relation number with a list {{29, 24}, {145, -24}, {1, 0}}
29

12
— is a relation number with a list {{31, 36}, {155, 24}, {341, -48}, {155, 12}, {1, 0}}
31

12
— is a relation number with a list {{35, 36}, {1, 0}}
35

12
— is a relation number with a list {{37, 36}, {1, 0}}
37

12
— is a relation number with a list
41
  {{41, 36}, {205, -24}, {451, 60}, {1189, -24}, {451, 60}}

12
— is a relation number with a list {{43, 48}, {215, -24}, {1, 0}}
43

12
— is a relation number with a list {{47, 48}, {1, 0}}
47

12
— is a relation number with a list {{49, 48}, {1, 0}}
49

12
— is a relation number with a list {{53, 48}, {265, 24}, {1, 0}}
53

12
— is a relation number with a list {{55, 60}, {1, 0}}
55

12
— is a relation number with a list {{59, 60}, {1, 0}}
59

12
— is a relation number with a list {{61, 60}, {1, 0}}
61

12
— is a relation number with a list {{65, 60}, {1, 0}}
65

12
— is a relation number with a list {{67, 72}, {335, -24}, {1, 0}}
67

12
— is a relation number with a list {{71, 72}, {1, 0}}
71

12
— is a relation number with a list {{73, 72}, {1, 0}}
73

12
— is a relation number with a list {{77, 72}, {385, 24}, {1, 0}}
77

12
— is a relation number with a list {{79, 84}, {395, 24}, {869, 48}, {395, 12}, {1, 0}}
79

```



```

12
83 — is a relation number with a list {{83, 84}, {1, 0}}

12
85 — is a relation number with a list {{85, 84}, {1, 0}}

12
89 — is a relation number with a list {{89, 84}, {445, -24}, {979, 24}, {445, 24}}

12
91 — is a relation number with a list {{91, 96}, {455, 24}, {1, 0}}

12
95 — is a relation number with a list {{95, 96}, {1, 0}}

12
97 — is a relation number with a list {{97, 96}, {1, 0}}

12
101 — is a relation number with a list {{101, 96}, {505, -24}, {1, 0}}

12
103 — is a relation number with a list
      {{103, 108}, {515, -24}, {1133, 36}, {1751, 36}, {1339, 36}, {721, 12}, {1, 0}}

12
107 — is a relation number with a list {{107, 108}, {1, 0}}

12
109 — is a relation number with a list {{109, 108}, {1, 0}}

12
113 — is a relation number with a list
      {{113, 108}, {565, 24}, {1243, 60}, {1921, -48}, {1, 0}}

12
115 — is a relation number with a list {{115, 120}, {1, 0}}

12
119 — is a relation number with a list {{119, 120}, {1, 0}}

known cases

known cases

13
4 — is a relation number with a list {{4, 13}, {36, 65}, {116, 117}, {1, 0}}

13
5 — is a relation number with a list {{5, 13}, {40, 39}, {1, 0}}

13
6 — is a relation number with a list {{6, 13}, {42, 13}, {1, 0}}

13
7 — is a relation number with a list
      {{7, 13}, {42, -13}, {21, -13}, {35, 26}, {63, -52}, {77, 65}, {84, -13}, {42, -13}}

13
8 — is a relation number with a list {{8, 13}, {20, 13}, {24, -13}, {1, 0}}

13
9 — is a relation number with a list {{9, 13}, {36, -13}, {1, 0}}

13
10 — is a relation number with a list {{10, 13}, {30, -13}, {20, 13}, {30, 13}}

```

```

13
— is a relation number with a list
11
  {{11, 13}, {22, 13}, {44, 13}, {55, 13}, {33, -13}, {66, -13}, {1, 0}}

13
— is a relation number with a list {{12, 13}, {1, 0}}
12

13
— is a relation number with a list {{14, 13}, {1, 0}}
14

13
— is a relation number with a list {{15, 13}, {30, 13}, {60, -13}, {1, 0}}
15

13
— is a relation number with a list {{16, 13}, {48, 13}, {1, 0}}
16

13
— is a relation number with a list {{17, 13}, {68, 13}, {51, -13}, {1, 0}}
17

13
— is a relation number with a list {{18, 13}, {45, -13}, {1, 0}}
18

13
— is a relation number with a list
19
  {{19, 13}, {114, 13}, {57, -13}, {95, 13}, {76, -13}, {38, 13}, {1, 0}}

13
— is a relation number with a list {{20, 26}, {60, 13}, {1, 0}}
20

13
— is a relation number with a list {{21, 26}, {105, -26}, {1, 0}}
21

13
— is a relation number with a list {{22, 26}, {1, 0}}
22

13
— is a relation number with a list {{23, 26}, {69, -13}, {92, 13}, {1, 0}}
23

13
— is a relation number with a list {{24, 26}, {1, 0}}
24

13
— is a relation number with a list {{25, 26}, {1, 0}}
25

13
— is a relation number with a list {{27, 26}, {1, 0}}
27

13
— is a relation number with a list {{28, 26}, {1, 0}}
28

13
— is a relation number with a list {{29, 26}, {87, 13}, {116, -13}, {1, 0}}
29

13
— is a relation number with a list {{30, 26}, {1, 0}}
30

13
— is a relation number with a list {{31, 26}, {155, 26}, {1, 0}}
31

13
— is a relation number with a list {{32, 26}, {96, -13}, {80, -13}, {1, 0}}
32

13
— is a relation number with a list {{33, 39}, {66, 13}, {1, 0}}
33

13
— is a relation number with a list {{34, 39}, {85, -13}, {102, -13}, {1, 0}}
34

```

```

13
35 — is a relation number with a list {{35, 39}, {140, -13}, {105, -13}, {1, 0}}
13
36 — is a relation number with a list {{36, 39}, {1, 0}}
13
37 — is a relation number with a list
    {{37, 39}, {74, 13}, {148, -13}, {185, -26}, {111, 13}, {222, -13}, {1, 0}}
13
38 — is a relation number with a list {{38, 39}, {1, 0}}
13
40 — is a relation number with a list {{40, 39}, {1, 0}}
13
41 — is a relation number with a list
    {{41, 39}, {82, 13}, {164, 13}, {205, -13}, {123, -13}, {246, 13}, {1, 0}}
13
42 — is a relation number with a list {{42, 39}, {1, 0}}
13
43 — is a relation number with a list {{43, 39}, {172, 13}, {129, 13}, {1, 0}}
13
44 — is a relation number with a list {{44, 39}, {110, 13}, {132, 13}, {1, 0}}
13
45 — is a relation number with a list {{45, 39}, {90, 13}, {1, 0}}
13
46 — is a relation number with a list {{46, 52}, {138, 13}, {230, -13}, {92, 13}, {1, 0}}
13
47 — is a relation number with a list {{47, 52}, {235, 26}, {1, 0}}
13
48 — is a relation number with a list {{48, 52}, {1, 0}}
13
49 — is a relation number with a list {{49, 52}, {147, -13}, {196, -13}, {1, 0}}
13
50 — is a relation number with a list {{50, 52}, {1, 0}}
13
51 — is a relation number with a list {{51, 52}, {1, 0}}
13
53 — is a relation number with a list {{53, 52}, {1, 0}}
13
54 — is a relation number with a list {{54, 52}, {1, 0}}
13
55 — is a relation number with a list {{55, 52}, {165, 13}, {220, 13}, {1, 0}}
13
56 — is a relation number with a list {{56, 52}, {1, 0}}
13
57 — is a relation number with a list {{57, 52}, {285, -26}, {1, 0}}
13
58 — is a relation number with a list {{58, 52}, {174, -13}, {145, 13}, {1, 0}}

```

```

13
— is a relation number with a list
59
  {{59, 65}, {354, -13}, {177, 13}, {295, 13}, {236, 13}, {118, 13}, {1, 0}}

13
— is a relation number with a list {{60, 65}, {1, 0}}
60

13
— is a relation number with a list {{61, 65}, {244, -13}, {183, 13}, {1, 0}}
61

13
— is a relation number with a list {{62, 65}, {186, -13}, {124, 13}, {186, -13}}
62

13
— is a relation number with a list {{63, 65}, {126, 13}, {252, 13}, {315, -26}, {1, 0}}
63

13
— is a relation number with a list {{64, 65}, {1, 0}}
64

13
— is a relation number with a list {{66, 65}, {1, 0}}
66

13
— is a relation number with a list
67
  {{67, 65}, {134, 13}, {268, -13}, {335, 26}, {201, 13}, {402, 13}, {1, 0}}

13
— is a relation number with a list {{68, 65}, {204, 13}, {1, 0}}
68

13
— is a relation number with a list {{69, 65}, {276, 13}, {1, 0}}
69

13
— is a relation number with a list {{70, 65}, {1, 0}}
70

13
— is a relation number with a list
71
  {{71, 65}, {426, 13}, {213, 13}, {355, 13}, {284, -13}, {142, 13}, {1, 0}}

13
— is a relation number with a list {{72, 78}, {1, 0}}
72

13
— is a relation number with a list {{73, 78}, {365, 26}, {1, 0}}
73

13
— is a relation number with a list {{74, 78}, {1, 0}}
74

13
— is a relation number with a list {{75, 78}, {1, 0}}
75

13
— is a relation number with a list {{76, 78}, {1, 0}}
76

13
— is a relation number with a list {{77, 78}, {1, 0}}
77

13
— is a relation number with a list {{79, 78}, {1, 0}}
79

13
— is a relation number with a list {{80, 78}, {1, 0}}
80

13
— is a relation number with a list {{81, 78}, {1, 0}}
81

```

```

13
— is a relation number with a list {{82, 78}, {1, 0}}
82
13
— is a relation number with a list {{83, 78}, {415, -26}, {1, 0}}
83
13
— is a relation number with a list {{84, 78}, {1, 0}}
84
13
— is a relation number with a list {{85, 91}, {510, -13}, {255, -13}, {1, 0}}
85
13
— is a relation number with a list {{86, 91}, {215, -13}, {258, 13}, {1, 0}}
86
13
— is a relation number with a list {{87, 91}, {348, -13}, {1, 0}}
87
13
— is a relation number with a list {{88, 91}, {264, -13}, {1, 0}}
88
13
— is a relation number with a list
89
  {{89, 91}, {178, 13}, {356, -13}, {445, 13}, {267, -13}, {534, -13}, {1, 0}}
13
— is a relation number with a list {{90, 91}, {1, 0}}
90
13
— is a relation number with a list {{92, 91}, {1, 0}}
92
13
— is a relation number with a list {{93, 91}, {186, 13}, {372, 13}, {465, 26}, {1, 0}}
93
13
— is a relation number with a list {{94, 91}, {282, 13}, {188, 13}, {282, -13}}
94
13
— is a relation number with a list {{95, 91}, {380, 13}, {285, -13}, {1, 0}}
95
13
— is a relation number with a list {{96, 91}, {240, 13}, {1, 0}}
96
13
— is a relation number with a list
97
  {{97, 91}, {582, 13}, {291, -13}, {485, -26}, {873, -52}, {1067, 39},
  {1358, -39}, {679, -39}, {1552, -39}, {776, 39}, {388, 13}, {194, 13}, {1, 0}}
13
— is a relation number with a list {{98, 104}, {294, 13}, {245, 13}, {1, 0}}
98
13
— is a relation number with a list {{99, 104}, {495, -26}, {1, 0}}
99
13
— is a relation number with a list {{100, 104}, {1, 0}}
100
13
— is a relation number with a list {{101, 104}, {303, -13}, {404, -13}, {1, 0}}
101
13
— is a relation number with a list {{102, 104}, {1, 0}}
102
13
— is a relation number with a list {{103, 104}, {1, 0}}
103

```

```

13
105 is a relation number with a list {{105, 104}, {1, 0}}
13
106 is a relation number with a list {{106, 104}, {1, 0}}
13
107 is a relation number with a list {{107, 104}, {321, 13}, {428, 13}, {1, 0}}
13
108 is a relation number with a list {{108, 104}, {1, 0}}
13
109 is a relation number with a list {{109, 104}, {545, 26}, {1, 0}}
13
110 is a relation number with a list {{110, 104}, {330, -13}, {1, 0}}
13
111 is a relation number with a list {{111, 117}, {222, 13}, {1, 0}}
13
112 is a relation number with a list {{112, 117}, {280, 13}, {336, 13}, {1, 0}}
13
113 is a relation number with a list {{113, 117}, {452, -13}, {339, -13}, {1, 0}}
13
114 is a relation number with a list {{114, 117}, {1, 0}}
13
115 is a relation number with a list {{115, 117}, {230, 13}, {460, 13}, {1, 0}}
13
116 is a relation number with a list {{116, 117}, {1, 0}}
13
118 is a relation number with a list {{118, 117}, {1, 0}}
13
119 is a relation number with a list
{{119, 117}, {238, 13}, {476, -13}, {595, -13}, {357, -13}, {714, 13}, {1, 0}}
13
120 is a relation number with a list {{120, 117}, {1, 0}}
13
121 is a relation number with a list {{121, 117}, {484, 13}, {363, 13}, {1, 0}}
13
122 is a relation number with a list {{122, 117}, {305, -13}, {366, -13}, {1, 0}}
13
123 is a relation number with a list {{123, 117}, {246, 13}, {1, 0}}
13
124 is a relation number with a list {{124, 130}, {372, 13}, {620, 13}, {1, 0}}
13
125 is a relation number with a list {{125, 130}, {1, 0}}
13
126 is a relation number with a list {{126, 130}, {1, 0}}
13
127 is a relation number with a list {{127, 130}, {381, -13}, {508, 13}, {1, 0}}

```

$\frac{13}{128}$  is a relation number with a list  $\{\{128, 130\}, \{1, 0\}\}$

$\frac{13}{129}$  is a relation number with a list  $\{\{129, 130\}, \{1, 0\}\}$

known cases

$\frac{14}{5}$  is a relation number with a list  $\{\{5, 14\}, \{45, 56\}, \{55, 28\}, \{1, 0\}\}$

$\frac{14}{9}$  is a relation number with a list  $\{\{9, 14\}, \{45, 14\}, \{1, 0\}\}$

$\frac{14}{11}$  is a relation number with a list  $\{\{11, 14\}, \{33, 14\}, \{55, 14\}, \{1, 0\}\}$

$\frac{14}{13}$  is a relation number with a list  $\{\{13, 14\}, \{1, 0\}\}$

$\frac{14}{15}$  is a relation number with a list  $\{\{15, 14\}, \{1, 0\}\}$

$\frac{14}{17}$  is a relation number with a list  $\{\{17, 14\}, \{51, -14\}, \{85, 28\}, \{1, 0\}\}$

$\frac{14}{19}$  is a relation number with a list  $\{\{19, 14\}, \{95, -14\}, \{57, 14\}, \{1, 0\}\}$

$\frac{14}{23}$  is a relation number with a list  $\{\{23, 28\}, \{115, -14\}, \{69, 14\}, \{1, 0\}\}$

$\frac{14}{25}$  is a relation number with a list  $\{\{25, 28\}, \{75, 14\}, \{1, 0\}\}$

$\frac{14}{27}$  is a relation number with a list  $\{\{27, 28\}, \{1, 0\}\}$

$\frac{14}{29}$  is a relation number with a list  $\{\{29, 28\}, \{1, 0\}\}$

$\frac{14}{31}$  is a relation number with a list  $\{\{31, 28\}, \{93, -14\}, \{155, 14\}, \{1, 0\}\}$

$\frac{14}{33}$  is a relation number with a list  $\{\{33, 28\}, \{165, 14\}, \{1, 0\}\}$

$\frac{14}{37}$  is a relation number with a list  $\{\{37, 42\}, \{185, -14\}, \{111, -14\}, \{1, 0\}\}$

$\frac{14}{39}$  is a relation number with a list  $\{\{39, 42\}, \{1, 0\}\}$

$\frac{14}{41}$  is a relation number with a list  $\{\{41, 42\}, \{1, 0\}\}$

$\frac{14}{43}$  is a relation number with a list  $\{\{43, 42\}, \{1, 0\}\}$

$\frac{14}{45}$  is a relation number with a list  $\{\{45, 42\}, \{1, 0\}\}$

$\frac{14}{47}$  is a relation number with a list  $\{\{47, 42\}, \{235, 14\}, \{141, 14\}, \{1, 0\}\}$

$\frac{14}{51}$  is a relation number with a list  $\{\{51, 56\}, \{255, 14\}, \{1, 0\}\}$

```

14
— is a relation number with a list {{53, 56}, {159, 14}, {265, -28}, {689, -28},
53 {583, -56}, {1219, -70}, {1537, -56}, {1325, -168}, {1007, 126}, {1, 0}}

14
— is a relation number with a list {{55, 56}, {1, 0}}
55

14
— is a relation number with a list {{57, 56}, {1, 0}}
57

14
— is a relation number with a list {{59, 56}, {177, -14}, {295, -14}, {1, 0}}
59

14
— is a relation number with a list {{61, 56}, {305, -14}, {183, 14}, {1, 0}}
61

14
— is a relation number with a list {{65, 70}, {1, 0}}
65

14
— is a relation number with a list {{67, 70}, {201, 14}, {335, 28}, {1, 0}}
67

14
— is a relation number with a list {{69, 70}, {1, 0}}
69

14
— is a relation number with a list {{71, 70}, {1, 0}}
71

14
— is a relation number with a list {{73, 70}, {219, -14}, {365, -28}, {1, 0}}
73

14
— is a relation number with a list {{75, 70}, {1, 0}}
75

14
— is a relation number with a list {{79, 84}, {395, 14}, {237, 14}, {1, 0}}
79

14
— is a relation number with a list {{81, 84}, {1, 0}}
81

14
— is a relation number with a list {{83, 84}, {1, 0}}
83

14
— is a relation number with a list {{85, 84}, {1, 0}}
85

14
— is a relation number with a list {{87, 84}, {1, 0}}
87

14
— is a relation number with a list {{89, 84}, {445, -14}, {267, -14}, {1, 0}}
89

14
— is a relation number with a list {{93, 98}, {465, -14}, {1, 0}}
93

14
— is a relation number with a list {{95, 98}, {285, 14}, {1, 0}}
95

14
— is a relation number with a list {{97, 98}, {1, 0}}
97

14
— is a relation number with a list {{99, 98}, {1, 0}}
99

14
— is a relation number with a list {{101, 98}, {303, -14}, {505, 14}, {1, 0}}
101

```



```

14
103 is a relation number with a list {{103, 98}, {515, 14}, {309, -14}, {1, 0}}

14
107 is a relation number with a list {{107, 112}, {535, -14}, {321, 14}, {1, 0}}

14
109 is a relation number with a list {{109, 112}, {327, 14}, {545, -14}, {1, 0}}

14
111 is a relation number with a list {{111, 112}, {1, 0}}

14
113 is a relation number with a list {{113, 112}, {1, 0}}

14
115 is a relation number with a list {{115, 112}, {345, -14}, {1, 0}}

14
117 is a relation number with a list {{117, 112}, {585, 14}, {1, 0}}

14
121 is a relation number with a list {{121, 126}, {605, 14}, {363, 14}, {1, 0}}

14
123 is a relation number with a list {{123, 126}, {1, 0}}

14
125 is a relation number with a list {{125, 126}, {1, 0}}

14
127 is a relation number with a list {{127, 126}, {1, 0}}

14
129 is a relation number with a list {{129, 126}, {1, 0}}

14
131 is a relation number with a list {{131, 126}, {655, -14}, {393, -14}, {1, 0}}

14
135 is a relation number with a list {{135, 140}, {1, 0}}

14
137 is a relation number with a list
    {{137, 140}, {411, 14}, {685, 28}, {1781, 14}, {411, -14}}

14
139 is a relation number with a list {{139, 140}, {1, 0}}

known cases

15
4 is a relation number with a list
    {{4, 15}, {44, 105}, {244, 495}, {1004, 1785}, {3124, 4575},
    {5804, 3465}, {2252, 1515}, {2948, -4995}, {8188, -10725}, {10148, 4845},
    {916, -615}, {1204, 2055}, {3404, 4545}, {4564, -1065}, {304, 75}, {1, 0}}

15
7 is a relation number with a list {{7, 15}, {56, 15}, {28, 15}, {14, 15}, {1, 0}}

15
8 is a relation number with a list {{8, 15}, {56, -15}, {1, 0}}

15
11 is a relation number with a list {{11, 15}, {44, 15}, {1, 0}}

```

```

15
13 — is a relation number with a list {{13, 15}, {26, 15}, {52, -15}, {91, 15}, {1, 0}}
15
14 — is a relation number with a list {{14, 15}, {1, 0}}
15
16 — is a relation number with a list {{16, 15}, {1, 0}}
15
17 — is a relation number with a list
    {{17, 15}, {34, 15}, {68, 15}, {119, -45}, {272, 45}, {34, 15}}
15
19 — is a relation number with a list {{19, 15}, {76, -15}, {1, 0}}
15
22 — is a relation number with a list {{22, 15}, {154, 15}, {44, 15}, {1, 0}}
15
23 — is a relation number with a list
    {{23, 30}, {161, 45}, {437, 105}, {391, 120}, {713, -30}, {161, -45}}
15
26 — is a relation number with a list {{26, 30}, {1, 0}}
15
28 — is a relation number with a list {{28, 30}, {1, 0}}
15
29 — is a relation number with a list {{29, 30}, {1, 0}}
15
31 — is a relation number with a list {{31, 30}, {1, 0}}
15
32 — is a relation number with a list {{32, 30}, {1, 0}}
15
34 — is a relation number with a list {{34, 30}, {1, 0}}
15
37 — is a relation number with a list {{37, 30}, {259, -45}, {407, 15}, {74, 15}, {1, 0}}
15
38 — is a relation number with a list {{38, 45}, {133, -15}, {1, 0}}
15
41 — is a relation number with a list {{41, 45}, {164, 15}, {1, 0}}
15
43 — is a relation number with a list {{43, 45}, {86, 15}, {172, 15}, {301, 15}, {1, 0}}
15
44 — is a relation number with a list {{44, 45}, {1, 0}}
15
46 — is a relation number with a list {{46, 45}, {1, 0}}
15
47 — is a relation number with a list {{47, 45}, {94, 15}, {188, -15}, {329, -30}, {1, 0}}
15
49 — is a relation number with a list {{49, 45}, {196, -15}, {1, 0}}
15
52 — is a relation number with a list {{52, 45}, {182, 15}, {1, 0}}

```

```

15
— is a relation number with a list {{53, 60}, {371, -30},
53
  {583, 60}, {901, -120}, {3127, 165}, {424, 15}, {212, 15}, {106, 15}, {1, 0}}

15
— is a relation number with a list {{56, 60}, {1, 0}}
56

15
— is a relation number with a list {{58, 60}, {1, 0}}
58

15
— is a relation number with a list {{59, 60}, {1, 0}}
59

15
— is a relation number with a list {{61, 60}, {1, 0}}
61

15
— is a relation number with a list {{62, 60}, {1, 0}}
62

15
— is a relation number with a list {{64, 60}, {1, 0}}
64

15
— is a relation number with a list {{67, 60}, {469, 30}, {737, -30},
67
  {871, 60}, {1943, -105}, {3484, 15}, {268, -15}, {134, 15}, {1, 0}}

15
— is a relation number with a list {{68, 75}, {476, 45}, {1292, 75}, {1, 0}}
68

15
— is a relation number with a list {{71, 75}, {284, 15}, {1, 0}}
71

15
— is a relation number with a list
73
  {{73, 75}, {146, 15}, {292, -15}, {511, -45}, {1168, 75}, {2336, -195}, {292, 15}}

15
— is a relation number with a list {{74, 75}, {1, 0}}
74

15
— is a relation number with a list {{76, 75}, {1, 0}}
76

15
— is a relation number with a list {{77, 75}, {154, 15}, {308, 15}, {1, 0}}
77

15
— is a relation number with a list {{79, 75}, {316, -15}, {1, 0}}
79

15
— is a relation number with a list {{82, 75}, {574, -45}, {451, 30}, {1, 0}}
82

15
— is a relation number with a list
83
  {{83, 90}, {581, -15}, {332, -15}, {166, 15}, {1, 0}}

15
— is a relation number with a list {{86, 90}, {1, 0}}
86

15
— is a relation number with a list {{88, 90}, {1, 0}}
88

15
— is a relation number with a list {{89, 90}, {1, 0}}
89

15
— is a relation number with a list {{91, 90}, {1, 0}}
91

```

```

15
— is a relation number with a list {{92, 90}, {1, 0}}
92
15
— is a relation number with a list {{94, 90}, {1, 0}}
94
15
— is a relation number with a list {{97, 90}, {679, 15}, {388, 15}, {194, 15}, {1, 0}}
97
15
— is a relation number with a list {{98, 105}, {1, 0}}
98
15
— is a relation number with a list {{101, 105}, {404, 15}, {1, 0}}
101
15
— is a relation number with a list
103
  {{103, 105}, {206, 15}, {412, 15}, {721, -30}, {1, 0}}
15
— is a relation number with a list {{104, 105}, {1, 0}}
104
15
— is a relation number with a list {{106, 105}, {1, 0}}
106
15
— is a relation number with a list
107
  {{107, 105}, {214, 15}, {428, -15}, {749, 30}, {1, 0}}
15
— is a relation number with a list {{109, 105}, {436, -15}, {1, 0}}
109
15
— is a relation number with a list {{112, 105}, {1, 0}}
112
15
— is a relation number with a list
113
  {{113, 120}, {791, -15}, {452, 15}, {226, 15}, {1, 0}}
15
— is a relation number with a list {{116, 120}, {1, 0}}
116
15
— is a relation number with a list {{118, 120}, {1, 0}}
118
15
— is a relation number with a list {{119, 120}, {1, 0}}
119
15
— is a relation number with a list {{121, 120}, {1, 0}}
121
15
— is a relation number with a list {{122, 120}, {1, 0}}
122
15
— is a relation number with a list {{124, 120}, {1, 0}}
124
15
— is a relation number with a list
127
  {{127, 120}, {889, 15}, {508, -15}, {254, 15}, {1, 0}}
15
— is a relation number with a list {{128, 135}, {896, 45}, {1, 0}}
128
15
— is a relation number with a list {{131, 135}, {524, 15}, {1, 0}}
131

```

```

15
133 is a relation number with a list {{133, 135}, {266, 15}, {532, -15}, {1, 0}}

15
134 is a relation number with a list {{134, 135}, {1, 0}}

15
136 is a relation number with a list {{136, 135}, {1, 0}}

15
137 is a relation number with a list {{137, 135}, {274, 15}, {548, 15},
    {959, 45}, {1918, 75}, {4384, -195}, {12878, 75}, {3014, -45}, {1, 0}}

15
139 is a relation number with a list {{139, 135}, {556, -15}, {1, 0}}

15
142 is a relation number with a list {{142, 135}, {994, -45}, {284, 15}, {1, 0}}

15
143 is a relation number with a list {{143, 150}, {1001, -30}, {1, 0}}

15
146 is a relation number with a list {{146, 150}, {1, 0}}

15
148 is a relation number with a list {{148, 150}, {1, 0}}

15
149 is a relation number with a list {{149, 150}, {1, 0}}

known cases

16
5 is a relation number with a list {{5, 16}, {55, 96}, {205, 176}, {145, -48}, {1, 0}}

16
7 is a relation number with a list {{7, 16}, {63, 32}, {1, 0}}

16
9 is a relation number with a list {{9, 16}, {63, -32}, {1, 0}}

16
11 is a relation number with a list
    {{11, 16}, {55, -16}, {77, 48}, {209, 80}, {341, 112}, {55, 32}, {99, -64},
    {319, -224}, {1045, 576}, {1177, 512}, {1683, 736}, {2321, 1344}, {4037, 2832},
    {13255, -7408}, {17171, 6560}, {27599, 8128}, {35365, -13472}, {55561, -13440},
    {19811, -3760}, {11121, 7168}, {35365, 24032}, {124663, 83024},
    {455235, -251104}, {516703, -244128}, {312917, 45504}, {61721, 38112},
    {159533, 44864}, {219153, 144032}, {758021, -481776}, {2260841, -1277456},
    {3234781, -63392}, {19679, -10336}, {10923, 2480}, {11033, -4816}, {15411, -8144},
    {9647, 5392}, {12507, -4736}, {18711, -2336}, {253, 64}, {33, 16}, {1, 0}}

16
13 is a relation number with a list {{13, 16}, {39, -16}, {91, 16}, {65, 32}, {1, 0}}

16
15 is a relation number with a list {{15, 16}, {1, 0}}

16
17 is a relation number with a list {{17, 16}, {1, 0}}

16
19 is a relation number with a list {{19, 16}, {57, 16}, {133, 32}, {95, -32}, {1, 0}}

```

```

16
— is a relation number with a list {{21, 16}, {105, 16}, {1, 0}}
21
16
— is a relation number with a list {{23, 16}, {161, 32}, {1, 0}}
23
16
— is a relation number with a list {{25, 32}, {175, -16}, {1, 0}}
25
16
— is a relation number with a list {{27, 32}, {135, 16}, {189, -16}, {1, 0}}
27
16
— is a relation number with a list
29
  {{29, 32}, {87, -16}, {203, -16}, {145, -16}, {1, 0}}
16
— is a relation number with a list {{31, 32}, {1, 0}}
31
16
— is a relation number with a list {{33, 32}, {1, 0}}
33
16
— is a relation number with a list {{35, 32}, {105, 16}, {1, 0}}
35
16
— is a relation number with a list
37
  {{37, 32}, {185, -16}, {259, 32}, {111, -16}, {1, 0}}
16
— is a relation number with a list {{39, 32}, {273, 16}, {1, 0}}
39
16
— is a relation number with a list {{41, 48}, {287, 48}, {1, 0}}
41
16
— is a relation number with a list {{43, 48}, {215, 16}, {301, 16}, {129, -16}, {1, 0}}
43
16
— is a relation number with a list {{45, 48}, {1, 0}}
45
16
— is a relation number with a list {{47, 48}, {1, 0}}
47
16
— is a relation number with a list {{49, 48}, {1, 0}}
49
16
— is a relation number with a list {{51, 48}, {1, 0}}
51
16
— is a relation number with a list
53
  {{53, 48}, {265, -16}, {371, -48}, {689, 48}, {901, 96}, {1961, -240}, {2173, -256},
  {6625, 432}, {7685, -304}, {4505, 208}, {3763, 336}, {3551, -416}, {10229, 432},
  {7367, -656}, {8003, -944}, {23903, 480}, {5141, -608}, {14681, -1200},
  {14893, -656}, {10335, 448}, {1643, -64}, {1113, 32}, {371, -16}, {159, 16}, {1, 0}}
16
— is a relation number with a list {{55, 48}, {385, -48}, {1, 0}}
55
16
— is a relation number with a list {{57, 64}, {133, 16}, {285, 32}, {1, 0}}
57

```

```

16
59 is a relation number with a list {{59, 64}, {295, -16}, {413, -48},
    {1121, 96}, {1829, -208}, {2537, -112}, {2301, -256}, {177, -16}, {1, 0}}

16
61 is a relation number with a list {{61, 64}, {183, -16}, {427, 32}, {671, 16}, {1, 0}}

16
63 is a relation number with a list {{63, 64}, {1, 0}}

16
65 is a relation number with a list {{65, 64}, {1, 0}}

16
67 is a relation number with a list
    {{67, 64}, {201, 16}, {469, 48}, {737, -48}, {1139, 48}, {871, -96}, {469, -48}}

16
69 is a relation number with a list {{69, 64}, {345, 16}, {483, 16}, {1, 0}}

16
71 is a relation number with a list {{71, 64}, {497, -48}, {1207, 128},
    {3905, 288}, {9017, -128}, {4047, 32}, {1065, 112}, {3905, -32}, {1, 0}}

16
73 is a relation number with a list {{73, 80}, {511, -16}, {1, 0}}

16
75 is a relation number with a list {{75, 80}, {1, 0}}

16
77 is a relation number with a list {{77, 80}, {231, -16}, {1, 0}}

16
79 is a relation number with a list {{79, 80}, {1, 0}}

16
81 is a relation number with a list {{81, 80}, {1, 0}}

16
83 is a relation number with a list {{83, 80}, {249, 16}, {581, 16}, {415, -32}, {1, 0}}

16
85 is a relation number with a list {{85, 80}, {1, 0}}

16
87 is a relation number with a list {{87, 80}, {609, 16}, {1, 0}}

16
89 is a relation number with a list
    {{89, 96}, {623, -32}, {1335, 32}, {801, 32}, {1, 0}}

16
91 is a relation number with a list {{91, 96}, {455, -16}, {1, 0}}

16
93 is a relation number with a list {{93, 96}, {1, 0}}

16
95 is a relation number with a list {{95, 96}, {1, 0}}

16
97 is a relation number with a list {{97, 96}, {1, 0}}

16
99 is a relation number with a list {{99, 96}, {1, 0}}

```

```

16
101 is a relation number with a list
    {{101, 96}, {505, 16}, {707, -48}, {1313, 64}, {3131, -16}, {505, 16}}

16
103 is a relation number with a list
    {{103, 96}, {721, 32}, {1545, 64}, {927, -32}, {1, 0}}

16
105 is a relation number with a list {{105, 112}, {1, 0}}

16
107 is a relation number with a list {{107, 112}, {535, 16}, {749, 32},
    {1391, 96}, {5029, -256}, {9737, -272}, {5885, 64}, {321, 16}, {1, 0}}

16
109 is a relation number with a list
    {{109, 112}, {327, -16}, {763, 48}, {545, -32}, {1, 0}}

16
111 is a relation number with a list {{111, 112}, {1, 0}}

16
113 is a relation number with a list {{113, 112}, {1, 0}}

16
115 is a relation number with a list
    {{115, 112}, {345, 16}, {805, -48}, {1265, 64}, {345, 16}}

16
117 is a relation number with a list {{117, 112}, {585, -16}, {819, -32}, {1, 0}}

16
119 is a relation number with a list {{119, 112}, {1, 0}}

16
121 is a relation number with a list
    {{121, 128}, {847, -32}, {1815, -32}, {1089, -16}, {1, 0}}

16
123 is a relation number with a list {{123, 128}, {615, 16}, {287, -16}, {1, 0}}

16
125 is a relation number with a list {{125, 128}, {375, -16}, {875, 16}, {1, 0}}

16
127 is a relation number with a list {{127, 128}, {1, 0}}

16
129 is a relation number with a list {{129, 128}, {1, 0}}

16
131 is a relation number with a list
    {{131, 128}, {393, 16}, {917, 32}, {1441, 32}, {1, 0}}

16
133 is a relation number with a list {{133, 128}, {665, -16}, {1, 0}}

16
135 is a relation number with a list {{135, 128}, {945, 32}, {1, 0}}

16
137 is a relation number with a list {{137, 144}, {959, -16}, {1, 0}}

```



```

16
139 is a relation number with a list
    {{139, 144}, {695, -16}, {973, 16}, {417, -16}, {1, 0}}

16
141 is a relation number with a list {{141, 144}, {1, 0}}

16
143 is a relation number with a list {{143, 144}, {1, 0}}

16
145 is a relation number with a list {{145, 144}, {1, 0}}

16
147 is a relation number with a list {{147, 144}, {1, 0}}

16
149 is a relation number with a list
    {{149, 144}, {745, 16}, {1043, -32}, {1937, -16}, {1, 0}}

16
151 is a relation number with a list {{151, 144}, {1057, 16}, {1, 0}}

16
153 is a relation number with a list {{153, 160}, {357, 16}, {765, -32}, {1, 0}}

16
155 is a relation number with a list {{155, 160}, {1, 0}}

16
157 is a relation number with a list
    {{157, 160}, {471, -16}, {1099, -48}, {785, 16}, {1, 0}}

16
159 is a relation number with a list {{159, 160}, {1, 0}}

known cases

known cases

known cases

17
5 is a relation number with a list {{5, 17}, {60, 119}, {295, 408},
    {565, -119}, {30, 17}, {20, -17}, {15, 17}, {10, 17}, {35, 34}, {1, 0}}

17
6 is a relation number with a list {{6, 17}, {66, 85}, {57, 68}, {33, -17}, {1, 0}}

17
7 is a relation number with a list
    {{7, 17}, {70, 51}, {133, 34}, {21, 17}, {28, -17}, {42, 17}, {56, -17}, {35, -34}, {1, 0}}

17
8 is a relation number with a list {{8, 17}, {72, 17}, {1, 0}}

17
9 is a relation number with a list {{9, 17}, {72, -17}, {36, -17}, {18, 17}, {1, 0}}

17
10 is a relation number with a list
    {{10, 17}, {70, -51}, {95, 68}, {270, 221}, {490, -289}, {440, -51}, {95, -68}}

```

```

17
11 — is a relation number with a list {{11, 17}, {66, 17},
    {22, 17}, {55, 17}, {44, -17}, {77, -51}, {275, 136}, {33, 17}, {1, 0}}

17
12 — is a relation number with a list {{12, 17}, {30, -17}, {1, 0}}

17
13 — is a relation number with a list {{13, 17}, {52, -17}, {1, 0}}

17
14 — is a relation number with a list {{14, 17}, {42, 17}, {56, -17}, {70, 17}, {1, 0}}

17
15 — is a relation number with a list {{15, 17}, {30, 17}, {60, 17}, {120, 17}, {1, 0}}

17
16 — is a relation number with a list {{16, 17}, {1, 0}}

17
18 — is a relation number with a list {{18, 17}, {1, 0}}

17
19 — is a relation number with a list {{19, 17}, {38, 17}, {76, -17}, {152, -51}, {1, 0}}

17
20 — is a relation number with a list {{20, 17}, {60, -17}, {40, 17}, {60, 17}}

17
21 — is a relation number with a list {{21, 17}, {84, 17}, {1, 0}}

17
22 — is a relation number with a list {{22, 17}, {55, 17}, {44, 17}, {154, -17}, {1, 0}}

17
23 — is a relation number with a list {{23, 17}, {138, -17},
    {46, 17}, {115, 34}, {299, -102}, {161, -34}, {207, 17}, {69, -17}, {1, 0}}

17
24 — is a relation number with a list {{24, 17}, {56, 17}, {120, -17}, {1, 0}}

17
25 — is a relation number with a list {{25, 17}, {200, 17}, {100, -17}, {50, 17}, {1, 0}}

17
26 — is a relation number with a list {{26, 34}, {52, 17}, {1, 0}}

17
27 — is a relation number with a list {{27, 34}, {189, 34}, {135, 34}, {1, 0}}

17
28 — is a relation number with a list {{28, 34}, {84, -17}, {1, 0}}

17
29 — is a relation number with a list {{29, 34}, {145, 34},
    {261, 68}, {319, 85}, {609, 34}, {87, -17}, {58, 17}, {203, 17}, {1, 0}}

17
30 — is a relation number with a list {{30, 34}, {1, 0}}

17
31 — is a relation number with a list {{31, 34}, {93, 17},
    {248, -17}, {217, 51}, {403, 34}, {155, -34}, {465, 34}, {341, 68}, {1, 0}}

17
32 — is a relation number with a list {{32, 34}, {1, 0}}

```

```

17
33 — is a relation number with a list {{33, 34}, {1, 0}}

17
35 — is a relation number with a list {{35, 34}, {1, 0}}

17
36 — is a relation number with a list {{36, 34}, {1, 0}}

17
37 — is a relation number with a list {{37, 34}, {111, -17},
    {296, -51}, {370, 17}, {148, -17}, {185, 34}, {555, -17}, {222, 17}, {1, 0}}

17
38 — is a relation number with a list {{38, 34}, {1, 0}}

17
39 — is a relation number with a list
    {{39, 34}, {195, -34}, {117, -17}, {78, 17}, {91, 17}, {78, 17}}

17
40 — is a relation number with a list {{40, 34}, {120, 17}, {1, 0}}

17
41 — is a relation number with a list {{41, 34}, {287, -34}, {615, -119},
    {820, -119}, {533, 17}, {246, -17}, {328, -17}, {205, -17}, {1, 0}}

17
42 — is a relation number with a list {{42, 34}, {84, 17}, {1, 0}}

17
43 — is a relation number with a list {{43, 51}, {344, -17}, {172, 17}, {86, 17}, {1, 0}}

17
44 — is a relation number with a list {{44, 51}, {308, 17}, {1, 0}}

17
45 — is a relation number with a list {{45, 51}, {90, 17}, {1, 0}}

17
46 — is a relation number with a list
    {{46, 51}, {115, 17}, {92, 17}, {322, -51}, {368, 51}, {506, -85}, {92, 17}}

17
47 — is a relation number with a list {{47, 51}, {188, -17}, {1, 0}}

17
48 — is a relation number with a list {{48, 51}, {1, 0}}

17
49 — is a relation number with a list {{49, 51}, {98, 17}, {196, -17}, {392, 17}, {1, 0}}

17
50 — is a relation number with a list {{50, 51}, {1, 0}}

17
52 — is a relation number with a list {{52, 51}, {1, 0}}

17
53 — is a relation number with a list
    {{53, 51}, {106, 17}, {212, 17}, {424, -51}, {848, 17}, {106, 17}}

17
54 — is a relation number with a list {{54, 51}, {1, 0}}

```

```

17
— is a relation number with a list {{55, 51}, {220, 17}, {1, 0}}
55
17
— is a relation number with a list {{56, 51}, {140, -17}, {1, 0}}
56
17
— is a relation number with a list
57
  {{57, 51}, {114, 17}, {285, -34}, {247, 17}, {456, -17}, {1, 0}}
17
— is a relation number with a list {{58, 51}, {406, -17}, {1, 0}}
58
17
— is a relation number with a list {{59, 51}, {472, 17}, {236, 17}, {118, 17}, {1, 0}}
59
17
— is a relation number with a list {{60, 68}, {1, 0}}
60
17
— is a relation number with a list {{61, 68}, {427, 17}, {122, 17},
61
  {183, 17}, {244, -17}, {366, -17}, {488, -51}, {1342, 119}, {2013, -34},
  {427, -51}, {1159, 119}, {1891, 119}, {793, 34}, {671, 17}, {488, -51}}
17
— is a relation number with a list {{62, 68}, {186, -17}, {1, 0}}
62
17
— is a relation number with a list {{63, 68}, {315, -34}, {1, 0}}
63
17
— is a relation number with a list {{64, 68}, {1, 0}}
64
17
— is a relation number with a list {{65, 68}, {195, 17}, {520, 17}, {455, -34}, {1, 0}}
65
17
— is a relation number with a list {{66, 68}, {1, 0}}
66
17
— is a relation number with a list {{67, 68}, {1, 0}}
67
17
— is a relation number with a list {{69, 68}, {1, 0}}
69
17
— is a relation number with a list {{70, 68}, {1, 0}}
70
17
— is a relation number with a list {{71, 68}, {213, -17},
71
  {568, -17}, {497, -17}, {284, 17}, {355, -17}, {142, 17}, {426, -17}, {1, 0}}
17
— is a relation number with a list {{72, 68}, {1, 0}}
72
17
— is a relation number with a list {{73, 68}, {365, 34}, {657, -34},
73
  {803, -51}, {949, -34}, {219, -17}, {146, 17}, {511, -51}, {1, 0}}
17
— is a relation number with a list {{74, 68}, {222, 17}, {1, 0}}
74
17
— is a relation number with a list {{75, 68}, {525, -17}, {150, 17}, {1, 0}}
75

```

```

17
— is a relation number with a list {{76, 68}, {1, 0}}
76
17
— is a relation number with a list
77
  {{77, 85}, {616, -17}, {308, -17}, {154, 17}, {1, 0}}
17
— is a relation number with a list {{78, 85}, {273, 17}, {1, 0}}
78
17
— is a relation number with a list {{79, 85}, {474, 17},
79
  {158, 17}, {395, -17}, {316, 17}, {553, -34}, {711, 68}, {2449, 102}, {1, 0}}
17
— is a relation number with a list {{80, 85}, {1, 0}}
80
17
— is a relation number with a list {{81, 85}, {324, -17}, {1, 0}}
81
17
— is a relation number with a list {{82, 85}, {246, 17}, {328, 17}, {205, 17}, {1, 0}}
82
17
— is a relation number with a list {{83, 85}, {166, 17}, {332, 17}, {664, -51}, {1, 0}}
83
17
— is a relation number with a list {{84, 85}, {1, 0}}
84
17
— is a relation number with a list {{86, 85}, {1, 0}}
86
17
— is a relation number with a list {{87, 85}, {174, 17}, {348, -17}, {696, 17}, {1, 0}}
87
17
— is a relation number with a list {{88, 85}, {264, -17}, {1, 0}}
88
17
— is a relation number with a list {{89, 85}, {356, 17}, {1, 0}}
89
17
— is a relation number with a list {{90, 85}, {1, 0}}
90
17
— is a relation number with a list
91
  {{91, 85}, {546, -17}, {182, 17}, {455, -17}, {364, -17}, {1, 0}}
17
— is a relation number with a list {{92, 85}, {322, -17}, {1, 0}}
92
17
— is a relation number with a list {{93, 85}, {744, 17}, {372, -17}, {186, 17}, {1, 0}}
93
17
— is a relation number with a list {{94, 102}, {188, 17}, {1, 0}}
94
17
— is a relation number with a list
95
  {{95, 102}, {665, -51}, {190, 17}, {285, -17}, {380, -17}, {570, 17}, {760, 17}, {1, 0}}
17
— is a relation number with a list {{96, 102}, {1, 0}}
96

```

```

17
— is a relation number with a list {{97, 102}, {485, -34},
97
  {873, 68}, {1067, -51}, {388, -17}, {291, 17}, {194, 17}, {679, -17}, {1, 0}}

17
— is a relation number with a list {{98, 102}, {1, 0}}
98

17
— is a relation number with a list {{99, 102}, {1, 0}}
99

17
— is a relation number with a list {{100, 102}, {1, 0}}
100

17
— is a relation number with a list {{101, 102}, {1, 0}}
101

17
— is a relation number with a list {{103, 102}, {1, 0}}
103

17
— is a relation number with a list {{104, 102}, {1, 0}}
104

17
— is a relation number with a list {{105, 102}, {1, 0}}
105

17
— is a relation number with a list {{106, 102}, {1, 0}}
106

17
— is a relation number with a list {{107, 102}, {535, 34},
107
  {963, 34}, {1177, 85}, {1391, -34}, {321, 17}, {214, 17}, {749, -34}, {1, 0}}

17
— is a relation number with a list {{108, 102}, {1, 0}}
108

17
— is a relation number with a list {{109, 102}, {763, 51},
109
  {218, 17}, {327, -17}, {436, -17}, {654, 17}, {872, -51}, {545, -34}, {1, 0}}

17
— is a relation number with a list {{110, 102}, {220, 17}, {1, 0}}
110

17
— is a relation number with a list
111
  {{111, 119}, {888, -17}, {444, 17}, {222, 17}, {1, 0}}

17
— is a relation number with a list {{112, 119}, {1, 0}}
112

17
— is a relation number with a list
113
  {{113, 119}, {678, 17}, {226, 17}, {565, -34}, {1469, 85}, {2712, -187}, {10509, 578},
  {11865, -731}, {19097, 714}, {20453, -680}, {5989, -255}, {14012, 697},
  {8136, 425}, {6893, 323}, {12430, -901}, {20792, -1411}, {42149, 918}, {8927, -323},
  {13221, 697}, {2486, 153}, {4294, -153}, {1130, 51}, {904, 51}, {1582, -51}, {1, 0}}

17
— is a relation number with a list
114
  {{114, 119}, {285, 17}, {228, 17}, {399, 17}, {456, 17}, {1, 0}}

17
— is a relation number with a list {{115, 119}, {460, -17}, {1, 0}}
115

```

```

17
116 is a relation number with a list {{116, 119}, {348, 17}, {232, 17}, {348, -17}}

17
117 is a relation number with a list
    {{117, 119}, {234, 17}, {468, -17}, {312, -17}, {234, 17}}

17
118 is a relation number with a list {{118, 119}, {1, 0}}

17
120 is a relation number with a list {{120, 119}, {1, 0}}

17
121 is a relation number with a list
    {{121, 119}, {242, 17}, {484, 17}, {968, 17}, {1, 0}}

17
122 is a relation number with a list
    {{122, 119}, {366, -17}, {488, 17}, {305, -17}, {1, 0}}

17
123 is a relation number with a list {{123, 119}, {492, 17}, {1, 0}}

17
124 is a relation number with a list {{124, 119}, {310, -17}, {1, 0}}

17
125 is a relation number with a list {{125, 119}, {750, -17}, {250, 17}, {1, 0}}

17
126 is a relation number with a list {{126, 119}, {1, 0}}

17
127 is a relation number with a list
    {{127, 119}, {1016, 17}, {508, 17}, {254, 17}, {1, 0}}

17
128 is a relation number with a list {{128, 136}, {1, 0}}

17
129 is a relation number with a list {{129, 136}, {301, -17}, {645, -17}, {1, 0}}

17
130 is a relation number with a list {{130, 136}, {390, -17}, {1, 0}}

17
131 is a relation number with a list {{131, 136}, {655, 34},
    {1179, 17}, {786, -17}, {524, 17}, {393, 17}, {262, 17}, {917, -34}, {1, 0}}

17
132 is a relation number with a list {{132, 136}, {1, 0}}

17
133 is a relation number with a list {{133, 136}, {399, 17}, {1064, -51}, {1, 0}}

17
134 is a relation number with a list {{134, 136}, {1, 0}}

17
135 is a relation number with a list {{135, 136}, {1, 0}}

17
137 is a relation number with a list {{137, 136}, {1, 0}}

```

```

17
138 is a relation number with a list {{138, 136}, {1, 0}}

17
139 is a relation number with a list {{139, 136}, {417, -17},
    {1112, 51}, {1390, 51}, {1807, 17}, {695, -17}, {278, 17}, {834, 17}, {1, 0}}

17
140 is a relation number with a list {{140, 136}, {1, 0}}

17
141 is a relation number with a list
    {{141, 136}, {705, -34}, {423, 17}, {282, 17}, {987, -17}, {1, 0}}

17
142 is a relation number with a list {{142, 136}, {426, 17}, {1, 0}}

17
143 is a relation number with a list {{143, 136}, {1001, 51},
    {2717, 136}, {429, -17}, {572, 17}, {858, 17}, {1144, -17}, {715, 34}, {1, 0}}

17
144 is a relation number with a list {{144, 136}, {1, 0}}

17
145 is a relation number with a list
    {{145, 153}, {1160, -17}, {580, -17}, {290, 17}, {1, 0}}

17
146 is a relation number with a list {{146, 153}, {511, 17}, {1, 0}}

17
147 is a relation number with a list
    {{147, 153}, {294, 17}, {735, 34}, {1911, 85}, {2009, -17}, {1, 0}}

17
148 is a relation number with a list {{148, 153}, {370, -17}, {1, 0}}

17
149 is a relation number with a list {{149, 153}, {596, -17}, {1, 0}}

17
150 is a relation number with a list {{150, 153}, {1, 0}}

17
151 is a relation number with a list
    {{151, 153}, {302, 17}, {604, 17}, {1208, 17}, {1, 0}}

17
152 is a relation number with a list {{152, 153}, {1, 0}}

17
154 is a relation number with a list {{154, 153}, {1, 0}}

17
155 is a relation number with a list
    {{155, 153}, {310, 17}, {620, -17}, {1240, -51}, {2480, -17}, {310, 17}}

17
156 is a relation number with a list {{156, 153}, {1, 0}}

17
157 is a relation number with a list {{157, 153}, {628, 17}, {1, 0}}

```



```

17
158 is a relation number with a list
    {{158, 153}, {395, 17}, {316, 17}, {1106, 51}, {1264, 51}, {1738, -17}, {316, 17}}

17
159 is a relation number with a list
    {{159, 153}, {318, 17}, {795, 17}, {636, 17}, {1113, -34}, {477, 17}, {1, 0}}

17
160 is a relation number with a list {{160, 153}, {560, -17}, {1, 0}}

17
161 is a relation number with a list
    {{161, 153}, {1288, 17}, {644, -17}, {322, 17}, {1, 0}}

17
162 is a relation number with a list {{162, 170}, {324, 17}, {1, 0}}

17
163 is a relation number with a list
    {{163, 170}, {1141, 17}, {326, 17}, {489, 17}, {652, 17}, {978, 17},
    {1304, -51}, {3586, 85}, {2608, -17}, {1141, -34}, {2445, -68}, {489, 17}}

17
164 is a relation number with a list {{164, 170}, {492, -17}, {1, 0}}

17
165 is a relation number with a list {{165, 170}, {1, 0}}

17
166 is a relation number with a list {{166, 170}, {1, 0}}

17
167 is a relation number with a list {{167, 170}, {501, 17}, {1336, -17},
    {1169, -17}, {668, -17}, {835, -34}, {2505, 68}, {1837, 51}, {1, 0}}

17
168 is a relation number with a list {{168, 170}, {1, 0}}

17
169 is a relation number with a list {{169, 170}, {1, 0}}

18
5 is a relation number with a list {{5, 18}, {65, 144}, {395, 702}, {1535, 2016},
    {2405, -1422}, {2195, -792}, {905, 702}, {1015, -144}, {35, 36}, {1, 0}}

18
7 is a relation number with a list {{7, 18}, {77, 72}, {35, -36}, {1, 0}}

18
11 is a relation number with a list {{11, 18}, {77, 54}, {253, 180},
    {803, -648}, {1705, 1242}, {5093, -3006}, {10109, -18}, {77, -54}}

18
13 is a relation number with a list
    {{13, 18}, {65, 36}, {91, 36}, {221, 144}, {871, 540}, {2717, 504},
    {2561, -540}, {1807, -486}, {1781, -1080}, {4927, 396}, {2275, -1152},
    {377, -162}, {689, -198}, {1235, 846}, {5057, -3006}, {12415, 4698},
    {21827, -630}, {2899, 162}, {221, 36}, {65, 18}, {91, 18}, {1, 0}}

18
17 is a relation number with a list {{17, 18}, {1, 0}}

```

```

18
— is a relation number with a list {{19, 18}, {1, 0}}
19

18
— is a relation number with a list {{23, 18}, {115, -36}, {161, 54}, {1, 0}}
23

18
— is a relation number with a list {{25, 18}, {175, -54}, {325, 54}, {1, 0}}
25

18
— is a relation number with a list
29
  {{29, 36}, {203, -36}, {377, 108}, {1537, 270}, {2407, -360}, {3277, 270},
  {1073, -162}, {1769, 306}, {1943, -432}, {6235, -918}, {5539, -882},
  {7163, 1098}, {15167, -3600}, {22243, 6048}, {56521, 18}, {1, 0}}

18
— is a relation number with a list
31
  {{31, 36}, {155, -36}, {341, 72}, {589, 162}, {1829, 288}, {3131, -162},
  {1643, -252}, {3751, -900}, {4681, -720}, {11129, 2934}, {18817, -3546},
  {33697, 7470}, {113243, 31446}, {388771, -71874}, {911431, -111222},
  {671305, 60228}, {272707, -33084}, {249085, -13194}, {49631, 5562},
  {13237, -3330}, {2573, 144}, {589, -18}, {155, 18}, {217, -54}, {1, 0}}

18
— is a relation number with a list {{35, 36}, {1, 0}}
35

18
— is a relation number with a list {{37, 36}, {1, 0}}
37

18
— is a relation number with a list {{41, 36}, {205, 36}, {451, -90}, {1, 0}}
41

18
— is a relation number with a list
43
  {{43, 36}, {301, 36}, {559, -90}, {817, -108}, {2021, 414}, {2107, -162}, {1, 0}}

18
— is a relation number with a list {{47, 54}, {329, -18}, {235, -36}, {799, -144},
47
  {3055, -252}, {1457, -126}, {2585, -18}, {329, -36}, {235, 18}, {1, 0}}

18
— is a relation number with a list {{49, 54}, {245, -36}, {1, 0}}
49

18
— is a relation number with a list {{53, 54}, {1, 0}}
53

18
— is a relation number with a list {{55, 54}, {1, 0}}
55

18
— is a relation number with a list {{59, 54}, {295, 36}, {413, -18}, {1, 0}}
59

18
— is a relation number with a list {{61, 54}, {427, 18}, {305, -18}, {1, 0}}
61

18
— is a relation number with a list {{65, 72}, {455, -18}, {1, 0}}
65

18
— is a relation number with a list
67
  {{67, 72}, {335, 36}, {737, 36}, {1139, -36}, {871, 72}, {469, 36}, {1, 0}}

```

```

18
— is a relation number with a list {{71, 72}, {1, 0}}
71
18
— is a relation number with a list {{73, 72}, {1, 0}}
73
18
— is a relation number with a list {{77, 72}, {385, -36}, {1, 0}}
77
18
— is a relation number with a list {{79, 72}, {553, 18}, {395, 18}, {1, 0}}
79
18
— is a relation number with a list {{83, 90}, {581, -36}, {415, -18}, {1, 0}}
83
18
— is a relation number with a list {{85, 90}, {1, 0}}
85
18
— is a relation number with a list {{89, 90}, {1, 0}}
89
18
— is a relation number with a list {{91, 90}, {1, 0}}
91
18
— is a relation number with a list {{95, 90}, {1, 0}}
95
18
— is a relation number with a list {{97, 90}, {679, 36}, {485, 18}, {1, 0}}
97
18
— is a relation number with a list {{101, 108}, {707, 54}, {505, -36}, {1, 0}}
101
18
— is a relation number with a list {{103, 108}, {515, 36}, {1133, -54}, {1, 0}}
103
18
— is a relation number with a list {{107, 108}, {1, 0}}
107
18
— is a relation number with a list {{109, 108}, {1, 0}}
109
18
— is a relation number with a list
113
{{113, 108}, {565, -36}, {1243, -90}, {1921, 72}, {2599, 144}, {791, 18}, {1, 0}}
18
— is a relation number with a list {{115, 108}, {805, -54}, {1, 0}}
115
18
— is a relation number with a list {{119, 126}, {1, 0}}
119
18
— is a relation number with a list {{121, 126}, {605, -36}, {847, -54},
121
{2057, 108}, {605, 18}, {847, -36}, {2057, 72}, {3751, 216}, {9559, 540},
{19481, 1314}, {27709, 1764}, {62315, -234}, {781, -18}, {847, -36}}
18
— is a relation number with a list {{125, 126}, {1, 0}}
125
18
— is a relation number with a list {{127, 126}, {1, 0}}
127
18
— is a relation number with a list {{131, 126}, {655, 36}, {917, 54}, {1, 0}}
131

```

```

18
133 is a relation number with a list {{133, 126}, {1, 0}}

18
137 is a relation number with a list
{{137, 144}, {959, 54}, {1781, 90}, {2603, -18}, {959, -54}}

18
139 is a relation number with a list
{{139, 144}, {695, -36}, {1529, -54}, {2363, 144}, {8201, -162}, {8479, -540},
{22379, -288}, {11815, 252}, {4031, -54}, {2641, -18}, {695, -18}, {973, -18}, {1, 0}}

18
143 is a relation number with a list {{143, 144}, {1, 0}}

18
145 is a relation number with a list {{145, 144}, {1, 0}}

18
149 is a relation number with a list {{149, 144}, {745, 36}, {1639, -18}, {1, 0}}

18
151 is a relation number with a list
{{151, 144}, {1057, -54}, {3473, -126}, {8305, 216}, {14647, -558}, {20989, 810},
{10721, 378}, {20687, 360}, {25217, 252}, {2567, 108}, {3775, -108}, {755, 18}, {1, 0}}

18
155 is a relation number with a list {{155, 162}, {1085, -36}, {1, 0}}

18
157 is a relation number with a list {{157, 162}, {785, 36}, {1099, 18}, {1, 0}}

18
161 is a relation number with a list {{161, 162}, {1, 0}}

18
163 is a relation number with a list {{163, 162}, {1, 0}}

18
167 is a relation number with a list
{{167, 162}, {835, -36}, {1169, 36}, {2839, -108}, {5177, -180}, {7181, -126}, {1, 0}}

18
169 is a relation number with a list
{{169, 162}, {1183, 36}, {845, 36}, {2873, -36}, {1183, 36}}

18
173 is a relation number with a list {{173, 180}, {1211, -18}, {865, 36}, {1, 0}}

18
175 is a relation number with a list {{175, 180}, {1, 0}}

18
179 is a relation number with a list {{179, 180}, {1, 0}}

known cases

known cases

known cases

```

```

19
5 is a relation number with a list
  {{5, 19}, {70, 171}, {505, 1064}, {2795, 5301}, {12530, 21109}, {42895, 57456},
  {72805, -10621}, {7710, -5491}, {11095, 14706}, {18055, -4921},
  {8145, -6346}, {8995, 2451}, {4045, 3116}, {4645, -2071},
  {2515, -798}, {605, 608}, {15, -19}, {20, 19}, {1, 0}}

19
6 is a relation number with a list {{6, 19}, {78, 133},
  {330, 247}, {498, -95}, {138, -133}, {15, -19}, {12, 19}, {42, 19}, {12, 19}}

19
7 is a relation number with a list {{7, 19}, {84, 95}, {77, -38}, {1, 0}}

19
8 is a relation number with a list {{8, 19}, {88, 57}, {104, 19}, {72, -19}, {1, 0}}

19
9 is a relation number with a list {{9, 19}, {90, 19}, {45, 19},
  {63, 38}, {117, -95}, {198, -19}, {72, -19}, {36, 19}, {18, 19}, {1, 0}}

19
10 is a relation number with a list {{10, 19}, {90, -19}, {1, 0}}

19
11 is a relation number with a list
  {{11, 19}, {88, -57}, {286, 133}, {220, -57}, {88, 19}, {77, 57},
  {220, -133}, {506, -285}, {704, -513}, {2101, 1615}, {5346, -703},
  {3058, 2451}, {6677, 3895}, {12243, -551}, {121, 76}, {341, -247},
  {1034, 855}, {1969, -798}, {4103, -1691}, {7931, -4902}, {20603, -17252},
  {36861, 1235}, {2079, 779}, {2838, 1235}, {4048, -399}, {638, 19}, {88, -57}}

19
12 is a relation number with a list {{12, 19}, {42, 19}, {1, 0}}

19
13 is a relation number with a list {{13, 19}, {78, -19}, {26, 19},
  {91, -19}, {52, 19}, {65, 38}, {143, -76}, {117, -38}, {39, 19}, {1, 0}}

19
14 is a relation number with a list
  {{14, 19}, {70, 19}, {42, -19}, {28, 19}, {63, -38}, {91, 19}, {28, 19}}

19
15 is a relation number with a list {{15, 19}, {60, 19}, {1, 0}}

19
16 is a relation number with a list {{16, 19}, {48, -19}, {72, -19}, {1, 0}}

19
17 is a relation number with a list {{17, 19}, {34, 19}, {68, -19},
  {136, 19}, {51, -19}, {102, -19}, {119, -57}, {85, -19}, {153, 19}, {1, 0}}

19
18 is a relation number with a list {{18, 19}, {1, 0}}

19
20 is a relation number with a list {{20, 19}, {1, 0}}

19
21 is a relation number with a list {{21, 19}, {42, 19}, {84, 19}, {56, -19}, {1, 0}}

```

```

19
22 — is a relation number with a list
    {{22, 19}, {66, 19}, {99, 38}, {330, 19}, {154, 19}, {1, 0}}

19
23 — is a relation number with a list {{23, 19}, {92, -19}, {69, -19},
    {161, 38}, {207, 19}, {46, 19}, {184, -19}, {138, -19}, {115, 38}, {1, 0}}

19
24 — is a relation number with a list {{24, 19}, {120, -19}, {1, 0}}

19
25 — is a relation number with a list
    {{25, 19}, {150, 19}, {50, 19}, {175, 57}, {100, -19}, {1, 0}}

19
26 — is a relation number with a list
    {{26, 19}, {91, -19}, {52, 19}, {130, -19}, {78, -19}, {1, 0}}

19
27 — is a relation number with a list {{27, 19}, {72, 19}, {108, 19}, {54, 19}, {1, 0}}

19
28 — is a relation number with a list
    {{28, 19}, {252, 19}, {70, -19}, {84, -19}, {56, 19}, {1, 0}}

19
29 — is a relation number with a list {{29, 38}, {261, -76}, {957, 304},
    {1305, 266}, {725, -114}, {1189, -190}, {1421, 76}, {667, -19}, {58, 19}, {1, 0}}

19
30 — is a relation number with a list {{30, 38}, {60, 19}, {1, 0}}

19
31 — is a relation number with a list {{31, 38}, {217, 19}, {248, -19}, {1, 0}}

19
32 — is a relation number with a list {{32, 38}, {96, 19}, {1, 0}}

19
33 — is a relation number with a list
    {{33, 38}, {165, -19}, {66, 19}, {99, -19}, {132, -19}, {1, 0}}

19
34 — is a relation number with a list {{34, 38}, {1, 0}}

19
35 — is a relation number with a list
    {{35, 38}, {105, -19}, {315, -19}, {280, 57}, {1, 0}}

19
36 — is a relation number with a list {{36, 38}, {1, 0}}

19
37 — is a relation number with a list {{37, 38}, {1, 0}}

19
39 — is a relation number with a list {{39, 38}, {1, 0}}

19
40 — is a relation number with a list {{40, 38}, {1, 0}}

```

```

19
41 — is a relation number with a list {{41, 38}, {123, 19}, {369, -76},
    {451, -19}, {205, 19}, {164, -19}, {287, -19}, {82, 19}, {246, -19}, {1, 0}}

19
42 — is a relation number with a list {{42, 38}, {1, 0}}

19
43 — is a relation number with a list {{43, 38}, {215, 19}, {258, 19},
    {344, -57}, {86, 19}, {387, 38}, {301, 38}, {129, 19}, {172, 19}, {1, 0}}

19
44 — is a relation number with a list {{44, 38}, {132, -19}, {1, 0}}

19
45 — is a relation number with a list {{45, 38}, {315, -19}, {120, -19}, {90, 19}, {1, 0}}

19
46 — is a relation number with a list {{46, 38}, {92, 19}, {138, -19}, {230, -19}, {1, 0}}

19
47 — is a relation number with a list
    {{47, 38}, {423, 76}, {1551, 190}, {1457, 95}, {1504, 209}, {1927, -304}, {4841, -589},
    {6063, -722}, {13489, -1216}, {5311, 817}, {19176, 361}, {2021, -190},
    {3243, -247}, {1504, -57}, {1034, -171}, {376, 19}, {188, 19}, {94, 19}, {1, 0}}

19
48 — is a relation number with a list {{48, 57}, {1, 0}}

19
49 — is a relation number with a list {{49, 57}, {392, -57}, {1, 0}}

19
50 — is a relation number with a list
    {{50, 57}, {350, -57}, {200, 19}, {225, 38}, {150, -19}, {1, 0}}

19
51 — is a relation number with a list
    {{51, 57}, {102, 19}, {357, 38}, {255, -19}, {136, -19}, {1, 0}}

19
52 — is a relation number with a list {{52, 57}, {260, -19}, {156, -19}, {1, 0}}

19
53 — is a relation number with a list {{53, 57}, {212, 19}, {159, -19}, {371, 57},
    {1484, 171}, {2915, 342}, {8639, 456}, {1325, 57}, {742, 95}, {954, 95}, {212, 19}}

19
54 — is a relation number with a list {{54, 57}, {1, 0}}

19
55 — is a relation number with a list
    {{55, 57}, {110, 19}, {220, 19}, {440, 19}, {165, 19}, {330, -19}, {385, 19}, {1, 0}}

19
56 — is a relation number with a list {{56, 57}, {1, 0}}

19
58 — is a relation number with a list {{58, 57}, {1, 0}}

19
59 — is a relation number with a list {{59, 57}, {118, 19}, {236, -19},
    {472, -57}, {944, -19}, {354, -19}, {413, 57}, {826, -95}, {1711, 95}, {1, 0}}

```

```

19
— is a relation number with a list {{60, 57}, {1, 0}}
60
19
— is a relation number with a list {{61, 57}, {244, -19}, {183, 19},
61
  {427, 38}, {549, -76}, {1037, -114}, {671, -57}, {793, 19}, {305, -19}, {1, 0}}
19
— is a relation number with a list
62
  {{62, 57}, {310, 19}, {186, 19}, {124, 19}, {558, 19}, {434, -19}, {186, -19}}
19
— is a relation number with a list {{63, 57}, {126, 19}, {1, 0}}
63
19
— is a relation number with a list {{64, 57}, {448, 57}, {1, 0}}
64
19
— is a relation number with a list {{65, 57}, {520, 57}, {455, -19}, {1, 0}}
65
19
— is a relation number with a list {{66, 57}, {1, 0}}
66
19
— is a relation number with a list {{67, 76}, {603, 38}, {335, 19},
67
  {469, 57}, {871, 114}, {2747, 152}, {737, -57}, {268, 19}, {134, 19}, {1, 0}}
19
— is a relation number with a list {{68, 76}, {1, 0}}
68
19
— is a relation number with a list
69
  {{69, 76}, {161, -19}, {207, 19}, {138, 19}, {345, -19}, {1, 0}}
19
— is a relation number with a list {{70, 76}, {210, 19}, {1, 0}}
70
19
— is a relation number with a list {{71, 76}, {355, 19}, {426, 19},
71
  {568, -19}, {142, 19}, {639, -19}, {497, 19}, {213, -19}, {284, 19}, {1, 0}}
19
— is a relation number with a list {{72, 76}, {1, 0}}
72
19
— is a relation number with a list {{73, 76}, {219, -19}, {657, 19}, {584, -19},
73
  {365, -38}, {1095, -76}, {2263, -247}, {2920, 209}, {438, 19}, {1, 0}}
19
— is a relation number with a list {{74, 76}, {1, 0}}
74
19
— is a relation number with a list {{75, 76}, {1, 0}}
75
19
— is a relation number with a list {{77, 76}, {1, 0}}
77
19
— is a relation number with a list {{78, 76}, {1, 0}}
78

```



```

19
— is a relation number with a list
79
  {{79, 76}, {237, 19}, {711, -38}, {869, 76}, {2607, -266}, {4187, -133}, {5056, 437},
  {14852, 1197}, {38552, 1843}, {11929, 722}, {27255, 1957}, {11297, 266}, {9875, -361},
  {10112, 665}, {10823, 475}, {8058, -703}, {25675, 38}, {1027, -38}, {1, 0}}

19
— is a relation number with a list {{80, 76}, {1, 0}}
80

19
— is a relation number with a list {{81, 76}, {405, -19}, {162, 19}, {1, 0}}
81

19
— is a relation number with a list {{82, 76}, {246, -19}, {1, 0}}
82

19
— is a relation number with a list {{83, 76}, {581, 57}, {913, -76}, {1, 0}}
83

19
— is a relation number with a list {{84, 76}, {1, 0}}
84

19
— is a relation number with a list {{85, 76}, {765, -38}, {1, 0}}
85

19
— is a relation number with a list
86
  {{86, 95}, {387, 19}, {301, 19}, {258, 19}, {344, 19}, {1, 0}}

19
— is a relation number with a list {{87, 95}, {232, -19}, {348, 19}, {174, 19}, {1, 0}}
87

19
— is a relation number with a list {{88, 95}, {616, 19}, {1, 0}}
88

19
— is a relation number with a list {{89, 95}, {534, -19}, {178, 19},
89
  {623, -38}, {1335, 38}, {445, -38}, {979, 38}, {801, 38}, {267, 19}, {1, 0}}

19
— is a relation number with a list {{90, 95}, {1, 0}}
90

19
— is a relation number with a list {{91, 95}, {364, 19}, {273, 19}, {1, 0}}
91

19
— is a relation number with a list {{92, 95}, {276, -19}, {414, 19}, {1, 0}}
92

19
— is a relation number with a list
93
  {{93, 95}, {186, 19}, {372, -19}, {248, -19}, {1, 0}}

19
— is a relation number with a list {{94, 95}, {1, 0}}
94

19
— is a relation number with a list {{96, 95}, {1, 0}}
96

19
— is a relation number with a list
97
  {{97, 95}, {194, 19}, {388, 19}, {776, 19}, {291, -19}, {582, -19}, {679, -19},
  {485, 38}, {873, 76}, {3589, 342}, {16393, 1064}, {42001, -3743}, {80316, -1235},
  {3977, 171}, {4268, -133}, {1164, 95}, {2328, 95}, {4559, -285}, {1, 0}}

```

```

19
98 is a relation number with a list
  {{98, 95}, {294, 19}, {882, -19}, {392, -19}, {1, 0}}

19
99 is a relation number with a list {{99, 95}, {396, -19}, {1, 0}}

19
100 is a relation number with a list {{100, 95}, {1, 0}}

19
101 is a relation number with a list
  {{101, 95}, {606, 19}, {202, 19}, {707, -57}, {2323, -76}, {3333, 152},
   {1111, -95}, {2929, 228}, {3535, 247}, {7777, 76}, {2525, 76}, {1717, -76},
   {3131, 19}, {404, -19}, {505, -19}, {808, -57}, {1010, -57}, {1616, -19}, {1, 0}}

19
102 is a relation number with a list
  {{102, 95}, {714, -19}, {408, -19}, {306, -19}, {1, 0}}

19
103 is a relation number with a list {{103, 95}, {824, 57}, {2678, -57}, {1, 0}}

19
104 is a relation number with a list
  {{104, 95}, {468, -19}, {728, -19}, {312, -19}, {1, 0}}

19
105 is a relation number with a list {{105, 114}, {1, 0}}

19
106 is a relation number with a list
  {{106, 114}, {212, 19}, {318, 19}, {530, -19}, {1, 0}}

19
107 is a relation number with a list
  {{107, 114}, {749, 38}, {1177, -95}, {3959, -323}, {8881, 133}, {3210, 19}, {1, 0}}

19
108 is a relation number with a list {{108, 114}, {1, 0}}

19
109 is a relation number with a list {{109, 114}, {545, 19}, {654, -19},
  {872, 57}, {1853, 76}, {3161, 19}, {763, -57}, {2398, 57}, {436, -19}, {1, 0}}

19
110 is a relation number with a list {{110, 114}, {1, 0}}

19
111 is a relation number with a list {{111, 114}, {1, 0}}

19
112 is a relation number with a list {{112, 114}, {1, 0}}

19
113 is a relation number with a list {{113, 114}, {1, 0}}

19
115 is a relation number with a list {{115, 114}, {1, 0}}

19
116 is a relation number with a list {{116, 114}, {1, 0}}

```

```

19
117 is a relation number with a list {{117, 114}, {1, 0}}

19
118 is a relation number with a list {{118, 114}, {1, 0}}

19
119 is a relation number with a list
    {{119, 114}, {595, -19}, {714, 19}, {952, 19}, {238, 19}, {1071, -38}, {1, 0}}

19
120 is a relation number with a list {{120, 114}, {1, 0}}

19
121 is a relation number with a list {{121, 114}, {847, -38}, {1, 0}}

19
122 is a relation number with a list
    {{122, 114}, {244, 19}, {366, 19}, {305, 19}, {1, 0}}

19
123 is a relation number with a list {{123, 114}, {1, 0}}

19
124 is a relation number with a list
    {{124, 133}, {279, -19}, {372, -19}, {248, 19}, {1, 0}}

19
125 is a relation number with a list {{125, 133}, {1000, -57},
    {3250, 209}, {2350, 133}, {1100, 19}, {250, 19}, {375, -19}, {1, 0}}

19
126 is a relation number with a list {{126, 133}, {1, 0}}

19
127 is a relation number with a list {{127, 133}, {762, -19}, {254, 19},
    {889, 19}, {508, 19}, {635, -38}, {1397, 19}, {1143, -19}, {381, -19}, {1, 0}}

19
128 is a relation number with a list {{128, 133}, {640, -19}, {384, 19}, {1, 0}}

19
129 is a relation number with a list {{129, 133}, {516, 19}, {1, 0}}

19
130 is a relation number with a list {{130, 133}, {390, -19}, {585, 38}, {390, 19}}

19
131 is a relation number with a list {{131, 133}, {262, 19}, {524, 19}, {1048, -57},
    {2882, 57}, {3275, 133}, {6550, -323}, {11790, 437}, {1179, 38}, {1, 0}}

19
132 is a relation number with a list {{132, 133}, {1, 0}}

19
134 is a relation number with a list {{134, 133}, {1, 0}}

19
135 is a relation number with a list
    {{135, 133}, {270, 19}, {540, -19}, {1080, 19}, {1, 0}}

19
136 is a relation number with a list {{136, 133}, {408, 19}, {1224, 19}, {1, 0}}

```

```

19
137 is a relation number with a list {{137, 133}, {548, -19}, {411, -19},
    {959, -57}, {1370, 19}, {274, 19}, {1096, 19}, {822, 19}, {685, 38}, {1, 0}}

19
138 is a relation number with a list {{138, 133}, {690, 19}, {1, 0}}

19
139 is a relation number with a list {{139, 133}, {834, 19}, {278, 19},
    {973, 19}, {556, -19}, {695, 19}, {1112, -57}, {3892, -57}, {2224, -19}, {1, 0}}

19
140 is a relation number with a list {{140, 133}, {1, 0}}

19
141 is a relation number with a list
    {{141, 133}, {376, 19}, {564, -19}, {282, 19}, {1, 0}}

19
142 is a relation number with a list
    {{142, 133}, {639, 38}, {994, 57}, {3550, 19}, {426, -19}, {568, 19}, {1, 0}}

19
143 is a relation number with a list {{143, 152}, {1287, -19}, {715, -38},
    {1001, -19}, {858, -19}, {429, 19}, {1144, 19}, {572, -19}, {286, 19}, {1, 0}}

19
144 is a relation number with a list {{144, 152}, {1, 0}}

19
145 is a relation number with a list {{145, 152}, {1015, 38}, {1595, -76}, {1, 0}}

19
146 is a relation number with a list {{146, 152}, {438, 19}, {1, 0}}

19
147 is a relation number with a list
    {{147, 152}, {735, -19}, {294, 19}, {441, 19}, {588, -19}, {1, 0}}

19
148 is a relation number with a list {{148, 152}, {1, 0}}

19
149 is a relation number with a list {{149, 152}, {447, -19}, {1341, -76}, {4023, 38},
    {745, 38}, {2235, 38}, {1043, 57}, {2533, 95}, {4768, -171}, {2980, 19}, {447, 19}}

19
150 is a relation number with a list {{150, 152}, {1, 0}}

19
151 is a relation number with a list {{151, 152}, {1, 0}}

19
153 is a relation number with a list {{153, 152}, {1, 0}}

19
154 is a relation number with a list {{154, 152}, {1, 0}}

19
155 is a relation number with a list
    {{155, 152}, {465, 19}, {1395, 38}, {1705, -38}, {1, 0}}

19
156 is a relation number with a list {{156, 152}, {1, 0}}

```

```

19
157 is a relation number with a list {{157, 152}, {785, 19}, {942, 19},
    {1256, 57}, {314, 19}, {1413, -76}, {4867, 152}, {471, -19}, {628, 19}, {1, 0}}

19
158 is a relation number with a list {{158, 152}, {474, -19}, {1, 0}}

19
159 is a relation number with a list {{159, 152}, {1113, -38}, {1749, 19}, {1, 0}}

19
160 is a relation number with a list {{160, 152}, {1, 0}}

19
161 is a relation number with a list {{161, 152}, {1449, 19}, {805, 19}, {1, 0}}

19
162 is a relation number with a list {{162, 171}, {1, 0}}

19
163 is a relation number with a list {{163, 171}, {1304, -57}, {1141, -19}, {1, 0}}

19
164 is a relation number with a list
    {{164, 171}, {1148, 19}, {328, 19}, {820, -19}, {492, 19}, {1, 0}}

19
165 is a relation number with a list {{165, 171}, {330, 19}, {385, -19}, {1, 0}}

19
166 is a relation number with a list
    {{166, 171}, {830, 19}, {498, 19}, {332, 19}, {747, 38}, {1079, 57}, {332, 19}}

19
167 is a relation number with a list {{167, 171}, {668, 19}, {501, -19},
    {1169, 19}, {1503, 76}, {2839, -95}, {1837, -19}, {1002, -19}, {835, 38}, {1, 0}}

19
168 is a relation number with a list {{168, 171}, {1, 0}}

19
169 is a relation number with a list {{169, 171}, {338, 19}, {676, -19},
    {1352, 19}, {507, 19}, {1014, -19}, {1183, -19}, {845, 19}, {1521, -38}, {1, 0}}

19
170 is a relation number with a list {{170, 171}, {1, 0}}

19
172 is a relation number with a list {{172, 171}, {1, 0}}

19
173 is a relation number with a list
    {{173, 171}, {346, 19}, {692, 19}, {1384, -57}, {2768, -133}, {4325, 209}, {11072, 323},
    {15570, -551}, {24566, -893}, {75774, -3629}, {75255, -323}, {692, 19}}

19
174 is a relation number with a list {{174, 171}, {1, 0}}

19
175 is a relation number with a list {{175, 171}, {700, -19}, {525, 19}, {1, 0}}

19
176 is a relation number with a list {{176, 171}, {880, -19}, {528, -19}, {1, 0}}

```

```

19
177 is a relation number with a list
    {{177, 171}, {354, 19}, {1239, -38}, {885, -38}, {1947, -38}, {531, -19}, {1, 0}}

19
178 is a relation number with a list
    {{178, 171}, {1246, -19}, {712, 19}, {801, -19}, {534, -19}, {1, 0}}

19
179 is a relation number with a list {{179, 171}, {1432, 57}, {1253, -38}, {1, 0}}

19
180 is a relation number with a list {{180, 171}, {1, 0}}

19
181 is a relation number with a list
    {{181, 190}, {1629, -19}, {905, 19}, {1267, 19}, {1086, -19}, {543, -19},
    {1448, -57}, {4163, 171}, {10679, -437}, {34571, 741}, {46336, 2071},
    {140094, 7201}, {592775, -3344}, {160547, 1444}, {47603, 1520},
    {87423, -190}, {4163, 133}, {7240, -247}, {13937, 646}, {49775, -1976},
    {67875, -1406}, {70047, 2869}, {215571, -1178}, {543, -19}}

19
182 is a relation number with a list
    {{182, 190}, {364, 19}, {546, -19}, {455, 19}, {1, 0}}

19
183 is a relation number with a list
    {{183, 190}, {427, -19}, {549, -19}, {366, 19}, {915, -38}, {1, 0}}

19
184 is a relation number with a list {{184, 190}, {552, 19}, {1, 0}}

19
185 is a relation number with a list {{185, 190}, {1, 0}}

19
186 is a relation number with a list {{186, 190}, {1, 0}}

19
187 is a relation number with a list {{187, 190}, {561, -19}, {1683, -38}, {1, 0}}

19
188 is a relation number with a list {{188, 190}, {1, 0}}

19
189 is a relation number with a list {{189, 190}, {1, 0}}

known cases

```

```

20
— is a relation number with a list
7
{{7, 20}, {91, 120}, {203, -260}, {399, -460}, {427, -440}, {91, -40}, {77, -60},
{119, -80}, {273, 220}, {371, 480}, {763, 1000}, {1659, -2260}, {4207, 3800},
{2849, 2180}, {4683, 1880}, {6461, -5300}, {8127, 9340}, {8491, 7400},
{7637, 8160}, {3661, -4820}, {8113, 10560}, {17129, 23960}, {47817, -31100},
{100681, -69960}, {215047, 124700}, {240471, -185840}, {382417, -208260},
{238721, 93700}, {296653, 191680}, {606949, 392380}, {1244677, 809560},
{2621101, 1821940}, {5594127, -3229640}, {6056071, 5304420}, {5261557, 7064900},
{12623401, -13387440}, {5348273, 2027400}, {5137489, 486740}, {1516557, 925840},
{2345861, 221580}, {640633, 279320}, {573951, 315380}, {397663, 64700},
{66241, 74380}, {56973, -32320}, {53669, 72900}, {134617, -125680},
{62559, 13940}, {47593, -38400}, {64351, -84940}, {144123, 182800},
{270739, 267480}, {22813, -17860}, {34671, -25960}, {60977, -7500},
{6839, 6120}, {5033, -300}, {469, -580}, {777, -380}, {119, 60}, {1, 0}}

20
— is a relation number with a list {{9, 20}, {99, 40}, {171, -20}, {1, 0}}
9

20
— is a relation number with a list
11
{{11, 20}, {99, -40}, {209, -60}, {319, -80}, {1, 0}}

20
— is a relation number with a list
13
{{13, 20}, {91, 20}, {117, -80}, {481, -300}, {1547, -860}, {2249, 800}, {1963, -1340},
{8099, -4960}, {23673, -8360}, {18291, -3880}, {14417, 6080}, {29341, -11240},
{56927, -29040}, {14989, 8560}, {27703, 16580}, {70941, 2740}, {299, 20}, {1, 0}}

20
— is a relation number with a list {{17, 20}, {51, 20}, {153, 20}, {119, -60}, {1, 0}}
17

20
— is a relation number with a list {{19, 20}, {1, 0}}
19

20
— is a relation number with a list {{21, 20}, {1, 0}}
21

20
— is a relation number with a list
23
{{23, 20}, {69, -20}, {207, 80}, {759, 140}, {1357, -320}, {1771, 340},
{1633, -700}, {5359, -2120}, {23023, 8720}, {72151, -12340}, {43447, -18420},
{151961, -27240}, {264017, -62220}, {348151, 82640}, {404593, 141620},
{466141, -14540}, {19803, -7240}, {44091, 13160}, {106053, 26020},
{45379, 6560}, {12443, 600}, {3611, -1240}, {2507, 180}, {299, 20}, {1, 0}}

20
— is a relation number with a list {{27, 20}, {189, -20}, {1, 0}}
27

20
— is a relation number with a list {{29, 20}, {261, 40}, {551, -20}, {261, 40}}
29

20
— is a relation number with a list {{31, 40}, {279, 20}, {1, 0}}
31

20
— is a relation number with a list {{33, 40}, {77, -20}, {1, 0}}
33

```

```

20
— is a relation number with a list {{37, 40}, {111, 20}, {333, -20},
37
  {259, 40}, {703, -40}, {629, 120}, {1073, -200}, {2701, -100}, {1, 0}}

20
— is a relation number with a list {{39, 40}, {1, 0}}
39

20
— is a relation number with a list {{41, 40}, {1, 0}}
41

20
— is a relation number with a list
43
  {{43, 40}, {129, -20}, {387, 40}, {559, 100}, {1763, -200}, {1591, -280},
  {3827, -420}, {2021, -200}, {903, -200}, {4171, 840}, {1247, -160},
  {1419, 280}, {817, -120}, {989, 100}, {473, 100}, {1161, 20}, {1, 0}}

20
— is a relation number with a list
47
  {{47, 40}, {329, 60}, {1363, -80}, {141, 20}, {1, 0}}

20
— is a relation number with a list {{49, 40}, {441, -20}, {1, 0}}
49

20
— is a relation number with a list {{51, 60}, {1, 0}}
51

20
— is a relation number with a list
53
  {{53, 60}, {371, 40}, {583, -80}, {1219, -100}, {1007, 20}, {371, -60},
  {583, -100}, {901, -140}, {3233, -100}, {1749, -20}, {477, 20}, {159, 20}, {1, 0}}

20
— is a relation number with a list {{57, 60}, {1, 0}}
57

20
— is a relation number with a list {{59, 60}, {1, 0}}
59

20
— is a relation number with a list {{61, 60}, {1, 0}}
61

20
— is a relation number with a list {{63, 60}, {1, 0}}
63

20
— is a relation number with a list {{67, 60}, {469, -40}, {737, 40},
67
  {1139, -40}, {1273, -20}, {469, -60}, {737, 60}, {1139, -60}, {1, 0}}

20
— is a relation number with a list {{69, 60}, {1, 0}}
69

20
— is a relation number with a list {{71, 80}, {639, 80}, {1, 0}}
71

20
— is a relation number with a list {{73, 80}, {511, 40}, {657, -40},
73
  {1241, 140}, {1387, 40}, {949, -60}, {803, -20}, {219, -20}, {1, 0}}

20
— is a relation number with a list
77
  {{77, 80}, {231, 20}, {693, 80}, {189, -20}, {693, 80}}

20
— is a relation number with a list {{79, 80}, {1, 0}}
79

```



```

20
— is a relation number with a list {{81, 80}, {1, 0}}
81

20
— is a relation number with a list
83
  {{83, 80}, {249, -20}, {747, -40}, {1079, -60}, {1, 0}}

20
— is a relation number with a list {{87, 80}, {609, -40}, {261, -20}, {1, 0}}
87

20
— is a relation number with a list {{89, 80}, {801, -80}, {1, 0}}
89

20
— is a relation number with a list
91
  {{91, 100}, {819, 80}, {1729, 60}, {1001, 40}, {1, 0}}

20
— is a relation number with a list {{93, 100}, {217, -20}, {1, 0}}
93

20
— is a relation number with a list {{97, 100}, {291, 20}, {873, 40}, {679, 40}, {1, 0}}
97

20
— is a relation number with a list {{99, 100}, {1, 0}}
99

20
— is a relation number with a list {{101, 100}, {1, 0}}
101

20
— is a relation number with a list
103
  {{103, 100}, {309, -20}, {927, -80}, {3399, 320}, {12463, 920}, {42951, -3020},
  {69113, -2400}, {50161, 3700}, {168817, 12260}, {290769, -20660}, {157487, 12620},
  {622841, -30480}, {1363823, 38400}, {1913431, 131740}, {6454907, 217960},
  {8640979, -637700}, {29542563, 2582480}, {116934149, -6472480},
  {44239427, 3368600}, {46105581, -2183260}, {26483463, 1390700},
  {6196789, 54160}, {2322547, 166720}, {1187899, -103320}, {5292037, -366160},
  {17077091, -1239140}, {27899507, -2385700}, {75075979, -2096520},
  {41070323, 621420}, {5830109, -521160}, {10026947, 835960}, {471019, -40020},
  {949763, 64820}, {2321311, 84640}, {3711193, 70480}, {2497441, 14660},
  {539823, 42500}, {1305731, -67320}, {2745053, -4700}, {26059, 1660},
  {51603, -640}, {24411, -440}, {21733, 1100}, {27501, -1160}, {34917, -2560},
  {95069, 5240}, {77147, 440}, {15141, 1220}, {51603, -4600}, {103309, 7640},
  {376053, 16300}, {118759, -4480}, {226703, 21240}, {714511, 32120},
  {810713, 2540}, {46659, -1120}, {39243, 1060}, {2369, 160}, {3193, 260},
  {7519, 500}, {1957, -180}, {2369, 140}, {1133, 100}, {3399, -260}, {1957, -180}}

20
— is a relation number with a list
107
  {{107, 100}, {749, 60}, {3103, 40}, {1819, 140}, {1, 0}}

20
— is a relation number with a list
109
  {{109, 100}, {981, -80}, {2289, 100}, {1199, 100}, {1, 0}}

20
— is a relation number with a list {{111, 120}, {1, 0}}
111

```

```

20
113 is a relation number with a list {{113, 120}, {791, 20}, {1017, 80},
    {2599, 160}, {4407, 140}, {7571, -260}, {3503, -240}, {10961, -40}, {1, 0}}

20
117 is a relation number with a list {{117, 120}, {1, 0}}

20
119 is a relation number with a list {{119, 120}, {1, 0}}

20
121 is a relation number with a list {{121, 120}, {1, 0}}

20
123 is a relation number with a list {{123, 120}, {1, 0}}

20
127 is a relation number with a list
    {{127, 120}, {889, -20}, {1143, -20}, {381, -20}, {1, 0}}

20
129 is a relation number with a list {{129, 120}, {1, 0}}

20
131 is a relation number with a list {{131, 140}, {1179, 20}, {1, 0}}

20
133 is a relation number with a list {{133, 140}, {1, 0}}

20
137 is a relation number with a list
    {{137, 140}, {411, 20}, {1233, -40}, {959, 20}, {1, 0}}

20
139 is a relation number with a list {{139, 140}, {1, 0}}

20
141 is a relation number with a list {{141, 140}, {1, 0}}

20
143 is a relation number with a list
    {{143, 140}, {429, -20}, {1287, 20}, {1001, 60}, {2717, 160}, {429, -20}}

20
147 is a relation number with a list {{147, 140}, {1, 0}}

20
149 is a relation number with a list {{149, 140}, {1341, -20}, {1, 0}}

20
151 is a relation number with a list {{151, 160}, {1359, -40}, {1, 0}}

20
153 is a relation number with a list {{153, 160}, {1071, 20}, {1, 0}}

20
157 is a relation number with a list {{157, 160}, {471, 20}, {1413, -80}, {4239, 140},
    {6123, 140}, {5809, 220}, {13973, 720}, {46001, 1700}, {15857, 260}, {471, -20}}

20
159 is a relation number with a list {{159, 160}, {1, 0}}

20
161 is a relation number with a list {{161, 160}, {1, 0}}

```

```

20
163 is a relation number with a list
{{163, 160}, {489, -20}, {1467, -20}, {1141, -40}, {3097, 60}, {3749, -120}, {4727, 160},
{11899, 200}, {16137, 920}, {68949, 2320}, {106113, -580}, {4401, 40}, {1, 0}}

20
167 is a relation number with a list
{{167, 160}, {1169, -20}, {1503, 80}, {2839, -100}, {6513, -320}, {18871, 800},
{54943, -2000}, {157481, 5480}, {240313, 5800}, {419671, 13660},
{632763, -7820}, {109719, 5080}, {340847, 8860}, {695889, -20500},
{185537, 1620}, {127421, 4140}, {153473, 7060}, {308449, 3060},
{102037, 2220}, {13861, -560}, {23213, -1000}, {35571, -860}, {51937, -560},
{23881, -860}, {33233, 340}, {14529, 640}, {31897, 80}, {3841, -20}, {1, 0}}

20
169 is a relation number with a list {{169, 160}, {1521, 40}, {1, 0}}

20
171 is a relation number with a list {{171, 180}, {1, 0}}

20
173 is a relation number with a list
{{173, 180}, {1211, -60}, {1903, -40}, {2941, 120}, {10207, 480}, {21971, -780},
{22663, 1300}, {97399, -300}, {17473, -620}, {19549, -1040}, {36503, -1540},
{79061, 1360}, {31313, -20}, {1211, -40}, {1903, -100}, {519, -20}, {1, 0}}

20
177 is a relation number with a list {{177, 180}, {1, 0}}

20
179 is a relation number with a list {{179, 180}, {1, 0}}

20
181 is a relation number with a list {{181, 180}, {1, 0}}

20
183 is a relation number with a list {{183, 180}, {1, 0}}

20
187 is a relation number with a list {{187, 180}, {1309, 60}, {1, 0}}

20
189 is a relation number with a list {{189, 180}, {1, 0}}

20
191 is a relation number with a list {{191, 200}, {1719, -40}, {1, 0}}

20
193 is a relation number with a list
{{193, 200}, {1351, 40}, {1737, 20}, {579, -20}, {1, 0}}

20
197 is a relation number with a list
{{197, 200}, {591, 20}, {1773, 20}, {1379, -20}, {1, 0}}

20
199 is a relation number with a list {{199, 200}, {1, 0}}

known cases
known cases
known cases

```

```

21
— is a relation number with a list {{8, 21}, {104, 105}, {1, 0}}
8

21
— is a relation number with a list {{10, 21}, {110, 21}, {1, 0}}
10

21
— is a relation number with a list
11
  {{11, 21}, {110, -21}, {55, -21}, {88, 63}, {275, 168}, {671, -567}, {1144, 315},
  {1276, -1029}, {2717, -945}, {1298, 483}, {1661, 1029}, {4367, -2982}, {15235, -3717},
  {4037, -2352}, {7337, -2142}, {10021, -4431}, {12749, -63}, {253, -210},
  {473, 399}, {814, -273}, {55, -42}, {143, 84}, {275, 126}, {253, -63}, {1, 0}}

21
— is a relation number with a list {{13, 21}, {104, 63}, {286, 105}, {377, -147},
13
  {832, 567}, {3445, 1806}, {2171, 1071}, {377, -84}, {533, -231}, {923, -21}, {1, 0}}

21
— is a relation number with a list {{16, 21}, {80, -21}, {1, 0}}
16

21
— is a relation number with a list {{17, 21}, {68, -21}, {85, -42}, {1, 0}}
17

21
— is a relation number with a list
19
  {{19, 21}, {38, 21}, {76, 21}, {152, -63}, {494, -105}, {589, 42}, {1, 0}}

21
— is a relation number with a list {{20, 21}, {1, 0}}
20

21
— is a relation number with a list {{22, 21}, {1, 0}}
22

21
— is a relation number with a list
23
  {{23, 21}, {46, 21}, {92, -21}, {184, 21}, {115, 42}, {253, -42}, {1, 0}}

21
— is a relation number with a list {{25, 21}, {100, 21}, {1, 0}}
25

21
— is a relation number with a list {{26, 21}, {130, 21}, {52, 21}, {65, -21}, {1, 0}}
26

21
— is a relation number with a list {{29, 21}, {232, -63}, {580, 147}, {232, -63}}
29

21
— is a relation number with a list
31
  {{31, 21}, {310, 21}, {155, -21}, {248, 21}, {124, 21}, {62, 21}, {1, 0}}

21
— is a relation number with a list {{32, 42}, {80, -21}, {1, 0}}
32

21
— is a relation number with a list {{34, 42}, {68, 21}, {170, -21}, {1, 0}}
34

21
— is a relation number with a list {{37, 42}, {185, 21}, {148, -21}, {1, 0}}
37

21
— is a relation number with a list {{38, 42}, {1, 0}}
38

21
— is a relation number with a list {{40, 42}, {1, 0}}
40

```

```

21
— is a relation number with a list {{41, 42}, {1, 0}}
41

21
— is a relation number with a list {{43, 42}, {1, 0}}
43

21
— is a relation number with a list {{44, 42}, {1, 0}}
44

21
— is a relation number with a list {{46, 42}, {1, 0}}
46

21
— is a relation number with a list {{47, 42}, {235, -21}, {188, 21}, {1, 0}}
47

21
— is a relation number with a list {{50, 42}, {100, 21}, {1, 0}}
50

21
— is a relation number with a list {{52, 42}, {130, 21}, {1, 0}}
52

21
— is a relation number with a list
53
{{53, 63}, {530, 21}, {265, -42}, {689, -42}, {901, -84}, {1219, 105},
{2173, -399}, {9434, 1281}, {24751, -756}, {10441, -1302}, {1325, -231},
{3233, -567}, {8957, 1659}, {35086, 4515}, {54802, -441}, {6254, -1071},
{9116, -1029}, {7685, -273}, {2173, 168}, {583, 105}, {2491, 357}, {424, 63},
{901, -126}, {1007, 105}, {2279, -147}, {3869, 126}, {1961, 315}, {3763, 294},
{3127, 525}, {1219, 189}, {4505, -693}, {18338, 399}, {848, 21}, {424, -63}}

21
— is a relation number with a list {{55, 63}, {440, 63}, {1, 0}}
55

21
— is a relation number with a list {{58, 63}, {290, 21}, {116, 21}, {290, 21}}
58

21
— is a relation number with a list {{59, 63}, {236, -21}, {295, 21}, {1, 0}}
59

21
— is a relation number with a list {{61, 63}, {122, 21}, {244, -21},
61
{488, -63}, {976, 147}, {3233, -63}, {1220, -63}, {1403, 21}, {244, -21}}

21
— is a relation number with a list {{62, 63}, {1, 0}}
62

21
— is a relation number with a list {{64, 63}, {1, 0}}
64

21
— is a relation number with a list {{65, 63}, {130, 21}, {260, 21}, {520, 21}, {1, 0}}
65

21
— is a relation number with a list {{67, 63}, {268, 21}, {335, -42}, {1, 0}}
67

21
— is a relation number with a list {{68, 63}, {340, -21}, {1, 0}}
68

21
— is a relation number with a list {{71, 63}, {568, -63}, {1, 0}}
71

21
— is a relation number with a list
73
{{73, 63}, {730, -21}, {365, -42}, {949, 63}, {292, -21}, {146, 21}, {1, 0}}

```

```

21
— is a relation number with a list {{74, 84}, {185, 21}, {148, 21}, {1, 0}}
74

21
— is a relation number with a list {{76, 84}, {1, 0}}
76

21
— is a relation number with a list {{79, 84}, {395, -21}, {316, -21}, {1, 0}}
79

21
— is a relation number with a list {{80, 84}, {1, 0}}
80

21
— is a relation number with a list {{82, 84}, {1, 0}}
82

21
— is a relation number with a list {{83, 84}, {1, 0}}
83

21
— is a relation number with a list {{85, 84}, {1, 0}}
85

21
— is a relation number with a list {{86, 84}, {1, 0}}
86

21
— is a relation number with a list {{88, 84}, {1, 0}}
88

21
— is a relation number with a list {{89, 84}, {445, 21}, {356, 21}, {1, 0}}
89

21
— is a relation number with a list {{92, 84}, {1, 0}}
92

21
— is a relation number with a list {{94, 84}, {235, -21}, {188, 21}, {1, 0}}
94

21
— is a relation number with a list {{95, 105}, {190, 21}, {1, 0}}
95

21
— is a relation number with a list
97
  {{97, 105}, {776, 63}, {1940, -189}, {4850, -483}, {1940, 189}}

21
— is a relation number with a list {{100, 105}, {1, 0}}
100

21
— is a relation number with a list {{101, 105}, {404, -21}, {505, -21}, {1, 0}}
101

21
— is a relation number with a list
103
  {{103, 105}, {206, 21}, {412, 21}, {824, 21}, {515, -42}, {1133, 63}, {1, 0}}

21
— is a relation number with a list {{104, 105}, {1, 0}}
104

21
— is a relation number with a list {{106, 105}, {1, 0}}
106

21
— is a relation number with a list
107
  {{107, 105}, {214, 21}, {428, -21}, {856, -63}, {2782, 189}, {5671, -189}, {1, 0}}

21
— is a relation number with a list {{109, 105}, {436, 21}, {545, 21}, {1, 0}}
109

```

```

21
110 is a relation number with a list {{110, 105}, {1, 0}}

21
113 is a relation number with a list
      {{113, 105}, {904, -63}, {2486, -189}, {3277, -42}, {1, 0}}

21
115 is a relation number with a list {{115, 105}, {230, 21}, {1, 0}}

21
116 is a relation number with a list {{116, 126}, {290, 21}, {1, 0}}

21
118 is a relation number with a list {{118, 126}, {236, 21}, {295, -21}, {1, 0}}

21
121 is a relation number with a list {{121, 126}, {605, -21}, {484, 21}, {1, 0}}

21
122 is a relation number with a list {{122, 126}, {1, 0}}

21
124 is a relation number with a list {{124, 126}, {1, 0}}

21
125 is a relation number with a list {{125, 126}, {1, 0}}

21
127 is a relation number with a list {{127, 126}, {1, 0}}

21
128 is a relation number with a list {{128, 126}, {1, 0}}

21
130 is a relation number with a list {{130, 126}, {1, 0}}

21
131 is a relation number with a list {{131, 126}, {655, 21}, {524, -21}, {1, 0}}

21
134 is a relation number with a list {{134, 126}, {268, 21}, {670, 21}, {1, 0}}

21
136 is a relation number with a list {{136, 126}, {340, -21}, {1, 0}}

21
137 is a relation number with a list
      {{137, 147}, {1370, 21}, {685, 42}, {1781, 21}, {548, -21}, {274, 21}, {1, 0}}

21
139 is a relation number with a list {{139, 147}, {1112, 63}, {3058, 21}, {1112, -63}}

21
142 is a relation number with a list {{142, 147}, {710, 21}, {284, 21}, {710, -21}}

21
143 is a relation number with a list {{143, 147}, {572, -21}, {715, 42}, {1, 0}}

21
145 is a relation number with a list
      {{145, 147}, {290, 21}, {580, -21}, {1160, 21}, {1, 0}}

21
146 is a relation number with a list {{146, 147}, {1, 0}}

```

```

21
148 is a relation number with a list {{148, 147}, {1, 0}}

21
149 is a relation number with a list
{{149, 147}, {298, 21}, {596, 21}, {1192, -63}, {745, 42}, {1639, -21}, {1, 0}}

21
151 is a relation number with a list {{151, 147}, {604, 21}, {755, -21}, {1, 0}}

21
152 is a relation number with a list {{152, 147}, {760, -21}, {1, 0}}

21
155 is a relation number with a list
{{155, 147}, {1240, -63}, {620, 21}, {310, 21}, {1, 0}}

21
157 is a relation number with a list
{{157, 147}, {1570, -21}, {785, 42}, {2041, -42}, {2669, 168}, {2983, -42}, {1, 0}}

21
158 is a relation number with a list {{158, 168}, {395, -21}, {316, 21}, {1, 0}}

21
160 is a relation number with a list {{160, 168}, {1, 0}}

21
163 is a relation number with a list {{163, 168}, {815, 21}, {652, 21}, {1, 0}}

21
164 is a relation number with a list {{164, 168}, {1, 0}}

21
166 is a relation number with a list {{166, 168}, {1, 0}}

21
167 is a relation number with a list {{167, 168}, {1, 0}}

21
169 is a relation number with a list {{169, 168}, {1, 0}}

21
170 is a relation number with a list {{170, 168}, {1, 0}}

21
172 is a relation number with a list {{172, 168}, {1, 0}}

21
173 is a relation number with a list {{173, 168}, {865, -21}, {692, -21}, {1, 0}}

21
176 is a relation number with a list {{176, 168}, {1, 0}}

21
178 is a relation number with a list {{178, 168}, {445, 21}, {356, 21}, {1, 0}}

21
179 is a relation number with a list {{179, 189}, {1790, -21},
{895, 21}, {1432, -63}, {3043, -147}, {7876, 441}, {11098, 483}, {1969, -63},
{2864, 147}, {12709, -525}, {19511, -126}, {3401, -189}, {1, 0}}

21
181 is a relation number with a list {{181, 189}, {1448, 63}, {1, 0}}

```



```

21
184 is a relation number with a list {{184, 189}, {920, -21}, {1, 0}}

21
185 is a relation number with a list {{185, 189}, {740, -21}, {1, 0}}

21
187 is a relation number with a list {{187, 189}, {374, 21},
    {748, 21}, {1496, -63}, {2992, 21}, {1870, -63}, {3740, 21}, {374, 21}}

21
188 is a relation number with a list {{188, 189}, {1, 0}}

21
190 is a relation number with a list {{190, 189}, {1, 0}}

21
191 is a relation number with a list
    {{191, 189}, {382, 21}, {764, -21}, {1528, 21}, {955, -21}, {1910, -21}, {1, 0}}

21
193 is a relation number with a list {{193, 189}, {772, 21}, {965, 42}, {1, 0}}

21
194 is a relation number with a list
    {{194, 189}, {970, 21}, {388, 21}, {485, 21}, {1, 0}}

21
197 is a relation number with a list {{197, 189}, {1576, -63}, {1, 0}}

21
199 is a relation number with a list
    {{199, 189}, {1990, 21}, {995, 21}, {1592, -21}, {796, -21}, {398, 21}, {1, 0}}

21
200 is a relation number with a list {{200, 210}, {1, 0}}

21
202 is a relation number with a list {{202, 210}, {404, 21}, {505, 21}, {1, 0}}

21
205 is a relation number with a list {{205, 210}, {1, 0}}

21
206 is a relation number with a list {{206, 210}, {1, 0}}

21
208 is a relation number with a list {{208, 210}, {1, 0}}

21
209 is a relation number with a list {{209, 210}, {1, 0}}

known cases

known cases

22
7 is a relation number with a list
    {{7, 22}, {105, 176}, {497, 330}, {1141, 1276}, {945, -22}, {1, 0}}

22
9 is a relation number with a list
    {{9, 22}, {117, 88}, {261, 154}, {423, -352}, {639, -44}, {63, -22}, {1, 0}}

```

```

22
— is a relation number with a list
13
  {{13, 22}, {117, -88}, {377, 132}, {247, -44}, {221, -176}, {585, -308},
  {403, -88}, {481, 330}, {1963, 968}, {351, 110}, {273, 44}, {117, -22}, {91, 22},
  {39, 22}, {65, 44}, {273, 110}, {689, 264}, {1339, 1100}, {3107, -1474},
  {2067, -1672}, {5135, 4334}, {10413, 3476}, {195, 22}, {39, -22}}

22
— is a relation number with a list {{15, 22}, {105, -22}, {1, 0}}
15

22
— is a relation number with a list
17
  {{17, 22}, {85, -44}, {51, 22}, {119, 66}, {221, 22}, {1, 0}}

22
— is a relation number with a list
19
  {{19, 22}, {57, -22}, {171, 22}, {95, 22}, {133, -44}, {1, 0}}

22
— is a relation number with a list {{21, 22}, {1, 0}}
21

22
— is a relation number with a list {{23, 22}, {1, 0}}
23

22
— is a relation number with a list {{25, 22}, {75, 22}, {225, -44}, {1, 0}}
25

22
— is a relation number with a list {{27, 22}, {135, 44}, {1, 0}}
27

22
— is a relation number with a list
29
  {{29, 22}, {203, 22}, {145, -22}, {261, 44}, {87, -22}, {1, 0}}

22
— is a relation number with a list
31
  {{31, 22}, {279, 88}, {465, 88}, {775, -22}, {155, -22}, {1, 0}}

22
— is a relation number with a list {{35, 44}, {315, 44}, {1, 0}}
35

22
— is a relation number with a list
37
  {{37, 44}, {259, 66}, {185, -22}, {333, -22}, {111, -22}, {1, 0}}

22
— is a relation number with a list
39
  {{39, 44}, {195, 44}, {741, 44}, {273, -22}, {117, -22}, {91, 22}, {1, 0}}

22
— is a relation number with a list
41
  {{41, 44}, {123, -22}, {369, -88}, {697, 132}, {1517, -286}, {3567, -242}, {2583, 220},
  {2337, -242}, {3403, 792}, {9635, 1452}, {21689, -1342}, {8897, 2266}, {6847, -1056},
  {20951, 1672}, {32185, 528}, {943, 110}, {1927, -374}, {2337, -286}, {2009, 132},
  {1189, 308}, {1763, -330}, {4633, -1100}, {9553, 1034}, {10127, -1078}, {17425, 2552},
  {17999, 1606}, {13653, -88}, {533, 110}, {697, -22}, {287, -22}, {1, 0}}

22
— is a relation number with a list {{43, 44}, {1, 0}}
43

```

```

22
— is a relation number with a list {{45, 44}, {1, 0}}
45

22
— is a relation number with a list {{47, 44}, {141, 22},
47
{423, 44}, {799, 176}, {3807, 638}, {987, 44}, {893, -22}, {423, 44}}

22
— is a relation number with a list {{49, 44}, {245, -44}, {931, 66}, {1, 0}}
49

22
— is a relation number with a list {{51, 44}, {119, -22}, {153, 22}, {1, 0}}
51

22
— is a relation number with a list
53
{{53, 44}, {477, -44}, {371, 22}, {159, 22}, {265, -44}, {1, 0}}

22
— is a relation number with a list {{57, 66}, {1, 0}}
57

22
— is a relation number with a list
59
{{59, 66}, {413, -44}, {1003, 22}, {531, 88}, {177, -22}, {1, 0}}

22
— is a relation number with a list
61
{{61, 66}, {305, 44}, {183, 22}, {427, -44}, {793, 110}, {1403, 132}, {2989, -506},
{2867, -154}, {3599, 308}, {5917, 418}, {3965, -242}, {5673, -440},
{2867, -44}, {427, -66}, {1891, 66}, {1403, 22}, {305, -22}, {183, 22}}

22
— is a relation number with a list {{63, 66}, {1, 0}}
63

22
— is a relation number with a list {{65, 66}, {1, 0}}
65

22
— is a relation number with a list {{67, 66}, {1, 0}}
67

22
— is a relation number with a list {{69, 66}, {1, 0}}
69

22
— is a relation number with a list
71
{{71, 66}, {355, -44}, {213, -22}, {497, 22}, {639, 22}, {1, 0}}

22
— is a relation number with a list
73
{{73, 66}, {511, 44}, {1241, 154}, {657, -44}, {219, -22}, {1, 0}}

22
— is a relation number with a list {{75, 66}, {1, 0}}
75

22
— is a relation number with a list
79
{{79, 88}, {711, -22}, {553, -44}, {1501, 132}, {3871, -352}, {1, 0}}

22
— is a relation number with a list {{81, 88}, {567, -44}, {405, 44}, {1, 0}}
81

```

```

22
83 is a relation number with a list
  {{83, 88}, {415, -44}, {1577, 110}, {3071, 176}, {6557, 704}, {18343, 88},
  {3237, -418}, {8881, -616}, {21331, -242}, {2905, -66}, {1, 0}}

22
85 is a relation number with a list
  {{85, 88}, {255, -22}, {765, 88}, {2295, 242}, {9945, -22}, {1, 0}}

22
87 is a relation number with a list {{87, 88}, {1, 0}}

22
89 is a relation number with a list {{89, 88}, {1, 0}}

22
91 is a relation number with a list {{91, 88}, {273, 22}, {819, 22}, {455, 22}, {1, 0}}

22
93 is a relation number with a list
  {{93, 88}, {465, 44}, {1767, 88}, {651, 22}, {279, -22}, {651, 44}, {279, 22}}

22
95 is a relation number with a list {{95, 88}, {665, 44}, {1, 0}}

22
97 is a relation number with a list
  {{97, 88}, {873, 22}, {679, 22}, {291, -22}, {485, -44}, {1, 0}}

22
101 is a relation number with a list
  {{101, 110}, {909, -22}, {707, -66}, {1919, -22}, {505, -22}, {1, 0}}

22
103 is a relation number with a list
  {{103, 110}, {721, 66}, {515, 22}, {927, 88}, {4223, -44}, {1, 0}}

22
105 is a relation number with a list {{105, 110}, {1, 0}}

22
107 is a relation number with a list
  {{107, 110}, {321, -22}, {963, -22}, {535, 44}, {749, -66}, {2461, 22}, {321, 22}}

22
109 is a relation number with a list {{109, 110}, {1, 0}}

22
111 is a relation number with a list {{111, 110}, {1, 0}}

22
113 is a relation number with a list
  {{113, 110}, {339, 22}, {1017, -88}, {4407, -352}, {19097, -1122},
  {2599, 220}, {4633, 396}, {13447, -242}, {11865, -374}, {11639, -792},
  {27233, -638}, {22713, 1342}, {11413, -550}, {15481, -1144}, {60455, -198},
  {7345, 506}, {27685, 2112}, {25877, 1870}, {34239, 2002}, {23165, 726},
  {7571, 506}, {2147, 88}, {3955, -66}, {565, -22}, {791, 22}, {1, 0}}

22
115 is a relation number with a list {{115, 110}, {1, 0}}

```

```

22
117 is a relation number with a list {{117, 110}, {273, -22}, {1, 0}}

22
119 is a relation number with a list {{119, 110}, {1071, 22}, {1, 0}}

22
123 is a relation number with a list {{123, 132}, {1, 0}}

22
125 is a relation number with a list {{125, 132}, {875, -22}, {1, 0}}

22
127 is a relation number with a list
{{127, 132}, {635, -44}, {2413, -154}, {6477, 484}, {23495, 418},
{11049, -506}, {10541, 352}, {2413, 22}, {889, -22}, {1143, -22}, {1, 0}}

22
129 is a relation number with a list {{129, 132}, {1, 0}}

22
131 is a relation number with a list {{131, 132}, {1, 0}}

22
133 is a relation number with a list {{133, 132}, {1, 0}}

22
135 is a relation number with a list {{135, 132}, {1, 0}}

22
137 is a relation number with a list
{{137, 132}, {685, 44}, {2603, -176}, {5069, -308}, {19317, 1232},
{54115, -3674}, {136315, -132}, {5617, 44}, {2055, -88}, {4247, 220},
{9179, 660}, {8357, -506}, {33565, -748}, {13015, 66}, {1781, -110},
{2877, 176}, {8357, -44}, {411, 22}, {959, 66}, {4247, -176}, {3151, 176},
{2329, -176}, {5617, 242}, {6987, -506}, {13289, 1034}, {20961, -286},
{11371, -836}, {45621, -2684}, {959, -44}, {1233, 88}, {1, 0}}

22
139 is a relation number with a list
{{139, 132}, {973, 22}, {695, -22}, {1251, 88}, {2641, 110}, {1, 0}}

22
141 is a relation number with a list {{141, 132}, {1, 0}}

22
145 is a relation number with a list {{145, 154}, {1305, 44}, {435, -22}, {1, 0}}

22
147 is a relation number with a list {{147, 154}, {1, 0}}

22
149 is a relation number with a list
{{149, 154}, {745, 44}, {447, -22}, {1043, -44}, {1937, -22}, {1, 0}}

22
151 is a relation number with a list
{{151, 154}, {453, -22}, {1359, -44}, {755, 44}, {1057, 22}, {1, 0}}

22
153 is a relation number with a list {{153, 154}, {1, 0}}

```

```

22
155 is a relation number with a list {{155, 154}, {1, 0}}

22
157 is a relation number with a list
{{157, 154}, {471, 22}, {1413, 88}, {785, -44}, {1099, -22}, {1, 0}}

22
159 is a relation number with a list {{159, 154}, {795, -44}, {1, 0}}

22
161 is a relation number with a list {{161, 154}, {1, 0}}

22
163 is a relation number with a list
{{163, 154}, {1467, -44}, {2445, 88}, {3097, -132}, {9943, -44}, {1, 0}}

22
167 is a relation number with a list
{{167, 176}, {1503, -88}, {1169, -66}, {3173, 154}, {10187, -220},
{11189, 110}, {5177, 44}, {2505, -88}, {6847, -264}, {2839, -44},
{3507, -44}, {2171, -88}, {4843, 22}, {501, -22}, {835, 44}, {1, 0}}

22
169 is a relation number with a list
{{169, 176}, {1183, -22}, {845, -22}, {1521, 44}, {3211, 88}, {7267, -264},
{21125, 616}, {2353, 44}, {3549, 44}, {2535, 154}, {11999, -528},
{24505, -88}, {6929, -440}, {18759, 1100}, {767, 22}, {507, -22}, {1, 0}}

22
171 is a relation number with a list {{171, 176}, {855, 44}, {1, 0}}

22
173 is a relation number with a list
{{173, 176}, {519, -22}, {1557, 44}, {2941, 132}, {6401, 44}, {3633, 220},
{18511, -396}, {17473, -374}, {18165, 22}, {1211, 44}, {3633, -220}}

22
175 is a relation number with a list {{175, 176}, {1, 0}}

22
177 is a relation number with a list {{177, 176}, {1, 0}}

22
179 is a relation number with a list
{{179, 176}, {537, 22}, {1611, -22}, {895, 22}, {1253, 66}, {1, 0}}

22
181 is a relation number with a list
{{181, 176}, {905, -44}, {3439, 22}, {1267, -22}, {1629, 22}, {1, 0}}

22
183 is a relation number with a list
{{183, 176}, {1281, 22}, {915, -44}, {549, -22}, {1, 0}}

22
185 is a relation number with a list
{{185, 176}, {1665, 88}, {1295, 44}, {3515, 198}, {9065, 22}, {1, 0}}

22
189 is a relation number with a list {{189, 198}, {1, 0}}

```

```

22
191 is a relation number with a list
    {{191, 198}, {1337, 66}, {3247, -110}, {10123, 22}, {573, -22}, {1, 0}}

22
193 is a relation number with a list
    {{193, 198}, {965, -44}, {579, -22}, {1351, 66}, {5983, -220},
    {8299, 110}, {9457, -330}, {21809, -946}, {9843, 308}, {2509, 44}, {1, 0}}

22
195 is a relation number with a list {{195, 198}, {1, 0}}

22
197 is a relation number with a list {{197, 198}, {1, 0}}

22
199 is a relation number with a list {{199, 198}, {1, 0}}

22
201 is a relation number with a list {{201, 198}, {1, 0}}

22
203 is a relation number with a list {{203, 198}, {1015, 44}, {609, 22}, {1, 0}}

22
205 is a relation number with a list {{205, 198}, {1435, -66},
    {3485, 66}, {2665, -88}, {1025, 22}, {1845, 44}, {615, 22}, {1, 0}}

22
207 is a relation number with a list {{207, 198}, {1, 0}}

22
211 is a relation number with a list
    {{211, 220}, {1899, -88}, {7807, -154}, {9917, 440}, {42833, 946}, {55493, 2882},
    {155085, -6358}, {526023, -25234}, {821001, 17050}, {548811, -7436}, {306583, 2662},
    {95583, 3586}, {261429, 6578}, {356801, -11484}, {168167, -3432}, {1, 0}}

22
213 is a relation number with a list
    {{213, 220}, {1491, -44}, {1065, 22}, {639, -22}, {1, 0}}

22
215 is a relation number with a list {{215, 220}, {1, 0}}

22
217 is a relation number with a list
    {{217, 220}, {651, -22}, {1953, 22}, {1085, -44}, {3255, -22}, {1, 0}}

22
219 is a relation number with a list {{219, 220}, {1, 0}}

known cases
known cases
known cases
known cases

```

$\frac{23}{6}$  is a relation number with a list  
 $\{\{6, 23\}, \{102, 253\}, \{906, 1955\}, \{6294, 12\,397\}, \{36\,618, 65\,987\}, \{176\,214, 279\,565\},$   
 $\{620\,106, 699\,683\}, \{238\,731, -268\,778\}, \{90\,141, 115\,253\}, \{75\,336, -56\,971\},$   
 $\{110\,190, 80\,569\}, \{177\,726, -197\,869\}, \{40\,286, -67\,551\}, \{163\,590, -221\,789\},$   
 $\{349\,194, -78\,43\}, \{7482, -12\,995\}, \{33\,078, -48\,829\}, \{94\,506, -69\,299\},$   
 $\{151\,242, 163\,967\}, \{25\,450, -35\,259\}, \{58\,854, -14\,053\}, \{3963, -5888\}, \{11\,550, -8947\},$   
 $\{15\,618, 6187\}, \{5886, 10\,189\}, \{25\,818, 37\,835\}, \{72\,102, 49\,381\}, \{136\,326, -226\,297\},$   
 $\{539\,826, -711\,551\}, \{1\,030\,350, 319\,631\}, \{47\,638, 30\,475\}, \{39\,936, 61\,663\},$   
 $\{130\,362, 129\,743\}, \{3714, -4577\}, \{5178, 7613\}, \{14\,610, 10\,327\}, \{25\,698, -36\,547\},$   
 $\{65\,094, -30\,245\}, \{13\,812, 15\,157\}, \{2690, 621\}, \{309, -253\}, \{168, -115\}, \{318, 529\},$   
 $\{1266, 1679\}, \{2478, -575\}, \{267, 161\}, \{330, 299\}, \{62, -115\}, \{318, -529\}\}$

$\frac{23}{7}$  is a relation number with a list  
 $\{\{7, 23\}, \{112, 207\}, \{665, 736\}, \{497, -253\}, \{63, -92\}, \{203, -23\}, \{28, -23\},$   
 $\{35, -46\}, \{77, 69\}, \{56, -69\}, \{91, -115\}, \{168, 253\}, \{595, 184\}, \{301, 299\}, \{14, 23\},$   
 $\{63, 46\}, \{119, -69\}, \{133, 46\}, \{35, 23\}, \{77, 92\}, \{105, 46\}, \{91, 23\}, \{1, 0\}\}$

$\frac{23}{8}$  is a relation number with a list  
 $\{\{8, 23\}, \{120, 161\}, \{328, -345\}, \{136, 23\}, \{1, 0\}\}$

$\frac{23}{9}$  is a relation number with a list  
 $\{\{9, 23\}, \{126, 115\}, \{99, 23\}, \{63, 46\}, \{153, 23\}, \{72, -23\}, \{1, 0\}\}$

$\frac{23}{10}$  is a relation number with a list  
 $\{\{10, 23\}, \{130, 69\}, \{40, 23\}, \{30, 23\}, \{70, 69\}, \{1, 0\}\}$

$\frac{23}{11}$  is a relation number with a list  $\{\{11, 23\}, \{132, 23\}, \{66, 23\},$   
 $\{33, 23\}, \{110, 23\}, \{55, -23\}, \{99, -46\}, \{77, -23\}, \{88, -69\}, \{209, 115\},$   
 $\{231, 184\}, \{517, -138\}, \{385, -92\}, \{187, 161\}, \{286, -23\}, \{110, -23\}\}$

$\frac{23}{12}$  is a relation number with a list  $\{\{12, 23\}, \{132, -23\}, \{1, 0\}\}$

$\frac{23}{13}$  is a relation number with a list  $\{\{13, 23\}, \{130, -69\}, \{104, -23\}, \{143, 46\},$   
 $\{65, 23\}, \{52, -23\}, \{78, -23\}, \{117, -92\}, \{325, -46\}, \{39, 23\}, \{91, 23\}, \{1, 0\}\}$

$\frac{23}{14}$  is a relation number with a list  
 $\{\{14, 23\}, \{63, 46\}, \{119, -69\}, \{133, 46\}, \{35, 23\}, \{154, -69\}, \{112, 69\},$   
 $\{182, 115\}, \{336, -253\}, \{581, 138\}, \{406, -69\}, \{56, 23\}, \{35, 23\}\}$

$\frac{23}{15}$  is a relation number with a list  $\{\{15, 23\}, \{120, 23\}, \{1, 0\}\}$

$\frac{23}{16}$  is a relation number with a list  $\{\{16, 23\}, \{56, -23\}, \{40, 23\}, \{48, 23\}, \{1, 0\}\}$

$\frac{23}{17}$  is a relation number with a list  $\{\{17, 23\}, \{102, 23\}, \{170, -69\}, \{544, 299\},$   
 $\{918, -115\}, \{34, 23\}, \{187, -115\}, \{731, -23\}, \{85, 46\}, \{119, 23\}, \{68, 23\}, \{1, 0\}\}$



```

23
— is a relation number with a list {{18, 23}, {45, 23}, {1, 0}}
18
23
— is a relation number with a list {{19, 23}, {76, 23}, {133, -46}, {95, -46},
19
{57, 23}, {209, -69}, {38, 23}, {152, -69}, {266, -23}, {190, -23}, {114, -23}, {1, 0}}
23
— is a relation number with a list {{20, 23}, {60, 23}, {90, -23}, {1, 0}}
20
23
— is a relation number with a list
21
{{21, 23}, {42, 23}, {84, -23}, {56, -23}, {210, -23}, {1, 0}}
23
— is a relation number with a list {{22, 23}, {1, 0}}
22
23
— is a relation number with a list {{24, 23}, {1, 0}}
24
23
— is a relation number with a list {{25, 23}, {50, 23}, {100, 23}, {200, 23},
25
{175, 69}, {800, -253}, {1025, 276}, {1975, 368}, {675, -23}, {200, -23}}
23
— is a relation number with a list {{26, 23}, {78, -23}, {234, 23}, {52, 23}, {78, 23}}
26
23
— is a relation number with a list
27
{{27, 23}, {108, -23}, {189, -23}, {135, -46}, {1, 0}}
23
— is a relation number with a list {{28, 23}, {70, -23}, {1, 0}}
28
23
— is a relation number with a list
29
{{29, 23}, {174, -23}, {290, -23}, {261, 46}, {435, 46}, {609, -115},
{986, -207}, {1421, 368}, {1479, -115}, {464, 23}, {116, 23}, {1, 0}}
23
— is a relation number with a list {{30, 23}, {105, 23}, {1, 0}}
30
23
— is a relation number with a list
31
{{31, 23}, {248, -23}, {155, 23}, {186, -23}, {62, 23}, {217, -69},
{310, -69}, {1054, 207}, {589, -138}, {1147, -23}, {93, 23}, {1, 0}}
23
— is a relation number with a list {{32, 23}, {72, -23}, {96, 23}, {1, 0}}
32
23
— is a relation number with a list
33
{{33, 23}, {110, 23}, {165, 46}, {209, -69}, {66, 23}, {1, 0}}
23
— is a relation number with a list
34
{{34, 23}, {374, 23}, {102, -23}, {85, -23}, {238, -23}, {136, -23}, {1, 0}}
23
— is a relation number with a list
35
{{35, 46}, {385, -92}, {595, -92}, {1505, -253}, {91, -23}, {1, 0}}

```

```

23
36 is a relation number with a list {{36, 46}, {180, -23}, {1, 0}}

23
37 is a relation number with a list
    {{37, 46}, {333, -46}, {407, 69}, {259, 23}, {222, 23}, {296, 69}, {740, -207},
    {3256, -437}, {7289, 1955}, {19 647, 943}, {5772, 989}, {5994, 667}, {333, -46}}

23
38 is a relation number with a list
    {{38, 46}, {76, 23}, {266, 69}, {95, -23}, {114, 23}, {1, 0}}

23
39 is a relation number with a list {{39, 46}, {273, -23}, {1, 0}}

23
40 is a relation number with a list {{40, 46}, {120, -23}, {1, 0}}

23
41 is a relation number with a list {{41, 46}, {205, -46}, {861, 46},
    {533, -92}, {779, -161}, {1066, 23}, {328, 23}, {246, -23}, {287, -23},
    {451, 69}, {1312, 115}, {1927, 391}, {1148, 69}, {1025, 46}, {533, 92}}

23
42 is a relation number with a list {{42, 46}, {1, 0}}

23
43 is a relation number with a list
    {{43, 46}, {129, 23}, {387, 46}, {817, -207}, {473, 46}, {559, -115},
    {688, 161}, {1892, -161}, {1720, -437}, {1204, 115}, {2322, -23}, {1, 0}}

23
44 is a relation number with a list {{44, 46}, {1, 0}}

23
45 is a relation number with a list {{45, 46}, {1, 0}}

23
47 is a relation number with a list {{47, 46}, {1, 0}}

23
48 is a relation number with a list {{48, 46}, {1, 0}}

23
49 is a relation number with a list
    {{49, 46}, {147, -23}, {441, -92}, {931, 138}, {245, -46}, {105, 23}, {490, 23}, {1, 0}}

23
50 is a relation number with a list {{50, 46}, {1, 0}}

23
51 is a relation number with a list {{51, 46}, {255, 46}, {357, 23},
    {561, 92}, {153, -23}, {136, 23}, {102, 23}, {510, 23}, {204, -23}, {1, 0}}

23
52 is a relation number with a list {{52, 46}, {156, 23}, {130, -23},
    {104, 23}, {572, 69}, {260, -23}, {364, -69}, {247, -23}, {156, -23}}

23
53 is a relation number with a list
    {{53, 46}, {371, 23}, {159, -23}, {106, 23}, {477, 23}, {318, 23},
    {212, -23}, {265, 46}, {583, 92}, {1643, -115}, {1749, -23}, {1, 0}}

```

```

23
— is a relation number with a list {{54, 46}, {108, 23}, {189, 23}, {270, -23}, {1, 0}}
54

23
— is a relation number with a list {{55, 46}, {495, 46}, {1, 0}}
55

23
— is a relation number with a list {{56, 46}, {280, 23}, {1, 0}}
56

23
— is a relation number with a list {{57, 46}, {627, 92}, {969, -161}, {1, 0}}
57

23
— is a relation number with a list
58
  {{58, 69}, {319, 23}, {174, -23}, {290, -23}, {261, 46}, {435, 46},
  {609, -115}, {493, 92}, {1914, 23}, {145, -23}, {203, -23}, {116, 23}, {1, 0}}

23
— is a relation number with a list
59
  {{59, 69}, {590, 69}, {1829, 207}, {2006, 299}, {5133, 368}, {1121, 138},
  {1003, -69}, {1888, -345}, {9617, -1610}, {2537, 46}, {413, -23}, {1, 0}}

23
— is a relation number with a list {{60, 69}, {1, 0}}
60

23
— is a relation number with a list
61
  {{61, 69}, {488, 23}, {305, 23}, {366, 23}, {122, 23}, {427, -46},
  {793, -115}, {732, 115}, {2562, 253}, {1952, -23}, {183, 23}, {1, 0}}

23
— is a relation number with a list {{62, 69}, {434, 69}, {620, 69}, {1, 0}}
62

23
— is a relation number with a list {{63, 69}, {126, 23}, {231, -23}, {1, 0}}
63

23
— is a relation number with a list {{64, 69}, {160, -23}, {1, 0}}
64

23
— is a relation number with a list {{65, 69}, {260, 23}, {455, 46}, {1, 0}}
65

23
— is a relation number with a list {{66, 69}, {1, 0}}
66

23
— is a relation number with a list
67
  {{67, 69}, {134, 23}, {268, 23}, {536, -69}, {1072, -161}, {3685, -598},
  {6499, 92}, {2211, -92}, {201, -23}, {402, 23}, {737, 23}, {1, 0}}

23
— is a relation number with a list {{68, 69}, {1, 0}}
68

23
— is a relation number with a list {{70, 69}, {1, 0}}
70

23
— is a relation number with a list
71
  {{71, 69}, {142, 23}, {284, -23}, {568, 23}, {497, -23}, {639, -23}, {355, 23},
  {710, 23}, {213, 23}, {426, -23}, {781, 115}, {1704, 115}, {1491, 46},
  {1349, 207}, {7100, -897}, {5396, 759}, {5893, 437}, {15052, 1771},
  {62764, 3749}, {68799, 1265}, {34719, -161}, {4047, -368}, {1, 0}}

```

```

23
— is a relation number with a list {{72, 69}, {1, 0}}
72

23
— is a relation number with a list
73
  {{73, 69}, {292, -23}, {511, 69}, {2044, -115}, {1898, 23}, {803, 92},
  {1825, 184}, {1095, 23}, {657, -23}, {730, 69}, {2117, 299}, {1752, -253},
  {1387, 115}, {511, 23}, {365, -46}, {219, -23}, {803, -92}}

23
— is a relation number with a list {{74, 69}, {185, 23}, {1, 0}}
74

23
— is a relation number with a list {{75, 69}, {150, 23}, {825, 46}, {1, 0}}
75

23
— is a relation number with a list
76
  {{76, 69}, {532, -69}, {190, 23}, {228, -23}, {1, 0}}

23
— is a relation number with a list
77
  {{77, 69}, {616, -23}, {385, 46}, {1309, 23}, {154, 23}, {1, 0}}

23
— is a relation number with a list {{78, 69}, {1, 0}}
78

23
— is a relation number with a list
79
  {{79, 69}, {790, -69}, {2449, 253}, {6399, 506}, {14141, 1196}, {16669, -2277},
  {57670, 4807}, {1106, -115}, {3476, -23}, {237, -23}, {553, -46}, {1, 0}}

23
— is a relation number with a list {{80, 69}, {440, -23}, {240, 23}, {1, 0}}
80

23
— is a relation number with a list {{81, 92}, {891, -115}, {2349, -23}, {1, 0}}
81

23
— is a relation number with a list
82
  {{82, 92}, {410, 23}, {164, 23}, {246, 23}, {287, 23}, {902, 115}, {369, 23}, {1, 0}}

23
— is a relation number with a list
83
  {{83, 92}, {747, 23}, {913, -115}, {581, 46}, {1411, 92}, {2573, -207},
  {7387, -805}, {11786, -1495}, {14442, 23}, {166, 23}, {415, -46}, {1, 0}}

23
— is a relation number with a list {{84, 92}, {1, 0}}
84

23
— is a relation number with a list {{85, 92}, {595, 69}, {442, 23}, {1, 0}}
85

23
— is a relation number with a list
86
  {{86, 92}, {258, -23}, {430, -23}, {301, 23}, {1, 0}}

23
— is a relation number with a list {{87, 92}, {435, 46}, {609, 46},
87
  {957, -46}, {261, 23}, {696, -23}, {174, 23}, {290, 23}, {261, 23}}

23
— is a relation number with a list {{88, 92}, {1, 0}}
88

```

```

23
— is a relation number with a list
89
  {{89, 92}, {267, 23}, {801, 23}, {356, -23}, {979, -23}, {890, -23},
  {623, -46}, {1869, 230}, {2581, -207}, {8633, -575}, {712, -23}, {1, 0}}

23
— is a relation number with a list {{90, 92}, {1, 0}}
90

23
— is a relation number with a list {{91, 92}, {1, 0}}
91

23
— is a relation number with a list {{93, 92}, {1, 0}}
93

23
— is a relation number with a list {{94, 92}, {1, 0}}
94

23
— is a relation number with a list
95
  {{95, 92}, {285, -23}, {855, 92}, {2565, 46}, {1045, -69}, {190, 23}, {570, -23}, {1, 0}}

23
— is a relation number with a list {{96, 92}, {1, 0}}
96

23
— is a relation number with a list
97
  {{97, 92}, {485, -46}, {2037, 115}, {3201, 230}, {1843, -23}, {291, -23},
  {776, 23}, {582, -23}, {679, 23}, {1067, 46}, {873, -92}, {4365, 391},
  {6208, -345}, {194, 23}, {970, -69}, {388, 23}, {291, -23}}

23
— is a relation number with a list {{98, 92}, {294, 23}, {245, 23}, {392, -23}, {1, 0}}
98

23
— is a relation number with a list {{99, 92}, {231, -23}, {1, 0}}
99

23
— is a relation number with a list {{100, 92}, {1, 0}}
100

23
— is a relation number with a list
101
  {{101, 92}, {909, -23}, {1111, 46}, {707, -23}, {606, -23}, {808, 69},
  {2020, -69}, {1919, 23}, {1010, 23}, {202, 23}, {505, -23}, {1, 0}}

23
— is a relation number with a list {{102, 92}, {510, -23}, {204, 23}, {1, 0}}
102

23
— is a relation number with a list
103
  {{103, 92}, {1133, 115}, {1751, -115}, {2678, 115}, {3399, -299}, {11330, -437},
  {3296, 115}, {4017, -184}, {3193, -299}, {9888, -115}, {206, 23}, {1, 0}}

23
— is a relation number with a list
104
  {{104, 115}, {1144, -69}, {3016, -161}, {4472, -69}, {1, 0}}

23
— is a relation number with a list {{105, 115}, {210, 23}, {1, 0}}
105

23
— is a relation number with a list
106
  {{106, 115}, {954, 23}, {583, -46}, {795, 23}, {265, 23}, {583, 46}}

```

```

23
107 is a relation number with a list
{{107, 115}, {856, 23}, {535, 46}, {1819, 161}, {5136, -437}, {11556, -437},
{20758, -2139}, {67624, -3703}, {103790, 5359}, {210683, -15318},
{403283, -8027}, {206831, -14168}, {608723, -54188}, {1354085, 23184},
{1007191, 99199}, {1626507, 125603}, {677524, -41009}, {2100303, -126707},
{5747612, -32499}, {504077, 10097}, {82711, 4140}, {9523, -828},
{44191, 3105}, {77147, 575}, {10379, -943}, {642, -23}, {214, 23}, {749, 46},
{1391, 138}, {1177, 92}, {2033, 207}, {3959, -23}, {321, 23}, {1, 0}}

23
108 is a relation number with a list {{108, 115}, {756, -23}, {1, 0}}

23
109 is a relation number with a list
{{109, 115}, {654, 23}, {1090, -23}, {981, -23}, {872, -69}, {2725, 46},
{1199, -46}, {327, 23}, {545, -23}, {763, -69}, {436, 23}, {1, 0}}

23
110 is a relation number with a list {{110, 115}, {1, 0}}

23
111 is a relation number with a list
{{111, 115}, {444, 23}, {777, -23}, {555, 23}, {1, 0}}

23
112 is a relation number with a list {{112, 115}, {336, 23}, {252, -23}, {1, 0}}

23
113 is a relation number with a list
{{113, 115}, {226, 23}, {452, -23}, {904, 23}, {791, 23}, {1017, -92}, {565, -46},
{1469, -115}, {2938, -161}, {4520, 207}, {3842, 69}, {2486, -207}, {226, 23}}

23
114 is a relation number with a list {{114, 115}, {1, 0}}

23
116 is a relation number with a list {{116, 115}, {1, 0}}

23
117 is a relation number with a list
{{117, 115}, {234, 23}, {468, 23}, {312, -23}, {390, -23}, {1, 0}}

23
118 is a relation number with a list
{{118, 115}, {354, -23}, {1062, -23}, {236, 23}, {354, -23}}

23
119 is a relation number with a list {{119, 115}, {476, -23}, {1, 0}}

23
120 is a relation number with a list {{120, 115}, {1, 0}}

23
121 is a relation number with a list
{{121, 115}, {726, -23}, {1210, 23}, {1089, -92}, {1815, 92},
{3025, -207}, {9680, -713}, {36542, 2921}, {15741, 782}, {12221, -621},
{24079, 1909}, {89298, 6647}, {349327, 7475}, {241758, 14605},
{789767, 34247}, {252406, 17779}, {423500, -22241}, {111441, -920}, {1, 0}}

```

```

23
122 is a relation number with a list {{122, 115}, {854, 23}, {366, -23}, {1, 0}}

23
123 is a relation number with a list {{123, 115}, {984, -23}, {615, -46},
    {2091, -184}, {2747, 161}, {1230, 23}, {1353, 46}, {2337, -23}, {369, -23}, {1, 0}}

23
124 is a relation number with a list
    {{124, 115}, {1116, -23}, {1364, 69}, {496, -23}, {310, 23}, {1364, 69}}

23
125 is a relation number with a list
    {{125, 115}, {250, 23}, {375, 23}, {875, -23}, {1, 0}}

23
126 is a relation number with a list {{126, 115}, {462, 23}, {1, 0}}

23
127 is a relation number with a list
    {{127, 138}, {1397, -69}, {2159, -161}, {8382, -713}, {22098, -1495}, {41529, 1840},
    {100457, 2829}, {176149, -8372}, {42799, -1357}, {79375, -161}, {254, 23}, {1, 0}}

23
128 is a relation number with a list {{128, 138}, {640, 23}, {1, 0}}

23
129 is a relation number with a list {{129, 138}, {1, 0}}

23
130 is a relation number with a list {{130, 138}, {260, 23}, {910, -69}, {1, 0}}

23
131 is a relation number with a list
    {{131, 138}, {917, -46}, {393, 23}, {262, 23}, {1179, -92}, {2227, -69}, {2489, 138},
    {655, 23}, {1441, -23}, {1048, 69}, {1703, 69}, {2882, 69}, {2096, 161}, {393, -23}}

23
132 is a relation number with a list {{132, 138}, {1, 0}}

23
133 is a relation number with a list
    {{133, 138}, {665, 46}, {399, -23}, {1064, 69}, {551, -23}, {1, 0}}

23
134 is a relation number with a list {{134, 138}, {1, 0}}

23
135 is a relation number with a list {{135, 138}, {1, 0}}

23
136 is a relation number with a list {{136, 138}, {1, 0}}

23
137 is a relation number with a list {{137, 138}, {1, 0}}

23
139 is a relation number with a list {{139, 138}, {1, 0}}

23
140 is a relation number with a list {{140, 138}, {1, 0}}

23
141 is a relation number with a list {{141, 138}, {1, 0}}

```

```

23
142 is a relation number with a list {{142, 138}, {1, 0}}

23
143 is a relation number with a list {{143, 138}, {715, -46}, {3003, -184},
    {8437, -529}, {3861, -115}, {7007, -460}, {15301, 667}, {440, 23},
    {429, -23}, {1144, -23}, {858, -23}, {1001, -69}, {374, -23}, {858, 23}}

23
144 is a relation number with a list {{144, 138}, {1, 0}}

23
145 is a relation number with a list {{145, 138}, {1015, 46},
    {435, -23}, {290, 23}, {1305, -23}, {870, 23}, {580, -23}, {1, 0}}

23
146 is a relation number with a list
    {{146, 138}, {292, 23}, {1022, 23}, {365, -23}, {438, -23}, {1, 0}}

23
147 is a relation number with a list {{147, 138}, {1, 0}}

23
148 is a relation number with a list {{148, 138}, {740, -23}, {1, 0}}

23
149 is a relation number with a list
    {{149, 138}, {1639, 69}, {2533, -115}, {447, -23}, {1490, 23}, {745, 23},
    {1341, -92}, {5811, 253}, {1192, 23}, {596, -23}, {298, 23}, {1, 0}}

23
150 is a relation number with a list {{150, 161}, {330, -23}, {600, 23}, {1, 0}}

23
151 is a relation number with a list
    {{151, 161}, {1510, 69}, {1208, 69}, {5134, -253}, {11174, -759}, {31861, -1863},
    {28690, -1633}, {106304, 3703}, {163533, -11155}, {572592, 27301}, {110079, 2231},
    {114760, 4761}, {74896, 207}, {5738, 207}, {8758, -575}, {20083, -1173},
    {21442, -759}, {28690, -989}, {1359, -92}, {3171, -115}, {7399, 460}, {5889, 391},
    {3624, -23}, {1510, 23}, {1208, 23}, {1661, 69}, {755, -46}, {2869, 46},
    {2567, -92}, {1359, 23}, {302, 23}, {453, 23}, {1057, 69}, {3322, -207}, {1510, 23}}

23
152 is a relation number with a list {{152, 161}, {684, -23}, {456, 23}, {1, 0}}

23
153 is a relation number with a list {{153, 161}, {1224, 23}, {765, -46}, {1, 0}}

23
154 is a relation number with a list {{154, 161}, {1, 0}}

23
155 is a relation number with a list
    {{155, 161}, {930, 23}, {310, 23}, {1705, 23}, {465, -23}, {1, 0}}

23
156 is a relation number with a list {{156, 161}, {390, -23}, {1, 0}}

23
157 is a relation number with a list
    {{157, 161}, {628, 23}, {1099, 69}, {785, -23}, {471, -23}, {1727, -69},
    {314, 23}, {1256, 69}, {2198, -115}, {2041, -115}, {4553, 46}, {1, 0}}

```



```

23
158 is a relation number with a list
    {{158, 161}, {474, 23}, {711, 46}, {3318, 23}, {474, 23}}

23
159 is a relation number with a list
    {{159, 161}, {318, 23}, {636, 23}, {1272, 23}, {1113, -46}, {477, -23}, {318, 23}}

23
160 is a relation number with a list {{160, 161}, {1, 0}}

23
162 is a relation number with a list {{162, 161}, {1, 0}}

23
163 is a relation number with a list
    {{163, 161}, {326, 23}, {652, -23}, {1304, -69}, {1141, -23}, {1467, 23},
    {815, 46}, {2119, -23}, {489, -23}, {978, -23}, {1793, -46}, {1, 0}}

23
164 is a relation number with a list {{164, 161}, {492, -23}, {738, -23}, {1, 0}}

23
165 is a relation number with a list
    {{165, 161}, {660, -23}, {385, -23}, {330, 23}, {440, -23}, {1, 0}}

23
166 is a relation number with a list {{166, 161}, {415, 23}, {1, 0}}

23
167 is a relation number with a list
    {{167, 161}, {1002, -23}, {1670, -69}, {2338, 69}, {1336, 69}, {4175, 23}, {1837, -46},
    {501, 23}, {835, -46}, {1169, 46}, {3173, -184}, {7515, 322}, {18203, 1127},
    {28557, -575}, {32231, -1633}, {71643, -3565}, {57281, -3680}, {267033, -10649},
    {134936, 5681}, {235136, -9591}, {774713, 1242}, {49265, 2921}, {65464, -943},
    {66299, -2254}, {155811, 9844}, {282731, -8510}, {317467, 21689}, {1313956, -2783},
    {63460, -1541}, {46593, -667}, {16199, -161}, {10354, -207}, {668, 23}, {1, 0}}

23
168 is a relation number with a list {{168, 161}, {1, 0}}

23
169 is a relation number with a list
    {{169, 161}, {1352, -23}, {845, -23}, {1014, 23}, {338, 23}, {1183, -23}, {1690, 23},
    {1859, 92}, {3211, -184}, {14027, -552}, {38363, 690}, {46813, -1932},
    {75205, 1012}, {53573, 3335}, {35997, 230}, {19097, 115}, {1183, -46}, {1, 0}}

23
170 is a relation number with a list
    {{170, 161}, {765, 23}, {510, 23}, {340, 23}, {1, 0}}

23
171 is a relation number with a list
    {{171, 161}, {570, -23}, {855, 23}, {684, -23}, {342, 23}, {1, 0}}

23
172 is a relation number with a list
    {{172, 161}, {1892, 115}, {1118, -69}, {1204, 23}, {344, 23}, {1, 0}}

```

$\frac{23}{173}$  is a relation number with a list  
 $\{\{173, 184\}, \{1903, 46\}, \{2941, 138\}, \{7439, 138\}, \{2249, 46\}, \{865, -23\},$   
 $\{1557, 46\}, \{1211, -69\}, \{5363, -184\}, \{4671, -161\}, \{346, 23\}, \{1, 0\}\}$

$\frac{23}{174}$  is a relation number with a list  $\{\{174, 184\}, \{870, -23\}, \{348, 23\}, \{1, 0\}\}$

$\frac{23}{175}$  is a relation number with a list  $\{\{175, 184\}, \{1575, 92\}, \{1925, -92\}, \{1, 0\}\}$

$\frac{23}{176}$  is a relation number with a list  $\{\{176, 184\}, \{1, 0\}\}$

$\frac{23}{177}$  is a relation number with a list  $\{\{177, 184\}, \{1239, -46\}, \{1, 0\}\}$

$\frac{23}{178}$  is a relation number with a list  
 $\{\{178, 184\}, \{534, -23\}, \{445, 23\}, \{712, 23\}, \{1, 0\}\}$

$\frac{23}{179}$  is a relation number with a list  $\{\{179, 184\}, \{895, -46\}, \{3759, -23\},$   
 $\{1790, 23\}, \{716, 23\}, \{537, -23\}, \{1432, -69\}, \{3043, -161\}, \{2864, 115\},$   
 $\{1969, -92\}, \{6623, -299\}, \{8055, 299\}, \{3222, -115\}, \{358, 23\}, \{1790, 23\}\}$

$\frac{23}{180}$  is a relation number with a list  $\{\{180, 184\}, \{1, 0\}\}$

$\frac{23}{181}$  is a relation number with a list  
 $\{\{181, 184\}, \{543, 23\}, \{1629, -23\}, \{724, 23\}, \{1991, 115\}, \{6516, 115\},$   
 $\{7059, -184\}, \{12127, 598\}, \{30227, 690\}, \{24073, 529\}, \{47241, 299\}, \{1, 0\}\}$

$\frac{23}{182}$  is a relation number with a list  $\{\{182, 184\}, \{1, 0\}\}$

$\frac{23}{183}$  is a relation number with a list  $\{\{183, 184\}, \{1, 0\}\}$

$\frac{23}{185}$  is a relation number with a list  $\{\{185, 184\}, \{1, 0\}\}$

$\frac{23}{186}$  is a relation number with a list  $\{\{186, 184\}, \{1, 0\}\}$

$\frac{23}{187}$  is a relation number with a list  
 $\{\{187, 184\}, \{561, -23\}, \{1683, 46\}, \{3553, 138\}, \{6545, -46\}, \{2431, 69\},$   
 $\{2992, 23\}, \{374, 23\}, \{1122, 23\}, \{935, -46\}, \{2805, 23\}, \{1, 0\}\}$

$\frac{23}{188}$  is a relation number with a list  $\{\{188, 184\}, \{1, 0\}\}$

$\frac{23}{189}$  is a relation number with a list  $\{\{189, 184\}, \{945, 46\}, \{1, 0\}\}$

$\frac{23}{190}$  is a relation number with a list  $\{\{190, 184\}, \{570, 23\}, \{1, 0\}\}$

```

23
191 is a relation number with a list
    {{191, 184}, {1337, 46}, {573, 23}, {382, 23}, {1719, -46}, {3247, -184},
    {12415, -736}, {18527, 23}, {2101, -92}, {2865, -23}, {1910, 23}, {1, 0}}

23
192 is a relation number with a list {{192, 184}, {1, 0}}

23
193 is a relation number with a list
    {{193, 184}, {1737, -92}, {2123, 46}, {1351, 23}, {1158, -23}, {1544, -23},
    {579, -23}, {772, -23}, {1930, 69}, {386, 23}, {965, 46}, {1, 0}}

23
194 is a relation number with a list {{194, 184}, {970, 23},
    {388, 23}, {582, 23}, {679, -23}, {1067, -46}, {1746, -23}, {1, 0}}

23
195 is a relation number with a list {{195, 184}, {2145, -46}, {3315, -23}, {1, 0}}

23
196 is a relation number with a list {{196, 207}, {539, -23}, {490, 23}, {1, 0}}

23
197 is a relation number with a list
    {{197, 207}, {1970, -69}, {6107, 46}, {2167, 46}, {985, -23}, {788, 23},
    {1182, -23}, {1773, 23}, {394, 23}, {591, -23}, {1379, 23}, {1, 0}}

23
198 is a relation number with a list {{198, 207}, {1, 0}}

23
199 is a relation number with a list
    {{199, 207}, {1592, 23}, {995, -23}, {1194, -23}, {398, 23}, {1393, 69},
    {2587, -23}, {2189, -23}, {796, 23}, {1791, -23}, {597, 23}, {1, 0}}

23
200 is a relation number with a list {{200, 207}, {1400, -23}, {600, -23}, {1, 0}}

23
201 is a relation number with a list {{201, 207}, {402, 23}, {737, 23}, {1, 0}}

23
202 is a relation number with a list {{202, 207}, {505, 23}, {1, 0}}

23
203 is a relation number with a list {{203, 207}, {812, 23}, {1, 0}}

23
204 is a relation number with a list {{204, 207}, {1, 0}}

23
205 is a relation number with a list
    {{205, 207}, {410, 23}, {820, -23}, {1640, -69}, {3280, 161}, {2460, -23}, {1, 0}}

23
206 is a relation number with a list {{206, 207}, {1, 0}}

23
208 is a relation number with a list {{208, 207}, {1, 0}}

```

```

23
209 is a relation number with a list {{209, 207}, {418, 23}, {836, 23}, {1672, 23},
    {1463, 23}, {1881, -46}, {1045, -46}, {2717, 46}, {627, 23}, {1254, -23}, {1, 0}}

23
210 is a relation number with a list {{210, 207}, {1, 0}}

23
211 is a relation number with a list
    {{211, 207}, {844, -23}, {1477, 23}, {1055, 23}, {633, -23}, {2321, 46},
    {4431, 46}, {3165, 46}, {1899, 23}, {2110, -23}, {1266, 23}, {1, 0}}

23
212 is a relation number with a list {{212, 207}, {530, -23}, {1, 0}}

23
213 is a relation number with a list {{213, 207}, {426, 23}, {2343, -92}, {9159, 184},
    {2911, 138}, {2769, 92}, {639, -23}, {1065, -46}, {1491, 23}, {852, -23}, {1, 0}}

23
214 is a relation number with a list {{214, 207}, {1498, 23}, {642, 23}, {1, 0}}

23
215 is a relation number with a list {{215, 207}, {1720, -23}, {1, 0}}

23
216 is a relation number with a list {{216, 207}, {1, 0}}

23
217 is a relation number with a list {{217, 207}, {2170, 69}, {1, 0}}

23
218 is a relation number with a list
    {{218, 207}, {1199, 46}, {654, 23}, {1090, -23}, {981, -23}, {872, 23}, {1, 0}}

23
219 is a relation number with a list {{219, 230}, {2409, -23}, {438, 23}, {1, 0}}

23
220 is a relation number with a list {{220, 230}, {1, 0}}

23
221 is a relation number with a list {{221, 230}, {1989, 92}, {7735, -207},
    {1292, -23}, {884, -23}, {2210, -23}, {442, 23}, {1105, 23}, {1, 0}}

23
222 is a relation number with a list
    {{222, 230}, {444, 23}, {777, -23}, {555, 23}, {1, 0}}

23
223 is a relation number with a list
    {{223, 230}, {1561, 69}, {5798, 161}, {446, 23}, {2007, -46}, {3791, 92},
    {4237, -23}, {1115, 46}, {2453, -115}, {8474, -299}, {22746, -989}, {1, 0}}

23
224 is a relation number with a list {{224, 230}, {672, -23}, {1120, 23}, {1, 0}}

23
225 is a relation number with a list {{225, 230}, {1, 0}}

23
226 is a relation number with a list {{226, 230}, {1, 0}}

```

```

23
— is a relation number with a list
227
  {{227, 230}, {681, 23}, {2043, -46}, {4313, 46}, {2497, -69}, {2951, -115},
  {8853, 92}, {4767, 115}, {11804, -207}, {1135, 46}, {3405, -92}, {1, 0}}

23
— is a relation number with a list {{228, 230}, {1, 0}}
228

23
— is a relation number with a list {{229, 230}, {1, 0}}
229

known cases

24
— is a relation number with a list {{7, 24}, {119, 240},
7
  {847, 1224}, {2639, 480}, {1673, -2376}, {4921, -240}, {17, -24}, {1, 0}}

24
— is a relation number with a list {{11, 24}, {143, 48}, {1, 0}}
11

24
— is a relation number with a list {{13, 24}, {143, -48}, {1, 0}}
13

24
— is a relation number with a list {{17, 24}, {119, -72}, {425, 24}, {119, -72}}
17

24
— is a relation number with a list {{19, 24}, {95, 24}, {1, 0}}
19

24
— is a relation number with a list {{23, 24}, {1, 0}}
23

24
— is a relation number with a list {{25, 24}, {1, 0}}
25

24
— is a relation number with a list {{29, 24}, {145, -24}, {1, 0}}
29

24
— is a relation number with a list {{31, 24}, {217, 72}, {1, 0}}
31

24
— is a relation number with a list {{35, 24}, {385, 48}, {1, 0}}
35

24
— is a relation number with a list
37
  {{37, 48}, {407, 72}, {925, -264}, {4847, 336}, {5291, -1296},
  {3959, 840}, {8917, -2160}, {10249, -144}, {925, 72}, {407, -24}, {1, 0}}

24
— is a relation number with a list {{41, 48}, {287, 48}, {1, 0}}
41

24
— is a relation number with a list {{43, 48}, {215, -24}, {1, 0}}
43

24
— is a relation number with a list {{47, 48}, {1, 0}}
47

24
— is a relation number with a list {{49, 48}, {1, 0}}
49

24
— is a relation number with a list {{53, 48}, {265, 24}, {1, 0}}
53

24
— is a relation number with a list {{55, 48}, {385, -48}, {1, 0}}
55

```

```

24
— is a relation number with a list {{59, 48}, {649, -72}, {1, 0}}
59

24
— is a relation number with a list {{61, 72}, {671, 96}, {1, 0}}
61

24
— is a relation number with a list {{65, 72}, {455, 24}, {1, 0}}
65

24
— is a relation number with a list {{67, 72}, {335, -24}, {1, 0}}
67

24
— is a relation number with a list {{71, 72}, {1, 0}}
71

24
— is a relation number with a list {{73, 72}, {1, 0}}
73

24
— is a relation number with a list {{77, 72}, {385, 24}, {1, 0}}
77

24
— is a relation number with a list {{79, 72}, {553, -24}, {1, 0}}
79

24
— is a relation number with a list {{83, 72}, {913, -96}, {3901, 72},
83    {{1079, 48}, {1909, 120}, {913, 72}, {1909, 96}, {913, -48}, {1, 0}}

24
— is a relation number with a list {{85, 96}, {935, 24}, {1, 0}}
85

24
— is a relation number with a list {{89, 96}, {623, 24}, {1, 0}}
89

24
— is a relation number with a list {{91, 96}, {455, 24}, {1, 0}}
91

24
— is a relation number with a list {{95, 96}, {1, 0}}
95

24
— is a relation number with a list {{97, 96}, {1, 0}}
97

24
— is a relation number with a list {{101, 96}, {505, -24}, {1, 0}}
101

24
— is a relation number with a list {{103, 96}, {721, -24}, {1, 0}}
103

24
— is a relation number with a list {{107, 96}, {1177, -24}, {1, 0}}
107

24
— is a relation number with a list {{109, 120}, {1199, 120}, {1, 0}}
109

24
— is a relation number with a list
113    {{113, 120}, {791, 48}, {2599, -96}, {791, 72}, {1, 0}}

24
— is a relation number with a list {{115, 120}, {1, 0}}
115

24
— is a relation number with a list {{119, 120}, {1, 0}}
119

24
— is a relation number with a list {{121, 120}, {1, 0}}
121

```

```

24
125 is a relation number with a list {{125, 120}, {1, 0}}

24
127 is a relation number with a list
{{127, 120}, {889, -48}, {2921, 24}, {889, -24}, {1, 0}}

24
131 is a relation number with a list {{131, 120}, {1441, -120}, {1, 0}}

24
133 is a relation number with a list
{{133, 144}, {1463, 120}, {3059, -48}, {1729, 144}, {1, 0}}

24
137 is a relation number with a list
{{137, 144}, {959, -72}, {3151, 72}, {2329, -72}, {3425, -264}, {959, 48}, {1, 0}}

24
139 is a relation number with a list {{139, 144}, {695, 24}, {1, 0}}

24
143 is a relation number with a list {{143, 144}, {1, 0}}

24
145 is a relation number with a list {{145, 144}, {1, 0}}

24
149 is a relation number with a list {{149, 144}, {745, -24}, {1, 0}}

24
151 is a relation number with a list
{{151, 144}, {1057, 72}, {3473, 168}, {8305, -288}, {7097, -504}, {6191, -336},
{21593, 744}, {2567, 144}, {3775, -144}, {4681, -168}, {3473, -24}, {1057, -72}}

24
155 is a relation number with a list {{155, 144}, {341, -24}, {1, 0}}

24
157 is a relation number with a list {{157, 168}, {1727, 24}, {1, 0}}

24
161 is a relation number with a list {{161, 168}, {1, 0}}

24
163 is a relation number with a list {{163, 168}, {815, -24}, {1, 0}}

24
167 is a relation number with a list {{167, 168}, {1, 0}}

24
169 is a relation number with a list {{169, 168}, {1, 0}}

24
173 is a relation number with a list {{173, 168}, {865, 24}, {1, 0}}

24
175 is a relation number with a list {{175, 168}, {1, 0}}

24
179 is a relation number with a list {{179, 168}, {1969, -24}, {1, 0}}

```

```

24
181 is a relation number with a list
    {{181, 192}, {1991, 96}, {4525, 24}, {1991, -120}, {8869, 552},
    {6697, -432}, {38915, 792}, {19367, -456}, {38915, 24}, {1991, 120}}

24
185 is a relation number with a list {{185, 192}, {1295, -72}, {1, 0}}

24
187 is a relation number with a list {{187, 192}, {935, -24}, {1, 0}}

24
191 is a relation number with a list {{191, 192}, {1, 0}}

24
193 is a relation number with a list {{193, 192}, {1, 0}}

24
197 is a relation number with a list {{197, 192}, {985, 24}, {1, 0}}

24
199 is a relation number with a list
    {{199, 192}, {1393, 72}, {4975, -72}, {1393, -48}, {1, 0}}

24
203 is a relation number with a list
    {{203, 192}, {2233, -96}, {5075, -288}, {22127, 912}, {48517, 1584},
    {119161, 2472}, {102515, 4896}, {8729, 432}, {18067, 120}, {10759, -192}, {1, 0}}

24
205 is a relation number with a list
    {{205, 216}, {2255, 72}, {4715, -144}, {7585, 216}, {1025, -24}, {1435, 48}, {1, 0}}

24
209 is a relation number with a list
    {{209, 216}, {1463, 48}, {4807, 96}, {1463, 72}, {4807, 144}, {1045, -24}, {1, 0}}

24
211 is a relation number with a list {{211, 216}, {1055, 24}, {1, 0}}

24
215 is a relation number with a list {{215, 216}, {1, 0}}

24
217 is a relation number with a list {{217, 216}, {1, 0}}

24
221 is a relation number with a list {{221, 216}, {1105, -24}, {1, 0}}

24
223 is a relation number with a list
    {{223, 216}, {1561, -48}, {5129, 216}, {12265, -648}, {10481, 120}, {9143, 192},
    {16279, -768}, {33673, -936}, {5129, 72}, {3791, 144}, {10481, 528},
    {17617, -192}, {10481, -48}, {3791, -96}, {10481, 24}, {1561, 24}, {1, 0}}

24
227 is a relation number with a list
    {{227, 216}, {2497, -72}, {5221, -216}, {8399, -192}, {11123, 72},
    {7945, 384}, {27013, 1368}, {78769, -2400}, {97837, -3432}, {383857, 7968},
    {316211, 3408}, {166391, 432}, {16117, -768}, {2497, 96}, {1, 0}}

```



```

24
229 is a relation number with a list
{{229, 240}, {2519, -48}, {5267, 48}, {2977, -72}, {5725, -288},
{8015, -408}, {33205, -528}, {13511, 552}, {60227, 168}, {19007, 624},
{65723, -1752}, {195337, -8232}, {510899, 11088}, {194879, 6576},
{549829, -7680}, {716999, 30408}, {2929597, 98304}, {4470767, -21120},
{1528117, 31920}, {925847, -32280}, {2352517, -4440}, {156407, 456}, {1, 0}}

24
233 is a relation number with a list {{233, 240}, {1631, 24}, {1, 0}}

24
235 is a relation number with a list {{235, 240}, {1, 0}}

24
239 is a relation number with a list {{239, 240}, {1, 0}}

known cases

known cases

known cases

known cases

25
7 is a relation number with a list
{{7, 25}, {126, 275}, {1043, 1800}, {5299, 6325}, {7182, 7025}, {1099, -1850},
{5257, -5825}, {3976, -1825}, {2282, 3525}, {8701, 6400}, {16107, -12725},
{23674, -4525}, {7343, -5450}, {13251, 9175}, {28532, -37675},
{64001, 35150}, {44093, 68900}, {173649, 137875}, {250418, 70775},
{228774, 321625}, {649957, 69900}, {145999, -32125}, {102382, -140775},
{268751, 25600}, {89257, -139575}, {352226, -280925}, {499107, -183950},
{369201, -30925}, {13293, -20900}, {53249, -43875}, {65618, -72775},
{50099, -27350}, {32207, -38600}, {44751, -49450}, {32893, -6275},
{10626, -5975}, {9268, 8725}, {3801, 6775}, {20818, 26925}, {42749, -35800},
{48643, -76875}, {197624, -167675}, {209643, 323725}, {798574, 585975},
{1488193, -1213150}, {1925301, -1615975}, {2165282, -3578675},
{9893751, -10284100}, {390349, 525375}, {945182, -301975}, {274799, -150975},
{190057, -300725}, {774676, -661625}, {791357, 1021175}, {1608726, -1402775},
{1441657, 478125}, {50974, 69975}, {133007, -14800}, {193, 325}, {924, 1025},
{707, 400}, {651, -475}, {1232, 1075}, {1099, -325}, {868, 825}, {301, 400},
{693, -325}, {301, -125}, {357, 400}, {301, 425}, {868, 125}, {1, 0}}

25
8 is a relation number with a list {{8, 25}, {136, 225}, {712, 425}, {552, 25}, {1, 0}}

25
9 is a relation number with a list
{{9, 25}, {144, 175}, {279, -25}, {36, -25}, {99, 50}, {1, 0}}

25
11 is a relation number with a list
{{11, 25}, {154, 75}, {44, 25}, {66, 25}, {99, -50}, {1, 0}}

25
12 is a relation number with a list {{12, 25}, {156, 25}, {1, 0}}

```

```

25
— is a relation number with a list
13
  {{13, 25}, {156, -25}, {78, -25}, {39, -25}, {143, 50}, {91, 50}, {117, 25},
  {104, 75}, {377, 250}, {1599, -175}, {312, 125}, {806, 75}, {247, -25}, {39, 25}}

25
— is a relation number with a list
14
  {{14, 25}, {154, -75}, {28, 25}, {42, -25}, {56, -25}, {42, -25}}

25
— is a relation number with a list {{16, 25}, {72, 25}, {48, -25}, {1, 0}}
16

25
— is a relation number with a list {{17, 25}, {136, -25}, {187, 125}, {1054, 575},
17
  {1632, -175}, {969, -125}, {527, -200}, {1241, -250}, {153, -25}, {51, 25}, {1, 0}}

25
— is a relation number with a list {{18, 25}, {42, 25}, {72, -25}, {1, 0}}
18

25
— is a relation number with a list
19
  {{19, 25}, {114, -25}, {209, -75}, {304, -175}, {874, -125}, {1, 0}}

25
— is a relation number with a list {{21, 25}, {84, -25}, {63, -25}, {84, -25}}
21

25
— is a relation number with a list {{22, 25}, {66, -25}, {99, 50}, {1, 0}}
22

25
— is a relation number with a list {{23, 25}, {46, 25}, {92, 25}, {184, 25},
23
  {207, -100}, {161, -25}, {253, -25}, {69, 25}, {138, 25}, {276, 25}, {1, 0}}

25
— is a relation number with a list {{24, 25}, {1, 0}}
24

25
— is a relation number with a list {{26, 25}, {1, 0}}
26

25
— is a relation number with a list {{27, 25}, {54, 25}, {108, -25}, {72, -25}, {1, 0}}
27

25
— is a relation number with a list {{28, 25}, {84, 25}, {252, 25}, {1, 0}}
28

25
— is a relation number with a list {{29, 25}, {116, 25}, {261, -50}, {319, -75},
29
  {551, 200}, {1421, 325}, {3509, 350}, {261, 25}, {319, -100}, {551, -50}, {1, 0}}

25
— is a relation number with a list
31
  {{31, 25}, {186, 25}, {341, -50}, {279, -25}, {124, 25}, {1, 0}}

25
— is a relation number with a list {{32, 25}, {224, -75}, {1, 0}}
32

25
— is a relation number with a list {{33, 25}, {264, 25}, {1, 0}}
33

25
— is a relation number with a list {{34, 25}, {153, -25}, {102, -25}, {1, 0}}
34

25
— is a relation number with a list {{36, 25}, {132, 25}, {252, 25}, {1, 0}}
36

```

```

25
37 — is a relation number with a list {{37, 25}, {444, 25}, {222, -25}, {111, 25},
    {407, 100}, {259, 25}, {333, 25}, {296, -75}, {148, -25}, {74, 25}, {1, 0}}

25
38 — is a relation number with a list {{38, 50}, {114, -25},
    {418, 125}, {817, 225}, {1577, -125}, {912, -25}, {228, -25}, {114, 25}}

25
39 — is a relation number with a list {{39, 50}, {429, -25}, {156, 25}, {78, 25}, {1, 0}}

25
41 — is a relation number with a list
    {{41, 50}, {369, -25}, {246, -25}, {164, 25}, {451, 75}, {1, 0}}

25
42 — is a relation number with a list {{42, 50}, {84, 25}, {126, -25}, {1, 0}}

25
43 — is a relation number with a list {{43, 50}, {301, -50}, {1, 0}}

25
44 — is a relation number with a list {{44, 50}, {132, 25}, {154, 25}, {1, 0}}

25
46 — is a relation number with a list {{46, 50}, {1, 0}}

25
47 — is a relation number with a list {{47, 50}, {141, -25}, {423, 50},
    {1081, 50}, {893, 25}, {329, 50}, {987, -250}, {611, 50}, {517, -125},
    {799, 75}, {1222, -275}, {5734, -725}, {3102, -575}, {10669, 1350},
    {6157, -1225}, {1504, 25}, {188, -25}, {564, -25}, {517, 75}, {376, 75}, {1, 0}}

25
48 — is a relation number with a list {{48, 50}, {1, 0}}

25
49 — is a relation number with a list {{49, 50}, {1, 0}}

25
51 — is a relation number with a list {{51, 50}, {1, 0}}

25
52 — is a relation number with a list {{52, 50}, {1, 0}}

25
53 — is a relation number with a list
    {{53, 50}, {159, 25}, {477, -25}, {106, 25}, {318, -25}, {371, -75},
    {212, -25}, {636, -125}, {583, -25}, {424, 75}, {1378, -75}, {1484, 225},
    {4823, -550}, {6731, 575}, {8957, -900}, {2279, 400}, {6413, -25}, {636, 125}}

25
54 — is a relation number with a list {{54, 50}, {1, 0}}

25
56 — is a relation number with a list {{56, 50}, {168, -25}, {1, 0}}

25
57 — is a relation number with a list {{57, 50}, {399, 50}, {1, 0}}

25
58 — is a relation number with a list
    {{58, 50}, {116, 25}, {261, -50}, {638, 125}, {377, 50}, {1334, -25}, {261, -50}}

```

```

25
— is a relation number with a list
59
  {{59, 50}, {531, 25}, {354, -25}, {236, 25}, {649, 100}, {2891, -225},
    {2006, -325}, {3304, 425}, {5664, -1075}, {17051, 1600}, {32391, 1675},
    {33394, -225}, {5546, 825}, {13511, 2850}, {43601, -1875},
    {28084, -3525}, {6844, -825}, {14396, 125}, {1239, 25}, {649, -100}}

25
— is a relation number with a list
61
  {{61, 50}, {671, 25}, {244, -25}, {366, 25}, {549, 50}, {1, 0}}

25
— is a relation number with a list
62
  {{62, 50}, {186, 25}, {341, -50}, {279, -25}, {124, 25}, {1, 0}}

25
— is a relation number with a list {{63, 75}, {252, 25}, {126, 25}, {1, 0}}
63

25
— is a relation number with a list
64
  {{64, 75}, {704, -125}, {1472, -25}, {192, 25}, {1, 0}}

25
— is a relation number with a list {{66, 75}, {1, 0}}
66

25
— is a relation number with a list {{67, 75}, {536, -25}, {737, -25}, {804, 125},
67
  {3618, 275}, {2881, 150}, {2077, -25}, {134, 25}, {603, 100}, {201, 25}, {1, 0}}

25
— is a relation number with a list {{68, 75}, {476, -25}, {1, 0}}
68

25
— is a relation number with a list {{69, 75}, {138, 25}, {276, 25}, {1, 0}}
69

25
— is a relation number with a list {{71, 75}, {284, -25}, {639, 25},
71
  {781, -125}, {2201, -350}, {7171, 400}, {2059, -125}, {4189, -25}, {781, 125}}

25
— is a relation number with a list {{72, 75}, {1, 0}}
72

25
— is a relation number with a list
73
  {{73, 75}, {146, 25}, {292, -25}, {584, 25}, {657, 25}, {511, 75}, {1022, 125},
    {1606, -225}, {2263, -150}, {949, 100}, {3577, -50}, {1679, 200}, {5767, 775},
    {24966, -3275}, {90082, -7725}, {191114, -25125}, {721678, 104075},
    {499831, -65775}, {1924937, 187000}, {4010401, -83250}, {1051273, 43175},
    {1100329, 137175}, {213817, -18050}, {203159, -4275}, {148993, 5925},
    {63364, -1475}, {4453, -600}, {18469, 475}, {4088, 325}, {10001, 250}, {1, 0}}

25
— is a relation number with a list {{74, 75}, {1, 0}}
74

25
— is a relation number with a list {{76, 75}, {1, 0}}
76

25
— is a relation number with a list
77
  {{77, 75}, {154, 25}, {308, 25}, {616, -75}, {176, -25}, {1, 0}}

```

```

25
— is a relation number with a list {{78, 75}, {1, 0}}
78

25
— is a relation number with a list
79
{{79, 75}, {316, 25}, {711, 50}, {869, 100}, {2449, -150}, {3871, 400},
{10191, 650}, {16511, 900}, {24569, 1125}, {14299, 1625}, {25754, 2025},
{45109, -2950}, {67861, 3175}, {93694, 13625}, {132799, 16275},
{205321, -13775}, {103016, 12425}, {285664, -12825}, {277606, 41025},
{755951, 108175}, {100646, -10025}, {31284, 25}, {711, -50}}

25
— is a relation number with a list {{81, 75}, {162, 25}, {324, -25}, {1, 0}}
81

25
— is a relation number with a list {{82, 75}, {574, 25}, {1, 0}}
82

25
— is a relation number with a list {{83, 75}, {664, 25}, {913, 125}, {3154, -75},
83
{332, -25}, {581, 25}, {498, -25}, {166, 25}, {747, -50}, {249, 25}, {1, 0}}

25
— is a relation number with a list {{84, 75}, {1, 0}}
84

25
— is a relation number with a list
86
{{86, 75}, {946, 125}, {2322, 25}, {258, 25}, {344, -25}, {258, 25}}

25
— is a relation number with a list {{87, 75}, {348, -25}, {174, 25}, {1, 0}}
87

25
— is a relation number with a list {{88, 100}, {264, -25}, {1, 0}}
88

25
— is a relation number with a list
89
{{89, 100}, {979, -100}, {1869, -25}, {534, -25}, {801, 25}, {1, 0}}

25
— is a relation number with a list
91
{{91, 100}, {819, -100}, {1729, -75}, {364, -25}, {1001, 75}, {182, 25}, {1, 0}}

25
— is a relation number with a list {{92, 100}, {1, 0}}
92

25
— is a relation number with a list {{93, 100}, {651, -25}, {1, 0}}
93

25
— is a relation number with a list {{94, 100}, {282, 25}, {658, 75},
94
{1598, 175}, {2162, -225}, {4136, -425}, {5358, 25}, {376, -25}, {1, 0}}

25
— is a relation number with a list {{96, 100}, {1, 0}}
96

25
— is a relation number with a list
97
{{97, 100}, {291, -25}, {873, -50}, {2231, -250}, {1843, 25}, {679, 25}, {388, 25},
{1164, -25}, {1067, -50}, {1649, -175}, {7178, -325}, {2716, -25}, {873, -50}}

25
— is a relation number with a list {{98, 100}, {1, 0}}
98

```

```

25
— is a relation number with a list {{99, 100}, {1, 0}}
99

25
— is a relation number with a list {{101, 100}, {1, 0}}
101

25
— is a relation number with a list {{102, 100}, {1, 0}}
102

25
— is a relation number with a list
103
{{103, 100}, {309, 25}, {927, 100}, {2781, 175}, {1957, 25}, {721, -50},
{2163, 100}, {3811, -125}, {6283, -675}, {21424, -1925}, {25647, 925},
{26059, -400}, {6077, 100}, {2369, 50}, {1957, -75}, {721, -25}, {412, -25},
{1236, 125}, {1442, 75}, {1751, 75}, {2678, -75}, {2266, 25}, {927, -100}}

25
— is a relation number with a list {{104, 100}, {1, 0}}
104

25
— is a relation number with a list
106
{{106, 100}, {318, -25}, {742, 25}, {424, -25}, {1, 0}}

25
— is a relation number with a list {{107, 100}, {749, 25}, {1, 0}}
107

25
— is a relation number with a list {{108, 100}, {1, 0}}
108

25
— is a relation number with a list
109
{{109, 100}, {981, 100}, {2071, 25}, {436, -25}, {1199, 25}, {1, 0}}

25
— is a relation number with a list
111
{{111, 100}, {1221, 100}, {777, 25}, {222, 25}, {1, 0}}

25
— is a relation number with a list
112
{{112, 100}, {336, 25}, {616, 25}, {252, -25}, {1, 0}}

25
— is a relation number with a list {{113, 125}, {1356, -25}, {678, 25},
113
{339, -25}, {1243, 75}, {3616, 325}, {4633, -175}, {9379, 975}, {41923, 1125},
{33674, 475}, {5763, -125}, {1469, -150}, {3503, -100}, {339, 25}}

25
— is a relation number with a list {{114, 125}, {627, 25}, {1, 0}}
114

25
— is a relation number with a list
116
{{116, 125}, {261, -25}, {1276, 125}, {377, 25}, {1, 0}}

25
— is a relation number with a list {{117, 125}, {936, -25}, {1287, 100}, {1, 0}}
117

25
— is a relation number with a list {{118, 125}, {413, -25}, {708, -25},
118
{472, 25}, {354, -25}, {236, 25}, {1298, -75}, {2714, -225}, {826, 25}, {1, 0}}

```

```

25
119 is a relation number with a list
{{119, 125}, {714, -25}, {1309, -50}, {1071, -100}, {3451, 300}, {17731, 1550},
{81039, -2825}, {105434, 3925}, {9197, 900}, {23443, -1250}, {36533, 2925},
{170527, -10175}, {17136, -775}, {10234, 225}, {12971, -475}, {17374, -1775},
{44744, 4425}, {58786, -4475}, {10387, 300}, {13447, 1025}, {14518, -25}, {1, 0}}

25
121 is a relation number with a list {{121, 125}, {484, -25}, {1089, -100}, {1, 0}}

25
122 is a relation number with a list {{122, 125}, {366, -25}, {549, -50}, {1, 0}}

25
123 is a relation number with a list
{{123, 125}, {246, 25}, {492, 25}, {328, -25}, {1, 0}}

25
124 is a relation number with a list {{124, 125}, {1, 0}}

25
126 is a relation number with a list {{126, 125}, {1, 0}}

25
127 is a relation number with a list
{{127, 125}, {254, 25}, {508, -25}, {1016, 25}, {1143, -25}, {889, 25},
{1397, 125}, {2794, -75}, {2413, -25}, {1524, -125}, {3048, -275},
{2921, 150}, {9017, -475}, {1016, -75}, {4318, 175}, {7239, 575},
{29972, -2225}, {132969, 5350}, {99187, 3925}, {134874, -5975},
{323977, -6475}, {28829, 550}, {29083, 1150}, {42291, -3800}, {62357, -3875},
{45339, -1250}, {43053, 2275}, {21844, -825}, {50038, 3575}, {1524, -125}}

25
128 is a relation number with a list {{128, 125}, {384, 25}, {576, 25}, {1, 0}}

25
129 is a relation number with a list {{129, 125}, {516, 25}, {387, -25}, {516, 25}}

25
131 is a relation number with a list
{{131, 125}, {786, 25}, {1441, -25}, {1179, -100}, {2751, -25}, {1, 0}}

25
132 is a relation number with a list {{132, 125}, {462, 25}, {1, 0}}

25
133 is a relation number with a list
{{133, 125}, {1064, 25}, {1463, -25}, {1596, 25}, {532, -25}, {1, 0}}

25
134 is a relation number with a list {{134, 125}, {603, 50}, {402, 25}, {1, 0}}

25
136 is a relation number with a list {{136, 125}, {748, -25}, {1, 0}}

25
137 is a relation number with a list {{137, 125}, {1644, 25}, {822, 25}, {411, 25},
{1507, 125}, {959, -25}, {1233, -50}, {2329, 50}, {2877, -25}, {274, 25}, {1, 0}}

25
138 is a relation number with a list {{138, 150}, {1, 0}}

```

```

25
139 is a relation number with a list
{{139, 150}, {1529, 50}, {2919, -125}, {6116, 225}, {5699, -500}, {27661, 150},
{8479, -500}, {2919, 200}, {11259, 550}, {36001, -1250}, {34611, -550},
{5421, 400}, {24881, -1900}, {25159, -1650}, {56851, -4400}, {48511, 850},
{8479, 725}, {30719, -1325}, {33916, -1175}, {22101, 350}, {7089, 200},
{12371, 1100}, {37669, -2925}, {49484, -2825}, {189874, 17025}, {361261, 27375},
{748654, 34925}, {2116831, -94850}, {4188209, 374800}, {9091851, -230000},
{15032711, -474700}, {21918771, -1034525}, {26930694, 1510525},
{35967084, -2958175}, {65188776, -825325}, {1653961, -105175}, {4008621, 199825},
{1684819, -102625}, {5951841, -348700}, {3327799, 11225}, {722661, 575},
{15846, -125}, {4031, -25}, {834, -25}, {1251, -100}, {6811, 425}, {1529, -50}}

25
141 is a relation number with a list {{141, 150}, {1, 0}}

25
142 is a relation number with a list
{{142, 150}, {284, 25}, {639, -25}, {1562, -25}, {852, 25}, {1, 0}}

25
143 is a relation number with a list {{143, 150}, {1001, 75}, {286, 25}, {1, 0}}

25
144 is a relation number with a list {{144, 150}, {1, 0}}

25
146 is a relation number with a list {{146, 150}, {1, 0}}

25
147 is a relation number with a list {{147, 150}, {1, 0}}

25
148 is a relation number with a list {{148, 150}, {1, 0}}

25
149 is a relation number with a list {{149, 150}, {1, 0}}

25
151 is a relation number with a list {{151, 150}, {1, 0}}

25
152 is a relation number with a list {{152, 150}, {1, 0}}

25
153 is a relation number with a list {{153, 150}, {1, 0}}

25
154 is a relation number with a list {{154, 150}, {1, 0}}

25
156 is a relation number with a list {{156, 150}, {1, 0}}

25
157 is a relation number with a list {{157, 150}, {1099, -75}, {4082, 75},
{5024, -225}, {11618, -175}, {10676, -275}, {7693, 300}, {16799, 1050}, {1, 0}}

25
158 is a relation number with a list {{158, 150}, {316, 25}, {711, 50},
{1738, -75}, {1027, -75}, {3634, -225}, {2686, 75}, {1106, 25}, {474, 25}, {1, 0}}

25
159 is a relation number with a list {{159, 150}, {1, 0}}

```



```

25
161 is a relation number with a list
{{161, 150}, {1771, -50}, {483, -25}, {1288, -25}, {1932, 125}, {1311, 25}, {1771, -100},
{4669, 150}, {3059, -75}, {2576, 75}, {4186, -275}, {9821, -50}, {483, -25}}

25
162 is a relation number with a list {{162, 150}, {1, 0}}

25
163 is a relation number with a list
{{163, 175}, {1956, -25}, {978, -25}, {489, -25}, {1793, -50}, {1141, -75},
{2608, 175}, {2771, -50}, {3423, 250}, {12551, -325}, {20212, 275},
{22331, 300}, {21353, -225}, {3586, -175}, {14018, -575},
{35534, -1075}, {9617, 300}, {2771, 25}, {652, 25}, {326, 25}, {1, 0}}

25
164 is a relation number with a list {{164, 175}, {451, -25}, {1, 0}}

25
166 is a relation number with a list {{166, 175}, {1494, -25}, {498, -25}, {1, 0}}

25
167 is a relation number with a list
{{167, 175}, {1336, -25}, {1837, -50}, {2171, -100}, {4843, 25},
{1169, 25}, {1002, 25}, {334, 25}, {1503, -100}, {501, 25}, {1, 0}}

25
168 is a relation number with a list {{168, 175}, {1, 0}}

25
169 is a relation number with a list
{{169, 175}, {1014, -25}, {1859, 100}, {6929, -500}, {11999, -700},
{16731, 500}, {39039, -2125}, {133341, -4075}, {191646, 8275},
{223249, 11425}, {887419, 38300}, {1101711, -46300},
{1603641, -3725}, {309946, -12375}, {96499, 7050}, {371969, 19100},
{1532661, 53750}, {4409041, 47400}, {142129, 75}, {676, -25}, {1, 0}}

25
171 is a relation number with a list {{171, 175}, {684, -25}, {1, 0}}

25
172 is a relation number with a list {{172, 175}, {516, -25}, {1548, 25}, {1, 0}}

25
173 is a relation number with a list
{{173, 175}, {346, 25}, {692, -25}, {1384, -75}, {5882, -225}, {5536, 275},
{6228, -125}, {3806, 175}, {7612, 525}, {45326, -875}, {30102, -875},
{60896, -1775}, {94458, -6775}, {67816, -3925}, {188743, 2850},
{111239, -5275}, {80272, 3825}, {9169, -550}, {31313, 125}, {10726, 75}, {1, 0}}

25
174 is a relation number with a list {{174, 175}, {1, 0}}

25
176 is a relation number with a list {{176, 175}, {1, 0}}

25
177 is a relation number with a list
{{177, 175}, {354, 25}, {708, 25}, {1416, 25}, {531, 25}, {354, 25}}

```

$\frac{25}{178}$  is a relation number with a list  $\{\{178, 175\}, \{534, 25\}, \{801, -25\}, \{1, 0\}\}$

$\frac{25}{179}$  is a relation number with a list  $\{\{179, 175\}, \{716, 25\}, \{1611, 25\}, \{1969, 75\}, \{3401, 125\}, \{4654, 275\}, \{3759, 125\}, \{1611, 100\}, \{1969, 25\}, \{1074, 25\}, \{1, 0\}\}$

$\frac{25}{181}$  is a relation number with a list  $\{\{181, 175\}, \{1086, 25\}, \{1991, 125\}, \{1629, 100\}, \{5249, -25\}, \{1, 0\}\}$

$\frac{25}{182}$  is a relation number with a list  $\{\{182, 175\}, \{1, 0\}\}$

$\frac{25}{183}$  is a relation number with a list  $\{\{183, 175\}, \{1464, 25\}, \{2013, 100\}, \{2379, 100\}, \{1281, 25\}, \{366, 25\}, \{549, -25\}, \{1, 0\}\}$

$\frac{25}{184}$  is a relation number with a list  $\{\{184, 175\}, \{1656, 25\}, \{552, -25\}, \{1, 0\}\}$

$\frac{25}{186}$  is a relation number with a list  $\{\{186, 175\}, \{1023, 50\}, \{2139, 50\}, \{1023, 25\}, \{1, 0\}\}$

$\frac{25}{187}$  is a relation number with a list  $\{\{187, 175\}, \{2244, 25\}, \{1122, -25\}, \{561, 25\}, \{1, 0\}\}$

$\frac{25}{188}$  is a relation number with a list  $\{\{188, 200\}, \{564, -25\}, \{2068, 25\}, \{1316, 25\}, \{1692, 25\}, \{376, 25\}, \{1, 0\}\}$

$\frac{25}{189}$  is a relation number with a list  $\{\{189, 200\}, \{2079, -125\}, \{414, -25\}, \{2079, 50\}, \{1, 0\}\}$

$\frac{25}{191}$  is a relation number with a list  $\{\{191, 200\}, \{1719, 50\}, \{3629, 50\}, \{4011, -100\}, \{2101, -125\}, \{4584, -125\}, \{7831, 300\}, \{5921, -50\}, \{4011, -100\}\}$

$\frac{25}{192}$  is a relation number with a list  $\{\{192, 200\}, \{1, 0\}\}$

$\frac{25}{193}$  is a relation number with a list  $\{\{193, 200\}, \{1351, 75\}, \{1, 0\}\}$

$\frac{25}{194}$  is a relation number with a list  $\{\{194, 200\}, \{582, 25\}, \{679, -25\}, \{388, 25\}, \{1164, -25\}, \{1067, -50\}, \{3298, 75\}, \{1, 0\}\}$

$\frac{25}{196}$  is a relation number with a list  $\{\{196, 200\}, \{1, 0\}\}$

```

25
197 is a relation number with a list
{{197, 200}, {591, -25}, {1773, -25}, {394, 25}, {1182, 25}, {1379, 25},
{788, 25}, {2364, -125}, {2167, -125}, {8274, -475}, {39203, 950},
{49841, -2600}, {86877, -5050}, {202319, 6475}, {314018, 375},
{28171, -1200}, {112487, 6275}, {91211, 2350}, {86483, -2000}, {95151, 4475},
{231672, -425}, {9259, -300}, {8077, -350}, {5319, -100}, {3743, -225},
{16154, -775}, {23837, 1425}, {76436, 575}, {7683, -175}, {3349, 50}, {1, 0}}

25
198 is a relation number with a list {{198, 200}, {1, 0}}

25
199 is a relation number with a list {{199, 200}, {1, 0}}

25
201 is a relation number with a list {{201, 200}, {1, 0}}

25
202 is a relation number with a list {{202, 200}, {1, 0}}

25
203 is a relation number with a list
{{203, 200}, {609, 25}, {1827, -100}, {5481, -50}, {551, 25}, {1, 0}}

25
204 is a relation number with a list {{204, 200}, {1, 0}}

25
206 is a relation number with a list
{{206, 200}, {618, -25}, {1442, 75}, {1751, 75}, {2678, -75}, {2266, 25},
{1854, 25}, {412, 25}, {1236, 25}, {2266, -75}, {1648, 75}, {1, 0}}

25
207 is a relation number with a list
{{207, 200}, {483, -25}, {1656, 25}, {414, 25}, {2277, 50}, {1, 0}}

25
208 is a relation number with a list {{208, 200}, {1, 0}}

25
209 is a relation number with a list {{209, 200}, {1881, -50}, {1, 0}}

25
211 is a relation number with a list {{211, 200}, {2321, 125},
{11394, 625}, {30384, -1325}, {19201, -250}, {10339, 75}, {2321, 125}}

25
212 is a relation number with a list
{{212, 200}, {636, 25}, {2332, 75}, {1484, -25}, {477, 25}, {1, 0}}

25
213 is a relation number with a list {{213, 225}, {852, 25}, {426, 25}, {1, 0}}

25
214 is a relation number with a list
{{214, 225}, {2354, -25}, {428, 25}, {642, 25}, {856, 25}, {642, -25}}

25
216 is a relation number with a list {{216, 225}, {1, 0}}

```

```

25
217 is a relation number with a list
    {{217, 225}, {1736, -25}, {2387, 75}, {2821, -25}, {868, 25}, {1, 0}}

25
218 is a relation number with a list
    {{218, 225}, {763, -25}, {1308, 25}, {872, 25}, {654, 25}, {436, 25}, {1199, -25}, {1, 0}}

25
219 is a relation number with a list {{219, 225}, {438, 25}, {876, -25}, {1, 0}}

25
221 is a relation number with a list
    {{221, 225}, {884, -25}, {1989, 100}, {2431, -100}, {6851, 375}, {22321, -450},
    {39559, 1000}, {97461, -500}, {663, 25}, {2652, -125}, {5967, 50}, {1, 0}}

25
222 is a relation number with a list {{222, 225}, {1, 0}}

25
223 is a relation number with a list
    {{223, 225}, {446, 25}, {892, 25}, {1784, 25}, {2007, -50}, {1561, 50}, {2453, -125},
    {10481, -325}, {18063, 425}, {47276, 625}, {49952, 625}, {10704, -175}, {6467, 125},
    {7359, 175}, {2007, 100}, {1561, 75}, {3122, 75}, {6244, 75}, {4237, 100}, {8251, 100},
    {10927, -250}, {16279, -825}, {49283, 1650}, {48391, 950}, {13157, 550},
    {9589, -100}, {2453, 25}, {669, 25}, {1338, -25}, {2676, -125}, {11373, 175}, {446, 25}}

25
224 is a relation number with a list {{224, 225}, {1, 0}}

25
226 is a relation number with a list {{226, 225}, {1, 0}}

25
227 is a relation number with a list {{227, 225}, {454, 25}, {908, -25}, {1816, -75},
    {3632, 175}, {9761, 50}, {2497, 75}, {4994, -25}, {1362, -25}, {2724, 25}, {1, 0}}

25
228 is a relation number with a list {{228, 225}, {1, 0}}

25
229 is a relation number with a list
    {{229, 225}, {916, 25}, {2061, -100}, {8931, 475}, {21526, -675},
    {16946, -825}, {86791, -575}, {7786, -75}, {3206, 25}, {1374, 25}, {1, 0}}

25
231 is a relation number with a list {{231, 225}, {462, 25}, {924, 25}, {1, 0}}

25
232 is a relation number with a list {{232, 225}, {812, 25}, {696, 25}, {1, 0}}

25
233 is a relation number with a list {{233, 225}, {1864, 25}, {2563, -50}, {3029, 50},
    {4893, -100}, {1631, 25}, {1398, -25}, {466, 25}, {2097, 25}, {699, 25}, {1, 0}}

25
234 is a relation number with a list {{234, 225}, {1, 0}}

25
236 is a relation number with a list {{236, 225}, {2596, 25}, {1, 0}}

```

$\frac{25}{237}$  is a relation number with a list  $\{\{237, 225\}, \{948, -25\}, \{474, 25\}, \{1, 0\}\}$

$\frac{25}{238}$  is a relation number with a list

$\{\{238, 250\}, \{714, -25\}, \{1309, -50\}, \{2142, 25\}, \{952, 25\}, \{1, 0\}\}$

$\frac{25}{239}$  is a relation number with a list

$\{\{239, 250\}, \{2629, -75\}, \{956, -25\}, \{1434, 25\}, \{2151, -100\},$   
 $\{11711, -600\}, \{69071, -1100\}, \{54731, -450\}, \{40391, 1925\}, \{8126, -225\},$   
 $\{6214, 175\}, \{20554, -975\}, \{18881, 25\}, \{1434, -25\}\}$

$\frac{25}{241}$  is a relation number with a list

$\{\{241, 250\}, \{2169, 50\}, \{4579, 175\}, \{6989, 125\}, \{2651, 125\},$   
 $\{6266, 225\}, \{8194, 175\}, \{7471, -325\}, \{964, 25\}, \{2651, 25\}, \{1, 0\}\}$

$\frac{25}{242}$  is a relation number with a list

$\{\{242, 250\}, \{484, 25\}, \{2178, -25\}, \{726, 25\}, \{1, 0\}\}$

$\frac{25}{243}$  is a relation number with a list  $\{\{243, 250\}, \{1701, -25\}, \{1, 0\}\}$

$\frac{25}{244}$  is a relation number with a list

$\{\{244, 250\}, \{732, 25\}, \{1708, -25\}, \{488, 25\}, \{732, -25\}\}$

$\frac{25}{246}$  is a relation number with a list  $\{\{246, 250\}, \{1, 0\}\}$

$\frac{25}{247}$  is a relation number with a list  $\{\{247, 250\}, \{741, -25\}, \{2223, 100\},$   
 $\{5681, -25\}, \{1482, -25\}, \{1729, -50\}, \{5187, -250\}, \{1197, 25\}, \{741, -25\}\}$

$\frac{25}{248}$  is a relation number with a list  $\{\{248, 250\}, \{1, 0\}\}$

$\frac{25}{249}$  is a relation number with a list  $\{\{249, 250\}, \{1, 0\}\}$

known cases

known cases

$\frac{26}{7}$  is a relation number with a list

$\{\{7, 26\}, \{133, 312\}, \{1253, 2470\}, \{8519, 14352\}, \{40831, 51194\},$   
 $\{72541, -88920\}, \{114653, 196586\}, \{573531, 754156\}, \{1264375, -582842\},$   
 $\{690837, 1052038\}, \{2528407, 2026960\}, \{3510129, 1151098\}, \{397845, 669136\},$   
 $\{1899037, 2369614\}, \{3294039, -4352296\}, \{7407799, 2951390\},$   
 $\{10124597, 16945916\}, \{47749233, 58732882\}, \{76885543, -125555300\},$   
 $\{340688299, -386526582\}, \{320867981, 322095358\}, \{8591639, 11070436\},$   
 $\{17351579, -13044330\}, \{30150743, 20678164\}, \{66308053, -101539906\},$   
 $\{246622971, -205248836\}, \{289618945, -361014342\}, \{499767779, 670820072\},$   
 $\{1197366051, -248380886\}, \{311768653, -577329506\}, \{1858925971, -2863275636\},$   
 $\{7030447655, -6070161838\}, \{6722000719, 7443729618\}, \{5052102293, 4188746796\},$   
 $\{6043488479, 6873984650\}, \{5813473197, -4932091658\}, \{6169670773, 11307198422\},$   
 $\{35962693543, 54425329920\}, \{129238454639, 99051236362\},$

```

{211310527939, -91509020668}, {198047406221, 95041507002},
{55750745519, 44067956088}, {81779526017, 4723167410},
{10399760329, -5565509352}, {5118808625, 933129964}, {3172111635, -5250219182},
{14546752829, -17279261948}, {19127563833, -21135640552},
{14056537033, -8680500218}, {23131243821, -25152546952},
{14149121917, 18406184446}, {29799437703, -18159665368},
{45639251231, -42399561282}, {22677829643, 40130825722},
{122170972553, 172862118000}, {354838018129, 107934955622},
{217232058841, -51317243484}, {83741594335, -48180496858},
{88335795667, 9159094100}, {22786017331, 20520119958},
{15861281611, 25814176310}, {69670262893, 78076028004},
{58840355777, 109117482630}, {351939887971, 543382919768},
{1340101222579, 1173838388346}, {1163839839631, -428798661694},
{857893018157, -184869149868}, {465169118281, -433686961682},
{220375096193, 238335554522}, {125723208303, 199538784562},
{516709033813, 522433490800}, {40071198909, 63862605950},
{166539849287, 171538341416}, {34989444903, -31121231726},
{27077492239, -16701536878}, {44279070619, -47554361296},
{22927034739, -7749701336}, {2254484883, 4005103388},
{12254329535, 17480357414}, {36582195153, 13514222956},
{27723316005, 8372755898}, {18235338177, -9121964800}, {60139961, -32067828},
{27969865, 16698656}, {37992129, 24223030}, {73177517, 102240996},
{203444353, 39963482}, {25388601, -3157180}, {918127, -1639144},
{5047119, -7272434}, {15577205, -6951152}, {11724307, -5110638},
{10521217, 3304340}, {4257379, 7317258}, {21419153, 28336048},
{48418265, -18513066}, {49846531, -55552796}, {39943855, -56219098},
{113926701, -29622632}, {31946789, -29960580}, {13903463, -3158324},
{8891169, 10916074}, {14174335, -23764988}, {67134571, -83002062},
{111072437, 168459668}, {401710617, 312850330}, {622022009, -120415152},
{139623743, 194298884}, {382725987, 61461478}, {97699833, 67345252},
{212482067, -317802342}, {737241925, -513710756}, {1564718183, 2215835102},
{4557818433, 1418194180}, {2122651251, 2043226042}, {79425209, -21829392},
{55246513, -52395590}, {19956461, 3850860}, {4915127, 8699834},
{26492949, 37503544}, {77074165, 23750662}, {40755253, 14877980},
{27150809, -3299998}, {5255775, -3578536}, {11740673, 18558462},
{47724523, 47353280}, {2598701, 3294148}, {4868129, -4977414}, {764995, 744978},
{140119, 10426}, {32067, -46124}, {98399, -42614}, {92197, 44148}, {27307, 4758},
{8687, -1040}, {2569, 2262}, {2149, -130}, {427, -676}, {1743, -1742}, {1, 0}

26
— is a relation number with a list
9
{{9, 26}, {153, 208}, {495, -442}, {159, 52}, {1, 0}}

26
— is a relation number with a list
11
{{11, 26}, {165, 104}, {473, -26}, {55, -26}, {33, 26}, {77, -78}, {1, 0}}

26
— is a relation number with a list
15
{{15, 26}, {165, -104}, {645, 442}, {3045, 1352}, {5115, 2548}, {285, 182},
{1185, -676}, {2505, 1456}, {6105, -676}, {35, 26}, {45, -26}, {105, 26}, {1, 0}}

```

```

26
— is a relation number with a list {{17, 26}, {153, 26}, {51, 26}, {1, 0}}
17

26
— is a relation number with a list
19
  {{19, 26}, {133, 52}, {437, 208}, {399, 130}, {171, -104}, {703, 52},
    {475, 312}, {2831, 1820}, {15371, 7488}, {7505, -1508}, {665, 442},
    {4161, -2704}, {23693, -13468}, {61617, 2938}, {1539, 1040},
    {9481, -6188}, {55005, -32968}, {207689, 57980}, {460389, 158392},
    {280953, 66248}, {303259, 13754}, {12749, -364}, {171, 104}}

26
— is a relation number with a list {{21, 26}, {105, -26}, {1, 0}}
21

26
— is a relation number with a list {{23, 26}, {69, 26}, {207, 104}, {1, 0}}
23

26
— is a relation number with a list {{25, 26}, {1, 0}}
25

26
— is a relation number with a list {{27, 26}, {1, 0}}
27

26
— is a relation number with a list {{29, 26}, {87, -26}, {261, -52}, {1, 0}}
29

26
— is a relation number with a list {{31, 26}, {155, 26}, {1, 0}}
31

26
— is a relation number with a list {{33, 26}, {231, -52}, {253, 26}, {231, 52}}
33

26
— is a relation number with a list {{35, 26}, {315, -26}, {105, 26}, {1, 0}}
35

26
— is a relation number with a list
37
  {{37, 26}, {407, 104}, {333, -104}, {777, -26}, {111, 26}, {259, 52}, {1, 0}}

26
— is a relation number with a list
41
  {{41, 52}, {451, -130}, {2501, -572}, {8733, -1300}, {15047, -3952},
    {31201, 3744}, {51209, -8866}, {81467, 1872}, {36941, -6474}, {78023, 18044},
    {239727, -20306}, {161745, 11986}, {243007, 29120}, {411927, -112190},
    {1510153, -188500}, {88273, -3536}, {5207, -312}, {3977, 182}, {1107, 260},
    {2747, 208}, {1763, -416}, {4059, 962}, {8651, 1040}, {13571, -390}, {3239, -442},
    {5945, 728}, {4961, 1534}, {14719, -2444}, {2255, -104}, {1353, -26}, {1, 0}}

26
— is a relation number with a list {{43, 52}, {387, 104}, {1247, 52}, {1, 0}}
43

26
— is a relation number with a list {{45, 52}, {315, 26}, {1, 0}}
45

26
— is a relation number with a list {{47, 52}, {235, 26}, {1, 0}}
47

26
— is a relation number with a list {{49, 52}, {147, 26},
49
  {441, -104}, {1225, 104}, {1127, 286}, {833, 130}, {2597, -520}, {147, -26}}

26
— is a relation number with a list {{51, 52}, {1, 0}}
51

```

```

26
— is a relation number with a list {{53, 52}, {1, 0}}
53

26
— is a relation number with a list {{55, 52}, {165, -26}, {495, -26}, {1, 0}}
55

26
— is a relation number with a list {{57, 52}, {285, -26}, {1, 0}}
57

26
— is a relation number with a list
59
  {{59, 52}, {413, -26}, {177, -26}, {295, -26}, {531, 104}, {649, 130}, {1, 0}}

26
— is a relation number with a list
61
  {{61, 52}, {549, -104}, {1769, -312}, {6283, 286}, {549, 104}}

26
— is a relation number with a list
63
  {{63, 52}, {693, 130}, {387, 52}, {1449, 286}, {133, 26}, {1, 0}}

26
— is a relation number with a list
67
  {{67, 78}, {737, -78}, {2345, 234}, {335, -52}, {1541, 104}, {1273, -52}, {1675, -234},
  {2479, -286}, {6365, -598}, {14271, 1300}, {1943, 364}, {8241, -1196}, {8777, -1612},
  {48039, 3848}, {124821, 15626}, {12529, -1612}, {24589, 3042}, {16951, -104}, {1, 0}}

26
— is a relation number with a list {{69, 78}, {1, 0}}
69

26
— is a relation number with a list
71
  {{71, 78}, {497, -78}, {2059, -260}, {1491, -104}, {2485, -104}, {781, -52}, {1, 0}}

26
— is a relation number with a list {{73, 78}, {365, 26}, {1, 0}}
73

26
— is a relation number with a list {{75, 78}, {1, 0}}
75

26
— is a relation number with a list {{77, 78}, {1, 0}}
77

26
— is a relation number with a list {{79, 78}, {1, 0}}
79

26
— is a relation number with a list {{81, 78}, {1, 0}}
81

26
— is a relation number with a list {{83, 78}, {415, -26}, {1, 0}}
83

26
— is a relation number with a list
85
  {{85, 78}, {595, 78}, {2465, 156}, {2635, -364}, {7395, 728}, {1955, -182}, {3995, -416},
  {2805, 208}, {8585, -702}, {13685, -1066}, {2941, 130}, {4165, 416}, {1, 0}}

26
— is a relation number with a list {{87, 78}, {1, 0}}
87

```



```

26
89 is a relation number with a list
  {{89, 78}, {979, 78}, {3115, 338}, {6497, -286}, {7209, 182}, {6319, 416},
  {7031, 52}, {979, 52}, {801, 52}, {1869, 260}, {4361, 208}, {623, 52}, {1, 0}}

26
93 is a relation number with a list
  {{93, 104}, {1023, 52}, {1581, 26}, {465, 52}, {1, 0}}

26
95 is a relation number with a list {{95, 104}, {855, -52}, {2185, -156}, {1, 0}}

26
97 is a relation number with a list
  {{97, 104}, {679, -78}, {2231, -208}, {5529, -572}, {18527, 858},
  {33853, -1560}, {45299, 5616}, {35987, 4576}, {60237, -7930}, {310691, 19708},
  {449789, 17316}, {41419, -3250}, {80607, -8840}, {101559, -13598},
  {618181, 6578}, {14647, 1872}, {31913, -1950}, {69161, -3770},
  {126197, 6396}, {167131, 6760}, {181293, -23998}, {1037027, 104078},
  {364041, -45032}, {367145, -38064}, {1309015, -167362}, {2898457, -80912},
  {1394375, -286}, {12125, 1508}, {5917, 364}, {9021, -962}, {35211, 1066},
  {3201, -416}, {12319, 728}, {5529, 520}, {18527, -780}, {18721, 390}, {1, 0}}

26
99 is a relation number with a list {{99, 104}, {495, -26}, {1, 0}}

26
101 is a relation number with a list {{101, 104}, {303, 26}, {909, -52}, {2525, -52},
  {2323, -130}, {1717, -130}, {2727, 208}, {2323, 78}, {1717, 78}, {1, 0}}

26
103 is a relation number with a list {{103, 104}, {1, 0}}

26
105 is a relation number with a list {{105, 104}, {1, 0}}

26
107 is a relation number with a list {{107, 104}, {321, -26}, {963, 26}, {1, 0}}

26
109 is a relation number with a list {{109, 104}, {545, 26}, {1, 0}}

26
111 is a relation number with a list {{111, 104}, {259, 26}, {1, 0}}

26
113 is a relation number with a list {{113, 104}, {1017, 52}, {2599, 104}, {1, 0}}

26
115 is a relation number with a list
  {{115, 104}, {1265, -52}, {1955, 208}, {9545, 182}, {1863, -26}, {1035, -52}, {1, 0}}

26
119 is a relation number with a list
  {{119, 130}, {1309, -26}, {1071, -52}, {357, 26}, {1, 0}}

26
121 is a relation number with a list {{121, 130}, {1089, -52}, {363, -26}, {1, 0}}

26
123 is a relation number with a list {{123, 130}, {861, 26}, {1, 0}}

```

```

26
125 is a relation number with a list {{125, 130}, {1, 0}}

26
127 is a relation number with a list {{127, 130}, {381, 26}, {1143, -26}, {1, 0}}

26
129 is a relation number with a list {{129, 130}, {1, 0}}

26
131 is a relation number with a list {{131, 130}, {1, 0}}

26
133 is a relation number with a list {{133, 130}, {399, -26}, {1197, 52}, {1, 0}}

26
135 is a relation number with a list {{135, 130}, {1, 0}}

26
137 is a relation number with a list {{137, 130}, {959, -26}, {411, -26},
    {685, 52}, {1233, 104}, {2055, 182}, {7261, 130}, {2603, -26}, {411, 26}}

26
139 is a relation number with a list {{139, 130}, {1251, 52}, {417, -26}, {1, 0}}

26
141 is a relation number with a list
    {{141, 130}, {1551, 26}, {423, 26}, {987, 26}, {1, 0}}

26
145 is a relation number with a list {{145, 156}, {1595, -26}, {1305, -26}, {1, 0}}

26
147 is a relation number with a list {{147, 156}, {1, 0}}

26
149 is a relation number with a list
    {{149, 156}, {1043, 52}, {447, 26}, {745, -26}, {1341, -104}, {1639, 52},
    {3725, 52}, {2831, 156}, {3427, -78}, {745, 52}, {2533, -208}, {5513, -208},
    {15347, -1144}, {70775, 2444}, {15049, 858}, {58855, -4602}, {144679, 4056},
    {199213, -13390}, {243913, -5304}, {10579, 208}, {4321, -78}, {4619, -338},
    {16837, 416}, {29353, 520}, {34717, -1274}, {47531, 936}, {30545, -884},
    {58855, -1794}, {51703, -3354}, {207557, 7306}, {445361, 598}, {1, 0}}

26
151 is a relation number with a list {{151, 156}, {755, -26}, {1, 0}}

26
153 is a relation number with a list {{153, 156}, {1, 0}}

26
155 is a relation number with a list {{155, 156}, {1, 0}}

26
157 is a relation number with a list {{157, 156}, {1, 0}}

26
159 is a relation number with a list {{159, 156}, {1, 0}}

26
161 is a relation number with a list {{161, 156}, {805, 26}, {1, 0}}

```

```

26
163 is a relation number with a list
  {{163, 156}, {1141, -52}, {489, -26}, {815, -52}, {2771, 78}, {6031, -208}, {1, 0}}

26
165 is a relation number with a list {{165, 156}, {1, 0}}

26
167 is a relation number with a list {{167, 156}, {1837, 26}, {1503, 104},
  {7849, 260}, {8183, 104}, {5511, -208}, {17201, 78}, {6179, 442}, {1503, -104}}

26
171 is a relation number with a list {{171, 182}, {1881, 52}, {1, 0}}

26
173 is a relation number with a list {{173, 182}, {1557, 104}, {519, 26}, {1, 0}}

26
175 is a relation number with a list {{175, 182}, {1, 0}}

26
177 is a relation number with a list {{177, 182}, {885, 26}, {1, 0}}

26
179 is a relation number with a list {{179, 182}, {537, 26}, {1611, 26}, {1, 0}}

26
181 is a relation number with a list {{181, 182}, {1, 0}}

26
183 is a relation number with a list {{183, 182}, {1, 0}}

26
185 is a relation number with a list {{185, 182}, {555, -26}, {1665, 104}, {1, 0}}

26
187 is a relation number with a list {{187, 182}, {935, -26}, {1, 0}}

26
189 is a relation number with a list {{189, 182}, {1, 0}}

26
191 is a relation number with a list {{191, 182}, {1719, -104}, {9359, -520}, {1, 0}}

26
193 is a relation number with a list
  {{193, 182}, {2123, -52}, {1737, -26}, {965, -52}, {4439, -130}, {3667, 104},
  {5211, -286}, {12159, 494}, {36863, -988}, {59251, 884}, {4439, 182},
  {13703, 52}, {4825, -286}, {7141, 364}, {26827, -1586}, {26055, 728},
  {29529, -1274}, {43811, 2002}, {44969, 1326}, {22195, 1222}, {38407, -2158},
  {84341, -3900}, {281587, -5980}, {101711, -3172}, {39951, 1352},
  {117537, -7592}, {705801, -39026}, {643269, 7228}, {4439, 130}}

26
197 is a relation number with a list
  {{197, 208}, {2167, -78}, {3349, -104}, {4137, 260}, {4531, 208}, {8865, -26}, {1, 0}}

26
199 is a relation number with a list {{199, 208}, {1791, 26}, {597, -26}, {1, 0}}

26
201 is a relation number with a list {{201, 208}, {1407, 52}, {1, 0}}

```

```

26
203 is a relation number with a list {{203, 208}, {1015, 26}, {1, 0}}

26
205 is a relation number with a list
{{205, 208}, {615, 26}, {1845, 52}, {1025, 52}, {615, -26}}

26
207 is a relation number with a list {{207, 208}, {1, 0}}

26
209 is a relation number with a list {{209, 208}, {1, 0}}

26
211 is a relation number with a list
{{211, 208}, {633, -26}, {1899, -104}, {5697, -182}, {11605, 208},
{9073, -286}, {16669, 780}, {60979, -728}, {36503, 676}, {1, 0}}

26
213 is a relation number with a list {{213, 208}, {1065, -26}, {1, 0}}

26
215 is a relation number with a list {{215, 208}, {1505, -52}, {645, 26}, {1, 0}}

26
217 is a relation number with a list {{217, 208}, {1953, -26}, {651, -26}, {1, 0}}

26
219 is a relation number with a list {{219, 208}, {803, 26}, {1, 0}}

26
223 is a relation number with a list
{{223, 234}, {2453, -130}, {3791, -182}, {6913, 286}, {10927, 78}, {1561, -78}, {1, 0}}

26
225 is a relation number with a list {{225, 234}, {1, 0}}

26
227 is a relation number with a list
{{227, 234}, {1589, 26}, {681, -26}, {1135, -52}, {2043, 104}, {8399, 442}, {1, 0}}

26
229 is a relation number with a list {{229, 234}, {1145, -26}, {1, 0}}

26
231 is a relation number with a list {{231, 234}, {1, 0}}

26
233 is a relation number with a list {{233, 234}, {1, 0}}

26
235 is a relation number with a list {{235, 234}, {1, 0}}

26
237 is a relation number with a list {{237, 234}, {1, 0}}

26
239 is a relation number with a list {{239, 234}, {1195, 26}, {1, 0}}

26
241 is a relation number with a list {{241, 234}, {1687, -26}, {723, 26},
{1205, -26}, {2169, 52}, {3615, -52}, {6025, 182}, {4579, -104}, {723, -26}}

26
243 is a relation number with a list {{243, 234}, {1, 0}}

```

```

26
245 is a relation number with a list {{245, 234}, {539, 26}, {1, 0}}

26
249 is a relation number with a list
{{249, 260}, {2739, -104}, {8715, -416}, {1743, -52}, {6225, -52}, {1245, 26}, {1, 0}}

26
251 is a relation number with a list {{251, 260}, {2259, 26}, {753, 26}, {1, 0}}

26
253 is a relation number with a list {{253, 260}, {1771, -78}, {1, 0}}

26
255 is a relation number with a list {{255, 260}, {1, 0}}

26
257 is a relation number with a list {{257, 260}, {771, 26},
{{2313, 104}, {6425, 78}, {7453, -312}, {8995, 104}, {13107, 208}, {771, 26}}

26
259 is a relation number with a list {{259, 260}, {1, 0}}

known cases

known cases

known cases

27
7 is a relation number with a list
{{7, 27}, {140, 351}, {1477, 3240}, {12341, 24921}, {88060, 165213}, {540071, 926640},
{2705983, 3950883}, {8714300, 5956119}, {19307267, -32778054},
{94295509, -134264871}, {279785534, -139318677}, {8037260, -14204079},
{43167733, -67075560}, {167354789, -175982409}, {60393340, 67148163},
{47283761, 77103522}, {208738327, 265408893}, {396693962, -327756969},
{482558951, -432999972}, {346912853, -354814938}, {55314595, -76570974},
{148794653, -37925415}, {20349049, 30010338}, {67629023, 50782437},
{117926102, -99380763}, {129817373, -194941188}, {455866705, -393754689},
{434784112, 597766041}, {1140873503, 216149796}, {420871661, -110313549},
{142677745, 221866398}, {554320571, 585028845}, {214957918, 50415075},
{93083326, -6130161}, {7916377, -12376530}, {31221071, -33788421},
{17971450, 28563597}, {74145029, 86042790}, {83284327, 40179564},
{20476393, -34664544}, {99317057, -140428269}, {287778484, -127004841},
{236381614, 22723767}, {64007608, -87820119}, {166687577, -28196964},
{17459449, -4652019}, {8040389, 1551204}, {1990583, 3180465},
{8329174, 9863559}, {10740695, 13811877}, {21498274, -13761225},
{42169232, -66324177}, {169084615, -187914276}, {131807627, -209802609},
{545964874, -637246251}, {638969639, -468470601}, {1193493266, 1324179819},
{914805871, 1316352060}, {2810823323, 1627282683}, {3106194301, 590056380},
{1091386807, -79240167}, {17975531, 9905976}, {12854947, -19758465},
{48324626, -48085731}, {1672265, -1191537}, {3365096, 4638897},
{8916607, 1920348}, {4795931, 5056155}, {1821568, -262845}, {2621, -2889},
{1876, -1485}, {2737, 162}, {119, -216}, {679, -1107}, {2996, -3807}, {5677, 4752},
{6475, 8289}, {12698, -9045}, {25571, 35316}, {68215, 15903}, {32221, -12960},
{44107, 79407}, {247100, 397251}, {1051057, 1273320}, {1555841, -2912139},
{9494086, -16235073}, {47186909, -68361138}, {148219603, -93176217},
{266929817, -377352918}, {772961707, -339953301}, {651385735, 132814728},

```

```
{88 815 335, 98 017 209}, {64 413 118, 59 231 331}, {36 272 509, -5 105 430},
{534 499, -982 152}, {3 133 571, -5 211 567}, {14 545 972, -19 624 923},
{35 552 657, 242 784}, {743 351, -1 167 723}, {2 970 604, -3 283 983}, {2 193 653, -2 395 818},
{1 415 155, 395 361}, {1 164 023, 1 722 276}, {3 907 771, 3 016 899}, {6 236 104, -2 935 251},
{2 559 214, -804 249}, {1 025 269, -1 675 134}, {4 549 055, -5 820 417},
{8 899 534, 6 416 145}, {17 383 723, -22 138 488}, {33 283 355, 26 590 761},
{46 848 158, 5 435 289}, {14 486 101, 17 827 938}, {23 392 859, -34 565 967},
{78 211 756, -59 712 147}, {129 497 263, 81 504 414}, {234 580 955, 334 281 357},
{697 902 814, 351 941 355}, {41 859 272, -41 731 605}, {893 669, 874 530},
{133 973, -79 326}, {172 753, -111 051}, {345 443, -555 066}, {1 467 361, -1 774 359},
{2 148 986, 4 131 567}, {13 878 067, 24 608 718}, {75 114 557, 117 466 551},
{296 463 958, 321 237 981}, {173 418 161, -241 970 004}, {479 862 901, -157 109 733},
{59 735 914, 52 281 639}, {52 179 925, -36 559 377}, {109 343 836, 165 839 157},
{395 467 247, 364 499 568}, {216 773 753, 43 114 977}, {8 392 076, 10 479 915},
{14 614 873, -16 987 752}, {16 610 153, -9 221 202}, {12 825 757, 15 077 637},
{15 763 160, 16 058 061}, {294 901, -133 407}, {196 609, -175 500}, {147 763, -88 614},
{206 255, -175 257}, {216 986, -389 853}, {1 210 069, -1 938 438}, {5 098 583, -6 096 897},
{6 988 198, -11 230 677}, {29 697 353, -35 932 194}, {43 643 887, 83 184 651},
{276 785 348, 485 308 071}, {1 459 659 061, 2 232 957 024}, {5 413 085 741, 5 248 345 833},
{1 153 179 356, 1 154 600 703}, {9 949 429, 15 208 938}, {36 816 563, 35 544 177},
{1 272 386, 1 189 755}, {578 417, -595 863}, {122 122, -68 337}, {101 864, 85 455},
{114 863, 155 142}, {281 953, 1539}, {2212, 2241}, {203, -27}, {91, -162}, {497, -783},
{2002, -2241}, {1673, 2781}, {7756, 10 449}, {18 851, -432}, {1099, -1215},
{812, -891}, {553, -162}, {469, 675}, {1442, 837}, {1624, 405}, {28, 27}, {1, 0}}
```

27  
8 is a relation number with a list

```
{{8, 27}, {152, 297}, {1160, 1539}, {3032, -2079}, {7624, 9099}, {5900, 3429},
{3832, -783}, {664, -459}, {1640, 1863}, {892, -1431}, {4312, -3105},
{9656, 7749}, {15 256, 10 503}, {38 024, -44 307}, {25 132, 7587},
{18 968, -3321}, {3832, 351}, {58, 81}, {184, -27}, {20, -27}, {56, 27}, {1, 0}}
```

27  
10 is a relation number with a list

```
{{10, 27}, {170, 189}, {95, 81}, {70, 27}, {110, 27}, {1, 0}}
```

27  
11 is a relation number with a list

```
{{11, 27}, {176, 135}, {451, 378}, {803, 216},
{671, -729}, {638, 189}, {781, 162}, {319, -216}, {1133, 405}, {902, -27}, {1, 0}}
```

27  
13 is a relation number with a list

```
{{13, 27}, {182, 27}, {91, 27},
{130, 81}, {416, -189}, {494, -405}, {1157, -459}, {2860, 27}, {26, 27}, {1, 0}}
```

27  
14 is a relation number with a list

```
{{14, 27}, {182, -27}, {1, 0}}
```

27  
16 is a relation number with a list

```
{{16, 27}, {176, -135}, {328, 27}, {1, 0}}
```

27  
17 is a relation number with a list

```
{{17, 27}, {170, 81}, {136, 81}, {442, 27}, {170, -81}}
```

```

27
— is a relation number with a list
19
  {{19, 27}, {152, -81}, {190, -81}, {532, -27}, {152, 81}}

27
— is a relation number with a list {{20, 27}, {140, 27}, {1, 0}}
20

27
— is a relation number with a list {{22, 27}, {55, -27}, {1, 0}}
22

27
— is a relation number with a list
23
  {{23, 27}, {92, 27}, {253, 27}, {230, 81}, {299, -108}, {575, -216}, {1679, -945},
  {4853, -1053}, {9476, 1971}, {8717, -4401}, {1955, 243}, {253, -54},
  {391, -135}, {322, 81}, {46, 27}, {184, 27}, {115, 54}, {161, -81}, {1, 0}}

27
— is a relation number with a list {{25, 27}, {50, 27}, {100, -27},
25
  {200, 27}, {275, 81}, {800, 297}, {2275, -54}, {175, -27}, {325, 27}, {1, 0}}

27
— is a relation number with a list {{26, 27}, {1, 0}}
26

27
— is a relation number with a list {{28, 27}, {1, 0}}
28

27
— is a relation number with a list {{29, 27}, {58, 27}, {116, 27}, {232, -81},
29
  {319, -27}, {145, -27}, {290, 27}, {203, -27}, {377, 81}, {812, -81}, {58, 27}}

```

```

27
— is a relation number with a list
31
{{31, 27}, {124, -27}, {341, -54}, {527, 162}, {1271, -513}, {7595, -2673},
{13144, 2727}, {15221, -4995}, {7316, -1917}, {10912, 2403}, {34193, 14850},
{139283, -24894}, {312511, -44847}, {43958, 11961}, {120466, 48897},
{702832, 291519}, {3713614, -666225}, {8795816, -2329641}, {16205188, 1647891},
{8485382, 648837}, {1565531, -338958}, {4007029, 37719}, {273265, -20736},
{114607, -43902}, {530069, -24057}, {25265, 2403}, {36208, -11421},
{60295, 13554}, {188449, -72225}, {875006, -47331}, {714488, -222669},
{1440911, 627183}, {5782895, -704187}, {4631369, -1660932},
{10894237, 4046247}, {38579624, 8972775}, {83344244, -12204567},
{64719475, -16238448}, {7263827, -2732832}, {28974739, 9009603},
{60323830, 16597143}, {188007002, -23267331}, {57918974, -15049449},
{70643482, -25692633}, {199466927, -72174672}, {528769759, -65292183},
{199401145, 60005907}, {600886144, -233226675}, {3062610311, -772277436},
{821482423, 329605713}, {5030400907, 1455143265}, {20614104472, -8753218857},
{96337669498, -19628777169}, {55992706757, 23277995811},
{292538169185, -42756055794}, {209380862563, 48889890117},
{428460364945, 22885967367}, {197563465868, -21179365353},
{215424508421, -93676932972}, {870189916787, 127644465384},
{722961567931, -178921200942}, {225579689053, -45323521974},
{32175545327, 3836078244}, {46094500625, -1522043811},
{13428775145, -399238281}, {4505118679, 604947582}, {8385053755, -3155958963},
{33567517154, 10126053999}, {98870009867, -30542682987},
{224500788086, 30841549713}, {266908142945, 26214510843},
{147654069965, 41038244703}, {511466174257, 64226030814},
{2342072255, -990079929}, {11219284307, -1377573642}, {6159550301, 213374034},
{877197235, 261499401}, {2873669992, 597859839}, {3584505293, 198275877},
{481724717, -146948148}, {1267288463, -140323104}, {135796337, 26130249},
{159497852, -23467185}, {147945733, -45653031}, {340585840, 67952439},
{25532995, -6123816}, {32169661, 6292863}, {21865726, 4635333},
{40639109, -2113911}, {14718800, -1433241}, {11978090, -2700351},
{36477266, 11600685}, {51931541, -2224341}, {23922638, -6447033},
{57830314, -1615329}, {9967430, -2012661}, {2972125, 265491}, {1603444, -149067},
{1125083, -278478}, {346301, 114075}, {126356, 14661}, {173383, -1458}, {3689, 216},
{527, -189}, {1240, 459}, {4247, 567}, {8618, 2565}, {28613, 4752}, {3131, 54}, {1, 0}}

27
— is a relation number with a list {{32, 27}, {80, 27}, {1, 0}}
32

27
— is a relation number with a list
34
{{34, 27}, {238, -27}, {170, -27}, {136, -27}, {1, 0}}

27
— is a relation number with a list {{35, 27}, {280, 81}, {1295, -162}, {1, 0}}
35

27
— is a relation number with a list {{37, 27}, {370, -81}, {1295, 162}, {1, 0}}
37

27
— is a relation number with a list
38
{{38, 27}, {418, 135}, {494, -135}, {874, 81}, {646, 135}, {1102, 351}, {931, 54},
{247, -27}, {76, 27}, {95, 27}, {494, 27}, {152, -27}, {190, -27}, {1, 0}}

```



```

27
40 is a relation number with a list {{40, 27}, {520, 27}, {140, -27}, {1, 0}}

27
41 is a relation number with a list
    {{41, 54}, {533, -108}, {287, 81}, {1517, -324}, {4223, -621},
     {5084, -1323}, {8528, -1917}, {35260, -8937}, {20008, -2511}, {3280, -729},
     {14924, -405}, {2501, 135}, {2624, -351}, {6847, -864},
     {2665, 324}, {2993, -513}, {3485, 378}, {3403, -189}, {1, 0}}

27
43 is a relation number with a list {{43, 54}, {473, 54}, {559, 135},
    {817, 162}, {301, -27}, {172, 27}, {430, 81}, {1075, 108}, {215, -54}, {1, 0}}

27
44 is a relation number with a list {{44, 54}, {220, 27}, {1, 0}}

27
46 is a relation number with a list
    {{46, 54}, {92, 27}, {253, 27}, {115, -27}, {322, 81}, {1, 0}}

27
47 is a relation number with a list
    {{47, 54}, {329, -81}, {235, -27}, {376, -27}, {94, 27}, {611, -135},
     {3008, -567}, {8131, 1377}, {6157, -1053}, {7567, 1674}, {37741, 8046},
     {116983, 25056}, {389959, -57537}, {601600, -60561}, {188470, 31347},
     {388, -81}, {799, 135}, {517, -108}, {1081, 108}, {1, 0}}

27
49 is a relation number with a list {{49, 54}, {245, 54}, {1225, 54}, {833, 108},
    {1519, -270}, {4949, -405}, {4361, -621}, {98, 27}, {490, 27}, {196, 27}, {1, 0}}

27
50 is a relation number with a list {{50, 54}, {1, 0}}

27
52 is a relation number with a list {{52, 54}, {1, 0}}

27
53 is a relation number with a list {{53, 54}, {1, 0}}

27
55 is a relation number with a list {{55, 54}, {1, 0}}

27
56 is a relation number with a list {{56, 54}, {1, 0}}

27
58 is a relation number with a list {{58, 54}, {1, 0}}

27
59 is a relation number with a list
    {{59, 54}, {295, -54}, {1475, 189}, {2183, -162}, {4543, 837}, {21122, 1053},
     {3658, 189}, {3953, 297}, {5428, 135}, {1652, -351}, {6077, 1242}, {7847, -1458},
     {32863, 4212}, {49147, -1107}, {25901, 5805}, {158179, -19440}, {156881, 1728},
     {21653, -2862}, {73337, 1053}, {22007, -1701}, {6254, 189}, {1003, 135}, {3422, 135},
     {2773, 351}, {2065, 81}, {2360, 459}, {3835, 756}, {3245, 54}, {295, -54}}

```

```

27
— is a relation number with a list
61
{{61, 54}, {427, 81}, {1342, 189}, {1159, 243}, {3416, 297}, {9028, 1863},
{17507, 2592}, {38857, -3321}, {60695, -12339}, {61000, -3321}, {74542, -4617},
{40870, 7803}, {113155, -24867}, {681980, 7587}, {51850, -3807}, {88328, -2349},
{56974, -8019}, {51301, 10395}, {41114, 2835}, {86071, 17550}, {102419, 17442},
{136213, 21276}, {521977, -88398}, {513071, -58050}, {572119, -4212},
{43493, 6669}, {194590, 23841}, {235582, -5535}, {147803, 10530}, {23363, 1188},
{24217, 2565}, {69052, 3645}, {12383, 2376}, {30683, -4455}, {30622, 675},
{15067, 1161}, {1586, 81}, {2074, -351}, {1952, -189}, {3782, 189}, {122, 27},
{793, 108}, {2257, -405}, {10553, 1350}, {15067, -2322}, {69235, 11583},
{16043, 3537}, {100162, 5913}, {21899, -2052}, {41053, -2025}, {33733, -4077},
{68137, -7425}, {80032, 7587}, {208925, -432}, {9943, -54}, {427, -81}}

27
— is a relation number with a list
62
{{62, 54}, {124, 27}, {341, 54}, {1054, 135}, {806, 27}, {124, 27}}

27
— is a relation number with a list {{64, 54}, {320, -27}, {1, 0}}
64

27
— is a relation number with a list {{65, 54}, {715, -54}, {1, 0}}
65

27
— is a relation number with a list
67
{{67, 54}, {871, 108}, {469, 54}, {1139, 54}, {335, -27}, {737, -27},
{536, -81}, {2077, 405}, {3484, 459}, {12596, -297}, {8174, -135},
{4087, 810}, {2479, 324}, {7571, -351}, {10117, -945}, {18626, 3267},
{65392, -8073}, {54136, 4509}, {1876, -297}, {6298, 405}, {12194, 2349},
{30083, -216}, {3953, -135}, {2546, 189}, {5963, 648}, {8777, 972},
{1943, 135}, {3551, 459}, {8107, -1350}, {469, 81}, {1139, 81}, {335, 27}}

27
— is a relation number with a list {{68, 81}, {221, 27}, {170, -27}, {136, 27}, {1, 0}}
68

27
— is a relation number with a list {{70, 81}, {770, -27}, {182, 27}, {1, 0}}
70

27
— is a relation number with a list
71
{{71, 81}, {710, -81}, {1349, 108}, {3763, 513}, {12212, -729}, {12851, -1998},
{61273, -2052}, {20377, -1539}, {26270, 621}, {13348, -1593}, {42884, 1053},
{20519, 3267}, {65107, 9126}, {86975, -13554}, {401221, -46872},
{1464517, -13662}, {190493, -28269}, {524690, 11799}, {392914, -58779},
{1316269, 168885}, {2471581, 227826}, {2449855, -337851}, {6027758, -1064961},
{25702568, -2581497}, {7980542, 1195047}, {27319877, -1734345},
{30504653, -4465476}, {53511209, -8540532}, {161029207, 5986818},
{43656409, 6580980}, {171142021, -11674341}, {282089674, -29310093},
{781799176, -110781}, {1253789, -236763}, {4968154, 193509}, {4478680, -113859},
{2710709, 162675}, {3888386, 279531}, {1778408, -234117}, {6711488, -1243485},
{35078473, 5090472}, {39393001, -1893024}, {25595713, -1865430},
{36941797, 6010929}, {62211833, 931581}, {14490674, -15795},
{472789, -42687}, {229472, 23463}, {366218, 5319}, {56303, 7749},
{146260, -6021}, {124676, -783}, {12709, 2403}, {49274, 1971}, {1, 0}}

```

```

27
— is a relation number with a list {{73, 81}, {584, -81}, {1241, 54}, {1, 0}}
73

27
— is a relation number with a list
74
{{74, 81}, {259, 27}, {814, 81}, {148, 27}, {481, -54}, {185, -27}, {148, 27}}

27
— is a relation number with a list {{76, 81}, {190, 27}, {1, 0}}
76

27
— is a relation number with a list {{77, 81}, {308, 27}, {1, 0}}
77

27
— is a relation number with a list {{79, 81}, {158, 27}, {316, 27},
79
{632, 27}, {869, 54}, {395, -54}, {1343, -135}, {553, 81}, {1106, 27}, {1, 0}}

27
— is a relation number with a list {{80, 81}, {1, 0}}
80

27
— is a relation number with a list {{82, 81}, {1, 0}}
82

27
— is a relation number with a list {{83, 81}, {166, 27}, {332, -27},
83
{664, -81}, {1328, 189}, {415, 27}, {830, 81}, {1660, 243}, {3403, -243}, {1, 0}}

27
— is a relation number with a list {{85, 81}, {340, -27},
85
{935, -81}, {3145, -108}, {1105, -54}, {425, 27}, {595, -27}, {1, 0}}

27
— is a relation number with a list {{86, 81}, {215, -27}, {1, 0}}
86

27
— is a relation number with a list {{88, 81}, {308, -27}, {1, 0}}
88

27
— is a relation number with a list
89
{{89, 81}, {712, 81}, {1513, 135}, {2492, -81}, {1691, 27}, {890, 27}, {1, 0}}

27
— is a relation number with a list {{91, 81}, {910, 81}, {247, 27}, {364, -27}, {1, 0}}
91

27
— is a relation number with a list
92
{{92, 81}, {1012, 27}, {1196, 27}, {184, 27}, {230, -27}, {1196, 27}}

27
— is a relation number with a list
94
{{94, 81}, {611, -54}, {1598, -27}, {470, 27}, {1034, -135}, {2162, 135}, {1, 0}}

27
— is a relation number with a list
95
{{95, 108}, {1235, -81}, {380, -27}, {190, 27}, {1, 0}}

```

```

27
— is a relation number with a list
97
{{97, 108}, {1067, -81}, {1358, 81}, {1843, -162}, {5917, 756}, {12707, 945},
{40934, 513}, {10282, -1107}, {30943, -4023}, {120377, -11853}, {179159, -2754},
{14453, -1620}, {12319, -594}, {15035, -972}, {44135, 3996}, {17363, 972},
{12901, -918}, {4753, -405}, {10379, -1161}, {6790, -783}, {24929, -378}, {1843, 243},
{9797, 972}, {7469, 729}, {17363, -1782}, {44329, 108}, {4753, -108}, {1, 0}}

27
— is a relation number with a list {{98, 108}, {490, -27}, {196, 27}, {1, 0}}
98

27
— is a relation number with a list {{100, 108}, {1, 0}}
100

27
— is a relation number with a list
101
{{101, 108}, {707, 54}, {505, 54}, {1919, -189}, {2929, -297}, {4141, 108},
{3737, -81}, {1111, 135}, {3131, 243}, {2828, -351}, {2020, 189}, {5959, 27},
{808, 81}, {202, 27}, {1313, -81}, {1717, 81}, {1616, -27}, {404, 27}, {1, 0}}

27
— is a relation number with a list
103
{{103, 108}, {515, -54}, {2575, 162}, {1751, -162}, {3193, -54}, {721, -81},
{824, -81}, {1442, -27}, {1133, -108}, {5459, 324}, {5047, -297}, {206, 27},
{1030, -81}, {2369, 270}, {6283, 189}, {4738, -405}, {12566, -1107}, {40067, 1512},
{77765, -7344}, {310957, 22815}, {870659, -67635}, {885388, 3645}, {35741, -675},
{3502, -243}, {10300, -729}, {9682, 1053}, {21115, -2241}, {97438, -945}, {1, 0}}

27
— is a relation number with a list {{104, 108}, {1, 0}}
104

27
— is a relation number with a list {{106, 108}, {1, 0}}
106

27
— is a relation number with a list {{107, 108}, {1, 0}}
107

27
— is a relation number with a list {{109, 108}, {1, 0}}
109

27
— is a relation number with a list {{110, 108}, {1, 0}}
110

27
— is a relation number with a list {{112, 108}, {1, 0}}
112

27
— is a relation number with a list
113
{{113, 108}, {565, 54}, {2825, 27}, {1130, -81}, {452, -27}, {791, 27},
{904, 27}, {1469, -108}, {4859, -567}, {27572, -1809}, {49381, -3834},
{52093, -2403}, {87349, 216}, {9605, -837}, {44974, 2133}, {20453, 1566},
{10735, -27}, {1243, 81}, {3164, 81}, {565, -27}, {226, 27}, {1130, 81}}

27
— is a relation number with a list {{115, 108}, {805, -54}, {1, 0}}
115

27
— is a relation number with a list {{116, 108}, {1, 0}}
116

```

```

27
118 is a relation number with a list
    {{118, 108}, {590, 27}, {236, 27}, {826, 27}, {1298, 81}, {1, 0}}

27
119 is a relation number with a list {{119, 108}, {1309, 81}, {1547, 162},
    {8687, 432}, {5593, -621}, {476, -27}, {1190, -27}, {238, 27}, {595, 27}, {1, 0}}

27
121 is a relation number with a list
    {{121, 108}, {1573, 81}, {374, -27}, {484, 27}, {242, 27}, {1, 0}}

27
122 is a relation number with a list
    {{122, 135}, {1586, 27}, {854, -81}, {2257, -54}, {671, 27}, {244, 27}, {1, 0}}

27
124 is a relation number with a list
    {{124, 135}, {341, -27}, {310, 27}, {806, -81}, {1, 0}}

27
125 is a relation number with a list
    {{125, 135}, {250, 27}, {875, -27}, {1375, -108}, {3625, 189},
    {4250, -243}, {14875, -1458}, {7375, 189}, {500, -27}, {325, -27}, {1, 0}}

27
127 is a relation number with a list
    {{127, 135}, {1016, -81}, {4699, 297}, {6731, -513}, {7874, 135}, {5588, 513},
    {6985, 189}, {1016, -27}, {1270, -81}, {3302, -243}, {12700, 1161}, {9017, 162},
    {6985, 216}, {9271, -162}, {4699, 405}, {20447, 729}, {4445, -27}, {1270, -81}}

27
128 is a relation number with a list {{128, 135}, {896, -81}, {640, 27}, {1, 0}}

27
130 is a relation number with a list {{130, 135}, {1, 0}}

27
131 is a relation number with a list
    {{131, 135}, {524, 27}, {1441, -27}, {1310, -27}, {1703, 27},
    {262, 27}, {1048, -81}, {655, -54}, {917, -81}, {3406, -81}, {524, -27}}

27
133 is a relation number with a list {{133, 135}, {266, 27}, {532, -27}, {1064, -81},
    {1463, -81}, {665, 27}, {1330, -81}, {4522, 243}, {665, 54}, {2261, -162}, {1, 0}}

27
134 is a relation number with a list {{134, 135}, {1, 0}}

27
136 is a relation number with a list {{136, 135}, {1, 0}}

27
137 is a relation number with a list
    {{137, 135}, {274, 27}, {548, 27}, {1096, 27}, {1507, -135}, {3014, -81}, {2329, -81},
    {2740, -243}, {9179, -729}, {40826, 3321}, {133438, 7911}, {143713, -7533},
    {80282, -3591}, {175360, -8127}, {470458, 783}, {17125, 729}, {49046, 3213},
    {116587, 3618}, {111107, -7965}, {55211, 3105}, {93023, -3726}, {17399, -459},
    {5891, 189}, {4384, -27}, {1370, 81}, {959, 54}, {1781, -27}, {1, 0}}

```

```

27
139 is a relation number with a list
{{139, 135}, {556, -27}, {1529, -108}, {2363, 135}, {9313, -675}, {19043, 1350},
{19877, -1539}, {18070, -189}, {10286, 297}, {15151, -81}, {556, -27}}

27
140 is a relation number with a list {{140, 135}, {1, 0}}

27
142 is a relation number with a list
{{142, 135}, {994, 81}, {781, 54}, {3550, 243}, {13490, -1161},
{31382, -1107}, {13703, -216}, {6745, 54}, {710, 27}, {568, -27}, {1, 0}}

27
143 is a relation number with a list {{143, 135}, {1144, 81}, {1430, -27}, {1, 0}}

27
145 is a relation number with a list {{145, 135}, {290, 27},
{1015, 54}, {1595, -108}, {725, 27}, {580, -27}, {1885, -54}, {1, 0}}

27
146 is a relation number with a list {{146, 135}, {803, 54}, {511, 27}, {1, 0}}

27
148 is a relation number with a list
{{148, 135}, {1924, -27}, {1036, -27}, {740, 27}, {1628, 135}, {296, 27}, {1, 0}}

27
149 is a relation number with a list {{149, 162}, {1937, 81}, {1043, 27}, {1490, 27},
{745, -27}, {1639, -135}, {2831, -108}, {3427, 54}, {3725, -54}, {1, 0}}

27
151 is a relation number with a list
{{151, 162}, {1661, -108}, {6191, 297}, {6946, -135}, {9211, -621},
{15704, 1107}, {31106, 297}, {11929, -54}, {755, 54}, {1, 0}}

27
152 is a relation number with a list {{152, 162}, {760, -27}, {1, 0}}

27
154 is a relation number with a list {{154, 162}, {308, 27}, {1, 0}}

27
155 is a relation number with a list {{155, 162}, {1085, 27}, {1, 0}}

27
157 is a relation number with a list
{{157, 162}, {785, -54}, {3925, -297}, {10048, 27}, {628, 27}, {1099, 81},
{5495, -432}, {18997, -783}, {32185, -1161}, {50711, -864}, {41605, -297},
{3925, -54}, {2669, 216}, {12089, 648}, {35011, 621}, {36895, 2322}, {40349, 3213},
{222940, -6021}, {25591, 918}, {17741, -729}, {38465, -1998}, {78971, -1323},
{64213, -2106}, {162181, 4050}, {28417, 540}, {31871, -2565}, {171287, 9693},
{500359, 27081}, {2025457, 71793}, {2394721, 152064}, {6013571, -87885},
{5870387, 335853}, {25259102, 601857}, {2966044, -126009}, {9133004, -634959},
{38241746, -1039473}, {34344535, -2181519}, {87883733, -5118066},
{137627927, 1192536}, {76347059, 3411666}, {202593899, 13016727},
{890776081, -52145856}, {674555053, 49546701}, {2998505477, -43833852},
{2795155937, -152176266}, {8789354393, 293046606}, {320874559, 13678524},
{984155599, -52717689}, {2744437244, -218841939}, {15779750191, -920110590},
{21645615277, 719916903}, {7552985359, 20822508}, {876852065, 48382974},

```

```

{935 489 681, 34 748 541}, {427 185 382, -19 110 789}, {1 059 439 768, -85 247 505},
{5 725 744 156, 401 691 339}, {16 024 269 370, -317 079 387}, {23 044 360 619, -1 738 094 058},
{70 514 644 805, 6 033 847 059}, {296 968 624 771, 23 035 721 976},
{391 834 463 969, 22 211 066 754}, {1 250 463 803 671, -46 370 835 882},
{243 156 127 451, 4 122 591 660}, {12 054 536 773, -448 051 284}, {6 727 119 515, -226 431 477},
{10 334 492 815, 4 352 589}, {227 105 053, 19 399 662}, {893 469 887, 27 334 206},
{1 343 749 027, 99 251 001}, {7 185 102 959, 481 103 280}, {4 937 059 837, 32 102 163},
{1 047 702 605, 4 948 749}, {224 852 731, -3 574 773}, {56 200 976, 661 473},
{3 803 953, 163 836}, {5 608 825, -321 273}, {23 107 888, 1 221 723}, {16 461 293, 692 253},
{23 986 303, -1 432 863}, {58 461 776, 3 772 899}, {293 321 687, -12 981 141},
{823 395 292, 55 596 969}, {1 657 801 151, 109 362 258}, {2 726 663 117, -180 039 213},
{4 093 762 754, -105 240 681}, {1 667 937 385, -114 091 713}, {6 819 814 670, 319 883 391},
{16 055 363 063, 521 651 313}, {18 184 939 480, -588 252 861}, {7 991 176 127, 279 026 478},
{15 792 902 395, -351 527 526}, {4 056 295 175, 81 047 007}, {619 337 525, 49 657 374},
{3 681 498 809, 198 719 730}, {14 785 641 577, -685 953 846}, {47 938 856 495, 519 348 537},
{24 930 201 287, 77 890 626}, {816 551 819, 11 756 799}, {837 232 016, -25 956 045},
{1 042 256 432, 47 456 631}, {280 943 650, -10 157 967}, {546 269 882, -2 255 715},
{60 735 764, 982 881}, {31 848 706, -951 669}, {69 649 753, -5 676 237},
{240 980 713, 20 566 737}, {913 760 567, 71 036 568}, {1 525 226 269, 126 161 361},
{1 772 520 109, -6 505 758}, {463 767 481, 15 426 477}, {152 787 847, 4 600 125},
{154 444 354, 5 086 287}, {291 351 808, -3 134 349}, {22 395 893, -902 151},
{24 787 474, 964 845}, {46 863 872, 1 647 783}, {113 973 836, 3 894 183},
{163 677 053, -7 875 495}, {268 209 694, -8 928 603}, {55 201 828, 3 218 913},
{75 408 199, -393 930}, {26 308 333, 1 494 072}, {91 839 191, 2 340 711},
{86 579 534, -4 745 223}, {182 986 640, 10 256 949}, {257 235 394, -17 775 369},
{1 315 695 796, -75 539 061}, {4 950 486 163, 59 372 325}, {3 545 560 516, 175 263 885},
{6 324 402 112, 325 529 145}, {21 877 692 049, -1 565 603 181}, {6 398 140 145, 428 987 232},
{5 756 928 595, -27 932 364}, {449 272 927, 18 638 181}, {307 183 531, 20 668 662},
{446 884 643, -17 163 468}, {634 475, -32 643}, {2 238 506, -120 393}, {7 686 877, 394 443},
{30 216 220, -429 489}, {23 862 430, -1 770 093}, {133 641 697, -2 108 997},
{121 657 102, 3 638 223}, {250 531 651, 11 095 218}, {731 362 991, 18 911 988},
{974 112 937, 46 224 810}, {532 532 539, 22 314 879}, {474 855 449, 8 074 674},
{243 399 769, -11 967 048}, {637 233 013, -15 833 205}, {613 055 641, 44 505 639},
{1 573 658 885, 48 974 787}, {1 015 115 057, 7 788 771}, {404 247 839, -28 528 875},
{760 443 473, -32 618 673}, {1 603 597 058, 118 647 261}, {9 021 941 572, -9 090 873},
{595 902 292, 7 453 107}, {54 364 076, -1 483 299}, {81 323 959, -4 878 090},
{251 760 647, -13 475 376}, {670 625 029, 39 686 490}, {635 112 257, -5 060 691},
{396 563 474, 23 857 281}, {1 414 617 571, -96 420 402}, {4 975 088 063, -262 587 960},
{2 211 058 789, 159 765 588}, {4 028 532 551, -142 218 720}, {7 286 117 387, 226 138 986},
{7 798 164 095, 635 596 632}, {26 847 708 227, -1 788 008 310}, {4 330 621 589, 55 925 613},
{3 822 853 916, 233 686 053}, {13 168 699 676, 453 816 945}, {1 257 298 547, -104 434 245},
{641 754 299, 48 266 496}, {2 243 506 607, -138 679 668}, {3 867 211 283, 174 331 953},
{5 009 605 769, -198 669 267}, {6 731 232 758, 64 139 607}, {537 878 389, 12 732 012},
{492 019 945, -31 831 596}, {2 283 722 785, 108 087 183}, {2 181 034 894, 90 978 201},
{383 383 010, 23 690 313}, {681 066 314, -28 654 587}, {1 043 072 518, 14 222 709},
{755 917 477, 22 990 014}, {432 218 645, 32 766 957}, {980 968 028, 83 367 009},
{3 051 464 560, 30 733 587}, {1 387 793 179, 51 871 779}, {2 000 942 078, 114 796 089},
{7 757 144 705, -653 451 597}, {13 231 090 063, 198 433 044}, {10 036 049 945, -86 979 798},
{5 239 588 475, -139 692 411}, {10 789 533 451, -334 589 805}, {12 977 571 487, 1 032 880 383},
{70 630 138 244, -4 256 624 439}, {271 998 923 383, 13 413 648 141},
{584 975 808 391, -6 676 881 084}, {406 587 139 157, -569 105 217},

```

```

{38624232383, -2998528200}, {55991572069, -1058141691},
{14120195978, 1002896343}, {12504606632, 470141955}, {29708506021, -2284801101},
{956398156, 8636139}, {347483861, 18568710}, {835495753, -41607810},
{524309821, -40335138}, {7374761, 139563}, {3466246, 144531}, {392186, -29511},
{1341251, -20007}, {122774, 4887}, {94043, 7128}, {216503, 2106}, {65155, 5508},
{147737, -918}, {9577, -810}, {22451, -243}, {14915, 324}, {1727, 81},
{4082, 81}, {5024, -243}, {12403, -243}, {1570, -81}, {4867, -162}, {1099, 81}}

27
158 is a relation number with a list {{158, 162}, {1, 0}}

27
160 is a relation number with a list {{160, 162}, {1, 0}}

27
161 is a relation number with a list {{161, 162}, {1, 0}}

27
163 is a relation number with a list {{163, 162}, {1, 0}}

27
164 is a relation number with a list {{164, 162}, {1, 0}}

27
166 is a relation number with a list {{166, 162}, {1, 0}}

27
167 is a relation number with a list
{{167, 162}, {835, 54}, {4175, 243}, {7348, 189}, {3841, 108}, {7849, -270},
{3173, 54}, {2171, 108}, {1837, -81}, {4342, 189}, {835, 27}, {334, 27},
{1670, -81}, {5177, 135}, {7849, -297}, {21209, -1593}, {83500, 3969},
{25217, -1728}, {117401, 3861}, {262357, 8532}, {356545, 16281}, {273379, 21411},
{828988, 43119}, {1624409, 109890}, {3998147, -252234}, {6278699, 503199},
{40131937, -314928}, {22725527, -1154358}, {60392711, -2504034},
{49414465, -2737098}, {24499067, -1588761}, {111497884, 5075973},
{28978174, 314523}, {7023686, 289305}, {13421122, 576531}, {26871803, 700731},
{40752175, -1574073}, {29011741, 201015}, {10952027, -73548}, {1106375, -59859},
{4828471, 152010}, {5986783, -219672}, {9291713, -631152}, {29319689, 1115586},
{52513651, -482220}, {8070943, -372006}, {18902563, 1002942},
{25606945, -1889514}, {141323917, -4334040}, {283800301, -10357416},
{693061523, -48910527}, {1388462215, -86709069}, {186557537, -2655963},
{106901209, 5823333}, {347562905, 17218926}, {531792295, 38273607},
{674379901, 41165010}, {2628536747, 74988558}, {657515239, -20884176},
{1687665761, 59472441}, {3747047971, 238935231}, {12677926075, -957416652},
{38662103033, 2631157614}, {134478616559, -4562285958},
{362778070759, 583890741}, {30380739866, -727369173},
{28183821800, -1559324709}, {19368165346, -502684245}, {39498874903, 929675556},
{75567759017, -3572226549}, {92017248496, -1480226643},
{40613837210, 2321892999}, {190656589909, -12965204844},
{638187619417, -1591510869}, {1375921684, -50697657}, {1183185815, -49594059},
{1180957367, 72079092}, {4624546465, 74309724}, {2896377359, -233743725},
{15272594053, 472346613}, {26302906979, -1916865810}, {89046798287, 3387259836},
{163333106017, 11122266195}, {584648113636, 33060475755},
{1743555142318, 116743524075}, {1268819040769, -8019780570},
{282849688403, -13127870043}, {995896574681, -61830764073},
{1102926368671, 16673737167}, {410772513383, -4803439077},

```



```

{387982288913, -13285455030}, {451583538181, -28355625180},
{351779604733, 14802014601}, {579280530397, -36876963285},
{1795397321221, 62702682174}, {3837737124775, 76684054617},
{590243785475, 18799900389}, {1243627860472, -77465950749},
{696832297496, 19259780157}, {581195377948, 21548813427},
{103971625027, -1358133291}, {100974609460, -1745048043},
{39775564678, 2037926871}, {164156447914, 4689644985}, {3151864313, -58132566},
{2121860083, -102592278}, {5440485085, 420522111}, {4392493786, 79010397},
{5358770482, -198915669}, {1996081027, -21211038}, {374656985, -28992816},
{375687041, -17385408}, {1134253145, -30752784}, {601177121, -15689025},
{834026557, -58057452}, {3544112243, 45408627}, {373969279, 25478334},
{1370357077, -45341775}, {1687339109, 66416787}, {4495545478, 189232659},
{7688402446, -525975903}, {33606428533, 903981033}, {26574762104, 586687671},
{29027423803, -577346346}, {26737786001, -1313577000},
{77863082167, -5360444541}, {424778853316, 2395570599},
{127397167931, 8714498724}, {554492259143, -20946101580},
{1652234216521, -25339023747}, {868011385322, -21501863289},
{1325454578254, 52204707495}, {3396260776793, -67350708063},
{4797137398381, 386208078894}, {27160955426051, -1372633744167},
{48717149367263, 813500218602}, {15508246059119, -459190673028},
{17407549580111, 696197821419}, {434875454212, -26389177515},
{2112318533324, 32670859167}, {1884981192677, 29600409177},
{1577314106717, -97986076596}, {1592659157227, 116055889236},
{5364589776859, -300098008674}, {6208121338591, -69044569992},
{983623435063, -78669329355}, {6526000374184, 476555719437},
{24345209554978, -863768261619}, {26669604350882, -1958177075787},
{124394076592712, 5229696877677}, {186814294746512, 2542374640629},
{203897978759365, -3975474203802}, {191848659032321, -12537786817413},
{631570080778042, 50502390720471}, {4168486764209527, 327411254097774},
{14672543023276345, -116905677115023}, {9614572967164351, -684626840801262},
{4976131723096061, -90233154228132}, {2222476171649767, 22608026242290},
{1150563184192949, 55156433575050}, {1289560787477867, -37482397909362},
{2531596179446353, -120060734242059}, {1723566980640038, 13415527469763},
{1065370573232458, 1201044309147}, {7393260184523, -238942869435},
{2332784249654, -75154711599}, {499027744195, 35419800987},
{526138572959, -39395647701}, {2337190525282, -155298009753},
{1289303290829, -86938780275}, {2467995020432, 154158582213},
{243436739008, 4327915779}, {179267049128, -1820449107},
{144127119214, -1089139527}, {60237175550, 3153645441},
{53091332557, 3057443010}, {186171831629, -1100853963},
{21294484294, -1373108679}, {112767513190, -7705204677},
{469363013155, -3276465876}, {138341612129, -10371210516},
{587151195307, -23276701566}, {874020578219, 69434893170},
{4781716509497, 751201965}, {52772379424, -2530192005},
{60395997727, 2663302194}, {143612106745, -3615713343},
{169743304825, 66505131}, {3709155671, -287636292}, {5029392875, 60273639},
{4455699946, -19659051}, {1153073377, -72589149}, {1394952169, -56296323},
{2080136302, -15178995}, {102535829, 1488132}, {24261593, -1398465},
{81443896, 3472713}, {262439999, -14082795}, {857228702, -4268889},
{136603829, 6163695}, {167424013, 732051}, {36016222, 30105}, {1777214, 142857},
{10509310, 69579}, {481127, 29430}, {1711249, -65232}, {2541239, 199449},

```

```

{8616866, 127521}, {9111854, -671571}, {48453380, 2479437}, {189605120, 15100101},
{1118264231, 9444087}, {644948155, 13066704}, {781503053, 34176087},
{759340316, -60097113}, {3660999551, -26050356}, {2020807715, 103083057},
{6822521975, 433809081}, {19776694607, 1094765814}, {11841962485, 941856363},
{67162429078, -5269664169}, {224315254873, 9636999111},
{444933978440, 26799311457}, {1779270826943, 127179640809},
{207772111961, -8920263591}, {435210244456, -12054028041},
{211294241660, 2496640293}, {153670601915, 5425180524},
{294846389581, 279411849}, {11170443962, -294219189}, {1650831740, 24831603},
{1994972314, -46147941}, {1772012117, 28604232}, {242194589, 272754},
{1830821, 34236}, {2724271, -8451}, {509183, -11826}, {111055, 108},
{5177, -378}, {19205, 1026}, {48263, 324}, {2171, -54}, {1837, -108}, {1, 0}}

27
169 is a relation number with a list
{{169, 162}, {1183, -27}, {845, -27}, {1352, -27}, {338, 27}, {1, 0}}

27
170 is a relation number with a list {{170, 162}, {340, 27}, {374, -27}, {340, 27}}

27
172 is a relation number with a list {{172, 162}, {860, 27}, {1, 0}}

27
173 is a relation number with a list
{{173, 162}, {1903, 108}, {7093, 135}, {10726, 81}, {5882, 243}, {8650, 189},
{7612, 567}, {41693, 486}, {17819, -648}, {55879, 1269}, {7439, 108}, {2249, -81},
{3287, 162}, {8131, 108}, {5363, 270}, {6401, 243}, {14359, -540}, {38233, -2052},
{130615, 8451}, {666050, 6723}, {81829, 918}, {21971, 1080}, {64183, -3483},
{257597, 486}, {2941, 81}, {4325, -162}, {8477, 243}, {4844, 297}, {15916, -783},
{44288, 2781}, {35984, 1863}, {101551, 5319}, {84770, -5913}, {343924, -3105},
{126463, 4266}, {262441, -756}, {18857, -1296}, {100859, 3834}, {203275, -2943},
{35984, 1917}, {75947, 243}, {19376, 297}, {12283, -378}, {32351, 243},
{5536, -297}, {18511, -621}, {20587, 1404}, {81829, -243}, {10726, 189},
{8131, 297}, {19376, -27}, {1730, 81}, {5017, -81}, {865, -27}, {1, 0}}

27
175 is a relation number with a list {{175, 162}, {2275, -81}, {1, 0}}

27
176 is a relation number with a list {{176, 189}, {2288, 81}, {440, 27}, {1, 0}}

27
178 is a relation number with a list
{{178, 189}, {1958, -81}, {1246, -27}, {356, 27}, {445, -27}, {1157, 54},
{4094, 297}, {5696, 351}, {7120, -81}, {712, -27}, {890, 27}, {1, 0}}

27
179 is a relation number with a list {{179, 189}, {1790, -81}, {1432, -27}, {1, 0}}

27
181 is a relation number with a list {{181, 189}, {1448, -81}, {1810, 81}, {5068, 297},
{3439, -108}, {3077, -189}, {9593, 135}, {1448, 27}, {1810, -27}, {1, 0}}

27
182 is a relation number with a list {{182, 189}, {1, 0}}

27
184 is a relation number with a list {{184, 189}, {460, 27}, {1, 0}}

```

```

27
185 is a relation number with a list {{185, 189}, {740, 27},
    {2035, -54}, {3145, -108}, {2405, 27}, {370, 27}, {1480, -27}, {1, 0}}

27
187 is a relation number with a list {{187, 189}, {374, 27},
    {748, 27}, {1496, -81}, {7106, 243}, {11033, -756}, {3377, 27}, {374, 27}}

27
188 is a relation number with a list {{188, 189}, {1, 0}}

27
190 is a relation number with a list {{190, 189}, {1, 0}}

27
191 is a relation number with a list
    {{191, 189}, {382, 27}, {764, -27}, {1528, 27}, {2101, -108}, {9359, 540},
    {34189, 1647}, {76018, -2943}, {95500, -4887}, {427840, 26217},
    {1598288, 36855}, {2582893, 102006}, {6253913, 33804}, {33043, 1242},
    {93781, 1404}, {54817, 3051}, {19291, 837}, {7640, 27}, {1, 0}}

27
193 is a relation number with a list
    {{193, 189}, {772, -27}, {2123, -135}, {7141, 81}, {2509, -162}, {15247, 729},
    {11966, -81}, {4246, 189}, {16984, 837}, {47092, -3159}, {56549, 540}, {29143, 1782},
    {121783, 3186}, {137995, -2862}, {119467, -837}, {43232, -1755}, {124099, -8505},
    {670868, 45981}, {3637471, -223560}, {11678623, -668358}, {61091641, -795609},
    {32858636, 1858005}, {112992622, 4971969}, {262994345, -2999187},
    {180283423, -1239840}, {97778239, -6749163}, {634961701, 29844126},
    {1589365615, -21092292}, {1436636995, -51206256}, {552332611, 7666704},
    {63675139, 958986}, {73738159, -598320}, {27946207, 1811430},
    {149528101, -6007473}, {127133732, 3381669}, {264350170, 13007223},
    {811702030, 12202299}, {1129436579, 15017508}, {602831447, 31025322},
    {2576613497, -139913865}, {11225637911, -306133452}, {19550863909, -1088332686},
    {7551016727, -167402349}, {3456827246, 92385441}, {7443224297, 128628702},
    {3327400867, -154299897}, {12968995331, 750833577}, {39531132746, 1124065917},
    {36443350643, -2281858830}, {12813392941, -567856764},
    {47731337783, 2757298860}, {165450632459, -198018243}, {17875406977, 706951854},
    {38910851011, 354534597}, {16975249187, 443320776}, {24908521907, -1554387057},
    {7397496035, 119328849}, {172272379, 9400779}, {590262901, -2313711},
    {51453028, -264519}, {24738161, -859518}, {36257173, -1497177},
    {62710525, 553014}, {42448999, -160596}, {9969415, -311958}, {2555513, 146718},
    {11832251, 176661}, {778948, 12663}, {1188494, 50031}, {2364250, -64233},
    {2387603, 38340}, {2030939, 12474}, {448339, -24084}, {1786601, -100629},
    {4771153, 64854}, {5412299, 354915}, {17094782, -854847}, {416494, -23841},
    {2161021, -66528}, {6200125, 170721}, {10454617, -689796}, {20781661, 604206},
    {46060801, 624456}, {28745999, 123822}, {3723935, -66744}, {2649697, -92313},
    {5284340, 74169}, {3539813, -46386}, {2794061, 37719}, {551015, 33777},
    {2042519, -53082}, {4902779, 43389}, {34354, -2025}, {13703, -243}, {18335, -729},
    {21230, -1107}, {38021, -891}, {56356, -1485}, {14282, 891}, {5018, -27}, {772, 27}}

27
194 is a relation number with a list {{194, 189}, {485, -27}, {1, 0}}

27
196 is a relation number with a list {{196, 189}, {1, 0}}

```

$\frac{27}{197}$  is a relation number with a list  $\{\{197, 189\}, \{1576, 81\}, \{7289, -27\}, \{1, 0\}\}$   
 $\frac{27}{199}$  is a relation number with a list  $\{\{199, 189\}, \{1990, 81\}, \{6965, -54\}, \{1, 0\}\}$   
 $\frac{27}{200}$  is a relation number with a list  $\{\{200, 189\}, \{2200, 81\}, \{1300, 27\}, \{1, 0\}\}$   
 $\frac{27}{202}$  is a relation number with a list  
 $\{\{202, 189\}, \{2626, -81\}, \{3434, 81\}, \{3232, -27\}, \{808, 27\}, \{1, 0\}\}$   
 $\frac{27}{203}$  is a relation number with a list  $\{\{203, 216\}, \{2639, 27\}, \{1, 0\}\}$   
 $\frac{27}{205}$  is a relation number with a list  $\{\{205, 216\}, \{2255, -27\}, \{2665, -81\},$   
 $\{1640, -27\}, \{1435, 54\}, \{4715, 108\}, \{7585, -162\}, \{5945, 324\}, \{23165, -702\}, \{1, 0\}\}$   
 $\frac{27}{206}$  is a relation number with a list  
 $\{\{206, 216\}, \{1030, 27\}, \{412, 27\}, \{1442, 81\}, \{1648, 81\}, \{2884, 27\}, \{1030, -27\}\}$   
 $\frac{27}{208}$  is a relation number with a list  $\{\{208, 216\}, \{1, 0\}\}$   
 $\frac{27}{209}$  is a relation number with a list  $\{\{209, 216\}, \{1463, 27\},$   
 $\{1045, -27\}, \{1672, 27\}, \{418, 27\}, \{2717, 27\}, \{2090, 27\}, \{1, 0\}\}$   
 $\frac{27}{211}$  is a relation number with a list  $\{\{211, 216\}, \{1055, 54\}, \{5275, 81\},$   
 $\{2110, 81\}, \{844, 27\}, \{1477, 27\}, \{1688, -81\}, \{2743, -108\}, \{9073, 432\}, \{1, 0\}\}$   
 $\frac{27}{212}$  is a relation number with a list  $\{\{212, 216\}, \{1, 0\}\}$   
 $\frac{27}{214}$  is a relation number with a list  $\{\{214, 216\}, \{1, 0\}\}$   
 $\frac{27}{215}$  is a relation number with a list  $\{\{215, 216\}, \{1, 0\}\}$   
 $\frac{27}{217}$  is a relation number with a list  $\{\{217, 216\}, \{1, 0\}\}$   
 $\frac{27}{218}$  is a relation number with a list  $\{\{218, 216\}, \{1, 0\}\}$   
 $\frac{27}{220}$  is a relation number with a list  $\{\{220, 216\}, \{1, 0\}\}$   
 $\frac{27}{221}$  is a relation number with a list  
 $\{\{221, 216\}, \{1105, -54\}, \{5525, 216\}, \{1547, -81\}, \{1768, 27\}, \{1, 0\}\}$

```

27
223 is a relation number with a list
{{223, 216}, {1561, -27}, {1115, -54}, {4237, 243}, {23638, -189}, {2899, -27},
{2230, -81}, {8474, -405}, {6913, -81}, {6244, 81}, {1561, -81}, {4906, -243},
{10258, 459}, {35680, -1323}, {9143, -540}, {8251, -459}, {2453, -108},
{6913, -189}, {17840, -1053}, {13603, -702}, {59095, 864}, {76489, -1809},
{113953, -3294}, {298151, 12582}, {851191, -23193}, {1549850, -82161},
{2499607, -139320}, {1818119, 29889}, {1139530, -42687}, {2903237, 28350},
{2572751, 92070}, {1161607, 2268}, {87193, -972}, {64001, -216}, {14495, -783},
{85186, -729}, {23861, 783}, {82733, 4320}, {145619, -6345}, {70468, -1377},
{53743, -1242}, {75151, -3996}, {172379, -6345}, {237272, -7263},
{536761, -5076}, {288785, 13068}, {287447, -9288}, {107263, 6291},
{70468, 3645}, {270499, -5940}, {611243, -7506}, {726311, -2997}, {231251, 3645},
{360368, -16173}, {1017326, -34533}, {3538787, 11475}, {1000601, 14796},
{1232521, -16470}, {608567, -11340}, {845839, -31455}, {768458, 36315},
{1302989, 52434}, {1753003, -19197}, {1354948, -15579}, {94775, -2808},
{155431, 5157}, {160783, 1458}, {89869, -1296}, {99235, -648}, {20293, 459},
{21631, 216}, {6913, -378}, {24307, 1053}, {19624, -405}, {41032, -891},
{10258, 27}, {446, 27}, {2899, -54}, {3791, 108}, {2453, 27}, {892, 27}, {1, 0}}

27
224 is a relation number with a list {{224, 216}, {1, 0}}

27
226 is a relation number with a list {{226, 216}, {1130, -27}, {452, 27},
{791, -27}, {904, -27}, {2938, -135}, {3616, 135}, {6554, 27}, {791, -27}}

27
227 is a relation number with a list
{{227, 216}, {2497, 27}, {2951, 162}, {7945, -81}, {1589, -54}, {5221, 162},
{8399, -189}, {18841, -324}, {11123, 540}, {49259, 459}, {33142, 1701},
{186821, 8370}, {608587, 17928}, {219055, -5076}, {178649, -4806}, {187729, 3159},
{305996, -10827}, {644680, -3969}, {386354, 18117}, {1338619, -27135},
{2043908, -81945}, {1070759, 7101}, {338684, -567}, {41995, 1161}, {45173, 270},
{18841, 783}, {11123, 459}, {24289, 189}, {20884, -675}, {9307, 459}, {28829, 1323},
{62879, -1161}, {41995, 1188}, {94205, 756}, {66965, 3618}, {403379, -5643},
{618802, -29727}, {1240555, -39501}, {3637448, 118881}, {10864901, 152334},
{11165449, 50544}, {1083925, 837}, {2270, -81}, {454, 27}, {1135, -54}, {1, 0}}

27
229 is a relation number with a list
{{229, 216}, {2977, -27}, {1603, 54}, {3893, 27}, {1145, -27}, {2519, 54},
{4351, -54}, {5267, -54}, {5725, 216}, {24503, -351}, {15343, 783},
{72593, 432}, {3893, -216}, {1145, -54}, {2519, 108}, {8015, 162}, {17633, -324},
{31373, -216}, {12137, 621}, {64807, 2970}, {122057, -3753}, {410368, -11475},
{625628, -27729}, {2779831, 122634}, {9331979, 524016}, {22970761, -832572},
{78147395, -2832597}, {266858509, -12072294}, {290381389, 8650341},
{854216945, 33382611}, {3144385489, 140825628}, {10584763117, -198545634},
{14162393935, -382298751}, {3970893892, 3993273}, {361941370, 18299007},
{924878330, -46694583}, {2064052570, -14776533}, {1067609450, -14808393},
{321780266, -14536935}, {450602384, 18092781}, {393225289, -16957026},
{735935239, 21475611}, {1320062485, -62582841}, {1333426696, -24792021},
{1223418302, 51785595}, {4450838962, 210841083}, {5307354151, 99248706},
{10802555857, -197994564}, {19956242327, 635286537}, {60080366720, -3277321587},

```

```

{249 284 397 266, 13 675 220 685}, {716 867 310 344, 4 331 025 801},
{477 000 730 438, 20 519 785 863}, {1 155 455 129 881, 67 119 131 925},
{3 304 444 158 724, 175 610 035 557}, {7 361 552 360 711, -288 724 203 675},
{32 849 424 563 444, -275 546 245 851}, {13 607 479 343 075, -529 453 844 604},
{36 255 421 208 041, 1 554 544 242 792}, {114 706 929 855 925, 4 356 287 674 218},
{330 550 124 712 853, -15 712 251 636 492}, {135 760 439 353 309, 3 399 480 358 407},
{50 099 471 100 359, 1 233 037 233 441}, {104 207 702 795 338, 223 920 860 373},
{19 351 123 313 497, 1 083 260 220 975}, {33 791 392 068 137, -1 050 038 978 553},
{43 543 148 766 989, 834 767 296 992}, {30 972 095 059 745, 1 271 660 950 548},
{103 561 184 469 797, -1 836 138 116 772}, {168 876 034 099 385, -2 341 518 110 433},
{65 661 203 939 861, -2 029 381 175 790}, {165 110 446 039 049, 2 483 802 592 578},
{270 099 758 718 329, -4 434 021 745 524}, {86 005 016 727 415, 1 358 031 410 496},
{102 829 671 352 243, -4 235 389 045 650}, {270 296 544 771 247, -13 833 343 573 020},
{1 458 804 811 816 037, 71 856 907 293 222}, {4 961 666 502 915 713, 75 232 310 740 506},
{839 515 364 309 407, -5 303 170 381 140}, {369 707 696 446 723, 6 093 714 219 912},
{460 031 451 651 161, 14 766 863 112 270}, {517 241 194 111 139, 27 449 324 085 195},
{983 775 643 232 614, -22 380 421 478 427}, {220 504 516 361 846, 3 441 747 692 277},
{53 280 068 851 022, 2 919 032 133 183}, {168 885 313 903 712, -8 557 878 023 397},
{520 344 463 208 212, -3 466 964 135 079}, {68 664 034 716 898, -550 350 859 239},
{29 729 395 546 733, -157 305 947 913}, {327 151 420 696, -3 595 251 555},
{3 771 815 261, 150 984 702}, {641 724 181, 1 947 213}, {196 048 961, -6 727 860},
{215 493 809, 9 181 647}, {988 347 512, 5 056 155}, {548 978 723, -7 221 987},
{24 665 819, 929 070}, {95 967 259, 2 226 393}, {53 210 440, 1 672 677}, {72 186 296, -45 873},
{4 077 574, -71 847}, {4 054 445, 199 773}, {13 507 565, -437 238}, {10 720 177, 275 373},
{4 435 730, 221 373}, {1 893 830, 7587}, {668 680, -2943}, {141 751, -5427},
{148 621, 1350}, {27 709, -1215}, {54 044, -2133}, {164 651, -3132}, {308 005, -9072},
{101 447, -3726}, {193 505, -9099}, {555 554, 12 393}, {487 999, -18 684},
{507 235, 27 324}, {2 729 909, -141 723}, {8 512 388, -337 959}, {14 521 577, -345 816},
{617 155, 23 544}, {1 147 519, -20 304}, {2 246 261, -117 558}, {2 898 911, 80 865},
{2 800 441, -27 837}, {2 540 984, 83 241}, {9 042 523, 128 493}, {10 994 977, -391 176},
{9 629 221, 111 213}, {10 604 990, -460 377}, {3 737 051, -119 826}, {5 139 905, -169 479},
{12 717 515, 174 879}, {11 141 308, -639 171}, {63 066 829, 2 346 381}, {65 369 882, 2 194 371},
{105 625 792, -4 363 119}, {208 604 344, 9 251 901}, {959 367 791, 30 466 098},
{3 416 394 437, 129 028 815}, {14 116 761 563, -411 991 407}, {24 973 303 025, -123 613 803},
{759 093 551, -25 525 179}, {1 525 556 551, 89 454 375}, {1 106 568 304, 1 457 811},
{20 553 895, -588 411}, {9 272 210, 278 829}, {16 225 337, 721 818}, {79 083 089, -2 539 404},
{82 798 385, 4 211 784}, {329 140 555, 5 675 589}, {9 986 003, 127 575}, {8 050 037, -208 386},
{17 636 893, -107 163}, {10 305 458, 239 247}, {4 084 673, -114 723}, {10 386 295, 555 282},
{37 570 427, 1 301 751}, {41 300 608, -1 061 235}, {20 050 553, -473 202},
{40 319 801, 975 591}, {73 410 530, -1 629 801}, {15 912 065, 118 476}, {8 308 349, -297 432},
{4 522 063, -133 704}, {5 466 917, -321 192}, {1 523 537, -83 889}, {3 099 515, 158 004},
{13 869 385, -207 306}, {4 606 793, 218 241}, {5 434 628, -2403}, {219 382, 7101},
{171 521, -8289}, {583 492, -28 107}, {1 546 895, 53 028}, {2 080 007, -118 638},
{12 704 233, 206 280}, {19 494 083, 1 028 889}, {12 551 032, -324 837}, {26 932 919, 1 351 242},
{21 049 909, 798 957}, {63 439 183, 3 447 657}, {316 330 753, 6 284 034},
{487 553 137, 1 933 011}, {99 469 585, -2 998 971}, {115 311 118, 6 612 975},
{661 934 347, 31 522 716}, {9 775 781, 50 625}, {1 180 724, 38 529}, {3 131 575, 38 259},
{1 296 827, -45 954}, {2 316 335, 127 629}, {4 353 977, -33 966}, {1 449 341, 82 404},
{7 770 199, 368 361}, {7 927 522, 232 929}, {1 817 344, -12 987}, {191 444, -5481},
{89 539, -1134}, {10 763, -459}, {47 174, 567}, {25 877, -1350}, {51 983, -2700},
{156 407, 8694}, {19 465, 1134}, {42 823, 2187}, {209 993, -5643}, {275 258, 5913},

```

```

{607537, 6912}, {164651, 9018}, {532883, -8235}, {547768, 12879}, {1380641, -19197},
{353347, -19953}, {1329803, 22356}, {2472971, -128790}, {5945069, -53136},
{1411327, 20871}, {1809329, -86265}, {512044, 13041}, {788905, 9909},
{873635, -3051}, {240221, 9396}, {933175, 48816}, {1298659, 1323}, {120683, -4158},
{23129, -459}, {40991, 1215}, {73051, -2619}, {64349, 378}, {20381, 54}, {5267, -54}}

27
230 is a relation number with a list {{230, 243}, {2990, -81}, {1610, -81}, {1, 0}}

27
232 is a relation number with a list {{232, 243}, {1276, 27}, {1624, 27}, {1, 0}}

27
233 is a relation number with a list {{233, 243}, {2330, 81}, {4427, 108}, {1, 0}}

27
235 is a relation number with a list {{235, 243}, {1880, -81},
{3995, -216}, {25145, 1242}, {14335, 729}, {2303, 27}, {1880, 81}}

27
236 is a relation number with a list {{236, 243}, {1652, -81}, {1888, -27}, {1, 0}}

27
238 is a relation number with a list {{238, 243}, {595, -27}, {1, 0}}

27
239 is a relation number with a list
{{239, 243}, {956, 27}, {2629, -81}, {8843, -378}, {35611, -1836}, {173753, -6966},
{94883, 3429}, {269831, 3510}, {104921, 2673}, {161086, 1917}, {13862, -675},
{74807, 756}, {8843, 135}, {16013, 297}, {5975, -108}, {8365, -297},
{11711, 459}, {53297, -1323}, {90103, -648}, {7409, -27}, {2629, 81}}

27
241 is a relation number with a list {{241, 243}, {482, 27}, {964, -27},
{1928, 27}, {2651, -27}, {1205, -27}, {2410, 27}, {1687, 81}, {3374, 135}, {1, 0}}

27
242 is a relation number with a list {{242, 243}, {1, 0}}

27
244 is a relation number with a list {{244, 243}, {1, 0}}

27
245 is a relation number with a list
{{245, 243}, {490, 27}, {980, 27}, {1960, -81}, {3920, 27}, {1, 0}}

27
247 is a relation number with a list
{{247, 243}, {988, -27}, {2717, 135}, {4199, -162}, {1, 0}}

27
248 is a relation number with a list {{248, 243}, {620, 27}, {1, 0}}

27
250 is a relation number with a list {{250, 243}, {1750, 81}, {4000, -189},
{3875, -189}, {5875, -243}, {5375, -189}, {20750, -189}, {1000, -27}, {1, 0}}

27
251 is a relation number with a list
{{251, 243}, {2008, 81}, {4267, -135}, {13303, -459}, {2008, 81}}

```

$\frac{27}{253}$  is a relation number with a list  $\{(253, 243), \{2530, -81\}, \{4807, 27\}, \{1, 0\}\}$   
 $\frac{27}{254}$  is a relation number with a list  $\{(254, 243), \{1397, -27\}, \{889, 27\}, \{1, 0\}\}$   
 $\frac{27}{256}$  is a relation number with a list  $\{(256, 243), \{3328, 81\}, \{896, -27\}, \{1280, -27\}, \{2816, -81\}, \{608, 27\}, \{832, 27\}, \{1280, -27\}\}$   
 $\frac{27}{257}$  is a relation number with a list  $\{(257, 270), \{3341, 108\}, \{1799, 27\}, \{2570, 81\}, \{5654, -27\}, \{2827, -108\}, \{4883, -54\}, \{5911, -216\}, \{20303, -54\}, \{1, 0\}\}$   
 $\frac{27}{259}$  is a relation number with a list  $\{(259, 270), \{2849, -135\}, \{518, 27\}, \{1295, -27\}, \{1, 0\}\}$   
 $\frac{27}{260}$  is a relation number with a list  $\{(260, 270), \{1, 0\}\}$   
 $\frac{27}{262}$  is a relation number with a list  $\{(262, 270), \{524, 27\}, \{1441, -27\}, \{1310, -27\}, \{1703, 27\}, \{1, 0\}\}$   
 $\frac{27}{263}$  is a relation number with a list  $\{(263, 270), \{1841, 54\}, \{1315, 27\}, \{2104, 27\}, \{526, 27\}, \{3419, 81\}, \{4471, 189\}, \{17095, -567\}, \{22355, 54\}, \{1, 0\}\}$   
 $\frac{27}{265}$  is a relation number with a list  $\{(265, 270), \{1, 0\}\}$   
 $\frac{27}{266}$  is a relation number with a list  $\{(266, 270), \{1, 0\}\}$   
 $\frac{27}{268}$  is a relation number with a list  $\{(268, 270), \{1, 0\}\}$   
 $\frac{27}{269}$  is a relation number with a list  $\{(269, 270), \{1, 0\}\}$   
known cases  
known cases  
 $\frac{28}{9}$  is a relation number with a list  $\{(9, 28), \{171, 280\}, \{981, 532\}, \{747, -140\}, \{423, 56\}, \{225, 196\}, \{261, 140\}, \{171, -196\}, \{75, -112\}, \{333, -28\}, \{1, 0\}\}$   
 $\frac{28}{11}$  is a relation number with a list  $\{(11, 28), \{187, 168\}, \{209, 252\}, \{473, -364\}, \{1199, -952\}, \{2717, 3360\}, \{7073, -952\}, \{4499, 980\}, \{4411, 448\}, \{759, 868\}, \{1199, -392\}, \{253, 196\}, \{627, 560\}, \{737, 532\}, \{2255, 112\}, \{165, -28\}, \{33, -28\}, \{55, -28\}, \{1, 0\}\}$   
 $\frac{28}{13}$  is a relation number with a list  $\{(13, 28), \{195, 56\}, \{351, -28\}, \{1, 0\}\}$   
 $\frac{28}{15}$  is a relation number with a list  $\{(15, 28), \{195, -56\}, \{135, -28\}, \{1, 0\}\}$   
No answers up to 5000 iterations for  $\frac{28}{17}$



```

28
— is a relation number with a list {{19, 28}, {171, -28}, {57, -28}, {1, 0}}
19

28
— is a relation number with a list
23
  {{23, 28}, {115, 56}, {69, 28}, {299, -84}, {851, -140}, {253, -140}, {621, 196},
  {759, -112}, {575, -224}, {2231, -280}, {207, -112}, {391, 196}, {1, 0}}

28
— is a relation number with a list {{25, 28}, {75, -28}, {225, -56}, {1, 0}}
25

28
— is a relation number with a list {{27, 28}, {1, 0}}
27

28
— is a relation number with a list {{29, 28}, {1, 0}}
29

28
— is a relation number with a list
31
  {{31, 28}, {93, 28}, {279, 112}, {1705, 392}, {4247, 644}, {8091, 1960}, {7781, -2492},
  {9455, -392}, {1457, -308}, {2573, 252}, {1643, 392}, {2325, -448}, {2635, 392},
  {3379, 56}, {589, 140}, {899, 280}, {1829, 420}, {4619, 504}, {2573, -644}, {93, -28}}

28
— is a relation number with a list {{33, 28}, {165, -56}, {1, 0}}
33

28
— is a relation number with a list {{37, 28}, {333, 28}, {111, -28}, {1, 0}}
37

28
— is a relation number with a list
39
  {{39, 28}, {429, -140}, {117, 28}, {195, -28}, {1, 0}}

28
— is a relation number with a list {{41, 28}, {533, 56}, {1107, -28}, {533, 56}}
41

28
— is a relation number with a list {{43, 56}, {559, 140}, {1, 0}}
43

28
— is a relation number with a list {{45, 56}, {495, -56}, {1, 0}}
45

28
— is a relation number with a list
47
  {{47, 56}, {423, -112}, {1175, -336}, {7849, -1764}, {37271, 5908},
  {85681, 22456}, {194721, -11396}, {46483, -9464}, {39339, -476}, {7943, -1288},
  {10105, -336}, {1175, 308}, {2679, -112}, {423, -28}, {141, 28}, {1, 0}}

28
— is a relation number with a list
51
  {{51, 56}, {255, -56}, {1275, 56}, {663, 56}, {153, -28}, {663, 28}, {153, 28}}

28
— is a relation number with a list {{53, 56}, {159, -28}, {477, -28}, {1, 0}}
53

28
— is a relation number with a list {{55, 56}, {1, 0}}
55

28
— is a relation number with a list {{57, 56}, {1, 0}}
57

```

28  
 — is a relation number with a list  
 59

{ {59, 56}, {177, 28}, {531, -112}, {1711, 112}, {1829, -336}, {8791, 1036},  
 {29677, 4788}, {55991, -9800}, {165731, 27636}, {5015, -224},  
 {5133, -1036}, {2773, 588}, {9853, -1960}, {3127, 112},  
 {531, -56}, {1593, -280}, {5133, -532}, {11033, -28}, {1, 0} }

28  
 — is a relation number with a list  
 61

{ {61, 56}, {305, 56}, {1525, -84}, {793, -28}, {549, 56}, {671, -28}, {1, 0} }

28  
 — is a relation number with a list { {65, 56}, {585, 112}, {325, 56}, {715, 56}, {1, 0} }  
 65

28  
 67 is a relation number with a list

```
{ {67, 56}, {737, 56}, {603, -28}, {871, 56}, {1675, -252}, {5963, -560},
  {13199, -1092}, {6365, 1316}, {14405, 2128}, {32897, -5096}, {155507, -16492},
  {474293, 84308}, {2114185, -347396}, {1997203, 94724}, {535933, 75292},
  {595563, 66724}, {331851, -32620}, {378617, 29652}, {459553, -66164},
  {240865, 3948}, {2479, 336}, {8509, 1176}, {18559, 1232}, {5293, 700},
  {20569, -3920}, {64923, 8680}, {278921, -1260}, {30887, 5936}, {80869, -7840},
  {165423, 27776}, {82611, 3304}, {737, -84}, {1273, -224}, {4757, -896},
  {18559, 2016}, {27805, -4368}, {106999, 20356}, {349673, 48664}, {604675, -24612},
  {711875, -135996}, {2136965, -181132}, {2453473, -168140}, {4598009, -263956},
  {7420719, 922124}, {2929709, 564508}, {7180323, -1187480}, {3714681, -388556},
  {11448893, 2110192}, {60161511, -9469880}, {223929477, 20595316},
  {175472933, 13421296}, {66737695, 6734672}, {40804675, -7852824},
  {103217185, -8512728}, {71318083, -4065908}, {125173487, 10859296},
  {344250355, -8243732}, {133088063, -3858876}, {126380693, 5534368},
  {60954657, 11301164}, {298072079, 9773372}, {326351573, -27112736},
  {66915647, 1155308}, {6178539, 56644}, {290981, 25424}, {758239, 119028},
  {2952757, 570948}, {6567139, -169148}, {1985411, -283220}, {192357, -4172},
  {29815, -5404}, {174803, -3192}, {50719, 1904}, {46163, 7476}, {87569, -11452},
  {271149, -25928}, {795223, -75516}, {2375351, 96152}, {1906083, -69608},
  {1786689, -183680}, {3357437, -321412}, {9602239, -1470224}, {46185043, 1998948},
  {14019013, -820400}, {4838271, -373772}, {1391255, 41664}, {1094981, 45864},
  {385585, -11228}, {256811, -1008}, {15343, -2996}, {24321, 2548}, {77653, -8456},
  {103783, -2716}, {38525, -4872}, {30217, -1904}, {16549, 3080}, {76983, 13328},
  {199995, 26404}, {752879, 118748}, {2706197, 39480}, {1200841, -135940},
  {1515473, 241332}, {4521227, -835968}, {22872929, 1343160}, {2627003, -32144},
  {589935, -65212}, {202809, 38108}, {822023, 148512}, {4626283, -283444},
  {6108993, -1119664}, {34215091, -3523268}, {68178463, 8119020},
  {216162301, 1955436}, {59703365, -6260912}, {194685585, 12675404},
  {305153175, -43434832}, {74326517, 9678088}, {207578529, -41187244},
  {110034703, -466228}, {327965, 12404}, {365887, 66528}, {2227549, -197204},
  {3906435, -152348}, {3659071, -496832}, {12143549, 2236668},
  {64334003, -11458356}, {295880911, 25799508}, {809783641, 36481816},
  {481307163, 30562168}, {515064175, 104841744}, {612684515, -111120828},
  {3620710351, -120567944}, {246026077, 44480324}, {1397343089, -60360328},
  {606721515, 12742184}, {328522239, -29969072}, {76216051, 1284332},
  {29511021, -280504}, {3892767, 728168}, {16879109, -590436}, {16316845, -1354668},
  {4075543, -492520}, {9070661, 1117676}, {8659951, -1116472},
  {18212275, -1307376}, {6096263, 972664}, {17438693, -421820}, {9652891, -23632},
  {739345, -38444}, {596903, -81228}, {1896569, 105896}, {640453, 131572},
  {1166269, -42196}, {1019673, -155792}, {4748357, 516124}, {6917147, -108668},
  {2519535, -89824}, {299021, -19936}, {1273, -140}, {871, 84}, {2077, 420},
  {1541, 196}, {1809, -280}, {8643, -700}, {16281, 728}, {17755, -3164},
  {82343, 5516}, {26599, -2744}, {56347, -4536}, {128305, 17808}, {244483, -32928},
  {937129, 143640}, {4579517, -54740}, {1249081, 13552}, {153899, 7560},
  {180833, -22484}, {64387, 420}, {8509, -308}, {7705, 1316}, {12797, -2604},
  {14941, -364}, {1139, -112}, {1273, -56}, {1005, -28}, {201, 28}, {335, 56}, {1, 0}}
```

28  
— is a relation number with a list  
69

{ {69, 56}, {897, -140}, {1311, -28}, {345, -28}, {207, 28}, {253, 28}, {1, 0} }

28  
— is a relation number with a list  
71

{ {71, 84}, {923, -140}, {4047, 364}, {3053, 560}, {17963, -2744}, {88395, -14336},  
{168909, -18676}, {58575, -9296}, {198729, -33040}, {34719, -4508},  
{95495, 18788}, {110405, -15792}, {9869, 336}, {8875, -644}, {10011, -1652},  
{7029, -868}, {6035, 252}, {923, -56}, {1917, -196}, {3053, -532},  
{9869, -1148}, {32873, 3724}, {45653, 5656}, {28755, 4676}, {49629, -728},  
{8875, 812}, {4047, -196}, {4899, 392}, {13845, 532}, {923, -84}, {1, 0} }

28  
— is a relation number with a list  
73

{ {73, 84}, {803, 28}, {657, -28}, {949, 140}, {2263, 196}, {6497, 644}, {4161, 728},  
{15111, -980}, {30003, -2492}, {7227, 1036}, {1825, -28}, {365, 56}, {1971, -308},  
{8979, 1624}, {55845, 9968}, {289299, 49084}, {379965, 60368}, {1296261, -67900},  
{449753, 46032}, {771391, -105700}, {2298843, 219632}, {7484179, -1190728},  
{24806203, -1290772}, {20552055, 369404}, {9823537, -590968}, {16273087, -551460},  
{19762049, 2356760}, {66281737, -5918444}, {86056269, -2943920},  
{49828997, -4668748}, {111487863, -1281140}, {2093859, -360836},  
{5194461, 439880}, {6139227, 855568}, {10968323, -648956}, {4666817, 833476},  
{24384847, 4627896}, {90911791, -10866352}, {290611175, -12972596},  
{380626599, -71036924}, {1857264467, -199067568}, {4792913915, 175091056},  
{4778244419, -47611900}, {1244972587, -133002576}, {3500306419, -311105060},  
{5705005407, -828456860}, {6876060749, -182691992}, {4835151131, 354465804},  
{9298019125, -911459192}, {13390185965, 230981604}, {492535891, -47966128},  
{939846603, 103363736}, {698827467, 40337192}, {955949819, 11289544},  
{267283733, -3978408}, {53318981, -4108160}, {6358227, -73276},  
{1225305, 179368}, {2209783, -380044}, {5145113, 114660}, {1064851, -201460},  
{4201223, -203728}, {5625745, -232596}, {3171193, 49364}, {868481, -60704},  
{1359625, -259392}, {4574545, 365204}, {12636811, 2422084}, {38426543, -55244},  
{1699513, 121604}, {214839, 22540}, {770953, 128828}, {147095, 17696},  
{403471, 53760}, {1942457, -199220}, {3631239, 615020}, {4298313, -382424},  
{6690377, 310940}, {10972119, -1656200}, {45353513, -868476}, {14071553, 1368948},  
{27891329, 3650808}, {96004855, -8742524}, {11892357, -399028},  
{5729259, 561232}, {8536547, -1595860}, {40679031, -7277368},  
{217917921, 29738128}, {711824825, -13346256}, {326547761, 27732880},  
{456016327, 74424224}, {691381759, 129217872}, {3306345127, 555594452},  
{1987175705, -161562856}, {3534764609, 408112628}, {10092180139, 1175563788},  
{35616258569, -3849972420}, {70554995597, -10426085740},  
{177215134559, 13402047456}, {218161787063, -25792459728},  
{863013974447, 103264792008}, {2693381601959, 306784693516},  
{4940686697005, 345412307492}, {7658750624541, -1223328366568},  
{23270971034709, -44451722224}, {1586392978691, 202578228972},  
{2498998275205, -410412419256}, {2666234455837, -302813754460},  
{4313521404119, 596886389288}, {9878117574519, -1893697760584},  
{29902900326727, -604669265368}, {20009761629735, 1909006008896},  
{67138212476575, 10599222940908}, {258629862672271, -19860687486164},  
{32187550706147, -5358732882608}, {2566198966427, -422189323500},  
{2413600856171, -269585120952}, {924561964981, 175255938116},

```

{3 524 606 031 273, 626 550 333 416}, {17 132 805 753 279, 262 235 628 340},
{6 386 763 516 067, -454 539 235 276}, {1 694 638 220 819, -31 454 869 264},
{286 504 518 901, -11 529 572 684}, {126 640 268 527, 15 894 863 208},
{37 860 511 001, 1 422 172 696}, {39 285 080 743, 1 659 144 228},
{39 009 793 217, -1 416 245 348}, {47 090 586 471, -4 986 946 132},
{161 189 203 659, 6 908 907 908}, {166 755 489 575, -7 337 800 316},
{147 015 991 589, 28 152 164 432}, {456 627 368 317, -46 628 924 608},
{705 317 076 699, -113 012 009 348}, {1 988 886 504 603, 141 589 665 784},
{484 076 404 771, -61 650 324 904}, {666 212 195 653, -99 128 290 352},
{2 021 066 087 203, 259 534 319 324}, {4 030 218 119 397, -395 960 267 948},
{5 154 927 113 941, 753 385 204 936}, {8 670 160 404 603, 1 537 076 650 508},
{40 317 863 386 485, -3 955 893 791 864}, {55 401 559 152 685, 8 718 536 589 168},
{225 594 792 090 421, 30 746 605 944 572}, {756 904 184 924 441, -78 053 073 211 652},
{1 724 737 945 021 767, -256 015 547 953 312}, {4 918 075 017 553 441, -174 714 381 804 984},
{1 903 279 872 013 897, -343 722 213 152 668}, {11 610 898 703 854 103, -1 629 250 799 409 884},
{15 048 446 882 898 795, 2 276 839 138 208 488}, {64 928 177 172 925 333, 8 118 451 484 662 092},
{1 418 733 419 112 419, -43 952 687 512 440}, {894 061 566 146 747, -122 196 672 394 692},
{2 823 994 735 024 919, -254 948 582 818 244}, {1 427 903 653 769 155, 10 181 925 339 908},
{177 689 751 288 555, -6 424 154 253 496}, {159 619 450 081 309, -20 827 928 785 384},
{511 290 554 728 699, -48 452 763 861 880}, {1 583 358 885 894 613, -106 842 660 415 568},
{1 407 514 484 740 211, 241 354 237 484 920}, {2 964 598 632 359 557, -562 264 465 289 380},
{11 189 170 331 623 961, 1 872 059 689 419 220}, {3 152 709 757 069 207, -14 142 651 343 184},
{80 408 949 640 225, 14 634 514 250 132}, {528 255 622 438 245, 55 226 565 720 536},
{1 752 732 537 999 395, 2 146 543 276 192}, {72 512 261 411 237, 10 179 873 948 776},
{91 479 495 195 765, 6 282 261 615 308}, {201 073 319 471 415, 4 138 979 770 156},
{126 778 316 434 717, -10 381 726 494 916}, {160 424 690 187 925, -19 472 939 565 268},
{338 805 677 602 013, 7 956 900 795 984}, {243 897 133 646 827, -19 556 245 056 600},
{673 220 086 636 771, 121 722 529 429 536}, {4 169 401 565 652 485, 709 590 461 638 632},
{6 434 307 905 089 411, 26 924 357 812 380}, {44 793 681 066 857, -6 828 394 750 212},
{219 370 999 477 771, -6 380 990 251 860}, {176 465 156 760 763, 7 984 570 862 296},
{58 735 638 688 323, -2 873 518 355 120}, {92 364 825 772 379, 2 798 786 511 304},
{355 575 652 331, 6 413 114 624}, {208 367 404 803, -11 373 098 296},
{266 569 389 675, -12 269 829 208}, {245 780 261 773, -47 021 280 096},
{779 191 874 389, -145 004 168 764}, {3 954 485 231 537, 32 217 671 752},
{605 052 759 007, -31 139 729 376}, {978 046 762 999, -22 352 899 464},
{400 099 379 441, -56 328 871 564}, {423 201 329 989, -53 912 679 072},
{591 307 488 851, 79 976 740 844}, {2 297 332 114 839, -329 877 295 216},
{11 808 951 673, -773 351 628}, {15 233 439 469, 1 974 961 996},
{41 336 724 427, -1 475 587 960}, {1 479 092 931, 73 508 960}, {650 702 363, -124 704 216},
{1 984 233 659, 29 503 320}, {548 318 987, 50 601 040}, {605 349 069, 21 143 024},
{569 299 771, -14 909 860}, {198 931 643, -20 184 108}, {212 388 901, 7 083 636},
{8 773 067, 1 106 420}, {5 715 389, 342 888}, {8 300 611, 439 544}, {3 702 925, 580 188},
{16 191 181, -1 118 488}, {38 861 477, -7 120 764}, {237 808 961, 27 470 604},
{688 132 675, 106 176 308}, {3 728 462 371, 600 394 704}, {9 204 872 731, 1 461 180 000},
{31 958 869 363, -3 657 628 212}, {70 064 271 785, -1 732 813 124},
{54 877 518 225, -201 891 452}, {2 697 840 487, 251 042 148}, {4 644 489 293, -511 597 324},
{2 928 276 521, -281 844 304}, {8 017 844 113, 952 728 084}, {28 909 419 193, 3 017 884 044},
{92 667 751 031, -7 042 765 716}, {81 161 160 779, 15 093 342 880},
{415 694 585 667, -14 297 460 044}, {77 981 840 543, 3 164 919 968},
{83 304 581 961, -7 372 060 892}, {161 469 586 877, 19 241 416 432},
{550 292 645 733, -72 874 662 980}, {2 387 440 041 811, -174 532 164 436},

```

```

{4 088 749 001 389, 194 549 698 196}, {233 989 766 929, 21 707 024 556},
{349 487 732 651, 23 988 278 244}, {754 560 193 657, -14 622 222 300},
{423 061 713 839, -68 469 496 928}, {893 865 455 783, 144 514 278 076},
{1 954 924 474 871, 51 865 667 364}, {1 165 874 602 153, -208 715 486 308},
{6 308 537 045 735, 717 953 463 724}, {11 172 221 328 013, -987 775 917 436},
{22 388 095 243 841, -3 409 925 060 220}, {108 140 752 972 027, 52 659 542 628},
{1 602 173 769 605, -156 952 183 164}, {2 383 591 471 445, 427 796 048 288},
{13 372 491 734 659, -454 062 053 480}, {14 942 529 412 947, 1 241 756 964 112},
{3 025 546 583 019, 130 535 951 224}, {1 695 038 455 291, -223 151 604 788},
{6 582 729 959 949, 1 140 770 803 340}, {19 118 324 786 643, -2 612 651 735 792},
{60 572 672 435 227, -4 856 746 226 640}, {167 295 393 234 931, 30 466 101 667 176},
{1 092 436 597 630 723, 128 941 535 836 708}, {4 446 014 698 405 307, -819 192 121 346 228},
{25 553 948 692 214 191, -991 937 457 014 588}, {17 259 038 882 052 081, -407 524 208 784 952},
{10 440 614 255 139 081, -1 716 933 076 818 484}, {10 148 152 978 656 921, -777 962 979 302 740},
{2 528 300 083 654 973, 424 479 746 489 232}, {1 356 222 855 470 587, 224 682 577 389 984},
{593 299 552 539 859, 17 007 630 011 904}, {143 627 345 005 013, 25 511 641 777 972},
{689 302 913 385 787, -11 618 739 879 432}, {277 200 016 448 827, 2 418 340 644 440},
{66 368 509 309 429, 1 656 034 663 388}, {9 279 962 495 357, -130 350 334 044},
{1 831 480 811 009, 319 226 682 124}, {6 123 187 566 655, 182 651 090 748},
{6 347 314 870 721, -1 160 596 995 824}, {39 736 082 086 873, 6 723 841 093 816},
{44 308 406 749 679, 2 014 754 682 108}, {1 182 326 738 881, -144 651 038 700},
{1 833 645 337 513, -9 785 527 080}, {273 879 469 369, 21 004 139 548},
{60 272 832 885, 7 491 294 244}, {25 000 962 109, 268 102 744}, {4 920 704 941, 697 563 552},
{2 756 485 621, 172 595 808}, {368 453 411, -21 604 940}, {85 368 463, -5 445 356},
{128 278 009, 3 890 796}, {8 632 907, 739 564}, {17 655 853, 188 692}, {5 927 235, -133 756},
{3 063 883, -362 684}, {11 856 003, 809 116}, {20 493 801, 3 819 620}, {101 886 173, 5 274 864},
{121 454 261, 12 383 504}, {173 796 867, 29 269 576}, {132 902 997, 4 333 616},
{105 054 227, 6 004 208}, {217 736 443, 20 730 444}, {751 786 193, -71 540 672},
{2 566 767 527, 299 901 196}, {9 661 056 301, 340 876 508}, {8 505 527 621, -1 215 168 164},
{47 415 471, -7 719 796}, {80 058 735, -10 810 828}, {319 954 547, -52 856 692},
{205 450 835, 2 811 424}, {216 883, -16 968}, {270 173, -48 72}, {161 549, 16 128},
{19 637, 2352}, {59 933, 10 780}, {346 531, 10 556}, {132 641, -74 48}, {103 879, -14 112},
{371 935, -31 556}, {491 801, 39 956}, {900 017, 155 092}, {2 229 055, -206 976},
{3 480 713, 423 500}, {6 768 049, -236 068}, {5 688 379, -221 788}, {5 701 957, 881 160},
{30 294 781, -5 394 816}, {151 410 395, -12 704 972}, {76 596 637, -12 682 068},
{36 808 717, 6 024 228}, {48 424 477, -6 001 884}, {29 886 565, -2 530 612},
{35 096 867, -3 730 692}, {111 006 647, -16 873 164}, {518 701 573, 38 016 804},
{987 958 859, -122 624 824}, {508 099 491, 13 211 744}, {441 884 987, -52 483 480},
{1 607 251 731, -132 413 344}, {1 335 287 019, 64 958 684}, {2 105 710 185, 104 034 028},
{1 827 162 625, -114 640 456}, {517 180 983, 37 180 192}, {243 944 465, -689 556},
{11 560 207, 1 563 016}, {45 193 935, -7 242 452}, {126 963 279, 6 981 688},
{94 381 335, 2 848 384}, {28 080 399, 3 291 316}, {112 525 485, 18 696 692},
{25 209 309, 1 483 832}, {1 155 955, -135 016}, {4 320 797, -87 584}, {2 130 213, 142 912},
{983 091, 125 552}, {1 556 725, -208 796}, {6 946 169, 743 596}, {18 527 765, -2 569 812},
{39 352 913, -6 465 060}, {41 066 369, 595 140}, {124 757, -43 96}, {121 837, 62 16},
{181 259, 32 900}, {1 178 293, -141 960}, {3 110 749, 375 396}, {7 853 413, 293 496},
{5 181 467, 436 324}, {3 972 733, 147 896}, {1 493 507, 87 780}, {91 031, -16 604},
{584 803, -90 552}, {3 028 843, 360 192}, {10 753 411, 1 546 440}, {5 231 837, -513 128},
{7 340 661, -855 596}, {26 258 319, 2 028 404}, {8 098 109, 1 020 460}, {4 786 683, 781 928},
{6 943 395, 1 153 124}, {1 799 523, -29 764}, {998 859, 125 972}, {650 941, 42 056},
{1 467 373, 255 948}, {4 986 995, 443 996}, {7 521 847, 675 696}, {6 510 943, -621 152},

```

```

{21857879, -3424876}, {95529479, 6474160}, {115553233, 14925988},
{281390983, -10289244}, {261441835, -49161392}, {1141345875, -86569616},
{1163683291, -70762104}, {2298742771, 124623744}, {4052622667, -229050360},
{5130718349, 977102168}, {17900148157, 2670355744}, {57840969723, 4734227540},
{75207464739, -561775228}, {5140354349, -394906400}, {479693877, 58603804},
{793031485, 19607252}, {638122565, -37226644}, {384682041, -61658044},
{1075565721, 36966104}, {259055465, 15704612}, {568062129, 57002456},
{143257463, 14873880}, {400137601, -11451188}, {47740467, -6388228},
{220669583, 41501684}, {960764899, 81522420}, {1277802293, -69745284},
{1634264213, -76677188}, {1755158345, -211743364}, {4468434609, -31984456},
{685413863, -31220924}, {105591945, 11070332}, {373130375, 50576764},
{1393790971, -50129520}, {717997997, 79300564}, {313383233, 19255348},
{386729545, 70628824}, {2451736025, 453944652}, {13286931845, -2536542344},
{44108069125, 932207388}, {21485497897, 2123036188}, {18624929241, -2182144748},
{74049264843, -11118179884}, {275793587185, -34643601748},
{98931556327, -13422547320}, {363081931351, -4995837308},
{1614192133, 42699804}, {613230587, -59333176}, {1452614371, 126015400},
{4348641317, 808707872}, {22272442861, -764308916}, {7846353681, 1387095136},
{34763850855, 5414693312}, {166125441759, 12956526632},
{168586525361, 24123427804}, {20255256491, 2584431360},
{30674190397, -416403008}, {10193150235, -880192096}, {26948308941, 2235996952},
{8493222741, 344053696}, {7892735107, -897116192}, {13235675333, -507584028},
{2809814165, -410578084}, {4688966879, -602433216}, {9526415977, 130011504},
{35576185, -6445096}, {225890543, 37277268}, {162566255, -22343356},
{449881699, -78048712}, {1343971829, 27099492}, {803202283, -129797388},
{1782510715, 96629036}, {3152728891, -201675628}, {5407924461, 202414072},
{4179650259, -347845540}, {401775867, 34734560}, {1097836269, -9095576},
{199175171, -23586556}, {765238779, 39278876}, {1382629855, 215739048},
{6438276391, 932095248}, {6306495185, -312922624}, {3507117465, 24976028},
{764568785, 63694484}, {17153321, -1907360}, {943087, -29540},
{160089, 7280}, {5183, -644}, {2263, -140}, {1679, 84}, {1, 0}}

28
— is a relation number with a list {{75, 84}, {1, 0}}
75

28
— is a relation number with a list
79
{{79, 84}, {395, -56}, {237, 28}, {1027, 28}, {711, 56}, {1343, -140},
{4503, -112}, {1817, 168}, {2449, -252}, {5609, 28}, {711, -56}}

28
— is a relation number with a list {{81, 84}, {1, 0}}
81

28
— is a relation number with a list {{83, 84}, {1, 0}}
83

28
— is a relation number with a list {{85, 84}, {1, 0}}
85

28
— is a relation number with a list {{87, 84}, {1, 0}}
87

28
— is a relation number with a list {{89, 84}, {445, 56}, {267, -28},
89
{1157, -56}, {1691, 196}, {6497, 952}, {14863, -560}, {22873, -532}, {267, -28}}

```

```

28
— is a relation number with a list {{93, 84}, {1, 0}}
93

28
— is a relation number with a list {{95, 84}, {1045, -28}, {855, 112},
95 {3895, -308}, {2071, -252}, {209, 28}, {1235, 112}, {285, -28}, {1, 0}}

28
— is a relation number with a list {{97, 84}, {1261, 140}, {1, 0}}
97

28
— is a relation number with a list
99 {{99, 112}, {429, -56}, {1881, 224}, {979, -28}, {1, 0}}

28
— is a relation number with a list
101 {{101, 112}, {1111, 84}, {1919, -28}, {1313, -84}, {3131, -196}, {505, 56}, {1, 0}}

28
— is a relation number with a list
103 {{103, 112}, {927, 56}, {2575, -168}, {5665, -364}, {16377, 1876}, {52221, 5516},
{265431, -9100}, {157693, 5796}, {123703, -8316}, {106811, 14504}, {544149, 14672},
{132355, 56}, {2781, -280}, {1957, 112}, {5459, -336}, {8549, 252}, {1957, 112}}

28
— is a relation number with a list
107 {{107, 112}, {535, 56}, {2675, 308}, {10379, -364}, {18939, -700}, {4173, 448},
{15087, 560}, {3531, 140}, {3317, 224}, {4601, 112}, {963, -112}, {4815, -616},
{12091, -532}, {15515, 84}, {2675, 112}, {1391, 28}, {963, 28}, {1177, -84}, {1, 0}}

28
— is a relation number with a list {{109, 112}, {327, -28}, {981, 28}, {1, 0}}
109

28
— is a relation number with a list {{111, 112}, {1, 0}}
111

28
— is a relation number with a list {{113, 112}, {1, 0}}
113

28
— is a relation number with a list {{115, 112}, {345, 28}, {1035, -56}, {3105, 364},
115 {19665, 1232}, {5405, 448}, {3335, 364}, {1357, 112}, {299, 28}, {1035, 56}}

28
— is a relation number with a list {{117, 112}, {585, -56},
117 {325, -28}, {1287, -112}, {715, 84}, {533, 56}, {351, 28}, {1, 0}}

28
— is a relation number with a list
121 {{121, 112}, {1089, -56}, {3025, 224}, {13431, 868}, {49731, 1456}, {27467, -1792},
{71027, -3164}, {15609, 1316}, {22143, -392}, {23111, 700}, {1, 0}}

28
— is a relation number with a list {{123, 112}, {451, -28}, {1, 0}}
123

28
— is a relation number with a list
125 {{125, 112}, {1625, 168}, {1375, 112}, {3875, 112}, {1125, -28}, {1, 0}}

```



```

28
127 is a relation number with a list
    {{127, 140}, {1651, 56}, {3429, 308}, {5207, 84}, {1, 0}}

28
129 is a relation number with a list
    {{129, 140}, {1419, 112}, {4773, 56}, {1677, -56}, {1, 0}}

28
131 is a relation number with a list {{131, 140}, {1179, 56}, {393, 28}, {1, 0}}

28
135 is a relation number with a list {{135, 140}, {1, 0}}

28
137 is a relation number with a list {{137, 140}, {411, -28}, {1233, 56}, {1, 0}}

28
139 is a relation number with a list {{139, 140}, {1, 0}}

28
141 is a relation number with a list {{141, 140}, {1, 0}}

28
143 is a relation number with a list {{143, 140}, {429, 28}, {1287, -28}, {1, 0}}

28
145 is a relation number with a list {{145, 140}, {1, 0}}

28
149 is a relation number with a list {{149, 140}, {1341, -56}, {447, 28}, {1, 0}}

28
151 is a relation number with a list
    {{151, 140}, {1661, -112}, {2869, -112}, {6493, 56}, {453, 28}, {755, 28}, {1, 0}}

28
153 is a relation number with a list
    {{153, 140}, {1989, -56}, {459, 28}, {1683, -28}, {1, 0}}

28
155 is a relation number with a list {{155, 168}, {2015, 168}, {1, 0}}

28
157 is a relation number with a list
    {{157, 168}, {1727, 112}, {7379, 476}, {37209, -1736}, {118221, 1540}, {56363, -532},
    {4553, -112}, {6123, 112}, {5809, 28}, {2041, 28}, {471, -28}, {785, 56}, {1, 0}}

28
159 is a relation number with a list {{159, 168}, {1, 0}}

28
163 is a relation number with a list {{163, 168}, {815, 56},
    {4075, -28}, {2119, -168}, {10595, 84}, {1793, 140}, {4401, -140},
    {9943, -616}, {14181, -532}, {29829, -392}, {6031, 336}, {2771, -28}, {1, 0}}

28
165 is a relation number with a list {{165, 168}, {1, 0}}

28
167 is a relation number with a list {{167, 168}, {1, 0}}

28
169 is a relation number with a list {{169, 168}, {1, 0}}

```

```

28
171 is a relation number with a list {{171, 168}, {1, 0}}

28
173 is a relation number with a list
{{173, 168}, {865, -56}, {4325, 112}, {7439, -112}, {8131, 364},
{21279, 980}, {48613, 3556}, {202583, 7784}, {34427, -1792}, {65567, -2268},
{35465, 2044}, {124041, -7756}, {9515, 448}, {18511, -392}, {15051, 392},
{26815, -1624}, {137189, -7700}, {244103, -11172}, {290813, 2968},
{8823, 616}, {34427, 700}, {21971, 196}, {3287, -140}, {11591, 168}, {1, 0}}

28
177 is a relation number with a list {{177, 168}, {1, 0}}

28
179 is a relation number with a list {{179, 168}, {1969, -112},
{8413, 308}, {17363, 812}, {55669, -2688}, {139441, 1288}, {60323, 4088},
{178463, -5936}, {68557, -868}, {2685, -28}, {537, -28}, {895, 28}, {1, 0}}

28
181 is a relation number with a list {{181, 168}, {2353, -168}, {1, 0}}

28
183 is a relation number with a list
{{183, 196}, {793, 56}, {549, -28}, {2013, -112}, {1, 0}}

28
185 is a relation number with a list
{{185, 196}, {2035, 84}, {3515, 112}, {7955, 252}, {4033, -168}, {1, 0}}

28
187 is a relation number with a list {{187, 196}, {1683, -112}, {561, -28}, {1, 0}}

28
191 is a relation number with a list
{{191, 196}, {955, -56}, {573, -28}, {2483, 112}, {3629, 112}, {8595, -28}, {1, 0}}

28
193 is a relation number with a list
{{193, 196}, {579, -28}, {1737, 112}, {10615, -56}, {4825, 308},
{19879, 1120}, {54233, -3724}, {314011, -10164}, {207089, 8792},
{756367, -50876}, {1307189, -42420}, {1511383, 74144}, {5501079, -55720},
{2933793, 113260}, {2116631, -56784}, {3015239, -23212}, {447953, -4256},
{207089, -10220}, {518977, -14868}, {270779, 1792}, {36091, 280},
{5597, 364}, {26441, 1204}, {9071, 560}, {21423, -700}, {53461, 3248},
{288149, -196}, {5597, 336}, {22195, -448}, {39565, 364}, {21423, 1232},
{92447, -3640}, {279271, -13748}, {832023, 2212}, {60023, 224}, {1737, 112}}

28
195 is a relation number with a list {{195, 196}, {1, 0}}

28
197 is a relation number with a list {{197, 196}, {1, 0}}

28
199 is a relation number with a list {{199, 196}, {597, 28}, {1791, 28}, {1, 0}}

28
201 is a relation number with a list {{201, 196}, {1005, 56}, {1, 0}}

```

```

28
205 is a relation number with a list
    {{205, 196}, {1845, 112}, {2173, 140}, {2747, -112}, {2173, 140}}

28
207 is a relation number with a list {{207, 196}, {759, -28}, {1, 0}}

28
209 is a relation number with a list
    {{209, 196}, {2717, -168}, {6061, -196}, {3135, -196}, {1, 0}}

28
211 is a relation number with a list {{211, 224}, {2743, 56}, {1, 0}}

28
213 is a relation number with a list
    {{213, 224}, {2343, 28}, {639, 28}, {1065, 56}, {1, 0}}

28
215 is a relation number with a list {{215, 224}, {1935, -28}, {645, 28}, {1, 0}}

28
219 is a relation number with a list
    {{219, 224}, {1095, -56}, {1825, -112}, {2409, 140}, {6351, -196}, {17301, -896},
    {60663, -2324}, {52341, -364}, {5475, -28}, {2847, -56}, {657, -28}, {2847, 56}}

28
221 is a relation number with a list
    {{221, 224}, {663, -28}, {1989, -112}, {5967, -196}, {19227, 532}, {16575, -28}, {1, 0}}

28
223 is a relation number with a list {{223, 224}, {1, 0}}

28
225 is a relation number with a list {{225, 224}, {1, 0}}

28
227 is a relation number with a list
    {{227, 224}, {681, 28}, {2043, 56}, {6129, -140}, {7037, -336}, {4313, 196}, {1, 0}}

28
229 is a relation number with a list {{229, 224}, {1145, 56}, {5725, 224},
    {22671, 1372}, {149537, -3360}, {380827, -22148}, {987219, -2156}, {1, 0}}

28
233 is a relation number with a list {{233, 224}, {2097, 28}, {699, 28}, {1, 0}}

28
235 is a relation number with a list
    {{235, 224}, {2585, -28}, {2115, -28}, {3055, 28}, {705, 28}, {1, 0}}

28
237 is a relation number with a list {{237, 224}, {3081, -56}, {1, 0}}

28
239 is a relation number with a list
    {{239, 252}, {3107, -168}, {19837, -644}, {30353, 1008}, {27007, 448},
    {30353, 392}, {40391, -952}, {97273, 392}, {13623, -476}, {43259, 2268},
    {39913, -364}, {30353, 1652}, {147463, -2520}, {290863, -11088},
    {615425, 17668}, {706245, -2912}, {327669, 4984}, {304725, -13076},
    {950503, -7196}, {150809, -6048}, {93449, 336}, {9799, -56}, {1, 0}}

```

```

28
241 is a relation number with a list
{{241, 252}, {2651, -56}, {4579, -196}, {17111, 476}, {6025, 84}, {5543, -280},
{13737, 448}, {36391, 1960}, {204609, 3080}, {320289, -1960}, {194969, 3332},
{390179, 12964}, {303419, -13104}, {488507, 20272}, {476939, 9296},
{685163, 11424}, {66757, 196}, {19039, -784}, {53743, -1624}, {36391, 1820},
{2169, 112}, {9881, -560}, {47959, 1232}, {21449, -364}, {6507, 28},
{2651, -28}, {2169, -56}, {3615, 56}, {6025, -196}, {12291, 112}, {6989, -196},
{16147, 336}, {4579, 112}, {3133, -56}, {723, -28}, {1205, 28}, {1, 0}}

28
243 is a relation number with a list {{243, 252}, {1, 0}}

28
247 is a relation number with a list {{247, 252}, {1235, 56}, {741, -28}, {1, 0}}

28
249 is a relation number with a list {{249, 252}, {1, 0}}

28
251 is a relation number with a list {{251, 252}, {1, 0}}

28
253 is a relation number with a list {{253, 252}, {1, 0}}

28
255 is a relation number with a list {{255, 252}, {1, 0}}

28
257 is a relation number with a list
{{257, 252}, {1285, -56}, {771, 28}, {3341, 84}, {4883, 224}, {11565, 392},
{50115, -2464}, {214595, -1988}, {28013, 1232}, {83011, -84}, {4883, 224}}

28
261 is a relation number with a list {{261, 252}, {1, 0}}

28
263 is a relation number with a list
{{263, 252}, {2893, 56}, {4997, 168}, {11309, 364}, {6575, -168}, {6049, 252}, {1, 0}}

28
265 is a relation number with a list
{{265, 252}, {3445, 168}, {21995, -364}, {8215, -196}, {4505, 56},
{1325, 28}, {2385, 112}, {8745, 112}, {2385, -56}, {6095, 28}, {2385, -112}}

28
267 is a relation number with a list {{267, 280}, {3471, -140}, {7743, 28},
{1157, 56}, {5073, -56}, {6141, 140}, {5073, -140}, {2937, -140}, {1, 0}}

28
269 is a relation number with a list {{269, 280}, {2959, 140},
{5111, -112}, {11029, 280}, {29321, -980}, {21251, 392}, {22327, 868},
{64829, 2688}, {85273, 4116}, {312847, -28}, {807, 28}, {1345, 28}, {1, 0}}

28
271 is a relation number with a list {{271, 280}, {2439, -28}, {813, -28}, {1, 0}}

28
275 is a relation number with a list {{275, 280}, {1, 0}}

```

```

28
— is a relation number with a list
277
{{277, 280}, {831, -28}, {2493, -56}, {7479, -364}, {45705, -812}, {64541, -3108},
{201379, 5964}, {386969, -9156}, {669509, -32200}, {1853407, -73304},
{5763539, 85652}, {6884835, 63644}, {3125391, -62356}, {2102707, -56224},
{6210063, 119252}, {2481643, -79660}, {3374691, 107240}, {13919527, 157892},
{6933587, 282268}, {34102301, 1096536}, {30382745, -306348}, {15039161, 273028},
{6266017, 255584}, {34232491, -1590288}, {208815065, -2751084},
{74047363, -1412796}, {161205967, -259980}, {5087659, -15820},
{1767537, -84560}, {2277771, -61768}, {2117665, -15064}, {1761443, 77532},
{6036661, -119224}, {12122351, -59780}, {3597953, -170772}, {3252257, 35868},
{3249487, -81396}, {1759781, -44576}, {5904809, 186844}, {20553123, 183512},
{61217, 1596}, {157613, -4004}, {403589, -7616}, {16343, 28}, {2493, 56}}

28
— is a relation number with a list {{279, 280}, {1, 0}}
279
known cases
known cases
known cases
known cases
known cases
known cases

29
— is a relation number with a list
8
{{8, 29}, {168, 377}, {1672, 3045}, {10984, 15457}, {35784, 6061}, {2328, 1073},
{364, -493}, {1032, 203}, {136, 145}, {18, -29}, {88, -87}, {1, 0}}

29
— is a relation number with a list
9
{{9, 29}, {180, 319}, {1251, 1160}, {819, -116}, {63, -29}, {45, 29}, {117, 116}, {1, 0}}

29
— is a relation number with a list {{10, 29}, {190, 261}, {710, -551},
10
{1590, -899}, {1040, 1479}, {4390, -2059}, {1360, 1537}, {1770, 29}, {1, 0}}

29
— is a relation number with a list
11
{{11, 29}, {198, 203}, {55, -58}, {33, 29}, {44, -29}, {154, -87}, {220, -203},
{187, 232}, {495, 58}, {297, 145}, {77, -29}, {110, 29}, {66, 29}, {88, 87}, {1, 0}}

29
— is a relation number with a list {{12, 29}, {204, 145}, {708, 29}, {1, 0}}
12

29
— is a relation number with a list
13
{{13, 29}, {208, 87}, {442, 145}, {91, 58}, {325, -29}, {78, -29}, {117, 116}, {1, 0}}

29
— is a relation number with a list {{14, 29}, {210, 29}, {1, 0}}
14

29
— is a relation number with a list {{15, 29}, {210, -29}, {105, -29}, {165, 116},
15
{735, 319}, {1455, -841}, {3405, -551}, {495, 116}, {465, -58}, {1, 0}}

```

```

29
16 — is a relation number with a list {{16, 29}, {208, -87}, {272, -203}, {552, 377},
    {2800, 957}, {1136, -899}, {1896, -319}, {72, -29}, {112, -29}, {1, 0}}

No answers up to 5000 iterations for  $\frac{29}{17}$ 

29
18 — is a relation number with a list
    {{18, 29}, {99, 58}, {153, -29}, {72, -29}, {63, -29}, {45, 29}, {234, -145},
    {504, -319}, {603, 464}, {1251, 145}, {54, 29}, {36, 29}, {42, -29}, {234, -145}}

29
19 — is a relation number with a list {{19, 29}, {190, 29}, {247, -174},
    {1387, 928}, {8721, 4321}, {1501, -377}, {133, 58}, {323, 116}, {475, -29},
    {209, 87}, {665, -377}, {1691, -580}, {931, -348}, {2147, 58}, {1, 0}}

29
20 — is a relation number with a list {{20, 29}, {90, -29}, {60, 29}, {1, 0}}

29
21 — is a relation number with a list
    {{21, 29}, {56, 29}, {42, 29}, {273, -145}, {119, 29}, {1, 0}}

29
22 — is a relation number with a list {{22, 29}, {154, -29}, {99, -58},
    {374, -203}, {352, -87}, {44, 29}, {154, 87}, {220, -87}, {451, -232},
    {143, -87}, {341, 58}, {77, -29}, {110, 29}, {66, 29}, {88, -29}, {1, 0}}

29
23 — is a relation number with a list {{23, 29}, {138, 29}, {161, -58},
    {299, -174}, {1127, -261}, {1909, -1189}, {10787, 145}, {1311, 29}, {138, -29}}

29
24 — is a relation number with a list {{24, 29}, {120, 29}, {1, 0}}

29
25 — is a relation number with a list {{25, 29}, {100, -29}, {325, 29}, {150, 29}, {1, 0}}

29
26 — is a relation number with a list {{26, 29}, {78, 29}, {234, 29}, {1, 0}}

29
27 — is a relation number with a list
    {{27, 29}, {54, 29}, {108, 29}, {72, -29}, {378, 29}, {1, 0}}

29
28 — is a relation number with a list {{28, 29}, {1, 0}}

29
30 — is a relation number with a list {{30, 29}, {1, 0}}

29
31 — is a relation number with a list
    {{31, 29}, {62, 29}, {124, -29}, {248, 29}, {403, -145}, {992, -145}, {713, -174},
    {527, 29}, {155, 29}, {310, 29}, {279, -116}, {1457, 493}, {682, 29}, {434, -87}, {1, 0}}

29
32 — is a relation number with a list {{32, 29}, {96, -29}, {72, 29}, {112, 29}, {1, 0}}

```

```

29
— is a relation number with a list {{33, 29}, {132, 29},
33
  {143, 58}, {297, 116}, {561, 203}, {176, 29}, {66, 29}, {264, 29}, {1, 0}}

29
— is a relation number with a list {{34, 29}, {170, -29}, {68, 29}, {85, 29}, {1, 0}}
34

29
— is a relation number with a list {{35, 29}, {210, -29}, {1, 0}}
35

29
— is a relation number with a list {{36, 29}, {252, 29}, {1, 0}}
36

29
— is a relation number with a list {{37, 29}, {296, -87}, {1295, -174},
37
  {2849, 261}, {814, -87}, {1147, 377}, {592, 29}, {444, 29}, {333, 29}, {518, -145},
  {2294, -29}, {111, -29}, {185, 58}, {407, -87}, {1036, -29}, {296, -87}}

29
— is a relation number with a list {{38, 29}, {171, 29}, {114, 29}, {1, 0}}
38

29
— is a relation number with a list {{39, 29}, {390, -29}, {1, 0}}
39

29
— is a relation number with a list {{40, 29}, {110, -29}, {120, -29}, {1, 0}}
40

29
— is a relation number with a list
41
  {{41, 29}, {492, 145}, {2337, -667}, {13571, -1450}, {21361, 986},
  {13571, -2030}, {26199, 9106}, {45879, 16066}, {95079, 13804},
  {63509, 18009}, {349607, 3480}, {65887, 2871}, {5986, 841}, {4059, 29}, {1, 0}}

29
— is a relation number with a list {{42, 29}, {182, 29}, {168, 29}, {1, 0}}
42

29
— is a relation number with a list
43
  {{43, 29}, {602, 29}, {301, -29}, {473, 29}, {387, -58}, {817, -261}, {1462, -377},
  {1978, 203}, {2236, 319}, {129, -29}, {559, -116}, {903, 116}, {1075, 87},
  {1333, 145}, {1204, -261}, {4343, -493}, {4042, -609}, {9503, 551}, {5848, 29},
  {430, -87}, {215, -29}, {516, 145}, {2752, -667}, {3612, 551}, {10535, -2378},
  {43989, -13253}, {181890, 43471}, {344258, 11861}, {12427, -1218},
  {10621, -2233}, {23392, 1363}, {9503, 928}, {9589, 1102}, {14147, 319},
  {4773, 841}, {11739, 3422}, {63339, 18995}, {273222, 79721}, {1464537, 464870},
  {3006861, -289420}, {4844423, 623616}, {6213715, -1671618}, {20328551, 3329809},
  {15036971, 1204805}, {24910373, 1406558}, {17529853, -1369699},
  {11878062, 2821555}, {25449206, 1182939}, {24744436, -802053},
  {5125901, -81751}, {1049716, -24447}, {1505, 87}, {1118, -29}, {559, 116}}

29
— is a relation number with a list
44
  {{44, 58}, {154, -29}, {396, 29}, {110, -29}, {132, 29}, {572, -145}, {88, 29}, {1, 0}}

29
— is a relation number with a list {{45, 58}, {585, 29}, {1, 0}}
45

29
— is a relation number with a list
46
  {{46, 58}, {138, 29}, {322, 87}, {299, -58}, {207, -29}, {92, 29}, {230, 29}, {1, 0}}

```

29  
47 is a relation number with a list

```
{ {47, 58}, {517, 145}, {2961, 493}, {141, 29}, {188, 29}, {658, 145}, {3149, 957},
{13066, -3393}, {23782, -1943}, {21902, 3277}, {48739, -3654}, {58139, 7627},
{135219, -24737}, {542098, -159181}, {3034085, 6873}, {145324, -35641},
{129720, 5713}, {78913, 23635}, {376376, -50315}, {1136037, -261928},
{4151275, 496509}, {8422541, 2548375}, {36538552, 7048305}, {60960269, -7253712},
{137736931, -977996}, {160505, -12354}, {4559, 1160}, {3807, -493}, {6439, -667},
{10857, -2146}, {5969, -1421}, {13395, -667}, {2585, 551}, {7990, -1247},
{23876, 319}, {2303, 638}, {11703, -1102}, {19693, 3190}, {25991, 5597},
{93718, 26071}, {496602, 319}, {3807, -899}, {9917, 580}, {2679, 812},
{11421, 2929}, {13865, -783}, {10763, -3045}, {66599, 19836}, {333277, -95903},
{2141696, -543025}, {1428988, -47589}, {61946, 18415}, {314947, 88189},
{1777023, 240961}, {4243912, 850831}, {481421, 112288}, {1516643, -337270},
{7875461, -1273709}, {10960729, 1002704}, {3243705, 907352}, {18128041, 2096004},
{34591765, 8207087}, {82880599, -23379655}, {499986987, -135166651},
{1911941999, 454288132}, {4455105137, -639615068}, {22200339, -4194763},
{57646628, 16261315}, {347735704, 93959507}, {1320809228, -341259849},
{2078817896, -635560433}, {8090420059, 80427527}, {1539727896, 20085719},
{323005949, 52478922}, {382223599, 108108404}, {2359870799, -712823509},
{10405812784, -1399665483}, {28583256941, 4761633047}, {632556973, 154216606},
{737455803, -32234254}, {184805833, 32631235}, {516134119, 58660620},
{555138667, -16790188}, {49935761, 11958266}, {98826759, 13234585},
{290679208, 83959727}, {1823601269, -554695963}, {7497128860, 1684617859},
{35656898928, -8827221811}, {16356549148, -1093532841}, {2182842949, 215342893},
{1382458893, -114962641}, {136638447, -7479071}, {94712943, -876931},
{206565, -47792}, {723659, -13659}, {12596, -3103}, {8648, -1769}, {9259, -2552},
{44603, 9860}, {220759, -54781}, {76845, -14297}, {251920, -50199},
{43475, 1247}, {7990, 551}, {12925, -1972}, {41313, -9280}, {197071, 50228},
{180527, -21547}, {383097, -67193}, {942867, 249226}, {2539739, -744111},
{14448082, 685879}, {2097281, -115362}, {975955, -2349}, {52640, -12963},
{37036, 7743}, {78913, -23084}, {454067, 35728}, {488659, 129862},
{1447083, 146653}, {914009, -125135}, {1789008, -362065}, {1001899, -292349},
{5868044, 742429}, {3355236, 300121}, {2533535, 36482}, {765019, -173478},
{3342029, 94946}, {889193, 73254}, {476815, -87522}, {1842635, 434246},
{4965597, -1037591}, {10450826, -2820279}, {39023630, -11917347},
{153764683, 9141177}, {76860322, -2815233}, {39904457, -9206456},
{144695751, 13698353}, {281348204, 50568721}, {1037013734, 182708265},
{2784085232, 1910665}, {246327, -65192}, {678727, 132501}, {762434, 111853},
{965239, 103066}, {1769315, 477282}, {6571211, 1895208}, {41622589, 12028707},
{260213996, -76881059}, {1389828493, -183194769}, {3559293973, -174486301},
{3269693791, -130973599}, {218370648, -42250303}, {334599251, 78784329},
{914710945, -247909342}, {3615541881, 497407739}, {6283322276, 116502541},
{367302086, -36422579}, {144585912, -16822117}, {320217627, 315143},
{1519933, -193575}, {1347349, -46748}, {392121, 19633}, {25333, -522},
{11515, 3219}, {63967, 6583}, {87561, 14761}, {47235, 5713}, {71957, 2117},
{987, -232}, {2773, -638}, {10387, 2059}, {4324, 725}, {1222, -145}, {2914, 377},
{4794, 29}, {423, 58}, {799, -232}, {4841, 1044}, {17813, -5104}, {117547, -22301},
{283974, 3161}, {24252, 1073}, {20069, -899}, {13677, -58}, {517, -145}}
```



```

29
— is a relation number with a list {{48, 58}, {120, 29}, {1, 0}}
48
29
— is a relation number with a list {{49, 58}, {441, 29}, {294, 29}, {196, 29}, {1, 0}}
49
29
— is a relation number with a list
50
  {{50, 58}, {100, 29}, {325, -29}, {150, -29}, {1, 0}}
29
— is a relation number with a list {{51, 58}, {119, 29}, {1, 0}}
51
29
— is a relation number with a list {{52, 58}, {156, -29}, {572, 87}, {481, -58},
52
  {442, -29}, {364, -87}, {208, 29}, {130, 29}, {182, -29}, {104, 29}, {156, -29}}
29
— is a relation number with a list
53
  {{53, 58}, {265, -29}, {212, -29}, {477, 29}, {689, 29}, {371, 87}, {1219, -58}, {1, 0}}
29
— is a relation number with a list {{54, 58}, {1, 0}}
54
29
— is a relation number with a list
55
  {{55, 58}, {165, 29}, {495, -29}, {110, 29}, {330, -29}, {1, 0}}
29
— is a relation number with a list {{56, 58}, {1, 0}}
56
29
— is a relation number with a list {{57, 58}, {1, 0}}
57
29
— is a relation number with a list {{59, 58}, {1, 0}}
59
29
— is a relation number with a list {{60, 58}, {1, 0}}
60
29
— is a relation number with a list {{61, 58}, {183, -29},
61
  {549, 58}, {1647, -377}, {8479, 1189}, {9516, 145}, {3294, 551}, {732, 145},
  {427, -87}, {488, -29}, {305, 29}, {854, -145}, {976, 29}, {610, -29}, {1, 0}}
29
— is a relation number with a list {{62, 58}, {1, 0}}
62
29
— is a relation number with a list {{63, 58}, {315, 29}, {252, 29}, {1, 0}}
63
29
— is a relation number with a list {{64, 58}, {192, 29}, {352, 29}, {1, 0}}
64
29
— is a relation number with a list {{65, 58}, {455, -87}, {260, 29}, {1, 0}}
65
29
— is a relation number with a list {{66, 58}, {132, 29}, {858, -29}, {132, 29}}
66

```

```

29
— is a relation number with a list
67
{{67, 58}, {603, -29}, {402, 29}, {268, 29}, {469, -87}, {2278, 87}, {1072, -203},
{3819, -377}, {3283, 319}, {6231, -203}, {4154, -783}, {16013, 2987}, {72226, 12557},
{208772, -28043}, {835557, -70586}, {768825, 70412}, {382369, 81983},
{1845582, 98977}, {2343727, 469684}, {314431, -30421}, {684807, 36656},
{781019, -89581}, {1689070, 153207}, {254131, 35148}, {542365, 7366},
{182173, -20416}, {105257, 1102}, {35845, 3741}, {104855, 21663}, {231820, -46661},
{99495, -17458}, {351951, -49010}, {595027, 64467}, {993208, 20329},
{195171, -10411}, {176746, 9019}, {243478, 28043}, {596903, -70354},
{2282757, 226577}, {1138129, -90654}, {2704991, 219733}, {4569065, 878526},
{11821145, -2538138}, {58259515, -6462389}, {6566938, -934351},
{1774227, 370301}, {5177626, -158485}, {3509393, -14442}, {871, -145}, {1, 0}}

29
— is a relation number with a list {{68, 58}, {170, -29}, {1, 0}}
68

29
— is a relation number with a list
69
{{69, 58}, {759, -145}, {2346, -145}, {1794, -203}, {759, -116},
{3657, 319}, {10212, 551}, {17733, -754}, {8349, -203}, {1794, 319},
{2760, -377}, {8349, -1450}, {8073, -580}, {3243, 493},
{4784, 725}, {6693, 203}, {138, 29}, {483, 29}, {690, 29}, {138, 29}}

29
— is a relation number with a list {{70, 58}, {210, -29}, {1, 0}}
70

29
— is a relation number with a list
71
{{71, 58}, {923, -29}, {355, 29}, {497, 29}, {284, -29}, {426, -29}, {639, -29}, {1, 0}}

29
— is a relation number with a list {{72, 58}, {252, 29}, {1, 0}}
72

29
— is a relation number with a list
73
{{73, 87}, {1022, 145}, {511, 29}, {803, 116}, {657, -116}, {2847, 551}, {6716, 203},
{1241, 29}, {438, -29}, {219, -29}, {949, -145}, {4818, -899}, {23579, -58},
{1971, 319}, {4161, 145}, {3212, -377}, {13213, 1276}, {33069, 1189}, {16279, -2726},
{5621, 261}, {8833, -1508}, {15695, -2146}, {49129, -522}, {4453, 812},
{28689, 2291}, {79862, -8613}, {171185, -16704}, {302585, -17342}, {567283, 86188},
{2630409, -21982}, {542463, 96193}, {2532735, 20996}, {568013, 46835},
{437489, -56985}, {1342543, -106807}, {3354204, -198041}, {911989, -34887},
{359671, 25143}, {559837, 56231}, {180529, -16994}, {467565, -59653},
{705107, -127107}, {4200055, -732279}, {14134187, -2693143}, {48798456, -2742559},
{41435238, 2679919}, {90261069, 16348402}, {571542039, -58178611},
{747817183, 87945777}, {3189721130, -84294271}, {982665264, -92500169},
{2543071435, -319316448}, {836590877, 45998234}, {629454545, 107126377},
{971171341, -104069661}, {2521740616, 417213691}, {1347468310, -55251467},
{1564616446, -303997343}, {3257970363, -189348656}, {2850154403, -235414460},
{1838204459, 340638988}, {9855694887, 1374989818}, {16845929753, -9023321},
{44570442, 3577991}, {119322150, -23218357}, {235816645, -8689531},
{87549484, -8296987}, {271368229, -41142851}, {1214116144, 109507451},
{695995359, -24203980}, {432164453, 50072850}, {1349857381, 98394941},
{2020040889, 39507280}, {377381457, 35576881}, {1019389082, -167335597},

```

```

{1122411500, -176482081}, {4636888022, 11167929}, {160416551, -13193782},
{152655191, 7155402}, {174597677, -32541422}, {868011391, 38261295},
{875882762, -9447127}, {197103577, -15072518}, {84741539, 10632937},
{23502861, -1253902}, {23453221, -1635484}, {40620485, -6431997},
{148080719, 1076915}, {38949223, -1249900}, {14769579, 2635172},
{76026069, -11154734}, {150166037, -20874432}, {295285949, 1136365},
{12333423, 338198}, {11555535, 1735679}, {43377914, -6078313},
{60569779, -10601443}, {221838167, -19242080}, {661875889, 89986855},
{2333656992, 79555903}, {1937113765, -348725841}, {11332613513, -1554996501},
{32677574438, 3318774993}, {37242810916, -5549146201},
{116888511843, -12828787478}, {104347991493, 16924682953},
{204392245575, 17548063444}, {451469649969, -25551933553},
{617956240905, -98624575151}, {1913241669927, -359099796284},
{8595216261011, 1102018604892}, {16128078203125, 2844223796009},
{68420313823817, 9817043810871}, {21826478216440, 3031597244377},
{44186717923473, -6890560847456}, {207564757227801, -8267547924050},
{63952316238223, 6206153623846}, {138026939982699, 14388254595742},
{427459236154633, -31467145887712}, {954898857953455, 21041358242686},
{586754803378705, -95641465898677}, {942138583024939, 129383390036872},
{2661204251978955, -69729099452279}, {839388513841769, -88388595342812},
{3204054370221653, -88149875338431}, {2238096636784001, -211192717963652},
{6206698039580483, 623021029332842}, {1716394523599401, 203773890944125},
{6292847911387273, -123896873152649}, {1890161216041298, 33840189699929},
{356926722294998, -59856120814899}, {161330189390908, 11371703338715},
{155223013369554, 28503165091649}, {927624717525557, -130319644877389},
{1123265847019882, -142527215294491}, {1237486899531358, 80794636845829},
{1866416319606379, -33615978044619}, {1173726915136805, 122591017875862},
{3809378244392495, 130743565257884}, {1300484189711707, 244927564791134},
{5536784700190701, 283355374352198}, {9513563440287907, -1788138233987899},
{41819675735434076, 2372275639714957}, {64333861898765950, 5724891526143589},
{99284023116612383, -15940499060002252},
{265795099231717583, -2168258025124547},
{65746563677923954, 1571848437396479}, {19788160569155972, 3170815406808373},
{55718573366318582, 10121767488348369}, {365878304155329136,
-12144449902544297}, {112770916767016498, 9443262934397399},
{40021406539917170, -5704852357904497}, {6383122524755443, -589417637481885},
{7334418590806316, -677609546024415}, {8707908328744177, 1035212182109201},
{31113393646551537, 1409797588492667}, {7142809079038999, 763269459735719},
{19957027723479544, 221730452949303}, {93947937086002, -11330854761445},
{240980226594266, 34434439963877}, {4442280159729, -722316319613},
{7911903669723, 703353999394}, {12775706376397, 592035802952},
{18182934063931, 121530591682}, {3405792250937, 599168546121},
{13812988882597, 159510116215}, {4700559651884, -440164792903},
{10311474113577, -638682369449}, {6756602774689, -993605190028},
{14500249552011, -2351671554095}, {28486076603193, -1926224512100},
{29732248716411, -1122905867536}, {39178819714675, -4151185061253},
{132725253928054, 13322314959783}, {36346383893648, -5117705689391},
{38138416957503, 5179433909932}, {137413709922467, -4024380934701},
{42687344412209, -5494043915104}, {92345504329479, -2471998048145},
{64355088012322, -1495818247443}, {2547946175929, 122629895697},
{1991559260684, -249141233029}, {114654059004, 13856357209},

```

```

{277 633 697 236, 18 878 528 605}, {404 728 924 247, 68 911 921 814},
{638 210 284 501, 40 141 557 038}, {295 987 851 811, 9 271 713 801},
{51 610 256 933, -245 848 776}, {1 312 979 971, 212 738 026}, {2 668 282 495, -370 163 627},
{5 631 008 738, -178 231 883}, {5 286 040 814, 411 323 327}, {4 464 857 901, 126 478 570},
{2 781 880 423, 391 890 978}, {2 820 981 121, -529 215 664}, {12 767 904 473, 1 944 706 360},
{61 687 923 431, 5 073 403 898}, {58 916 595 815, -4 125 083 366},
{85 076 294 443, 3 045 802 633}, {15 051 087 513, -1 113 223 696},
{38 985 228 863, 3 828 916 313}, {50 812 798 509, -3 091 796 749},
{98 115 688 325, 8 163 628 673}, {11 106 530 177, 300 158 294}, {49 150 827, 3 752 600},
{26 792 971, -2 798 558}, {87 060 457, -3 219 232}, {10 307 089, -1 611 907},
{46 402 231, -7 066 633}, {223 686 600, -17 306 591}, {94 833 059, -17 514 695},
{529 949 632, -15 405 119}, {450 817 778, -50 021 723}, {45 425 783, -6 322 261},
{85 406 788, 13 477 083}, {331 733 170, 61 336 189}, {1 828 812 425, 118 454 647},
{3 795 468 560, -399 544 049}, {14 568 764 687, -228 758 322}, {5 239 058 233, 49 199 834},
{1 742 935 517, 129 592 677}, {4 250 842 268, -671 879 163}, {16 028 412 170, 1 892 432 381},
{64 893 577 906, 9 249 361 123}, {10 807 653 285, 1 131 507 094},
{37 041 488 815, 5 690 654 108}, {203 895 565 693, -10 419 708 439},
{328 398 025 351, -22 118 221 091}, {246 396 244 022, 48 495 109 147},
{286 210 974 951, 15 435 207 718}, {515 231 933 443, 101 316 910 820},
{631 258 692 039, 123 688 462 397}, {935 595 743 942, 109 057 237 397},
{3 352 115 662 063, 28 795 987 813}, {860 018 530 115, 52 199 928 979},
{1 811 835 650 923, 211 743 180 072}, {6 851 266 789 925, 873 164 586 894},
{9 785 643 081 571, -1 541 858 817 934}, {39 017 782 699 591, -4 054 188 393 881},
{111 259 390 462 987, -13 436 798 808 144}, {274 844 999 841 955, 1 778 686 440 423},
{62 152 084 923 530, -6 391 338 727 429}, {128 575 071 605 480, 6 867 813 553 957},
{139 677 172 138 319, -1 956 664 396 378}, {55 041 999 670 113, 10 225 498 147 049},
{285 759 152 245 364, -48 183 949 043 627}, {244 151 567 197 054, 25 726 415 065 259},
{920 809 707 509 779, 49 022 716 354 072}, {775 398 934 883 997, 117 764 025 873 716},
{3 573 294 974 937 095, -79 605 044 410 658}, {652 037 718 603 595, 112 537 221 853 464},
{1 692 549 713 754 797, -146 624 039 321 100}, {4 886 529 341 183 419, -943 789 038 681 822},
{12 233 642 787 524 557, -857 435 827 403 552}, {16 756 507 882 862 517, -2 682 561 189 128 927},
{48 263 274 610 493 715, -4 096 149 860 614 721},
{65 008 231 332 454 401, -10 883 313 650 387 443},
{21 290 491 600 528 761, -557 556 988 037 243}, {7 542 802 023 287 471, 1 248 718 249 373 223},
{3 685 954 474 513 709, 370 868 571 702 145}, {1 659 380 703 065 093, -45 958 392 552 536},
{356 135 695 687 181, 40 522 880 627 584}, {625 626 787 158 475, 24 269 740 640 468},
{393 212 273 039 589, -53 407 298 266 097}, {1 413 366 517 914 430, 31 587 817 487 649},
{590 224 639 173 575, 38 817 342 036 373}, {581 409 129 842 540, 62 016 966 118 189},
{1 697 719 738 855 247, -193 817 733 476 520}, {3 404 709 957 640 609, 623 134 438 090 390},
{21 099 757 004 772 107, 3 578 337 738 242 915}, {27 029 668 002 032 959, -3 511 135 310 706 227},
{77 337 257 304 030 561, 10 528 717 482 443 747}, {265 445 149 665 476 236,
30 440 686 052 754 135}, {622 034 811 079 701 467, 1 817 393 379 113 664},
{35 498 105 866 471 667, 5 751 831 317 090 553}, {72 059 611 366 769 477, -9 512 628 161 221 446},
{295 023 216 379 152 643, -8 784 166 833 198 276},
{265 607 284 319 978 093, 8 152 843 595 033 214}, {250 868 465 076 611 737, 2 802 868 567 101 984},
{101 448 535 267 378 079, -3 102 040 826 255 497},
{67 073 275 930 892 506, 13 284 596 536 280 577}, {47 471 407 212 742 333, 7 991 831 153 332 662},
{35 009 318 629 515 647, 724 409 241 647 976}, {17 350 277 220 134 327, -2 258 732 415 467 120},
{52 529 493 562 992 209, -2 055 581 706 711 096},
{66 841 049 239 228 951, -9 262 296 610 443 930}, {146 363 026 526 865 193,
21 582 939 647 854 578}, {344 381 223 592 530 269, 66 153 156 531 280 650},

```

```

{993 927 188 337 272 387, 91 006 981 011 284 838}, {521 921 003 440 840 663,
- 8 678 227 616 942 006}, {89 596 288 975 382 119, 7 164 217 458 431 728},
{258 313 272 848 815 185, - 9 899 866 752 116 119}, {66 921 822 447 114 643,
- 4 884 971 862 137 434}, {107 148 204 465 088 609, 16 077 145 444 244 226},
{393 602 396 057 331 029, 77 269 148 122 237 238}, {529 735 847 568 573 247,
- 41 313 401 408 090 563}, {535 701 063 772 097 256, 36 499 783 729 357 867},
{861 085 528 283 764 677, 72 116 370 795 689 477}, {314 697 252 309 160 431,
- 13 792 967 913 312 575}, {185 493 707 883 101 962, - 24 763 279 321 872 389},
{887 004 941 989 652 447, - 45 860 259 147 374 742}, {1 143 181 327 835 861 477,
- 168 815 225 283 289 319}, {2 812 343 187 742 954 188, 33 956 967 734 882 123},
{444 214 800 415 127 533, - 8 294 138 228 014 453}, {267 812 464 528 663 817,
- 32 875 427 546 554 577}, {351 060 223 404 585 673, - 29 047 441 878 474 028},
{181 837 222 991 505 601, - 25 598 811 431 943 627}, {193 124 636 656 715 476,
- 27 415 328 873 337 219}, {88 865 421 664 910 839, 10 934 992 412 103 792},
{101 140 212 869 876 719, - 5 325 327 403 114 924}, {2 993 568 619 399 101, - 127 965 569 345 819},
{3 676 318 284 504 272, - 578 755 308 768 851}, {14 876 409 528 055 118, - 880 491 866 219 425},
{6 712 510 430 282 811, 277 176 652 143 553}, {4 399 766 855 140 347, - 740 335 428 984 203},
{3 083 937 469 835 583, 138 949 171 871 423}, {1 975 065 272 492 221, - 56 705 079 818 550},
{701 714 044 463 117, - 41 975 876 553 465}, {866 937 557 042 524, - 35 359 674 447 723},
{1 244 964 202 990 223, 108 382 132 853 884}, {3 851 534 136 617 427, 261 588 166 696 177},
{5 277 050 559 241 644, - 228 673 210 436 413}, {1 282 370 501 902 585, 118 205 916 508 616},
{1 306 304 317 529 943, 192 995 883 121 195}, {3 260 681 095 244 806, 160 030 249 729 383},
{4 385 555 347 971 658, - 513 240 203 155 679}, {17 053 273 071 350 069, - 3 180 992 764 360 255},
{83 826 575 217 061 962, 894 305 860 106 567}, {17 386 821 205 739 528, - 3 120 487 586 436 695},
{97 535 614 840 286 866, - 4 686 556 631 352 973}, {64 391 432 523 166 391, 9 576 578 455 428 270},
{193 057 016 532 699 427, - 8 845 277 725 242 471},
{112 353 819 852 350 255, 20 833 344 352 916 773},
{597 658 160 406 946 470, 96 279 070 491 572 569},
{1 458 812 834 398 307 088, 74 031 510 670 950 049},
{1 592 668 668 510 654 116, 290 035 645 421 752 235},
{10 401 802 222 338 184 693, 511 488 112 513 436 710},
{12 558 917 961 069 885 989, 2 414 517 883 382 429 751},
{35 501 983 723 514 818 082, 7 017 472 120 024 814 391},
{30 267 488 007 524 467 271, - 4 759 570 106 448 969 826},
{124 834 917 924 637 326 995, - 304 941 898 153 189 353},
{8 298 755 338 750 358 114, 816 602 171 342 145 685},
{9 689 554 649 009 792 272, 1 872 831 489 904 585 165},
{23 753 995 562 541 250 631, 4 605 435 771 366 939 563},
{53 057 619 516 578 355 568, - 1 046 140 138 053 918 525},
{21 573 509 264 518 712 111, - 764 453 730 822 630 702},
{12 322 750 508 408 829 215, - 1 956 390 676 320 308 101},
{42 661 670 885 549 584 457, - 7 234 222 858 402 990 085},
{54 287 637 335 389 991 869, 10 506 548 315 042 463 317},
{128 107 390 492 970 295 732, 3 598 371 320 811 073 601},
{104 680 325 104 669 834 992, - 13 169 098 635 474 793 577},
{49 089 870 476 381 494 552, 5 772 886 048 042 071 417},
{209 225 588 787 791 818 673, - 5 835 607 887 484 724 296},
{62 509 546 801 052 686 759, 3 845 861 088 864 673 989},
{71 231 164 682 906 914 255, - 2 225 260 486 070 649 953},
{1 666 526 391 166 450 407, - 243 056 452 504 978 874},
{2 545 420 674 893 324 903, - 458 380 231 442 235 340},

```

```

{14 954 832 104 486 361 001, -2 184 007 298 971 982 018},
{24 324 986 147 178 458 125, 4 818 922 245 628 597 314},
{16 817 369 089 589 423 515, -2 304 926 626 632 176 113},
{49 850 437 330 985 922 852, -9 830 856 610 056 608 281},
{50 819 262 491 310 345 631, 9 132 536 519 675 826 155},
{290 244 833 752 356 624 827, 25 141 287 117 227 056 711},
{835 894 650 768 868 066 465, 157 092 468 302 466 552 767},
{3 681 558 575 727 077 091 990, -232 545 561 436 131 858 169},
{2 859 439 729 325 382 626 122, -63 301 169 361 572 194 253},
{794 758 887 988 273 585 801, 114 906 640 370 969 680 126},
{699 894 406 421 534 780 913, -46 977 437 673 454 328 728},
{348 002 583 660 450 950 511, -26 837 093 040 942 757 931},
{64 212 688 641 757 889 216, -5 096 779 751 526 158 973},
{149 317 713 349 998 952 609, 16 156 947 575 110 731 687},
{285 078 517 702 172 822 098, 46 953 472 522 396 859 611},
{245 110 827 448 791 503 536, 19 555 687 826 431 353 123},
{665 257 343 521 574 355 599, -106 163 638 581 156 153 844},
{2 064 112 378 528 532 575 055, -370 036 975 384 029 338 977},
{11 395 991 585 621 972 492 911, -150 349 233 927 820 087 097},
{2 230 164 081 141 851 231 653, 344 026 950 191 630 349 653},
{12 118 173 739 421 046 762 655, 1 043 622 265 138 991 133 094},
{29 586 421 284 019 818 916 529, -5 663 366 404 195 003 517 560},
{92 680 016 202 270 496 997 217, -8 426 772 594 943 632 917 329},
{1 057 210 973 990 951 818 346, -127 905 089 739 290 218 953},
{2 479 828 693 593 994 870 706, -470 834 714 967 738 569 127},
{9 172 823 669 137 047 830 183, -1 574 948 197 511 087 002 740},
{20 211 182 662 851 615 596 761, 2 563 818 950 942 831 579 678},
{21 853 932 962 445 703 968 399, 3 838 603 294 054 926 626 500},
{85 971 136 537 521 472 713 873, -6 994 702 428 955 100 315 068},
{148 533 639 474 399 632 113 161, 20 445 351 492 007 868 527 913},
{395 381 069 215 152 326 497 210, -78 181 259 883 345 798 615 651},
{326 658 195 284 903 339 583 715, 2 574 291 303 930 143 644 057},
{20 206 422 938 417 934 441 252, -3 297 455 598 890 043 929 653},
{30 783 322 190 669 973 023 382, 3 865 561 426 075 893 869 051},
{10 305 352 909 413 988 818 898, 293 620 988 752 783 540 303},
{2 089 136 123 859 238 305 389, -143 868 333 236 742 410 803},
{5 028 887 852 508 543 535 888, 513 501 495 957 006 773 499},
{7 747 278 815 491 266 534 446, -553 375 947 451 073 177 931},
{1 135 235 865 669 169 076, 6 596 510 759 019 189},
{46 429 103 604 405 464, 1 989 886 535 500 525}, {48 305 070 016 217 397, -8 255 765 699 727 923},
{89 755 265 296 960 293, -3 484 525 719 881 134},
{61 495 449 656 290 943, 10 073 385 766 057 392}, {77 024 859 376 101 143, 983 159 199 362 280},
{24 706 253 286 561 119, 3 066 930 907 255 931}, {12 468 840 081 497 983, 984 089 019 342 308},
{23 675 153 406 497 533, 3 403 085 016 880 388}, {10 690 244 951 558 359, -2 110 247 211 430 518},
{10 147 649 291 621 137, -860 244 799 270 376}, {12 796 045 872 506 375, 1 797 542 077 802 948},
{15 567 346 935 658 947, 1 350 512 997 200 153}, {46 633 059 244 230 897, -5 960 139 337 892 264},
{76 508 048 500 226 695, 9 579 655 349 805 982}, {9 431 183 770 144 753, 1 305 838 717 519 417},
{21 192 830 568 144 882, 2 716 459 923 599 395}, {39 335 963 907 470 294, 4 844 430 962 398 971},
{42 377 683 204 332 398, 109 089 413 502 549}, {3 722 325 870 067 178, 569 866 210 895 107},
{19 471 845 252 495 683, -2 923 280 496 550 016},
{72 351 630 304 873 317, 12 202 476 907 202 081},

```

```

{63 015 873 098 759 337, 10 432 494 200 340 523}, {30 726 276 460 282 527, 4 779 678 329 132 377},
{149 519 073 440 643 345, -7 471 410 448 294 589}, {6 633 106 656 864 245, 46 479 208 139 698},
{979 667 819 217 537, 109 665 762 182 555}, {534 654 951 058 434, 65 491 909 528 201},
{782 536 262 796 298, 117 850 843 279 363}, {3 096 633 731 624 739, 8 075 392 932 830},
{274 351 399 611 977, 44 559 123 223 485}, {510 756 199 787 891, 6 365 629 539 317},
{109 926 074 904 763, -15 670 932 597 248}, {16 756 910 853 971, 1 000 979 847 572},
{18 961 498 496 969, 2 254 972 005 614}, {67 285 739 000 161, 4 233 249 751 904},
{32 576 763 212 119, 1 567 661 201 896}, {25 120 908 021 881, -4 664 340 903 065},
{131 341 855 978 588, 24 741 425 907 123}, {557 335 030 337 029, 34 867 556 450 243},
{39 848 719 280 707, 3 348 794 496 932}, {24 587 471 820 821, -271 353 480 211},
{7 715 726 121 740, 1 417 895 217 283}, {45 716 252 578 725, -5 461 155 284 891},
{147 971 751 870 581, 12 818 755 021 148}, {427 291 511 973 235, 82 706 542 132 126},
{1 004 392 495 820 165, 52 499 004 662 023}, {504 532 728 646 144, 24 241 950 135 551},
{332 020 366 631 171, -54 981 836 334 244}, {155 442 449 676 611, 148 107 057 883},
{5 107 160 339 347, -667 455 647 304}, {16 971 393 253 205, 1 529 839 918 937},
{10 450 252 577 554, -411 381 372 733}, {12 097 432 923 717, -1 195 863 103 663},
{10 132 537 757 351, 1 257 597 394 107}, {5 238 378 128 135, 240 630 434 191},
{4 050 873 956 891, 135 742 581 430}, {1 562 454 478 657, 22 009 063 786},
{13 800 660 877, -302 540 325}, {8 482 167 329, -1 501 953 094},
{38 657 240 155, 2 143 675 157}, {5 189 375 017, -188 186 655}, {5 829 146 579, -156 504 387},
{2 809 350 980, -264 384 851}, {7 218 413 813, -773 029 220}, {19 064 010 809, -3 417 513 961},
{105 198 325 861, -1 268 175 365}, {4 396 748 682, 4 161 587}, {149 560 721, -6 723 186},
{120 495 917, -12 110 168}, {44 220 699, 5 685 914}, {92 462 749, -11 022 175},
{312 830 477, -58 968 049}, {1 313 286 936, -130 933 753}, {288 306 638, -51 943 727},
{1 704 967 852, -272 003 905}, {5 324 942 806, -817 790 923}, {29 170 336 815, 1 757 657 404},
{51 818 250 869, -4 796 995 270}, {69 254 888 373, -7 478 152 367},
{142 460 746 110, 20 034 827 509}, {161 837 608 931, -16 165 607 692},
{13 251 836 803, -857 418 060}, {28 511 310 919, 5 366 948 742},
{122 389 406 257, 2 823 665 678}, {70 940 093 519, 8 855 827 585}, {6 823 517 247, 1 325 878 927},
{14 170 950 676, 1 086 713 955}, {3 187 856 053, -453 621 132}, {913 093 417, -105 390 205},
{2 585 545 244, 503 544 081}, {4 951 213 247, -612 768 376}, {3 581 835 447, -621 542 587},
{10 761 665 475, -1 654 395 074}, {59 794 303 139, 2 001 334 167},
{17 937 696 583, 3 547 225 248}, {14 714 635 039, 1 743 685 436},
{55 856 063 223, -5 847 333 046}, {191 060 508 301, -28 549 186 880},
{641 217 389 707, 46 249 074 952}, {457 685 152 333, 78 399 979 675},
{928 174 977 341, 176 434 216 413}, {3 358 284 355 148, -461 431 831 891},
{9 363 091 829 503, -208 263 899 272}, {641 205 554 801, -80 265 015 524},
{66 763 565 543, -2 129 093 667}, {55 601 316 218, -806 478 893}, {3 338 100 127, 524 798 065},
{13 819 756 801, -120 023 866}, {1 241 891 403, 118 631 924}, {4 056 767 899, 602 166 817},
{11 563 186 860, 1 977 770 159}, {22 150 688 862, -3 583 801 991},
{47 295 014 868, 1 420 482 553}, {30 593 615 187, -5 687 425 190},
{157 423 714 301, 22 585 276 241}, {49 145 015 178, -8 762 741 297},
{250 494 580 092, 42 610 841 585}, {377 444 267 514, 38 224 439 857},
{350 409 567 088, -6 308 097 081}, {207 602 469 704, -34 342 197 039},
{113 097 985 310, 9 062 467 433}, {317 431 456 322, 31 045 586 079},
{509 218 473 836, 41 112 809 059}, {1 158 127 854 344, -219 312 259 677},
{4 494 358 585 007, 59 076 148 878}, {333 702 730 367, -62 146 788 909},
{1 676 721 365 006, 125 947 931 509}, {2 876 072 643 397, 53 803 749 909},
{1 786 594 570 060, -330 784 546 923}, {9 685 043 987 485, -1 062 372 557 949},
{9 029 440 513 912, 1 361 639 541 995}, {36 648 648 443 869, 2 513 678 285 124},
{77 126 385 808 343, 336 980 126 382}, {3 070 608 718 855, -202 932 007 586},

```

```

{1943888169745, -141675162963}, {2888180156801, 16053732942},
{108899411407, -3864434469}, {50752978075, 166271413}, {2934389030, 480651249},
{3685152128, -47607879}, {1412217485, -109267737}, {603206008, 68761929},
{1142548769, -26839210}, {842220053, -48221084}, {1639698625, -263203507},
{4414863559, 78492966}, {1405794799, 145322248}, {3462220713, 394697888},
{6574400367, -83716823}, {2863691450, 423173829}, {7192350769, 537898090},
{14576318727, -1267586027}, {46199687390, -767277621}, {11901199490, 723218907},
{24067879394, -4572293961}, {88067899997, 16081321657},
{559274294976, 63049182721}, {596289514449, -101829756970},
{1072298998083, 191881764907}, {5766386169207, -262831941745},
{1161908090359, -199625157509}, {2616528392735, 20437491987},
{38647543127, 2682958664}, {79286893663, 6870783878},
{230863439729, -43002856509}, {1156988474432, 78170383195},
{1136410964989, 162424133626}, {40731838689, 3814889303},
{89931886012, 7324006289}, {149198169712, 1217907113},
{44121578651, -1268467134}, {20058285847, -3022220790},
{80099956859, -2121597979}, {38015943039, 3854412997},
{38557645963, -5658570799}, {76821522990, -14178281453},
{432898447925, -3174409919}, {86045022693, 7543960936},
{223486024981, 18016431250}, {532086048613, 46939584556},
{1149795150281, -227553818716}, {877902139173, 128842161524},
{1751488379135, 335676755718}, {5336635839785, -935997822246},
{20392629839443, 3518387287646}, {52391653709609, -7084799519474},
{204258166350243, -30328434168968}, {586983716774909, 115307885043551},
{762433283672242, -63289136229825}, {216346370746966, 20967255082347},
{487188854415208, -17716601239741}, {645365328780673, -11421853881948},
{414665001796499, 10145672279569}, {95452001605590, 17751689772863},
{488629350113075, -62917853059826}, {1074083628683909, -100595049237729},
{2369719643971030, -187725205663303}, {5161686164589357, -649790005916408},
{2674273440159211, -372546546290851}, {4850675976997542, -218165733190999},
{3725178816076172, 352422604841989}, {11057298114556611, 628901516847821},
{19193830775404191, -160131895365875}, {1605756800559057, 207367404286577},
{3882317662549807, 285085269811989}, {7947956381716847, 1290626611786720},
{14906359902746471, -531531241957968}, {1714414338405791, 19135794393987},
{569922464871847, -38467663532265}, {517751632185344, -71410735668623},
{1304983222863759, -28803777364409}, {643366626970842, -58003727639729},
{388770474169079, -64309360516808}, {212744707980863, 38257857080160},
{1226577718507081, 130800036165198}, {3604549690481827, -475208143061243},
{14389428142592541, 392105446058381}, {8648555394431588, -1137877678588821},
{33176020502365540, 3987980572441413}, {92868842366899228, -4022232309319603},
{26097445436030207, -3333565511063511},
{41688741630885313, -5068931520241932},
{83022131233339561, -723660382656653},
{249577292760495594, -32540489437060859},
{784503459727363294, -117760745844533789},
{2906988566459245717, 512716926223201110},
{12359848334237148839, 1852278269857257746},
{44245267497746842959, 5398783005588233398},
{77015252071991231575, -3625142388506829121},
{64770119674390862482, -7329439490130715973},
{87223008785347433075, 15295537277814411404},

```



```

{332 165 686 352 349 580 477, -60 924 368 763 395 831 524},
{2 010 700 505 082 040 868 561, 345 149 681 426 557 875 866},
{4 394 423 593 843 366 224 355, -755 707 852 352 331 964 408},
{10 207 116 979 755 666 032 789, -1 601 676 008 153 744 807 974},
{43 585 447 950 823 394 500 985, 4 281 020 363 915 657 561 733},
{56 592 834 751 677 778 506 815, -2 234 703 970 885 464 757 421},
{52 942 190 006 504 648 704 170, 5 121 241 378 910 093 247 547},
{126 273 663 870 471 284 695 100, 22 706 048 527 482 412 644 831},
{727 271 792 492 892 955 693 678, 75 955 606 723 419 141 183 501},
{2 356 752 056 114 787 298 317 236, 72 704 514 176 334 062 196 195},
{2 205 154 980 463 103 486 846 708, 51 306 704 727 454 941 536 931},
{75 432 565 674 506 944 616 725, 405 768 184 661 517 607 162},
{2 943 117 095 079 113 024 711, -391 489 892 176 306 652 751},
{13 782 549 090 187 834 402 681, 1 202 465 990 826 057 042 758},
{40 545 892 950 388 106 061 039, 7 243 654 620 627 158 931 599},
{212 870 538 456 363 869 584 515, -21 396 736 738 559 132 038 157},
{80 068 511 833 603 908 185 015, 3 367 873 482 609 056 170 306},
{55 512 977 677 981 112 870 017, -3 270 656 295 173 771 589 387},
{6 437 091 818 029 302 918 026, 938 229 640 493 134 656 537},
{9 527 643 575 852 696 474 509, -361 586 405 380 918 150 575},
{9 226 983 624 264 192 847 807, -737 209 295 195 639 401 498},
{26 041 816 569 375 714 131 691, 2 089 382 623 809 367 417 639},
{70 753 431 107 421 273 761 679, 11 987 294 406 904 579 084 312},
{85 434 479 382 452 654 326 089, 7 360 350 136 641 087 966 746},
{210 949 724 778 549 293 064 999, -34 493 887 214 969 599 746 296},
{291 007 308 677 413 704 867 279, 25 270 383 118 040 365 168 666},
{893 322 077 952 159 432 440 049, -70 331 100 451 698 469 589 233},
{1 531 702 638 154 209 072 058 540, 266 293 455 552 392 324 978 649},
{4 822 240 946 690 576 080 374 842, -282 574 658 882 625 157 568 717},
{1 348 437 435 074 233 324 585 669, 263 594 272 376 005 827 708 202},
{2 224 023 343 176 905 581 260 107, -194 972 814 453 845 273 793 696},
{5 790 534 045 476 352 575 649 923, -430 920 607 008 987 888 815 334},
{13 765 329 268 244 231 536 692 413, 1 353 306 546 898 627 779 281 712},
{16 955 257 345 830 623 302 896 389, -2 243 374 753 610 050 698 187 479},
{72 397 069 862 634 106 630 051 339, -8 796 521 837 128 416 205 313 115},
{147 817 347 089 294 720 090 888 587, 3 795 463 718 187 476 039 450 266},
{15 018 868 161 229 717 680 040 451, -2 614 466 125 213 923 685 705 560},
{48 758 787 073 929 183 696 082 357, -2 843 263 974 992 656 859 437 730},
{30 900 863 430 943 247 251 789 131, 1 128 382 859 166 472 482 032 581},
{31 720 415 041 739 787 294 389 412, -5 836 876 670 891 026 904 238 719},
{185 130 313 171 779 652 443 294 641, 15 177 516 612 484 618 526 645 671},
{219 008 309 003 388 799 018 900 997, -23 084 198 169 137 604 131 930 070},
{821 288 360 123 976 413 701 716 791, -53 820 271 580 242 636 058 991 895},
{1 020 852 908 684 591 715 629 200 718, 126 563 236 539 980 684 576 717 805},
{609 332 194 626 475 448 128 454 294, 40 704 233 468 234 579 065 377 409},
{89 885 439 984 156 363 211 099 393, -7 652 138 498 050 761 510 684 570},
{141 636 205 449 052 568 949 427 631, -4 058 267 453 599 135 683 506 020},
{29 430 346 164 954 138 049 664 037, 3 965 839 597 781 424 265 714 435},
{121 871 235 575 344 277 845 398 416, -981 311 966 201 293 604 206 853},
{13 764 278 946 022 577 433 651 012, -551 757 605 975 094 853 861 481},
{2 165 267 844 899 955 640 678 949, -149 914 936 402 178 931 747 606},

```

```

{4 851 487 674 669 893 523 509 945, 620 029 579 525 341 723 393 672},
{7 938 674 191 897 339 245 678 463, -1 110 080 923 016 798 770 129 070},
{12 271 864 346 921 593 398 573 029, 1 841 203 894 189 382 184 639 579},
{45 009 092 605 497 978 254 993 752, 8 634 711 401 922 099 907 044 301},
{133 994 098 499 785 946 543 374 031, -8 432 455 028 529 301 266 507 983},
{67 538 282 837 849 781 615 019 881, -1 527 148 024 837 779 287 633 140},
{25 095 191 384 086 986 018 805 633, -1 819 257 162 147 634 024 630 221},
{27 331 848 676 531 993 799 274 653, 2 511 480 515 775 450 343 929 705},
{21 493 900 780 851 078 828 503 446, -4 025 946 479 850 244 880 038 347},
{99 584 291 856 789 373 266 754 903, -16 967 911 564 297 427 295 521 998},
{162 291 959 616 648 906 965 527 205, 13 686 725 717 362 223 559 332 019},
{142 258 676 393 937 629 491 362 679, 18 115 996 298 796 619 819 328 619},
{194 858 461 739 779 021 618 437 929, -6 505 789 569 536 018 620 716 598},
{23 011 450 280 012 201 223 380 803, -437 183 646 588 441 302 184 934},
{11 627 658 209 788 708 846 711 027, -420 040 601 606 906 801 901 715},
{9 743 940 369 941 757 277 200 489, -304 079 450 181 936 177 757 181},
{978 051 380 745 369 994 860 881, -50 965 173 252 620 407 712 072},
{709 055 493 027 504 128 200 449, -58 623 114 956 782 142 000 855},
{407 202 288 866 644 965 883 797, -73 589 778 071 804 526 659 909},
{2 506 555 708 185 300 167 522 961, 393 278 762 435 312 305 203 092},
{10 722 468 750 860 122 550 221 857, -1 107 926 457 627 747 989 969 311},
{26 046 095 255 467 086 511 401 469, -1 898 000 090 001 301 809 570 993},
{38 391 138 332 233 134 049 247 609, 1 292 539 382 247 799 402 057 476},
{28 108 148 869 661 904 910 796 983, -5 025 367 537 492 617 455 608 076},
{149 216 113 936 447 387 068 157 529, 11 186 024 415 839 905 083 233 246},
{277 239 146 728 589 331 987 149 163, 45 627 086 659 003 010 892 584 765},
{253 793 754 543 702 464 109 761 829, 3 645 502 842 517 628 678 659 484},
{101 575 443 574 802 667 937 349 723, 16 341 512 300 116 415 927 474 021},
{257 424 993 509 604 583 192 908 581, -34 246 283 479 753 622 926 344 223},
{1 207 805 025 974 981 215 902 699 819, 100 913 916 400 476 442 035 573 844},
{230 823 870 643 734 462 265 600 557, -30 943 569 927 054 892 484 653 732},
{1 037 978 324 267 565 685 730 783 609, -197 142 837 294 225 994 791 179 651},
{3 815 282 059 139 806 959 566 630 842, -750 487 157 608 776 846 511 037 129},
{4 587 777 790 002 359 071 835 499 381, -109 306 651 987 937 295 348 389 027},
{226 416 324 843 535 294 169 301 969, -25 827 205 170 503 388 211 003 522},
{440 082 083 442 649 580 270 270 217, -37 712 441 980 721 374 380 526 445},
{910 107 083 798 504 597 611 439 979, -139 386 851 040 943 322 904 502 051},
{4 788 863 764 631 202 378 565 429 594, 663 113 470 214 556 477 617 864 913},
{10 736 071 538 439 413 572 547 389 819, 1 492 121 397 413 678 624 424 448 892},
{21 259 188 227 687 413 715 066 072 975, -865 740 205 762 487 411 260 566 659},
{28 055 134 895 358 324 350 710 825 500, -3 672 108 428 548 671 539 946 902 893},
{96 486 474 911 266 501 727 101 028 012, -247 788 921 249 715 263 348 810 543},
{7 050 671 794 290 292 762 202 055 305, -1 282 880 399 085 228 736 474 709 049},
{46 447 695 317 082 882 827 481 234 380, -1 391 148 297 920 081 187 519 801 877},
{39 405 508 457 574 865 670 927 388 047, -7 628 367 232 850 493 445 913 132 635},
{92 248 077 412 535 086 219 405 915 656, -7 173 360 402 842 699 559 308 363 035},
{73 409 371 182 660 587 767 004 677 327, -1 271 974 939 727 135 107 153 081 523},
{26 657 798 470 467 136 694 805 723 511, -2 456 588 314 876 982 072 952 361 648},
{26 621 128 502 115 625 859 928 587 041, -452 838 651 555 699 755 913 125 877},
{7 033 691 595 958 160 943 046 298 246, -473 253 441 823 506 971 494 027 275},
{4 753 032 291 794 384 943 580 094 167, 560 064 865 216 434 390 998 112 237},

```

```

{19 893 476 014 592 416 538 449 327 783, 1 370 296 501 677 787 281 558 734 006},
{48 250 920 271 930 666 000 012 808 411, -4 190 775 589 191 532 238 693 647 923},
{148 802 236 280 843 623 094 700 566 545, 10 360 532 247 662 328 099 546 131 954},
{274 099 291 390 685 168 176 994 500 797, -5 902 463 075 569 078 047 240 362 725},
{188 777 263 759 053 194 287 460 527 631, 19 082 440 607 775 875 236 633 408 853},
{149 441 389 265 505 739 757 769 945 627, -27 574 237 791 031 653 665 573 726 636},
{844 624 622 655 365 414 382 795 808 631, 295 495 255 149 311 215 946 321 350},
{7 240 391 020 279 022 199 285 494 163, 1 436 915 583 205 999 497 575 221 357},
{4 074 356 610 178 803 932 885 278 594, -312 863 935 373 617 683 704 048 469},
{520 157 873 489 505 265 483 340 281, 97 757 303 516 559 083 999 973 606},
{2 290 108 981 189 818 720 293 474 323, -141 871 413 647 871 020 167 488 994},
{1 472 144 486 143 415 025 796 480 587, 170 228 197 772 027 082 098 822 156},
{4 373 378 447 752 496 055 783 073 641, -265 071 794 977 748 235 351 497 537},
{9 652 770 151 922 273 181 615 252 577, -176 930 457 639 599 107 587 928 096},
{5 723 566 332 664 474 707 617 867 319, -726 549 768 797 191 161 499 179 314},
{6 484 722 693 052 984 659 416 405 089, -1 060 443 865 055 287 095 280 330 615},
{8 910 343 698 652 132 404 612 762 127, 461 560 587 129 254 019 096 717 667},
{10 270 555 653 330 341 049 584 231 142, 1 053 252 838 892 541 702 231 052 363},
{19 124 009 698 440 546 009 019 351 624, -915 363 916 583 512 172 242 000 979},
{7 200 176 136 364 301 388 574 832 255, 1 033 655 185 185 579 995 865 891 822},
{35 410 159 934 758 582 486 410 499, -6 760 547 077 581 103 759 987 351},
{117 341 991 920 273 649 112 583 312, 19 248 493 782 706 741 506 047 713},
{135 125 133 354 423 605 569 683 482, 9 464 011 216 559 272 413 519 413},
{191 915 271 549 346 799 970 054 100, 4 709 998 611 847 231 499 463 449},
{87 211 022 156 447 480 080 153 557, 2 624 846 888 162 637 843 887 833},
{43 148 463 836 871 479 925 419 964, 3 060 946 617 214 999 642 045 117},
{21 550 417 297 888 400 385 547 798, 859 861 377 135 331 530 895 737},
{3 933 449 473 873 184 260 269 229, 265 751 904 949 150 496 316 121},
{3 856 524 326 577 342 466 498 778, 516 681 775 967 604 315 088 089},
{17 501 888 320 700 195 044 397 315, 2 953 744 899 038 837 173 518 022},
{16 102 418 367 896 443 759 889 641, 1 869 560 873 533 291 090 049 956},
{52 824 953 054 931 851 690 877 299, 10 418 843 494 414 488 690 025 701},
{53 343 697 548 736 801 574 661 962, -2 312 373 412 964 528 969 864 763},
{11 614 960 690 342 374 547 386 149, 1 920 752 096 567 027 519 671 450},
{6 602 712 098 635 288 343 093 777, 1 196 156 534 291 116 013 616 737},
{41 918 578 819 132 764 918 285 085, -4 056 496 472 097 346 896 058 276},
{98 813 829 165 628 604 912 269 725, 17 914 228 309 850 338 774 685 252},
{633 022 470 623 560 224 716 450 451, -50 365 266 065 427 708 854 964 281},
{1 585 997 140 570 999 299 060 219 746, -103 657 528 721 775 582 854 432 635},
{2 272 797 311 338 685 605 792 306 133, -343 862 935 996 808 499 828 171 083},
{9 799 756 566 645 094 189 357 075 704, 1 743 670 456 585 563 104 605 377 107},
{48 345 430 619 384 763 994 088 646 474, 7 152 089 761 515 634 333 670 419 603},
{125 501 432 919 401 372 937 113 224 531, -23 535 216 335 485 167 292 696 314 389},
{571 250 640 664 214 162 575 110 638 778, 97 410 695 647 907 249 515 712 449 555},
{964 587 925 295 741 419 898 976 274 296, 169 676 023 702 134 105 412 387 444 637},
{3 903 179 834 945 614 518 000 432 727 398, 18 276 594 502 875 622 376 543 839 531},
{584 831 372 893 112 952 336 272 053 228, 59 790 229 829 828 247 423 413 923 301},
{954 177 554 577 375 098 544 304 124 086, 183 995 263 421 531 558 548 562 163 163},
{2 496 690 335 289 363 323 509 011 503 783, -454 048 182 933 422 381 361 245 247 127},
{16 530 807 705 424 353 419 303 324 574 804, -310 351 363 913 378 417 467 039 158 811},
{5 999 535 515 116 702 429 168 188 520 933, 1 178 121 658 759 590 654 478 397 174 887},

```

```

{7 951 687 156 268 688 444 662 793 194 354, 712 866 796 869 528 021 156 321 558 817},
{8 041 124 521 383 255 471 857 691 457 791, 928 566 884 875 127 202 740 667 815 353},
{23 066 353 301 980 922 755 007 278 268 178, -3 641 961 769 827 747 179 980 017 802 411},
{88 664 535 860 054 096 284 283 516 120 976, 15 919 973 261 924 460 490 962 477 685 181},
{500 437 170 938 964 666 288 868 549 278 030, 30 664 797 679 238 383 259 234 027 260 927},
{715 429 789 193 988 992 302 060 256 533 454, -35 164 441 922 521 942 816 710 249 894 265},
{886 289 404 279 159 925 653 433 881 315 242, -102 391 259 403 424 224 145 230 736 706 083},
{2 571 930 915 671 040 690 715 920 679 883 865, 322 480 075 063 375 756 912 365 724 524 544},
{577 406 993 025 471 614 559 373 490 811 551, 85 183 125 402 113 754 833 584 535 106 957},
{1 377 866 589 620 700 857 127 432 610 411 804, -197 279 906 559 734 603 897 547 737 857 649},
{225 771 209 713 220 021 344 313 485 196 947, -38 645 973 893 131 171 048 873 525 221 014},
{445 638 256 126 391 361 271 719 627 427 001, -11 393 917 344 514 809 734 669 742 785 546},
{93 110 017 392 906 058 230 775 091 721 611, -17 999 923 729 388 437 326 308 914 873 792},
{227 059 108 455 362 626 743 827 766 743 523, 39 029 022 248 928 220 844 724 262 616 369},
{519 396 827 789 088 977 689 800 053 692 443, 39 581 541 340 159 398 089 359 264 609 609},
{353 085 696 792 226 584 553 461 805 029 398, -56 152 815 681 596 679 107 708 467 921 877},
{1 180 322 597 293 195 223 226 402 817 363 928, 120 901 960 634 181 510 919 352 188 716 475},
{2 094 881 660 549 251 675 599 692 095 460 006, 328 502 760 214 493 326 398 273 490 159 543},
{9 042 152 246 147 295 356 333 734 278 700 604, -1 163 913 654 587 205 766 566 419 582 411 205},
{19 648 460 310 175 606 662 426 433 782 999 628, -895 383 200 695 876 647 692 909 891 884 519},
{3 647 817 674 758 609 837 683 620 207 564 670, 151 986 451 347 134 484 635 512 917 543 937},
{10 427 497 198 901 069 485 643 615 243 286, 1 582 352 983 901 509 980 738 226 952 917},
{47 375 079 253 893 527 705 250 060 180 709, -2 590 346 041 557 162 556 719 191 241 799},
{54 666 086 928 115 922 954 237 101 467 871, 6 354 720 996 988 172 963 004 292 542 020},
{184 427 349 268 767 261 034 511 792 952 557, -24 300 676 988 828 360 271 846 890 173 694},
{728 398 864 855 752 343 239 222 975 900 635, 37 765 824 500 896 221 439 003 834 642 532},
{791 918 551 726 861 920 564 958 591 554 471, -74 474 838 841 575 304 369 900 788 844 711},
{1 993 241 313 724 049 207 788 356 258 826 550, -106 185 897 249 687 564 299 109 819 018 147},
{1 773 223 583 461 059 514 315 312 083 831 739, 2 826 346 842 562 261 416 050 285 005 214},
{80 600 261 740 077 270 980 187 146 066 953, 14 207 627 140 285 560 761 361 717 495 008},
{339 121 580 419 434 831 922 770 599 925 935, 40 599 474 338 727 776 832 687 488 382 456},
{1 045 782 356 801 721 060 072 760 579 238 951, 55 627 127 675 766 404 748 236 000 063 027},
{812 714 039 762 366 000 491 809 802 975 026, 136 386 706 934 970 017 562 502 073 776 903},
{409 252 734 864 149 656 473 792 697 106 616, -38 858 538 106 499 743 677 181 780 486 471},
{1 327 956 454 436 369 250 190 102 841 853 245, 198 951 557 209 090 312 029 271 180 050 458},
{4 723 424 559 990 194 183 080 065 550 497 153, 487 967 802 061 407 913 295 740 948 307 518},
{11 406 502 625 543 601 341 046 107 078 195 971, 629 153 314 258 530 700 954 703 131 653 450},
{5 967 236 728 973 556 841 885 901 715 672 583, 887 816 082 455 894 322 033 988 263 638 929},
{18 065 736 919 892 349 101 697 177 475 394 160, -219 377 634 459 694 884 604 933 367 862 697},
{5 604 275 276 407 905 178 762 815 677 669 438, -430 075 793 491 908 065 353 949 791 416 663},
{970 167 153 956 324 028 787 192 415 455 787, -177 414 505 136 615 570 549 088 418 544 568},
{6 065 907 863 946 970 851 047 773 559 505 131, -902 537 775 352 241 124 029 657 757 476 149},
{18 385 529 136 866 342 252 667 644 226 437 576, 150 694 522 328 460 575 449 192 417 673 845},
{58 211 133 973 099 494 230 356 726 679 478, -6 786 080 497 246 736 809 559 743 830 059},
{209 042 106 654 843 005 064 710 648 746 869, -2 880 871 070 066 060 590 627 096 048 915},
{1 261 481 459 979 418 051 067 362 823 926, -125 947 752 350 634 489 999 220 819 073},
{146 287 362 534 340 028 486 288 223 308, -12 149 001 975 139 543 584 590 488 257},
{36 451 734 784 581 899 397 772 588 352, -3 546 749 199 907 503 118 123 330 505},
{71 849 723 342 001 379 807 367 681 046, -2 025 324 575 955 123 106 250 185 043},
{70 325 512 400 761 189 468 617 931 493, -8 161 032 426 773 678 907 638 849 694},
{228 035 899 134 740 211 109 615 249 969, -38 371 859 206 511 341 869 102 270 197},

```

```

{160 253 695 615 932 327 664 881 098 549, -1 067 046 996 017 533 455 943 407},
{22 598 320 561 067 575 781 701 253, 2 902 304 447 413 719 072 624 810},
{45 268 396 331 678 906 348 697 571, 3 931 801 687 076 033 853 823 866},
{139 665 345 666 045 492 494 783 933, -9 604 055 737 692 986 236 763 173},
{320 870 799 152 498 977 136 447 326, -63 719 260 635 190 388 575 765 559},
{166 038 206 287 933 500 806 225 763, 31 681 189 341 445 170 407 728 522},
{557 154 949 391 658 360 033 570 169, 99 371 543 520 279 297 165 067 736},
{2 852 424 756 291 271 875 849 046 031, -455 192 435 957 357 098 560 437 750},
{8 852 720 259 940 437 767 508 625 763, -1 577 541 142 086 324 943 956 458 159},
{44 714 441 258 158 368 424 798 992 943, 8 580 876 263 814 650 964 780 010 373},
{132 134 375 553 213 292 865 622 698 694, -3 496 891 543 150 012 683 890 737 915},
{54 567 725 313 564 805 922 449 971 548, -4 857 991 447 590 888 610 395 174 653},
{82 476 815 474 747 278 191 522 676 645, 5 779 009 756 610 086 826 025 316 766},
{114 659 558 401 042 571 783 281 660 233, 11 920 523 976 753 992 608 936 982 537},
{331 834 739 754 306 864 344 436 055 001, 52 575 067 095 921 463 683 497 797 610},
{1 196 056 614 050 800 003 771 796 661 893, 36 813 672 525 751 768 415 108 738 418},
{1 315 393 805 552 269 257 647 143 373 741, 74 629 576 502 083 993 496 968 189 549},
{2 039 515 718 422 711 646 774 734 784 293, 223 570 926 852 121 410 272 981 905 546},
{1 998 548 503 014 183 665 206 527 309 667, -352 144 782 749 080 229 671 980 231 953},
{8 345 374 124 061 733 036 250 847 989 723, -815 715 746 746 212 609 427 590 103 263},
{13 739 815 931 771 306 764 171 127 867 789, 493 863 942 801 094 001 794 001 774 468},
{6 451 336 066 130 745 882 447 292 663 995, -172 034 360 793 795 990 227 871 706 274},
{6 275 784 014 445 627 473 463 748 732 441, 92 909 953 089 354 085 918 969 267 537},
{3 072 774 081 022 876 938 909 786 585 475, 541 719 864 175 515 938 467 337 522 849},
{12 960 792 594 205 964 508 279 414 268 187, 1 644 914 050 198 073 011 347 704 807 631},
{14 491 945 938 639 229 522 662 366 078 853, 819 837 029 119 995 915 472 082 495 286},
{19 353 802 743 010 877 775 963 675 049 535, 1 659 872 715 041 991 924 285 547 864 562},
{41 220 898 136 990 848 028 791 650 740 257, -6 542 731 186 981 271 433 876 431 095 599},
{143 409 304 102 535 018 063 913 684 166 399, -21 852 821 145 685 907 949 308 583 312 911},
{697 912 405 960 442 643 430 987 128 750 394, -68 261 297 969 271 458 837 346 848 329 669},
{1 116 858 117 544 148 019 198 861 118 120 392, -102 557 772 351 566 931 777 872 028 334 261},
{823 248 617 585 440 816 114 377 129 622 967, -35 293 959 835 463 628 822 048 033 770 440},
{838 590 519 993 746 784 130 881 761 907 831, 88 650 529 799 501 040 077 679 408 218 384},
{2 973 709 881 271 331 910 518 997 419 793 375, 564 804 664 619 149 528 064 369 048 297 657},
{10 927 118 746 817 651 724 392 109 016 271 570, 2 162 548 833 370 421 027 242 221 988 100 471},
{8 349 344 337 484 900 937 212 932 531 152 695, -1 343 350 476 000 115 759 268 508 339 412 897},
{21 114 628 148 347 065 856 937 422 111 297 849, 2 591 450 808 495 370 370 853 999 369 867 443},
{27 960 582 668 039 510 977 696 182 122 156 265, 346 220 590 799 312 250 366 367 887 678 974},
{6 079 818 629 449 035 044 512 024 928 365 917, -1 121 398 983 963 216 702 655 989 646 782 692},
{34 516 130 803 205 461 779 941 598 695 029 361, 409 199 646 818 747 140 494 100 619 591 002},
{10 465 314 341 441 244 425 911 705 405 119 089, 769 398 720 336 039 633 328 575 404 948 967},
{22 357 545 258 221 662 170 249 569 284 150 777, -2 875 519 256 714 876 553 213 058 596 312 465},
{47 202 442 071 306 568 648 207 662 503 472 839, 3 644 699 976 531 256 894 440 341 385 497 128},
{13 042 006 522 783 281 504 724 612 083 257 225, -1 828 472 982 720 474 588 833 944 824 339 169},
{17 716 781 993 017 034 950 750 876 840 462 066, 246 771 962 122 974 985 858 098 221 796 805},
{3 708 347 428 112 974 265 350 244 410 276 262, -336 203 851 644 091 168 437 265 331 219 653},
{737 669 382 041 913 115 443 780 980 785 767, 73 045 058 119 705 652 313 198 892 117 775},
{526 972 461 674 531 238 760 820 351 385 241, 98 658 630 217 483 192 814 275 908 785 250},
{2 458 589 672 859 415 052 329 178 944 506 343, 365 179 956 691 872 313 485 657 427 148 077},
{7 129 911 750 809 453 371 140 882 323 704 308, -1 166 260 578 763 290 804 072 577 298 428 465},
{9 661 424 310 768 723 909 495 552 918 746 814, -698 820 739 166 175 899 241 118 646 093 461},

```

```

{8 910 820 741 714 923 631 247 893 238 999 720, 1 455 102 710 688 936 613 277 761 780 796 813},
{13 154 926 863 435 188 465 436 546 457 975 466, 1 703 900 883 136 080 852 109 528 551 238 989},
{34 768 454 720 702 459 655 096 782 491 360 558, -75 631 837 381 272 478 238 594 785 033 791},
{1 619 904 651 850 264 429 947 759 565 381 046, -270 589 763 398 876 434 012 241 604 375 079},
{265 276 783 638 574 711 175 374 443 468 244, 46 258 239 460 573 399 276 437 024 472 723},
{895 903 678 115 194 967 277 082 345 870 862, -173 689 015 031 914 497 052 252 207 436 245},
{2 004 478 015 760 441 187 154 955 534 343 501, 61 493 674 079 073 370 526 676 089 145 683},
{1 811 365 705 975 542 936 450 944 744 874 774, -171 536 388 049 829 049 235 513 608 892 247},
{5 514 023 067 798 092 175 198 461 564 615 839, -620 857 559 990 808 700 116 168 362 416 051},
{5 379 732 964 700 587 186 834 919 890 389 260, 442 363 858 744 684 467 624 588 905 042 143},
{5 209 766 162 799 270 999 809 271 181 498 712, -821 568 442 307 372 821 096 815 797 887 977},
{20 465 952 153 717 487 345 671 476 774 472 050, -3 062 327 970 566 299 074 707 145 229 139 771},
{70 835 085 738 002 250 941 333 407 553 963 331, -1 569 782 685 872 800 674 999 638 718 269 221},
{14 225 135 782 014 101 343 525 561 924 932 178, -1 572 509 307 506 520 792 167 791 961 589 253},
{5 296 297 055 245 237 623 126 701 755 909 773, 927 283 608 409 653 526 368 848 457 081 626},
{19 520 535 450 525 898 061 306 396 020 338 759, 2 100 895 936 605 695 232 621 588 130 416 865},
{44 710 457 538 448 790 642 983 507 800 849 102, -6 489 794 128 265 540 591 482 909 438 769 069},
{52 421 399 236 929 525 309 970 653 749 009 813, -5 218 635 363 081 199 585 452 077 416 290 090},
{17 158 329 246 579 650 247 841 209 785 950 649, 753 682 829 940 265 912 602 796 451 698 142},
{12 875 436 469 391 999 167 686 928 026 783 041, 1 245 047 027 183 160 085 367 503 417 046 457},
{31 022 532 421 909 076 922 868 251 511 248 383, 4 620 294 879 609 828 487 413 296 611 741 748},
{96 325 816 681 259 741 698 812 208 278 901 269, 7 116 256 717 370 090 054 308 612 559 198 029},
{241 029 747 420 270 891 490 110 831 140 593 001, -40 729 022 889 396 310 045 815 422 090 141 252},
{244 140 463 875 808 721 289 064 202 218 579 303, -33 387 863 654 234 304 174 223 746 248 493 993},
{761 055 535 620 307 221 073 352 428 975 858 696, -18 617 002 047 990 844 594 802 468 983 907 825},
{163 633 029 354 170 733 889 062 353 598 435 417, -6 061 794 012 969 398 530 638 577 071 265 336},
{2 584 856 708 220 929 987 083 594 778 191 815, -66 078 095 061 358 065 546 218 080 089 317},
{570 203 060 441 476 447 019 544 793 716 996, -66 801 435 248 191 439 190 320 129 072 873},
{2 263 719 545 833 994 915 613 554 859 536 853, 380 075 538 242 231 735 359 596 071 184 884},
{1 221 558 904 215 871 247 713 574 432 788 923, -84 735 268 822 160 893 982 861 999 235 029},
{2 574 355 271 510 167 432 605 970 375 391 741, -49 540 141 240 085 900 838 804 775 415 159},
{126 441 327 123 857 003 867 090 072 346 471, -138 059 810 899 431 568 403 053 041 769},
{1 566 555 181 628 833 677 775 515 717 109, 121 083 945 305 369 884 000 415 984 225},
{550 135 835 891 161 438 782 121 680 568, -97 243 491 761 217 025 355 556 581 865},
{2 432 733 371 358 272 074 638 900 175 406, 333 776 619 312 278 040 658 414 919 879},
{7 029 683 640 579 782 672 189 688 746 469, -767 833 231 180 734 229 764 598 010 866},
{8 700 472 876 581 746 114 506 385 353 275, -750 190 057 920 582 373 761 369 808 018},
{22 031 970 747 962 693 055 993 821 034 693, 2 249 313 815 250 340 794 950 888 313 580},
{33 665 220 531 472 187 226 599 533 380 811, -3 713 651 733 106 095 088 173 235 706 104},
{17 691 910 146 765 194 611 950 077 888 875, 3 006 853 291 356 909 332 059 794 719 033},
{25 492 300 900 467 080 769 834 401 048 579, 3 295 435 409 000 379 460 379 476 866 665},
{63 596 313 122 124 708 663 703 213 586 093, 12 076 102 888 399 224 220 708 215 308 345},
{234 753 303 649 386 891 891 836 004 238 864, 42 232 055 339 582 014 909 381 948 929 137},
{1 360 649 072 331 679 422 205 265 321 524 934, 160 250 899 740 817 287 830 407 672 629 691},
{5 740 856 831 575 301 728 026 287 655 580 638, 295 243 892 334 199 675 129 188 731 293 573},
{9 579 270 037 462 076 741 734 228 553 200 823, -1 279 976 496 841 798 415 045 329 030 047 845},
{45 218 722 848 572 612 058 435 550 029 211 284, -3 620 273 131 875 548 017 854 844 477 936 025},
{129 607 504 422 820 616 624 951 389 460 465 832, -6 840 375 047 339 807 897 678 284 262 377 145},
{26 252 367 794 408 540 458 328 841 303 094 379, -1 245 717 021 134 959 332 413 291 228 761 231},
{6 738 655 591 930 796 868 429 961 434 922 544, 80 663 123 500 923 696 459 082 421 438 745},
{2 704 415 096 715 935 291 706 223 513 038 628, -516 624 604 282 352 892 233 531 704 883 165},

```

```

{8 854 321 497 204 470 629 315 244 169 464 619, 978 575 909 418 733 808 754 416 914 203 112},
{3 441 096 807 818 243 588 360 911 739 472 603, 351 466 234 281 111 446 630 586 748 817 788},
{5 370 284 054 479 574 089 981 769 655 485 221, -56 228 925 002 070 079 188 232 114 262 128},
{2 021 570 437 498 206 382 461 471 898 571 891, 89 263 395 873 856 527 906 513 857 670 629},
{2 298 599 734 836 044 435 349 318 433 238 048, -124 231 375 891 293 381 341 105 555 882 989},
{4 511 137 718 192 676 139 613 160 383 328 239, 108 411 410 777 594 368 806 071 941 340 462},
{3 076 332 016 038 976 567 655 864 166 895 045, -581 405 989 630 389 980 759 411 100 871 016},
{12 359 050 955 752 946 461 693 032 365 417 445, 1 745 202 475 495 490 671 712 050 559 346 697},
{10 412 254 791 769 358 458 733 526 849 311 318, -827 850 217 605 252 943 122 235 709 209 953},
{25 535 256 708 221 875 535 454 228 040 519 183, -431 792 570 030 320 674 940 295 680 417 785},
{4 343 140 579 605 767 120 305 151 398 500 364, -464 427 714 210 526 574 760 913 026 427 209},
{11 920 254 074 905 040 164 356 193 727 850 259, -755 119 340 029 766 623 789 016 316 123 208},
{11 800 841 686 699 484 587 568 915 098 838 037, -1 132 355 396 613 620 524 689 239 805 137 828},
{34 842 003 601 119 391 869 385 744 464 562 261, 386 119 425 216 306 975 399 460 482 936 274},
{6 661 639 210 578 778 090 703 973 021 724 873, -923 732 756 122 333 411 381 403 840 586 717},
{14 272 223 993 738 427 405 492 668 046 103 342, 604 960 170 480 246 409 040 375 528 182 851},
{18 017 867 138 486 508 037 773 158 010 810 986, -1 215 395 430 035 352 263 063 447 887 743 855},
{15 553 694 779 195 641 297 034 902 290 319 247, 2 219 755 702 807 696 483 136 211 834 484 781},
{1 124 554 746 548 911 800 943 619 771 581 940, -124 790 091 207 944 793 159 074 924 297 047},
{105 406 574 450 832 363 372 018 062 321 741, 18 821 474 397 594 499 906 683 813 960 043},
{549 125 851 235 628 432 970 191 965 011 741, -65 092 314 380 571 817 341 159 488 781 181},
{2 072 275 541 946 934 279 586 871 997 647 389, 187 657 547 461 634 932 014 750 847 612 769},
{587 103 950 433 352 001 996 725 195 205 890, -61 750 531 074 146 886 435 473 179 025 093},
{2 219 299 302 492 530 952 134 481 438 287 920, 99 591 523 735 777 667 878 585 787 300 989},
{2 064 861 962 295 824 892 808 370 589 629 826, -112 407 427 003 439 793 123 302 237 896 085},
{3 031 564 165 075 329 010 991 912 447 521 608, 224 497 904 232 344 269 551 789 056 145 883},
{8 132 674 074 956 825 679 518 806 712 015 042, -234 405 353 224 971 080 976 122 013 140 129},
{5 220 470 017 952 837 289 118 853 595 931 529, 520 507 988 641 269 033 509 317 448 871 681},
{1 123 479 602 430 727 643 874 574 826 674 487, 60 408 924 350 397 772 881 174 483 350 378},
{1 773 167 096 558 592 983 345 046 059 736 735, -183 398 398 110 610 309 338 915 169 588 664},
{4 439 632 571 968 238 033 219 711 438 943 065, -721 434 152 947 792 948 491 700 206 805 488},
{8 105 018 762 548 064 985 674 244 462 040 001, -1 147 861 578 582 006 426 841 383 173 697 056},
{5 109 103 010 603 459 838 273 043 969 724 457, -578 505 104 876 691 793 576 460 994 920 987},
{7 113 334 129 933 940 185 802 663 873 203 098, -156 803 323 744 841 271 989 015 656 293 259},
{4 174 472 983 374 055 079 678 031 820 470 339, 161 823 334 091 425 243 084 603 111 900 022},
{2 404 160 319 219 090 558 080 383 491 907 009, -352 174 743 629 611 043 642 144 220 980 522},
{4 457 590 691 737 632 561 267 702 011 835 085, -853 599 206 899 628 939 485 805 774 562 469},
{13 840 409 978 482 614 060 223 139 148 660 020, -1 832 046 444 276 284 017 927 090 194 806 177},
{59 565 195 028 119 040 073 131 515 914 625 908, -8 237 923 744 443 773 167 005 755 082 503 983},
{138 680 203 641 921 836 998 659 814 608 155 971, 4 645 059 282 632 860 213 682 356 511 479 854},
{49 024 963 105 669 767 062 194 293 745 494 377, -8 002 932 959 661 875 576 047 822 371 882 385},
{73 537 670 381 991 493 231 237 244 536 604 891, 57 795 609 820 974 374 777 485 088 624 755},
{1 580 792 348 982 461 542 163 461 831 906 763, -176 822 494 622 839 039 314 585 131 448 678},
{774 537 491 485 556 251 749 717 632 587 747, -15 062 887 456 140 741 420 985 082 217 408},
{462 106 879 233 626 067 401 926 083 495 547, 1 869 448 395 574 310 897 337 471 118 602},
{25 778 163 454 303 130 448 662 355 662 269, 3 341 409 284 153 734 147 475 006 936 365},
{69 577 089 781 652 219 373 052 087 491 523, 4 839 045 996 657 260 061 264 148 923 266},
{133 622 545 476 892 231 620 842 187 303 327, -18 330 145 419 487 454 144 579 649 458 779},
{387 741 510 455 043 840 441 278 799 706 802, 48 208 072 442 709 578 338 476 914 488 247},
{151 615 956 675 806 602 542 834 317 460 298, 25 791 492 034 145 719 023 235 004 652 699},
{228 708 673 621 942 946 550 026 863 280 408, 25 215 358 709 598 873 618 452 327 993 637},

```

```

{129 242 502 195 375 130 828 781 527 650 275, - 7 623 640 116 701 905 102 951 492 997 199},
{26 234 724 564 679 682 261 751 291 053 884, 4 158 993 506 736 721 333 106 463 455 531},
{93 495 737 270 932 861 207 213 253 410 954, 6 469 388 363 610 468 274 669 437 851 827},
{213 473 913 168 200 291 414 402 014 432 448, - 36 562 880 843 652 948 909 486 523 272 053},
{430 946 148 241 370 349 103 750 139 590 510, - 70 074 257 098 209 277 335 429 893 879 811},
{766 544 212 604 372 011 655 466 670 750 012, 61 377 818 323 262 504 460 810 468 414 289},
{2 190 758 668 941 202 943 179 096 633 833 712, 129 073 792 440 978 897 406 711 976 354 217},
{255 193 586 546 996 829 655 508 385 722 321, 5 792 643 825 669 935 623 808 141 116 128},
{23 159 849 878 935 341 180 362 892 726 297, - 359 462 897 324 084 867 541 299 849 782},
{11 258 384 864 155 405 013 538 270 838 177, 594 262 829 082 085 112 713 318 169 240},
{2 380 448 853 507 485 345 078 529 548 959, 119 070 608 226 765 543 636 793 074 402},
{70 321 705 031 263 518 985 231 552 913, - 4 052 240 595 450 744 009 135 859 807},
{104 653 888 327 863 570 584 301 342 162, - 4 789 737 021 927 534 192 764 718 529},
{52 583 809 281 579 260 926 139 979 748, - 5 469 991 588 585 560 593 751 027 051},
{154 475 782 112 173 185 830 031 225 626, - 30 260 254 701 352 113 964 344 049 963},
{231 739 128 195 120 968 606 701 234 203, 459 396 168 476 422 387 323 517 157},
{14 852 527 659 298 233 882 346 856 475, - 1 865 994 943 932 024 568 237 398 589},
{5 506 528 127 531 274 439 320 253 301, 591 088 807 020 924 414 236 734 871},
{13 631 207 097 035 693 916 843 680 726, - 171 613 615 038 010 756 714 709 601},
{5 382 400 159 397 621 955 858 424 031, 301 488 673 940 094 490 228 470 105},
{3 240 905 921 257 757 382 544 763 707, - 121 459 236 256 015 737 437 653 178},
{2 810 022 408 790 729 563 846 663 227, - 63 957 929 193 717 726 125 644 974},
{301 232 728 498 078 154 765 240 917, 1 884 777 287 607 801 151 706 703},
{24 209 538 899 412 154 071 704 099, - 2 943 909 212 337 503 894 974 741},
{48 053 359 651 984 972 569 150 483, - 4 918 773 473 470 575 435 087 544},
{82 809 381 038 617 070 065 921 861, - 2 795 187 824 577 381 608 870 571},
{76 376 520 005 419 608 614 254 637, - 8 340 789 642 839 917 192 087 924},
{95 587 165 049 805 833 638 822 433, - 1 309 909 912 109 752 167 437 508},
{36 258 534 206 074 584 115 651, - 860 934 052 313 962 441 985},
{7 249 192 648 835 793 316 513, 507 771 851 727 812 090 373},
{10 248 230 899 188 955 744 243, 426 410 043 413 605 210 278},
{1 050 459 580 157 440 922 683, - 170 006 376 593 586 866 631},
{2 220 756 403 502 139 771 481, - 59 409 329 388 433 767 881},
{1 650 618 777 496 596 271 532, 253 195 829 052 678 001 139},
{8 887 897 888 666 930 760 193, - 829 251 769 383 782 299 202},
{17 072 624 942 491 240 765 117, - 505 101 793 753 944 756 823},
{7 361 031 295 430 310 581 145, - 1 142 758 074 828 157 260 026},
{36 827 247 791 679 792 532 197, 4 358 675 821 822 381 670 188},
{142 922 408 848 353 959 460 589, - 22 481 036 782 494 753 776 858},
{586 641 735 197 136 886 359 193, - 9 769 489 984 873 355 424 111},
{34 480 535 645 695 946 614 909, - 889 922 954 529 089 860 339},
{16 531 549 408 514 729 496 776, - 708 902 791 558 242 305 733},
{16 555 319 795 286 421 938 941, 864 263 236 884 611 542 235},
{9 805 235 496 952 592 462 748, 767 527 654 412 219 258 291},
{12 601 552 759 656 826 337 555, - 962 459 452 495 737 339 078},
{6 539 331 036 493 587 856 493, - 118 496 175 004 177 922 091},
{1 609 023 022 257 556 328 624, 298 592 197 798 681 131 485},
{8 472 528 428 282 998 997 527, 1 602 436 651 341 505 809 779},
{33 605 197 525 009 306 250 136, - 3 172 214 233 267 732 479 085},
{94 108 609 988 309 824 445 327, 7 257 965 905 723 793 528 179},
{17 881 115 385 262 873 733 000, 2 927 748 648 556 913 117 933},

```



```

{22 967 515 056 261 836 854 346, 3 871 780 899 084 175 665 975},
{19 211 434 691 754 851 329 792, -258 232 698 172 830 782 383},
{7 461 696 968 472 260 641 850, -1 065 572 274 641 669 693 659},
{196 446 356 581 813 395 301, 19 436 387 459 080 833 274},
{152 021 185 343 369 566 953, 29 840 796 512 524 100 815},
{205 655 802 994 681 590 094, -27 491 631 912 256 873 979},
{964 649 711 448 493 473 593, -90 804 086 306 648 325 522},
{2 496 252 368 498 581 821 877, -312 934 998 316 207 988 141},
{527 616 116 268 992 077 323, -2 245 719 167 282 022 118},
{9 335 827 086 667 789 711, 752 357 258 325 975 282},
{22 450 419 033 194 301 871, 1 410 122 162 237 174 688},
{8 142 096 069 835 999 001, 566 084 249 943 878 912},
{15 834 909 655 383 679 009, -2 709 913 590 300 768 723},
{30 993 747 708 728 133 017, 822 336 792 643 052 123},
{18 618 680 054 672 878 961, -858 890 346 722 148 555},
{20 214 252 844 650 415 177, -1 543 561 675 021 461 253},
{10 800 428 064 113 578 824, -1 124 895 970 516 829 917},
{32 742 809 796 994 585 258, 4 072 900 304 207 243 737},
{11 651 337 523 574 381 426, 1 090 455 854 333 560 929},
{25 088 411 808 919 581 889, 129 757 423 641 052 159},
{3 301 720 372 345 609 746, 290 795 547 904 221 601},
{7 516 762 214 139 565 855, 325 297 880 976 233 468},
{2 548 499 473 092 314 643, 461 140 536 572 250 467},
{15 939 093 482 906 735 607, -2 003 415 950 302 001 036},
{6 441 090 724 176 905 713, 398 364 823 218 333 935},
{4 909 509 345 900 080 969, -174 663 322 411 420 300},
{1 382 351 241 762 817 537, -119 898 176 365 198 377},
{4 119 161 847 228 098 051, 570 670 054 822 848 406},
{9 086 416 833 175 622 257, -1 657 155 284 851 471 094},
{58 446 749 851 033 475 451, -4 879 476 501 008 705 747},
{7 808 675 758 182 526 449, -537 032 598 127 846 324},
{18 017 364 602 667 294 003, 3 415 463 671 733 362 057},
{68 623 375 812 035 311 414, 3 976 778 352 409 179 763},
{74 324 498 938 785 647 339, -4 956 888 387 113 955 771},
{2 104 361 358 429 313 498, -126 128 258 446 839 599},
{2 906 789 567 188 057 005, -30 653 292 115 356 193},
{384 942 415 267 037 090, -56 144 615 868 876 461},
{589 102 394 502 164 001, -113 928 657 053 245 861},
{1 420 514 974 223 232 808, 147 920 552 744 644 907},
{4 284 410 385 294 787 126, -586 044 089 519 448 623},
{13 293 428 382 081 213 845, -533 610 526 113 699 999},
{3 418 938 265 573 887 490, -434 473 803 941 535 403},
{4 150 208 114 962 888 582, 391 044 244 656 034 985},
{11 043 336 066 505 226 469, 2 163 321 119 569 185 454},
{16 551 324 212 128 841 527, 118 035 541 678 295 638},
{1 923 431 533 224 011 111, 211 462 226 098 327 541},
{1 479 819 378 751 616 666, 152 032 757 524 226 025},
{2 957 098 343 816 981 632, -525 752 015 210 524 401},
{14 411 203 563 570 028 502, -1 695 093 621 203 167 849},
{61 658 648 989 869 196 147, 1 269 175 395 351 342 822},
{38 759 012 911 301 955 563, -265 307 332 339 255 212},

```

```

{24 142 389 770 694 611, 3 235 414 151 210 872}, {109 097 821 991 951 011, 19 484 079 766 710 141},
{569 885 932 406 617 955, -63 979 573 123 929 003},
{432 906 476 738 244 256, 27 142 108 100 991 843}, {99 809 460 066 641 936, 1 142 781 184 181 861},
{28 287 284 125 862 117, 4 761 126 752 809 966}, {20 401 776 542 830 567, 944 806 618 978 195},
{28 029 742 452 349 779, -2 160 264 189 396 433}, {3 919 516 715 681 050, 435 389 110 462 959},
{74 074 670 552 587, 2 327 232 192 927}, {28 963 452 338 621, 2 702 485 084 824},
{55 763 502 394 339, 2 092 206 957 471}, {53 004 238 388 594, -5 335 760 047 649},
{25 795 432 416 408, 105 462 616 985}, {3 132 338 378 941, -232 649 424 347},
{7 876 397 957 390, -1 338 507 924 981}, {11 289 420 252 208, -955 361 488 835},
{12 768 985 808 276, -1 275 162 522 717}, {1 267 322 420 738, 52 653 475 349},
{265 647 902 426, 44 574 794 549}, {131 463 135 364, -16 004 969 413},
{249 906 744 380, 22 973 493 731}, {204 523 126 253, 29 162 134 186},
{28 337 647 423, 1 183 117 147}, {4 172 979 665, -164 081 391}, {5 178 976 970, 366 469 317},
{3 533 676 836, 80 261 009}, {160 048 120, 9 623 737}, {259 544 857, 19 215 226},
{691 186 411, -29 806 983}, {410 683 546, -54 982 405}, {1 883 889 903, -271 742 470},
{1 336 439 251, 193 374 059}, {1 254 078 826, -166 826 763}, {5 879 075 294, 500 738 389},
{9 474 332 302, 1 083 856 063}, {20 467 175 345, 2 186 464 251}, {57 596 787 278, -554 518 135},
{5 336 209 626, 202 405 993}, {5 376 727 984, -176 085 535}, {5 980 422 873, 975 321 910},
{9 379 873 149, 399 730 867}, {13 582 614 184, 2 201 188 131}, {27 410 434 054, -2 649 414 567},
{66 889 052 032, -7 400 721 439}, {20 626 812 913, 565 415 987}, {19 844 128 813, 1 858 946 806},
{44 112 881 869, 4 491 247 458}, {58 370 267 903, -3 226 423 768},
{21 508 725 767, 3 718 809 084}, {58 701 397 801, 8 363 737 344},
{11 332 256 689, -1 699 507 880}, {41 193 788 383, -6 853 170 032}, {5 458 077 943, 590 699 173},
{10 350 333 178, 2 003 277 689}, {24 377 965 509, 973 312 442}, {3 296 275 507, 339 925 472},
{7 517 482 549, -923 382 040}, {9 521 114 717, 675 602 618}, {4 575 498 745, 242 066 219},
{1 734 437 368, 243 765 677}, {2 049 666 917, -118 632 881}, {2 402 279 620, -71 227 973},
{1 421 416 726, 117 590 447}, {754 189 426, -104 572 811}, {1 619 121 677, 84 737 449},
{665 040 658, 109 366 395}, {645 487 024, 34 529 923}, {772 450 449, -65 773 363},
{1 228 583 211, -79 217 531}, {2 839 501 805, 142 773 438}, {1 165 587 715, 227 498 011},
{2 051 129 180, 310 712 003}, {9 041 403 393, -1 131 233 885}, {618 141 151, 70 931 477},
{1 477 676 366, 105 201 241}, {354 706 416, -70 401 647}, {196 967 213, 24 998 203},
{220 344 003, 13 343 480}, {474 146 461, -32 276 275}, {729 829 472, 36 710 027},
{319 087 964, -17 851 559}, {163 527 154, 3 906 967}, {41 278 580, -6 436 811},
{194 013 122, -7 444 967}, {32 410 540, -2 714 951}, {12 327 656, 2 299 903},
{60 454 293, -219 704}, {2 605 589, -511 937}, {3 350 992, -97 353},
{2 992 270, 25 491}, {717 079, -133 226}, {3 719 277, 617 149}, {1 195 959, -83 288},
{2 184 671, -4843}, {34 894, 6873}, {38 617, -4524}, {153 227, 25 897},
{157 315, -15 631}, {73 365, -4408}, {114 683, 2871}, {11 461, -145}, {438, 29}}

29
— is a relation number with a list {{74, 87}, {962, -29}, {370, 29}, {518, 87},
74
{148, 29}, {222, -29}, {185, 29}, {814, -87}, {2294, -145}, {962, 87}, {185, 29}}

29
— is a relation number with a list {{75, 87}, {300, 29}, {150, 29}, {1, 0}}
75

29
— is a relation number with a list
76
{{76, 87}, {836, 87}, {1292, 145}, {988, -87}, {2356, -319}, {9348, 725},
{5852, 725}, {494, -87}, {532, 29}, {190, -29}, {494, -29}, {1, 0}}

```

```

29
77  is a relation number with a list
    {{77, 87}, {770, -29}, {1001, -29}, {154, 29}, {693, -116}, {231, -29}, {1, 0}}

29
78  is a relation number with a list {{78, 87}, {1, 0}}

29
79  is a relation number with a list
    {{79, 87}, {632, 87}, {1817, 203}, {790, -87}, {553, 29}, {158, 29}, {1027, 29},
    {948, -145}, {5293, -203}, {1185, 58}, {1975, 232}, {8927, 1334}, {32469, 1885},
    {33496, 1363}, {45741, -6931}, {219304, -15979}, {347758, -14239}, {475738, -77053},
    {1060180, 139693}, {4531756, 609145}, {21151539, 1535521}, {27314645, -983419},
    {17465873, 751825}, {13737942, -1122329}, {21329526, -2535905},
    {82340594, 11247563}, {285004587, 51581981}, {1934496621, 185813527},
    {6032546729, -822085620}, {21957843731, -460969732}, {13327568995, 2169817613},
    {24384402043, 1342103760}, {17896214677, 914252608}, {30718161157, -4568233990},
    {99498665067, -4357778960}, {57689830027, 5428067808},
    {159494353019, -18977437049}, {606313673533, 58778368410},
    {1463869165207, -192836137623}, {6226774926383, -766392090514},
    {7555417979409, 472197898292}, {19876932223, 3438418292},
    {59532624791, -9390064976}, {252186559865, -1216628184},
    {27217536383, 3798848794}, {49421991175, -8309193999},
    {34220652701, 3201714869}, {78858657782, 7597559287},
    {227762128048, 14945006537}, {283375369447, 36392948656},
    {613689364279, 53575921153}, {1923984296084, -5138526617},
    {171851964754, -27434212019}, {572488718560, -65761883901},
    {1530090687371, 140079088890}, {851563943101, -125268247025},
    {1999789099846, 352894165077}, {9288495358664, -601032418171},
    {21567717801821, 22019945717}, {805084645362, -33648697129},
    {196242772986, -7176919391}, {194810004891, 5123635639},
    {8836198111, -691242144}, {11846031119, -1922930521}, {24367391447, 153349390},
    {1197763477, 196587346}, {1440912679, 191064093}, {6920405135, 148347963},
    {4103980954, 332708155}, {8807164426, 419866437}, {792429329, -7785717},
    {135390595, 18667503}, {372727846, -30332869}, {689940022, -116874553},
    {893276384, 51565335}, {1316589431, 207221617}, {5787518591, -625749385},
    {12306155954, 257744779}, {5181881602, 562469181}, {9453058867, -676367522},
    {1270828839, -215246497}, {1631361297, 236557147}, {1938559828, -185810685},
    {6355785262, -680225943}, {18466390225, 492562303}, {19085216106, -3123370499},
    {27254455848, 3373736779}, {20900367664, -2004834699},
    {67309633246, -10130343945}, {284619175151, -35546481953},
    {19538242633, 3356308649}, {47369131619, -4318354736},
    {10488867683, -1530576993}, {17788530172, -3153786221},
    {89600785166, -13982308269}, {450847908608, 53905563805},
    {1548668455272, 279049712491}, {9924755754246, -185338663513},
    {6599033961024, 107173288183}, {3611082599438, -513166066429},
    {1494690620365, 62489249619}, {399058268789, 44000584225},
    {241187850356, 23090979691}, {811966222234, 35806095985},
    {914344848259, -143516965143}, {4206201534679, -529499593894},
    {2353822101367, 355526587210}, {10654256719137, -709206541681},
    {1276528919838, 204590055761}, {3870098236488, 535255703351},
    {9741356729449, -626092370059}, {21813574128105, 1416209914531},

```

```

{45 063 607 401 060, -3 915 775 010 471}, {152 129 725 242 768, -25 724 308 251 799},
{175 073 817 174 054, -24 342 968 836 007}, {369 169 790 438 395, -25 842 197 310 523},
{582 943 219 194 767, 98 384 558 879 853}, {581 766 592 663 729, -84 224 167 445 943},
{616 403 777 171 888, 91 739 904 159 145}, {2 036 268 603 428 033, 227 457 634 644 375},
{857 158 561 336 018, -33 923 999 077 299}, {715 628 167 879 897, -53 006 450 079 151},
{2 090 508 525 029 143, 350 500 238 161 464}, {986 939 411 231 639, -155 158 531 786 892},
{4 423 069 420 312 673, 731 743 147 222 116}, {2 576 232 421 418 183, 119 668 712 967 851},
{4 461 861 846 088 581, 373 563 589 709 557}, {1 651 197 203 662 137, 189 124 848 437 360},
{4 023 188 149 654 137, -172 197 667 061 570}, {4 948 702 771 804 133, -887 328 828 544 549},
{29 646 345 757 589 719, 4 801 962 748 429 357}, {65 930 972 094 072 583, -7 885 082 768 380 525},
{225 174 485 815 242 257, 38 350 369 008 523 381},
{389 290 530 635 944 291, -28 692 656 011 447 438}, {980 125 628 421 267 439,
107 962 111 672 695 268}, {668 863 245 993 792 133, -64 615 895 372 251 233},
{1 793 639 089 431 104 437, 162 740 072 529 066 889}, {276 365 037 298 123 982,
-27 742 274 874 483 183}, {83 559 204 289 919 992, 13 811 846 312 712 425},
{54 361 986 677 989 918, -6 425 771 060 198 415}, {233 509 637 515 805 242,
6 676 452 418 377 267}, {13 129 573 064 529 137, -2 090 621 343 239 510},
{46 281 755 402 274 083, 4 735 965 360 781 040}, {85 153 958 237 369 043, 967 312 024 936 156},
{2 409 503 395 997 885, 350 542 759 592 714}, {3 499 377 770 937 927, 567 919 686 585 688},
{7 256 912 462 480 121, -421 152 911 663 555}, {7 687 724 171 775 194, 593 831 520 069 883},
{2 534 761 541 529 515, -388 585 842 257 507}, {14 641 808 987 569 686, -1 550 766 105 164 863},
{54 108 209 245 787 601, -3 335 479 159 074 271},
{58 502 873 347 341 935, -5 793 993 758 323 189}, {44 471 925 364 693 555, -621 666 450 175 391},
{22 756 664 786 833 163, -1 010 624 776 763 989}, {38 528 701 220 348 136,
-5 021 326 336 158 485}, {129 710 848 044 659 776, 15 761 783 767 139 707},
{285 709 654 695 827 480, -13 388 194 220 620 907}, {360 048 508 960 286 207,
-309 696 862 135 197}, {10 186 394 532 884 416, -1 709 113 589 743 949},
{5 394 673 440 762 962, 357 998 587 435 755}, {1 950 875 708 904 323, 352 262 752 098 198},
{12 853 363 491 104 335, 481 182 425 408 868}, {10 946 397 599 872 979, -1 848 730 929 239 211},
{11 533 050 069 420 673, 2 105 599 505 482 687}, {79 399 150 818 571 802, -8 536 781 376 127 139},
{202 881 356 240 776 529, -4 126 817 589 453 170},
{52 716 254 248 124 721, 2 957 528 715 800 677}, {41 021 748 266 709 735, 7 293 094 689 130 277},
{216 208 769 577 682 233, -20 580 047 222 690 702},
{803 568 239 881 323 631, -144 060 747 120 729 628},
{4 802 903 184 601 276 823, 802 252 767 846 220 774},
{838 460 375 607 777 859, 26 617 212 058 241 508},
{1 049 942 410 220 081 363, -175 650 265 488 271 567},
{312 775 434 054 295 081, -16 401 154 230 615 058},
{91 126 790 136 109 341, 8 921 469 502 165 667}, {151 055 514 041 761 009,
-16 063 767 477 569 274}, {512 046 932 747 365 897, 46 728 538 230 448 583},
{155 392 035 217 912 764, 16 217 459 361 214 603}, {535 822 113 144 428 014,
95 680 064 493 399 361}, {3 022 403 631 461 484 008, 207 704 489 662 985 337},
{7 359 933 365 180 387 713, -198 168 537 282 329 445}, {2 188 101 373 001 661 592,
-393 999 805 760 791 507}, {13 895 899 463 483 908 550, 519 826 343 125 312 753},
{11 013 532 271 063 326 699, -636 858 846 034 330 997}, {14 767 619 189 896 280 250,
-1 522 625 943 510 514 013}, {36 232 579 371 499 930 520, 582 345 537 818 178 347},
{10 045 326 115 056 967 474, 1 755 000 170 676 283 325}, {38 289 317 811 057 865 604,
1 910 710 126 786 035 365}, {5 934 106 751 635 506 016, 640 434 066 443 027 531},
{13 445 812 138 212 400 723, 1 236 246 691 004 286 219}, {12 079 215 563 945 067 194,
-112 355 300 769 587 633}, {4 357 396 614 461 376 430, -721 235 174 851 684 573},
{2 368 859 662 750 250 368, 414 793 269 045 769 421}, {9 472 096 170 424 926 482,

```

```

-1 474 780 906 756 217 021}, {49 249 447 661 122 324 124, -8 034 224 633 294 506 715},
{82 483 889 047 067 422 886, 1 153 069 535 101 824 421}, {42 432 280 940 850 898 654,
2 365 948 292 880 634 865}, {12 228 278 149 041 784 364, 1 622 272 021 074 065 353},
{59 241 943 544 508 338 340, 2 322 765 736 977 329 153}, {90 847 283 735 275 351 402,
16 595 524 119 777 213 925}, {621 703 387 774 753 260 383, -58 274 980 269 335 129 123},
{1 526 390 219 846 719 637 630, 121 159 757 676 982 087 677},
{3 846 243 766 369 752 671 509, 311 765 024 190 058 014 230},
{8 300 014 611 035 463 559 171, 254 710 458 353 474 950 402},
{8 329 010 655 707 574 523 505, 1 280 268 259 805 069 149 527},
{49 996 505 871 304 852 331 536, 8 977 693 824 855 794 221 383},
{305 702 909 148 563 126 744 198, -35 917 480 621 202 882 052 669},
{1 386 798 898 938 762 126 656 017, -216 987 491 878 701 558 828 351},
{6 705 041 865 657 669 121 186 969, 87 399 517 892 789 910 800 204},
{1 952 959 954 885 166 823 870 381, 264 531 591 744 260 071 118 194},
{7 997 866 201 352 359 757 398 817, 346 516 774 701 241 431 603 657},
{2 210 450 274 680 739 610 661 774, -213 832 657 275 461 790 811 213},
{5 697 772 452 163 614 501 421 876, -160 081 077 901 246 482 568 419},
{5 146 561 830 219 450 812 255 432, -578 304 358 897 078 698 460 123},
{4 596 014 588 486 340 436 968 325, 133 140 266 985 615 125 866 192},
{5 047 685 724 804 928 499 523 205, 599 606 453 909 285 549 191 562},
{19 815 893 388 920 884 373 266 011, -3 550 411 127 887 195 129 980 529},
{117 439 296 893 780 626 122 755 877, -21 291 916 712 575 725 274 822 298},
{814 664 067 152 224 316 568 054 969, -112 261 968 117 745 944 843 994 972},
{2 277 592 935 912 213 510 147 123 035, 328 167 133 330 932 505 893 159 847},
{1 546 582 794 940 808 457 294 675 626, 190 511 004 211 249 528 504 894 683},
{1 777 086 138 814 166 111 185 934 798, 46 363 578 396 955 838 456 065 903},
{1 206 342 618 657 695 738 579 008 236, 120 045 636 035 645 271 569 334 049},
{465 014 405 798 198 807 967 751 934, -75 678 234 402 692 712 347 029 633},
{864 654 951 181 360 176 960 356 744, 52 114 141 692 711 895 536 007 929},
{1 681 551 149 984 621 724 990 465 871, 203 930 698 008 395 824 466 317 556},
{3 958 339 707 478 955 211 534 108 417, 126 849 614 995 083 898 922 876 987},
{2 054 129 767 876 993 249 068 823 780, 218 500 312 591 039 978 211 755 833},
{6 922 529 410 053 042 167 878 681 357, -526 747 080 507 431 089 364 609 642},
{5 910 571 713 058 602 484 961 724 869, -388 652 095 589 714 677 349 599 657},
{6 382 432 057 817 703 652 700 671 106, -245 580 288 330 823 092 034 157 625},
{209 779 663 912 042 474 806 744 376, -5 103 853 120 753 019 019 115 977},
{41 213 190 932 326 906 816 156 201, 5 275 711 055 599 700 490 474 594},
{78 407 303 485 185 071 503 603 529, -13 827 183 329 273 313 045 429 220},
{359 907 922 745 929 734 748 771 489, 35 402 697 227 076 560 187 452 868},
{464 595 087 537 966 497 065 181 911, 68 052 060 462 890 601 160 113 196},
{929 777 520 479 149 173 393 226 419, 84 858 989 283 860 438 154 311 420},
{290 037 569 821 936 058 031 736 879, 3 717 568 912 711 183 581 338 047},
{5 308 375 806 635 356 302 167 827, -557 342 696 528 209 064 078 014},
{20 939 041 533 092 012 750 372 727, -2 088 828 578 803 258 856 379 356},
{4 009 703 859 694 510 739 754 193, -162 797 772 447 691 644 834 708},
{4 758 995 668 324 650 107 967 053, 632 212 369 318 222 575 900 011},
{23 597 559 611 469 309 439 409 765, 2 029 594 626 337 123 370 447 221},
{59 848 496 461 517 509 470 594 073, -6 550 066 851 670 032 056 082 398},
{70 933 688 922 490 456 302 346 789, 3 323 700 680 655 627 763 935 338},
{89 741 995 669 059 587 516 670 589, -973 760 091 772 802 900 596 610},
{12 329 310 850 975 932 280 815 051, 14 095 149 076 857 111 625 027},

```

```

{311 622 710 649 190 895 602 346, 30 414 692 400 001 595 859 327},
{590 587 145 284 820 023 717 004, 17 984 758 513 321 166 991 589},
{229 880 966 727 500 473 429 207, 13 777 705 253 421 901 342 938},
{342 861 783 873 076 102 658 381, 44 307 178 535 022 487 500 777},
{916 055 908 161 199 990 478 965, -137 530 226 206 675 281 689 233},
{3 685 798 347 556 631 526 307 614, 40 771 204 085 087 581 254 895},
{1 294 808 412 001 187 855 998 056, -106 240 796 724 171 394 377 287},
{1 573 589 253 579 358 754 178 348, 271 677 379 132 498 553 910 547},
{4 461 526 676 034 972 973 509 786, -171 429 953 173 907 138 513 095},
{343 483 587 557 602 401 375 964, -51 452 728 697 648 101 146 957},
{1 318 155 552 748 810 225 566 065, 193 726 475 497 440 847 175 083},
{2 996 452 282 928 780 668 101 764, 95 097 383 412 109 164 931 939},
{3 686 454 914 438 296 167 902 436, 606 840 319 459 370 061 706 235},
{3 587 626 816 883 988 015 537 054, 529 215 657 203 102 112 505 421},
{9 233 739 899 480 414 988 070 547, -1 132 828 247 916 150 231 617 495},
{13 517 999 375 945 837 675 316 373, -171 967 354 442 611 759 615 691},
{67 421 625 020 491 334 323 216, -1 280 618 711 309 010 860 421},
{35 642 167 632 013 061 048 663, -3 501 791 308 196 118 777 245},
{49 316 109 454 097 988 820 827, -5 090 784 074 928 508 249 700},
{125 746 772 319 780 400 417 667, -13 269 926 124 479 297 754 853},
{499 077 538 757 870 929 295 210, 50 909 908 873 344 865 940 873},
{791 702 448 070 640 678 968 080, 46 866 489 090 314 016 760 153},
{397 201 450 711 110 870 407 159, -57 249 451 229 043 007 024 362},
{280 031 923 483 024 122 306 625, -340 623 340 270 547 141 902},
{3 123 484 670 115 361 391 299, -537 544 198 247 324 868 531},
{8 040 661 030 118 437 771 073, 1 143 100 797 892 009 739 827},
{3 077 480 145 075 197 790 436, -71 669 075 068 684 652 547},
{338 916 547 381 139 257 715, -61 113 629 149 099 408 177},
{2 193 452 973 563 118 116 413, -3 172 884 562 698 048 395},
{78 189 518 362 567 361 972, 7 664 452 364 956 473 943},
{122 054 582 327 207 180 818, -21 776 116 647 503 310 555},
{679 567 287 067 201 918 448, -25 916 649 083 213 016 091},
{453 018 461 389 416 506 478, -51 840 283 098 930 242 653},
{1 069 982 833 575 498 514 521, 167 597 279 538 342 723 877},
{5 087 533 351 289 931 529 461, 167 156 345 404 314 420 706},
{5 754 596 143 679 413 754 199, 530 671 173 014 029 194 880},
{6 540 153 998 517 683 768 999, -1 109 150 246 978 963 381 387},
{9 065 051 185 131 625 026 517, 1 103 267 060 841 331 560 031},
{18 874 261 173 676 831 155 251, -2 912 743 490 701 456 700 964},
{110 426 218 127 979 185 007 893, 13 110 504 162 032 745 831 102},
{437 832 601 705 660 250 367 083, 71 389 668 081 790 926 177 660},
{750 072 863 978 260 770 788 717, 132 919 713 810 961 053 383 800},
{3 748 188 092 112 938 411 612 557, 506 679 790 835 364 269 947 056},
{15 912 934 944 965 693 236 670 035, -862 496 445 880 092 636 765 071},
{30 651 914 610 798 036 217 001 803, -625 407 296 946 833 472 056 891},
{549 607 771 852 490 810 917 376, 22 737 705 908 348 258 998 731},
{308 323 574 118 475 000 878 728, -14 634 377 430 011 594 894 299},
{79 130 198 970 289 139 777 471, 5 795 965 377 633 397 551 219},
{159 051 989 009 695 649 228 005, 9 208 120 613 156 411 439 739},
{198 601 148 296 895 725 442 918, -1 600 661 511 273 374 468 799},
{9 410 551 020 786 013 635 518, 1 364 465 233 496 994 571 345},

```

```

{11 115 743 481 742 920 747 863, -1 700 720 721 779 504 757 917},
{62 354 824 086 375 392 046 924, -2 981 536 283 587 709 139 301},
{20 337 591 648 353 490 393 363, -3 360 975 997 482 865 147 637},
{13 567 117 413 047 661 095 739, -1 559 389 068 814 003 572 806},
{36 923 352 295 991 313 701 685, 1 204 458 597 651 435 718 259},
{32 774 274 265 052 291 583 176, 1 096 272 424 677 485 185 347},
{8 997 979 546 508 854 201 486, -726 071 194 234 290 807 977},
{22 524 892 040 091 795 955 198, 520 794 442 056 020 839 503},
{10 327 751 502 949 088 668 951, -560 438 184 419 407 924 774},
{18 949 270 488 579 935 818 501, -2 538 248 657 577 418 051 840},
{93 340 860 957 502 746 994 059, 5 064 556 134 997 619 182 694},
{172 129 191 676 102 534 739 793, 20 979 942 871 877 218 664 168},
{338 882 247 385 698 048 689 471, 40 217 926 569 336 168 697 999},
{1 353 967 951 649 687 229 332 841, 195 058 938 382 043 682 788 575},
{904 124 744 944 865 464 787 536, -142 537 021 340 304 990 593 969},
{3 863 306 735 339 806 176 674 038, 84 982 435 620 146 666 979 953},
{3 088 673 462 223 286 843 516 087, -89 288 629 386 285 596 834 335},
{2 877 856 737 440 014 609 165 402, -341 197 236 715 374 124 272 049},
{11 714 028 653 644 707 584 131 790, -1 154 062 893 752 794 809 404 131},
{13 698 577 573 223 999 717 147 920, -656 316 793 522 336 115 695 789},
{6 641 932 168 859 638 284 628 271, 647 296 424 523 797 249 605 090},
{13 348 465 966 111 597 297 612 309, 2 135 719 687 096 904 031 364 520},
{42 197 679 638 883 675 644 589 931, -1 671 306 805 469 803 428 838 211},
{32 785 750 668 948 603 967 137 824, 354 793 550 095 714 761 236 595},
{11 434 780 751 284 828 736 315 636, -1 354 353 751 436 258 336 639 047},
{47 396 108 443 786 201 413 057 540, -2 602 517 639 175 813 077 117 473},
{43 512 484 151 103 715 970 499 054, 2 049 290 365 441 158 311 240 435},
{37 713 531 670 311 923 321 543 601, -4 236 555 070 256 712 600 577 447},
{32 821 652 997 880 716 608 620 338, -2 668 886 592 493 652 480 960 351},
{62 806 097 148 594 060 130 593 954, -3 343 416 050 251 081 513 778 843},
{56 785 816 687 942 601 865 120 977, -6 860 674 958 700 774 375 403 154},
{150 132 944 448 576 142 089 763 855, 9 127 613 580 196 814 292 916 884},
{323 199 046 068 741 958 844 403 169, 9 225 346 051 230 597 002 128 122},
{24 642 807 778 014 037 823 593 021, -3 931 275 504 111 632 371 372 113},
{83 357 225 514 195 244 033 467 097, -4 575 886 354 988 314 683 897 457},
{78 310 418 828 040 798 141 716 809, 12 214 191 856 826 695 661 053 264},
{396 996 147 279 369 309 856 380 775, -55 208 183 788 057 750 382 428 819},
{832 570 000 274 239 517 170 944 318, -82 669 049 492 749 065 383 985 649},
{464 480 922 393 160 203 155 938 412, -51 640 017 809 928 774 476 079 815},
{22 059 793 799 702 603 173 613 917, -1 779 683 856 807 170 637 049 183},
{55 583 413 923 307 886 792 873 959, 2 233 241 469 594 292 064 929 906},
{19 562 202 507 403 771 599 521 589, 3 100 465 900 376 678 891 463 401},
{75 793 161 306 352 161 808 553 457, -5 468 448 312 747 611 017 840 084},
{60 444 090 697 037 002 855 409 801, 10 429 011 972 031 035 303 913 467},
{168 268 509 676 787 508 477 609 079, -20 889 057 839 200 008 046 396 516},
{91 327 710 091 808 084 408 519 129, -7 492 834 607 442 560 418 417 393},
{111 681 889 397 291 391 613 322 627, -17 973 844 174 034 361 725 746 369},
{303 267 123 893 732 479 448 708 627, 27 303 091 364 413 838 250 380 550},
{231 716 391 929 240 436 867 283 583, 30 433 026 033 005 668 251 195 125},
{928 077 490 449 587 822 239 915 943, -19 402 340 642 051 235 962 099 224},
{255 553 969 140 848 811 326 897 911, 31 809 699 565 669 812 452 919 320},

```

```

{85 033 436 623 734 624 579 924 729, -15 433 008 098 827 007 842 705 219},
{597 604 345 568 966 375 628 220 215, -97 034 842 838 237 891 303 633 489},
{1 216 227 794 623 583 196 707 123 199, -75 875 334 228 052 704 422 340 098},
{175 573 311 004 454 150 024 848 849, -211 913 142 583 363 073 508 935},
{8 112 051 575 153 195 210 603 014, -1 125 912 040 682 114 238 932 419},
{18 222 715 939 893 247 508 010 399, -1 985 482 741 231 907 020 978 564},
{27 916 330 235 680 661 217 062 517, -3 136 634 626 673 975 803 861 051},
{24 757 130 946 424 560 397 268 418, 2 416 495 873 694 331 656 147 443},
{46 781 604 549 018 263 027 725 052, 2 000 239 197 335 417 217 365 825},
{61 312 137 813 989 695 236 575 083, 469 985 497 853 553 424 751 544},
{16 907 824 349 192 251 491 074 677, -111 163 856 397 782 728 767 186},
{862 535 961 612 860 758 529 995, 83 614 848 747 859 818 865 166},
{2 084 610 456 606 743 020 388 465, -281 557 697 961 605 047 897 321},
{8 982 819 099 165 107 123 470 222, 839 375 748 761 261 292 876 895},
{19 774 816 839 492 600 755 874 217, -978 694 340 651 429 513 437 102},
{15 873 472 090 656 828 483 441 983, -1 566 232 934 530 977 912 700 329},
{16 680 276 882 416 899 158 656 747, -1 269 609 526 658 628 368 884 051},
{13 852 889 832 523 698 689 962 636, 1 405 608 189 711 969 493 328 691},
{16 052 173 103 083 703 222 617 646, 915 780 605 148 340 098 708 385},
{34 118 345 377 327 065 776 529 436, 2 800 067 581 317 960 621 229 001},
{40 885 217 719 411 527 420 732 496, -3 922 125 733 400 280 897 828 361},
{131 452 870 447 288 756 953 461 994, -20 318 825 877 505 181 942 334 355},
{753 653 299 398 355 558 657 013 256, 54 757 997 389 924 388 660 906 291},
{1 023 734 460 786 284 725 058 310 622, 183 733 299 279 860 439 083 239 675},
{6 214 561 456 537 354 845 849 066 812, -827 162 371 748 218 444 819 761 853},
{31 816 263 878 423 024 304 013 212 948, -4 730 500 667 911 074 870 609 687 701},
{102 482 022 959 405 483 430 113 475 761, -2 490 278 351 830 024 395 668 949 731},
{30 068 232 215 584 173 407 236 406 410, 1 946 709 148 908 307 154 525 175 631},
{68 540 003 574 805 721 059 342 983 655, 2 828 495 902 791 765 659 062 556 419},
{51 832 050 716 464 274 105 488 738 321, -4 872 287 595 014 657 094 945 143 351},
{139 285 913 467 059 361 173 719 244 660, -24 131 456 251 535 403 325 952 216 551},
{434 723 099 330 091 643 777 530 317 034, -8 597 722 797 967 593 383 705 909 279},
{297 100 305 934 193 884 526 213 439 405, 24 847 275 310 962 207 596 803 055 111},
{84 292 825 990 855 924 198 434 532 233, -13 529 773 802 802 077 229 214 893 140},
{246 020 470 749 433 405 028 468 698 047, 14 883 614 145 760 265 346 543 782 704},
{553 076 608 550 797 363 159 273 025 759, 42 363 215 242 391 457 745 996 944 638},
{186 030 021 576 964 584 443 706 891 735, 508 426 163 271 054 408 347 320 637},
{4 262 380 239 064 991 901 584 451 153, 515 785 003 548 776 345 557 570 555},
{10 751 916 643 307 709 832 787 050 327, 1 277 954 184 666 801 533 120 927 075},
{41 734 370 111 890 507 857 751 064 433, -6 283 102 103 902 085 150 832 407 656},
{177 540 224 618 502 967 647 987 343 561, -25 018 884 570 123 735 037 822 880 064},
{190 234 577 583 308 968 274 947 465 927, -21 169 387 398 675 292 807 534 837 300},
{22 902 811 376 724 692 436 419 512 067, -683 262 024 629 084 034 836 513 283},
{25 919 699 392 469 015 093 733 224 845, -3 111 258 209 867 027 403 732 933 213},
{81 341 063 369 090 873 245 710 972 139, -6 914 377 039 886 524 477 117 603 115},
{128 885 427 654 246 217 896 320 954 039, -21 512 679 971 466 893 243 401 657 783},
{15 061 521 789 856 183 563 030 420 061, 2 125 407 681 459 221 144 429 321 780},
{14 509 773 551 689 208 609 988 240 479, -2 536 715 392 159 321 869 439 113 108},
{56 130 985 300 071 085 925 068 615 351, -5 649 936 386 763 128 241 777 133 478},
{29 101 906 837 255 522 923 514 834 891, -2 340 120 734 032 197 011 518 719 760},
{80 616 184 280 663 544 037 925 623 909, -7 309 840 965 309 935 269 484 448 886},

```



```

{16 426 759 318 086 229 814 138 206 877, 1 409 879 456 364 022 603 902 815 798},
{38 851 738 504 281 273 182 951 033 221, 2 715 767 668 675 826 677 052 738 126},
{65 648 300 282 756 276 632 803 257 103, -2 343 042 450 551 315 312 348 246 323},
{3 405 821 718 236 383 077 136 444 661, -65 077 458 483 578 446 782 086 289},
{1 721 716 290 134 003 712 968 653 007, -84 939 735 252 205 379 218 645 975},
{1 810 805 222 101 794 159 062 947 053, -62 979 408 854 347 665 510 314 995},
{1 232 213 139 268 763 118 158 836 358, -272 161 604 451 319 529 024 233},
{10 633 849 258 125 031 768 362 614, -1 920 622 753 583 168 950 061 477},
{70 301 093 806 544 572 628 493 592, -3 111 186 294 002 509 114 230 469},
{99 239 085 485 537 822 905 768 405, -9 223 046 742 968 590 733 653 534},
{174 939 866 282 217 337 989 217 051, 22 217 941 504 299 290 508 499 575},
{221 489 594 421 981 900 223 584 371, 33 521 371 049 273 168 089 885 837},
{1 039 640 230 911 491 836 043 702 552, 23 292 280 462 265 831 239 165 941},
{672 478 801 347 175 007 782 418 647, -112 075 008 753 475 014 984 856 360},
{2 271 157 279 668 511 989 158 473, 137 840 023 680 429 120 733 820},
{5 191 635 161 750 038 535 970 887, -545 378 865 252 513 452 647 642},
{20 710 125 771 232 583 249 937 107, -2 529 777 039 918 139 588 799 024},
{37 280 846 699 109 856 624 048 285, 5 428 225 417 514 917 186 915 129},
{56 621 766 656 070 531 064 251 822, 7 659 507 124 510 826 007 494 171},
{237 412 125 975 085 171 931 617 375, -4 957 944 416 078 794 801 863 366},
{44 967 273 739 061 306 068 111 247, -4 489 764 830 872 286 898 432 414},
{5 500 408 996 736 529 619 181 453, 676 774 808 472 210 673 233 422},
{6 810 631 787 748 694 431 812 083, 962 997 733 368 505 097 167 445},
{5 502 164 679 363 541 379 557 472, -674 893 958 301 041 631 016 581},
{8 138 028 023 461 458 182 561 096, 456 170 056 836 460 153 448 229},
{5 769 606 967 991 141 781 055 054, -32 165 689 831 834 425 446 273},
{943 930 559 329 590 467 602 773, -115 546 413 880 655 497 301 606},
{1 545 180 614 463 372 646 004 075, -52 675 492 635 013 302 701 674},
{1 389 714 915 790 962 544 786 791, -80 175 811 033 097 617 349 518},
{2 111 364 130 035 940 937 753 815, -133 427 322 648 404 206 575 402},
{1 854 369 554 743 583 028 756 743, 329 989 421 964 962 477 568 363},
{9 919 791 186 649 155 095 621 365, -579 067 994 855 092 887 253 372},
{5 975 186 654 893 504 972 809 239, 315 510 341 006 453 406 234 581},
{1 541 276 114 099 669 906 176 200, -30 781 223 165 783 645 939 099},
{174 981 509 028 521 128 478 750, 9 164 673 060 437 332 628 679},
{67 364 949 536 732 874 174 071, 6 870 911 516 418 300 698 632},
{106 189 084 568 560 492 167 671, 2 929 234 947 708 166 581 166},
{58 193 489 634 253 124 409 905, -3 574 277 021 266 823 464 591},
{79 399 526 224 731 969 139 471, 9 098 730 575 266 149 467 521},
{196 634 867 260 406 709 389 222, 3 024 480 826 353 251 849 061},
{3 445 470 248 181 796 820 303, -111 868 265 997 260 532 798},
{1 773 233 820 929 096 018 365, -275 482 065 927 974 661 568},
{9 506 972 603 538 595 867 603, -823 675 195 452 837 745 354},
{29 793 249 609 741 109 054 955, -550 234 649 035 349 453 264},
{6 365 706 384 746 847 717 221, 930 250 295 770 850 055 293},
{11 537 609 166 279 110 916 570, -1 489 250 340 889 538 141 957},
{29 735 091 306 138 343 307 794, -2 418 768 976 791 442 673 831},
{56 079 223 186 641 466 523 938, -5 808 353 575 214 822 337 107},
{158 340 692 675 033 790 923 428, -6 140 582 755 596 623 903 171},
{103 842 258 667 796 014 162 422, -10 444 994 178 235 032 399 277},
{48 006 966 049 790 476 597 492, -3 117 545 056 956 739 221 441},

```

```

{98 259 425 439 711 673 794 283, 6 203 350 174 613 421 509 192},
{78 540 010 974 142 557 870 331, 64 771 778 353 384 698 809},
{2 224 337 312 533 461 013 894, -217 797 168 641 160 618 347},
{3 662 884 463 626 531 603 496, 273 864 725 287 582 220 435},
{8 108 799 756 149 056 289 439, 798 777 215 462 559 632 642},
{9 561 180 520 353 337 078 501, -73 007 973 703 889 717 200},
{226 258 753 641 054 101 221, 36 696 175 319 322 386 101},
{480 454 436 284 462 984 585, 77 088 249 770 888 440 619},
{1 416 070 075 071 454 928 809, -147 906 573 477 867 814 207},
{4 976 657 116 870 633 847 619, 723 374 515 694 718 214 939},
{6 870 194 946 399 098 899 366, 858 730 086 043 830 208 137},
{27 986 385 828 121 507 330, 3 865 872 532 167 783 333},
{73 096 970 132 814 895 921, 10 240 215 201 154 227 626},
{111 821 634 254 088 900 581, -11 991 959 455 291 490 166},
{307 625 933 360 773 637 873, -43 956 992 668 034 254 930},
{5 768 209 921 825 584 323, -5 982 795 227 916 250},
{62 830 447 031 226 517, -11 353 996 700 176 410},
{418 189 120 416 723 497, -24 109 032 236 821 692},
{658 510 218 869 623 907, 29 239 247 946 184 388},
{1 105 406 227 516 744 343, 124 791 609 566 794 306},
{1 399 742 428 167 948 469, -95 776 675 769 919 713},
{2 915 708 962 086 930 854, 74 092 584 511 670 449},
{2 061 755 124 410 884 097, -201 460 366 151 770 105},
{3 724 965 568 561 460 713, 493 340 160 837 862 061},
{17 518 701 733 173 426 225, -388 377 749 581 277 969},
{3 294 537 159 257 491 980, -447 165 755 380 685 051},
{12 985 772 855 823 033 217, -1 957 589 741 756 704 560},
{56 671 071 581 437 997 537, 9 026 456 294 578 223 531},
{198 474 371 303 523 851 729, -15 486 758 779 230 682 841},
{225 425 933 291 526 991 116, -17 815 435 957 412 019 301},
{487 803 998 231 511 523 963, -25 118 883 284 838 748 125},
{833 072 049 746 449 457 452, -149 524 226 896 157 233 563},
{5 061 791 618 809 021 570 154, 663 657 701 090 475 208 353},
{19 550 129 203 267 627 636 930, -2 192 550 433 447 181 835 877},
{14 443 151 122 803 701 991 077, -1 751 751 511 130 138 832 308},
{33 901 983 667 244 715 276 427, -1 493 017 609 014 332 648 785},
{34 556 285 866 709 916 004 612, 3 781 421 349 964 075 745 107},
{41 356 003 645 625 509 593 271, -4 894 069 232 113 909 352 967},
{174 072 533 308 424 546 793 265, -3 231 206 100 721 988 985 303},
{32 595 094 314 465 814 634 663, 3 994 238 444 256 356 262 864},
{50 653 754 072 782 198 008 329, -560 235 788 325 369 386 987},
{18 370 116 756 417 301 180 421, 2 945 596 792 583 313 866 324},
{55 026 344 072 476 020 615 683, -9 692 381 705 179 662 462 400},
{247 107 746 529 554 378 538 643, 40 014 645 913 539 969 707 256},
{554 569 812 816 850 263 313 453, -96 063 139 248 298 370 056 424},
{1 722 912 791 162 256 604 982 189, -551 889 567 533 810 274 172},
{6 828 655 585 626 607 640 805, 985 007 433 729 017 141 653},
{5 245 319 587 644 475 710 514, -795 704 711 838 027 302 027},
{25 644 458 222 515 516 890 325, -3 035 846 994 804 070 085 892},
{107 256 898 862 553 540 051 931, -3 595 198 639 087 157 430 582},
{47 325 764 494 833 446 376 791, 6 056 708 619 496 587 410 522},

```

```

{89 104 452 430 000 979 683 415, 12 158 459 655 344 609 281 237},
{315 623 552 564 508 462 465 724, 33 623 829 291 642 319 394 331},
{1 027 718 026 238 479 445 422 855, 15 437 459 275 042 885 052 914},
{520 747 869 962 114 396 668 257, -72 595 619 773 857 475 885 564},
{993 703 992 063 853 172 075 411, 101 384 674 797 257 782 799 820},
{1 591 277 716 789 247 817 900 331, 168 569 589 958 845 463 466 554},
{5 857 961 165 611 453 089 406 255, 414 652 760 971 667 087 823 736},
{4 172 978 448 640 994 930 042 129, 588 658 303 820 359 274 838 985},
{4 137 255 429 979 920 487 369 486, -576 913 384 925 142 833 861 551},
{7 810 077 104 809 731 376 751 691, 295 687 864 732 897 882 061 327},
{9 653 217 118 596 529 009 417 931, -1 445 760 902 241 515 278 064 534},
{36 901 626 570 432 157 025 670 753, 5 845 777 551 253 625 575 254 962},
{144 329 939 769 921 882 357 137 499, -15 020 463 070 578 912 405 654 043},
{464 100 583 933 512 094 252 831 549, -5 945 677 405 315 984 932 125 596},
{26 681 959 190 356 294 215 769 819, 434 360 840 492 399 834 882 828},
{14 689 885 705 272 438 745 467 569, 1 959 568 263 236 240 858 131 298},
{76 859 721 146 881 466 345 330 157, 13 734 252 715 943 880 702 842 507},
{438 117 816 753 763 611 866 265 915, 40 790 450 643 142 452 435 593 602},
{835 594 085 343 465 829 095 832 853, 151 662 161 528 019 668 747 227 975},
{5 875 931 822 147 522 487 615 264 763, 960 615 024 775 926 078 400 079 453},
{8 867 092 205 865 315 359 968 255 555, 1 023 390 738 156 826 711 342 650 772},
{27 130 530 566 143 878 327 132 510 047, -1 173 398 803 688 300 425 249 887 812},
{11 246 288 423 724 515 164 422 139 309, -1 874 049 613 701 801 001 053 480 450},
{157 268 579 583 023 489 999 272 111, -26 343 489 084 119 306 188 536 746},
{62 596 038 813 695 423 423 920 835, -9 889 000 700 678 892 317 332 301},
{257 700 734 160 143 492 074 235 291, -24 439 025 921 312 364 446 181 051},
{879 155 526 969 108 829 866 745 330, -5 684 821 743 221 137 825 287 951},
{157 355 615 183 235 111 178 078 925, -13 006 711 684 397 780 072 053 271},
{100 730 922 666 478 274 761 734 167, 7 830 652 947 516 628 820 806 067},
{84 337 686 447 794 092 790 831 616, 566 494 864 168 270 228 249 027},
{5 533 816 748 975 526 243 599 153, -62 270 397 820 110 773 239 467},
{651 643 904 132 273 402 359 390, -104 070 693 939 786 914 548 797},
{2 150 359 498 990 601 290 262 032, -327 860 078 113 110 880 038 643},
{11 428 222 776 292 814 730 669 051, 729 923 853 531 332 141 579 191},
{19 794 151 536 471 463 233 242 395, 465 675 779 396 652 841 981 071},
{18 162 651 229 184 108 783 548 982, 3 215 427 527 386 386 601 691 883},
{89 263 200 875 602 655 301 582 964, 8 121 258 287 612 370 238 078 555},
{5 580 582 762 539 968 065 210 139, -377 509 334 348 259 847 288 988},
{6 482 522 962 030 441 885 849 799, -1 112 346 848 328 947 899 174 685},
{15 133 092 107 516 395 226 666 569, -1 007 570 347 679 032 233 216 189},
{1 543 414 494 142 026 545 474 986, -278 274 603 141 929 023 718 891},
{9 972 416 852 054 260 150 230 440, 19 129 948 751 111 023 917 749},
{451 370 665 307 918 437 573 669, 20 028 690 004 015 038 784 100},
{733 847 177 969 768 902 389 849, 34 055 122 173 189 012 205 894},
{1 213 875 277 390 759 925 045 701, -16 755 939 454 182 255 937 120},
{588 363 298 481 362 308 271 819, -27 830 432 883 473 641 319 866},
{310 012 426 344 851 403 816 007, -36 365 629 237 289 518 666 631},
{1 364 980 706 469 586 870 510 088, -133 528 491 845 369 993 295 079},
{2 345 967 253 255 068 067 184 542, -214 616 626 255 575 199 675 537},
{1 170 435 208 944 471 210 462 835, 198 229 660 061 365 596 728 608},
{1 496 477 362 474 067 222 796 227, 270 710 802 502 630 951 751 701},

```

```

{10 095 208 750 795 760 529 404 341, 848 863 344 551 171 673 847 967},
{7 200 959 321 645 664 984 929 777, -975 450 951 275 383 574 823 718},
{29 451 410 354 720 416 931 936 329, -1 381 684 619 005 370 294 832 269},
{34 446 635 093 003 618 496 235 720, 4 651 620 912 169 979 967 966 229},
{148 937 807 917 286 938 917 297 243, -15 235 555 624 764 602 786 507 660},
{270 002 118 098 368 026 874 569 203, 14 232 475 391 440 666 306 888 904},
{32 778 232 781 366 003 549 277 867, -5 341 583 628 317 555 049 256 235},
{57 569 749 905 393 187 045 496 103, 678 880 010 103 638 278 222 495},
{10 669 025 319 869 261 669 861 788, 1 199 166 288 735 617 007 307 527},
{9 754 231 021 352 020 276 570 445, -1 636 792 631 640 031 064 204 563},
{5 255 456 710 565 122 583 897 707, 48 992 727 055 704 951 739 658},
{1 045 558 332 770 727 072 589 779, 32 299 912 039 794 338 685 692},
{944 930 652 287 350 537 163 165, 123 580 109 190 181 122 699 763},
{3 453 107 477 493 777 110 360 181, 377 942 700 286 530 415 624 571},
{4 078 230 818 285 266 209 384 318, -83 968 128 066 051 614 303 251},
{2 860 389 099 149 768 426 523 499, 333 384 607 698 334 413 310 135},
{11 065 717 240 684 062 168 149 564, -1 964 791 604 636 433 622 918 081},
{57 119 558 583 628 625 979 354 838, 8 442 962 177 966 723 630 667 233},
{156 512 956 308 936 715 389 947 647, 22 455 466 364 805 756 667 184 557},
{53 349 351 331 582 921 147 195 908, 8 156 614 953 096 222 120 901 025},
{296 009 313 867 160 062 229 790 093, 7 597 299 881 168 716 094 179 483},
{22 545 138 375 169 370 013 569 776, 3 965 941 542 526 571 834 848 891},
{98 790 359 519 214 818 646 362 030, 13 073 957 817 806 744 878 589 381},
{458 302 938 835 892 090 205 888 422, -23 415 941 563 122 418 879 135 967},
{791 255 501 697 946 702 769 642 522, 107 094 101 265 877 087 883 161 661},
{3 286 146 634 107 759 919 413 360 705, 16 285 054 132 451 162 505 059 534},
{271 309 751 142 617 622 084 547 877, 8 212 067 596 697 953 567 063 265},
{24 610 115 675 227 195 345 350 428, -1 701 362 770 663 995 810 757 681},
{62 491 913 988 569 065 584 688 626, 3 232 759 269 582 526 035 406 757},
{84 489 541 453 584 602 044 859 197, 7 266 797 268 771 105 222 357 427},
{214 250 035 961 824 189 250 964 233, -23 535 752 584 179 206 009 961 552},
{191 832 753 632 695 477 743 510 935, -28 414 375 174 810 563 159 022 798},
{558 361 934 687 298 685 202 243 429, -9 915 717 712 095 644 355 118 627},
{243 457 681 985 465 503 932 425 043, 20 993 174 139 463 039 317 311 204},
{668 372 207 359 186 462 149 442 995, 59 002 003 664 886 372 620 224 099},
{1 528 663 196 589 472 702 831 254 574, 171 919 534 984 787 145 138 829 629},
{1 470 396 843 615 316 670 038 754 873, -87 495 015 429 771 987 763 777 616},
{1 344 455 076 573 762 633 691 703 321, 2 628 230 484 295 523 479 804 470},
{94 715 579 458 085 649 486 640 201, 983 852 825 551 151 559 692 376},
{20 990 948 208 832 880 737 596 295, 668 993 717 762 043 925 787 254},
{19 919 293 698 552 004 017 122 259, 1 665 483 186 669 105 384 334 603},
{5 253 858 776 703 586 996 545 183, -426 215 953 701 432 233 482 993},
{11 002 119 250 625 615 385 192 093, -1 361 039 251 968 301 263 326 503},
{8 990 613 555 457 217 007 825 451, 1 389 508 873 903 651 798 332 296},
{51 631 264 650 789 191 208 702 325, -3 948 293 255 754 789 834 460 066},
{23 972 733 752 176 945 496 995 893, -3 911 056 338 051 185 790 056 209},
{40 005 262 185 716 629 776 032 481, -578 454 869 316 746 609 329 360},
{7 258 220 026 027 984 852 224 639, -402 966 665 493 912 109 845 427},
{380 783 723 867 783 125 549 287, 35 785 099 573 120 868 184 503},
{1 015 337 343 487 167 533 939 434, 154 727 307 002 221 892 841 335},
{5 352 550 636 742 471 560 042 969, -434 295 091 236 414 959 180 951},

```

```

{11 139 753 810 533 871 939 853 003, -1 595 098 485 602 626 205 093 905},
{2 048 911 506 076 408 168 542 228, -345 407 708 332 537 356 287 009},
{1 859 244 769 586 461 565 206 254, -13 093 987 556 073 101 924 449},
{8 015 606 697 593 737 174 816, -1 313 124 450 438 480 633 361},
{10 811 939 602 065 416 597 350, -544 395 382 648 525 549 419},
{6 001 476 021 502 456 891 370, -1 054 234 295 721 228 393 299},
{25 590 450 473 168 164 005 496, -1 261 156 125 325 372 188 043},
{29 018 909 366 196 899 326 244, -3 758 734 602 256 419 005 401},
{83 026 428 696 501 764 640 156, -7 840 527 459 534 186 492 881},
{254 330 495 311 568 655 741 265, -34 131 122 446 779 483 714 006},
{1 217 598 416 544 869 309 714 617, -14 559 629 260 044 278 085 672},
{427 424 862 609 153 909 064 649, 51 891 127 876 937 923 956 395},
{971 371 327 898 390 875 665 631, 177 026 271 903 580 937 652 214},
{6 812 957 502 058 408 804 960 319, -1 020 679 017 821 702 533 868 708},
{26 211 854 192 787 205 637 530 323, 3 657 057 943 020 427 923 640 148},
{48 383 438 739 892 603 591 893 673, 4 731 430 975 700 286 136 702 524},
{84 461 189 648 289 635 764 606 207, 1 726 161 034 692 310 545 284 712},
{9 535 383 079 052 895 393 229 799, 146 167 656 887 526 286 341 963},
{2 724 345 127 731 255 699 174 116, -453 667 820 448 423 167 751 915},
{184 718 198 216 618 720 347 454, 30 645 714 209 351 884 944 181},
{66 669 123 880 085 443 907 072, -1 862 687 077 977 158 488 229},
{30 621 263 240 288 671 864 588, 1 022 959 646 412 871 292 247},
{5 334 566 015 699 885 322 938, -525 217 222 728 684 632 155},
{6 509 109 284 630 081 109 652, -872 022 907 937 858 255 961},
{31 990 965 396 140 792 116 075, 1 571 303 930 231 955 098 031},
{44 626 056 528 633 522 280 945, -6 920 725 140 067 663 321 111},
{245 034 749 369 975 845 988 041, -7 040 496 313 753 032 723 223},
{109 227 107 299 043 646 656 356, -5 145 165 433 911 940 719 567},
{93 112 021 764 538 432 090 471, 3 696 279 759 682 940 970 459},
{55 697 194 024 727 718 490 684, 5 764 825 394 199 758 093 885},
{154 133 733 464 319 133 405 114, -2 775 305 335 172 801 442 403},
{101 385 859 123 262 042 186 866, -4 056 441 653 596 728 335 159},
{1 989 395 115 837 129 176 611, -135 909 615 510 253 262 118},
{3 890 680 228 516 910 657 561, -688 935 476 157 375 489 566},
{19 191 677 645 760 040 106 965, -1 934 467 178 710 745 246 006},
{12 086 537 166 445 575 894 505, 1 970 683 749 600 294 282 804},
{20 732 338 838 661 005 616 799, 3 471 908 289 013 333 686 536},
{7 829 760 738 100 723 690 943, -1 230 237 952 717 997 077 509},
{35 418 308 721 626 556 845 231, -6 177 194 840 795 300 267 744},
{129 943 965 528 474 336 137 407, 10 988 898 710 707 740 394 206},
{151 902 701 001 465 338 852 135, 24 065 017 862 695 056 039 886},
{593 494 912 198 305 206 412 701, -59 650 577 249 086 254 794 765},
{237 857 963 112 029 981 260 971, -2 611 615 466 982 714 943 699},
{15 875 493 711 630 789 364 598, -2 347 671 039 669 275 424 791},
{44 098 081 718 276 950 106 181, 7 399 074 562 602 542 306 948},
{23 412 886 929 725 995 105 053, -93 814 174 465 875 829 088},
{3 211 878 252 694 011 188 813, 337 056 289 528 773 449 174},
{12 536 086 764 904 140 931 233, 983 680 938 534 752 224 552},
{19 889 469 447 763 401 047 497, 2 602 379 954 951 092 414 209},
{73 436 045 155 781 723 027 825, 10 072 268 066 982 177 030 089},
{231 483 326 265 612 221 558 958, 30 935 150 008 999 709 087 309},

```

```

{1 180 044 820 006 526 377 875 805, -155 209 208 543 903 865 018 919},
{4 868 679 019 231 658 839 768 213, -249 128 739 006 616 745 441 440},
{8 997 765 111 153 409 455 786 373, -136 692 015 194 913 126 668 378},
{1 888 723 445 157 695 441 799 425, -294 592 553 439 466 600 728 938},
{9 572 281 837 150 771 156 637 963, 1 324 317 556 023 993 539 850 689},
{23 862 656 653 642 493 836 968 060, -495 425 928 124 609 785 528 289},
{6 494 756 189 236 706 397 204 852, -992 232 223 036 175 989 607 599},
{35 618 680 389 305 516 873 818 939, -64 925 111 017 539 049 411 013},
{1 991 239 186 550 278 973 348 642, 12 355 227 731 070 579 548 833},
{161 754 225 985 337 612 935 791, 26 012 853 321 706 766 608 351},
{448 491 378 352 664 049 569 115, 79 382 505 241 073 938 641 349},
{2 196 488 594 408 587 000 039 341, 179 229 603 712 021 936 056 557},
{3 612 934 639 281 577 621 491 903, -429 799 913 469 548 839 581 580},
{13 788 291 190 489 765 482 301 777, 1 476 479 135 518 583 355 425 569},
{39 498 338 694 978 707 394 260 824, 646 730 475 144 539 313 195 759},
{3 774 597 181 782 933 856 242 475, -175 922 540 202 761 697 385 364},
{6 337 683 164 470 118 680 836 649, 61 067 053 321 074 646 626 838},
{1 049 940 092 809 920 900 005 737, 186 176 395 095 105 186 127 429},
{5 302 343 943 096 107 123 948 123, 863 505 227 971 460 583 983 293},
{9 583 693 446 120 145 983 820 835, 1 373 684 037 439 051 488 031 032},
{2 535 490 460 303 940 159 314 731, 376 671 571 571 501 566 496 349},
{7 995 632 715 029 093 686 617 248, -405 997 352 143 089 966 895 091},
{9 820 831 898 783 746 451 481 188, -372 248 745 032 067 600 561 103},
{11 246 797 708 049 118 114 508 290, -507 651 683 685 606 555 147 607},
{6 198 392 690 296 138 199 613 944, 851 985 144 971 058 601 547 639},
{18 525 237 364 399 511 113 657 209, -697 209 441 917 487 224 073 109},
{23 653 987 822 438 870 969 021 986, 2 980 889 188 641 445 782 663 895},
{15 256 929 248 722 928 090 844 746, -263 159 510 971 350 822 233 773},
{499 468 621 618 148 298 412 952, 71 137 151 006 689 970 401 691},
{119 176 601 134 161 942 488 085, 20 043 240 794 214 870 394 709},
{85 544 646 859 055 110 533 351, -13 292 757 608 418 934 936 961},
{457 259 995 474 778 572 015 215, -42 998 240 778 874 701 404 129},
{1 241 931 594 334 608 330 986 116, 205 568 443 683 943 294 594 779},
{673 153 646 244 936 509 977 918, -69 157 239 004 030 107 996 447},
{1 455 080 759 833 801 028 937 608, 121 986 180 662 653 235 619 233},
{691 519 241 324 986 080 961 852, 9 347 473 728 048 325 573 769},
{15 311 349 496 610 908 267 266, -2 148 946 824 364 043 019 605},
{21 229 016 358 945 963 272 449, 1 677 662 103 183 950 410 983},
{45 866 687 613 185 973 556 070, 2 161 801 775 798 877 848 903},
{37 039 175 391 353 559 599 453, -5 974 230 883 284 750 810 002},
{94 309 417 239 959 324 415 839, 12 714 537 428 396 910 222 888},
{419 304 764 053 295 275 594 217, -73 005 557 116 377 522 083 317},
{1 479 557 712 952 618 695 549 115, -206 977 575 551 560 108 331 472},
{2 426 460 043 244 137 041 076 069, -318 163 372 706 925 324 746 946},
{9 388 908 134 489 978 995 060 421, 1 008 977 946 360 192 604 410 437},
{24 340 422 762 611 398 873 952 552, -706 569 339 336 874 202 228 845},
{25 048 152 787 456 403 855 573 938, -649 628 630 177 438 294 181 727},
{22 701 739 367 631 479 783 559 785, 1 319 362 417 335 631 793 022 223},
{21 533 683 561 133 404 872 377 526, 1 467 622 076 511 194 726 143 879},
{37 971 159 336 226 765 562 672 061, -4 431 903 968 376 666 776 253 553},
{151 362 133 953 895 598 465 183 364, 16 740 523 527 353 711 615 905 303},

```

```

{55 096 354 409 263 319 840 815 323, 7 860 497 123 457 674 619 343 192},
{5 757 089 059 708 202 927 625 341, -349 098 424 972 036 222 946 786},
{13 549 626 552 294 245 477 664 435, 2 264 705 694 287 603 110 161 016},
{3 050 001 461 078 481 480 831 219, 227 576 472 850 924 816 986 776},
{7 229 077 807 300 249 940 247 349, -597 443 390 118 088 038 680 289},
{4 720 812 944 772 284 610 626 599, -408 198 252 788 463 282 064 008},
{14 027 721 006 452 707 157 178 263, 1 351 162 538 354 788 582 436 154},
{40 771 554 209 480 885 292 521 117, 1 974 429 080 349 567 450 661 397},
{54 625 061 750 942 462 538 089 380, 4 438 005 515 911 403 155 176 677},
{108 150 649 240 444 349 401 571 224, -6 705 405 404 467 191 169 018 333},
{68 268 858 748 573 965 084 953 784, -3 451 900 650 610 067 710 209 643},
{60 763 186 826 563 740 419 887 004, 5 034 467 655 863 935 611 363 349},
{27 616 421 539 524 533 598 618 464, 2 353 669 354 994 615 828 875 675},
{49 581 246 912 457 651 483 281 244, -3 932 770 125 426 309 593 183 885},
{122 036 412 728 665 485 020 631 619, -2 898 397 862 449 307 444 653 068},
{23 992 497 957 771 215 271 018 277, 18 258 235 612 260 155 290 930},
{92 932 697 648 326 280 164 303, 9 590 161 018 407 847 222 444},
{234 544 090 324 423 172 750 823, 17 263 451 377 102 197 122 681},
{564 394 087 445 599 370 370 169, 86 465 819 075 466 581 550 534},
{3 228 465 040 530 669 338 201 951, 279 996 711 422 145 941 648 820},
{10 388 144 226 271 474 965 127 231, 760 476 194 754 731 925 339 906},
{20 423 277 523 286 987 180 884 787, -100 399 317 236 720 507 355 478},
{3 335 073 814 385 210 830 097 487, -585 940 445 206 911 417 323 740},
{14 264 939 691 644 356 233 751 287, -839 176 468 137 250 904 957 273},
{83 761 068 423 822 891 265 966, 2 826 525 487 094 231 963 071},
{81 740 998 931 321 342 466 956, -13 252 187 112 618 596 971 317},
{176 002 224 193 171 090 485 266, -13 188 199 293 940 224 212 987},
{359 895 036 383 905 881 598 365, 15 039 198 070 699 053 386 947},
{82 611 667 716 840 575 380 677, -5 390 366 727 672 170 030 260},
{138 737 177 338 883 969 215 383, -18 408 273 478 239 649 378 276},
{673 791 828 475 624 839 055 175, -29 794 219 962 848 990 199 746},
{906 543 222 922 252 907 579 657, 24 271 551 074 977 311 366 385},
{671 170 818 699 298 574 849 548, -53 580 755 434 226 191 487 169},
{2 004 941 153 705 711 244 208 271, -183 066 659 237 823 992 668 575},
{694 575 734 917 861 336 538 266, -71 071 766 024 876 595 609 837},
{1 275 212 101 141 464 945 248 216, -2 720 499 189 556 553 739 069},
{55 459 482 084 141 911 636 455, -9 024 548 643 276 176 284 804},
{103 663 027 734 303 460 282 849, 10 077 470 872 336 587 625 165},
{228 177 201 864 069 138 464 721, -41 492 314 257 308 946 659 675},
{1 636 534 815 624 428 008 141 334, -274 126 392 586 368 036 994 155},
{649 659 651 608 636 892 064 084, -45 936 765 362 909 357 931 599},
{517 049 985 704 564 600 714 142, -22 744 436 793 698 833 640 723},
{479 692 783 490 177 268 776 473, 35 912 947 054 721 681 095 887},
{1 013 133 270 524 837 747 865 418, -138 154 635 357 523 364 371 471},
{3 638 015 018 751 761 583 944 559, -230 425 252 099 932 019 838 137},
{3 854 332 172 924 907 943 785 007, -189 863 681 481 196 949 330 818},
{4 507 624 920 776 547 616 323 113, -106 951 035 461 661 176 117 755},
{1 238 833 079 555 479 330 814 837, 191 336 892 643 565 963 646 408},
{7 174 126 171 832 600 365 974 731, -685 625 403 928 826 386 865 454},
{25 111 898 471 002 583 288 295 089, 1 145 344 152 337 265 971 342 368},
{6 768 157 552 964 178 417 723 553, -1 039 700 879 016 134 924 611 764},

```

```

{40 270 139 411 752 518 310 144 805, - 6 559 886 983 610 634 448 900 974},
{71 954 583 297 008 217 722 377 919, 10 043 084 146 212 616 245 420 434},
{130 586 547 608 072 416 350 355 599, - 21 522 529 294 515 990 798 182 047},
{114 658 375 437 141 253 339 802 043, - 16 688 478 734 056 261 990 933 993},
{170 717 080 398 953 867 142 136 732, 2 355 617 927 623 113 871 617 475},
{87 894 579 197 083 802 468 604 028, - 7 496 775 873 376 303 250 284 043},
{163 271 771 391 115 086 249 554 552, - 7 106 778 198 504 638 320 862 123},
{14 546 046 784 836 015 291 667 883, 768 231 354 959 255 662 934 252},
{3 977 567 791 797 542 022 549 495, 634 755 495 046 729 001 172 382},
{13 353 750 899 856 273 225 701 037, 1 125 585 868 712 866 593 209 308},
{12 109 082 451 151 945 532 042 061, - 19 159 303 403 443 033 353 112},
{402 700 175 948 452 875 277, 58 160 689 286 932 973 398},
{349 547 275 746 157 142 211, 24 639 165 053 662 904 954},
{363 318 234 595 241 355 545, - 54 055 733 531 896 200 559},
{1 190 680 110 114 531 821 072, - 100 448 088 109 494 182 559},
{1 161 058 828 752 471 201 244, - 162 618 946 218 461 247 275},
{1 795 370 212 636 155 155 201, - 324 757 673 251 837 388 956},
{12 100 890 323 114 665 104 265, - 996 737 689 332 083 337 566},
{11 063 006 039 243 539 224 367, - 1 581 311 284 789 139 204 091},
{487 663 388 154 381 137 330, - 29 349 046 227 407 710 151},
{890 361 419 212 444 883 723, 30 683 916 520 572 248 818},
{527 840 115 849 668 001, 69 189 801 291 504 760},
{2 028 585 264 107 236 241, - 253 300 522 107 750 003},
{2 181 087 245 236 217, - 294 401 660 348 831}, {9 501 774 200 757 600, 1 158 220 259 705 551},
{18 644 957 725 942 168, 2 522 830 103 065 145}, {77 826 613 354 406 087, - 681 263 768 542 604},
{12 840 955 503 389 249, - 1 968 384 479 661 027},
{74 081 132 484 797 260, - 7 663 664 744 180 427},
{201 885 681 603 553 790, 12 550 044 764 627 413},
{85 712 264 191 699 378, - 15 394 326 504 523 269},
{525 641 891 999 778 644, 58 408 892 490 737 187}, {3 013 092 931 627 081, 230 247 810 208 759},
{1 569 840 514 143 906, - 251 081 184 970 631}, {5 004 918 941 289 480, 374 322 365 438 431},
{10 959 527 056 600 283, 1 409 644 179 891 018}, {25 092 484 219 701 019, - 827 909 091 694 794},
{20 161 706 039 718 721, 1 205 375 127 840 213}, {26 044 019 551 627 100, 379 993 634 444 173},
{13 867 756 776 646 123, 524 676 032 535 971}, {17 868 214 526 159 283, 2 094 098 626 649 111},
{77 315 175 980 934 564, 4 855 330 275 512 815}, {29 238 565 754 367 604, 2 822 106 304 864 559},
{80 382 713 752 039 106, - 13 114 229 643 207 087},
{134 089 535 530 930 136, - 2 346 583 100 240 217},
{26 409 606 561 783 593, - 1 181 416 620 967 526},
{33 056 831 139 343 659, 3 746 375 859 106 318}, {52 183 575 816 443 037, - 8 623 750 082 655 817},
{34 844 950 320 142 665, - 3 343 488 908 806 048},
{111 394 837 334 492 615, - 18 784 969 413 377 602},
{103 883 352 516 066 763, - 3 228 830 212 429 049},
{44 302 071 748 638 405, 5 126 986 526 563 609}, {145 423 752 244 292 004, 22 035 286 182 180 521},
{697 036 831 446 759 797, 50 332 350 894 982 370},
{601 670 405 556 477 257, - 661 395 381 061 304},
{15 751 905 535 441 257, 209 129 474 094 053}, {5 308 403 292 595 278, 931 993 467 580 763},
{22 401 043 518 254 700, 381 026 925 227 023}, {6 284 060 541 032 903, - 112 635 650 284 128},
{1 859 334 115 382 935, 25 191 543 340 207}, {382 367 251 598 257, - 25 054 656 168 855},
{517 245 316 169 128, - 80 569 208 364 265}, {2 672 575 212 699 502, - 478 535 979 641 323},
{15 692 612 546 726 444, - 2 519 712 633 467 991}, {45 372 602 927 561 342, 811 889 535 666 015},
{7 363 674 509 104 342, 735 631 218 291 423}, {581 623 769 018 848, 40 837 257 418 961},

```



```

{782 271 047 118 126, 67 352 652 165 233}, {2 050 901 530 308 930, -50 821 411 525 397},
{1 425 560 474 150 950, 171 564 565 481 237}, {4 190 472 073 783 266, -290 870 355 557 371},
{9 344 680 582 425 688, 1 033 522 394 922 307}, {3 395 343 221 869 075, -613 590 632 244 197},
{22 609 845 156 092 453, -1 325 239 510 431 055}, {6 381 104 822 396 922, 715 468 463 642 645},
{4 590 796 680 563 757, 775 782 853 697 683}, {5 048 134 888 164 939, -134 122 809 536 620},
{3 834 018 063 903 059, -663 692 867 183 092}, {11 702 991 996 443 947, 879 316 067 432 704},
{21 478 766 465 684 805, -1 495 524 945 521 879}, {42 771 961 041 901 421, 7 462 326 287 583 327},
{158 157 738 004 284 739, -8 944 738 475 505 943},
{224 956 809 830 956 565, -36 577 399 243 633 838},
{433 900 735 163 129 423, -22 574 239 548 926 888},
{394 224 514 947 965 529, -46 780 985 100 768 404},
{1 578 154 097 203 645 463, -219 763 482 284 320 238},
{3 144 967 975 858 899 963, -44 086 372 630 647 107},
{1 172 006 007 553 473 914, -40 983 010 575 476 541},
{1 303 602 631 692 316 225, -112 105 889 012 545 586},
{3 291 774 880 200 233 753, 397 753 830 970 247 473},
{8 669 794 362 622 063 551, -403 274 760 444 100 643},
{15 880 927 070 380 053 792, -2 710 169 047 171 193 837},
{30 026 889 799 121 629 170, 4 675 300 557 967 127 393},
{156 031 829 654 190 320 148, 25 683 701 549 920 586 759},
{152 440 008 018 677 167 926, 14 488 772 171 587 577 825},
{547 982 383 634 108 863 771, 62 335 539 613 378 089 751},
{1 029 960 358 017 221 575 052, -9 380 351 324 052 206 853},
{148 384 722 653 173 123 462, -21 537 022 579 474 242 481},
{187 580 396 848 579 338 495, -20 040 883 502 800 925 126},
{569 783 180 546 309 976 519, 90 057 518 300 801 782 798},
{2 325 607 588 578 443 098 749, 284 911 533 735 507 943 450},
{3 658 910 176 855 984 540 771, -325 440 951 223 991 183 907},
{6 245 717 357 974 439 905 726, -489 786 574 621 299 352 367},
{9 599 140 856 093 682 328 555, -67 948 365 599 435 502 362},
{1 455 283 219 288 843 145 527, -25 741 976 105 220 987 828},
{948 744 077 991 499 692 851, -56 022 743 010 591 917 994},
{287 761 701 896 470 130 713, -10 833 085 832 866 569 720},
{373 797 631 683 252 886 433, 32 512 667 975 117 207 382},
{1 276 504 432 600 124 813 249, 225 549 596 274 536 624 683},
{6 066 658 458 720 499 853 071, -2 408 454 762 368 464 989},
{18 887 927 167 412 883 380, 3 062 268 352 624 079 871},
{40 631 047 081 803 928 166, 3 276 087 883 162 782 353},
{104 121 406 224 192 654 470, -8 741 531 451 799 799 903},
{61 380 724 594 990 604 914, -7 916 121 774 860 792 697},
{153 911 718 707 763 196 298, 3 881 996 571 262 627 885},
{108 083 387 276 611 609 058, 10 731 711 986 377 628 749},
{60 535 125 613 990 403 872, 3 378 557 979 308 303 235},
{22 034 523 071 165 294 282, 18 458 610 659 065 041},
{399 586 404 910 809 088, 8 605 927 859 616 641},
{293 384 146 107 044 558, 33 680 434 800 527 891},
{769 441 600 718 810 419, -118 675 136 740 317 068},
{4 533 871 641 875 732 869, 610 659 965 696 945 542},
{20 480 898 677 772 011 925, 3 132 309 822 560 848 768},
{114 176 336 332 160 426 629, 4 024 517 964 476 671 802},
{117 696 832 818 275 677 667, 15 500 753 850 492 989 239},

```

```

{498 426 640 867 790 663 355, 56 207 636 901 705 807 854},
{587 925 208 557 366 979 149, 91 830 254 530 260 044 113},
{2 918 550 828 688 730 443 209, -244 977 211 398 219 552 686},
{1 672 880 939 102 430 932 817, -297 857 406 971 742 751 150},
{9 026 816 715 514 020 352 557, 335 244 096 978 485 802 001},
{1 957 138 329 502 607 816 130, 98 114 155 867 953 119 231},
{406 438 240 659 910 910 710, 7 321 773 965 192 863 671},
{282 907 009 880 266 934 414, 44 691 498 764 528 916 675},
{1 165 883 366 154 381 314 756, 106 768 390 400 107 644 877},
{676 945 331 497 419 532 389, 14 260 409 739 036 041 243},
{529 779 827 255 321 923 472, -40 284 465 330 406 092 235},
{480 460 458 843 375 228 943, -7 784 665 959 779 140 891},
{172 917 622 371 588 997 621, -19 772 281 427 584 696 321},
{397 599 927 657 188 272 172, -43 488 209 279 581 887 133},
{490 277 487 135 151 750 025, -16 038 211 422 809 409 282},
{545 658 290 783 255 079 643, 65 189 049 284 394 170 520},
{1 907 525 824 140 035 523 157, 248 317 902 322 491 228 031},
{6 242 374 160 751 649 786 189, 1 006 425 665 335 605 570 302},
{16 101 793 330 303 292 785 783, 2 667 423 947 280 670 683 729},
{7 682 722 082 922 225 989 311, -791 489 561 736 402 399 984},
{18 341 709 220 902 042 831 791, 1 930 382 887 866 508 850 667},
{76 007 452 963 280 608 315 441, -12 992 897 765 812 576 345 238},
{154 044 756 895 993 130 722 973, 8 573 567 806 681 958 648 588},
{22 077 626 318 287 871 177 269, 3 461 532 023 381 648 885 944},
{103 366 300 061 840 251 066 795, 7 848 891 713 560 756 083 761},
{105 125 915 058 483 336 254 258, 2 614 032 875 903 932 870 591},
{44 603 401 763 755 693 018 822, -6 345 611 220 499 382 566 297},
{14 545 734 400 541 189 324 697, 616 612 009 349 816 491 955},
{19 983 352 084 498 112 095 617, 2 637 277 503 809 013 026 824},
{88 074 567 731 945 377 399 025, -14 357 900 201 437 400 417 446},
{152 246 155 342 357 016 653 571, -16 517 532 387 389 194 255 814},
{283 480 744 612 487 199 748 355, 47 928 115 053 312 822 210 059},
{322 947 710 883 788 947 447 921, 7 292 527 245 959 744 540 411},
{164 044 452 863 254 825 917 123, -26 078 845 421 634 605 560 261},
{598 139 046 342 328 211 889 003, -84 098 521 279 416 582 260 242},
{746 502 393 526 558 749 317 411, -67 002 600 131 063 295 712 054},
{748 429 574 704 137 222 300 543, -73 145 971 594 764 798 118 099},
{1 340 618 841 762 650 048 444 687, 126 979 091 271 836 858 274 623},
{4 435 941 815 976 876 013 517 114, -261 045 982 880 473 495 442 333},
{145 351 546 302 699 311 201 213, -26 486 392 381 763 095 640 674},
{1 020 647 167 116 822 806 829 597, 155 582 686 376 502 386 011 436},
{5 406 099 363 976 817 724 785 945, -383 927 295 490 950 721 324 274},
{2 458 260 941 177 102 473 442 611, 351 329 580 273 412 494 045 828},
{82 643 538 206 013 805 376 615, 3 776 908 989 986 713 018 563},
{35 428 306 321 816 601 509 909, 746 725 444 868 319 724 780},
{26 244 622 627 440 381 174 671, 1 186 698 281 627 304 784 294},
{10 843 574 099 534 397 696 037, -1 784 096 172 657 362 502 062},
{10 980 768 023 627 592 009 535, 138 421 904 144 386 257 077},
{45 437 596 221 077 700 452, 4 984 912 710 335 288 661},
{45 297 164 416 748 097 737, -5 265 648 213 343 537 869},
{165 399 890 764 155 703 636, -9 028 700 324 640 354 401},

```

```

{227 779 508 729 716 629 022, 39 270 038 637 665 675 419},
{619 417 124 605 916 455 868, 81 000 524 713 045 579 651},
{2 258 378 774 777 406 325 860, 233 159 506 509 377 278 451},
{5 784 086 934 992 950 233 350, 689 850 758 330 840 710 021},
{20 957 188 599 351 739 701 378, 646 193 633 852 831 795 713},
{22 040 392 968 828 656 846 398, 2 504 634 079 738 442 351 539},
{39 603 786 156 568 621 078 787, 5 667 289 720 496 727 114 337},
{5 312 109 065 769 029 004 188, 787 497 760 244 930 852 617},
{15 829 645 219 693 470 166 349, 1 707 383 587 260 804 201 046},
{36 592 241 813 352 356 197 865, 557 352 433 196 148 371 484},
{15 248 483 429 881 469 286 241, 749 514 179 181 504 911 092},
{20 397 787 853 858 314 087 679, -690 744 174 979 198 964 764},
{25 638 454 245 894 733 564 039, -1 900 716 996 715 226 595 578},
{73 401 529 799 146 237 900 475, 11 512 549 475 338 179 894 688},
{341 772 402 822 255 524 055 413, 31 266 120 286 933 029 613 911},
{170 238 706 386 616 334 111 032, 29 684 084 781 340 629 726 311},
{621 398 381 812 768 095 499 886, -63 960 030 311 950 916 796 709},
{1 437 951 783 232 544 724 909 116, -225 714 784 310 788 588 549 149},
{6 609 383 112 057 242 295 523 538, -847 863 254 886 220 191 695 705},
{13 708 311 235 569 019 805 326 058, 1 563 053 644 751 642 402 088 241},
{28 374 553 808 465 183 263 980 769, 1 510 467 448 745 361 321 931 589},
{25 621 889 698 037 866 364 834 338, 2 944 621 120 765 514 042 626 563},
{69 496 330 719 289 041 485 573 591, -3 023 267 050 166 244 459 464 208},
{3 066 103 328 231 905 486 152 247, 225 397 444 528 819 527 241 868},
{7 067 410 718 553 863 723 478 495, 354 163 602 051 540 080 375 143},
{1 253 044 475 678 092 837 924 835, 79 754 899 631 450 489 465 388},
{1 819 679 555 584 084 488 188 467, -288 784 361 929 575 358 687 299},
{6 870 897 336 523 954 549 109 167, -113 911 366 705 413 623 416 968},
{2 861 011 401 731 834 383 195 873, 453 204 256 247 118 357 833 235},
{11 201 083 275 680 814 659 520 577, -1 202 974 325 499 075 378 451 278},
{29 570 833 348 941 764 023 266 925, 2 661 072 640 937 607 255 167 613},
{23 623 709 591 618 653 097 431 378, 2 096 866 788 924 358 527 706 755},
{44 095 818 162 606 034 119 908 767, 3 781 751 424 318 628 818 282 475},
{101 530 715 408 183 424 258 993 707, -592 210 942 708 962 364 739 069},
{20 748 892 191 117 931 200 419 732, -1 084 572 812 558 406 195 740 459},
{11 218 691 448 148 865 026 729 869, 802 078 085 387 920 679 269 438},
{821 738 035 279 934 160 338 777, -17 527 798 116 631 934 903 932},
{163 409 619 939 575 631 536 133, 5 022 424 635 480 500 010 619},
{184 101 049 471 188 636 329 226, 8 716 841 239 911 672 848 255},
{82 743 291 210 437 014 753 809, -9 974 291 886 996 691 073 812},
{232 967 533 042 615 406 901 727, -18 291 513 197 768 706 206 455},
{380 948 943 741 844 128 792 852, 46 609 369 394 173 393 475 425},
{637 845 098 488 101 498 166 708, -64 190 522 904 341 094 547 153},
{320 750 313 869 446 337 080 938, 8 068 506 972 065 680 112 053},
{157 207 236 041 288 524 693 378, -2 613 211 588 492 027 875 129},
{32 748 717 809 581 322 665 402, -2 075 134 729 812 074 615 657},
{35 821 591 525 537 823 623 690, 6 139 265 795 822 722 218 623},
{80 106 256 702 482 265 355 792, -14 504 490 149 086 560 016 945},
{546 734 051 170 930 484 924 362, -58 344 327 636 616 244 444 117},
{1 709 173 092 869 358 509 257 411, -217 276 087 691 673 470 841 516},
{2 293 813 084 458 311 340 502 643, 324 157 902 505 234 861 143 904},

```

```

{1951913586811717687129885, -186434368307120214740444},
{6918022395500727638310155, 508848154587206947732354},
{16262289728893400765481279, 1588904837805086007532637},
{29486066716560714522237811, -4364507906602365578830009},
{84173601742811717836207908, 4905251761372475794022323},
{61961422158890717688444943, 844242004968324178353936},
{26208707900041160820001585, -651308236722081637384901},
{12353896061473730643838055, -1568631161675840804238324},
{15417105322706667415414423, -585900200859890528899010},
{14512307927611579459172877, 1659610323291714531460753},
{33510613579094254593938100, 4205793722373124362274613},
{10723159791368484036445516, -1604321133633443445247883},
{40059963381183986342883535, -5608636044084808781019808},
{63161374734635665183845441, -2551646485430887165136503},
{49753204689784601620803586, 677891386492137728867991},
{21103544592825245661779197, -674676066406244347798040},
{14898336204301999523156603, 1390685681091251735542370},
{31537296728439795856947893, -5671327716047029909576343},
{196762895859548304440303035, 14658384763140616367762387},
{490107621158903041091968316, 78534850950777944319019877},
{1492982720884594639050075266, 175626795210372919468722057},
{6925016444692169257305436513, -1164043600349023393607671688},
{4680367434755717242906895585, -818472063913901302363537738},
{18206730949487555130672136597, -2175542081832062782836463168},
{63389149291653176570454068987, -8981782614029227644053045913},
{40817008482438061904537060084, -5338262437890270261405653779},
{149238190634043914749945441692, -16546384205379892665248825795},
{25337890064365580253774753423, 4312008195125918150215758988},
{42198569404804363154064239895, 144862461826943250587762138},
{3443848039946301409011161223, 66358048556558976788739545},
{534868314586465336260314243, 59003914933136508269652556},
{302813334870704184841857881, -7382389554591759828877178},
{10693687462920516773593057, 1695320469270631476875081},
{41219407136441505075063109, -2250255872066098448279632},
{56469313700886907476348907, 8792961751480537159669385},
{293211912168291076948275163, 48835462958321329424009537},
{15731619050684931933217339, 369621177403993986800371},
{12805234637257950436690506, -996138497410672096670473},
{11420700497382158782025797, -960830528070442197161926},
{8632001317588659129467885, -143412548785784830659086},
{2152622844883973903895275, -266744834799869913441444},
{1474469152316153112734117, 36330345361785325496637},
{1190925593846573377612000, 190129242379141509249677},
{3961861026166221447001102, 476669672152125817682463},
{1173178826698797753770442, -1102548275727150749390301},
{31303178514843775736306651, -4827007932033014479471829},
{184949342889009419898578483, 26023153909741717670493307},
{220193976144574300204901386, 35061656276983447253104103},
{776099040131215718215864672, -79100314093656506025038583},
{1177423963622598020727171482, 197859886427031109962457909},
{769093040227502484758501788, -103039899091578406150499471},

```

```

{3 777 285 980 329 837 694 695 433 789, 179 439 877 808 239 570 781 497 225},
{714 835 162 187 729 954 435 373 056, 5 726 752 091 620 919 006 708 551},
{79 699 091 925 908 790 852 469 701, -13 563 985 013 111 791 139 794 264},
{133 100 634 068 194 522 917 374 757, -3 359 165 426 296 419 213 026 498},
{100 012 655 709 317 402 691 127 877, 8 379 522 993 981 260 281 005 253},
{42 787 997 258 159 933 793 877 561, -2 288 890 443 015 772 820 391 325},
{55 372 771 572 040 233 691 051 506, -2 118 077 537 228 643 307 622 579},
{23 917 692 723 545 107 736 291 708, -509 787 584 438 082 533 870 689},
{3 343 575 858 536 937 094 823 325, -230 604 837 237 667 162 771 544},
{9 093 542 839 558 148 465 715 011, -1 527 102 246 384 167 535 804 171},
{5 456 580 461 001 683 179 691 185, 458 166 044 818 491 877 103 409},
{3 271 554 068 797 328 298 428 117, -166 610 707 070 027 662 910 301},
{4 792 145 735 654 771 822 454 337, 848 251 120 077 518 534 999 470},
{23 491 517 800 016 811 615 856 157, 1 975 909 989 874 773 644 897 926},
{17 332 764 199 957 297 710 597 445, 2 969 617 698 235 171 169 306 221},
{38 310 417 166 844 615 113 950 599, 4 476 602 640 110 025 108 069 874},
{156 341 520 937 503 257 835 583 093, -9 304 461 187 355 694 127 501 588},
{144 911 220 555 939 844 223 568 337, -9 681 180 701 578 350 696 599 166},
{24 212 707 451 097 881 808 113 087, 427 295 892 561 638 835 966 532},
{11 309 515 568 327 015 516 359 723, -543 620 931 966 080 702 173 044},
{8 415 396 233 893 659 112 661 879, -302 691 576 715 391 613 655 130},
{4 737 465 216 847 179 504 859 119, -434 338 579 230 326 812 039 696},
{3 180 473 220 226 818 778 625 423, 454 798 667 920 443 558 427 367},
{246 278 962 086 604 298 925 534, -37 832 860 612 822 210 323 095},
{1 465 533 914 048 942 693 554 349, -239 088 834 935 349 544 962 289},
{2 449 071 450 510 788 478 668 585, -8 467 157 853 750 969 626 296},
{162 963 631 363 902 276 854 239, -10 862 452 660 442 723 053 305},
{2 120 475 123 653 053 318 456, -334 469 014 161 476 258 983},
{8 979 222 056 051 465 400 082, -53 691 144 023 207 082 201},
{1 011 279 329 894 731 128 685, -158 080 045 726 786 961 594},
{4 961 125 387 186 739 370 559, 259 884 660 987 729 935 637},
{1 842 029 445 169 776 883 024, 245 247 492 743 248 608 603},
{9 476 089 245 320 746 878 200, 1 496 834 512 344 245 449 563},
{39 111 491 529 166 660 284 938, 3 390 862 743 971 780 564 773},
{124 730 050 481 081 812 894 702, 6 843 726 564 308 265 049 745},
{121 894 813 559 110 317 944 068, 3 700 029 990 854 323 176 239},
{16 287 914 987 505 402 873 701, 673 924 358 523 373 931 918},
{8 984 700 252 609 852 105 851, 469 126 637 131 713 063 106},
{5 632 237 621 477 008 640 123, -154 540 456 607 307 383 540},
{5 433 713 505 501 483 781 957, -240 770 123 151 230 412 818},
{8 215 946 831 168 441 315 703, 924 956 834 981 268 575 504},
{8 584 510 009 375 093 242 807, -592 245 960 315 316 288 205},
{23 152 258 631 892 551 427 023, 4 206 151 438 245 759 412 843},
{164 687 349 808 978 398 952 765, -30 011 713 972 024 261 359 522},
{1 155 673 615 959 710 280 257 245, 174 482 307 311 217 387 594 732},
{5 190 500 282 286 103 199 564 441, -446 487 628 167 452 740 090 391},
{13 220 749 202 143 044 840 099 829, 1 300 217 713 392 841 118 529 936},
{17 267 193 388 956 058 729 237 051, 1 299 759 706 444 432 536 447 328},
{29 255 059 209 096 424 678 321 173, -4 710 972 692 636 198 692 979 318},
{78 148 621 209 059 369 115 175 935, 770 248 368 010 963 462 498 783},
{27 929 347 156 212 692 821 109 308, -665 649 878 792 222 549 596 391},

```

```

{2 207 872 491 791 686 693 190 006, -95 174 094 747 702 337 115 001},
{1 490 596 694 968 102 224 053 657, 141 781 428 311 888 823 178 019},
{5 450 922 300 551 311 641 459 608, 805 096 027 866 203 546 328 547},
{14 595 241 666 456 941 444 377 459, 690 377 088 785 307 468 441 695},
{7 688 501 355 273 283 961 047 256, 914 926 131 057 271 493 766 841},
{29 158 292 238 393 848 862 089 712, -2 646 573 929 943 290 207 662 745},
{3 632 341 712 394 869 646 161 843, 263 087 591 870 472 315 844 046},
{4 019 881 329 547 679 276 729 279, -124 782 798 319 746 035 830 428},
{2 119 710 881 948 684 282 291 057, 257 741 242 798 974 238 050 979},
{4 564 694 224 994 339 852 774 775, 253 791 215 321 113 302 665 041},
{280 264 412 070 268 020 481 077, 12 459 182 763 259 922 632 526},
{486 828 911 005 428 082 674 895, -87 980 644 170 117 838 428 316},
{3 243 341 367 207 036 883 705 079, -193 091 109 219 227 697 893 210},
{3 097 391 672 066 884 457 879 789, 472 974 079 341 577 492 795 483},
{16 860 723 782 608 481 343 398 768, -228 674 569 581 131 377 028 149},
{4 834 354 945 224 003 978 056 382, 318 924 742 289 617 346 788 951},
{3 988 221 059 499 758 321 547 243, 306 535 877 166 088 718 823 448},
{257 117 850 907 793 170 551 101, -40 619 410 407 883 619 496 415},
{1 058 709 688 378 824 832 236 269, -99 811 299 388 788 711 371 033},
{3 097 953 786 930 228 434 762 426, -75 472 142 549 443 349 242 475},
{284 079 449 841 038 149 855 129, -18 206 469 162 530 138 123 522},
{570 700 483 996 080 749 576 617, -28 172 458 327 263 292 850 031},
{572 854 078 614 376 513 503 763, 87 546 058 956 150 596 590 594},
{3 157 498 392 215 535 347 801 205, 38 351 472 154 016 167 031 804},
{1 001 536 371 310 562 444 268 883, 88 545 564 166 638 118 672 252},
{2 175 278 072 725 907 971 054 769, -191 578 620 474 347 871 035 063},
{5 365 146 553 138 429 783 857 004, 621 162 404 401 400 591 455 655},
{17 799 891 831 459 867 600 267 389, 3 201 270 114 298 078 379 585 967},
{111 210 579 491 959 611 502 624 627, -7 955 518 376 371 326 146 067 531},
{13 167 544 401 877 408 843 343 753, 110 731 542 476 140 989 892 559},
{751 223 069 886 147 355 790 672, 76 701 927 351 250 990 560 543},
{1 247 900 086 482 641 435 365 882, -104 283 493 610 146 974 119 131},
{276 645 110 290 658 071 031 510, 12 581 260 103 436 159 803 539},
{11 266 346 810 058 127 061 492, -1 340 133 006 841 885 897 501},
{43 077 337 670 520 150 637 236, 4 821 891 790 068 110 038 673},
{25 255 386 767 334 337 154 859, -819 896 144 994 276 888 998},
{12 750 104 471 571 465 922 241, -754 057 905 680 165 825 232},
{5 441 514 074 316 895 429 537, -354 960 193 744 102 638 282},
{9 251 782 284 273 112 569 253, -872 064 293 741 549 993 054},
{26 933 070 803 831 050 992 939, -314 685 011 856 833 479 957},
{10 257 377 052 673 634 385 677, -1 497 447 882 205 696 606 086},
{17 755 891 698 533 106 697 075, 974 642 610 271 782 565 944},
{16 773 652 377 640 620 296 557, -3 049 650 831 193 909 591 715},
{120 415 956 152 304 143 044 907, 19 905 787 283 507 455 954 200},
{77 517 363 649 493 178 256 853, 7 491 435 638 334 345 449 135},
{205 637 574 025 828 177 474 737, -12 074 270 318 322 623 115 031},
{29 623 310 533 143 177 017 590, 3 078 068 657 340 466 936 471},
{91 432 707 180 657 895 422 480, -8 220 087 756 813 941 515 849},
{79 927 606 600 658 561 103 139, -3 895 628 848 805 658 438 113},
{148 567 338 716 561 021 681 486, -19 469 585 965 639 284 307 789},
{567 958 571 675 706 969 685 254, 78 659 442 549 193 145 807 653},

```

```

{1 370 055 432 677 040 973 502 957, 178 915 068 074 736 255 778 903},
{4 839 943 841 747 076 745 533 093, 79 215 587 732 820 666 424 607},
{615 646 213 556 271 396 933 214, -69 876 485 660 235 381 693 639},
{1 046 130 433 481 916 026 453 423, 143 926 468 504 697 600 125 459},
{3 052 967 161 973 593 220 441 590, 163 096 366 651 590 993 100 361},
{3 623 240 548 124 216 228 756 251, 415 890 312 448 649 599 999 491},
{9 462 008 849 176 783 527 894 272, -1 594 773 801 985 843 706 536 941},
{8 424 083 056 324 018 194 862 546, -800 651 338 931 734 951 829 347},
{30 263 452 082 080 235 745 561 409, -3 404 755 139 354 470 700 768 741},
{29 968 189 596 690 044 347 223 540, 4 952 112 220 442 794 656 077 579},
{20 185 785 648 628 836 449 887 214, -1 511 647 774 165 065 505 018 701},
{42 214 802 174 155 805 886 883 979, 4 552 409 441 012 318 340 954 053},
{98 206 259 198 550 324 645 502 658, -863 643 623 059 688 370 905 393},
{19 679 992 590 077 821 379 259 376, 3 209 136 525 382 325 858 656 463},
{33 588 701 584 925 431 958 327 242, -5 408 838 105 170 789 604 383 605},
{89 718 163 358 154 852 230 023 348, 850 493 312 069 384 427 350 929},
{32 892 881 678 689 501 295 888 437, -5 258 641 157 809 430 561 866 331},
{105 941 743 814 800 516 050 545 629, 12 357 427 987 755 803 588 813 720},
{416 733 537 925 135 583 653 450 229, -58 368 005 982 409 856 228 937 806},
{644 442 187 813 060 614 019 961 373, -116 292 150 015 487 524 048 128 237},
{4 211 546 270 109 297 891 235 835 871, -88 984 085 472 913 866 970 469 803},
{2 314 245 977 705 345 346 276 655 270, -233 476 083 655 890 169 955 924 277},
{1 620 673 849 430 951 909 324 412 500, 1 752 499 468 161 825 471 855 383},
{30 664 530 880 195 519 203 525 225, -3 368 258 664 429 266 924 337 557},
{27 666 029 126 237 233 874 489 748, -2 039 447 639 495 956 119 309 155},
{70 012 788 309 785 991 871 235 338, 6 910 981 673 310 120 949 537 817},
{71 334 754 558 097 807 692 716 272, -3 942 138 009 532 911 883 527 769},
{29 725 360 533 926 109 348 097 970, 5 014 492 297 936 137 932 323 879},
{28 565 867 041 566 741 421 779 016, 2 330 874 030 216 610 267 938 567},
{47 034 915 638 426 038 314 780 748, -5 786 750 203 494 196 711 524 835},
{58 532 206 827 324 705 183 983 372, -5 936 633 698 310 585 057 982 553},
{65 896 282 306 710 486 271 530 482, 9 388 346 331 125 106 471 592 629},
{14 050 781 117 944 536 660 184 241, -1 055 601 214 994 881 059 744 213},
{25 909 260 517 875 547 797 248 288, 2 206 453 321 297 028 876 179 365},
{44 886 167 677 415 098 635 423 268, 6 939 396 340 261 509 474 235 513},
{256 733 381 231 837 301 410 805 010, -17 251 085 756 552 022 997 167 533},
{160 599 504 199 000 440 189 930 815, 6 888 062 100 099 771 122 009 112},
{171 751 995 839 750 646 313 977 881, -23 276 903 132 306 925 512 523 531},
{696 280 239 174 571 250 378 739 956, -49 699 542 991 007 067 047 786 657},
{38 444 346 737 312 625 068 413 882, -2 993 979 881 781 292 958 022 907},
{37 713 946 341 690 487 484 828 811, 1 170 289 819 539 734 443 042 516},
{20 909 097 197 099 839 289 995 621, 346 999 229 832 134 001 390 712},
{7 042 329 166 572 137 317 679 179, -1 023 807 731 065 360 780 509 171},
{9 821 671 119 945 663 524 916 422, 1 561 492 089 285 864 585 583 025},
{35 764 768 154 207 604 902 043 488, 5 198 324 569 429 063 280 889 983},
{49 256 802 711 871 207 070 725 047, 5 209 414 822 927 989 622 015 474},
{187 393 475 136 024 737 334 276 699, -1 196 288 149 047 102 090 703 448},
{33 477 376 885 252 981 587 006 323, -3 806 545 559 186 425 064 623 392},
{61 741 118 646 562 675 573 732 195, 6 079 102 596 561 394 139 462 683},
{75 057 321 794 950 000 149 323 835, 11 853 413 420 624 186 718 607 012},
{311 010 460 425 185 507 176 859 277, 23 072 485 309 778 628 427 784 932},

```

```

{874 383 960 447 003 671 636 757 719, -103 132 003 790 509 099 328 988 386},
{3 896 906 479 711 539 283 383 199 849, 435 631 541 939 753 751 853 927 300},
{1 878 414 421 953 314 180 869 522 229, 62 334 918 813 954 391 651 227 250},
{660 981 745 239 912 075 283 673 591, 71 681 216 186 586 767 478 209 930},
{1 252 213 165 289 862 270 402 953 459, 146 737 831 640 708 173 813 675 562},
{5 405 758 238 644 392 219 690 001 321, 314 064 889 297 019 410 821 658 828},
{5 265 754 527 009 916 622 022 298 355, -317 854 209 873 929 412 208 021 953},
{10 883 596 226 903 787 455 611 912 834, 1 139 017 472 682 714 484 984 711 083},
{40 019 701 493 945 234 144 580 641 684, -1 837 721 355 270 257 716 867 724 253},
{32 403 297 438 034 414 494 234 058 678, 2 441 411 010 198 761 607 316 641 051},
{52 531 390 130 590 574 330 300 276 185, 34 721 225 053 223 233 874 388 679},
{144 046 619 958 103 210 333 816 218, 6 672 624 552 575 171 814 368 495},
{217 338 495 685 494 997 000 963 088, 31 340 060 652 327 051 869 895 311},
{161 312 381 582 754 920 976 023 031, 11 204 585 273 700 797 832 650 833},
{351 406 832 324 556 354 193 998 151, -17 819 876 819 218 488 959 592 100},
{394 265 620 725 260 574 829 664 071, -39 533 908 627 632 621 566 940 310},
{84 803 778 534 185 626 339 383 291, 10 128 683 492 618 668 545 100 390},
{298 170 536 865 665 960 307 833 509, 33 980 945 489 910 385 411 156 097},
{604 979 830 938 673 163 013 137 756, -19 520 248 555 347 526 866 496 991},
{11 682 067 890 913 418 013 248 235, -1 707 817 053 318 593 474 732 311},
{21 539 467 103 022 168 480 357 418, 500 366 430 017 883 734 027 163},
{1 873 138 368 000 265 457 963 311, 335 305 916 926 247 874 052 800},
{10 957 073 551 020 521 121 925 631, 1 666 350 674 942 440 579 587 067},
{55 883 112 712 548 471 879 523 202, -8 557 379 118 130 855 065 390 481},
{317 464 748 035 033 572 678 603 035, -23 193 203 567 609 812 442 720 711},
{571 968 051 008 800 320 039 466 601, -57 403 517 061 317 013 611 149 690},
{163 302 448 745 215 469 690 393 621, -21 053 760 187 030 547 473 953 486},
{405 082 987 331 283 897 997 507 093, 27 532 207 197 190 928 148 594 221},
{624 109 529 499 821 914 281 091 538, -113 112 885 040 696 999 341 919 517},
{4 310 854 678 804 446 459 863 619 556, -558 875 931 303 591 280 042 406 293},
{12 652 068 958 318 418 657 574 832 252, -2 293 105 198 058 585 214 582 831 373},
{87 418 416 172 614 317 763 850 322 894, -11 386 517 379 129 885 654 411 463 097},
{290 224 105 973 556 630 243 869 168 678, 47 231 169 332 714 913 324 104 988 039},
{540 130 108 204 104 873 639 899 995 076, -35 974 200 189 721 662 276 527 429 563},
{40 851 323 304 115 219 867 095 578 849, 7 288 709 134 455 281 011 252 551 333},
{227 593 588 706 700 829 833 158 602 771, 9 021 073 409 175 438 796 253 461 940},
{163 273 524 707 873 934 218 942 287 409, -6 565 410 780 711 589 630 051 393 048},
{68 077 839 983 348 716 055 060 564 489, -6 135 137 562 510 597 422 546 072 927},
{46 714 816 862 839 408 157 247 221 068, -4 518 509 303 835 937 853 484 780 129},
{120 848 182 133 922 340 169 554 162 462, -2 066 307 723 672 218 028 632 241 695},
{79 184 398 713 761 866 201 847 388 008, 11 167 833 832 357 620 283 893 988 543},
{79 755 389 093 423 412 952 567 988 353, 3 940 030 841 335 935 734 787 754 807},
{75 427 009 069 671 162 288 218 484 827, 6 690 083 386 740 179 124 920 013 806},
{145 051 253 426 806 161 213 768 303 919, -3 950 038 950 991 504 219 835 468 016},
{86 914 833 030 480 098 691 377 001 167, -7 001 373 236 724 693 474 761 701 906},
{228 969 980 992 918 382 544 689 685 305, 35 257 414 824 855 945 323 850 943 311},
{1 376 613 871 458 834 137 525 138 009 681, -246 699 844 454 571 964 091 395 904 817},
{8 183 230 426 219 214 114 835 756 118 459, 1 465 463 735 175 194 581 176 965 536 089},
{48 154 606 801 724 316 405 856 930 747 925, 7 967 417 842 046 162 648 905 253 558 194},
{27 657 880 206 339 900 481 607 342 502 119, -53 339 984 671 392 077 371 067 874 952},
{2 020 175 210 894 426 244 173 883 239 551, -235 641 042 550 281 159 663 557 925 398},

```



```

{7 946 939 592 590 231 231 052 909 033 449, 1 112 256 423 362 082 066 545 048 615 048},
{12 730 425 695 396 884 453 767 929 520 927, -922 433 164 062 394 388 841 528 601 471},
{14 507 449 516 654 322 211 064 201 073 693, -1 685 052 238 585 461 226 988 425 748 593},
{51 983 629 818 571 477 714 698 822 427 876, -459 061 166 558 815 929 735 390 580 885},
{8 667 721 796 596 934 713 375 256 241 809, -1 265 790 979 482 886 631 795 770 559 066},
{15 232 389 722 878 465 026 415 876 060 587, -651 973 827 719 788 287 995 990 436 652},
{18 722 343 140 543 417 798 139 585 389 689, -3 396 620 269 226 391 042 539 752 924 535},
{130 932 899 510 379 348 110 815 640 444 159, -20 050 853 348 912 659 174 573 714 370 389},
{744 422 840 628 732 022 784 828 451 736 556, -55 597 449 605 512 228 557 539 230 589 405},
{1 710 823 664 808 771 071 408 657 871 868 989, 3 968 619 850 363 405 928 546 960 518 078},
{27 532 234 869 306 180 188 513 197 612 309, 211 105 552 047 600 134 028 049 871 633},
{6 992 535 146 334 858 424 470 429 701 501, 1 276 058 669 200 089 501 407 651 655 701},
{48 367 102 226 418 462 477 141 542 416 684, -5 721 438 391 380 429 021 993 346 800 925},
{205 052 012 534 627 393 794 386 672 733 436, -360 086 323 798 620 329 584 763 657 659},
{12 868 649 163 781 674 591 835 970 511 735, -103 212 561 128 836 683 025 963 524 151},
{2 600 757 208 509 952 126 348 130 564 060, -438 582 752 101 617 293 820 553 455 611},
{2 428 405 023 880 379 289 440 023 398 874, -118 115 520 791 334 754 716 358 831 117},
{4 109 652 106 274 394 208 677 452 312 057, 279 487 326 164 248 251 581 250 160 801},
{6 529 965 108 957 035 638 262 707 896 682, -505 816 571 560 595 399 139 436 614 241},
{3 606 375 385 125 659 493 447 478 987 629, 243 729 595 574 077 553 543 255 572 669},
{3 915 915 330 354 800 966 407 013 590 074, -567 295 271 317 190 472 506 505 133 789},
{4 356 973 940 377 054 949 943 265 369 471, 33 252 515 245 786 323 533 760 252 743},
{70 661 011 144 678 794 633 108 550 902, 7 124 632 989 724 755 618 010 022 495},
{46 240 181 452 932 162 212 342 249 792, -2 695 959 979 950 893 351 759 713 169},
{32 300 081 707 591 043 361 742 947 601, 445 017 930 240 496 537 942 389 367},
{14 711 948 797 251 108 736 066 619 010, 2 647 705 103 937 166 837 000 906 577},
{92 768 264 283 379 490 589 166 815 708, -4 843 665 422 326 922 369 716 860 935},
{58 351 079 474 269 279 599 170 177 497, 2 910 728 921 851 157 485 619 032 381},
{10 783 581 942 444 261 056 372 860 283, 352 840 178 250 971 783 914 304 985},
{12 202 623 083 533 275 352 676 945 908, -997 710 581 386 392 304 346 693 967},
{18 177 592 444 828 848 340 812 846 016, 1 254 309 270 480 567 736 394 346 399},
{48 763 749 989 971 102 472 067 717 970, -8 313 270 141 591 754 269 654 013 299},
{88 153 797 906 774 428 522 652 584 096, 9 543 242 629 683 162 705 977 192 701},
{178 904 524 930 451 169 339 770 133 173, 31 504 225 304 287 283 906 544 141 326},
{799 545 324 726 530 193 860 082 467 857, -140 801 959 335 467 517 534 213 335 098},
{3 576 048 071 615 717 996 270 605 875 749, 621 542 729 086 154 453 117 023 559 150},
{12 103 455 929 195 489 072 091 302 852 929, -228 426 972 320 619 340 585 043 323 681},
{250 714 699 989 542 334 363 470 870 956, 6 966 829 271 223 747 712 493 070 623},
{7 201 148 186 494 079 616 094 046 288, -539 944 566 773 686 447 974 260 113},
{14 367 636 656 456 307 601 864 520 701, -462 054 897 933 085 546 516 310 919},
{3 470 850 821 921 797 128 851 694 748, 446 847 129 567 651 766 531 377 691},
{8 210 170 954 933 943 268 546 815 620, 865 399 451 712 627 626 986 881 851},
{33 304 495 272 103 275 427 525 437 919, -4 987 648 091 233 682 333 725 272 985},
{127 114 267 956 067 571 775 566 365 104, 20 726 602 171 920 693 580 354 835 383},
{217 617 739 038 929 413 181 550 871 674, 39 701 715 346 556 822 654 367 367 777},
{1 509 623 822 185 478 692 867 408 590 331, -188 558 728 891 293 194 595 219 650 903},
{91 165 293 355 517 752 346 459 265 453, -3 885 015 919 040 929 591 253 425 502},
{142 984 250 188 533 368 062 807 833 653, 8 011 078 254 055 246 378 682 715 160},
{95 997 512 372 424 273 525 002 098 933, 1 437 494 618 312 381 401 167 978 854},
{24 855 537 305 917 147 906 946 258 515, -4 071 859 878 840 567 760 405 798 286},
{33 525 864 597 025 566 216 406 035 121, -1 695 893 641 603 879 310 410 590 148},

```

```

{30 968 650 569 109 579 352 655 659 281, - 2 443 268 111 396 491 625 970 586 280},
{62 712 955 444 540 131 011 995 026 361, 8 848 488 861 926 504 340 501 048 832},
{61 109 139 473 313 449 650 527 078 423, 3 624 083 554 107 877 889 154 458 965},
{39 522 194 775 117 482 742 799 194 578, 3 860 348 207 352 836 514 057 651 325},
{72 578 303 425 540 290 575 591 824 912, 11 898 156 573 945 569 501 519 111 043},
{93 959 754 567 483 011 751 695 533 666, 8 682 371 539 937 988 068 394 546 315},
{122 160 257 374 953 703 050 913 588 121, - 13 252 769 906 938 262 122 822 186 320},
{227 940 928 788 238 171 695 598 988 039, 40 799 913 467 899 959 755 791 818 577},
{1 331 825 609 513 765 360 293 001 950 417, 199 092 895 925 705 307 640 286 787 286},
{4 884 148 295 327 571 661 931 439 286 215, 407 897 995 040 118 718 747 795 117 091},
{839 583 967 154 384 080 326 067 391 283, 137 237 885 312 893 682 125 137 730 276},
{1 276 375 766 884 737 018 444 039 760 533, 65 303 869 944 935 175 200 127 270 595},
{2 346 428 929 103 352 359 121 946 457 993, 9 078 244 780 289 646 369 928 960 853},
{335 100 287 301 264 058 741 690 075 601, - 20 887 649 577 623 585 143 385 170 519},
{70 933 630 683 649 019 354 660 436 463, - 9 671 870 315 468 816 694 964 959 382},
{255 212 539 554 016 896 702 551 942 331, - 14 592 828 636 822 341 244 104 568 130},
{563 621 765 514 930 548 669 168 445 559, 88 561 312 369 489 667 898 464 554 784},
{2 548 057 412 541 410 760 992 108 231 545, 448 803 743 697 197 884 467 333 106 371},
{11 436 438 921 700 347 119 139 342 127 799, - 1 870 004 235 186 474 244 560 741 053 317},
{17 096 667 335 938 630 490 216 768 823 863, 2 893 468 784 993 684 315 028 939 084 269},
{20 867 484 547 854 556 596 592 388 858 329, 1 222 441 385 922 537 075 186 955 466 119},
{6 792 497 986 542 679 154 717 528 810 174, - 671 627 003 002 737 186 629 569 876 685},
{6 022 008 564 709 275 785 324 573 422 596, - 3 875 502 562 365 002 142 310 104 611},
{41 270 959 269 065 962 201 002 288 942, 3 162 722 983 059 750 551 595 383 429},
{12 289 278 653 847 197 390 722 044 835, 1 736 135 245 438 270 307 659 828 716},
{10 770 222 926 565 113 731 156 262 017, - 1 222 230 426 371 461 354 666 011 781},
{18 158 221 951 465 038 406 189 676 948, 3 236 733 907 461 831 918 450 261 827},
{99 712 337 971 170 295 256 439 627 106, 520 864 451 623 758 658 343 800 509},
{17 950 989 171 558 929 509 124 661 073, 1 610 669 958 640 810 786 531 239 873},
{18 455 950 494 290 857 725 200 775 130, - 1 481 487 474 391 930 225 875 431 003},
{53 569 963 325 427 906 160 952 644 426, 952 028 999 296 444 712 875 889 119},
{20 250 809 821 333 176 952 325 447 198, 871 875 144 588 482 745 367 649 421},
{15 616 838 168 047 830 900 691 330 685, 84 975 884 760 451 397 454 645 039},
{1 479 245 602 142 872 246 105 162 789, - 196 924 395 496 932 023 668 899 213},
{7 595 815 384 774 131 516 436 442 285, - 1 172 996 514 611 976 254 966 341 383},
{44 069 067 471 079 644 944 433 124 973, 4 396 791 041 449 549 532 739 584 481},
{7 991 407 470 147 819 745 945 132 877, 1 187 044 643 554 423 584 854 456 213},
{25 114 497 743 918 482 494 848 788 506, - 1 584 066 768 187 312 273 044 462 767},
{18 215 073 219 202 596 035 146 645 514, - 1 903 096 753 463 474 927 788 728 473},
{64 455 650 919 140 106 176 510 498 064, 8 379 032 638 419 855 058 438 325 783},
{203 552 204 869 280 008 988 692 547 800, 10 551 680 689 921 100 333 356 503 343},
{242 551 469 101 549 109 738 599 758 357, 32 241 844 940 421 133 401 308 866 234},
{1 215 279 943 323 776 640 277 822 549 685, 129 586 783 103 403 061 402 183 411 124},
{3 870 912 736 058 777 924 995 576 115 951, 290 580 100 359 577 056 163 604 016 289},
{7 376 343 079 357 819 394 629 188 431 326, 1 293 655 847 254 510 227 380 771 513 823},
{30 461 768 329 370 115 602 779 811 477 348, - 1 559 298 844 934 153 883 010 939 521 285},
{57 212 476 975 724 002 537 679 336 919 808, - 2 827 682 310 657 241 236 518 114 831 733},
{52 047 630 243 755 046 778 046 182 526 692, 5 886 202 835 631 819 261 398 947 524 597},
{73 327 426 877 574 799 389 003 270 379 799, - 7 409 752 487 769 720 400 154 673 465 430},
{60 837 742 009 669 964 390 933 677 685 579, 4 716 554 441 514 833 754 447 140 795 216},
{37 719 792 671 807 078 933 453 059 526 091, 1 247 865 728 238 801 815 052 403 873 243},

```

```

{22 421 845 146 798 934 068 594 522 975 279, -188 254 444 907 176 305 428 372 436 551},
{1 545 730 024 751 344 086 838 039 031 090, -119 184 202 571 821 274 716 341 102 189},
{289 504 085 904 266 273 477 228 491 993, -42 803 005 926 261 725 823 315 431 296},
{799 239 490 785 698 775 592 382 639 241, -139 263 073 514 224 595 478 956 351 108},
{2 870 777 073 672 254 985 227 081 925 153, 463 487 220 725 591 831 244 466 189 502},
{7 098 446 196 177 615 823 062 498 263 139, 134 868 213 927 931 577 637 204 985 412},
{3 915 962 218 217 865 545 039 911 132 063, -592 053 073 746 762 916 337 903 217 057},
{18 044 334 542 748 514 676 707 499 599 544, 405 105 330 070 871 917 635 842 518 295},
{14 647 019 524 817 007 735 527 684 174 749, 257 202 941 086 679 848 310 428 983 889},
{1 070 301 252 775 745 835 174 664 646 996, 111 528 276 757 668 178 962 113 914 161},
{3 553 539 669 273 940 401 271 485 074 506, 320 513 640 734 212 614 627 323 187 923},
{2 203 280 074 610 529 589 303 470 580 887, 247 808 161 358 921 862 092 455 235 570},
{2 132 476 831 961 606 392 761 496 600 197, -6 645 973 023 629 197 049 722 658 855},
{69 560 181 245 902 955 758 674 488 382, -11 197 882 763 102 294 553 337 335 577},
{187 457 888 715 845 886 653 387 518 680, 9 944 781 282 942 771 657 579 534 257},
{117 943 497 145 275 212 409 266 944 037, -6 314 866 797 622 494 143 247 196 337},
{161 078 788 754 621 928 681 953 122 914, 25 832 970 796 072 132 832 818 073 711},
{480 396 154 276 941 403 118 529 771 192, -75 370 771 520 119 332 602 921 042 335},
{2 225 550 487 341 807 192 579 277 857 378, -235 471 343 375 669 552 927 048 356 519},
{8 398 363 359 901 716 082 631 569 247 853, -104 575 055 501 963 056 200 199 289 983},
{2 556 354 659 829 055 342 634 457 887 827, 184 248 668 704 202 666 862 654 935 936},
{1 827 009 460 352 777 481 974 186 006 883, 199 191 067 368 901 134 300 015 407 782},
{2 708 898 468 580 714 588 649 739 610 755, -174 397 949 014 425 189 456 747 081 302},
{6 436 028 536 356 986 969 998 881 516 083, -398 118 550 975 799 055 446 162 650 540},
{5 224 405 938 791 964 545 962 049 487 997, -766 247 101 778 358 933 077 343 539 108},
{11 006 578 118 867 290 860 769 067 574 961, -72 320 500 108 018 013 909 409 715 633},
{1 095 106 093 435 666 976 564 473 100 855, -85 305 914 421 008 004 094 303 244 537},
{1 095 792 728 957 529 056 256 057 171 954, -99 134 221 196 846 470 654 299 197 695},
{419 987 367 585 212 445 642 513 787 411, 31 198 002 139 371 946 225 273 402 106},
{1 138 653 842 096 794 432 402 805 242 607, -43 278 951 557 239 428 432 364 679 368},
{1 058 687 027 076 974 159 744 562 744 081, 78 650 346 814 670 668 948 644 459 107},
{2 862 368 960 414 181 609 562 597 279 510, -91 080 818 249 467 786 777 238 700 607},
{3 070 223 979 773 737 337 987 607 294 747, -433 119 167 269 596 967 935 481 787 371},
{3 032 794 902 038 126 432 699 547 868 850, 296 023 974 717 987 165 969 008 849 541},
{5 731 857 233 802 127 067 747 290 501 760, 240 799 602 937 713 521 534 158 986 379},
{3 739 325 699 536 798 476 729 488 535 544, 194 125 469 337 596 122 246 659 638 475},
{4 024 400 787 675 300 169 393 476 957 001, 562 795 262 153 168 985 029 044 129 015},
{6 701 882 255 646 264 661 023 276 257 784, 177 502 451 273 132 690 026 762 058 473},
{3 413 660 525 889 427 239 500 875 171 010, -238 418 868 821 440 874 129 656 042 757},
{5 987 912 628 751 145 133 169 555 220 548, 947 759 946 701 726 383 722 412 021 729},
{23 806 882 934 722 159 635 971 564 123 746, -3 780 083 779 708 978 533 886 136 818 823},
{88 984 040 260 994 786 179 724 713 653 832, -4 641 371 658 786 023 254 116 830 666 129},
{63 040 320 780 767 203 768 889 548 793 099, 3 593 776 199 903 942 023 058 360 160 593},
{130 164 414 582 796 459 046 713 793 708 425, 2 782 922 453 241 540 610 392 080 291 203},
{50 002 316 844 920 021 695 404 418 271 164, 412 496 599 388 767 095 490 689 379 331},
{7 128 037 191 457 048 141 449 266 396 927, 1 187 776 381 749 907 464 975 287 471 825},
{108 933 175 650 664 776 205 783 712 183, -17 801 719 114 230 050 423 894 818 376},
{167 706 016 257 473 419 330 769 352 233, 9 612 453 820 569 949 342 982 233 605},
{339 249 803 314 958 159 505 639 094 892, 12 175 424 270 561 191 083 176 169 843},
{131 304 024 599 660 075 040 199 196 248, 2 145 713 863 676 581 939 405 795 363},
{32 822 834 315 697 562 179 208 649 295, 826 955 582 687 818 216 112 117 047},

```

```

{20 175 730 353 398 150 756 806 574 215, 1 327 035 831 420 808 364 187 257 972},
{21 345 237 684 795 998 225 818 666 165, 2 973 114 135 812 324 933 658 732 393},
{42 141 659 994 668 171 526 395 613 706, 2 830 167 391 443 864 518 760 213 957},
{24 557 219 282 193 904 145 600 056 271, 1 783 661 893 536 987 898 449 942 922},
{32 709 730 958 590 188 183 232 426 323, 3 179 145 519 304 354 601 756 842 838},
{72 543 785 478 184 731 087 455 837 497, 11 482 521 217 370 408 300 487 121 079},
{288 243 995 743 020 221 478 115 770 817, -45 180 607 231 893 159 524 659 411 762},
{1 355 667 835 781 239 882 082 584 719 355, -85 716 443 932 322 943 425 755 579 463},
{1 247 826 103 738 249 805 630 859 612 187, -99 342 133 474 825 006 699 789 365 478},
{3 446 108 883 323 547 235 845 768 983 133, 257 864 674 912 476 554 129 387 682 064},
{7 415 580 647 446 810 540 934 600 187 779, 1 316 083 097 431 185 246 984 616 273 953},
{37 992 517 034 083 774 336 874 699 019 181, -6 344 223 457 582 543 494 245 902 086 670},
{72 823 711 411 486 628 600 713 500 839, 8 560 564 783 206 805 983 827 513 677},
{333 488 359 352 595 395 044 995 658 066, 58 234 047 029 847 121 427 363 691 713},
{1 257 357 903 292 499 348 015 732 884 748, 15 127 904 323 404 127 802 351 096 153},
{137 605 711 546 582 493 226 760 419 871, -17 219 295 620 965 236 346 228 622 017},
{148 653 421 139 397 543 068 556 265, -24 501 231 204 878 649 723 904 723},
{130 036 678 899 925 933 285 106 233, 21 537 053 953 978 249 988 632 086},
{64 334 058 908 458 234 911 783 643, 1 053 654 758 448 907 382 893 698},
{4 828 372 802 915 879 866 177 135, -65 984 593 603 965 581 770 453},
{908 300 116 284 999 357 791 214, 122 043 104 732 791 217 540 837},
{4 265 872 269 281 405 965 423 045, 245 686 604 840 320 894 794 353},
{7 046 798 972 680 109 559 604 476, -1 285 155 200 675 224 220 464 321},
{49 060 814 575 015 088 125 346 809, 6 530 735 805 551 278 150 538 195},
{251 620 677 682 215 829 237 741 329, 38 274 376 636 202 877 846 305 269},
{1 287 696 742 925 140 939 225 248 766, -187 482 928 070 476 420 425 289 855},
{1 950 016 531 887 326 296 390 637 301, -221 254 605 462 511 071 236 254 826},
{3 260 718 464 746 594 234 116 834 507, -475 475 183 205 530 332 346 286 601},
{5 341 017 597 677 329 292 266 564 300, 310 631 924 879 827 394 105 034 779},
{4 761 715 102 900 823 805 996 871 503, 68 322 929 079 345 587 022 686 399},
{1 650 304 679 616 015 561 702 937 733, 54 761 025 260 560 164 504 821 926},
{590 439 822 137 639 498 104 116 287, -8 753 647 957 910 407 921 440 586},
{311 687 307 653 731 222 040 164 975, -5 037 030 045 185 103 831 923 944},
{48 075 856 671 872 027 590 444 687, -7 980 909 976 435 561 870 750 275},
{15 041 348 247 433 852 909 499 923, -1 040 023 505 291 441 981 591 403},
{38 000 514 694 939 548 210 402 199, 1 535 479 245 513 822 550 608 057},
{30 530 848 989 575 228 829 138 854, 1 979 934 891 426 980 482 916 591},
{65 714 223 835 471 205 245 809 131, 11 677 198 861 060 702 292 552 603},
{343 568 577 140 547 672 251 012 473, -39 657 935 852 514 753 681 838 776},
{1 054 874 797 034 723 759 957 384 369, 35 116 768 904 919 815 420 792 752},
{108 366 661 083 214 489 354 542 911, -10 386 927 383 808 168 969 044 862},
{355 293 592 365 491 173 463 448 989, -38 021 882 667 738 207 002 137 464},
{1 034 635 220 111 937 525 092 733 227, 34 693 687 805 257 669 888 280 960},
{487 857 709 617 613 152 899 950 267, -54 496 226 695 587 294 446 621 585},
{206 058 120 771 127 272 451 875 842, -6 368 643 386 241 477 488 423 479},
{178 661 060 500 599 432 963 636 606, 21 552 691 931 721 613 193 832 407},
{492 922 478 699 295 665 625 210 650, 74 146 625 384 283 787 525 671 803},
{2 062 208 020 264 576 917 304 865 709, 198 521 160 481 857 302 114 064 835},
{6 082 716 820 234 307 796 973 171 361, 52 899 342 527 935 945 674 998 088},
{55 898 067 787 750 496 477 091 961, 6 938 890 069 413 926 592 569 292},
{30 568 831 362 687 615 186 472 375, -1 679 701 812 237 788 806 991 057},

```

```

{26 401 700 650 185 916 190 034 571, 2 988 246 250 625 848 464 846 191},
{38 908 732 830 290 879 492 910 692, 6 738 739 685 790 928 112 656 875},
{120 372 717 471 920 445 459 414 082, -2 110 996 187 251 485 205 258 941},
{3 628 849 088 277 312 012 701 155, -255 053 919 383 077 468 093 214},
{4 589 443 136 223 969 292 296 561, 67 527 854 888 035 890 499 426},
{193 628 696 835 229 671 488 153, -3 783 882 779 841 229 369 429},
{51 403 330 002 830 918 134 646, 2 986 489 776 258 652 150 245},
{50 007 300 708 272 694 857 999, -2 709 742 701 120 985 971 982},
{97 322 634 959 500 841 623 517, 286 509 939 962 949 257 624},
{7 168 825 604 250 571 522 797, 1 050 062 625 324 466 463 527},
{14 347 409 068 634 804 029 468, 1 313 379 280 969 036 339 255},
{7 881 278 739 943 060 484 623, 395 631 797 124 042 438 683},
{2 477 219 000 485 274 833 923, -336 710 270 540 099 665 475},
{9 499 521 429 661 596 872 242, 1 297 217 382 794 031 166 211},
{33 100 980 258 166 917 992 435, 5 272 231 216 744 601 697 189},
{115 939 843 658 245 316 934 779, -9 095 691 609 975 730 619 359},
{182 027 634 443 695 308 234 152, -16 463 342 401 016 057 357 911},
{73 538 574 568 975 506 473 349, -4 835 748 414 269 733 668 617},
{79 185 520 039 430 614 083 426, -4 138 794 918 886 915 397 305},
{43 324 909 865 758 501 235 849, 7 020 898 980 679 598 203 184},
{94 761 762 552 792 049 322 855, -1 924 396 026 254 917 718 144},
{36 842 224 037 785 409 570 121, -3 259 318 124 093 618 051 495},
{78 188 249 147 693 269 290 404, 832 007 785 818 645 891 331},
{1 618 134 821 496 115 082 090, 205 258 216 478 803 056 341},
{1 890 541 916 410 440 122 402, -253 481 908 841 092 569 393},
{9 177 315 807 300 578 795 429, 188 257 688 519 518 795 227},
{3 737 563 482 311 531 484 826, 219 829 326 671 667 628 453},
{36 729 382 561 362 288 875, 492 788 935 107 026 787},
{18 153 218 161 512 891 850, 1 052 711 596 206 189 927},
{20 312 561 054 605 384 189, 1 142 608 803 844 478 204},
{20 097 395 753 022 655 157, -1 735 795 224 576 006 032},
{57 839 608 409 263 960 933, 9 734 254 852 745 879 030},
{44 707 735 869 693 746 513, 2 343 790 562 095 512 291},
{13 881 500 000 442 025 736, 1 712 796 171 855 915 693},
{14 151 319 421 981 315 168, 246 405 878 213 394 979},
{8 388 564 741 606 307 835, 989 985 074 560 765 831},
{37 026 047 464 494 313 773, -3 342 220 360 611 025 889},
{20 668 256 324 069 290 526, 1 512 441 751 353 383 679},
{39 968 327 395 368 397 420, -2 107 557 145 202 523 281},
{5 945 410 714 884 048 601, 627 581 362 082 337 723},
{23 477 098 035 297 718 426, -2 130 123 764 378 902 239},
{3 613 193 543 253 709 963, 168 220 333 097 277 470},
{6 364 757 308 659 764 347, -729 173 074 008 738 052},
{15 626 228 236 091 371 559, 242 569 195 215 651 018},
{8 042 179 640 886 806 153, 1 449 811 263 627 515 604},
{51 878 347 329 384 710 209, -271 388 113 751 712 762},
{3 414 190 621 798 240 693, -133 382 802 251 983 367},
{4 247 216 703 512 821 071, -376 492 683 018 664 354},
{8 357 978 034 293 540 983, 938 263 230 704 337 364},
{6 824 892 321 594 128 147, 1 037 411 353 938 253 154},
{34 521 985 321 917 870 549, -5 919 731 821 707 955 172},

```

```

{78 716 043 058 058 978 157, 5 326 611 649 873 194 476},
{93 467 403 513 076 179 657, -9 072 492 206 431 597 520},
{216 656 034 452 056 152 103, -939 226 181 682 840 803},
{24 111 867 817 725 797 810, 3 389 332 483 167 396 957},
{30 536 694 408 767 509 769, -1 274 876 975 372 941 653},
{4 767 887 014 464 102 337, -798 465 253 494 826 259},
{1 809 456 013 883 562 143, -23 160 394 784 848 374},
{232 672 432 565 728 709, -36 031 802 781 138 207},
{1 302 047 654 433 057 893, 21 288 743 218 588 905},
{271 311 129 831 640 352, -11 308 108 604 877 689},
{6 594 658 148 510 536, 56 569 061 144 447}, {1 889 838 425 791 277, -306 526 892 592 551},
{4 003 488 548 641 709, -701 463 925 320 985}, {16 218 305 259 451 879, 1 833 654 243 181 354},
{22 482 051 405 244 253, 3 693 603 820 793 288}, {25 313 849 958 277 475, 3 729 497 887 081 777},
{62 618 184 852 302 156, 4 193 156 658 741 045}, {22 054 037 276 268 001, 667 843 218 731 536},
{1 201 673 592 057 727, -174 868 003 257 896}, {1 769 792 029 056 055, 171 491 932 118 879},
{4 334 943 921 513 935, -773 914 115 964 724}, {24 374 721 167 678 311, -1 494 562 016 491 831},
{36 476 583 400 912 185, 2 440 844 591 298 266}, {10 750 752 016 382 595, 550 728 113 761 891},
{20 841 010 449 562 775, 2 395 464 053 619 761}, {56 735 116 608 190 846, -1 800 325 619 026 805},
{69 148 952 852 686 206, -10 077 033 012 925 441},
{109 831 980 785 558 599, -10 275 769 898 181 141},
{252 917 559 460 282 208, -23 802 570 690 951 333},
{703 946 733 074 413 945, 71 527 302 128 116 942},
{894 776 768 333 682 525, -66 796 782 190 789 243},
{2 087 069 388 420 366 914, 86 029 977 172 390 101},
{1 765 644 966 357 354 710, 314 886 674 547 515 879},
{9 770 331 393 291 504 556, 229 994 139 077 580 051},
{8 735 626 610 618 250 706, -1 070 957 066 637 956 007},
{13 269 636 123 653 609 350, -1 796 360 049 699 418 103},
{54 914 146 284 856 927 691, -803 941 447 444 456 450},
{19 444 100 832 077 238 189, 727 996 755 332 993 201},
{16 733 113 391 172 680 802, -2 228 926 011 862 542 761},
{86 765 281 594 485 241 594, -15 018 123 511 472 185 645},
{264 133 298 473 481 909 804, 22 907 860 333 243 113 907},
{850 121 016 509 401 109 320, 62 697 475 099 563 533 267},
{2 183 847 155 874 580 157 022, -143 108 062 964 545 111 361},
{2 940 870 701 105 875 441 953, -509 935 666 342 052 681 489},
{9 380 720 458 768 811 111 499, -1 037 749 696 339 183 311 757},
{3 236 882 145 576 743 149 194, 5 130 613 243 291 048 883},
{42 250 064 252 786 982 341, -2 070 997 528 836 093 591},
{65 578 980 409 143 731 159, 4 904 271 463 166 042 074},
{144 052 659 650 829 551 563, 17 276 813 829 124 931 855},
{461 213 772 408 577 641 117, 10 417 720 364 287 176 809},
{223 892 034 015 407 060 159, 1 117 758 595 547 126 821},
{26 884 877 572 553 980 761, -519 261 412 999 626 440},
{9 220 556 370 700 935 401, 404 517 234 515 735 348},
{6 583 861 829 717 230 637, -537 672 795 054 536 161},
{10 411 274 835 960 939 695, -435 686 598 276 207 824},
{3 571 078 290 775 798 399, 335 785 172 112 165 022},
{9 682 129 594 183 330 597, -1 647 632 297 883 617 609},
{16 089 471 256 351 629 503, 225 196 323 282 504 745},
{7 942 051 960 209 616 032, 297 888 766 197 961 063},

```

```

{7 974 633 443 691 280 851, -114 035 834 241 744 769},
{622 121 305 237 385 341, 102 258 801 003 117 502},
{676 911 438 275 745 991, -121 608 473 030 792 195},
{4 166 412 592 811 567 141, 430 413 785 265 334 259},
{10 880 295 527 500 260 471, 1 943 603 782 741 985 728},
{61 724 846 347 180 657 863, 5 064 716 460 568 868 579},
{74 911 656 807 984 558 285, -12 375 636 469 151 570 284},
{51 969 201 452 935 789 899, -4 732 889 304 847 049 137},
{7 313 891 130 158 298 032, 704 645 644 080 180 975},
{21 127 340 459 162 574 278, 1 377 763 942 967 175 779},
{36 409 623 857 740 069 847, 1 918 886 494 461 364 965},
{3 888 343 425 043 294 552, -291 176 244 940 396 123},
{8 141 127 024 633 451 287, 905 196 519 518 335 379},
{445 690 431 493 802 796, -13 881 518 898 332 489},
{117 064 313 025 888 692, 20 657 374 392 746 961},
{543 514 733 116 852 846, -35 788 044 329 416 751},
{528 831 385 872 524 899, 84 664 154 362 764 406},
{1 646 870 315 979 138 577, 38 447 551 654 018 377},
{503 578 006 348 479 086, -79 632 594 013 093 607},
{2 036 812 939 323 478 076, -309 448 320 413 547 945},
{10 216 698 982 137 245 581, -1 806 619 312 315 292 762},
{49 218 334 448 606 368 289, -1 816 993 214 138 421 714},
{12 601 895 682 649 578 869, -136 081 401 720 487 517},
{4 240 299 511 105 056 748, -145 528 767 300 809 193},
{1 577 255 491 145 621 929, 83 077 824 558 361 333},
{96 630 861 596 228 442, -811 779 809 715 037}, {2 296 074 970 984 081, -73 019 701 045 967},
{2 564 674 846 169 216, -119 778 873 347 297}, {3 896 161 964 202 341, 549 125 698 387 274},
{4 130 283 963 822 417, -588 295 315 692 097}, {965 123 564 241 302, -63 881 578 249 001},
{545 091 349 996 673, -44 224 064 613 004}, {1 137 803 396 609 375, -152 303 787 802 316},
{5 662 473 677 459 877, 439 778 230 427 398}, {4 316 822 129 607 463, 119 956 741 673 044},
{128 025 079 147 559, 16 720 112 214 342}, {453 129 666 806 983, 9 821 042 652 046},
{107 574 680 216 493, -13 926 421 951 226}, {303 098 936 071 885, -12 454 329 914 496},
{331 406 431 794 499, -10 647 858 481 592}, {104 502 690 346 613, 2 777 615 918 018},
{82 690 448 507 609, -6 948 606 295 009}, {54 733 335 567 421, 6 456 330 858 994},
{243 532 406 942 051, -26 337 695 151 080}, {512 958 896 004 149, -9 362 881 171 731},
{157 965 906 843 424, -14 169 689 711 363}, {165 846 281 456 049, -23 560 437 576 695},
{72 934 255 115 536, 12 858 822 384 615}, {333 275 656 180 166, -37 113 395 804 857},
{58 847 579 020 213, -5 951 246 045 665}, {52 525 633 478 523, 7 390 957 847 383},
{62 325 355 200 518, -10 966 454 375 611}, {274 396 313 198 692, -40 199 949 198 359},
{553 263 163 995 859, -73 749 685 406 583}, {2 902 011 221 287 595, 499 748 854 883 332},
{7 622 070 732 979 363, -308 504 882 750 046}, {7 153 555 525 971 173, 737 987 100 817 227},
{17 878 923 093 886 663, 767 359 889 925 384}, {18 142 004 422 623 649, 683 923 021 766 445},
{25 589 456 040 558 914, 2 331 668 002 694 529}, {4 652 467 137 391 495, 247 937 588 526 669},
{4 609 416 524 602 064, 717 702 032 488 317}, {23 953 142 044 100 798, 3 940 907 203 620 855},
{24 308 206 967 677 772, -982 635 625 255 475}, {20 357 009 433 019 137, 2 899 951 919 542 655},
{4 530 333 701 423 608, -402 475 230 779 359}, {8 145 386 865 202 061, 1 095 322 717 790 860},
{37 772 099 412 617 239, 3 336 250 429 586 806}, {84 794 230 285 827 467, 14 547 816 515 687 138},
{196 920 835 855 333 519, 7 320 822 309 763 602}, {58 567 954 154 415 065, 2 145 013 514 839 947},
{51 554 551 045 183 184, -869 727 552 869 643}, {19 009 408 644 065 513, 1 072 896 826 829 833},
{23 916 004 870 846 999, 3 034 079 953 172 683}, {28 174 145 608 222 735, -1 816 935 026 153 802},
{70 848 370 008 809 663, -12 507 909 915 278 520},

```

```

{331 728 069 146 055 103, 13 936 123 283 145 056},
{216 372 282 304 673 039, 11 035 458 298 594 422},
{342 613 809 710 016 679, 8 586 178 855 767 065},
{65 834 217 132 607 759, -1 632 378 824 870 283},
{42 586 066 885 918 681, -3 895 047 195 978 509}, {20 496 729 317 748 522, -780 020 363 305 291},
{17 079 789 873 065 524, 1 076 354 124 059 251}, {11 208 212 838 716 868, 1 370 576 335 756 799},
{19 244 570 060 335 604, 2 308 594 116 610 061}, {61 289 553 068 954 164, 2 389 361 642 607 907},
{65 874 121 469 262 022, 4 693 546 447 504 323}, {12 993 225 131 918 500, -1 243 694 550 951 483},
{43 946 090 169 889 930, -1 459 215 226 928 577},
{13 401 035 600 576 980, -2 132 550 451 600 043},
{47 852 898 387 161 038, 7 191 052 706 845 983}, {196 273 174 300 106 597, 8 304 006 255 682 919},
{238 815 091 066 393 261, -42 352 399 433 408 424},
{1 208 645 137 190 525 357, -203 599 328 662 024 160},
{1 023 115 947 747 948 637, -65 344 008 379 736 301},
{1 768 666 719 898 742 141, -31 882 566 057 897 749},
{1 194 921 350 434 909 734, 113 129 369 725 752 433},
{3 910 635 607 320 995 291, -323 921 528 918 579 161},
{1 862 603 563 545 583 361, -291 400 484 765 083 512},
{9 021 851 741 451 500 831, 162 094 659 440 107 219},
{4 380 485 788 365 771 207, 58 733 333 356 326 155},
{1 936 622 855 336 543 022, 336 451 976 664 388 609},
{6 485 031 367 333 301 928, -393 313 673 204 126 503},
{15 168 995 089 314 952 520, 2 338 411 532 580 357 383},
{89 943 545 612 791 849 538, -13 368 994 453 060 397 371},
{287 513 829 131 843 632 661, 720 049 788 801 095 199},
{16 903 108 616 325 212 540, 1 039 485 861 351 324 861},
{21 435 451 941 617 166 356, 3 432 280 982 590 382 459},
{66 499 517 639 914 856 558, 2 626 828 926 756 173 223},
{65 474 763 209 831 552 657, -8 795 871 720 009 596 946},
{308 389 232 411 385 548 765, -15 636 822 341 757 076 644},
{343 429 939 476 722 745 085, -25 383 217 890 426 338 474},
{942 873 768 150 433 490 529, -71 435 098 785 122 138 428},
{1 123 181 231 563 809 586 235, 128 925 677 176 701 595 978},
{2 934 839 179 093 877 427 793, -489 014 247 041 679 137 275},
{59 542 050 660 405 727 297, -10 438 149 315 807 744 976},
{243 860 773 520 818 662 161, 18 947 189 759 778 045 205},
{193 762 775 147 378 114 816, -3 137 737 038 246 939 259},
{61 376 776 690 637 420 118, 43 355 587 162 163 263},
{1 164 043 747 875 062 910, -6 633 797 114 510 497},
{247 210 974 022 348 865, 20 420 021 369 983 427},
{171 486 689 021 271 539, -23 539 369 012 305 981},
{530 177 368 875 244 088, 86 610 569 215 432 381},
{830 602 333 029 334 358, 134 332 582 288 584 423},
{1 943 940 304 528 397 780, -91 701 093 756 932 283},
{1 439 169 514 992 767 123, 151 851 860 127 203 465},
{5 727 719 133 986 939 102, -619 185 699 491 779 477},
{12 248 779 246 312 980 911, 544 590 241 084 116 388},
{21 155 721 454 531 209 625, -3 573 516 942 815 950 598},
{22 545 035 986 795 023 077, 922 958 951 069 049 724},
{31 127 671 729 888 546 379, 4 354 075 096 472 560 222},
{51 282 538 311 869 361 175, 5 117 692 130 246 098 888},

```



```

{8 343 743 743 261 411 305, -4 233 725 807 333 108},
{73 456 016 379 420 477, 10 885 937 513 007 608},
{216 898 150 718 989 541, 15 840 177 983 255 469},
{384 282 942 680 374 975, 18 218 952 482 031 474},
{133 110 304 059 407 659, 22 262 237 042 994 785}, {36 586 337 686 323 029, 669 309 936 844 734},
{17 830 998 370 849 939, -511 034 098 870 874}, {4 360 412 080 821 429, 355 253 828 577 071},
{7 691 924 893 829 583, -171 127 532 418 721}, {696 311 136 016 098, -28 142 863 689 935},
{573 576 042 349 883, -92 799 306 591 498}, {1 325 636 021 270 705, -31 757 002 339 017},
{644 488 080 472 711, -93 623 368 012 528}, {859 164 153 583 815, 142 290 497 794 717},
{428 272 178 425 527, -78 446 985 008 501}, {2 846 943 017 258 738, 73 170 272 974 249},
{529 112 670 220 867, 46 485 436 200 839}, {1 404 056 888 919 402, 64 456 441 503 767},
{1 104 801 108 914 288, 180 219 830 831 351}, {1 855 087 790 168 378, -63 246 835 368 109},
{1 653 435 594 964 143, -140 841 031 654 267}, {2 895 886 006 077 819, 495 973 883 439 403},
{6 316 626 270 129 321, 237 009 425 676 470}, {6 527 629 627 694 151, 446 003 138 964 478},
{12 830 979 085 068 501, -2 263 504 253 270 905}, {59 253 668 329 997 391, 4 806 063 191 193 967},
{124 891 892 817 913 173, 12 907 863 828 932 809},
{330 752 892 241 778 443, -48 396 293 117 431 167},
{633 671 606 838 938 354, 101 489 111 045 829 329},
{1 954 218 304 553 028 020, 126 555 732 716 517 771},
{4 414 702 790 615 654 945, 274 380 282 489 410 739},
{1 944 843 392 021 566 559, 258 146 733 641 133 111},
{9 506 107 691 492 367 991, 543 911 059 055 193 477},
{20 509 955 316 772 231 678, -2 204 851 969 049 440 785},
{52 636 720 030 853 904 427, -282 243 174 489 758 022},
{11 019 676 484 954 074 465, 1 973 975 397 359 862 552},
{65 109 896 037 202 966 913, 11 363 651 147 206 330 333},
{242 688 856 836 766 191 715, -6 845 295 279 145 721 657},
{245 178 243 266 608 763 880, -765 487 452 639 543 623},
{17 558 415 334 429 557 080, -2 464 060 628 319 966 497},
{24 489 283 958 993 536 479, 3 113 427 651 809 688 175},
{33 032 843 183 233 544 759, -3 441 176 312 263 391 645},
{108 934 675 212 629 363 589, -8 067 819 029 467 513 318},
{317 168 504 793 350 006 177, 55 212 979 340 139 236 987},
{1 114 640 328 551 347 843 855, 139 064 060 076 847 900 682},
{168 099 986 988 606 433 521, 2 109 697 524 320 738 240},
{53 389 381 607 157 428 641, 9 721 599 369 396 981 259},
{377 729 396 053 629 265 334, -63 954 598 087 657 368 743},
{473 857 205 312 880 822 796, 7 933 379 708 061 599 413},
{169 500 596 494 396 216 736, -4 519 617 400 475 178 267},
{177 344 313 169 184 035 390, 31 544 389 706 758 258 643},
{941 839 980 637 875 800 972, -71 835 697 346 702 589 793},
{630 097 295 328 628 559 377, 107 518 379 398 542 312 028},
{1 186 025 503 947 399 710 489, 213 577 043 837 838 768 568},
{7 539 503 967 290 999 172 601, -266 590 383 333 137 956 966},
{5 922 885 483 087 773 826 687, 681 597 565 991 650 890 056},
{16 707 916 256 129 650 521 543, 1 353 363 715 138 551 661 813},
{36 936 582 282 895 415 803 173, -1 556 254 980 405 513 227 357},
{32 669 442 500 115 230 618 205, 3 018 341 869 334 065 476 653},
{42 053 126 942 199 680 373 262, -6 890 650 464 013 185 790 157},
{56 028 708 491 524 684 953 280, -9 606 371 434 135 190 653 123},
{127 152 088 949 630 258 271 182, 12 086 010 731 763 101 624 205},

```

```

{457 728 298 881 344 908 010 767, 53 366 215 549 626 541 230 507},
{1 782 843 644 158 223 082 039 884, -289 161 483 059 347 184 109 549},
{3 782 104 918 369 058 213 224 610, -629 875 109 495 478 039 132 611},
{225 486 650 299 008 295 886 576, -13 211 775 947 631 053 411 293},
{70 030 275 953 150 643 673 005, 10 269 676 191 527 987 181 308},
{146 739 133 616 076 061 095 929, -3 310 455 548 520 017 997 647},
{85 248 069 014 426 266 757 419, -11 177 228 695 778 967 539 161},
{329 411 083 592 632 410 913 651, 36 539 674 950 027 303 752 312},
{43 766 714 348 547 494 284 597, -5 292 880 206 297 689 207 812},
{112 470 143 155 112 469 145 979, -5 272 453 829 383 067 007 858},
{138 140 406 307 376 896 495 919, -10 845 697 289 471 914 037 830},
{225 439 018 004 880 893 673 809, 29 249 133 698 465 270 185 980},
{675 770 075 044 460 157 308 449, -78 074 099 057 185 445 230 329},
{2 124 848 501 146 499 131 396 448, -72 207 595 570 802 972 170 793},
{2 435 430 137 863 822 137 032 629, -340 288 100 874 383 512 332 173},
{4 219 661 107 707 866 505 886 022, -549 938 119 709 484 975 484 593},
{14 207 664 147 473 050 541 267 038, 1 721 338 264 470 227 929 435 343},
{34 519 684 505 186 941 356 959 226, -3 403 889 222 733 440 319 797 689},
{37 982 589 950 350 514 559 604 544, -3 990 703 499 193 259 664 750 295},
{152 031 158 284 984 484 943 974 074, -19 587 860 799 014 769 779 049 339},
{369 066 520 463 560 189 785 230 402, 57 159 736 946 525 033 538 714 259},
{2 062 539 803 968 389 095 682 642 992, -27 189 969 711 860 358 653 977 091},
{307 933 636 506 854 799 549 657 996, 267 939 954 981 060 855 816 065},
{5 579 630 455 654 221 142 945 569, 685 068 694 899 704 679 668 945},
{7 827 390 820 070 112 741 926 711, -473 147 050 500 952 088 452 304},
{17 072 614 037 239 748 179 234 103, -224 355 700 041 445 558 935 502},
{1 704 885 893 100 970 310 740 129, -200 463 022 287 010 645 512 446},
{7 843 223 291 087 914 410 878 915, -1 438 368 741 215 995 808 224 756},
{51 458 987 215 626 894 210 655 665, -291 082 764 682 914 512 362 234},
{4 950 308 526 668 983 719 320 487, -628 085 824 913 131 525 710 395},
{5 875 867 738 249 410 422 651 167, 8 605 719 879 710 127 218 314},
{145 276 227 815 910 929 126 305, 13 428 355 915 538 181 153 409},
{192 419 293 145 716 021 334 326, -1 316 161 398 573 661 999 921},
{20 518 587 362 948 178 322 940, 1 473 204 820 996 656 425 401},
{8 396 130 349 395 918 981 246, 737 523 508 786 961 600 069},
{22 386 368 466 407 969 058 473, 739 891 388 083 666 166 590},
{14 980 519 087 940 740 801 067, -2 039 537 164 847 288 225 977},
{55 596 955 786 768 134 319 012, 2 148 636 667 320 017 008 713},
{21 140 207 520 632 324 694 554, 984 948 828 091 101 313 261},
{36 046 288 326 816 572 169 767, -1 582 133 325 943 294 449 083},
{27 079 475 420 456 812 572 218, -4 238 837 294 938 198 518 977},
{130 069 680 415 382 095 210 124, -638 461 182 110 526 952 915},
{13 935 658 078 066 851 578 344, -717 779 811 235 294 235 155},
{23 529 491 503 104 627 721 521, 3 757 252 825 452 760 833 752},
{77 891 989 480 656 954 801 711, 10 890 353 598 229 917 353 798},
{131 101 629 150 755 132 684 875, -5 928 526 710 648 924 765 208},
{53 249 279 801 824 240 173 621, 779 285 327 971 287 356 672},
{20 372 322 482 359 293 674 075, 1 735 960 961 537 319 754 488},
{36 277 515 430 994 927 002 699, -3 970 289 695 770 680 468 062},
{43 047 745 355 645 420 421 139, 2 393 852 088 221 861 304 882},
{3 285 786 355 498 562 272 223, 255 118 911 295 159 767 883},

```

```

{2 429 999 815 742 662 110 224, 362 186 730 471 690 077 995},
{8 319 276 507 174 306 423 539, -1 127 547 044 320 554 433 204},
{33 689 328 557 503 605 897 769, -2 507 435 524 447 445 827 583},
{86 320 672 435 258 000 996 010, -7 963 393 725 843 256 159 997},
{100 856 025 372 407 524 352 603, -284 560 324 166 427 991 038},
{9 611 978 781 869 226 486 929, -1 309 578 165 537 109 915 728},
{35 149 598 225 647 109 069 807, -232 538 516 037 641 517 256},
{2 866 302 013 095 957 167 929, -483 366 913 096 377 536 781},
{2 678 057 773 102 336 167 803, -154 309 325 876 582 262 468},
{4 329 139 422 834 578 761 913, 522 985 358 251 549 021 532},
{11 475 267 988 952 740 582 903, -808 558 176 561 738 299 502},
{12 280 827 849 983 946 800 125, -761 968 010 485 143 371 408},
{7 057 834 895 510 575 750 163, -605 904 786 483 870 324 033},
{16 828 780 841 373 582 920 407, -1 554 751 680 415 652 471 449},
{21 605 523 812 688 946 977 028, 3 858 257 961 448 039 738 051},
{121 977 892 523 944 024 650 962, 8 634 484 113 461 025 303 405},
{86 514 079 903 683 961 860 068, 15 199 249 250 211 723 364 167},
{369 831 832 209 323 887 669 786, 21 108 780 203 318 597 038 581},
{799 970 704 582 457 862 949 088, 94 367 156 309 320 304 245 029},
{3 557 642 874 523 738 890 119 624, -380 815 666 337 500 608 703 653},
{10 293 848 321 412 439 531 153 013, 145 597 936 143 603 446 936 717},
{3 444 806 437 889 010 906 957 626, -121 294 166 875 914 754 634 309},
{3 837 011 463 708 424 398 560 946, 277 423 185 572 483 154 875 311},
{3 706 137 610 200 841 805 779 232, -148 737 342 084 516 097 408 257},
{971 379 411 052 789 724 748 247, -16 966 385 165 250 666 571 398},
{339 341 074 046 636 684 106 319, 29 906 238 032 249 267 820 517},
{819 423 999 659 684 308 369 928, -43 816 915 971 887 076 885 781},
{1 034 694 900 687 442 044 332 969, 43 113 968 368 669 281 939 928},
{3 186 872 689 037 055 798 937, -527 481 684 123 735 400 355},
{1 736 624 159 276 828 347 753, -233 881 650 372 293 646 850},
{7 856 755 926 991 052 764 437, -1 171 896 818 696 727 455 428},
{27 375 222 506 997 114 461 161, 2 137 657 862 785 179 429 913},
{32 732 047 027 607 232 088 932, -657 109 220 680 615 113 679},
{9 749 706 507 458 364 006 422, -1 773 464 360 464 169 852 189},
{69 708 391 705 863 664 892 683, -12 157 902 231 729 780 228 766},
{255 882 713 076 686 301 913 127, 21 157 987 797 297 858 897 744},
{156 961 901 219 847 616 075 721, 532 188 823 342 940 014 417},
{2 670 331 639 255 366 006 226, 107 760 856 558 895 946 675},
{1 871 492 202 645 580 191 271, -269 066 066 625 413 881 473},
{945 650 834 853 041 344 160, 80 822 720 938 960 714 607},
{1 913 523 496 744 491 258 796, -63 100 869 996 729 130 589},
{1 619 294 350 566 769 948 954, -229 572 662 254 378 175 299},
{970 571 468 103 695 027 019, 34 331 850 579 629 783 798},
{733 092 498 050 825 373 325, 21 117 152 313 039 524 292},
{474 618 799 539 080 174 705, 74 016 509 881 690 880 482},
{2 411 059 479 665 856 453 227, -348 202 989 880 203 479 961},
{2 082 554 510 149 864 613 500, -13 317 072 836 819 469 081},
{402 200 660 876 167 512 256, -18 545 790 085 168 374 007},
{458 730 958 805 400 555 942, -50 436 763 628 781 302 825},
{379 206 805 563 137 610 843, 52 368 122 422 463 541 622},
{997 765 939 865 532 739 631, 108 128 066 094 810 371 147},

```

```

{1 944 454 255 966 912 545 332, -23 326 842 769 291 638 571},
{657 778 183 140 816 971 181, 88 882 440 069 878 746 739},
{2 812 487 109 481 593 776 632, -205 311 072 767 725 041 243},
{4 887 564 832 057 987 260 830, 72 050 430 078 953 257 227},
{937 288 651 555 904 217 874, 157 171 786 003 968 367 825},
{453 623 092 964 573 137 004, 72 419 123 382 025 182 125},
{1 509 559 861 121 341 496 066, 179 688 472 177 596 554 215},
{5 692 114 612 344 955 925 334, -431 183 689 185 391 873 253},
{6 851 405 581 854 064 270 555, 1 147 509 645 907 840 669 283},
{2 658 531 193 845 399 866 297, 106 973 793 546 959 777 314},
{1 249 277 941 458 970 757 687, -196 207 089 683 458 667 140},
{5 690 796 865 299 281 632 913, -877 173 203 274 827 470 119},
{33 792 854 006 375 028 163 721, 5 133 147 284 443 755 183 225},
{168 994 981 793 769 391 389 466, 28 734 292 429 388 738 652 587},
{269 451 049 822 480 201 558 424, 4 976 344 047 837 677 324 979},
{57 549 227 900 404 454 755 082, -8 256 473 045 163 422 593 117},
{19 440 589 843 420 768 342 223, 2 847 236 431 360 920 867 300},
{38 715 148 912 348 540 581 283, 2 458 563 635 521 717 682 228},
{49 127 671 223 916 444 414 835, 4 149 765 457 446 907 766 423},
{52 891 626 970 269 453 797 039, 2 239 061 726 793 536 097 396},
{66 822 503 349 257 590 696 735, -5 177 418 443 280 605 979 889},
{38 230 976 657 832 676 303 938, 2 025 533 357 936 470 238 929},
{20 078 414 293 860 400 621 327, 2 135 121 931 663 605 509 503},
{68 123 035 802 148 131 828 200, -6 375 699 902 829 225 016 663},
{158 763 387 188 894 125 052 347, -20 841 784 338 533 839 362 896},
{629 700 114 030 750 598 214 859, 28 410 796 310 725 569 952 121},
{368 345 020 388 256 682 187 563, -54 206 522 483 193 193 003 562},
{876 950 322 533 557 838 152 309, 97 375 129 398 195 095 592 531},
{45 358 478 034 356 247 742 870, 67 011 010 513 725 747 009},
{630 110 591 450 555 595 617, 26 177 821 283 015 129 030},
{145 587 571 997 207 412 863, -16 250 143 057 521 059 137},
{52 433 526 118 087 430 230, -5 837 954 752 594 264 087},
{8 537 265 765 614 777 687, 510 274 077 531 707 434},
{10 854 090 641 515 646 589, -467 521 921 972 766 896},
{7 985 828 455 218 630 499, 1 175 354 589 688 424 053},
{19 090 640 135 426 691 888, -1 749 578 015 058 122 443},
{12 222 724 386 799 743 815, -874 845 971 585 158 518},
{1 984 418 016 005 559 523, -90 606 651 042 306 013},
{705 336 247 088 648 277, -91 859 790 898 108 529},
{2 333 824 327 601 376 445, 403 160 898 627 544 231},
{6 726 144 068 947 226 339, 248 470 198 210 136 508},
{1 378 448 664 609 709 217, -105 353 577 773 660 481},
{699 320 130 617 714 156, -108 134 147 749 067 407},
{3 990 704 285 741 467 406, 247 054 805 279 565 083},
{2 988 364 700 205 660 162, -228 573 845 032 771 159},
{1 335 472 467 591 172 505, 81 425 200 959 535 374},
{2 580 870 926 849 915 159, -199 267 328 633 829 217},
{758 743 285 799 308 298, -133 863 967 373 778 143},
{3 510 800 957 025 484 240, 265 053 143 668 823 377},
{5 143 697 057 131 646 781, 169 079 853 318 118 642},
{5 632 815 149 458 914 159, 950 854 791 804 144 064},

```

```

{5 712 774 507 910 067 775, 377 871 273 524 653 844},
{3 531 726 998 180 549 085, 33 325 446 594 156 971},
{60 856 923 207 097 439, 3 395 936 969 035 193}, {21 325 436 607 346 765, -2 115 976 315 249 737},
{13 088 202 933 102 205, 996 427 767 406 702}, {10 636 714 588 391 241, 625 458 672 383 638},
{309 455 471 682 205, -3 711 404 110 523}, {111 305 510 194 884, -7 188 031 445 729},
{275 318 042 206 971, 38 542 216 344 535}, {436 279 695 822 854, 1 922 276 048 739},
{6 080 412 031 021, -80 408 797 553}, {2 421 870 057 553, 129 008 656 266},
{2 314 258 508 579, 2 771 357 334}, {13 835 640 431, 544 272 203},
{18 077 993 124, 3 180 152 093}, {79 230 635 286, 10 529 956 927},
{395 712 590 270, 39 702 905 387}, {104 000 624 400, -5 979 084 773},
{186 138 477 461, 5 957 504 510}, {115 011 174 429, 6 230 645 621},
{225 904 706 829, -5 341 261 615}, {124 165 800 921, -11 741 008 846},
{393 838 414 415, 60 098 127 844}, {2 121 029 958 947, -76 116 493 894},
{808 317 736 715, 78 718 368 326}, {1 669 590 222 945, 89 875 595 804},
{3 005 641 689 149, -480 151 132 922}, {9 854 056 437 743, -1 758 820 931 908},
{55 210 663 142 695, -2 923 584 581 383}, {26 658 068 382 978, -3 897 774 963 815},
{49 482 152 734 433, -869 465 176 026}, {6 111 621 624 871, -860 957 938 997},
{6 708 368 099 468, 936 156 955 541}, {12 266 283 443 799, 1 911 392 931 755},
{63 036 142 408 251, -10 978 906 604 962}, {224 146 480 500 159, -37 764 191 873 201},
{192 654 988 384 713, 13 070 197 823 633}, {268 440 338 612 778, -47 131 726 830 227},
{1 133 651 767 118 136, -21 949 418 612 491}, {609 722 057 780 284, -56 572 099 297 083},
{993 111 724 522 691, 94 475 842 774 665}, {3 643 681 133 891 296, 561 731 424 562 041},
{21 590 114 335 004 950, -3 176 127 513 913 461}, {50 779 482 728 752 883, 8 586 668 678 405 990},
{58 501 817 992 961 503, 8 864 403 487 803 686}, {280 371 507 311 479 621, 20 160 428 061 361 503},
{148 084 358 258 932 259, -16 231 471 331 583 676},
{158 088 185 699 654 825, -5 574 051 949 796 754},
{159 163 757 322 311 327, 27 067 512 406 261 850},
{256 064 052 105 522 067, 23 625 035 783 582 441},
{301 095 979 596 897 936, 12 613 539 442 185 673},
{128 688 394 229 099 064, -4 428 703 457 714 623},
{20 223 522 474 624 763, -947 811 983 334 306}, {25 238 195 143 742 623, -759 915 375 203 990},
{12 718 033 198 865 287, 659 071 637 014 071}, {15 458 095 552 237 102, 996 242 373 049 791},
{38 060 810 908 204 766, 5 126 993 010 428 907}, {171 576 926 980 990 943, 27 128 836 498 663 095},
{695 508 731 131 977 467, 100 671 429 943 513 969},
{726 110 999 337 004 964, 43 369 305 642 071 369},
{882 208 529 678 456 411, 136 160 562 724 812 420},
{5 154 367 113 036 969 389, -595 972 224 087 067 854},
{16 541 249 395 984 662 463, -1 495 027 966 342 420 438},
{7 579 399 531 224 973 955, -1 250 138 087 481 362 992},
{6 207 109 500 606 884 237, -782 864 009 043 060 627},
{4 408 403 167 270 461 541, 351 822 659 565 731 075},
{13 058 021 159 639 352 286, 966 714 726 930 628 591},
{37 602 816 373 766 391 052, 6 450 929 598 244 291 223},
{87 118 136 040 249 146 594, 2 057 765 823 202 310 087},
{54 665 745 794 417 712 260, 2 026 119 978 489 974 793},
{3 119 996 360 116 964 929, 280 638 434 417 024 413},
{2 604 912 940 846 014 494, 177 057 438 637 439 165},
{4 024 942 458 530 265 499, -689 942 947 593 145 994},
{9 062 502 935 260 226 735, 1 277 627 518 583 277 766},
{9 409 714 109 005 307 467, 760 807 313 984 467 821},
{22 122 080 954 143 795 585, 3 258 430 542 859 154 014},

```

```

{54 267 694 823 752 318 527, 1 557 670 007 223 340 295},
{19 809 678 896 102 752 042, 566 495 958 199 873 109},
{1 396 691 630 531 735 067, -147 446 725 238 487 332},
{5 504 017 167 442 577 241, 474 480 695 210 240 518},
{14 990 342 831 344 409 025, 1 035 513 619 693 721 003},
{38 959 020 294 952 883 657, -4 002 899 124 218 847 805},
{84 527 704 831 611 957 047, 5 937 456 114 966 602 625},
{110 862 218 544 282 103 463, -19 296 056 201 311 455 981},
{388 215 374 423 343 961 417, -43 215 413 780 530 720 438},
{57 144 618 513 169 279 475, -5 255 877 309 607 061 073},
{52 932 519 508 162 993 912, 7 164 884 921 346 897 015},
{219 487 679 640 042 469 753, 2 025 921 863 257 758 364},
{54 361 354 248 160 748 839, 404 356 493 903 496 444},
{14 029 141 142 285 802 097, 1 044 535 692 329 009 394},
{35 563 994 218 685 718 025, 4 187 496 984 481 426 476},
{163 057 449 083 910 191 143, -28 326 929 879 136 590 154},
{545 426 285 081 838 632 699, 35 409 929 551 708 042 027},
{1 127 910 002 691 222 181 226, -100 915 952 077 319 145 549},
{1 408 927 857 416 214 834 773, -214 339 733 398 675 117 026},
{7 224 571 833 586 367 768 311, 1 020 490 849 330 422 957 888},
{6 409 735 173 599 157 984 505, 618 791 259 524 049 461 482},
{17 523 983 690 334 406 205 115, -2 578 328 676 809 994 309 842},
{41 421 046 739 508 763 138 541, 6 020 438 622 485 706 132 835},
{57 039 865 813 403 203 513 016, 5 975 101 957 046 136 305 803},
{214 181 146 807 594 604 056 106, -292 300 878 525 007 326 001},
{5 956 374 947 625 506 307 533, -959 921 840 733 744 183 934},
{15 550 668 354 620 255 110 391, -1 623 673 902 879 256 649 553},
{54 199 583 259 612 599 425 981, 8 893 941 021 479 094 300 501},
{66 039 033 328 304 656 215 025, -401 786 253 837 827 182 396},
{11 540 928 213 178 865 864 399, -2 085 311 176 285 692 086 841},
{76 704 168 718 287 645 875 113, -4 203 776 022 570 203 396 139},
{81 859 824 649 894 794 824 269, -1 550 406 247 394 934 764 072},
{24 624 810 500 903 066 052 213, -4 070 730 042 719 708 286 394},
{15 833 989 322 200 490 374 071, -1 901 433 262 074 902 135 971},
{49 179 334 822 500 589 617 937, -5 787 839 364 421 866 319 413},
{227 252 972 662 927 065 948 007, -40 129 423 256 106 875 151 842},
{1 068 361 783 023 420 612 080 555, 32 756 922 530 752 225 569 078},
{996 716 178 820 823 704 222 501, -26 614 800 174 650 985 056 305},
{945 517 216 340 243 313 998 064, -20 037 623 377 145 077 224 511},
{296 164 491 539 550 071 237 713, 47 806 915 480 276 633 294 076},
{736 516 893 973 331 446 387 303, -8 391 132 161 596 187 910 338},
{150 316 163 523 514 088 072 839, 747 226 763 783 621 507 234},
{9 763 136 237 487 044 385 595, 1 687 936 944 045 483 945 966},
{28 794 348 716 082 883 925 879, 4 063 987 318 675 720 674 463},
{27 368 561 342 874 297 166 402, -438 988 232 052 848 621 487},
{11 951 985 492 216 928 102 432, 419 431 366 487 330 038 783},
{16 424 671 215 163 274 304 132, 2 988 529 519 604 455 670 197},
{117 079 865 754 138 680 298 613, 21 200 407 563 307 584 739 248},
{799 683 790 430 839 422 813 125, 86 496 657 371 688 901 415 658},
{1 675 896 052 765 505 495 704 037, 66 010 099 044 483 298 804 225},
{2 025 842 555 620 419 022 274 548, 9 151 763 869 306 409 056 139},

```

```

{260 916 499 792 507 048 558 491, -43 246 451 183 801 725 901 347},
{113 585 622 486 038 758 882 311, 2 601 372 578 399 965 466 189},
{69 106 906 121 218 008 770 395, -2 561 570 147 741 853 667 771},
{4 383 541 557 151 180 494 338, -388 627 313 588 668 174 079},
{8 582 647 506 390 615 778 051, 804 363 452 486 082 293 769},
{20 962 687 205 546 866 819 232, -1 983 403 484 541 348 017 095},
{67 525 338 828 228 948 136 227, 7 962 179 631 781 215 177 043},
{302 404 240 144 358 910 870 757, -37 042 717 761 669 450 273 245},
{478 937 346 029 261 386 098 963, 62 436 835 972 744 610 018 566},
{1 624 029 998 462 944 029 915 635, -163 206 755 221 469 571 967 634},
{634 966 746 388 383 491 095 695, 73 435 428 452 151 017 118 611},
{2 050 216 664 797 077 374 772 516, 219 490 598 266 423 457 088 259},
{5 909 301 151 542 034 617 276 615, -14 139 789 582 319 436 966 459},
{89 340 615 531 712 741 556 513, 1 982 023 658 061 302 948 719},
{11 814 522 597 374 600 268 482, 448 709 598 753 278 767 849},
{11 697 769 353 358 832 048 232, 1 095 115 390 379 288 037 415},
{27 531 495 324 253 572 703 307, 4 444 368 712 317 035 874 128},
{68 357 360 977 757 239 224 581, -199 790 169 605 294 110 722},
{2 300 714 846 985 615 254 903, 263 334 584 587 765 321 969},
{5 474 416 730 037 538 782 622, -707 472 034 194 394 018 331},
{14 643 403 937 891 455 758 054, 2 136 023 081 249 251 880 609},
{24 391 852 837 411 285 090 511, 1 379 631 181 481 482 253 048},
{34 879 165 911 176 241 683 887, 6 242 836 698 621 118 205 341},
{203 650 488 163 486 936 304 561, 30 120 319 760 676 574 054 338},
{568 148 262 738 677 483 988 595, -85 336 959 654 992 168 110 907},
{2 307 625 932 855 147 730 232 566, -35 205 711 589 723 445 997 275},
{1 260 131 533 261 376 741 419 136, 5 771 635 999 803 461 545 109},
{151 275 939 033 547 842 244 546, 11 705 853 404 940 558 256 843},
{71 112 263 223 673 792 458 627, -11 104 859 850 697 781 461 402},
{354 165 225 439 481 191 526 985, 32 786 208 050 757 313 662 887},
{512 161 986 389 091 442 416 988, 42 013 190 242 971 279 129 359},
{632 292 574 401 451 336 309 720, 69 538 418 979 677 348 159 281},
{509 297 483 164 061 027 219 089, 71 773 284 951 784 885 706 568},
{543 874 591 623 779 354 575 927, 79 884 847 918 742 225 051 116},
{1 210 228 160 785 881 441 768 915, -91 249 399 769 650 141 592 854},
{1 894 891 138 653 938 483 883 227, -252 773 085 477 776 877 909 696},
{9 912 883 684 450 526 742 713 045, -1 774 540 407 866 824 270 139 509},
{58 014 342 257 283 091 371 796 711, -8 886 136 616 855 914 918 152 616},
{330 900 510 795 956 731 366 456 479, -26 814 053 831 629 193 083 201 910},
{721 417 320 496 106 735 074 651 161, 282 384 707 581 879 810 834 798},
{5 972 982 672 098 347 052 360 591, -382 252 976 075 838 661 207 632},
{11 302 130 664 090 650 629 960 159, 1 155 801 251 631 734 262 214 165},
{20 214 666 325 908 667 382 337 789, -2 261 414 304 018 193 435 760 167},
{10 906 930 410 150 809 620 793 406, -1 519 715 365 433 687 627 293 577},
{21 244 905 317 084 702 149 330 993, -3 076 073 199 237 962 620 002 938},
{22 720 959 128 901 859 064 476 267, 1 132 230 494 147 610 610 301 209},
{6 031 590 430 022 101 817 714 873, 881 083 736 070 882 409 374 591},
{10 743 662 075 451 928 784 673 856, 1 384 151 981 867 464 666 999 119},
{26 034 748 579 535 295 554 208 584, -4 220 350 910 925 160 822 138 777},
{56 298 806 004 762 119 088 697 838, -2 741 317 074 358 296 630 535 575},
{100 239 351 984 206 702 051 389 723, -4 216 296 002 301 732 731 256 813},

```

```

{75 188 413 611 755 796 403 129 331, 1 877 663 461 697 428 196 009 655},
{6 468 136 364 834 816 456 707 349, 1 123 904 816 210 751 672 613 207},
{21 748 110 061 945 792 738 779 547, -970 162 635 577 130 444 409 486},
{31 958 034 260 664 913 979 897 545, 5 477 163 876 938 056 131 134 171},
{71 490 971 076 110 401 745 690 999, -12 799 609 831 078 251 954 528 325},
{419 228 344 918 369 688 536 837 129, -66 088 469 147 717 421 832 489 378},
{1 793 104 872 533 147 445 810 168 019, 44 837 904 769 440 224 954 338 890},
{32 494 141 312 462 636 707 618 899, 489 562 761 572 734 464 462 843},
{14 456 924 844 310 802 192 629 619, 1 526 651 285 827 125 919 098 614},
{56 647 998 477 466 844 738 625 347, -4 163 557 724 457 444 600 333 676},
{129 702 963 530 052 993 617 643 243, -4 366 301 750 149 948 781 001 347},
{101 601 028 981 192 115 179 376 193, 9 268 615 931 578 332 663 445 826},
{27 945 955 027 393 985 363 703 547, -3 857 096 551 596 940 363 288 567},
{74 756 054 131 016 822 834 002 662, -2 847 573 553 444 788 901 735 411},
{56 812 197 574 732 599 721 676 104, 4 447 904 801 149 009 816 252 875},
{79 834 622 376 157 703 279 290 409, 292 085 100 403 930 100 745 183},
{7 535 807 304 898 076 292 580 550, 944 250 846 640 177 960 405 057},
{1 437 757 989 644 443 862 132 574, -178 191 319 306 578 463 643 869},
{965 967 380 153 476 085 548 138, 106 710 597 287 038 830 815 869},
{440 188 361 040 002 048 220 043, 27 554 293 925 142 460 835 615},
{53 746 999 219 908 686 833 963, -6 498 998 421 587 178 161 155},
{138 645 935 929 689 662 033 117, -4 467 439 614 121 226 761 575},
{12 269 323 462 598 961 519 068, -1 621 277 966 224 370 415 921},
{55 371 121 108 484 142 855 700, 6 124 312 839 620 948 213 559},
{19 932 138 599 753 105 759 851, 907 888 001 859 409 828 695},
{3 270 397 851 158 927 243 681, 308 395 460 910 843 836 955},
{9 634 225 289 968 042 063 096, 393 059 016 695 394 333 827},
{15 187 760 065 928 486 323 741, 2 399 859 851 589 880 796 413},
{62 299 475 554 746 922 075 777, 6 633 506 393 305 824 415 611},
{205 235 523 184 565 684 486 962, -3 330 351 972 723 845 228 165},
{98 457 630 820 704 853 082 172, 10 099 083 609 701 682 193 631},
{200 123 216 828 645 539 476 902, 10 264 877 977 085 171 173 173},
{402 152 285 858 155 687 742 585, 72 797 746 905 771 880 621 492},
{2 736 101 450 541 572 082 922 993, 275 328 024 750 775 132 529 990},
{1 357 124 960 328 160 147 775 653, 169 230 973 533 477 803 064 122},
{258 896 592 766 680 137 751 483, -31 109 645 576 203 979 020 615},
{791 534 824 406 816 141 338 477, -133 154 668 084 907 446 545 969},
{584 061 544 107 654 497 049 623, 13 504 168 872 535 868 175 674},
{267 200 324 500 361 074 155 639, -12 118 804 836 947 207 231 233},
{46 342 828 914 278 690 412 527, -4 717 807 982 264 900 002 295},
{65 984 821 761 254 459 223 417, 9 372 685 457 842 419 647 300},
{29 705 860 952 244 213 693 043, -1 076 301 967 481 625 112 424},
{34 016 936 842 061 866 931 491, -2 382 754 428 933 375 448 791},
{52 011 612 122 574 241 224 943, 2 691 102 842 700 427 586 441},
{69 571 990 790 023 249 522 556, 8 284 442 759 594 616 173 991},
{260 419 448 348 039 290 319 612, -14 708 110 785 088 308 772 195},
{341 797 116 900 471 138 811 942, 32 712 302 515 356 554 650 027},
{1 159 253 248 005 541 792 622 088, 30 979 934 751 594 755 121 205},
{1 026 657 313 526 332 397 862 737, 186 169 623 178 747 208 649 673},
{7 138 473 618 145 917 468 788 779, 1 015 313 813 909 219 118 818 207},
{2 470 876 741 729 307 327 845 070, 391 089 464 737 268 606 124 193},

```



```

{9 822 856 311 149 959 596 893 048, -1 556 660 098 542 355 493 265 785},
{38 148 761 871 770 304 346 568 702, 3 059 635 107 964 668 366 869 203},
{113 218 105 519 348 431 586 923 014, -7 655 286 728 596 605 297 391 247},
{127 284 437 358 451 182 041 709 589, -2 653 017 860 312 429 983 616 994},
{4 773 174 987 091 116 580 583 717, -672 968 213 508 989 527 565 514},
{4 929 401 909 727 001 122 384 401, -688 197 651 002 477 184 950 527},
{8 849 449 864 063 205 390 726 248, 857 433 456 667 090 460 149 383},
{21 734 108 493 991 762 349 361 022, 3 910 494 081 686 363 249 880 281},
{136 579 623 693 986 954 843 732 456, -8 108 089 127 226 112 654 346 663},
{99 373 426 039 699 862 132 704 385, -16 080 305 692 470 366 550 559 053},
{228 435 758 905 335 363 518 655 293, -12 501 679 783 375 626 726 886 042},
{269 036 301 561 352 512 341 816 423, -31 089 560 190 605 359 101 588},
{1 007 433 923 554 960 542 764 191, -132 647 358 634 037 266 178 735},
{4 245 850 695 869 669 346 589 431, -431 082 607 930 586 065 014 802},
{5 133 055 291 459 112 981 128 531, 138 375 872 824 438 678 585 900},
{1 038 691 759 435 668 002 568 249, -125 771 485 924 999 963 358 171},
{2 569 069 890 817 795 360 527 599, 437 891 791 303 189 223 923 530},
{4 604 187 703 105 858 658 072 899, -790 554 452 174 758 542 081 890},
{10 991 981 785 472 714 959 056 839, 1 928 332 396 734 646 252 447 475},
{45 662 994 999 877 841 894 612 869, -1 476 972 063 959 626 924 439 654},
{9 727 979 646 776 828 278 295 995, -1 163 213 554 346 747 175 966 919},
{33 359 425 748 225 218 774 290 797, 6 073 050 391 268 375 068 682 575},
{236 539 729 558 784 131 039 355 838, -41 215 258 877 500 126 546 835 003},
{849 394 072 791 113 631 090 680 220, 137 976 576 519 687 807 120 253 037},
{1 701 234 480 165 956 281 163 797 842, 283 585 004 272 850 096 503 124 909},
{21 768 092 220 399 530 541 177 348, 3 040 194 014 566 749 498 413 581},
{38 451 995 356 150 440 130 300 199, 215 406 763 657 172 599 508 366},
{8 359 411 740 192 959 354 087 885, 1 394 734 567 204 566 254 171 896},
{710 657 379 720 615 504 535 789, -95 106 593 706 398 073 136 926},
{3 547 986 678 290 490 413 607 253, 301 132 034 188 796 930 634 264},
{5 182 220 826 030 747 566 309 285, 940 914 253 687 470 739 369 099},
{36 597 910 991 432 072 722 519 411, 6 275 831 079 059 186 953 364 945},
{83 508 963 150 920 870 815 950 461, -5 307 631 169 381 034 396 830 479},
{111 637 709 174 878 683 133 639 037, 9 493 550 220 154 652 681 818 971},
{180 506 583 891 194 774 806 900 585, -21 109 451 426 507 015 491 530 524},
{748 799 836 842 100 804 733 056 349, 18 391 325 851 958 780 494 812 602},
{414 317 323 968 526 448 786 566 307, 67 996 953 275 923 051 645 301 012},
{500 512 740 726 062 974 266 058 565, 43 516 081 574 896 252 665 422 313},
{1 712 738 815 642 672 559 801 726 089, -294 135 909 376 455 591 312 030 032},
{4 114 054 608 668 818 057 565 874 137, 583 398 172 753 461 903 002 837 723},
{2 391 124 552 172 194 187 134 796 004, -432 537 221 953 249 733 993 306 695},
{16 123 803 584 237 033 129 178 489 114, -1 342 747 106 924 204 742 086 455 979},
{856 225 790 579 521 707 140 371 914, -154 304 341 522 736 094 667 304 423},
{5 498 420 425 994 694 008 212 915 296, 79 597 991 396 445 688 475 944 841},
{486 562 551 555 378 766 444 980 093, 36 836 385 778 583 466 287 556 434},
{607 473 378 269 702 671 832 969 629, 11 119 240 967 867 162 273 546 259},
{322 705 122 076 309 003 753 894 664, -49 190 418 974 281 417 559 007 413},
{1 708 597 048 749 212 613 573 420 933, 122 804 029 571 232 053 468 228 129},
{842 089 854 594 854 663 560 056 967, -118 748 978 142 846 875 376 209 364},
{856 913 599 999 196 338 200 722 101, 55 727 334 301 183 101 413 994 774},
{1 659 283 253 034 535 542 273 238 789, 138 731 557 059 152 162 573 087 473},

```

```

{434 139 102 347 942 279 701 060 073, 36 565 774 583 086 772 951 674 520},
{367 365 219 278 820 661 803 699 193, -56 728 868 762 566 670 290 479 377},
{2 132 368 529 570 230 564 805 011 549, 215 028 534 152 424 417 635 319 211},
{1 415 428 144 367 075 312 306 264 319, 159 134 841 949 497 258 418 579 208},
{1 326 049 221 093 601 063 414 935 687, 84 564 102 503 326 734 487 451 530},
{2 131 137 097 810 508 382 358 814 647, 360 281 250 699 753 643 790 704 103},
{2 413 482 104 653 064 950 447 387 709, -111 441 677 204 028 061 805 171 049},
{3 020 548 713 008 640 332 043 654 151, -66 579 670 729 942 067 190 572 737},
{1 932 618 882 738 537 368 962 597 894, -293 697 364 932 219 689 075 406 065},
{9 737 751 071 173 035 910 654 320 319, 1 754 386 938 707 276 342 604 525 521},
{62 297 074 324 579 149 452 853 791 753, -1 385 290 531 586 577 840 484 607 741},
{3 238 968 148 531 416 147 330 970 768, 51 027 687 974 861 030 195 024 083},
{1 913 680 683 098 528 358 511 829 581, -183 754 914 025 775 252 328 013 229},
{6 014 391 884 421 290 983 304 085 989, 938 064 988 641 249 618 121 504 982},
{30 494 154 253 329 668 691 429 431 663, -4 251 262 269 821 314 907 137 494 113},
{58 090 150 801 856 682 975 890 856 888, 5 338 001 849 451 576 776 813 377 681},
{49 601 693 826 742 263 955 447 510 637, -2 913 161 518 863 298 807 706 335 598},
{6 157 892 479 228 553 730 744 632 209, 430 441 953 572 330 084 144 070 976},
{10 404 705 208 058 671 665 483 445 055, -370 124 393 144 319 614 532 053 141},
{3 256 553 801 400 074 228 290 611 453, -549 175 846 066 418 372 206 051 667},
{3 041 600 724 876 444 390 710 185 371, -160 050 183 984 070 189 306 977 226},
{51 131 105 149 752 716 331 828 083, 6 777 000 158 032 176 671 732 188},
{243 706 793 045 871 066 320 324 259, 1 388 911 439 275 328 246 276 402},
{51 136 002 642 401 234 534 358 811, -2 904 660 345 069 509 164 144 408},
{90 682 801 939 144 503 199 002 107, -3 552 197 216 044 651 341 419 967},
{132 271 728 563 298 102 555 445 765, -10 709 087 907 331 655 985 386 697},
{297 251 220 350 140 227 733 626 679, 26 922 347 994 628 706 701 303 969},
{87 326 000 328 731 867 523 358 580, 11 144 420 320 062 836 495 313 271},
{144 519 616 309 895 130 692 659 452, 21 466 374 978 052 365 370 012 475},
{453 855 674 381 242 724 896 801 967, -29 791 147 689 423 063 976 902 355},
{552 088 264 151 844 454 218 064 718, 78 483 078 419 652 250 481 505 371},
{2 706 715 214 278 700 847 527 121, -11 662 794 430 074 096 781 138},
{946 906 501 510 394 303 105, 155 557 601 435 381 482 932},
{1 071 310 538 950 327 035 527, 97 807 797 998 377 595 441},
{361 443 883 514 294 631 596, -31 263 990 339 632 946 871},
{1 084 196 044 342 757 737 624, 81 879 139 164 675 633 865},
{1 561 611 580 955 985 292 941, 162 703 964 579 510 411 434},
{5 168 817 122 290 386 890 521, 428 283 960 559 798 240 711},
{2 323 358 050 251 832 157 131, -280 697 980 233 221 291 071},
{6 144 162 462 498 884 456 477, 379 379 993 533 448 288 661},
{5 852 522 711 133 235 194 179, -106 502 292 124 591 383 587},
{403 165 101 823 981 345 374, -22 165 926 145 143 530 845},
{330 096 065 700 425 422 956, -54 665 093 638 836 130 171},
{166 334 805 525 282 712 470, 16 690 065 526 339 450 361},
{44 702 129 310 831 500 060, -5 743 784 161 461 133 719},
{98 603 374 487 748 005 668, -16 791 332 027 874 210 083},
{169 424 796 680 283 131 570, 20 443 063 388 234 405 087},
{464 542 876 378 223 379 046, 80 246 428 750 058 483 759},
{1 337 919 993 648 074 357 132, 45 289 566 787 456 145 555},
{1 640 593 788 073 190 751 922, 35 583 959 547 106 157 287},
{294 800 263 598 293 820 880, -2 530 471 134 481 181 207},

```

```

{99 923 871 744 346 046 781, 16 502 644 903 378 166 198},
{71 732 183 602 086 917 847, -12 894 422 544 846 780 208},
{445 113 781 692 507 308 679, 38 282 190 985 980 804 658},
{1 127 528 301 001 725 430 143, -126 973 529 622 227 082 931},
{1 203 443 782 267 146 982 644, -129 812 713 922 377 377 863},
{2 775 219 200 294 295 968 283, -67 690 879 800 144 106 847},
{8 442 849 417 380 583 076, 1 332 135 800 451 929 813},
{35 552 734 558 851 331 642, 830 697 632 493 481 291},
{13 213 827 431 100 745 809, 2 283 924 210 570 709 637},
{38 687 708 753 557 449 027, 4 193 610 150 877 967 578},
{74 672 174 256 803 525 175, 2 359 548 231 161 631 562},
{65 836 162 089 126 099 911, 6 937 330 303 765 982 290},
{268 614 959 063 348 484 779, -43 583 853 812 900 517 464},
{561 835 058 689 685 019 605, 63 010 788 451 931 457 879},
{415 700 952 838 150 003 174, 57 917 482 754 497 777 401},
{812 007 310 976 579 347 993, 104 301 640 455 805 220 034},
{1 770 059 200 919 130 570 041, 207 161 780 529 517 046 497},
{7 457 349 083 875 305 026 128, 59 266 687 463 128 953 905},
{810 029 381 836 510 106 258, 75 572 616 642 441 620 033},
{1 680 282 697 197 469 414 295, 197 889 642 047 949 107 843},
{7 676 079 304 296 247 572 529, -1 273 525 859 826 540 450 277},
{2 759 007 481 623 384 798 493, -341 321 663 755 711 312 726},
{2 246 299 554 637 849 438 115, 247 090 763 152 248 222 191},
{1 776 132 215 141 619 633 284, -39 766 763 797 821 851 431},
{1 056 400 305 068 730 807 769, 39 234 203 623 552 245 297},
{230 932 228 607 205 404 750, 37 083 752 923 314 384 787},
{665 947 174 318 208 586 212, -3 922 970 485 209 019 571},
{75 666 845 218 654 527 782, 4 373 862 954 920 212 407},
{103 582 823 815 862 432 177, 3 318 502 350 847 478 910},
{56 030 824 227 656 291 393, -5 225 918 508 700 075 669},
{114 888 070 075 518 736 314, -8 893 454 545 610 902 289},
{57 420 282 376 416 481 997, 6 997 969 429 456 555 880},
{113 485 628 320 358 761 603, 11 268 928 259 026 735 731},
{62 911 312 677 220 939 147, -10 421 688 270 266 132 634},
{30 113 461 394 307 324 097, -5 294 535 981 612 864 008},
{130 646 605 134 218 936 129, -13 361 580 744 117 190 579},
{234 566 982 249 284 603 219, 22 282 475 965 624 613 713},
{832 680 016 434 305 662 296, 73 688 485 545 645 203 249},
{1 746 427 359 144 465 698 003, 51 548 070 299 571 725 294},
{490 355 452 236 863 997 447, 67 792 150 662 799 351 105},
{1 249 021 410 184 214 637 248, -146 438 461 488 303 082 481},
{5 445 054 713 630 535 301 399, -424 266 861 053 336 768 095},
{5 562 743 924 964 572 023 044, 844 763 274 054 599 379 601},
{27 697 320 479 992 267 098 877, 4 435 297 013 464 246 746 610},
{85 757 533 537 336 142 918 143, 4 101 714 716 710 561 451 967},
{29 899 565 573 266 158 279 956, 5 238 234 199 379 033 947 287},
{120 857 330 217 635 586 897 514, -14 532 360 145 843 831 452 747},
{363 277 475 019 909 886 767 502, 52 138 750 759 305 422 148 405},
{133 808 643 323 017 393 435 307, 7 087 489 190 445 959 243 193},
{67 438 452 341 010 742 643 440, 9 473 768 023 809 287 422 873},
{88 644 017 773 312 723 982 991, 2 865 592 331 340 626 524},

```

```

{17 016 945 879 135 923 575, -1 499 623 317 455 011 696},
{41 166 061 583 332 798 601, 2 422 495 735 398 497 224},
{1 292 907 556 890 682 353, -108 674 268 868 563 487},
{883 509 893 034 279 789, 152 780 413 428 579 259},
{2 620 634 415 438 465 435, 436 412 840 665 041 944},
{170 432 344 408 887 909, 3 976 041 530 466 767},
{42 457 870 693 462 688, -2 391 268 220 692 833},
{46 211 625 041 656 174, 2 308 817 431 084 193}, {2 786 837 177 812 806, 299 697 158 566 379},
{7 075 457 306 516 205, 300 197 590 025 846}, {10 213 503 474 223 821, -1 220 044 997 928 608},
{35 798 335 772 801 603, -4 395 426 204 983 761}, {50 159 164 501 589 685, 2 605 629 051 547 646},
{51 524 789 252 568 469, -2 211 099 504 563 075}, {52 890 551 161 801 776, 62 808 167 748 259},
{479 839 503 648 142, 29 824 024 741 685}, {209 753 514 713 378, -30 843 940 689 503},
{486 171 538 938 297, -61 881 151 465 321}, {701 336 149 957 409, -2 986 738 372 962},
{43 242 047 404 219, -2 152 613 103 537}, {14 993 041 344 841, 560 579 618 198},
{11 266 059 373 895, 1 206 272 697 453}, {32 358 802 648 622, 267 160 637 011},
{2 556 880 052 989, 456 456 478 211}, {14 366 846 485 883, 857 277 925 562},
{16 343 381 645 009, -1 730 794 793 349}, {60 532 051 884 572, -3 409 028 827 539},
{65 606 893 879 270, 4 394 300 825 111}, {24 301 861 294 205, 766 755 369 976},
{18 510 533 057 133, 581 378 023 943}, {7 391 533 014 397, 198 044 666 702},
{5 046 547 367 417, 825 288 299 322}, {7 490 588 147 315, -795 254 107 122},
{26 330 793 474 143, -4 830 668 582 880}, {172 018 594 219 697, -2 746 420 652 238},
{79 466 642 832 463, 12 768 136 653 511}, {225 768 010 000 363, 14 160 422 461 213},
{63 101 200 944 555, -6 814 238 805 187}, {140 071 084 131 888, -24 139 873 226 893},
{376 684 263 128 130, -28 821 038 240 273}, {158 850 514 361 899, -2 685 669 800 456},
{31 283 694 664 605, -5 457 931 768 634}, {115 647 779 828 721, 6 646 785 034 376},
{209 542 305 301 991, -13 348 133 883 083}, {318 199 109 359 623, 3 237 164 828 600},
{75 599 536 389 017, 5 970 464 528 597}, {159 303 696 136 776, -3 838 121 762 555},
{149 896 013 352 186, -26 939 093 711 071}, {927 345 364 224 960, 85 680 892 096 849},
{1 196 411 458 389 941, -180 955 230 086 206}, {5 551 737 024 866 579, 29 607 277 469 571},
{1 140 060 013 608 751, 172 043 337 725 697}, {5 075 224 687 219 112, -550 023 534 691 079},
{9 876 017 124 952 679, 52 621 259 196 307}, {1 325 588 712 289 923, 222 397 155 234 404},
{694 743 310 203 579, 27 857 188 600 585}, {133 225 980 072 634, 40 378 968 815},
{1 245 194 203 971, -9 737 709 262}, {97 373 943 635, -17 108 006 772},
{416 653 662 763, -25 006 781 229}, {668 467 832 270, 12 440 310 931},
{261 407 682 316, -23 186 742 389}, {501 927 766 923, 10 767 001 999},
{325 584 835 370, -13 963 770 831}, {349 030 394 303, 49 987 837 428},
{69 872 947 747, 993 560 126}, {25 575 375 233, 3 383 818 890},
{118 118 895 073, -7 161 087 972}, {279 777 514 159, 50 492 878 866},
{1 831 200 963 923, 44 340 642 024}, {1 045 536 634 181, 48 669 434 817},
{1 854 801 738 896, -240 374 175 633}, {5 387 141 627 272, -786 023 313 713},
{9 086 703 928 801, -1 281 042 580 842}, {9 433 063 169 653, -782 033 181 731},
{3 844 534 121 599, 315 904 455 407}, {4 240 771 880 485, 48 627 261 393},
{805 811 004 226, -3 898 863 791}, {99 050 240 369, 17 128 520 937},
{293 949 934 987, 49 620 586 358}, {298 113 069 719, 19 594 497 802},
{331 452 612 431, -33 776 887 395}, {498 984 660 001, -79 199 656 560},
{1 879 150 930 639, -48 438 780 939}, {786 960 552 578, 71 168 398 967},
{324 544 951 339, 22 876 066 810}, {338 121 263 921, -54 597 681 575},
{832 278 783 209, -35 936 009 199}, {454 295 158 928, -3 912 912 145},
{31 390 658 532, 2 005 075 109}, {54 552 913 748, 1 805 091 573},
{31 613 158 082, 3 344 272 083}, {119 662 037 465, 638 070 267}, {23 318 645 749, 952 504 101},
{36 225 238 675, -4 539 410 571}, {7 113 625 547, 861 102 220}, {17 759 815 173, 2 832 817 150},

```

```

{60 270 069 567, 2 547 995 680}, {69 664 313 487, 3 292 147 976},
{41 807 273 289, -818 863 459}, {3 573 713 520, -408 606 781}, {8 196 053 211, -815 519 672},
{3 227 662 789, -444 789 182}, {9 016 942 685, 1 271 840 907}, {9 010 450 544, 1 246 419 333},
{22 555 701 827, -892 166 817}, {19 870 980 758, 2 462 928 037}, {13 236 960 498, 205 819 003},
{5 099 000 174, -586 362 629}, {14 082 815 473, -204 122 416}, {128 867 249, -5 572 495},
{55 289 256, 6 286 127}, {101 585 073, -11 824 634}, {382 094 007, -47 690 413},
{45 085 537, 5 945 609}, {195 867 465, 33 601 894}, {453 768 021, 10 619 510},
{226 801 811, -6 377 680}, {220 778 851, 17 564 314}, {597 021 249, -72 622 612},
{1 267 187 887, -155 143 504}, {2 057 148 545, -173 844 096}, {2 289 467 953, 286 681 936},
{315 015 265, 17 275 996}, {319 739 623, -43 669 592}, {1 110 145 841, -189 722 640},
{2 227 009 921, 272 909 082}, {3 455 243 935, -2 654 167}, {38 038 421, 227 128},
{8 535 555, -856 718}, {2 498 375, -186 528}, {5 807 369, 187 021}, {767 722, 119 915},
{3 810 328, -317 811}, {268 916, 33 205}, {258 804, -36 917}, {30 415, -2378},
{39 421, -261}, {790, -29}, {553, -58}, {2133, -116}, {3555, -29}, {948, -145}}

29
— is a relation number with a list {{80, 87}, {280, -29}, {1, 0}}
80

29
— is a relation number with a list {{81, 87}, {162, 29}, {324, 29}, {405, 29}, {1, 0}}
81

29
— is a relation number with a list {{82, 87}, {410, -29}, {164, 29}, {410, -29}}
82

```

29  
 83 is a relation number with a list

```
{ {83, 87}, {332, -29}, {1079, -145}, {5312, -899}, {6806, 899},
  {32038, 3741}, {135373, 20590}, {726831, 68701}, {2397040, 160457},
  {814645, 59914}, {2004533, -70209}, {2616824, 341475}, {9543008, 1666311},
  {37753214, -6394993}, {51189752, -5782861}, {71047751, 8323116},
  {320404319, -19127646}, {395550029, 67348121}, {708711851, 105416856},
  {2424109703, -279818158}, {7823058677, 1358044306}, {26992194197, 454413934},
  {15087083553, 816622049}, {32194593693, 287349313}, {952062871, -100697077},
  {3800501774, -390540419}, {8706900528, -1049015927}, {26126168296, 4215880539},
  {68963460146, -11516917233}, {11457589916, -873649273},
  {8312397461, 95401416}, {1035364327, -40266094}, {958991711, -8608128},
  {289628749, -6105515}, {221572152, 35159687}, {880964490, 147992191},
  {580058448, 79580611}, {1908516193, -63118877}, {1240840289, -36307507},
  {529959233, -50859417}, {1773300229, 115776178}, {3042577397, 41799875},
  {731518674, 108882443}, {2544649441, -146298939}, {4778100674, -456613903},
  {17592816452, -1017627893}, {24330808493, 548143471}, {17637148827, 2359266986},
  {93149233775, 542452888}, {12671025763, -751331014}, {8432922425, 485175887},
  {15349384718, -2634705651}, {38084482604, 5774545801},
  {193999054249, -4807686874}, {140401080987, -6591615494},
  {164103915879, 26271041768}, {537646217493, -73731047564},
  {1786897417235, 123699570238}, {4573585013949, 679066830632},
  {14930272439425, 1020066409069}, {30770066818630, 1342385660793},
  {8698680507547, 1036016474638}, {34075542966769, 2647979175025},
  {28899463610148, 2360593331653}, {47504521315896, -3246336821377},
  {98814073394997, -6757236929797}, {211191885812514, -29468822881105},
  {407540428516657, -25220356255668}, {333222459355427, 2398669135374},
  {15981688309397, 1933143631554}, {42872758328095, -4325101552853},
  {31395347636105, -3008711929496}, {108582952315035, 15847263104267},
  {194874821431222, -21635770080627}, {12689928563057, -67579666686},
  {1249048234613, -64275429509}, {2308651137186, 311599360979},
  {10578815657639, -10741936342}, {165306056173, 25217650901},
  {931052511122, -141220001467}, {4771462429201, 51297794920},
  {63702636203, 6525388861}, {128753949781, -1771437827},
  {46563961970, 605314651}, {3757091031, -357811019}, {14842904774, -1418136395},
  {54907888392, -2597217409}, {30404792649, -3101819207},
  {50912151943, 8410829255}, {37115642279, -2179434593}, {5416098434, 774616013},
  {515733531, 36861842}, {27577331, 4541168}, {27416809, 3321631},
  {70032163, 6535614}, {154346053, -3174572}, {100261925, -16760724},
  {25100777, -3313917}, {117076397, -11288366}, {347997171, 35780606},
  {814137787, -125212488}, {5175019207, -456198942}, {13016960135, -1479756146},
  {24970149857, 676617444}, {5369732393, 125898918}, {3645449723, -259919402},
  {545981885, -16893051}, {448552999, 8386800}, {336365717, -9047826},
  {132480865, -10353638}, {175663607, 81780}, {13861, -2146}, {81755, -6728},
  {84577, 3045}, {56689, 4756}, {31789, 5104}, {96695, -15573}, {270331, 29783},
  {189572, 21257}, {144503, 2784}, {21995, -522}, {5893, -87}, {1909, -116},
  {4399, -406}, {5561, 667}, {18675, 3161}, {24153, -754}, {2075, -232}, {1079, 29},
  {498, -29}, {415, 58}, {747, 116}, {4233, -725}, {9711, -899}, {14774, 2349},
  {56440, -2233}, {51045, -6989}, {176126, -26245}, {629887, -22475},
  {48721, 7105}, {84162, -1595}, {30959, 2581}, {1079, -87}, {2905, -116}, {415, -58}}
```

```

29
— is a relation number with a list {{84, 87}, {1, 0}}
84
29
— is a relation number with a list {{85, 87}, {170, 29}, {340, -29},
85
{680, -87}, {1360, -29}, {255, 29}, {510, -29}, {1020, 29}, {1, 0}}
29
— is a relation number with a list {{86, 87}, {1, 0}}
86
29
— is a relation number with a list {{88, 87}, {1, 0}}
88
29
— is a relation number with a list {{89, 87}, {178, 29}, {356, 29}, {712, 29},
89
{1157, 58}, {267, -29}, {534, 29}, {1068, 145}, {4717, 609}, {13795, -261},
{3382, 87}, {979, -87}, {1958, -87}, {3827, 261}, {7832, -261}, {178, 29}}
29
— is a relation number with a list {{90, 87}, {1, 0}}
90
29
— is a relation number with a list {{91, 87}, {364, 29}, {1, 0}}
91
29
— is a relation number with a list {{92, 87}, {460, 29}, {1, 0}}
92
29
— is a relation number with a list
93
{{93, 87}, {186, 29}, {372, -29}, {465, -58}, {1, 0}}
29
— is a relation number with a list
94
{{94, 87}, {329, 29}, {235, 29}, {282, 29}, {376, 29}, {1, 0}}
29
— is a relation number with a list
95
{{95, 87}, {760, -87}, {2185, 261}, {9215, -522}, {17195, 2349},
{14288, 1015}, {7410, -841}, {15105, 1508}, {475, -58}, {1045, -87}, {1, 0}}
29
— is a relation number with a list {{96, 87}, {1, 0}}
96
29
— is a relation number with a list {{97, 87}, {970, 29},
97
{1261, 174}, {4171, -580}, {10767, -1537}, {776, 87}, {679, 87}, {1649, -58},
{2425, 174}, {1067, 29}, {582, -29}, {194, 29}, {873, 58}, {291, -29}, {1, 0}}
29
— is a relation number with a list
98
{{98, 87}, {1078, -87}, {833, 87}, {1813, 29}, {1, 0}}
29
— is a relation number with a list {{99, 87}, {396, -29}, {990, -29}, {396, 29}}
99
29
— is a relation number with a list {{100, 87}, {1300, 29}, {1, 0}}
100
29
— is a relation number with a list
101
{{101, 87}, {1414, -145}, {3636, 29}, {1111, 58}, {909, 116}, {1919, -145}, {3434, 145},
{4646, 29}, {606, -29}, {303, -29}, {1313, 87}, {808, -29}, {404, 29}, {202, 29}, {1, 0}}

```

```

29
102 is a relation number with a list {{102, 116}, {714, -29}, {374, 29}, {1, 0}}
29
103 is a relation number with a list
{{103, 116}, {1339, 116}, {5459, 348}, {11227, -1073}, {51191, 4785},
{148732, 9657}, {399331, -17226}, {322699, 42862}, {2080291, 270918},
{8966459, -134647}, {5653670, -457649}, {16673846, -192067}, {3706249, -43732},
{1130013, 50170}, {2461391, -316419}, {7205983, 129253}, {3315055, -245949},
{12124954, -1435993}, {65612030, -120959}, {5381956, -336313},
{97644, -319}, {3090, 203}, {4635, 29}, {515, 58}, {721, -87}, {2575, -261},
{3605, 493}, {15862, 1653}, {68804, 4089}, {73027, -9947}, {349994, -39121},
{215785, 19633}, {18334, 1305}, {6592, 783}, {33784, 4553}, {197039, 25143},
{422815, 29261}, {1355583, -39469}, {1404611, -110577}, {3387670, -56289},
{1063990, -105937}, {475860, -59131}, {289636, 25607}, {819777, 98600},
{3190631, 274137}, {10198339, 477659}, {17252500, 623877}, {22253768, -1603091},
{19519118, 248153}, {8751807, -918749}, {44875349, 6187498}, {160974889, 2789916},
{86544617, 5041824}, {85861727, 11639991}, {451324370, 55271883},
{942378518, 121076595}, {2702126926, -298200997}, {1886749159, 96094255},
{3619001923, 291714625}, {12197921569, -862690028}, {12386901231, -1667719559},
{73425024754, -6390592801}, {322235906129, -23144758074},
{184442811421, -4892932316}, {153327508461, -14066543728},
{144660672341, -17415335084}, {549813141907, 63841587160},
{2550397680899, -113025276367}, {5065918580826, 230990740057},
{1635403144084, 151526019553}, {3232456312897, -135326011452},
{1582900080953, 122781385607}, {1365566989614, 41358147145},
{77057784387, 7496471899}, {215585735891, -16949049072},
{489445910635, -45715016549}, {1382184954612, 38740255955},
{1283818756104, -14147497373}, {371160998417, -5830735215},
{206623700329, 18809677675}, {29123671888, -2227767501},
{16757520625, 1728654272}, {54489275785, 6048299044}, {5622192067, -706427182},
{3010215067, -126120420}, {1717526339, -66131919}, {196066165, 21606972},
{165151951, -6438348}, {231244991, 12071714}, {193889775, -12190933},
{120010759, 5456930}, {4295203, 274195}, {9467451, 1079438}, {25491573, -3523529},
{85167610, -3235037}, {108834744, 3861901}, {72256148, -9103477},
{58881804, -7309073}, {42149660, -5189579}, {65201884, -2150089},
{72019042, 1590099}, {47852461, 2103921}, {55385366, 1611269},
{62028660, -8683093}, {128441927, 9722946}, {210493787, -6045659},
{113740634, 14245699}, {23170674, 543953}, {22588415, 1211446},
{44193077, -351828}, {14136853, 415773}, {58813, 3045}, {98674, 8033},
{234634, -31407}, {1522855, 195199}, {3989911, 115217}, {4396452, 511009},
{20870787, 252242}, {6725797, 530468}, {17539561, -316651}, {12746868, -314737},
{16206947, 476064}, {2139413, 243513}, {5377012, 654733}, {14332244, -1162465},
{39414392, 2335921}, {30515295, -32683}, {1094581, -23664}, {621811, 13630},
{532407, -54781}, {1586509, -164488}, {6012213, 14674}, {425081, 44457},
{2007367, -57623}, {972114, -86275}, {2378167, -181772}, {1558493, 145841},
{4713074, -424821}, {4124429, 370823}, {4673728, 33553}, {1015683, 24331},
{640557, 18821}, {66229, -725}, {26162, -1015}, {23484, -1247}, {21527, 1160},
{52839, -464}, {5871, -145}, {7313, -522}, {515, 29}, {721, 58}, {2575, 174},
{3605, 348}, {12875, -406}, {12051, 1102}, {7313, -261}, {515, -58}}

```



```

29
104 is a relation number with a list {{104, 116}, {312, 29}, {728, 29}, {312, -29}}

29
105 is a relation number with a list {{105, 116}, {1155, -58}, {1, 0}}

29
106 is a relation number with a list
{{106, 116}, {265, -29}, {212, 29}, {477, -29}, {689, -29}, {742, 29}, {636, 29}, {1, 0}}

29
107 is a relation number with a list
{{107, 116}, {963, 116}, {3745, 232}, {3531, -58}, {749, -87},
{3638, 435}, {16906, 725}, {24717, -2813}, {64200, 5191}, {204156, 2117},
{98868, 12151}, {177620, 377}, {5671, 377}, {1712, -29}, {1, 0}}

29
108 is a relation number with a list {{108, 116}, {1, 0}}

29
109 is a relation number with a list
{{109, 116}, {763, -58}, {981, -58}, {545, -58}, {2507, -319}, {4905, -464},
{21691, -1363}, {12753, -725}, {32373, 1508}, {76845, 812}, {32155, -2958},
{41747, 319}, {4578, 551}, {18530, 899}, {38041, 3219}, {63983, 6612},
{232933, 22968}, {354577, -43587}, {641029, 24389}, {753735, 51446},
{1957095, 120031}, {3989291, 346927}, {18867246, -2342765}, {13638734, -1355605},
{9012556, 904887}, {3958226, 359281}, {668715, 20329}, {233478, 20387},
{1005089, 82911}, {1107113, -93844}, {2072635, -248269}, {9426647, 526756},
{5990749, -37120}, {1572761, 138330}, {5573279, 249980}, {8035371, -544243},
{13981866, -196649}, {2156783, -203290}, {8655363, -869420}, {4233233, 159848},
{8413165, -483488}, {21131721, -2100383}, {13940119, 1006271},
{16096575, 1663411}, {58591315, 5750381}, {118538045, -3961371},
{33036265, 1105654}, {14535695, -630141}, {4627268, 256679}, {768014, -15747},
{391201, 51127}, {1941835, 110142}, {4438589, -196388}, {8538515, 960857},
{11902582, -230927}, {11512798, 666739}, {19427615, 311141},
{14919157, -1809484}, {48318065, -4404781}, {14663334, 266887},
{1684159, 34452}, {434801, -53476}, {762237, 52229}, {2310582, -160283},
{7261580, -83027}, {4167179, -180351}, {2082554, -265669}, {4664982, 411655},
{14908693, 1238532}, {5047681, -639073}, {7074427, 18038}, {384879, 20561},
{630020, -62089}, {995170, 116319}, {5635409, -684139}, {17690373, 734657},
{6387945, 198998}, {2180981, 221125}, {3299321, -401998}, {9083733, -315868},
{8331851, -1038084}, {2962511, 348348}, {18815689, 2078140},
{12254761, 1546831}, {13067683, -1721875}, {77097553, 3074638},
{25244727, -688808}, {26287421, -1852839}, {37896575, -307951},
{2027618, -120263}, {1836977, -87232}, {556445, -33408}, {1252519, -24157},
{397305, -9512}, {239691, 16472}, {805401, -81200}, {719291, 47734},
{357629, -30189}, {505651, 61857}, {1176655, -144797}, {1992411, 119857},
{4922222, 31407}, {945793, 99499}, {5362473, 568313}, {26994504, -2692099},
{8013026, 764237}, {40401504, -2690359}, {5026971, -347362}, {17865427, 163038},
{7494077, 173391}, {4170776, 35467}, {1561970, -125773}, {5743646, 43877},
{462269, 13978}, {108455, -5713}, {10028, 1073}, {40439, -1392}, {7739, 638},
{9047, -261}, {9592, 377}, {18203, 2349}, {64201, 174}, {545, 29}, {654, -29},
{1417, 145}, {3597, 464}, {12535, -551}, {15042, 29}, {981, -29}, {545, -29}}

```

```

29
110 is a relation number with a list {{110, 116}, {330, -29}, {1, 0}}

29
111 is a relation number with a list
{{111, 116}, {555, 29}, {444, -29}, {333, -29}, {1554, 29}, {444, -29}}

29
112 is a relation number with a list {{112, 116}, {1, 0}}

29
113 is a relation number with a list
{{113, 116}, {339, 29}, {1017, 116}, {3051, 203}, {678, -29}, {1243, -87},
{2825, 319}, {5198, -29}, {791, -29}, {904, -29}, {565, 58}, {1695, -29},
{1469, 116}, {4407, 464}, {26103, -1160}, {65201, -2784}, {132097, -9483},
{75145, -8381}, {32092, -87}, {1243, -58}, {2825, -29}, {1356, -145},
{5763, -116}, {4181, 232}, {565, -29}, {1582, -29}, {1469, -116}}

29
114 is a relation number with a list {{114, 116}, {1, 0}}

29
115 is a relation number with a list {{115, 116}, {1, 0}}

29
117 is a relation number with a list {{117, 116}, {1, 0}}

29
118 is a relation number with a list {{118, 116}, {1, 0}}

29
119 is a relation number with a list {{119, 116}, {357, -29}, {1071, -58},
{3213, 145}, {2737, -87}, {4760, 87}, {425, -29}, {1190, -29}, {1, 0}}

29
120 is a relation number with a list {{120, 116}, {1, 0}}

29
121 is a relation number with a list {{121, 116}, {605, -29},
{484, 29}, {1089, -116}, {495, 29}, {242, 29}, {1210, 29}, {968, -29}, {1, 0}}

29
122 is a relation number with a list
{{122, 116}, {366, 29}, {1342, -29}, {488, -29}, {305, 29}, {427, 29}, {488, -29}}

29
123 is a relation number with a list
{{123, 116}, {861, 58}, {369, -29}, {328, 29}, {369, -29}}

29
124 is a relation number with a list {{124, 116}, {1, 0}}

29
125 is a relation number with a list {{125, 116}, {1125, -116}, {875, 58}, {1, 0}}

29
126 is a relation number with a list {{126, 116}, {315, 29}, {252, 29}, {1, 0}}

```

```

29
127 is a relation number with a list
{{127, 116}, {1397, 58}, {635, -29}, {381, 29}, {508, -29}, {1778, 29}, {1143, 29},
{1524, -145}, {9017, -116}, {3937, 348}, {13843, -58}, {2413, 203}, {2921, 232},
{12065, 841}, {36957, -2900}, {94361, 2001}, {39878, -841}, {44577, -5017},
{73152, 2407}, {119634, 5191}, {30607, 2291}, {104648, 4205}, {60579, 5452},
{77089, 5887}, {70866, 3277}, {155956, 11165}, {44958, -1247}, {8382, 493}, {1, 0}}

29
128 is a relation number with a list
{{128, 116}, {384, -29}, {448, -29}, {832, 29}, {576, -29}, {1, 0}}

29
129 is a relation number with a list
{{129, 116}, {1677, -116}, {6837, 406}, {8385, 406}, {2021, 87},
{2580, 203}, {2537, -174}, {9417, -841}, {21414, 2233}, {118164, 4147},
{88064, 145}, {6321, 232}, {2451, 58}, {645, 29}, {301, 29},
{473, -29}, {387, -29}, {1290, 29}, {602, 29}, {301, -29}}

29
130 is a relation number with a list {{130, 116}, {910, 29}, {715, -29}, {1, 0}}

29
131 is a relation number with a list {{131, 145}, {1834, 87}, {917, 29},
{1441, 29}, {1179, 116}, {2489, -232}, {8253, -667}, {32619, -725},
{786, -29}, {393, 29}, {1703, -29}, {1048, 87}, {524, 29}, {262, 29}, {1, 0}}

29
132 is a relation number with a list {{132, 145}, {572, 29}, {264, 29}, {1, 0}}

29
133 is a relation number with a list {{133, 145}, {1596, -145}, {1, 0}}

29
134 is a relation number with a list {{134, 145}, {1474, 29},
{670, 29}, {402, -29}, {268, 29}, {938, 29}, {335, 29}, {871, -58}, {1, 0}}

29
135 is a relation number with a list {{135, 145}, {270, 29}, {1, 0}}

29
136 is a relation number with a list
{{136, 145}, {306, 29}, {884, -87}, {952, -29}, {680, 29}, {884, 87}}

29
137 is a relation number with a list
{{137, 145}, {1096, 87}, {4795, 261}, {13289, -812}, {40689, 725},
{12193, 1247}, {37949, -2146}, {93023, -1363}, {46443, 58},
{2055, -116}, {4521, -377}, {411, -29}, {685, -58}, {1507, -29}, {1, 0}}

29
138 is a relation number with a list {{138, 145}, {322, 29}, {1, 0}}

29
139 is a relation number with a list {{139, 145}, {834, 29}, {973, 29},
{1807, 116}, {6811, -493}, {12649, -87}, {4726, -261}, {3892, 261}, {3197, -261},
{9035, -464}, {30441, -986}, {17375, -696}, {3475, 319}, {4726, 29}, {1, 0}}

29
140 is a relation number with a list {{140, 145}, {1, 0}}

```

```

29
141 is a relation number with a list {{141, 145}, {564, -29}, {1833, 58},
    {1081, -58}, {329, 29}, {1410, 29}, {1551, 58}, {705, 29}, {423, -29}, {564, -29}}

29
142 is a relation number with a list {{142, 145}, {426, 29}, {639, 29}, {1, 0}}

29
143 is a relation number with a list
    {{143, 145}, {286, 29}, {572, 29}, {1144, 29}, {1, 0}}

29
144 is a relation number with a list {{144, 145}, {1, 0}}

29
146 is a relation number with a list {{146, 145}, {1, 0}}

29
147 is a relation number with a list
    {{147, 145}, {294, 29}, {588, -29}, {392, -29}, {294, 29}}

29
148 is a relation number with a list
    {{148, 145}, {444, -29}, {333, -29}, {1036, 87}, {296, 29}, {444, -29}}

29
149 is a relation number with a list {{149, 145}, {596, 29},
    {1937, -174}, {3427, 87}, {5066, 145}, {1341, 58}, {1043, -87}, {1, 0}}

29
150 is a relation number with a list {{150, 145}, {1, 0}}

29
151 is a relation number with a list
    {{151, 145}, {906, -29}, {1057, 87}, {1963, -58}, {1359, -116}, {4983, 290},
    {8003, 754}, {43941, -4147}, {253076, -5655}, {211249, 1914}, {107059, 1160},
    {51189, -1798}, {127595, -1943}, {97093, -4959}, {315137, 22533}, {49075, -58},
    {1057, -29}, {1963, 145}, {10117, -522}, {30049, 1972}, {70819, -1450},
    {34881, -2117}, {152359, 2204}, {42733, -3683}, {220913, 4582}, {147527, 11890},
    {731897, -31929}, {372970, 22069}, {332653, -10295}, {485163, 29464},
    {2074589, 66323}, {2804976, -220603}, {9492313, 496567}, {8688540, -108083},
    {6326900, -524233}, {5451704, 414033}, {10460525, 240758}, {16297581, -1205530},
    {87555689, -2933611}, {68348791, -3328765}, {234846374, 6511109},
    {67413950, -798341}, {53349206, 2400997}, {79618072, -4430765}, {20490398, 54375},
    {1355527, 120031}, {5313086, -242411}, {3013356, 144449}, {3031023, -273470},
    {3450803, -204276}, {3305239, -258593}, {8526970, -255577}, {14032279, -862953},
    {33979681, 212077}, {7151511, 433840}, {31720721, -1502809}, {24421532, -1793215},
    {103205178, -6716603}, {370876083, -17017055}, {528368177, 32708230},
    {760511047, -27043312}, {498044961, 29453705}, {402871624, -37265783},
    {1064850339, -99081835}, {3782526746, -293999129}, {5958751581, -237575482},
    {2924044181, 66671754}, {1436462245, -135868074}, {8771071919, 301953162},
    {2178963371, -19001119}, {930962414, 8463273}, {359984, -24737},
    {1671721, -117421}, {4201877, 23055}, {885917, 78445}, {3476322, -172289},
    {4611842, -329817}, {844996, -18821}, {294299, 15921}, {1165871, -58928},
    {1916039, 66584}, {2249447, -117885}, {1454432, 76357}, {550999, -4582},
    {175009, 13949}, {955528, -87667}, {1330159, -46255}, {1696636, 141781},
    {715136, 16733}, {661833, 15457}, {425518, 35931}, {853754, -14703},

```

```
{147980, -3393}, {198112, 17719}, {483653, -18154}, {982255, -88421},
{1453224, 45037}, {1818040, 166547}, {2110527, -17951}, {1161341, 34133},
{123669, 116}, {1963, 174}, {7399, 696}, {38807, -754}, {53303, -1247},
{48018, 3857}, {261834, -21025}, {1439634, -133429}, {4240835, -213846},
{5448835, -149669}, {9173401, 303108}, {12104311, -724072}, {30941863, 2370286},
{19349895, 1157506}, {49483757, -3720352}, {168996331, -10016919},
{194985092, 14656049}, {672924705, 16031084}, {57504273, -2086811},
{139891685, -7290919}, {205997824, 6821119}, {206002354, 1341453},
{87792608, -229419}, {11305219, -96947}, {5674580, 471337}, {2798936, 216079},
{1523741, -145000}, {10760109, -836621}, {17510564, -1462557}, {6058120, -215093},
{5362916, 479805}, {12844211, 914254}, {6742905, -512111}, {12904762, -498423},
{8189636, -234639}, {3432079, -163125}, {974554, 74037}, {1823023, -24157},
{1698448, -59595}, {4497988, -360325}, {26287288, 1124997}, {62265907, 2457605},
{124693082, 11883185}, {885046032, -75372073}, {2932245444, 118253503},
{3637911781, 309187821}, {10923652721, -533119673}, {39450148411, 2840633636},
{48127096443, -3759873374}, {113439870269, 1292785548},
{49113951205, 2871476847}, {45125565706, 268035197}, {14443544110, -1135570603},
{48149933079, -4228263626}, {247494012143, -20552293765},
{130839531413, 12490760433}, {895720989533, -6179914094},
{55349668647, -2279027350}, {98604849297, -3260736916},
{118194014367, 7018004930}, {167922485893, 4531712521},
{37617515016, -2044216409}, {124064567754, 1073931799},
{77239660430, 1011475021}, {55501383934, 3503841567}, {84572251838, 6917572449},
{235768749950, 3111345649}, {104721425474, -7235770541},
{516516322900, -1417861591}, {62620270176, 2378270831},
{118569514070, -5227160999}, {249933524957, 21293658001},
{844146029305, 27072853749}, {738022025986, -22439639227},
{375396344255, -125849038}, {1711750949, -64113780}, {2917487761, 155873057},
{6659148622, -516463523}, {8286453727, 5523456}, {191728777, -12866053},
{190564718, 3052337}, {199293424, 1604135}, {57483284, -652007},
{16106868, 534847}, {9280158, 559207}, {34180511, 897840}, {9451241, -561585},
{14451304, -1238561}, {62125628, -3879881}, {7177332, -30131},
{929254, -88131}, {6068237, 488128}, {31815851, 383380}, {708039, 37526},
{748205, -62321}, {53303, -2668}, {8607, -464}, {31559, -2668},
{69007, 5278}, {59343, -812}, {10117, -203}, {4983, 29}, {755, -29}, {1, 0}
```

29

is a relation number with a list

152

```
{{152, 145}, {1064, -87}, {760, 29}, {456, 29}, {1, 0}}
```

29

is a relation number with a list

153

```
{{153, 145}, {408, -29}, {306, 29}, {663, 29}, {612, -29}, {1, 0}}
```

29

is a relation number with a list {{154, 145}, {693, -58}, {462, -29}, {1, 0}}

154

29

is a relation number with a list

155

```
{{155, 145}, {310, 29}, {1395, -58}, {465, -29}, {1, 0}}
```

29

is a relation number with a list {{156, 145}, {1716, -29}, {780, -29}, {1, 0}}

156

```

29
157 is a relation number with a list {{157, 145}, {1884, 145}, {1, 0}}

29
158 is a relation number with a list
{{158, 145}, {2054, -87}, {2686, -29}, {869, 58}, {1, 0}}

29
159 is a relation number with a list
{{159, 145}, {742, -29}, {636, 29}, {318, 29}, {1, 0}}

29
160 is a relation number with a list {{160, 174}, {1120, 87}, {440, 29}, {1, 0}}

29
161 is a relation number with a list {{161, 174}, {2093, -116}, {805, 29}, {1, 0}}

29
162 is a relation number with a list {{162, 174}, {1, 0}}

29
163 is a relation number with a list {{163, 174}, {1793, 29}, {815, 58},
{489, -29}, {652, -29}, {2282, 145}, {6194, -493}, {35045, -696}, {39935, 232},
{5053, 58}, {1141, -87}, {1630, 29}, {978, 29}, {1304, -87}, {1, 0}}

29
164 is a relation number with a list {{164, 174}, {410, -29}, {1, 0}}

29
165 is a relation number with a list {{165, 174}, {1, 0}}

29
166 is a relation number with a list {{166, 174}, {332, 29},
{2158, -87}, {2822, 145}, {5561, 377}, {3901, 29}, {1162, 29}, {1, 0}}

29
167 is a relation number with a list
{{167, 174}, {1169, -29}, {1503, 116}, {835, 58}, {3841, -319},
{2171, -116}, {5511, 232}, {9519, -725}, {15698, -1131}, {22712, -435},
{15364, -609}, {23213, -928}, {2171, -29}, {668, -29}, {1, 0}}

29
168 is a relation number with a list {{168, 174}, {1, 0}}

29
169 is a relation number with a list
{{169, 174}, {845, 29}, {676, 29}, {1521, -58}, {1, 0}}

29
170 is a relation number with a list {{170, 174}, {1, 0}}

29
171 is a relation number with a list {{171, 174}, {1, 0}}

29
172 is a relation number with a list {{172, 174}, {1, 0}}

29
173 is a relation number with a list {{173, 174}, {1, 0}}

29
175 is a relation number with a list {{175, 174}, {1, 0}}

```

```

29
176 is a relation number with a list {{176, 174}, {1, 0}}

29
177 is a relation number with a list {{177, 174}, {1, 0}}

29
178 is a relation number with a list {{178, 174}, {1, 0}}

29
179 is a relation number with a list {{179, 174}, {895, -29},
    {716, -29}, {1611, -29}, {2327, -87}, {3938, 261}, {4117, 29}, {1, 0}}

29
180 is a relation number with a list {{180, 174}, {1, 0}}

29
181 is a relation number with a list {{181, 174}, {1267, 29},
    {1629, -29}, {905, -29}, {1086, -29}, {2353, 29}, {724, 29}, {1, 0}}

29
182 is a relation number with a list {{182, 174}, {364, 29}, {1, 0}}

29
183 is a relation number with a list {{183, 174}, {1, 0}}

29
184 is a relation number with a list {{184, 174}, {460, 29}, {1, 0}}

29
185 is a relation number with a list {{185, 174}, {2035, -29}, {1, 0}}

29
186 is a relation number with a list {{186, 174}, {1, 0}}

29
187 is a relation number with a list {{187, 174}, {2431, 116},
    {935, 58}, {1309, 87}, {748, 29}, {1122, -29}, {1683, -58}, {1, 0}}

29
188 is a relation number with a list
    {{188, 174}, {1316, -87}, {2068, -87}, {940, 29}, {564, -29}, {1222, -87}, {1, 0}}

29
189 is a relation number with a list {{189, 203}, {378, 29}, {1, 0}}

29
190 is a relation number with a list {{190, 203}, {1235, -58}, {1615, -87}, {1, 0}}

29
191 is a relation number with a list
    {{191, 203}, {2292, -145}, {5348, 87}, {7831, -29}, {1, 0}}

29
192 is a relation number with a list {{192, 203}, {1056, -29}, {1, 0}}

```

```

29
193 is a relation number with a list
{{193, 203}, {1930, -29}, {2509, -58}, {2895, 116}, {965, -58}, {4053, 232},
{21037, 522}, {30301, 580}, {27213, 1537}, {87429, 5510}, {141083, -3480},
{308221, -23055}, {1641658, -9483}, {212107, -13572}, {973685, -14094},
{231407, -8004}, {136837, 2697}, {137030, -5771}, {284482, 2407}, {88008, 1711},
{144171, 5278}, {321345, 4669}, {157488, -1885}, {164436, -6815},
{169068, 5713}, {448146, -25201}, {1056096, -55535}, {179683, 348},
{22195, 464}, {14861, -232}, {2509, 87}, {2702, -145}, {10229, 319}, {4053, 58},
{1351, -29}, {2316, 29}, {772, -29}, {2123, -145}, {10036, -667}, {5983, -174},
{12931, -551}, {49794, -1595}, {67357, -4205}, {14861, -986}, {13703, -870},
{41881, -2001}, {27020, 493}, {18335, 1276}, {90903, 406}, {7913, 116},
{4825, -87}, {7720, -551}, {1158, -29}, {386, 29}, {1737, 116}, {579, -29}, {1, 0}}

29
194 is a relation number with a list {{194, 203}, {1746, 29}, {582, 29}, {1, 0}}

29
195 is a relation number with a list {{195, 203}, {520, 29}, {390, 29}, {1, 0}}

29
196 is a relation number with a list {{196, 203}, {1, 0}}

29
197 is a relation number with a list
{{197, 203}, {1182, 29}, {1379, -29}, {2561, 58}, {1773, -58},
{4925, -174}, {10441, -464}, {45507, -2378}, {64025, 2784}, {1379, 58},
{2561, -116}, {1773, 116}, {6501, -116}, {985, 58}, {1, 0}}

29
198 is a relation number with a list {{198, 203}, {990, -29}, {396, 29}, {990, 29}}

29
199 is a relation number with a list
{{199, 203}, {796, -29}, {2587, -116}, {6965, 261}, {16318, 377},
{21293, 551}, {39004, -1653}, {132932, -377}, {29651, 1566}, {20497, -986},
{41591, 2262}, {174125, -6612}, {440387, 31929}, {1317181, -19488},
{1592597, -67367}, {4817989, 65772}, {3309967, 64989}, {889928, 35989},
{1949603, -58986}, {609935, -5394}, {82187, 4524}, {150245, 2581},
{108853, 6003}, {159001, -10295}, {910624, -58145}, {3919504, 147175},
{10789979, 587946}, {41183249, 2971253}, {82444307, -2568994},
{47063301, 3155519}, {53627316, -2745401}, {254860096, -10771441},
{727243112, 23913719}, {1956476858, -88120125}, {3548987492, 48525613},
{1316930857, 60869637}, {4418030243, 119779744}, {2750236715, -189661421},
{18842235400, -699324821}, {7867418633, 438141976}, {3808250065, -59788169},
{3620357449, -236719286}, {13844063641, -705175861}, {51631262221, -2628925690},
{188503064221, 1220592281}, {105838736453, -3881903489},
{204441107750, 2117262189}, {185731592017, 11727430901},
{379553177401, -10664427317}, {868874996189, -30318527340},
{2062097037529, 23254871480}, {1509718314009, -7526192201},
{606217360008, -4122719257}, {35348216571, -1372757224},
{68350779347, 4240696477}, {99427507285, 3511326293},
{220963845119, -9662817371}, {254909928386, -8778599483},
{65778132421, -2333342755}, {88462520919, -240374881}, {908377489, -46641860},
{4414247651, -275777646}, {359257685, -12618074}, {1184370987, 77954929},

```



```

{2 994 363 348, -196 091 417}, {10 545 426 507, -602 924 558}, {58 846 095 179, 75 875 484},
{6 622 800 595, 342 886 604}, {21 483 068 681, -640 931 726}, {61 413 390 597, 2 249 752 256},
{133 345 857 315, 757 549 049}, {3 427 713 509, -101 583 027}, {5 195 772 391, -228 644 874},
{12 548 882 489, -217 960 549}, {18 473 041 247, 301 329 459}, {18 296 905 352, 1 304 132 117},
{7 772 087 086, 153 294 609}, {9 141 656 627, 135 000 800}, {7 641 156 827, -140 309 192},
{12 827 631 341, 118 770 457}, {83 975 015, 4 582 928}, {294 979 889, 9 275 273},
{363 940 553, 10 500 378}, {710 962 723, -17 422 562}, {669 101 481, -43 171 198},
{4 285 168 689, 151 537 064}, {8 384 048 503, -389 024 589}, {34 723 998 545, 1 511 675 286},
{8 862 073 567, 86 322 067}, {5 790 767 466, -300 477 613}, {16 256 870 981, -567 751 212},
{41 374 919 233, -1 578 214 829}, {67 925 402 121, 2 692 903 141},
{119 961 895 604, -6 050 687 745}, {209 319 999 904, 14 433 997 479},
{1 430 802 493 919, 46 759 187 765}, {3 727 733 032 404, -70 041 254 807},
{3 093 758 998 967, 38 118 635 474}, {1 223 755 589 027, -82 849 930 205},
{3 779 679 445 552, -37 090 610 965}, {709 011 702 722, 45 076 326 233},
{2 429 693 884 194, -118 289 091 017}, {10 821 028 405 437, -114 477 703 522},
{10 816 332 401 447, 713 570 764 760}, {22 441 415 079 353, 1 375 232 418 631},
{87 101 579 870 143, -5 579 039 934 397}, {430 448 756 961 591, -18 887 892 924 095},
{790 583 278 226 206, -43 260 048 117 553}, {2 368 580 009 940 148, 20 499 204 539 653},
{1 856 215 615 260 400, -21 784 956 464 947}, {894 368 832 241 095, -34 146 173 435 368},
{1 307 096 261 383 873, 62 240 616 435 956}, {8 619 929 530 603, 40 208 541 064},
{3 045 046 838 493, 13 989 874 282}, {944 405 241 617, -31 447 091 978},
{197 503 973 123, -12 280 334 461}, {202 705 727 653, 8 035 987 290},
{359 403 035 197, -24 473 346 587}, {1 531 735 557 992, -40 594 411 091},
{2 159 560 629 734, -104 168 046 255}, {5 565 699 982 579, -358 688 377 489},
{34 489 497 391 755, 1 013 479 878 841}, {6 205 120 721 039, 31 663 211 172},
{172 865 065 927, -3 131 143 978}, {129 777 280 263, 1 007 158 487},
{29 086 747 440, -1 202 243 633}, {46 347 149 352, -2 852 731 247},
{139 986 430 600, 3 507 394 647}, {61 561 700 720, 1 790 108 607},
{138 903 608 318, -8 128 606 011}, {142 743 920 069, 4 953 872 133},
{182 755 985 812, -407 625 943}, {27 773 106 252, -170 820 817},
{14 066 696 881, -855 308 484}, {75 970 466 263, -4 140 293 721},
{287 590 677 715, 14 285 534 821}, {374 116 277 705, 7 809 636 519},
{148 508 766 193, 4 104 964 935}, {145 275 678 067, -8 774 248 758},
{773 423 612 981, 55 425 896 577}, {505 248 880 303, 14 631 653 127},
{1 364 936 849 258, 71 956 954 497}, {446 811 950 815, 5 491 915 397},
{391 393 927 942, 9 182 348 445}, {685 963 983 407, -27 924 529 809},
{2 417 703 101 782, -80 276 051 561}, {1 874 889 435 448, -127 878 831 375},
{8 615 314 000 223, 337 927 040 965}, {33 260 457 243 502, -610 537 143 753},
{57 998 844 687 160, -3 167 590 385 807}, {195 461 330 784 166, -3 695 566 975 101},
{80 340 060 341 213, -2 176 595 288 550}, {38 599 101 692 263, 17 869 060 529},
{384 258 974 977, -27 899 455 017}, {1 260 345 656 939, 41 937 671 313},
{440 887 992 251, -6 904 568 443}, {199 873 232 099, 5 028 138 494},
{249 209 224 539, 16 274 260 426}, {1 013 968 311 651, -12 235 154 288},
{308 349 356 347, 8 287 703 114}, {339 163 884 671, 18 198 459 233},
{1 314 761 310 444, 18 875 869 189}, {1 303 357 024 414, 42 431 047 269},
{2 389 082 744 075, -87 991 522 731}, {2 649 014 437 262, -138 635 432 379},
{2 973 303 190 139, 142 457 101 795}, {3 640 893 563 644, -228 091 863 633},
{1 706 674 642 316, -123 901 683 621}, {5 561 836 747 222, 340 867 351 719},
{21 483 864 823 882, -1 045 315 388 003}, {93 083 906 512 019, 4 542 891 193 862},
{442 990 444 321 021, 245 797 858 264}, {12 478 042 129 307, -183 246 241 883},
{3 442 238 571 337, 153 189 099 054}, {14 343 600 037 651, -869 469 873 069},

```

```

{85 984 331 640 853, 2 400 815 089 351}, {88 557 303 580 817, -264 781 965 690},
{23 905 281 031 043, -436 348 617 015}, {18 684 688 051 618, -299 240 851 711},
{26 219 293 861 664, 1 585 504 438 215}, {146 122 036 010 209, 3 897 107 571 300},
{383 882 118 549 691, -7 672 277 387 554}, {53 381 585 226 209, -2 054 906 526 402},
{9 150 907 588 357, -473 250 789 431}, {31 669 375 244 432, -1 874 205 379 329},
{38 231 124 628 039, -314 914 198 352}, {25 174 818 861 953, -300 158 140 677},
{7 654 526 028 085, -504 649 402 167}, {16 872 214 120 420, 384 128 713 387},
{5 860 404 452 992, 420 977 102 867}, {6 621 722 442 054, 178 349 098 825},
{4 538 351 320 271, -222 389 472 239}, {18 021 813 222 709, 391 499 641 502},
{2 553 113 009 783, 147 534 426 261}, {8 960 524 905 854, 631 637 811 191},
{23 401 514 286 820, -484 099 843 131}, {32 779 641 489 868, -797 215 194 509},
{18 669 884 484 801, -843 081 478 973}, {24 296 297 531 605, -1 361 890 016 242},
{43 326 829 389 449, -484 169 424 339}, {46 914 374 032 322, -634 962 392 593},
{14 495 760 892 440, -389 337 908 393}, {17 961 398 097 901, 1 046 461 481 923},
{34 139 028 136 790, -705 603 643 103}, {53 740 600 301 354, 552 680 838 115},
{25 981 241 835 601, 183 364 253 526}, {11 239 950 853 109, -453 865 123 616},
{21 228 770 220 909, 603 603 037 853}, {20 430 115 314 746, 1 026 885 110 107},
{21 409 790 591 406, -1 548 854 173 603}, {54 559 399 968 164, -1 861 845 402 719},
{112 610 774 573 287, 6 936 918 830 690}, {322 394 583 167 153, 17 965 216 937 583},
{194 885 020 158 859, 3 363 355 352 997}, {37 728 472 678 433, 1 462 819 106 843},
{60 659 995 797 515, 615 660 945 388}, {57 797 121 383 503, 3 823 913 082 983},
{87 246 602 612 842, -1 901 037 925 303}, {40 027 248 268 104, -846 030 680 663},
{52 497 449 111 657, -51 700 762 303}, {4 213 899 448 288, 151 007 738 919},
{2 849 131 047 356, -156 139 909 809}, {7 683 921 488 006, 281 646 632 737},
{15 813 018 417 293, 741 846 656 191}, {46 613 488 819 118, -1 816 766 003 907},
{123 863 029 210 336, 528 610 948 373}, {33 445 390 919 746, -2 033 352 966 225},
{181 436 948 569 054, -8 028 835 115 265}, {642 025 557 326 159, 7 192 460 491 522},
{377 418 142 559 499, 1 283 157 964 324}, {33 770 508 600 357, -560 745 849 968},
{25 025 762 853 123, 1 467 660 303 391}, {15 032 001 399 724, 715 508 923 877},
{1 256 485 663 093, -70 153 951 011}, {1 250 805 565 895, -74 784 998 276},
{4 087 341 554 603, -8 853 820 901}, {621 616 630 141, 40 750 745 190},
{2 060 735 005 909, 1 079 148 957}, {87 460 890 239, 1 923 824 330},
{176 870 282 411, -3 784 952 545}, {203 474 953 596, 11 902 333 555},
{225 921 349 039, -1 906 862 723}, {181 397 997 275, -9 377 305 527},
{642 609 260 138, 6 847 712 087}, {214 059 531 960, 9 867 921 727},
{603 914 460 766, -27 548 453 981}, {428 153 836 384, -8 554 092 213},
{89 395 921 066, 4 344 213 079}, {364 678 165 007, -14 193 535 569},
{866 398 197 613, 46 814 834 125}, {4 593 646 501 638, 55 810 218 497},
{3 424 508 391 916, 127 156 324 911}, {1 733 763 755 519, -38 204 682 389},
{2 896 056 554 786, -6 040 732 103}, {506 629 612 351, -20 818 552 161},
{1 389 887 736 913, -91 962 797 579}, {2 078 708 872 372, -124 951 301 501},
{9 047 187 375 855, -184 943 484 196}, {2 993 626 600 051, 158 153 366 440},
{2 246 185 099 491, -48 503 253 304}, {2 992 054 053 893, -59 531 898 030},
{3 076 371 326 207, -190 646 803 648}, {5 178 471 099 961, -206 135 559 402},
{4 991 340 867 289, -287 621 705 534}, {20 252 602 768 989, -1 160 417 262 005},
{104 576 353 665 896, -2 326 483 155 755}, {22 962 280 272 721, 1 185 998 993 087},
{85 231 581 409 532, 20 827 982 845}, {691 645 950 608, 12 270 921 467},
{890 395 342 744, -23 452 627 323}, {160 094 610 470, 998 763 277},
{58 204 743 850, 3 665 630 073}, {88 622 126 282, -6 232 580 095},
{271 834 985 448, -12 244 987 057}, {486 608 768 606, -25 716 013 059},
{397 100 423 485, 25 022 876 461}, {649 854 378 309, 39 674 616 728},

```

```

{2 997 041 621 539, 33 662 163 830}, {220 699 093 131, 9 037 286 762},
{757 037 957 757, 33 266 234 486}, {1 609 001 648 779, -54 607 100 862},
{5 053 749 032 419, 180 326 773 197}, {915 277 197 697, 5 241 839 900},
{406 912 175 797, 24 251 527 066}, {1 067 393 080 675, -4 011 777 959},
{51 768 572 619, 1 337 554 153}, {78 811 830 252, -2 015 031 331},
{44 896 060 257, -1 890 076 102}, {92 687 472 009, -2 077 002 794},
{154 753 090 479, 7 388 313 644}, {79 897 712 955, -3 207 866 726},
{59 492 083 805, -3 192 369 996}, {231 426 277 681, -5 501 682 365},
{70 768 051 849, -1 663 979 661}, {155 831 641 226, -9 505 052 151},
{746 410 555 190, -42 357 620 719}, {3 189 296 932 648, 63 272 056 537},
{5 113 127 053 802, -76 054 907 551}, {3 472 201 329 115, 45 049 057 301},
{681 359 470 662, 28 339 194 719}, {242 540 683 794, -15 720 214 759},
{1 340 755 019 391, -2 140 179 265}, {199 557 100 699, 10 322 109 200},
{683 968 153 901, -39 049 041 691}, {3 764 004 710 863, 91 433 102 487},
{3 034 254 270 304, 65 899 317 569}, {574 246 763 870, -24 455 481 659},
{2 342 366 456 887, -87 742 450 663}, {5 309 262 491 786, -334 619 564 401},
{8 885 457 187 370, 551 146 682 029}, {13 354 944 706 294, 691 103 276 427},
{44 572 508 382 019, 1 124 237 412 744}, {79 000 637 420 459, -4 982 786 750 765},
{144 066 167 764 419, 4 829 906 804 732}, {165 376 239 130 659, 2 850 743 805 892},
{6 586 579 395 677, 24 729 621 211}, {1 691 530 556 649, -8 894 438 591},
{315 857 647 441, -20 872 035 991}, {552 644 407 624, 34 343 062 399},
{627 926 438 760, -28 745 679 599}, {891 223 971 182, 5 808 394 833},
{505 372 784 867, -22 486 072 345}, {2 125 159 462 123, -138 975 926 193},
{8 063 593 276 372, 546 106 870 281}, {25 473 945 790 757, -1 019 044 019 956},
{428 786 920 457, 20 950 174 229}, {1 946 903 739 523, -86 709 934 924},
{7 817 749 067 805, -166 227 580 051}, {1 005 508 276 192, 36 798 213 883},
{2 379 343 768 849, 41 335 239 958}, {3 601 929 594 285, 172 756 252 118},
{5 164 388 338 407, 241 073 885 980}, {20 265 509 832 573, 721 459 278 292},
{12 865 358 039 003, -793 143 826 393}, {34 836 306 526 285, -459 543 225 422},
{17 706 742 551 613, 1 135 816 985 173}, {92 799 513 019 845, 3 872 721 049 988},
{29 012 643 793 533, -1 180 363 609 586}, {98 792 842 777 283, 4 541 207 309 326},
{221 629 887 549 911, 638 784 089 994}, {5 610 143 923 393, -396 441 267 341},
{11 933 269 943 181, -635 946 493 064}, {29 792 971 581 965, 644 361 665 301},
{30 314 660 645 681, 114 254 796 820}, {7 390 758 187 819, 118 756 143 151},
{5 547 585 178 943, 187 652 710 712}, {16 317 232 340 983, 703 320 649 800},
{28 030 621 721 017, 1 075 417 265 362}, {13 884 791 499 395, -473 617 806 732},
{29 825 145 729 233, 1 370 372 918 878}, {64 288 638 730 517, -1 012 024 060 919},
{95 699 332 491 501, 6 146 913 793 487}, {527 606 352 653 909, 6 961 881 887 111},
{297 837 482 538 873, 3 495 975 801 967}, {135 228 334 963 922, 5 966 722 338 263},
{399 249 484 409 273, -23 736 031 960 677}, {848 348 725 524 964, 25 579 427 870 651},
{841 293 552 902 719, -58 917 710 200 309}, {3 272 676 409 580 207, 198 442 991 473 434},
{19 420 120 655 047 337, -130 794 374 923 412}, {12 448 080 110 089 839, -631 495 058 520 422},
{36 182 391 003 401 599, -879 941 336 182 318}, {20 854 447 765 385 639, 1 158 916 016 194 320},
{1 202 064 696 312 079, 81 526 577 567 673}, {4 145 959 473 400 184, 89 207 383 994 601},
{8 441 542 120 059 062, 529 826 697 619 171}, {7 101 323 327 687 126, 120 840 959 204 663},
{5 630 359 812 210 209, -252 714 690 427 506}, {14 056 687 938 210 323, 921 328 138 607 131},
{47 116 405 961 568 242, -2 043 368 095 110 245}, {23 669 015 032 488 793, 381 655 812 642 399},
{1 264 575 083 350 945, 24 164 525 500 261}, {1 595 931 710 137 227, -75 291 643 908 218},
{2 946 630 424 865 151, 46 258 747 883 353}, {2 771 958 494 218 759, 85 445 430 729 900},
{7 503 237 461 529 841, -491 345 124 698 876}, {26 479 057 618 293 499, -1 308 751 306 218 099},
{60 502 267 292 372 281, 4 065 889 783 019 829}, {96 729 811 132 105 646, -5 622 731 135 666 409},

```

```

{227 532 983 329 561 907, 8 450 984 218 203 907}, {128 074 521 826 772 818,
-1 974 492 749 828 473}, {53 233 875 503 507 473, -2 718 665 747 387 906},
{226 748 449 405 878 753, 12 314 581 597 893 086}, {1 012 110 148 116 837 795,
-56 786 719 414 255 951}, {2 000 109 466 614 095 277, -66 899 151 842 170 064},
{1 366 152 641 550 321 957, -25 936 032 314 064 613}, {1 682 957 147 925 403 868,
10 914 133 581 415 999}, {433 934 701 080 664 378, 21 864 264 784 522 109},
{666 768 327 345 782 598, 21 537 273 640 131 919}, {176 543 944 163 071 309,
10 576 623 914 021 232}, {648 473 812 682 637 365, -25 721 563 455 438 038},
{1 081 510 533 040 596 585, -75 165 124 307 176 442}, {5 810 559 755 285 153 003,
283 910 073 217 867 276}, {26 339 299 894 633 689 117, -1 077 751 983 240 667 181},
{94 177 207 074 677 677 827, 5 116 421 077 069 253 653}, {414 243 909 798 791 302 527,
-8 074 655 566 756 775 042}, {484 858 702 944 959 301 615, 18 272 963 643 983 948 437},
{1 693 751 773 078 853 930 616, 66 102 452 381 372 451 077},
{4 957 485 778 529 129 679 814, -150 329 851 067 963 528 831},
{676 462 036 019 687 550 191, 45 932 269 534 820 109 086},
{2 491 879 393 520 203 133 701, -62 066 560 533 989 286 339},
{1 834 177 459 965 704 348 059, -55 804 683 981 206 673 367},
{1 468 045 171 409 058 737 348, -19 551 900 226 608 562 383},
{328 878 228 269 895 165 977, -8 742 927 979 607 708 790},
{667 253 956 084 355 840 557, -10 441 578 671 300 869 236},
{200 408 696 901 058 318 853, 4 298 743 934 204 241 691},
{324 821 333 301 667 084 176, -3 406 143 492 220 890 781},
{246 302 606 595 809 536 219, 4 150 993 964 078 184 112},
{277 398 580 324 138 048 589, 17 549 424 037 487 943 908},
{675 048 650 858 141 733 861, 49 125 880 338 391 474 624},
{2 530 021 101 988 443 264 125, 178 756 460 182 463 764 949},
{5 458 701 227 356 160 412 961, -224 474 984 995 184 840 044},
{14 189 015 906 873 126 129 095, 819 890 792 918 289 546 634},
{49 923 613 025 178 563 427 083, 3 101 659 197 453 572 209 920},
{59 116 107 318 360 205 604 237, -3 043 347 750 639 176 967 864},
{257 207 511 186 952 799 749 379, -5 906 176 293 044 964 927 992},
{530 184 895 698 105 759 371 531, 16 382 199 759 787 189 883 393},
{1 184 946 173 598 220 937 488 045, -20 873 612 890 890 602 932 998},
{965 102 475 326 142 508 875 359, -65 443 263 525 553 849 105 068},
{3 292 749 033 875 880 312 431 539, 67 317 514 324 842 682 290 969},
{1 156 024 440 240 812 845 362 458, 81 084 505 430 104 220 282 609},
{4 147 431 479 651 398 519 780 468, -182 971 603 163 255 344 605 565},
{12 122 163 227 591 406 823 357 873, -686 125 370 528 099 767 336 508},
{45 390 594 940 963 408 751 154 929, -2 369 957 390 771 040 417 890 947},
{71 919 498 746 414 521 434 160 264, 11 373 025 864 215 490 853 027},
{699 846 957 964 301 356 114 316, -19 501 698 832 027 075 727 581},
{440 625 797 746 000 645 641 400, 28 130 087 281 724 133 024 619},
{1 881 664 153 555 511 067 748 296, -113 640 087 343 522 475 446 861},
{9 993 248 925 589 831 954 819 859, -686 464 334 587 178 275 704 885},
{60 439 502 550 350 593 969 929 784, -4 317 864 670 230 295 004 312 909},
{2 109 963 741 833 681 999 737 458, 149 932 964 693 440 980 242 399},
{2 169 544 988 976 146 992 430 528, 117 164 295 859 193 754 842 329},
{11 258 749 837 358 335 565 170 877, -345 582 142 474 611 286 691 933},
{28 946 711 996 463 542 236 919 488, 1 277 005 315 467 326 464 103 499},
{84 457 641 597 708 321 054 736 811, 4 341 790 126 546 594 057 146 000},
{390 762 209 471 283 759 823 599 389, 9 837 536 087 252 440 873 231 215},

```

```

{545 107 569 743 961 146 024 192 989, 28 274 982 276 823 717 822 666 190},
{1 568 698 390 377 790 971 313 540 421, -88 385 728 037 198 013 602 577 965},
{4 426 698 144 062 881 433 039 726 851, 171 148 588 943 931 530 681 325 968},
{4 609 868 527 388 334 570 274 915 083, 202 714 981 099 066 748 368 893 211},
{10 462 631 540 149 927 799 716 125 230, -697 948 669 502 998 699 349 656 409},
{1 313 101 976 615 485 415 215 460 095, -33 084 194 342 605 221 108 308 479},
{2 042 893 620 655 962 394 258 933 935, 34 176 131 572 891 223 984 543 851},
{1 527 180 469 784 697 917 925 727 875, 98 121 889 037 075 714 589 489 026},
{8 511 181 206 894 189 585 713 211 659, 318 910 312 772 203 991 520 478 850},
{19 780 050 353 108 318 882 603 740 909, -47 714 426 175 592 065 835 659 492},
{4 265 865 442 715 299 399 794 705 929, 170 289 062 303 850 051 493 741 023},
{1 719 138 138 690 574 377 784 890 446, 66 288 157 392 800 000 883 377 667},
{866 436 750 922 903 391 402 850 304, -59 819 498 134 654 304 078 605 397},
{5 763 791 630 510 883 726 172 574 454, -144 786 651 472 493 984 878 327 127},
{5 507 211 249 386 258 123 141 614 574, -79 559 594 959 895 403 985 995 271},
{3 502 240 233 541 574 373 480 234 125, -10 681 156 044 937 344 174 212 304},
{234 610 890 377 028 616 618 915 813, 5 799 395 164 152 331 468 195 070},
{524 381 678 376 136 220 331 489 587, 7 818 179 909 433 279 536 658 275},
{112 161 264 377 191 783 701 647 238, 3 032 458 463 838 888 608 875 415},
{7 900 058 184 571 870 521 880 283, -196 499 767 485 845 977 801 653},
{7 973 429 542 468 250 553 018 437, 403 086 616 415 620 494 235 771},
{17 572 254 382 987 707 007 699 617, -830 032 192 809 239 157 330 712},
{28 174 088 464 743 256 047 178 335, -945 538 936 364 335 953 400 288},
{38 223 845 611 177 688 411 230 695, -1 228 263 083 704 184 336 023 418},
{29 390 313 253 246 824 906 442 663, -292 756 633 931 669 952 329 921},
{22 815 322 155 886 105 016 662 037, 1 588 656 809 268 769 027 539 607},
{114 251 238 398 544 387 590 400 261, -201 176 149 474 549 259 872 196},
{3 346 086 096 918 811 384 406 333, 49 165 612 405 486 271 761 678},
{562 066 215 803 236 017 833 571, 36 768 372 526 102 263 771 643},
{2 097 584 954 428 710 190 526 274, -19 370 893 850 284 145 655 539},
{1 100 155 301 006 469 485 884 338, -7 028 531 982 913 014 721 109},
{661 519 841 863 891 240 625 225, -47 357 970 630 424 088 951 434},
{296 857 645 447 154 934 275 349, -6 588 138 600 447 979 512 656},
{77 890 276 972 175 384 959 971, 5 658 366 924 912 353 390 212},
{264 045 135 342 914 938 096 403, -10 125 777 739 008 259 631 711},
{154 207 911 611 337 346 711 483, 7 496 105 844 846 156 992 881},
{638 851 914 955 958 077 664 582, -2 140 698 603 960 377 078 967},
{183 822 464 177 375 918 350 784, 2 612 150 567 173 534 726 591},
{193 412 970 570 469 010 393 386, 12 473 386 798 262 941 117 501},
{1 226 082 422 145 871 449 839 370, 19 250 617 051 321 997 189 081},
{1 185 456 758 608 537 682 100 986, -30 262 682 699 273 213 589 787},
{1 037 214 534 039 588 067 759 307, 23 800 813 628 158 930 812 267},
{1 994 231 854 281 572 708 107 759, -86 494 673 879 759 208 716 509},
{966 016 654 375 070 617 982 348, -37 731 945 393 691 346 537 315},
{2 987 771 246 319 974 005 580 558, 106 791 683 918 712 710 919 579},
{476 784 777 392 398 133 363 146, 9 701 707 111 552 614 765 375},
{278 824 656 337 681 962 094 429, -19 731 750 238 483 386 491 607},
{513 450 446 783 995 691 174 269, -35 747 575 095 050 684 237 845},
{2 583 894 695 203 936 257 043 361, 40 634 450 845 561 462 954 734},
{3 325 321 623 487 477 039 863 385, 151 852 625 347 973 297 398 129},
{3 071 790 699 419 165 076 195 147, 221 384 134 922 125 527 605 645},

```

```

{5 489 850 708 627 869 746 492 717, -53 875 612 008 245 090 729 970},
{1 086 881 526 412 772 084 880 377, -49 257 582 650 616 650 183 726},
{639 726 911 741 950 386 842 595, -13 472 785 391 110 733 618 249},
{1 294 693 673 589 435 450 193 508, -39 648 958 774 197 835 365 399},
{2 730 671 225 859 530 256 067 141, -68 597 460 208 638 543 787 819},
{2 632 209 314 716 287 593 678 181, -158 283 933 876 931 031 450 255},
{11 664 894 677 116 448 254 254 646, -799 773 375 029 232 219 260 109},
{66 009 483 716 084 971 894 750 811, -4 376 130 891 946 060 448 203 886},
{73 136 547 041 918 969 166 811 679, 3 113 313 636 820 949 092 241 624},
{304 536 345 612 390 869 005 611 073, -1 765 944 657 709 989 017 173 586},
{157 979 032 768 278 852 299 101 919, -6 091 935 355 638 061 904 431 379},
{81 846 009 183 840 686 006 673 065, -4 290 267 071 245 526 283 175 309},
{65 856 031 204 961 638 642 096 606, 379 649 505 587 452 237 316 223},
{35 156 680 928 147 915 691 615 373, -1 299 779 562 691 694 853 733 368},
{12 463 914 358 958 773 522 072 963, -734 528 301 314 465 019 088 666},
{4 590 285 914 039 228 684 437 441, -325 882 310 095 538 461 969 475},
{5 558 780 967 636 353 156 093 409, -44 691 041 090 850 805 610 405},
{3 401 282 601 799 798 820 234 611, 28 440 200 506 091 613 994 063},
{2 296 750 327 307 776 951 536 851, 30 339 352 366 834 328 285 320},
{1 799 050 061 754 767 631 346 331, -7 549 255 721 488 564 416 857},
{463 112 808 057 370 726 738 635, -17 548 262 744 050 833 229 673},
{1 364 737 365 697 763 490 660 263, 87 759 557 623 494 951 740 587},
{7 843 695 699 352 991 700 636 671, -318 384 986 077 749 719 105 698},
{23 069 861 565 559 504 124 150 021, -518 240 648 031 759 528 150 327},
{49 942 551 578 065 253 880 324 106, 1 237 045 035 232 241 200 349 309},
{91 689 283 586 345 567 403 997 454, 5 660 373 910 349 736 633 901 079},
{223 536 903 129 206 471 054 457 810, -13 736 127 901 430 390 357 578 129},
{748 012 484 557 724 841 308 341 454, -8 318 340 302 484 314 582 431 821},
{126 990 390 506 830 750 993 964 764, 8 303 499 600 759 665 645 525 063},
{485 141 402 591 717 495 906 674 981, 26 319 458 095 517 333 963 245 264},
{2 266 840 217 608 691 429 083 785 571, -47 924 627 788 195 380 986 938 720},
{2 862 159 601 138 196 016 835 480 469, 56 267 683 009 303 822 942 237 297},
{1 490 954 234 923 491 690 505 713 922, 101 017 444 287 360 688 176 268 321},
{4 837 178 447 996 807 795 523 867 707, 340 076 701 213 792 681 242 065 134},
{15 144 821 569 738 341 368 856 210 369, -742 799 730 790 778 496 154 330 403},
{57 476 563 830 631 517 708 150 859 491, 2 950 523 520 321 773 957 020 655 101},
{281 906 771 959 044 692 426 924 101 828, 12 007 701 069 801 132 395 194 860 867},
{1 140 199 823 370 110 820 151 018 075 513, 63 295 687 321 254 527 642 202 746 411},
{174 612 865 918 335 195 682 359 382 885, 24 237 946 225 201 701 517 684 964},
{537 561 084 445 451 842 423 543 571, -33 607 645 068 893 622 490 899 906},
{32 086 094 712 377 368 740 130 075, 1 437 209 301 341 018 135 341 544},
{93 030 526 492 118 982 760 605 293, 1 303 190 496 006 023 499 758 093},
{100 296 253 862 571 541 278 357 310, -3 753 757 205 667 376 549 659 673},
{209 982 947 399 077 486 928 318 339, 12 584 963 376 260 541 914 387 671},
{788 324 569 472 993 397 638 141 532, 22 984 626 434 553 102 218 432 855},
{1 362 606 868 939 396 520 073 467 938, 6 811 104 784 723 226 448 021 991},
{76 796 486 955 494 863 344 877 862, 1 244 662 577 854 347 190 665 567},
{74 145 981 423 457 832 801 071 108, 831 592 280 584 780 807 875 931},
{26 719 421 831 055 839 122 536 551, -1 945 895 074 817 721 673 911 234},
{104 098 734 062 060 598 131 924 275, -7 191 229 271 040 678 306 091 084},
{680 883 329 230 729 267 483 170 701, -41 915 772 335 707 633 172 591 522},

```

```

{2 035 963 400 022 020 207 619 563 451, - 33 689 544 967 223 983 320 157 490},
{2 903 549 695 727 660 473 612 696 149, 65 866 274 224 108 021 581 579 154},
{1 081 292 343 514 597 280 619 461 227, 28 641 480 951 085 970 859 662 835},
{1 409 702 592 707 252 797 497 574 097, 52 498 583 589 616 781 681 016 271},
{1 544 073 678 267 661 270 083 178 780, - 96 493 074 991 728 829 442 034 449},
{36 711 201 599 999 803 114 891 604, - 1 425 572 954 140 033 834 036 075},
{70 385 346 320 574 237 439 222 854, - 3 511 490 730 687 441 904 454 027},
{30 950 809 658 254 470 678 320 486, 328 366 773 369 139 903 350 057},
{16 782 259 349 508 632 919 610 472, - 687 720 997 356 533 987 383 881},
{55 114 127 177 411 627 257 068 272, - 317 459 888 704 372 847 509 615},
{24 654 797 972 700 393 711 342 862, - 1 497 866 779 737 368 759 259 851},
{137 096 969 883 596 219 073 863 954, 1 608 841 984 848 316 892 871 661},
{68 734 833 126 367 352 774 781 031, - 372 732 157 239 729 147 669 093},
{30 271 122 657 180 731 129 915 881, 819 584 478 088 374 222 134 560},
{10 647 103 385 733 902 723 504 961, - 180 578 428 231 024 008 432 685},
{1 397 752 099 406 241 030 667 346, 85 224 226 167 475 062 395 099},
{6 798 731 664 601 366 436 806 638, 116 532 009 094 001 470 164 035},
{7 935 152 292 706 952 291 228 992, 62 290 263 123 215 532 930 325},
{4 833 486 335 657 342 206 465 683, - 283 030 941 058 664 885 433 599},
{4 370 107 194 347 791 664 805 500, - 280 375 562 254 390 952 122 201},
{23 064 458 542 770 250 260 793 484, - 1 344 851 360 550 740 118 491 989},
{40 195 097 268 125 981 039 504 529, 1 823 120 736 232 157 157 275 303},
{17 201 773 132 686 192 310 124 737, - 683 677 122 692 377 280 478 618},
{21 859 168 009 975 299 333 698 113, 925 049 109 037 012 989 385 907},
{68 060 110 775 689 469 901 167 345, 4 363 071 710 704 253 883 778 412},
{348 058 282 520 139 855 618 162 153, - 5 976 228 809 900 548 903 291 217},
{285 965 297 635 695 826 227 041 833, 19 257 176 938 434 938 380 435 664},
{575 578 931 724 821 646 419 132 273, 26 225 281 316 332 067 937 134 282},
{274 074 189 662 285 791 366 564 269, 13 369 251 854 057 784 035 793 751},
{1 329 339 755 312 607 003 635 795 898, 51 639 185 851 136 371 229 471 363},
{2 642 536 286 570 791 017 761 448 460, 121 319 163 286 823 768 085 018 583},
{5 270 575 842 127 044 141 683 112 834, - 332 223 634 418 569 630 963 328 983},
{8 955 459 405 443 920 792 300 027 906, - 445 911 125 838 105 005 190 704 609},
{7 410 140 847 682 317 008 701 209 474, - 186 992 756 413 298 813 395 060 763},
{13 844 312 361 077 469 893 142 988 154, 896 327 106 736 718 718 779 705 825},
{79 481 746 245 311 133 178 032 755 021, 4 627 588 628 997 261 557 542 120 310},
{161 735 170 919 179 653 263 525 240 449, 1 681 703 453 911 392 458 183 213 309},
{58 036 229 393 509 478 309 415 794 215, - 3 642 651 347 366 543 228 185 382 109},
{48 992 240 706 687 454 968 513 586 271, - 3 348 804 036 778 961 896 954 127 091},
{246 724 149 154 397 723 673 865 698 706, - 16 728 731 274 318 973 181 003 080 685},
{837 157 172 116 987 934 194 921 802 231, 35 077 494 606 553 288 775 272 497 788},
{935 836 989 617 908 285 912 010 791 519, - 25 130 433 513 720 773 495 991 076 613},
{1 196 178 972 437 693 645 507 850 410 762, 54 252 352 981 125 651 544 520 454 771},
{522 814 163 732 932 994 151 680 754 200, - 22 619 577 118 900 216 593 300 584 971},
{510 214 109 647 374 488 647 692 673 533, 34 225 560 204 211 020 635 537 055 494},
{630 689 389 742 373 356 187 268 616 523, - 9 582 810 350 891 486 482 535 093 264},
{353 442 589 876 485 580 349 460 241 299, 1 231 023 960 727 278 793 474 318 763},
{27 603 916 403 556 757 843 820 507 282, - 409 790 196 637 875 001 718 492 705},
{29 446 672 535 007 413 007 617 713 353, - 15 000 051 594 991 838 475 726 398},
{312 679 553 648 381 873 592 021 721, 22 369 962 159 452 816 974 314 004},
{99 483 400 207 555 245 626 492 665, - 865 122 756 917 855 211 782 291},

```

```

{1 137 650 761 622 641 965 689 200, 71 171 207 734 752 716 654 309},
{216 623 864 546 898 655 169 056, 11 097 199 805 151 038 839 133},
{1 058 706 179 668 302 201 107 196, -48 369 349 439 475 353 864 243},
{1 078 482 092 030 961 197 323 850, 38 390 886 180 367 489 005 007},
{703 918 517 153 629 531 547 146, 48 785 657 372 080 187 874 909},
{4 162 943 474 956 873 358 385 580, 1 784 146 792 755 184 640 011},
{105 272 484 346 491 054 743 483, 2 197 236 586 877 052 337 550},
{38 779 492 897 884 034 324 483, -2 101 298 673 080 909 410 789},
{190 267 239 703 105 321 125 919, -2 247 635 587 066 728 074 776},
{155 575 254 315 746 480 778 159, -6 155 932 762 328 946 543 356},
{333 710 116 247 040 621 657 541, -9 252 557 999 417 896 290 069},
{122 987 625 331 274 687 796 343, 4 791 394 620 951 665 651 528},
{316 138 327 880 255 209 533 615, 13 991 071 833 007 593 667 393},
{1 125 608 531 504 969 518 468 376, 4 344 574 738 775 154 685 825},
{72 371 158 278 686 513 100 499, -246 784 705 937 826 329 803},
{12 584 648 341 776 295 175 780, 406 324 179 733 560 985 463},
{2 268 844 762 854 979 341 027, 147 227 127 918 993 129 028},
{12 027 130 969 946 398 715 793, -497 658 670 670 993 287 679},
{16 581 251 894 669 402 487 903, 36 821 535 275 951 621 812},
{2 300 643 077 743 361 828 097, -48 445 553 453 792 316 326},
{4 716 711 017 609 469 194 225, -17 626 578 764 748 874 224},
{1 435 206 177 302 590 463 593, -47 871 858 026 919 248 275},
{188 963 137 492 409 946 743, -1 420 461 682 473 641 613},
{8 305 010 959 706 830 586, 533 172 286 089 803 217},
{44 923 377 928 274 156 314, -1 355 318 305 141 149 079},
{39 376 897 864 631 104 693, -6 273 429 158 035 080},
{281 975 110 663 400 933, 15 656 893 518 534 630}, {30 054 438 625 741 007, 1 689 297 504 201 303},
{70 230 373 526 606 953, 1 570 839 201 442 482}, {91 020 717 122 642 663, 5 746 813 573 043 034},
{184 731 709 163 130 319, -12 946 444 951 680 708},
{692 814 488 080 480 993, 48 693 253 674 245 986},
{2 210 678 391 566 400 611, 25 182 603 472 596 784},
{1 072 752 090 401 159 819, -8 755 478 522 758 448},
{830 181 811 727 727 715, 48 602 459 388 441 442},
{784 060 422 720 416 999, -40 215 817 910 343 507},
{3 972 016 602 354 182 834, 100 764 499 941 130 703},
{8 398 019 825 366 997 983, 470 822 930 645 376 409},
{15 281 792 323 705 698 421, -159 979 026 201 057 769},
{15 162 644 127 573 633 197, 900 984 426 096 450 413},
{30 664 132 097 138 740 976, -550 206 156 605 996 347},
{29 335 121 886 613 836 744, -1 658 130 124 385 786 771},
{101 732 850 113 734 701 666, 3 809 309 966 024 131 937},
{222 585 274 814 455 265 967, -12 000 530 971 256 213 252},
{1 079 537 914 243 144 378 379, 28 311 730 135 424 605 013},
{734 741 650 304 868 189 115, -40 829 605 153 932 781 658},
{38 057 250 718 454 265 071, 155 260 941 520 778 377},
{3 645 689 126 848 978 494, 82 610 220 122 425 531},
{2 157 048 850 988 770 870, 93 556 079 281 944 629},
{1 046 546 473 304 836 197, 11 220 467 797 883 357},
{605 550 652 235 115 204, 26 721 218 057 890 943},
{1 798 435 256 178 920 515, -75 851 797 621 936 357},
{4 379 569 462 762 858 547, -222 981 449 530 893 845},

```



```

{15 931 846 043 148 652 247, 260 508 608 532 762 652},
{8 123 363 607 375 964 525, -246 284 203 546 718 352},
{799 006 823 482 477 109, -9 917 403 236 027 971},
{856 264 888 521 919 858, -22 953 883 036 317 259},
{1 387 272 019 458 073 725, 81 978 466 619 775 884},
{1 266 020 702 545 144 297, -78 112 681 982 595 660},
{3 227 340 373 899 133 663, -23 997 896 338 190 031},
{2 312 830 651 752 232 291, -56 941 951 141 995 515},
{4 336 079 668 847 180 976, -42 589 849 065 648 643},
{1 608 902 233 947 141 390, 34 706 937 728 323 117},
{2 464 236 590 411 323 592, 83 593 365 139 117 875},
{7 965 771 274 004 138 183, 383 305 103 660 939 023},
{16 643 544 672 240 678 700, -1 089 038 943 379 276 877},
{61 284 143 788 753 583 455, -2 378 226 732 614 319 203},
{109 400 500 584 524 448 777, -5 016 475 730 033 244 613},
{191 431 129 765 179 609 091, -6 013 286 883 422 070 209},
{197 816 050 361 000 881 803, -14 109 424 468 852 621 555},
{56 537 451 615 771 826 567, 1 766 535 866 004 656 892},
{1 652 476 820 938 398 577, -46 642 054 680 292 312},
{3 980 976 518 505 363 743, 508 026 091 622 760}, {16 728 845 333 860 217, 1 144 442 976 849 853},
{87 122 064 458 628 022, 787 092 066 194 969}, {48 785 822 913 693 863, -222 501 982 162 225},
{11 519 875 213 151 012, -629 724 044 675 423}, {36 783 639 389 686 202, -2 025 198 091 812 711},
{65 684 673 674 423 396, -984 608 534 811 417}, {56 535 533 430 367 057, -1 795 219 499 841 945},
{175 862 058 118 085 638, 1 545 267 249 758 317},
{59 383 262 518 137 500, 4 030 139 252 544 917}, {212 696 427 737 214 745, 3 897 296 350 897 787},
{329 319 440 870 544 460, -7 701 568 984 777 053},
{367 757 069 498 894 981, -21 577 196 394 043 232},
{188 001 429 231 847 363, 7 497 250 714 045 293}, {113 462 114 762 292 562, 3 831 688 428 764 127},
{296 219 082 025 618 352, 14 510 891 205 450 183},
{1 194 250 325 406 323 708, -70 952 803 006 456 739},
{2 377 517 814 984 730 145, -85 762 463 106 285 534},
{4 742 399 246 261 696 593, -210 855 035 516 163 809},
{20 614 104 516 312 466 205, 96 764 684 157 076 779},
{642 131 380 167 343 322, -20 676 421 182 469 751},
{231 302 378 645 427 159, -2 307 234 168 157 391},
{115 213 404 107 923 741, -5 812 486 817 570 612},
{206 230 116 454 211 301, 14 646 744 372 225 890},
{233 963 353 366 719 359, 16 613 355 957 559 045},
{273 897 622 217 653 071, -6 864 660 314 548 748},
{137 069 282 495 072 951, 7 772 804 201 814 624},
{565 397 434 380 465 919, 18 709 382 651 134 655},
{819 075 014 438 827 531, 22 923 740 638 580 514},
{1 229 750 061 464 123 627, -81 579 188 276 066 861},
{1 206 385 227 301 021 688, -60 209 288 851 245 723},
{437 690 604 945 338 372, 9 754 423 938 708 179},
{250 435 987 009 406 917, -6 858 444 036 804 850},
{661 962 028 122 134 067, 14 294 768 260 916 752},
{876 134 935 872 731 525, 35 743 863 385 736 598},
{3 474 868 105 366 001 575, -23 599 412 864 112 452},
{1 145 128 453 952 755 069, -23 698 714 683 819 576},
{1 510 439 676 753 668 779, -93 643 402 266 104 235},

```

```

{2 416 902 858 704 202 781, 32 197 591 398 823 438},
{414 617 254 696 541 269, 2 630 030 390 146 268},
{184 581 842 367 245 925, -12 297 680 079 547 007},
{23 211 593 634 123 180, -1 622 839 715 981 453}, {97 875 684 466 184 762, 5 110 582 645 043 799},
{154 148 227 860 163 619, 6 134 401 853 597 796}, {156 848 122 523 525 081, 9 310 972 289 790 301},
{286 242 874 179 097 164, -17 476 915 555 063 963},
{1 315 832 834 316 677 444, -26 324 589 863 228 005},
{78 935 110 099 838 394, 4 679 926 664 947 825},
{124 104 997 650 651 569, -8 937 107 202 437 926},
{201 886 133 512 399 605, 13 248 794 030 999 974},
{627 690 386 432 599 005, -16 191 570 694 400 969},
{752 393 259 158 718 414, 42 410 352 344 173 805},
{2 187 623 524 245 605 124, -150 875 507 037 389 891},
{14 997 918 718 707 183 350, 574 542 942 750 951 591},
{11 900 639 229 305 954 816, -127 378 939 754 590 767},
{10 825 168 593 673 683 515, -107 814 903 301 305 593},
{8 691 974 445 081 718 785, 78 218 169 800 424 988},
{1 941 761 849 674 478 283, 2 048 201 185 110 997},
{13 358 111 661 372 273, 740 202 773 885 656}, {6 857 884 554 662 535, 389 990 915 173 249},
{32 228 431 772 733 453, 2 234 103 679 305 320}, {189 245 072 229 335 627, 3 331 790 400 795 208},
{132 729 142 582 254 571, -5 383 402 390 894 598},
{369 327 520 831 965 421, -5 134 894 475 994 818},
{76 591 406 492 633 525, -5 019 680 293 846 518},
{257 944 214 902 215 245, 16 009 854 029 239 083},
{355 523 536 443 593 483, 25 553 233 382 814 344},
{442 124 452 245 659 267, 4 892 084 934 545 447},
{365 524 819 177 238 363, 14 711 054 685 506 639},
{448 058 044 125 094 788, 10 770 205 942 212 499},
{853 830 484 118 203 830, -28 002 496 720 013 491},
{2 737 360 921 042 020 900, 12 269 654 943 749 891},
{244 345 848 573 246 193, -15 303 706 369 980 898},
{102 177 215 943 186 825, -7 042 577 008 201 673},
{688 826 396 787 815 730, -3 871 482 382 204 693},
{59 195 981 679 305 176, 2 662 035 695 484 363},
{125 608 079 351 188 810, -1 091 051 042 580 553},
{27 304 681 430 617 785, 1 729 922 334 687 878}, {74 441 108 953 264 337, 2 887 913 229 420 342},
{128 282 367 321 246 445, 4 832 142 831 786 887},
{434 912 338 262 901 296, -10 908 648 930 806 273},
{285 290 174 900 575 176, 8 923 731 451 215 335},
{53 577 076 124 793 256, -3 471 342 060 625 513},
{299 882 097 866 701 639, 8 425 509 886 023 217},
{683 815 347 996 700 427, 17 398 741 537 527 106},
{1 047 621 178 595 515 307, -49 023 932 138 682 337},
{3 605 602 132 954 059 770, 227 588 133 837 827 667},
{7 125 793 681 785 397 498, 400 980 149 981 677 219},
{18 277 954 559 073 696 356, 113 595 713 415 659 699},
{2 180 104 868 655 521 417, -48 582 524 682 518 304},
{1 215 639 669 502 650 337, -75 521 170 373 466 989},
{1 452 887 761 908 524 087, 3 929 818 140 627 456},
{227 845 074 603 291 967, 14 851 476 064 840 824},
{1 009 513 792 505 241 793, 13 142 231 109 151 916},

```

```

{485 162 576 991 692 061, 673 120 394 776 663}, {31 288 300 814 110 438, -1 722 511 401 425 895},
{56 336 022 100 421 272, 2 030 657 841 438 399}, {103 957 094 510 926 100, 4 936 300 619 362 299},
{58 661 519 359 246 379, -772 493 646 835 534}, {9 551 562 250 586 795, 613 252 909 357 316},
{51 836 375 526 921 939, -1 172 614 165 664 780},
{48 029 095 296 652 181, -2 376 127 515 551 837},
{100 802 452 137 472 759, -2 775 628 943 686 315},
{175 082 222 788 318 381, 8 968 725 326 760 637},
{854 164 465 631 977 441, -42 109 138 786 257 009},
{2 384 356 291 460 614 939, -40 462 443 306 411 135},
{582 644 859 910 763 174, -14 238 048 627 965 765},
{221 911 633 330 805 009, -12 449 872 081 116 197},
{435 026 761 728 020 863, 5 086 013 919 049 856},
{471 716 626 743 083 847, 19 022 590 075 116 211},
{765 776 901 829 464 172, 8 755 957 985 802 019},
{797 702 855 873 015 281, -1 286 683 964 903 984},
{8 199 271 123 505 001, 348 216 591 410 222}, {31 427 486 997 725 073, -596 826 092 591 933},
{40 654 886 019 827 824, 276 764 830 316 587}, {5 879 263 305 382 535, -242 469 098 377 773},
{11 940 983 918 880 617, 472 664 207 401 369}, {24 751 368 035 432 008, 278 611 952 692 863},
{8 974 055 092 327 001, -517 149 930 330 555}, {36 318 749 064 805 634, -2 351 877 669 911 579},
{207 076 219 210 257 851, 14 807 327 172 820 115}, {45 045 880 635 528 041, 791 197 911 363 054},
{10 427 662 121 041 363, 590 957 131 519 846}, {41 703 683 016 857 135, -2 129 467 452 407 739},
{176 247 540 228 231 355, 12 814 984 507 032 781},
{629 286 331 175 288 221, 17 559 293 725 270 729},
{566 800 343 957 146 577, -25 139 557 159 003 057},
{2 270 484 669 284 823 066, 39 652 120 174 784 053},
{2 052 450 045 104 276 955, 114 152 145 894 464 617},
{455 427 618 221 144 049, -18 130 713 816 013 165},
{429 794 791 342 169 876, 24 725 835 224 082 333},
{1 881 662 914 021 272 785, -15 378 092 513 667 963},
{1 101 589 843 402 478 501, -10 109 738 286 428 888},
{73 954 333 835 787 909, -3 510 585 480 439 381}, {46 175 710 565 620 692, 1 222 349 020 261 709},
{54 436 888 660 525 750, 2 675 976 655 420 659}, {182 553 754 870 401 430, 453 134 203 420 541},
{11 806 492 507 242 007, -705 411 501 185 415}, {36 915 099 569 099 552, 507 617 001 721 393},
{28 047 369 755 865 263, 1 166 845 164 992 118}, {8 574 073 414 831 769, -202 596 084 169 332},
{12 942 538 064 245 175, -708 552 000 323 643}, {37 531 809 625 500 599, 1 204 103 983 974 197},
{40 712 638 337 797 908, 2 296 790 942 294 483}, {125 290 126 077 054 414, -602 395 477 082 267},
{1 618 498 055 367 278, 59 044 905 849 829}, {4 832 833 886 957 105, -222 863 264 878 264},
{13 961 430 132 575 897, -410 976 241 905 978}, {2 340 656 353 243 645, -79 889 763 101 178},
{4 746 791 438 587 117, 12 037 090 290 739}, {831 394 943 154 249, -27 780 172 994 519},
{400 039 089 582 879, -9 975 181 130 074}, {205 337 031 603 881, -10 110 901 719 760},
{620 680 444 527 519, -22 149 223 093 762}, {99 937 382 534 417, 5 117 570 823 383},
{480 392 752 715 357, 31 708 167 107 488}, {949 278 974 504 363, -53 583 047 061 246},
{3 027 958 647 014 935, 72 779 036 934 714}, {5 723 419 944 367 547, -303 902 558 182 957},
{10 095 003 560 618 564, 160 231 020 240 239}, {89 407 811 217 893, 3 327 261 700 320},
{85 222 683 458 653, -3 897 618 685 541}, {104 460 597 026 551, -741 836 362 612},
{27 527 690 246 459, -802 763 008 305}, {46 515 844 853 711, 2 938 744 353 249},
{100 308 894 856 327, -94 960 299 871}, {6 132 820 317 649, -128 820 410 770},
{10 061 320 462 889, 709 477 882 907}, {25 597 390 336 009, -564 273 915 989},
{40 807 759 184 296, 699 818 911 893}, {43 434 196 605 898, 12 619 574 431},
{473 338 535 196, -28 051 941 193}, {705 348 551 915, 31 703 974 297},
{1 564 362 358 819, -74 136 428 269}, {1 491 975 668 830, 31 654 889 709},

```

```

{834 974 648 893, -28 022 528 465}, {1 134 539 806 343, -44 905 021 667},
{2 370 938 668 932, 47 256 247 939}, {1 617 128 124 418, -22 482 159 259},
{315 881 103 770, 8 755 999 551}, {132 358 866 866, 6 480 882 909},
{545 500 528 514, 17 774 868 587}, {1 098 559 138 917, -15 185 127 059},
{1 040 768 143 131, 11 554 303 279}, {175 288 756 179, 293 017 711},
{12 768 835 199, 626 188 590}, {48 767 616 401, -3 311 564 868},
{180 265 467 181, 2 255 359 957}, {32 502 546 421, 1 155 807 702},
{27 846 222 235, -1 299 821 847}, {109 442 726 152, -3 481 507 681},
{301 681 620 159, 10 598 422 505}, {980 232 213 781, -33 632 579 770},
{972 592 689 749, -31 356 559 517}, {107 329 599 678, 802 434 379},
{39 124 814 492, -39 469 725}, {2 053 086 383, -75 444 457}, {3 201 122 756, -85 598 111},
{6 764 537 151, -275 648 132}, {25 206 563 651, -245 796 547}, {21 985 657 310, 854 412 703},
{45 585 520 632, 2 692 889 975}, {38 528 179 657, -2 492 467 060},
{227 093 577 643, 409 639 355}, {30 521 619 627, 1 456 495 739}, {12 893 387 508, -486 528 389},
{48 332 920 005, -1 789 722 559}, {2 071 771 488, 106 619 399}, {9 154 578 493, -128 088 447},
{11 999 452 444, 740 357 907}, {30 591 460 468, 215 506 569}, {2 083 993 670, -64 449 861},
{4 298 025 482, -298 613 899}, {23 368 748 304, -1 530 734 173}, {81 139 406 091, 2 816 624 159},
{107 996 209 480, 6 064 871 239}, {233 123 091 578, 16 108 249 607},
{1 513 911 818 920, -103 763 058 007}, {8 464 276 185 815, -320 438 690 812},
{26 441 174 715 897, 1 737 721 306 991}, {74 695 667 095 368, -2 523 002 946 487},
{197 889 838 549 158, 11 827 885 824 607}, {633 659 873 363 039, -45 189 438 955 068},
{200 537 870 425 313, 8 328 073 262 552}, {132 158 312 688 935, 990 941 829 738},
{72 246 817 422 419, -2 842 758 795 469}, {234 391 659 603 106, 14 969 834 798 811},
{1 020 013 738 396 130, -6 092 761 798 789}, {501 981 081 675 033, 31 141 775 235 920},
{738 822 902 162 287, -47 510 956 378 386}, {4 249 127 578 485 911, 166 386 366 327 099},
{15 306 671 257 713 937, 348 419 619 025 704}, {4 734 603 903 990 761, -338 763 876 701 996},
{1 609 983 597 599 417, 77 863 308 823 095}, {5 004 031 649 430 022, -180 952 855 278 903},
{12 467 011 377 473 138, -326 394 859 470 263}, {12 737 336 803 025 656, 14 241 332 608 823},
{1 111 504 696 840 906, 80 397 975 374 035}, {2 799 324 720 721 216, -89 467 154 027 461},
{5 142 746 228 115 075, 182 726 674 003 061}, {5 253 471 849 844 033, 380 285 858 581 918},
{14 035 503 890 260 981, 1 986 877 123 105}, {40 574 636 804 939, -774 866 130 228},
{56 038 008 583 517, 962 156 313 361}, {46 355 539 307 221, 2 319 870 592 691},
{8 332 636 773 201, -218 784 424 529}, {3 746 899 578 701, 144 346 868 409},
{1 217 680 986 667, 22 034 871 843}, {1 146 844 025 098, 39 610 879 049},
{372 421 997 277, -13 044 837 536}, {1 169 779 962 133, 38 865 968 519},
{756 380 406 037, 18 487 412 391}, {319 096 896 806, -5 371 997 555},
{427 659 171 139, -9 550 270 372}, {418 496 124 599, 9 910 758 729},
{446 607 338 219, 19 736 543 601}, {1 459 299 756 196, -99 660 253 311},
{7 085 204 650 331, 214 562 457 470}, {924 067 210 379, 9 738 760 077},
{221 884 390 264, 2 081 413 317}, {164 540 096 345, -6 571 765 168},
{48 947 461 855, -2 433 629 917}, {54 697 839 485, 1 941 204 552},
{68 478 293 771, -2 890 998 951}, {180 230 529 547, -2 515 720 565},
{179 368 875 467, 3 983 918 152}, {18 419 166 773, 960 658 263},
{33 165 295 424, -2 154 345 823}, {169 171 507 721, -9 611 535 830},
{763 391 306 581, 21 479 981 203}, {1 967 715 328 673, 26 771 016 848},
{2 654 643 697 721, 88 574 387 322}, {514 996 465 861, 10 384 937 207},
{845 828 503 311, 28 841 978 884}, {1 872 812 019 325, 8 184 351 841},
{279 505 900 536, 594 609 881}, {7 812 036 734, -70 135 137}, {5 380 268 873, 156 174 831},
{13 994 599 181, 487 582 104}, {28 911 085 165, -125 854 751}, {7 066 005 435, 331 830 209},
{19 416 638 154, 954 323 909}, {65 701 834 826, -1 582 327 029},
{150 424 178 008, 7 987 519 619}, {266 400 255 847, 2 191 657 136},

```

```

{195 401 034 255, -9 006 855 989}, {547 209 703 097, 37 993 534 897},
{3 044 742 693 261, 17 707 676 776}, {194 564 729 989, -7 974 567 668},
{631 846 085 443, -21 611 729 131}, {1 016 082 188 156, -6 638 015 465},
{92 698 580 189, 2 901 077 727}, {27 045 507 925, -1 883 912 123},
{133 476 902 397, -5 321 762 624}, {86 134 522 603, -4 640 324 684},
{404 297 632 207, -19 259 314 236}, {29 445 383 051, 708 634 111},
{63 132 672 589, -3 014 607 304}, {34 642 078 205, -845 970 049}, {8 496 066 996, -36 323 225},
{709 963 146, -14 015 845}, {964 144 851, -20 917 265}, {388 181 539, 23 582 771},
{2 160 583 397, -29 911 876}, {1 378 736 675, 75 179 426}, {5 075 894 393, 166 641 714},
{15 251 951 627, -177 992 169}, {11 019 606 493, 91 250 965}, {4 330 294 128, 141 446 717},
{10 856 265 701, 329 342 995}, {2 398 573 666, 174 430 563}, {8 647 388 984, 573 141 355},
{10 003 463 141, 347 422 987}, {14 288 892 918, -421 242 139}, {6 634 621 792, -289 149 923},
{3 149 460 963, 170 000 552}, {16 029 355 475, -1 127 002 698}, {50 012 222 897, 1 661 078 095},
{35 796 129 353, 1 913 695 036}, {112 251 189 869, -4 586 399 387},
{433 343 311 619, -28 586 018 127}, {906 054 903 086, -10 977 083 915},
{1 003 569 309 941, -9 292 209 580}, {2 124 384 899, -6 093 103}, {419 501 552, -10 140 343},
{745 750 311, 46 938 182}, {1 046 859 599, -34 695 049}, {1 195 617 671, 65 114 889},
{4 686 384 131, -18 004 708}, {1 026 850 149, 8 458 604}, {668 453 935, 27 243 151},
{2 512 343 160, 70 418 351}, {4 520 777 724, -178 308 965}, {12 547 666 201, -740 950 986},
{9 651 611 639, -234 962 031}, {3 615 505 232, 135 113 639}, {6 480 041 179, -446 441 109},
{43 098 515 744, 912 145 555}, {45 307 257 141, 3 247 707 448}, {31 968 779 069, 1 274 802 909},
{19 642 562 456, -1 075 294 973}, {57 163 335 458, 2 605 018 641},
{29 267 854 156, 1 951 380 913}, {569 048 261, 20 611 286}, {1 605 481 653, 109 718 020},
{8 017 440 753, 365 158 517}, {3 193 277 579, -71 631 479}, {5 997 656 224, 270 179 457},
{10 687 925 830, -748 080 607}, {42 744 669 068, 630 902 279}, {31 180 494 896, 1 679 400 527},
{144 894 908 283, 3 644 709 415}, {177 800 195 083, 199 099 819}, {807 286 484, -25 421 487},
{1 234 018 900, 23 582 713}, {1 535 846 976, -7 194 929}, {662 092 701, 15 497 194},
{853 041 559, 23 873 119}, {1 271 754 275, 67 855 969}, {3 484 318 064, 206 315 657},
{4 586 572 895, -284 717 998}, {6 185 900 473, 133 280 027}, {10 948 826 969, -601 755 510},
{23 328 330 011, -763 140 655}, {65 477 028 506, -805 066 071}, {53 068 674 245, 2 197 995 666},
{63 038 873 939, -3 554 201 778}, {186 414 854 935, 970 572 812},
{12 910 131 169, -637 728 009}, {30 958 626 811, -584 230 723}, {1 114 700 092, -47 798 235},
{3 052 796 713, -169 370 382}, {821 837 563, -50 664 305}, {2 230 527 917, -5 590 678},
{30 368 395, 1 733 127}, {164 750 309, -8 768 527}, {368 489 096, 26 555 561},
{654 462 842, -38 987 629}, {1 657 043 349, 31 220 443}, {469 614 130, -14 828 773},
{976 414 594, -37 197 227}, {1 848 051 708, -130 768 337}, {3 441 703 010, 57 945 857},
{4 556 591 953, 242 784 172}, {11 205 155 685, 673 313 822}, {47 994 678 511, -1 099 662 339},
{77 702 416 595, 3 686 918 306}, {55 149 301 631, 2 344 948 903},
{224 764 936 159, -8 079 183 051}, {288 985 664 531, 7 444 852 711},
{271 354 648 402, -18 392 334 035}, {901 542 062 477, -18 579 570 911},
{1 762 525 520 238, 101 428 273 517}, {7 610 729 219 351, 220 404 055 505},
{20 579 131 941 476, 1 124 127 600 445}, {68 622 191 559 734, 3 696 577 337 247},
{320 942 791 743 841, 12 710 031 340 823}, {635 209 636 429 934, 29 953 798 006 499},
{1 229 795 780 397 545, 46 662 276 456 866}, {3 298 741 911 286 771, 152 090 536 931 355},
{9 402 730 339 404 761, -120 579 881 800 763}, {497 587 769 895 847, -6 337 206 222 210},
{607 252 810 089 857, 22 186 244 770 132}, {1 636 616 057 962 307, -116 472 205 001 175},
{1 195 032 401 225 543, -15 958 888 063 376}, {374 956 502 003 743, 6 588 391 092 750},
{115 776 266 318 393, 4 919 792 704 584}, {457 452 959 732 977, 20 921 239 143 789},
{560 045 984 645 819, -974 774 080 512}, {89 373 218 067 619, -1 383 525 110 847},
{110 626 913 349 764, 1 255 827 302 605}, {22 708 033 384 276, -1 590 394 816 501},
{88 058 684 699 138, 4 328 247 631 251}, {297 252 682 749 482, -5 043 324 369 491},

```

```

{60 387 555 046 913, 399 152 618 687}, {22 986 415 410 024, -963 328 003 783},
{26 557 879 472 832, -1 809 914 360 783}, {117 576 351 843 687, 353 870 997 800},
{18 144 934 243 313, -974 060 947 921}, {72 082 529 670 014, 4 757 322 165 187},
{143 816 741 249 591, 3 587 275 039 468}, {64 822 194 503 329, -4 062 501 745 552},
{35 388 851 675 097, -1 237 738 950 311}, {100 609 998 900 478, -2 939 845 661 657},
{130 394 034 423 860, 4 037 230 652 117}, {239 328 057 667 084, 1 238 977 841 911},
{40 861 501 473 939, 2 414 252 587 960}, {35 977 711 754 819, 1 918 182 040 468},
{93 081 655 800 527, -1 907 650 625 856}, {78 251 748 416 983, 3 306 277 384 275},
{218 682 852 317 783, 11 286 263 150 028}, {844 526 640 982 949, 30 675 378 950 550},
{2 862 409 956 857 749, 152 626 378 956 735}, {7 460 757 420 722 984, 70 240 163 625 127},
{3 044 715 215 444 878, -220 678 393 036 143}, {8 911 675 125 163 676, -240 334 828 075 807},
{3 838 010 785 404 583, 273 866 191 804 005}, {772 935 929 554 087, -17 857 515 531 473},
{1 007 489 578 448 852, -29 963 447 042 519}, {2 242 256 578 362 006, 81 027 801 134 813},
{5 277 848 829 138 842, 27 276 302 541 835}, {2 690 965 274 372 713, -62 125 851 437 757},
{3 891 178 847 283 238, 112 192 270 251 713}, {7 074 571 693 816 683, 355 028 373 954 559},
{5 173 161 269 624 903, 213 864 241 321 581}, {8 043 476 103 484 841, 361 049 088 129 423},
{19 978 836 762 869 465, -938 450 824 457 698}, {54 002 520 402 303 593, 2 121 422 616 351 770},
{192 424 043 708 359 257, 1 537 678 477 438 025}, {42 632 571 692 620 268, 1 571 462 360 853 403},
{40 414 501 966 099 013, 574 831 307 846 378}, {35 085 772 953 658 047, 1 905 384 309 500 408},
{156 982 221 147 489 897, -9 734 226 056 215 387},
{245 686 245 360 697 295, -3 720 732 750 419 983},
{23 458 882 762 704 983, 1 417 143 599 601 564},
{125 879 127 673 799 395, -6 848 659 043 813 061},
{518 049 712 147 695 103, -3 978 879 663 036 105},
{158 275 834 647 289 147, -7 576 083 284 752 237},
{163 560 952 169 058 170, 6 003 088 173 889 753},
{294 036 723 332 932 961, -5 173 490 312 228 421},
{169 592 668 353 320 164, -8 484 825 124 554 069},
{20 662 993 414 481 984, -797 387 450 963 373}, {13 746 981 802 577 086, 417 111 235 660 453},
{3 520 105 869 354 737, 97 664 979 090 227}, {829 157 799 206 435, -18 627 776 596 812},
{1 809 337 382 370 895, 15 515 596 822 958}, {1 191 501 737 123 009, 37 842 999 961 060},
{3 655 378 927 699 651, 73 049 230 210 446}, {580 566 018 292 849, -15 280 068 748 034},
{15 242 232 356 157, -129 971 260 777}, {7 083 374 204 352, -58 018 089 823},
{1 028 281 943 254, -7 139 677 359}, {33 512 308 042, 361 831 521}, {27 466 658 789, 43 747 863},
{1 392 835 825, 22 146 488}, {476 190 881, 34 106 552}, {258 868 553, 3 217 492},
{292 369 407, 1 181 953}, {84 976 184, -77 169}, {2 609 885, -143 231},
{6 313 673, 19 604}, {235 815, -16 414}, {1 197 781, 50 083}, {837 989, 47 241},
{2 457 451, -89 813}, {6 467 500, 34 713}, {2 165 518, -34 829}, {1 217 880, -9251},
{647 148, -45 211}, {2 824 606, 58 783}, {601 378, 41 963}, {2 765 304, -112 027},
{7 038 829, -273 325}, {13 456 579, -516 577}, {5 089 823, 302 064}, {9 007 735, 272 774},
{1 232 407, 43 732}, {1 574 289, -15 254}, {622 273, -43 007}, {4 014 825, 217 732},
{19 034 151, -1 052 468}, {17 855 673, -1 274 492}, {2 544 215, -20 648},
{897 689, -53 563}, {2 563 518, -174 725}, {11 414 043, -160 138}, {8 804 755, 210 163},
{4 396 109, -180 902}, {10 837 739, 325 989}, {15 940 298, -171 013}, {7 181 711, 505 586},
{20 597 893, -1 446 288}, {69 622 339, -3 724 180}, {226 279 119, 15 654 142},
{1 417 105 069, 17 482 273}, {207 150 244, 7 384 067}, {78 877 232, -1 888 683},
{89 043 346, -460 897}, {17 954 775, -140 128}, {3 659 809, -151 844}, {3 095 047, 2523},
{134 126, 6119}, {97 908, -4901}, {22 288, 899}, {37 213, 58}, {4577, -203},
{18 308, 377}, {32 835, 1537}, {111 042, -1595}, {120 992, 29}, {796, -29}

```

```

29
200 is a relation number with a list {{200, 203}, {600, 29}, {900, -29}, {1, 0}}
29
201 is a relation number with a list
    {{201, 203}, {402, 29}, {804, -29}, {1608, 29}, {871, 58}, {1, 0}}
29
202 is a relation number with a list {{202, 203}, {1, 0}}
29
204 is a relation number with a list {{204, 203}, {1, 0}}
29
205 is a relation number with a list {{205, 203}, {410, 29}, {820, 29},
    {1640, -87}, {2665, 116}, {615, -29}, {1230, -29}, {2460, -29}, {1, 0}}
29
206 is a relation number with a list {{206, 203}, {618, -29}, {1854, 29}, {1, 0}}
29
207 is a relation number with a list
    {{207, 203}, {828, 29}, {2691, 29}, {414, 29}, {1656, -29}, {1, 0}}
29
208 is a relation number with a list {{208, 203}, {1040, 29}, {1, 0}}
29
209 is a relation number with a list {{209, 203}, {1254, -29}, {1463, 29},
    {2717, 29}, {1881, -58}, {5225, 203}, {11077, 609}, {1265, 29}, {1, 0}}
29
210 is a relation number with a list {{210, 203}, {1, 0}}
29
211 is a relation number with a list {{211, 203}, {1688, -87}, {7385, -87},
    {2110, 87}, {4642, -145}, {422, 29}, {2743, -87}, {8651, 522}, {47053, -203},
    {9073, 435}, {13082, -87}, {6752, 203}, {11183, -203}, {3798, -29}, {1, 0}}
29
212 is a relation number with a list {{212, 203}, {1908, -29}, {636, 29}, {1, 0}}
29
213 is a relation number with a list
    {{213, 203}, {2130, 29}, {2769, 145}, {2982, 29}, {1065, 58}, {1491, 58},
    {3621, -29}, {852, 29}, {2343, 116}, {4899, 29}, {426, 29}, {639, 29}, {1, 0}}
29
214 is a relation number with a list {{214, 203}, {1177, 29}, {1284, 29}, {856, -29},
    {749, 29}, {1070, 29}, {642, -29}, {428, 29}, {1498, 87}, {2033, -58}, {642, 29}}
29
215 is a relation number with a list
    {{215, 203}, {516, 29}, {1290, 29}, {602, 29}, {1505, 58}, {645, -29}, {1505, 58}}
29
216 is a relation number with a list {{216, 203}, {702, 29}, {1, 0}}
29
217 is a relation number with a list {{217, 203}, {434, 29}, {1, 0}}

```

```

29
218 is a relation number with a list {{218, 232}, {1526, 87},
    {4360, -203}, {10573, 377}, {3706, -145}, {6976, 29}, {2834, 87}, {4033, 174},
    {3379, 87}, {763, 29}, {981, 29}, {545, 29}, {654, -29}, {2834, -87}}

29
219 is a relation number with a list
    {{219, 232}, {949, 29}, {584, -29}, {876, 29}, {438, 29}, {1, 0}}

29
220 is a relation number with a list
    {{220, 232}, {660, 29}, {1540, -87}, {572, 29}, {440, 29}, {1, 0}}

29
221 is a relation number with a list {{221, 232}, {2431, 87},
    {1105, 58}, {663, 29}, {884, -29}, {3094, 87}, {494, -29}, {1, 0}}

29
222 is a relation number with a list
    {{222, 232}, {555, 29}, {444, 29}, {666, -29}, {1, 0}}

29
223 is a relation number with a list {{223, 232}, {2007, -58},
    {5129, 261}, {20293, -145}, {1561, 58}, {1115, -29}, {2899, -58}, {1, 0}}

29
224 is a relation number with a list {{224, 232}, {1, 0}}

29
225 is a relation number with a list {{225, 232}, {1575, -29}, {1, 0}}

29
226 is a relation number with a list
    {{226, 232}, {678, -29}, {2486, 145}, {2373, -58}, {565, 29}, {1582, 29},
    {2938, -145}, {4294, 145}, {6328, -145}, {5876, -203}, {1243, -29},
    {452, 29}, {1356, 29}, {791, -29}, {904, -29}, {1130, -29}, {1, 0}}

29
227 is a relation number with a list {{227, 232}, {1135, -29},
    {908, 29}, {2043, 58}, {2951, -29}, {1589, 87}, {5221, -261}, {1, 0}}

29
228 is a relation number with a list {{228, 232}, {1, 0}}

```



```

29
229 is a relation number with a list
229
{{229, 232}, {687, 29}, {2061, -116}, {6183, -58}, {5267, -58}, {2519, -116},
{7557, -232}, {22671, -1421}, {14885, -696}, {61601, -3364}, {240221, -9831},
{979433, -18705}, {1551017, 37729}, {945312, 20677}, {1335070, -1073},
{59082, 1189}, {84272, 5191}, {278464, -10237}, {472885, -8758}, {10763, 609},
{45571, -957}, {83585, -3132}, {224191, 7453}, {137629, -1305}, {138316, -1073},
{23129, -319}, {36182, -261}, {22213, 696}, {13511, -261}, {13969, -377},
{4580, 87}, {7099, -145}, {1374, -29}, {2519, 58}, {5725, 232}, {17175, -928},
{104653, 464}, {48319, -2233}, {184803, -3509}, {268846, -13543}, {461206, 5829},
{163735, 7801}, {19694, -725}, {27251, -377}, {24503, 551}, {59311, -1508},
{114271, 1972}, {24045, -928}, {19007, 696}, {49235, -2726}, {38243, 493},
{48319, -2755}, {291059, 4292}, {182513, 10991}, {992486, -3219}, {236786, 12499},
{159155, -261}, {12595, 754}, {51067, 1943}, {125721, -841}, {94348, -1421},
{128698, 551}, {54044, -2987}, {63662, 1247}, {14885, 928}, {8473, 58},
{1145, -58}, {3435, -203}, {3664, 87}, {2290, -87}, {6412, 377}, {687, 29}}

29
230 is a relation number with a list {{230, 232}, {1, 0}}
230

29
231 is a relation number with a list {{231, 232}, {1, 0}}
231

29
233 is a relation number with a list {{233, 232}, {1, 0}}
233

29
234 is a relation number with a list {{234, 232}, {1, 0}}
234

29
235 is a relation number with a list
235
{{235, 232}, {705, -29}, {2115, -29}, {470, 29}, {1410, 29}, {2585, -116},
{7755, -464}, {31255, 1044}, {3055, -58}, {893, -29}, {1410, 29}}

29
236 is a relation number with a list {{236, 232}, {1, 0}}
236

29
237 is a relation number with a list
237
{{237, 232}, {1185, 29}, {948, -29}, {711, 29}, {3318, 29}, {948, -29}}

29
238 is a relation number with a list
238
{{238, 232}, {714, 29}, {1309, 58}, {5950, -29}, {595, 29}, {1, 0}}

29
239 is a relation number with a list {{239, 232}, {1673, 29},
239
{2151, 116}, {12667, -58}, {5497, 145}, {3107, 29}, {956, -29}, {1, 0}}

29
240 is a relation number with a list {{240, 232}, {1, 0}}
240

```

```

29
241 is a relation number with a list
    {{241, 232}, {2169, 58}, {5543, -29}, {964, -29}, {1687, -87}, {8194, -261},
    {24823, -174}, {14219, -841}, {18798, -899}, {19521, 551}, {56876, 2755},
    {235939, -10962}, {1259225, 65917}, {1639282, -91901}, {3599576, 57797},
    {3895042, -131863}, {14664368, 16327}, {656002, -12093}, {718180, 23867},
    {522970, 25317}, {2093567, -55245}, {1384063, -9715}, {1092453, 24911},
    {875071, -1508}, {103871, -957}, {106522, -87}, {8194, -261}}

29
242 is a relation number with a list
    {{242, 232}, {605, -29}, {484, 29}, {2178, 29}, {726, -29}, {1, 0}}

29
243 is a relation number with a list {{243, 232}, {891, -29}, {648, 29}, {810, 29},
    {486, 29}, {1701, 58}, {4617, -232}, {5589, -319}, {4131, 232}, {1215, -29}, {1, 0}}

29
244 is a relation number with a list {{244, 232}, {732, -29}, {1708, 29}, {732, -29}}

29
245 is a relation number with a list
    {{245, 232}, {3185, -87}, {8330, -377}, {8820, -493}, {1890, 29}, {1, 0}}

29
246 is a relation number with a list {{246, 232}, {574, -29}, {1, 0}}

29
247 is a relation number with a list
    {{247, 261}, {3458, 87}, {5434, 203}, {11609, 290}, {2223, 116}, {1, 0}}

29
248 is a relation number with a list
    {{248, 261}, {806, 29}, {744, -29}, {1240, -29}, {1736, 87}, {1, 0}}

29
249 is a relation number with a list {{249, 261}, {996, 29}, {2490, -29}, {996, 29}}

29
250 is a relation number with a list {{250, 261}, {550, 29}, {1, 0}}

29
251 is a relation number with a list
    {{251, 261}, {2510, 29}, {3263, -116}, {3765, 29}, {1255, -29}, {2008, -87}, {1757, 87},
    {4267, 145}, {15562, 435}, {24598, -1189}, {93121, -2813}, {73292, -3219},
    {186995, 8584}, {465103, -5104}, {160389, -2465}, {41164, -435}, {40411, 1798},
    {214605, 4988}, {30371, -725}, {19829, 986}, {27359, 928}, {112197, -406},
    {35391, 319}, {4518, -203}, {13052, 319}, {6777, -203}, {19578, 1073}, {66264, 1363},
    {131273, 6728}, {825037, 27086}, {3126707, -65221}, {979151, -33234},
    {3856615, 124381}, {201804, -493}, {41917, 2175}, {148592, -3451},
    {49949, -551}, {48192, -899}, {88854, -203}, {15060, 493}, {55973, -870},
    {73543, 2552}, {116715, 6728}, {587089, -7047}, {549188, 7859}, {236442, -5713},
    {554459, -24621}, {2967824, 7743}, {566005, -18357}, {768562, -9889},
    {697780, -17081}, {637791, 13369}, {984171, 55651}, {4404297, -229100},
    {12900647, 625907}, {61093400, -1813457}, {141598638, -2902349},
    {154732213, -4484908}, {562131317, 21605377}, {98270265, -4231303},
    {238524296, 12727723}, {828912691, -34222436}, {1901130977, -23380699},
    {1830883858, 54463247}, {5237501540, 247707183}, {8948324947, 142290153},

```

```

{4 004 627 692, -88 001 167}, {10 899 923 490, -580 073 863}, {30 491 456 657, 1 158 930 190},
{90 177 200 967, -837 156 514}, {59 161 338 795, -1 770 302 941},
{186 076 777 242, 7 131 082 687}, {167 825 472 380, 6 003 904 597},
{71 247 940 336, -554 478 695}, {68 941 511 376, -3 763 136 077},
{302 470 559 490, -983 617 157}, {121 364 741 366, -5 512 073 645},
{24 879 415 176, -889 200 871}, {4 570 512 212, -182 984 983}, {1 032 203 113, 14 697 838},
{841 967 703, -7 449 868}, {33 287 369, -784 682}, {83 011 975, 4 456 343},
{416 294 042, -12 294 579}, {432 132 644, -9 576 583}, {297 788 659, 4 687 937},
{562 066 559, -7 752 889}, {968 496 301, -43 709 496}, {1 728 734 639, 14 301 959},
{452 402 400, 16 810 691}, {373 050 507, 4 458 953}, {376 887 795, 12 967 727},
{206 751 712, 6 179 349}, {711 131 945, -10 073 846}, {1 031 891 371, 24 862 657},
{3 097 395 973, -156 796 968}, {9 674 390 137, 234 501 163}, {15 020 455 954, -144 867 731},
{11 492 805 570, 509 741 671}, {58 044 468 613, -524 831 908}, {53 180 166 925, 2 702 045 333},
{216 045 673 485, -4 254 166 078}, {230 115 919 743, 4 311 753 698},
{399 836 410 999, 19 736 687 615}, {1 280 767 333 449, 70 664 216 422},
{2 211 670 901 103, 105 031 178 069}, {1 510 056 575 154, 18 053 812 453},
{1 622 381 395 398, -32 791 980 695}, {3 909 159 677 093, -100 980 973 399},
{7 303 669 652 468, 30 715 965 989}, {1 689 293 481 414, 97 385 917 001},
{8 466 955 991 647, -12 481 820 574}, {1 074 692 261 225, -28 746 169 699},
{2 782 079 572 862, -143 707 847 493}, {12 959 248 094 245, -135 862 256 223},
{13 135 772 018 060, -712 491 859 693}, {78 040 554 440 086, 1 497 298 496 937},
{45 439 182 439 862, -2 174 144 736 669}, {54 682 114 576 937, 2 374 895 617 541},
{14 938 358 746 994, 647 488 195 321}, {11 578 693 907 361, 648 473 595 572},
{23 551 534 046 685, 498 742 018 328}, {27 775 455 502 519, 28 708 061 089},
{3 500 855 539 883, 74 940 379 087}, {5 356 911 578 706, -242 253 981 617},
{6 858 319 766 132, 208 704 947 889}, {7 264 822 065 455, -344 503 379 549},
{7 593 024 826 426, 380 545 265 747}, {4 488 002 617 014, -106 574 991 793},
{2 975 093 388 708, 61 076 443 453}, {4 430 737 462 739, 27 348 918 727},
{53 369 870 215, 1 553 497 172}, {138 292 558 117, 6 455 198 740},
{686 079 528 827, 34 891 829 080}, {2 951 020 246 023, 106 968 691 762},
{11 069 883 951 563, 9 660 465 355}, {253 345 662 017, 4 717 253 564},
{347 893 640 189, -18 379 045 365}, {328 363 658 246, -15 348 150 733},
{1 519 175 706 103, 9 104 606 231}, {324 677 152 974, 3 006 320 525},
{1 371 395 226, -56 818 627}, {1 944 792 678, -105 554 171}, {11 249 217 600, -499 888 921},
{62 305 123 333, 3 095 920 752}, {97 063 781 543, 3 272 814 459},
{281 283 708 977, -9 003 564 634}, {545 474 536 073, 8 931 634 078},
{161 859 186 065, -2 263 302 622}, {275 749 282 469, -5 381 661 196},
{322 424 929 723, -9 714 782 384}, {461 114 873 801, 12 295 763 650},
{1 537 160 369 649, -67 033 240 943}, {1 155 647 182 040, 1 698 842 533},
{108 999 159 600, -1 770 489 817}, {193 573 472 554, -2 908 307 253},
{322 061 462 647, -14 220 649 757}, {1 258 383 922 764, -65 391 189 893},
{4 003 780 014 047, -222 604 144 188}, {776 739 915 587, -36 160 824 391},
{4 358 013 447 376, -13 087 959 869}, {69 574 439 251, -2 660 813 742},
{98 713 771 709, 5 041 182 607}, {529 579 988 181, 19 580 348 122},
{228 557 810 637, 2 950 922 144}, {335 538 192 799, 4 101 600 645},
{199 058 082 841, 5 441 656 860}, {573 088 465 729, 24 625 704 351},
{1 681 013 679 656, -34 010 736 667}, {3 636 383 326 223, -133 896 779 077},
{5 313 743 077 144, 158 522 826 353}, {19 084 287 733 358, -99 993 570 727},
{3 635 553 150 249, -104 253 115 783}, {3 339 781 441 156, -71 706 990 099},
{7 642 220 467 747, 339 140 286 589}, {39 659 537 073 800, 1 937 162 279 961},
{229 989 160 119 580, 7 923 582 539 451}, {51 521 885 350 751, 608 135 699 515},

```

```

{42 581 926 114 024, -127 512 464 689}, {1 816 510 117 602, 104 526 651 323},
{9 928 818 322 861, -148 359 606 964}, {2 830 111 275 477, -38 025 013 498},
{4 081 329 432 875, -113 317 945 498}, {472 732 131 697, 13 409 934 225},
{849 492 889 322, 28 841 741 983}, {3 283 675 325 565, 30 890 367 668},
{2 333 384 542 007, -64 750 383 969}, {595 050 499 873, -27 144 698 407},
{535 349 135 331, 9 479 691 767}, {1 126 085 491 129, 37 503 723 679},
{244 418 970 509, 9 633 853 766}, {896 729 216 109, 35 155 513 813},
{4 345 849 900 279, 213 948 694 075}, {16 785 880 713 529, -602 205 035 723},
{19 040 931 965 465, -642 969 750 242}, {62 288 295 990 545, 3 058 981 645 532},
{278 274 433 056 155, -3 825 110 585 348}, {240 618 558 236 499, -12 916 512 440 387},
{1 203 589 710 844 354, 43 660 809 257 519}, {4 747 150 039 910 678, 10 646 928 745 971},
{346 425 378 889 388, 9 312 164 371 163}, {470 699 586 245 607, -1 142 296 815 266},
{18 397 887 359 765, 246 563 166 959}, {23 681 890 702 160, 1 044 203 254 011},
{84 030 819 163 343, 40 964 936 058}, {2 945 562 404 635, 72 480 655 608},
{6 562 263 298 543, 3 910 246 320}, {218 363 369 333, -2 468 296 053},
{289 482 483 919, 15 935 175 316}, {664 981 385 981, 4 542 031 968},
{463 024 381 903, 16 616 364 291}, {560 688 379 495, -24 740 774 321},
{2 095 706 901 888, -85 535 780 981}, {10 714 593 281 887, 424 483 066 190},
{25 731 673 411 387, -482 109 117 338}, {45 152 438 310 723, -1 022 630 072 347},
{39 335 496 991 205, -2 174 781 172 177}, {47 548 408 896 769, -1 999 628 229 878},
{111 109 823 696 053, 1 248 476 136 685}, {1 142 669 696 912, 51 764 407 617},
{967 035 063 838, 32 284 818 835}, {378 884 804 212, -5 015 525 205},
{576 072 953 368, -5 709 537 313}, {148 169 126 495, -4 914 071 257},
{187 494 185 035, 1 340 576 098}, {46 803 639 935, -1 213 904 968},
{135 202 108 067, -7 729 066 892}, {955 800 696 653, 47 765 021 474},
{125 567 060 423, 5 620 527 932}, {480 776 925 669, 22 054 219 657},
{1 108 392 603 035, -28 973 373 012}, {1 858 511 573 329, 28 449 952 882},
{2 325 423 635 749, -113 271 813 835}, {13 374 398 151 286, 616 739 874 293},
{48 663 649 873 160, 2 628 107 078 377}, {318 866 538 616 753, 3 485 892 880 939},
{414 221 899 277 304, 13 509 585 535 001}, {1 148 388 329 239 477, 58 834 270 740 907},
{7 102 568 480 244 413, 3 676 716 094 429}, {212 600 562 296 165, 10 553 900 339 651},
{382 161 431 289 395, -217 590 219 899}, {18 324 291 834 501, 430 735 455 605},
{49 530 521 885 014, 615 749 482 359}, {67 911 387 369 794, -2 373 591 778 411},
{231 616 325 235 375, 7 041 594 149 411}, {189 826 705 492 188, 9 065 570 494 451},
{138 118 997 712 033, 6 531 780 043 400}, {238 855 816 958 883, 11 260 445 010 337},
{599 004 407 193 306, -11 143 203 412 747}, {684 872 850 853 032, 27 438 305 142 017},
{272 279 202 045 643, 2 408 565 496 676}, {27 936 531 235 005, 965 043 699 811},
{12 483 750 938 014, 88 113 299 647}, {7 112 740 576 860, 71 911 874 983},
{1 640 296 660 707, -45 827 631 698}, {2 384 018 185 671, -65 926 396 580},
{2 677 645 106 541, -150 949 729 813}, {9 901 957 553 343, 134 703 384 062},
{16 589 309 678 495, 689 927 302 328}, {7 794 660 078 373, 260 727 719 464},
{6 820 047 892 297, -40 843 733 835}, {214 770 195 148, 3 559 553 989},
{300 435 907 808, -9 056 627 993}, {393 363 193 789, -796 769 693},
{60 499 672 803, -2 720 866 130}, {160 795 103 693, 4 445 654 209},
{188 639 594 419, 4 313 548 508}, {290 291 523 183, -9 431 617 684},
{524 244 880 271, 5 101 139 933}, {294 305 739 828, 11 745 053 273},
{170 531 408 753, -7 416 441 527}, {11 733 338 368, 226 688 621}, {13 671 950 924, -32 243 215},
{207 768 764, -3 309 393}, {181 471 745, -8 016 557}, {730 175 566, -12 554 129},
{511 057 084, -21 625 271}, {1 995 304 420, -104 853 299}, {776 026 489, 41 988 665},
{5 077 860 269, -21 176 003}, {1 099 493 201, -20 212 565}, {2 011 687 441, 40 019 043},
{2 694 558 041, 82 429 745}, {6 431 509 544, 116 451 733}, {6 692 721 479, -154 595 375},

```

```

{11 325 208 854, 451 268 855}, {10 915 357 229, -233 837 585}, {18 827 325 766, -39 021 443},
{4 766 550 240, 118 523 087}, {6 432 316 760, 22 253 237}, {283 948 017, 8 416 177},
{552 702 251, -5 145 470}, {536 377 211, 9 896 279}, {496 514 395, 17 219 214},
{713 545 561, -35 063 726}, {3 080 031 291, 95 509 499}, {5 955 558 073, -110 348 596},
{819 793 861, 40 069 648}, {4 618 626 151, -81 414 803}, {5 526 422 620, 2 764 193},
{201 004 063, -2 894 867}, {315 818 240, 3 167 583}, {235 955 060, -4 472 873},
{277 909 459, -1 126 012}, {54 091 755, 1 394 987}, {78 497 238, 3 564 941},
{17 202 536, 405 391}, {44 204 614, -392 979}, {47 932 466, 1 046 523},
{52 105 592, 2 210 119}, {235 253 264, -11 126 749}, {399 475 285, 22 611 416},
{1 890 080 953, 2 307 646}, {29 838 629, 40 658}, {1 090 093, -3451}, {106 173, -4756},
{386 791, 12 847}, {346 631, -19 372}, {518 315, 11 687}, {1 025 837, -29 638},
{2 884 743, 106 604}, {1 615 185, 71 659}, {8 275 972, 181 163}, {14 439 026, -429 055},
{37 359 844, -219 095}, {26 455 651, -26 477}, {1 287 128, 46 313}, {2 418 636, 112 085},
{11 855 734, 632 171}, {39 034 265, -827 196}, {39 169 303, 548 506}, {56 569 627, 420 413},
{46 718 128, 2 430 577}, {134 828 415, 2 541 212}, {36 188 929, -1 878 011},
{127 186 720, -1 144 601}, {34 138 259, 636 202}, {54 378 899, -2 616 177},
{140 765 318, 6 111 547}, {50 133 987, -980 548}, {31 635 789, -1 223 771},
{45 746 507, 610 247}, {5 526 518, 73 283}, {7 603 543, -54 404}, {3 267 267, 65 656},
{3 898 783, 187 253}, {8 416 030, -326 743}, {19 901 288, -764 179}, {8 191 134, 307 429},
{27 471 699, -988 175}, {49 497 451, 2 122 278}, {171 949 307, -3 707 853},
{348 405 319, -4 829 080}, {178 601 309, 5 378 369}, {279 898 132, -8 260 157},
{237 748 706, 13 126 357}, {370 044 280, 2 648 367}, {182 502 100, 10 008 683},
{588 797 306, -4 870 405}, {130 946 449, -2 999 296}, {256 666 325, 11 456 421},
{1 160 890 813, 58 898 304}, {4 285 892 017, 72 007 986}, {8 681 372 893, -19 515 840},
{797 152 657, 17 106 781}, {1 723 378 550, 86 737 869}, {2 856 086 330, 7 875 501},
{682 853 783, -4 364 326}, {506 750 677, 16 982 951}, {687 201 103, 24 757 097},
{1 505 400 863, 47 476 625}, {3 476 635 387, 133 856 315}, {910 829 553, -27 878 512},
{2 299 497 093, 89 853 890}, {9 212 715 797, -200 561 767}, {3 294 496 735, 96 646 937},
{2 133 720 127, 98 888 753}, {10 499 942 189, -558 262 383}, {26 867 815 088, 432 628 293},
{11 260 091 422, 609 462 289}, {72 732 325 220, 1 714 979 699}, {176 497 643 362, 2 224 586 491},
{189 582 953 823, 10 771 043 816}, {1 078 254 551 115, 37 210 646 054},
{214 400 297 201, -1 073 556 771}, {78 075 306 749, -1 156 839 609},
{142 330 289 446, 5 634 895 953}, {365 930 545 871, 19 157 559 906},
{486 163 821 907, -22 100 160 152}, {9 965 060 687, -23 982 362}, {2 912 078 155, -36 621 548},
{4 429 066 935, -19 039 022}, {1 763 322 941, 92 992 125}, {885 385 934, -17 629 767},
{978 293 584, -16 904 013}, {536 931 670, 24 464 023}, {320 485 836, 6 218 731},
{724 932 176, 30 483 495}, {1 674 597 704, 87 819 395}, {1 513 328 949, 11 974 999},
{1 124 247 825, 18 181 724}, {757 784 813, -10 865 720}, {706 712 337, 32 778 961},
{3 620 626 055, 138 867 689}, {2 526 601 391, 117 537 348}, {14 637 587 833, 751 552 429},
{89 881 012 182, 1 715 801 675}, {165 490 595 582, -9 103 609 269},
{408 032 813 740, -22 130 720 439}, {2 429 641 305 338, 59 499 755 851},
{2 472 019 822 803, -82 622 412 677}, {1 669 791 934 257, 95 339 637 706},
{11 626 707 657 201, 249 597 139 216}, {26 193 829 373 701, 905 070 600 943},
{13 357 731 465 146, -304 158 143 795}, {6 331 942 320 334, 259 478 801 201},
{26 217 223 969 010, -1 510 617 281 929}, {134 719 274 230 467, -5 600 735 117 147},
{75 709 486 153 689, 2 532 580 622 294}, {67 251 061 297 881, 1 465 784 785 724},
{43 934 750 201 173, -2 430 871 973 500}, {44 942 724 221 423, 2 576 243 359 506},
{287 793 364 565 071, 14 867 585 724 635}, {1 332 618 185 048 506, 36 535 902 167 209},
{4 348 752 464 274 482, 126 492 374 840 855}, {12 050 941 641 038 412, -274 230 945 115 199},
{3 820 205 951 616 344, -23 059 569 361 307}, {1 928 323 152 515 118, -4 700 110 217 915},
{320 768 755 661 968, 6 222 157 033 639}, {698 635 931 902 260, -28 102 457 363 129},

```

```

{985301046167215, -4336114239691}, {251781553096858, -12023612517307},
{179291751413839, -6460809893769}, {404342328534943, -13426212532376},
{390544093479413, 14217480340649}, {1674703194754390, 85738690356319},
{10057723705369490, 558496137530421}, {1203100685299912, 66836366004087},
{11570403812846, 179157963171}, {18790812110519, 623401344900},
{22281712643269, -563512095211}, {64951562457921, -1141376111260},
{26825846858649, 1340545683728}, {3748229206339, -12470461709},
{1350321785570, 9820408359}, {1228536560972, -51900487913},
{4285862383940, 152360165403}, {4964215916656, -185771894455},
{12957933640879, 217660475734}, {25525420693411, 1401112232477},
{76655527715075, -2585419885273}, {227674279621865, -8684520054852},
{471066307123963, -2775026740772}, {172747940626527, -2030677452383},
{35229650666972, -905284899633}, {19191565097465, 1056591248913},
{43403576874781, -577658899484}, {19869012783731, -368135340697},
{2584199090657, 142974294320}, {2676110017147, 20276568812},
{99663575287, 173690454}, {8721072559, -268903631}, {29155248117, -124118521},
{3163683818, 84104901}, {8107907420, 435383989}, {41261481121, 365662218},
{14645727763, -405879360}, {8551771553, -106230799}, {13283714666, 572809711},
{27381919563, 1411073996}, {143449923389, 6127766845},
{630332774454, 8696332109}, {1053412514106, -7982920973},
{83596636830, 4388021233}, {56282584153, 2425421380},
{124970995663, 2347807346}, {134838787575, -2701726304},
{62129433875, 3372996554}, {355289471653, -15414869873},
{187613608074, -10720207135}, {1342880209356, 53162655377},
{3467270057681, 123996040660}, {1159389280549, -45830589988},
{3419757243099, -45247642979}, {4784969449555, -252588205016},
{3565817882999, -46347256018}, {733128427137, 28702132967},
{3294884531255, 28758158038}, {3088214421865, -82184660838},
{8735475184729, 442789682518}, {30199934873381, 515325793550},
{51276023463319, 988297410972}, {28975918713475, -324317249122},
{28032568945867, -433061857297}, {29229396387938, 631275791083},
{47868209528120, -1936884857087}, {139031886662805, 4254746950987},
{345065442661266, 8497724879041}, {838660622233165, -1193976572521},
{122756149179173, -1845510738164}, {224160639731565, -2959489740266},
{190905712691401, -7100476443120}, {202594969482589, 3258181885964},
{147510830758071, -264380149868}, {3336509936523, 54590671144},
{1626228181489, -13777639319}, {117152203597, -6631510504},
{555961354225, -5589911646}, {642585419021, 7547977175},
{252847145646, -4329719285}, {432580206116, 12786959473},
{546280407466, 9392385991}, {382027016988, 18144162185},
{250902386853, 2955356476}, {76031315357, -3896928824},
{478722541873, -17461171382}, {1824999554309, 45232949549},
{3936074659599, -15669616226}, {3000986873, -66875711}, {2113450622, -62860661},
{5976774852, -104479373}, {5384098341, -97502785}, {5382736666, -218716289},
{21377810309, 558971897}, {34356433973, 1370549802}, {23264919673, -53281874},
{4834075515, -30698066}, {3634267403, -147096700}, {10830674347, -619312690},
{75892012867, 2383712884}, {97086654671, -3801223807},
{438036242061, -7478359804}, {799933580125, 28616213304},
{331418489137, 16109754620}, {1728475828633, -49460837480},
{666024274917, 25557300757}, {385148263985, 6997428647},
{72711788400, 553197997}, {60955549043, -2000762693},

```

```

{234 099 731 503, 11 708 771 460}, {19 000 121 947, 515 635 747}, {19 678 573 692, 171 771 379},
{18 858 858 143, 463 621 811}, {37 558 663 108, 795 998 003}, {36 835 998 717, -234 247 268},
{14 853 587 891, -446 910 242}, {26 493 026 155, 1 080 577 323}, {130 873 136 920, 949 504 167},
{39 767 969 626, 599 148 091}, {56 273 100 620, 847 692 301}, {81 677 597 254, -4 276 871 367},
{104 677 361 531, 2 888 833 144}, {170 521 455 097, -3 865 117 187},
{114 531 016 119, -4 159 708 264}, {487 144 633 523, -25 302 441 159},
{1 605 961 127 002, -42 236 749 937}, {242 121 978 396, 817 457 249},
{38 812 805 692, -1 098 241 629}, {93 961 517 927, -4 255 858 054},
{83 492 825 489, 2 550 167 287}, {166 336 440 482, -5 892 891 263},
{335 206 764 618, -7 411 106 977}, {428 444 613 903, 20 871 768 379},
{2 475 493 036 056, -90 577 349 897}, {7 506 051 798 087, -186 854 841 049},
{7 996 397 187 877, 217 647 808 534}, {14 199 503 698 131, -490 456 359 917},
{5 956 415 604 962, -81 722 208 075}, {2 335 701 712 763, 2 765 960 173},
{309 063 014 501, 15 794 963 622}, {1 715 900 742 689, 493 735 498},
{42 641 671 889, 759 434 223}, {28 452 205 651, -45 794 509}, {3 467 706 062, 124 465 883},
{4 352 004 162, -66 022 357}, {1 373 321 400, 69 869 207}, {6 039 747 740, -91 684 457},
{2 868 031 922, 148 528 285}, {11 544 621 257, -66 940 149}, {7 759 822 879, 232 534 180},
{21 634 929 689, 874 054 867}, {54 326 938 486, 300 844 173}, {31 590 063 577, 1 134 920 220},
{47 113 348 333, -1 809 480 056}, {16 783 586 127, -420 866 734}, {12 821 891 483, 457 173 487},
{5 279 495 597, 74 011 393}, {6 196 360 194, -36 907 633}, {1 034 659 650, 59 054 933},
{7 110 615 144, -34 975 015}, {2 682 461 849, -100 804 377}, {9 853 338 830, 256 360 087},
{28 025 536 524, -413 822 083}, {28 705 645 120, 1 055 099 953}, {54 704 543 639, -628 613 599},
{3 805 292 026, 54 222 837}, {2 433 052 436, 116 669 175}, {4 267 059 989, -196 553 996},
{14 339 108 673, -366 240 014}, {13 992 779 877, 225 410 417}, {4 350 839 773, -225 578 704},
{16 275 943 647, -205 629 314}, {7 838 188 091, 6 663 359}, {521 554 657, -14 757 375},
{1 266 679 532, -45 365 425}, {891 644 368, -48 350 917}, {5 353 293 362, 234 079 793},
{7 666 011 127, -296 875 465}, {13 240 491 713, -443 376 708}, {15 263 191 277, 188 547 879},
{2 305 917 422, 97 373 735}, {7 794 106 718, -126 920 791}, {13 036 555 217, -226 592 138},
{26 552 985 537, -1 414 994 999}, {83 311 780 444, -985 818 663},
{121 184 283 661, -4 584 201 129}, {500 758 631 057, 6 497 014 681},
{122 613 655 620, 1 601 117 231}, {168 765 162 917, 7 593 615 722},
{428 109 875 283, -23 055 318 101}, {2 495 233 327 636, 21 007 034 471},
{1 155 547 377 663, -65 896 791 118}, {7 679 310 477 711, -317 674 645 393},
{13 834 866 058 029, 186 197 010 907}, {14 128 099 978 661, -602 128 278 494},
{70 066 542 898 049, 2 677 216 985 755}, {115 184 218 373 169, 6 574 624 216 955},
{792 913 400 537 271, -1 223 526 740 743}, {17 086 206 487 557, 854 940 064 375},
{3 161 294 785 693, 176 572 469 911}, {4 269 427 848 955, 75 555 812 389},
{9 350 617 761 718, 481 795 758 157}, {49 321 087 540 485, 1 263 236 045 792},
{13 775 320 403 847, 349 641 714 505}, {34 962 678 076 152, -1 109 207 000 221},
{133 518 428 660 920, 735 181 115 231}, {71 418 112 091 622, -2 997 569 427 145},
{131 412 094 124 358, -6 763 605 580 705}, {728 800 610 831 713, -13 583 907 998 415},
{1 187 335 691 756 947, -19 994 377 353 160}, {1 924 524 408 047 257, 95 585 707 335 009},
{3 215 375 598 116 327, -155 330 098 152 886}, {11 685 672 236 664 029, -166 130 825 914 253},
{14 185 120 089 246 069, -725 880 871 396 228}, {83 456 832 008 301 241, -1 009 934 891 395 313},
{92 308 758 354 944 238, -2 470 070 606 554 085},
{229 952 624 023 216 343, -8 918 398 645 532 304},
{483 360 930 916 513 811, 4 658 777 705 277 544}, {289 139 558 520 042 015, -123 515 188 637 069},
{2 384 017 913 465 014, -122 893 637 852 059}, {12 308 737 363 249 143, 440 447 647 152 925},
{5 972 986 015 222 007, -135 406 803 391 695}, {3 786 753 162 844 177, 138 930 812 244 429},
{8 940 929 293 393 094, -250 901 119 818 005}, {22 969 266 033 826 586, -715 488 884 020 601},
{18 479 058 037 005 854, -245 138 661 496 507}, {23 508 264 616 725 079, 940 365 284 518 686},

```

```

{217 741 556 759 821, -5 043 863 996 648}, {214 706 630 893 207, -866 010 206 245},
{16 038 964 143 803, 554 994 676 166}, {14 026 247 717 761, 64 710 019 768},
{3 972 469 545 645, -178 244 488 343}, {12 823 791 326 849, -290 368 747 963},
{11 939 170 535 727, 227 026 386 436}, {23 400 214 290 631, -207 804 258 407},
{20 498 394 249 360, 55 380 688 477}, {1 892 417 730 370, -92 783 078 993},
{9 225 793 778 010, 161 871 198 137}, {216 993 465 549, 10 352 462 804},
{102 471 587 085, -5 651 233 219}, {188 096 674 893, -5 861 003 414},
{136 685 976 895, -2 418 312 349}, {290 614 576 498, 2 610 706 643},
{207 360 920 375, 8 420 432 518}, {790 623 036 325, -12 550 214 493},
{10 159 660 234, -443 229 881}, {8 691 384 279, -213 706 220}, {17 713 255 991, 429 922 506},
{21 694 744 495, 128 292 491}, {3 341 692 516, 155 782 229}, {17 636 692 457, 384 934 922},
{17 648 802 705, -780 744 757}, {77 390 003 206, -745 504 421}, {35 756 601 078, 1 215 775 381},
{125 277 872 279, 1 198 567 970}, {143 512 907 321, -2 379 454 408},
{187 156 353 091, 8 218 930 484}, {471 641 058 291, 7 759 389 698},
{422 110 035 037, 3 180 598 722}, {228 308 342 239, -6 982 638 792},
{531 803 212 147, -29 216 234 585}, {1 483 658 393 867, 37 729 171 564},
{3 067 396 420 621, -98 788 285 429}, {1 244 852 652 822, -57 512 900 543},
{5 128 220 940 124, 215 651 285 989}, {11 899 890 826 612, -507 849 178 067},
{55 059 292 498 821, -241 499 673 637}, {660 905 694 165, -13 121 812 903},
{1 208 577 302 765, 57 699 075 787}, {778 925 479 262, 6 787 207 241},
{402 441 716 703, 16 809 237 578}, {245 976 277 419, -13 022 286 730},
{363 239 783 201, -4 905 590 932}, {56 739 612 483, 1 144 354 384},
{120 004 785 967, 3 934 040 269}, {489 566 055 372, -25 866 158 123},
{474 628 190 215, 21 578 330 643}, {23 866 066 681, -560 617 357},
{60 360 397 170, 1 236 748 007}, {60 304 048 423, 3 109 251 008},
{308 298 097 021, -3 220 171 890}, {210 439 509 169, 5 910 115 407},
{583 486 016 233, -315 149 003}, {36 448 131 680, 909 235 927}, {19 752 344 600, 3 877 677},
{136 051 538, 1 287 397}, {103 548 544, -114 695}, {5 281 291, 109 562},
{5 601 065, 320 392}, {38 754 651, -178 930}, {18 362 909, 357 599},
{31 465 360, -1 128 651}, {34 353 868, 1 480 189}, {77 689 771, 3 506 970},
{134 644 181, -6 470 973}, {312 809 252, -2 144 637}, {77 245 250, 2 818 887},
{284 960 551, 16 142 328}, {1 405 939 603, 9 256 597}, {266 848 391, -11 074 172},
{268 134 013, 8 549 258}, {779 860 765, -16 618 682}, {305 539 539, 5 726 224},
{514 466 417, 10 713 992}, {48 895 051, 178 988}, {7 863 077, 410 321},
{16 811 478, 45 385}, {4 776 028, -196 417}, {15 567 020, -739 007}, {12 016 123, 543 721},
{13 619 511, -426 532}, {7 407 763, 74 907}, {2 015 530, 60 813}, {2 183 951, 124 323},
{13 519 613, 35 467}, {1 678 186, -16 907}, {1 102 643, -39 556}, {1 236 175, -69 194},
{2 338 567, 75 342}, {744 215, -5858}, {62 499, 2726}, {49 949, 2523},
{128 261, 3944}, {474 641, -2842}, {6777, -29}, {2259, -29}, {753, -29}, {1, 0}

```

29  
— is a relation number with a list {{252, 261}, {1, 0}}

252  
29  
— is a relation number with a list {{253, 261}, {2024, 87}, {1, 0}}

253  
29  
— is a relation number with a list  
254  
{{254, 261}, {1778, 87}, {4826, 29}, {1524, 29}, {1651, 87}, {1, 0}}

29  
— is a relation number with a list {{255, 261}, {510, 29}, {1020, -29}, {1, 0}}

255



```

29
256 is a relation number with a list {{256, 261}, {1280, 29}, {1, 0}}

29
257 is a relation number with a list {{257, 261}, {1028, -29},
    {3341, 87}, {8995, 29}, {1285, 58}, {2313, 29}, {1799, 58}, {1, 0}}

29
258 is a relation number with a list {{258, 261}, {1, 0}}

29
259 is a relation number with a list {{259, 261}, {518, 29}, {1036, 29},
    {2072, -87}, {592, -29}, {3108, 145}, {2331, -116}, {2849, -58}, {1, 0}}

29
260 is a relation number with a list {{260, 261}, {1, 0}}

29
262 is a relation number with a list {{262, 261}, {1, 0}}

29
263 is a relation number with a list
    {{263, 261}, {526, 29}, {1052, -29}, {2104, 29}, {3419, -87}, {6838, -261},
    {13676, 725}, {26037, -1189}, {31823, 406}, {40765, -1102}, {2367, 116},
    {12361, 522}, {43921, -1682}, {49707, 1595}, {68906, 1595}, {84423, 580},
    {67591, -3480}, {386873, -19401}, {301661, 13224}, {655133, -10440},
    {680381, -30131}, {3322216, -134763}, {12323917, 110983}, {1263452, -67831},
    {6663631, 205001}, {26668726, -983419}, {30616619, 1311032},
    {121738229, -4212366}, {110561255, -1543757}, {154972487, -4109213},
    {309710641, -12096277}, {1260443543, -15317336}, {1162983633, -53089459},
    {1310914295, -58772328}, {4713769777, 135956466}, {11757818179, 545154238},
    {61956239991, 89645119}, {3014706406, -25160661}, {1202676382, -13471457},
    {977494467, 13897322}, {1231346801, -10953155}, {1208074983, 49935593},
    {2530257513, 19977346}, {1805607827, -77508532}, {6025748433, 212776393},
    {17886479827, 736535011}, {55135205069, -836806571}, {24729526271, -793093160},
    {37776875793, -307950130}, {26560421811, -1013155774},
    {57431753681, -483253796}, {19842835309, 192140022}, {13784630309, 373543635},
    {9595340918, 155873637}, {18100863488, 919400253}, {75518233436, -316204487},
    {14370045691, 766232925}, {49543909492, 612356257}, {14977146475, 794602059},
    {31636965898, 328862523}, {17401050470, 147228099}, {7399449244, 373273993},
    {17366052008, -511779095}, {9056989386, -223822145}, {27379243118, -1504148249},
    {80103129268, 1878910493}, {181475767853, 6112440316},
    {499027147901, -11823394801}, {642920926117, 9713713821},
    {477559063853, -25564861028}, {2149576763577, 86842359016},
    {5649821709449, 210872864871}, {11505103863884, 359875817695},
    {2872565519628, 59943675091}, {1244222686620, 12314058967},
    {132218240639, 2015632907}, {213958711649, -11078534267},
    {911705431488, 1722932195}, {72140987579, -287283164}, {8656228145, -150838367},
    {15370042438, -690192779}, {48865741900, 1679380923}, {43051819979, 191409048},
    {4001760923, -37075398}, {626482043, 10582245}, {560081644, 4018095},
    {411973457, 11944172}, {1544233167, 76337338}, {4598925041, -207512226},
    {8851546147, 81740618}, {6196122989, 317879237}, {41137798818, 1952311639},
    {36623906937, 584009540}, {44366543829, -1938528403}, {57757282720, 339069189},
    {30381915170, -1277425263}, {72664570346, -559766787}, {27644446532, 902811093},
    {90129403313, 1078038837}, {112000915685, 523735534}, {20642499433, 1103872037},

```

```

{87071218010, -2288080831}, {32650511616, -524088377},
{41299479646, -1217192611}, {22373180664, -588955867}, {1878420166, -34988123},
{2876819188, 2618033}, {104957777, -5718510}, {532469011, 22578008},
{2473036603, 61213374}, {6443932109, -243478519}, {29848031745, -1501521632},
{47971435385, -1821757409}, {159310343513, -4825624534},
{17025013333, -96053278}, {6202362401, 42683157}, {3499119268, 36471415},
{561918436, 11908995}, {577461473, 12017194}, {167310343, 5799623},
{231104412, 3678911}, {175416003, -431143}, {15569074, 85637},
{4434180, -31291}, {2404346, 10875}, {255373, -12093}, {373460, -9599},
{236963, -9976}, {647243, -16965}, {676699, 15225}, {1788137, 60755},
{6901646, -2813}, {356891, 7888}, {507853, 2581}, {158852, 4321},
{269575, -6873}, {401864, 9193}, {691164, 21025}, {699843, 26593},
{2215775, -91466}, {5415433, -169998}, {6444289, -57507}, {921815, 20764},
{2156337, -7801}, {857643, 28855}, {2105841, 73834}, {9295735, 56753},
{3092091, 75893}, {5134286, -145029}, {15325273, 724130}, {31176809, 1370105},
{88264378, -232377}, {10225966, 225939}, {15440993, -169708}, {640405, 4524},
{526789, -28072}, {1730277, -57913}, {1870719, -33379}, {393185, -20967},
{1364444, -52403}, {517058, 15399}, {1711604, -86565}, {5180048, -80765},
{2916144, -18763}, {2072177, 92133}, {11901013, 609957}, {78407401, 3849286},
{373902103, -18356507}, {1781026269, 81911834}, {5531962777, -193222157},
{18799181088, -1005410309}, {79850687929, 278050057}, {13234572910, 160888491},
{10971478424, -28724587}, {345532030, 10669361}, {1081581714, -56242745},
{3410994017, -123270706}, {10674052513, -535434134}, {9107733921, 220699222},
{15534310397, -195002148}, {17321559509, -283944945}, {241398232, 12744601},
{197036181, -5960921}, {85682244, 621209}, {11729274, -416875},
{14931562, 673757}, {28642804, 331499}, {35213070, 1762417},
{9276010, -173681}, {18651171, -433057}, {7816360, -125831}, {3902394, 39701},
{3076048, -73341}, {1124062, -46893}, {360310, 16559}, {1048844, 39759},
{3973930, -59943}, {4652996, 140099}, {7818727, -226026}, {24244129, 632084},
{59158431, 3158767}, {225691346, -9513827}, {694452026, -24823913},
{162412494, -7950611}, {894272062, -20243827}, {931986262, 19733891},
{1181760255, -22313267}, {221681648, 1833061}, {31226779, -39063},
{4061246, 26245}, {1769727, -72500}, {7818201, -101674}, {2813311, 61944},
{6793553, -188906}, {1857569, -90683}, {11548067, 344230}, {40963039, -195750},
{13489007, 576085}, {62870676, -1004821}, {113891361, 542300},
{2198943, 53128}, {5442785, 169099}, {8315271, -454720}, {34271793, 1337248},
{130620265, -6024344}, {503724689, -26367351}, {721940260, -8927853},
{319764079, -14338180}, {1137243297, -8957810}, {104824699, -2053838},
{20766743, 249690}, {11170399, 387469}, {17411126, -151873}, {14272747, 597574},
{18154627, 983477}, {118886783, -3529329}, {292035989, -5635396},
{264210589, -3698689}, {421765210, 3879823}, {298635711, 418354},
{18158835, 99673}, {4825787, 140070}, {16676041, 62350}, {7519433, -184730},
{14332711, -408813}, {6379328, 106053}, {4246924, -205581}, {18482851, -959088},
{68427077, -3248841}, {52972408, -1649839}, {46698280, -1371497},
{17721466, 800719}, {27785424, -812551}, {41735470, -2008453},
{116257309, 2634012}, {94885403, 2210322}, {41670509, 2230883},
{188378484, -5112613}, {207295811, -3987848}, {19010955, 671524},
{54778429, 1444809}, {32694319, -1451682}, {182618521, -803851},
{37962472, 2071963}, {175457294, 3210213}, {290462723, -11552585},
{433449774, 20540033}, {554688303, 19653967}, {1151210701, -35529582},
{3751452251, 169859293}, {3826072715, -46958511}, {5899964212, 10673131},

```

```

{598911753, 32673604}, {2836949703, 147030029}, {11408716976, -328960021},
{27584428617, 1350873215}, {149111615371, -6443578701},
{239147280224, -6990658075}, {385270192262, -11805698247},
{1135594520807, -25542530564}, {3083195285633, 81756536448},
{6194465139833, -327732733315}, {8536136598976, -401015267691},
{30196602073295, 1082211684787}, {27700501494883, -559876400504},
{70104719859181, -374106859515}, {38591865157388, -516438425153},
{37087399749881, 870296078980}, {88192222966117, 4502957024524},
{490999308907469, 6815683093782}, {71043178808395, -1383142786099},
{132261836661998, 833567331813}, {72422072318747, -3614205888192},
{36282047940541, 1626189373618}, {133046892608535, 2241277946789},
{213422855719792, 1123132717107}, {7269180468506, -386058113721},
{17337931046759, 208569007982}, {7022990058539, -128619077661},
{13428572970608, -229677523429}, {28213748883938, -1295775600801},
{77141669758892, 544355937223}, {41257684941562, -2136490719823},
{174727012675275, -3169235511524}, {110212659402665, 5029202920643},
{113038675939503, -1460254676515}, {157554317984024, -1842968996421},
{237213714806857, 12275415760966}, {1046954436656289, -3987717850378},
{1815357993125, -15733237122}, {1587395436985, 63022607034},
{3111358678505, 107222150022}, {503994229021, 23656827285},
{1893825137468, -42999175365}, {489553830304, -26707967107},
{2317141085414, -125634627167}, {14653780455304, -725585028281},
{37367010986892, -1294289599447}, {44022885429673, 601748600431},
{25047488329230, 832132072223}, {21967380748020, 847450765249},
{17447196043402, 285344138769}, {10836541143659, -233429410464},
{25981312988845, -1229883202197}, {40440390332204, 2062795135025},
{214479752861848, 1431629141857}, {69594643592626, -495694174849},
{51931746920458, 1337660896635}, {62338376704741, -1240332368952},
{84622421628083, 377217963739}, {33032208393861, 865285785056},
{39804671735779, -663469623636}, {921994466203, 35733008184},
{1857765350803, 25256786662}, {2955294754655, -125154824806},
{12734733701207, 618884784415}, {68865700906604, -3302014452773},
{125346484228427, -2323152096884}, {27280727870267, 336359000409},
{9375644167294, -445782714605}, {3736483234907, 181328326970},
{18781259074769, -57791807289}, {283591363028, 1767482343},
{208871482924, 4218730369}, {543104343338, 28308487779},
{1378928866231, -5278052200}, {356954654153, -10527067135},
{253960278931, -3700586122}, {362982997081, 12660363134},
{1096061390715, 54361945418}, {2320312859365, -30519699586},
{214526688027, -7624451219}, {274060174385, -10739515567},
{1358981583891, -22651332586}, {25871643747, 723389630},
{44810711379, 2451624533}, {179226553455, -7389332066},
{495119558073, 22023227966}, {2790046761923, -53198139313},
{6244545141161, -219870404059}, {23189716634867, 986026680986},
{124904935413611, 2357946447829}, {17417522508738, 202036081615},
{11156325830024, 238385624289}, {12571008540017, -318361603512},
{40740278801887, 1624105956343}, {36196661941056, 74307571073},
{2334079896815, -17230832821}, {2082293552740, 60421236477},
{7356507793286, -332692069309}, {9805236612344, 78034450045},
{7128376544738, -86573994031}, {7708275993548, 180013345315},
{8494335864211, 425017722718}, {1582889209187, -74627909394},

```

```

{4 129918 433 119, -45 359 615 111}, {576 879 458 734, 29 154 339 943},
{1 632 530 453 138, 72 961 732 113}, {7 198 927 169 476, 137 782 275 927},
{9 007 439 994 536, 480 969 160 833}, {34 446 178 119 533, -1 152 712 643 592},
{35 557 912 503 701, 1 259 171 953 805}, {79 188 720 653 343, -647 548 620 707},
{49 388 487 824 407, -1 483 041 792 930}, {117 852 576 979 571, -185 459 326 800},
{22 592 873 393 173, 1 048 784 762 780}, {126 342 935 040 581, 2 796 612 421 320},
{130 283 909 350 603, 2 847 842 740 461}, {188 533 314 888 589, -584 234 871 711},
{45 906 301 278 832, 1 796 424 824 313}, {210 595 712 319 478, -8 028 119 876 839},
{490 388 622 197 632, -2 537 992 606 673}, {146 240 915 862 409, -6 349 664 070 572},
{52 242 908 923 539, 619 581 557 294}, {52 089 283 151 709, 2 126 763 563 806},
{275 349 854 155 995, 12 826 939 450 448}, {1 573 825 058 202 381, 76 231 816 648 387},
{7 112 333 041 815 198, 341 523 147 438 703}, {15 688 753 306 559 595, 136 218 255 149 131},
{6 220 992 639 706 390, 155 222 774 650 213}, {3 177 474 922 539 810, -169 461 263 866 891},
{11 122 030 914 884 297, 418 501 464 904 097}, {46 684 771 669 422 686, -1 963 125 016 247 413},
{113 150 153 495 504 438, 4 759 930 580 465 905},
{286 191 454 583 125 166, 10 427 562 723 114 105}, {1 222 229 658 528 659 053,
47 037 581 933 297 635}, {196 585 066 851 897 191, 6 500 445 841 450 458},
{413 354 893 004 847 613, -22 386 896 137 092 548}, {2 732 770 547 278 799 987,
138 888 587 510 074 296}, {11 835 316 368 666 400 379, 13 278 258 071 437 748},
{1 154 156 305 041 497 593, 56 043 519 755 836 411}, {5 985 251 385 570 630 994,
-220 090 623 564 205 849}, {11 257 596 475 650 217 673, 458 766 749 044 457 486},
{55 643 501 871 300 722 451, 2 056 250 268 814 977 842}, {32 807 833 296 932 348 571,
1 772 346 644 937 354 289}, {227 956 027 658 751 707 960, 11 453 711 620 913 810 913},
{294 087 851 754 946 208 900, 3 472 080 137 272 008 981}, {273 246 457 164 907 829 555,
-9 261 951 640 675 960 053}, {1 212 980 210 562 565 645 205, 28 381 228 594 130 091 669},
{1 949 518 793 062 441 995 806, 59 545 149 547 506 901 483}, {4 068 910 347 390 153 073 979,
42 834 804 370 724 339 966}, {104 165 838 937 375 594 033, 2 180 108 025 727 770 101},
{126 068 076 257 588 524 345, -3 425 662 970 689 637 528}, {179 222 312 035 080 882 233,
-8 109 818 384 662 960 930}, {212 058 891 566 380 086 299, -5 036 551 350 096 185 643},
{137 742 268 795 496 084 059, -3 229 947 390 746 937 870}, {301 258 348 741 650 264 313,
-14 207 467 226 727 580 844}, {763 104 225 837 590 512 907, -34 202 693 675 872 794 408},
{2 799 625 786 686 316 449 853, -42 892 898 339 365 711 333},
{3 047 484 787 044 391 073 704, 144 338 839 506 398 142 509},
{4 305 088 398 837 911 306 945, -15 330 401 087 076 474 933},
{724 382 643 842 053 246 964, 38 150 871 562 796 526 779},
{127 269 868 834 240 363 131, 315 951 144 110 147 318},
{15 370 309 685 188 584 049, -48 724 807 231 185 951},
{5 784 792 136 997 494 292, -57 288 030 096 404 393},
{341 611 420 448 892 463, -519 861 098 696 241}, {16 484 473 236 539 138, -397 502 076 987 333},
{49 151 565 055 381 555, -1 567 714 135 443 344},
{145 288 263 295 765 333, 4 221 032 283 370 342},
{466 342 568 888 684 415, -21 148 201 302 423 844}, {284 602 881 899 639 761,
-7 351 114 435 376 321}, {549 822 824 049 667 354, -6 716 145 770 139 001},
{236 996 953 755 181 464, -10 680 251 066 438 353}, {534 266 167 200 414 574,
18 844 938 131 188 777}, {1 737 877 575 634 879 134, -26 137 514 952 480 421},
{3 366 817 846 818 064 524, 179 508 980 413 062 025}, {11 533 281 410 919 969 113,
-156 827 803 323 043 152}, {18 929 697 201 113 947 505, -500 388 017 469 649 324},
{22 367 482 698 707 150 241, 884 098 374 316 669 853}, {69 701 138 627 876 229 908,
1 947 565 957 632 764 419}, {108 155 027 735 565 053 288, 601 254 230 984 560 275},
{18 603 000 355 474 403 756, -181 194 331 546 410 929}, {15 784 153 770 957 467 853,
661 742 646 669 202 354}, {25 687 144 014 191 213 109, -1 260 529 910 105 709 635},

```

```

{125 331 548 576 256 367 567, 156 518 847 804 570 659}, {10 532 759 498 844 066 796,
- 515 214 039 800 836 937}, {60 089 898 843 587 278 728, - 2 983 644 827 769 841 951},
{109 671 601 794 085 643 204, 1 350 723 535 510 416 467}, {69 167 794 866 122 166 151,
- 3 222 464 542 982 950 030}, {393 458 378 895 296 682 023, 20 194 714 014 009 144 290},
{2 566 567 721 459 333 354 919, - 65 895 972 962 335 274 393},
{887 683 930 868 237 105 304, 5 615 728 840 713 053 095},
{104 877 571 356 150 385 322, - 3 312 534 945 813 919 343},
{295 492 837 302 393 851 002, - 8 540 539 698 750 563 873},
{901 051 716 469 357 637 439, - 39 014 845 863 816 698 252},
{975 798 801 213 850 920 109, - 39 133 749 848 585 233 811},
{669 320 535 205 120 318 658, 33 502 912 034 038 148 147},
{194 016 540 094 015 446 166, 2 839 158 026 280 918 675},
{250 847 902 718 112 757 958, - 122 381 400 978 804 753},
{8 933 922 858 927 236 996, - 322 300 576 769 657 205},
{23 799 735 433 892 327 672, 787 277 992 122 962 483},
{47 707 061 263 508 186 866, 1 895 608 928 233 584 187},
{83 328 409 166 837 116 233, 2 376 749 816 432 930 075},
{37 389 550 613 040 228 904, - 1 580 726 423 695 774 339},
{144 093 375 138 147 426 016, 2 626 848 465 588 806 229},
{100 805 393 409 309 060 277, - 1 704 882 761 880 029 185},
{57 152 650 555 869 989 206, - 941 932 554 917 988 297},
{80 276 882 355 479 087 593, - 122 796 887 934 169 621},
{8 490 258 962 043 114 283, 465 181 007 391 892 897},
{30 771 218 024 118 082 031, 193 739 479 507 840 883},
{8 773 474 236 326 630 258, 319 634 384 624 276 313},
{37 699 958 936 917 659 241, 923 249 302 906 182 259},
{40 308 032 828 018 918 414, 1 639 092 501 796 403 793},
{176 020 565 542 379 396 093, - 4 080 868 595 883 647 341},
{142 865 786 797 613 393 090, - 2 046 647 694 990 082 723},
{105 082 136 995 100 547 760, 5 266 173 624 733 464 469},
{63 471 236 386 579 046 060, 744 775 218 813 226 693},
{43 485 153 100 606 391 765, - 716 691 735 851 417 036},
{61 290 252 804 802 474 353, - 740 815 971 075 833 504},
{51 935 344 951 318 803 977, 126 425 024 121 623 258},
{6 664 410 181 777 381 043, - 181 130 061 783 562 249},
{9 836 753 408 393 030 710, - 87 878 728 525 817 433},
{1 489 681 049 111 229 718, - 48 752 990 165 598 075},
{5 697 012 903 867 689 641, 258 281 720 612 141 665},
{3 896 358 255 350 701 893, 45 531 585 567 721 493},
{5 091 181 213 490 130 815, - 185 721 989 042 731 114},
{20 168 814 955 470 763 831, 81 747 838 379 007 224},
{6 022 995 649 877 390 711, - 247 438 288 027 878 696},
{22 217 381 885 783 427 841, 1 069 015 482 768 374 433},
{61 001 075 368 690 471 276, 1 355 809 397 183 661 057},
{2 721 393 703 034 664 007, - 85 643 866 336 149 363},
{5 052 235 186 916 405 167, 240 713 968 753 176 029},
{725 395 264 776 649 246, - 38 412 646 299 907 589},
{1 169 038 924 379 470 535, 47 902 224 227 930 317},
{5 098 397 785 104 589 801, 230 308 595 912 485 945},
{8 313 081 532 863 439 893, 72 156 717 757 096 481},
{3 960 514 579 701 624 014, 198 655 245 827 685 737},

```

```

{3 311 258 592 099 860 938, -34 202 727 061 108 109},
{1 684 760 333 665 542 005, 78 258 721 016 548 747},
{9 712 992 047 713 502 827, -232 771 314 462 054 082},
{16 675 030 999 198 146 271, 542 031 877 540 657 097},
{33 652 744 799 864 842 568, -1 545 544 365 622 259 439},
{91 847 817 125 939 518 670, 1 369 925 321 810 728 057},
{16 521 808 495 254 317 813, -425 322 416 061 003 451},
{17 296 387 285 826 812 088, -665 370 530 517 596 123},
{853 831 506 870 709 930, -30 023 351 845 006 861},
{3 465 723 320 366 187 186, 129 050 487 968 549 155},
{4 902 281 808 360 319 737, 114 736 355 808 850 408},
{8 253 332 243 525 173 241, -143 574 288 550 506 005},
{18 304 220 386 485 041 428, 588 347 787 845 277 441},
{17 210 447 343 018 919 091, -878 386 479 958 153 163},
{93 965 233 365 909 916 447, 3 069 564 809 030 302 047},
{313 305 512 789 744 563 630, -12 714 643 517 328 282 691},
{1 199 431 262 730 638 458 635, 37 534 266 047 023 205 108},
{437 960 953 589 379 567 923, -19 888 390 767 218 822 368},
{109 501 814 878 720 142 501, -2 455 557 207 870 323 145},
{262 542 242 041 876 943 312, 8 922 000 336 368 409 823},
{1 000 513 091 531 774 371 035, 29 708 625 564 319 190 444},
{2 519 586 723 285 541 368 043, -34 264 267 492 526 589 240},
{4 199 865 715 455 099 993 571, 212 544 140 588 637 090 053},
{13 417 496 331 539 795 369 607, 321 731 167 229 717 168 939},
{25 040 938 024 489 665 893 553, 980 913 223 969 212 091 112},
{121 717 925 060 690 149 019 417, -2 974 182 814 776 270 039 647},
{58 799 000 771 010 645 406 930, -2 298 260 799 302 404 412 829},
{251 370 142 854 041 632 902 112, -5 345 056 706 960 269 812 085},
{40 101 615 877 054 306 072 771, 398 761 423 801 931 448 619},
{45 574 724 785 422 572 527 724, 658 093 047 021 103 801 735},
{43 738 094 274 165 884 706 367, -543 469 402 381 957 305 091},
{68 522 567 989 245 978 659 881, 626 235 242 269 693 558 004},
{69 149 691 026 387 160 248 035, -3 047 290 502 975 568 534 858},
{246 691 512 559 390 922 122 837, 12 587 356 417 754 123 506 795},
{1 329 626 954 266 877 127 435 569, 61 620 997 856 928 042 425 936},
{6 847 204 627 996 968 960 911 049, -351 008 297 778 333 343 592 161},
{45 488 829 150 830 550 575 160 973, 2 029 369 324 319 359 858 145 081},
{221 631 156 156 618 662 039 897 233, -3 921 029 787 364 655 336 187 555},
{491 163 473 192 840 028 294 664 726, 2 215 344 612 056 993 758 162 463},
{169 117 069 842 710 122 576 741 780, -4 551 048 223 474 528 752 275 829},
{191 539 106 002 122 949 286 996 141, 6 930 371 300 378 539 563 641 844},
{660 469 377 429 229 684 178 554 133, -2 002 105 854 340 996 380 573 997},
{59 320 834 367 668 931 057 462 651, 3 267 392 037 720 374 884 446 571},
{133 545 532 128 674 165 142 610 099, 5 242 033 523 386 557 461 652 787},
{656 104 533 574 690 122 139 381 512, 4 078 398 401 028 653 103 659 357},
{136 131 164 612 756 245 590 815 795, -6 861 867 160 022 041 275 757 956},
{290 924 968 561 044 520 102 294 475, 8 237 036 686 039 058 390 782 628},
{691 344 036 565 176 299 749 356 185, 31 848 794 090 161 499 755 005 224},
{2 453 640 989 033 070 748 379 549 409, 10 927 797 408 174 244 255 736 045},
{1 344 831 513 013 297 009 358 968 308, -56 511 997 169 876 991 514 125 319},
{3 013 038 213 766 456 975 750 348 524, -87 971 622 517 128 240 736 390 243},

```

```

{5 786 801 672 417 455 957 540 108 906, -165 354 417 807 677 809 214 840 381},
{158 576 073 883 316 989 557 064 827, 1 587 637 463 099 421 129 687 436},
{49 357 848 202 407 457 271 517 299, 1 523 875 858 752 821 170 904 441},
{156 174 849 969 418 288 077 274 181, 4 700 929 066 433 039 630 218 254},
{274 622 174 384 658 813 658 883 137, -5 198 489 533 279 130 257 968 209},
{236 113 741 212 528 673 532 600 220, -12 671 093 978 222 092 799 252 813},
{1 219 542 670 280 756 578 792 448 701, -29 359 454 653 629 592 368 849 756},
{3 564 813 820 153 497 083 900 396 413, -140 030 025 673 471 612 552 323 752},
{16 848 615 897 293 880 534 275 587 219, 328 746 671 566 892 552 274 368 764},
{21 706 875 261 560 776 858 371 207 065, 293 158 754 908 516 760 936 398 712},
{3 452 505 760 931 112 407 435 725 151, -180 241 430 928 756 294 161 032 143},
{7 342 584 773 887 361 232 918 096 142, 365 182 555 932 056 877 180 342 965},
{10 239 551 329 756 830 288 855 289 446, 71 552 028 189 564 546 231 384 265},
{2 001 771 544 713 346 752 810 301 913, 56 332 243 823 537 462 362 068 480},
{6 887 768 261 642 497 654 954 965 521, 374 374 976 130 744 888 790 742 620},
{39 191 915 809 030 579 717 780 368 943, -934 848 367 436 895 281 340 797 727},
{18 861 208 932 902 811 914 214 660 433, 454 257 638 209 837 812 239 809 799},
{57 231 922 312 428 940 562 483 345 875, 434 382 573 429 941 502 330 492 738},
{28 029 851 025 037 826 972 265 927 283, 114 912 274 866 785 424 119 725 399},
{2 299 683 166 405 742 905 079 429 199, -46 237 768 039 780 363 148 958 014},
{3 209 976 958 401 391 372 908 004 763, 126 170 709 352 836 672 863 057 696},
{14 651 526 064 664 807 000 200 901 469, -744 021 209 712 956 797 937 305 019},
{60 200 208 083 308 516 097 387 313 593, 3 174 251 165 676 983 720 998 935 846},
{29 078 348 977 747 920 218 818 947 503, -1 175 009 834 570 222 615 515 320 758},
{78 083 881 151 510 679 463 850 790 561, -932 763 022 013 008 622 361 231 314},
{70 539 939 464 077 786 211 564 271 345, -3 584 708 566 716 320 168 165 912 738},
{303 562 981 875 386 310 911 297 638 145, 5 542 074 404 515 077 003 400 517 114},
{329 042 028 083 989 084 517 201 221 875, -6 277 535 773 673 092 046 604 375 982},
{686 474 145 335 922 398 662 475 423 293, 14 295 181 730 510 975 570 651 094 152},
{80 326 057 377 035 244 331 623 751 211, 4 160 546 044 442 224 124 410 214 864},
{335 504 506 082 475 309 539 202 893 085, -15 620 193 702 392 847 291 925 342 418},
{1 967 355 281 375 310 815 506 694 706 741, 13 610 577 326 940 703 456 291 915 223},
{1 624 927 361 176 981 827 431 479 156 222, 3 908 161 047 482 671 262 366 640 871},
{228 187 893 437 876 858 530 426 327 982, 3 771 155 149 455 118 806 230 880 473},
{487 226 088 546 857 214 859 891 169 073, -24 771 909 928 523 370 917 568 749 737},
{2 159 784 936 209 483 518 260 246 150 421, 84 930 162 714 857 217 488 745 683 570},
{9 607 618 372 907 960 313 941 868 087 973, 89 333 976 133 121 845 203 241 525 771},
{10 638 626 010 399 328 586 160 990 862 585, -33 227 030 875 643 843 686 838 006 673},
{1 571 722 240 837 533 476 053 955 260 175, -73 320 340 011 351 649 036 741 278 749},
{8 414 711 457 576 146 572 268 150 895 298, 201 766 841 896 163 689 311 583 214 627},
{15 647 422 242 497 563 629 224 503 306 468, 422 136 535 701 762 268 744 977 566 463},
{7 461 420 863 010 597 328 667 670 349 631, -48 291 409 624 692 680 275 954 844 586},
{6 245 626 378 810 014 009 701 937 595 337, 304 378 488 941 219 349 593 571 180 240},
{38 482 656 795 320 783 253 684 040 891 889, 571 818 222 990 685 858 335 291 123 233},
{44 929 829 850 490 485 992 737 872 078 114, 1 760 998 844 547 632 401 185 562 718 419},
{225 164 848 337 712 543 216 817 512 005 140, 8 590 503 253 096 675 874 000 994 085 583},
{476 493 868 143 329 239 604 208 100 135 266, 32 950 337 309 550 351 054 216 870 775},
{252 398 490 615 778 586 203 921 348 367, -10 493 895 439 472 103 026 464 234 654},
{143 335 018 001 853 868 589 065 484 473, 5 980 846 793 013 265 596 968 391 323},
{53 995 223 012 165 009 140 263 614 377, -1 147 393 326 232 920 527 940 789 925},
{17 814 746 634 266 758 013 226 318 226, 747 564 587 188 065 741 187 220 057},

```

```

{33 349 309 518 913 600 895 211 306 346, - 1 712 571 105 099 295 346 916 525 737},
{213 150 591 293 098 186 898 694 461 209, - 3 843 555 004 243 569 846 724 412 838},
{461 582 373 701 585 321 488 011 596 297, 7 083 348 511 011 421 045 497 392 626},
{306 321 487 776 696 778 569 122 884 641, 5 191 483 476 492 853 529 498 667 473},
{6 302 180 531 644 546 448 495 482 042, - 152 231 978 061 952 797 040 736 591},
{15 956 060 380 478 705 464 049 116 293, 429 500 316 395 754 851 749 244 504},
{16 976 301 218 809 074 673 019 316 635, 643 890 737 833 374 180 950 122 252},
{61 842 355 242 173 989 667 144 315 829, - 1 134 711 427 298 417 439 317 957 899},
{149 061 367 179 848 977 275 305 946 008, 2 573 464 056 741 709 971 384 509 885},
{52 481 153 237 762 880 093 849 985 686, 245 694 277 422 491 056 037 403 791},
{25 622 020 361 004 151 214 613 929 644, 362 966 181 572 186 331 164 670 163},
{39 076 153 553 343 592 394 422 457 327, - 667 003 217 237 050 922 766 322 167},
{72 860 537 337 954 368 831 914 788 338, - 1 327 290 070 514 494 440 828 505 667},
{36 929 550 110 163 083 790 745 140 261, - 1 121 563 069 694 543 712 743 236 997},
{21 574 202 906 053 845 932 582 008 320, - 13 071 035 998 995 843 452 251 229},
{1 598 389 939 820 692 663 294 709 617, - 87 283 939 473 225 281 224 966 993},
{7 174 384 706 593 689 127 514 884 409, - 14 012 437 940 026 314 865 871 296},
{4 334 581 956 785 957 649 365 391, - 217 262 950 220 160 212 334 218},
{2 808 063 523 335 855 094 888 847, - 142 204 558 625 858 772 369 351},
{9 475 271 734 687 252 707 019 499, - 213 066 826 697 590 874 953 299},
{26 387 147 678 225 856 986 552 209, - 753 996 065 183 330 912 754 644},
{713 940 639 160 664 443 267 053, - 3 512 542 433 012 702 568 509},
{235 260 143 139 571 149 107 938, 10 085 710 603 257 246 036 077},
{864 954 206 604 130 943 157 921, - 17 963 114 242 790 398 383 353},
{716 602 135 900 448 859 084 951, 16 718 887 479 893 342 318 141},
{607 536 768 295 758 336 514 456, 24 321 849 510 794 149 373 285},
{133 990 471 687 089 626 046 947, 761 764 877 049 111 295 678},
{21 078 575 144 692 003 996 203, - 458 358 820 335 061 765 100},
{1 559 745 359 580 183 178 411, - 14 609 015 778 161 991 313},
{899 283 443 668 421 617 040, - 25 089 590 985 924 227 161},
{1 036 701 769 935 697 478 828, - 31 598 700 100 571 448 249},
{1 592 552 679 771 162 421 307, 57 038 725 202 783 740 280},
{1 191 817 613 483 746 618 179, - 19 629 480 509 818 295 542},
{1 467 723 472 789 554 799 229, - 16 334 012 795 000 643 878},
{614 809 514 012 328 395 033, 24 906 269 645 914 671 757},
{2 063 820 736 646 598 908 596, 49 169 104 112 234 796 081},
{337 070 285 690 044 549 978, 2 796 809 295 669 156 849},
{353 377 079 597 861 761 513, 4 784 291 582 820 990 514},
{173 710 850 624 474 105 549, 5 923 587 844 480 399 840},
{506 749 224 384 680 179 707, - 6 660 542 150 173 115 548},
{144 129 515 510 653 689 517, - 3 535 686 335 889 580 914},
{219 243 180 595 430 652 691, 11 231 570 916 280 771 768},
{1 417 106 523 038 597 841 947, 15 015 838 349 972 275 635},
{1 477 459 871 136 634 183 591, 39 233 659 764 771 641 133},
{3 529 249 580 192 991 198 769, 188 781 022 895 902 901 550},
{15 146 131 820 070 113 769 103, 453 764 679 750 156 584 820},
{45 209 013 126 830 921 621 309, - 300 471 492 911 561 342 268},
{36 370 056 995 437 433 931 667, 1 183 727 620 357 130 026 736},
{85 606 298 971 635 983 950 187, 182 404 347 427 033 540 025},
{15 427 587 457 957 717 435 506, 340 400 347 219 834 115 431},
{28 817 392 096 142 929 412 193, 552 962 869 888 392 576 221},

```



```

{16 653 912 691 933 563 008 363, 356 558 061 180 354 572 132},
{27 435 156 271 835 794 924 183, 5 478 914 815 339 304 343},
{586 435 146 589 194 719 666, 18 347 662 883 262 779 293},
{181 487 272 581 339 257 730, -2 566 334 225 943 378 869},
{190 006 312 148 488 837 847, 4 505 377 948 592 895 315},
{205 255 274 895 442 704 271, 8 013 432 638 381 665 409},
{813 715 083 752 396 843 469, -43 852 324 339 820 228 446},
{5 122 997 699 201 311 712 315, 235 295 652 943 971 818 398},
{14 072 253 043 875 960 911 983, 184 975 332 374 630 992 886},
{3 715 607 035 253 434 046 161, -106 468 112 694 865 955 779},
{2 834 327 084 587 968 805 352, -126 619 025 792 453 561 563},
{12 810 340 011 499 488 604 058, 600 324 155 762 067 181 267},
{53 529 110 750 468 460 729 613, -1 480 882 843 005 246 730 912},
{57 157 369 799 529 123 613 403, 1 284 279 588 302 103 142 382},
{167 060 670 279 231 179 765 981, -6 185 037 861 252 838 089 652},
{17 002 430 681 397 003 834 151, 655 137 973 870 048 251 368},
{8 194 196 115 977 934 472 671, 275 337 535 301 945 038 979},
{17 339 575 030 149 591 231 837, 241 025 490 207 654 510 821},
{3 750 449 642 803 322 933 325, -116 909 000 208 787 086 748},
{2 462 110 300 121 809 393 307, -68 985 482 670 816 050 971},
{5 619 540 995 250 500 153 687, 173 471 003 239 561 978 564},
{18 007 318 486 727 928 825 057, -45 876 834 867 931 676 881},
{5 859 013 105 104 909 753 288, -209 359 049 174 293 216 273},
{799 591 476 903 979 519 628, -43 495 994 478 864 322 701},
{4 382 520 562 802 909 995 630, 158 402 546 016 193 992 597},
{13 873 440 846 087 232 633 618, -356 051 417 900 452 934 673},
{3 304 450 884 003 568 299 427, -1 338 074 989 222 422 938},
{156 311 255 839 702 004 879, 7 196 884 192 009 921 554},
{531 311 649 127 778 828 267, -18 038 297 667 511 449 950},
{2 156 867 410 496 003 065 571, 12 517 440 013 620 899 010},
{1 017 212 504 293 818 628 813, 39 327 346 734 001 888 939},
{1 393 508 337 830 617 187 063, -48 085 725 624 667 154 214},
{257 136 489 884 064 992 609, 905 686 585 953 518 720},
{20 645 638 531 127 178 073, 838 531 800 240 763 835},
{83 543 652 896 574 381 926, 555 043 061 453 901 587},
{70 444 387 719 731 277 993, 1 608 684 851 205 381 380},
{88 827 127 859 347 217 201, -1 915 186 435 053 402 371},
{191 609 135 732 256 239 505, 3 378 053 016 888 038 387},
{247 190 078 585 192 469 702, 11 043 179 014 830 670 397},
{1 115 156 888 095 360 614 584, -46 781 539 306 267 479 317},
{1 998 814 532 080 487 813 312, -38 944 896 667 288 714 605},
{3 320 322 938 824 765 904 191, 8 831 440 098 923 245 969},
{78 515 591 408 514 580 239, -2 428 531 465 576 740 731},
{211 079 726 145 484 610 761, -10 280 104 070 582 241 052},
{1 263 046 805 563 264 700 053, 57 512 276 018 038 713 295},
{584 719 177 233 379 010 931, 25 834 878 151 171 861 570},
{2 494 034 324 059 910 762 077, 80 616 722 832 809 161 865},
{1 337 114 028 136 566 259 094, 28 935 664 926 706 391 393},
{1 597 315 116 623 003 069 208, 36 498 315 157 678 931 407},
{2 264 627 332 810 787 040 100, -110 010 039 482 915 164 641},
{11 988 459 534 903 462 765 943, -149 630 274 808 555 975 735},

```

```

{4 743 875 707 592 977 978 609, -121 090 548 358 483 582 280},
{5 613 556 583 987 104 928 207, -278 562 553 958 261 269 609},
{11 126 347 768 154 317 975 101, 349 626 699 047 678 779 813},
{16 228 836 160 678 983 454 645, -687 758 421 234 513 275 534},
{72 947 244 573 675 146 598 973, 3 920 989 355 001 160 552 344},
{408 058 484 064 235 724 533 069, 3 665 764 923 079 673 074 049},
{304 705 909 429 099 501 484 690, -10 267 588 841 729 178 287 943},
{873 621 781 390 047 801 396 800, 3 110 137 280 786 001 005 809},
{85 946 956 345 260 564 944 127, -2 940 594 865 426 063 118 441},
{176 132 480 198 945 175 955 894, 3 481 637 962 437 430 682 097},
{376 367 697 850 676 462 566 939, -2 657 129 258 946 995 179 697},
{248 444 769 906 572 325 859 205, -13 446 322 423 767 392 066 079},
{1 686 084 131 313 687 660 152 929, -3 940 377 854 467 076 328 344},
{104 566 274 732 125 203 493 689, -1 391 563 631 990 793 016 358},
{52 337 613 530 536 271 178 657, -2 403 973 159 244 846 787 301},
{144 596 340 859 644 191 336 795, -5 518 387 625 020 739 619 237},
{294 103 066 194 604 805 234 479, 7 996 759 501 519 893 946 734},
{467 360 300 109 024 219 000 577, 9 747 296 079 848 866 882 289},
{134 106 783 338 725 924 864 585, -5 311 751 090 031 590 628 992},
{345 320 601 127 209 853 763 455, 11 864 995 677 190 421 564 409},
{324 996 066 524 846 268 041 222, 2 755 932 142 194 429 355 905},
{53 632 604 827 352 136 314 384, 2 594 794 964 709 452 908 041},
{225 677 520 496 696 560 427 451, -10 547 050 817 774 682 059 292},
{1 101 826 224 061 626 378 949 897, 20 491 001 651 892 819 012 977},
{1 232 908 531 974 077 958 476 443, 48 790 128 631 771 990 585 809},
{3 459 848 155 281 664 977 610 334, -139 337 923 105 265 593 513 181},
{6 206 779 578 043 388 237 647 233, -311 604 623 375 780 009 286 503},
{6 657 289 931 191 742 345 783 501, -264 249 057 914 264 930 671 807},
{13 429 696 117 136 317 773 929 738, 102 025 554 315 627 894 403 097},
{9 909 064 814 486 407 554 394 358, 483 142 296 748 972 049 308 339},
{62 310 858 734 647 441 524 240 143, -3 392 400 244 652 787 843 935 915},
{328 133 089 025 979 467 682 535 999, 12 348 125 556 830 538 755 267 280},
{1 385 037 165 221 055 700 645 987 543, -40 379 707 303 378 758 439 832 991},
{3 189 431 746 324 791 300 908 118 287, -69 271 312 413 828 557 926 788 003},
{776 211 700 922 218 340 553 849 187, 12 289 993 324 848 541 304 665 584},
{510 777 943 127 942 688 658 274 885, 21 941 476 410 492 354 183 594 657},
{1 610 608 235 580 676 660 562 214 562, 87 549 578 777 481 770 050 660 519},
{9 130 260 025 119 262 308 035 532 860, -129 911 111 387 495 843 443 205 243},
{9 594 825 962 567 509 223 936 618 550, -311 114 715 965 975 039 201 070 109},
{13 079 051 115 339 568 710 993 920 027, -380 903 821 314 751 303 323 693 670},
{33 748 473 137 800 416 670 932 169 961, 297 787 263 793 510 850 735 063 191},
{25 908 742 562 160 611 459 817 726 414, 1 182 896 666 013 662 591 088 616 259},
{30 240 815 706 810 938 106 671 627 692, -989 732 054 106 188 932 757 103 169},
{115 950 906 236 481 646 714 024 053 861, 4 590 307 350 994 780 211 947 216 187},
{313 817 507 403 993 192 235 379 735 918, -3 869 965 224 696 340 831 686 066 609},
{92 135 265 544 060 820 496 593 574 907, -1 860 663 685 341 519 189 247 810 067},
{236 152 624 152 981 548 004 592 180 509, -5 398 667 136 522 023 381 933 524 472},
{365 235 951 598 707 450 527 001 716 117, 10 288 655 107 999 136 958 377 233 251},
{1 349 985 001 328 003 786 739 019 263 316, 26 478 382 022 716 074 510 368 027 709},
{108 482 721 425 711 495 204 289 408 709, -1 946 136 525 055 291 823 762 237 313},
{131 743 006 052 214 741 642 116 655 397, 3 396 069 043 922 119 357 649 382 034},

```

```

{185 069 591 776 701 199 533 031 153 327, 4 738 020 562 819 987 661 207 778 462},
{75 425 724 427 802 036 179 009 640 267, -1 436 338 217 654 489 888 255 158 644},
{184 152 891 373 999 037 309 120 948 495, -8 053 859 202 015 431 469 979 370 243},
{285 583 881 629 598 149 606 401 145 722, 8 319 030 942 571 006 318 500 510 267},
{719 786 180 114 374 846 451 938 517 372, -34 400 482 837 180 377 470 008 674 707},
{690 101 339 666 640 149 998 080 337 925, -7 957 132 413 101 248 746 559 792 284},
{570 494 411 843 313 120 539 478 375 929, 16 820 303 223 382 578 686 362 991 361},
{367 121 108 695 667 911 575 055 880 735, -11 306 954 643 130 481 628 479 507 398},
{1 393 521 310 374 527 358 956 162 371 737, -54 222 447 506 949 463 784 994 602 225},
{4 276 991 424 019 737 956 322 386 247 719, 112 281 112 969 640 450 736 941 466 865},
{2 711 301 498 604 417 847 794 563 301 287, -67 582 887 818 339 558 915 159 377 984},
{2 100 314 284 029 734 182 493 491 846 801, 58 406 953 352 347 828 537 293 833 199},
{614 377 640 209 150 595 309 657 019 469, 17 100 566 799 587 136 225 836 542 292},
{326 847 083 484 399 219 780 586 300 309, 7 572 519 658 952 646 767 062 908 079},
{323 158 133 301 512 513 579 769 515 856, -3 898 084 378 557 786 397 609 904 311},
{100 694 841 240 128 201 947 218 534 691, 3 698 714 645 633 021 068 822 892 517},
{218 170 547 513 634 502 407 114 860 516, 10 488 814 478 990 157 859 914 122 851},
{550 868 371 376 767 727 234 492 190 365, -25 161 916 542 161 007 495 770 551 538},
{708 467 440 853 677 107 856 965 132 873, -22 614 587 070 643 891 226 105 601 521},
{1 950 208 557 557 434 199 942 860 744 886, 73 539 831 358 438 243 859 713 206 241},
{9 301 491 838 664 775 062 851 101 612 323, 146 180 258 070 251 597 332 525 573 788},
{14 213 750 269 639 044 771 230 733 958 667, 736 983 555 236 025 563 683 728 922 781},
{55 509 495 400 649 033 106 089 603 992 764, -2 039 529 276 356 085 581 792 040 476 981},
{116 299 898 966 131 990 596 286 423 054 851, 2 209 416 062 641 372 392 787 891 743 383},
{210 177 069 065 376 256 247 093 747 589 824, -1 690 967 925 639 928 736 132 003 784 929},
{130 723 173 224 599 450 248 748 182 019 164, 2 120 046 693 257 319 483 308 159 070 245},
{189 286 822 184 196 079 402 069 928 374 838, 5 969 855 681 787 067 798 017 867 633 923},
{459 871 183 476 393 705 373 982 844 513 574, 1 883 065 748 092 200 038 451 295 995 753},
{106 026 067 718 883 645 860 921 467 608 446, 4 220 624 517 829 292 019 145 799 175 483},
{134 249 605 338 803 835 538 716 402 220 573, -214 883 415 072 405 416 016 698 329 896},
{13 815 148 421 231 511 062 374 192 644 301, 150 633 768 676 041 256 773 756 932 477},
{11 350 632 101 606 839 493 410 072 762 329, 434 218 421 057 221 901 523 020 003 573},
{16 030 679 533 315 424 152 438 352 060 353, -697 250 776 397 691 334 222 520 937 736},
{1 601 229 167 678 328 620 742 560 492 225, -70 331 173 626 645 531 393 686 117 757},
{4 309 998 168 178 392 145 113 916 856 918, -37 532 241 932 763 327 581 615 536 275},
{1 633 139 025 509 708 541 001 761 267 941, -33 418 644 261 135 047 167 468 417 340},
{1 150 504 884 194 006 563 702 280 792 097, 35 642 325 575 068 226 457 639 140 701},
{2 616 972 503 249 532 386 208 840 181 895, 139 899 371 430 905 328 694 441 195 243},
{10 813 390 685 606 909 913 197 684 790 886, 169 348 303 636 202 781 364 698 073 169},
{6 548 896 489 947 908 759 606 867 577 590, 232 939 447 581 101 770 183 828 446 693},
{6 993 684 869 066 568 142 893 491 458 918, 340 899 675 687 151 051 240 459 684 133},
{43 449 788 255 627 834 420 070 581 771 125, 1 373 169 814 625 040 692 804 314 312 146},
{129 302 848 654 222 018 162 546 245 214 861, -4 700 447 275 621 583 698 614 406 372 823},
{607 444 541 616 951 579 846 826 037 960 129, 30 567 250 507 302 654 636 565 333 028 923},
{1 025 823 223 153 697 888 618 403 748 621 053, -8 122 182 000 583 140 271 080 615 463 220},
{638 640 554 098 442 403 570 750 667 152 579, -23 520 626 360 039 309 140 007 644 687 150},
{942 497 945 251 217 935 913 140 537 676 127, 49 613 003 952 700 511 725 002 890 460 010},
{39 221 150 574 139 944 683 482 219 848 569, -402 065 479 526 674 200 817 752 918 571},
{47 673 068 321 695 400 120 939 903 075 307, 608 697 820 521 656 753 680 638 178 553},
{51 189 878 424 623 586 802 582 913 969 499, 2 041 210 140 182 979 131 706 220 642 963},
{41 981 353 972 915 538 110 905 646 496 512, -139 964 177 077 515 757 030 491 107 067},

```

```

{2 077 476 539 206 706 537 563 319 003 644, -70 554 362 286 788 691 411 015 373 751},
{8 258 208 650 026 469 987 338 642 359 495, -343 778 205 321 423 587 650 607 674 813},
{1 980 842 968 135 921 419 427 297 127 529, 12 190 081 986 024 438 932 498 304 079},
{1 591 067 523 190 088 151 356 400 950 253, 48 055 261 544 100 385 984 539 539 195},
{1 379 143 657 745 933 846 914 789 243 134, 16 485 176 993 980 337 036 949 347 359},
{1 475 748 163 833 004 081 695 410 910 786, 57 975 683 591 696 819 234 818 766 809},
{6 931 647 472 673 487 016 959 677 767 543, -38 918 158 922 225 019 708 873 854 613},
{1 108 593 528 085 012 809 174 623 010 827, 32 713 687 922 847 204 966 866 937 825},
{965 699 519 741 338 000 798 306 183 649, 21 502 250 710 968 226 319 399 250 852},
{500 163 472 337 064 280 135 607 533 733, 25 471 910 432 888 815 507 729 737 941},
{2 439 255 652 347 263 894 993 640 197 881, 25 071 388 666 463 285 232 817 109 592},
{1 928 040 297 185 534 808 930 089 241 191, 3 249 640 687 464 574 298 769 678 853},
{263 886 183 508 111 686 793 126 198 206, 10 821 735 288 650 992 694 223 512 897},
{1 095 273 120 668 307 740 653 376 722 314, -52 401 079 104 340 965 125 490 627 977},
{1 354 329 157 510 214 596 246 660 348 389, 42 509 689 471 131 840 224 225 996 347},
{1 572 978 163 859 128 514 214 313 630 045, -79 487 600 403 710 015 542 668 608 221},
{4 411 521 028 563 882 516 072 394 540 625, -11 744 830 018 796 321 184 148 403 502},
{1 192 720 386 429 507 531 027 561 321 401, 64 006 273 086 088 276 771 777 644 317},
{6 153 884 980 222 638 368 324 261 123 586, 130 481 777 831 835 745 277 571 995 579},
{5 586 494 019 232 243 493 213 238 151 099, -179 361 963 433 143 604 083 351 312 475},
{6 909 839 187 660 234 623 518 383 130 362, 66 932 360 098 828 525 645 345 763 527},
{4 157 003 637 475 774 778 563 375 102 303, 184 891 282 043 979 028 083 961 044 339},
{23 510 998 749 666 110 268 369 049 360 235, -630 476 134 471 640 168 562 147 230 438},
{48 229 406 618 656 520 302 805 282 349 627, -955 008 346 375 159 950 772 672 813 123},
{125 193 009 223 355 580 076 071 184 466 898, 2 685 252 835 862 455 647 474 705 396 137},
{266 648 878 353 296 698 428 111 886 855 283, -565 148 554 660 428 038 828 989 711 495},
{26 625 974 409 863 341 482 040 583 203 891, -1 099 071 387 379 220 662 264 765 034 818},
{65 292 672 656 417 989 561 476 482 852 117, -1 072 884 076 762 152 459 615 256 976 694},
{40 306 334 857 280 654 939 252 686 995 071, 2 169 752 552 507 858 954 802 474 072 063},
{241 687 437 416 958 948 124 506 258 395 138, -10 996 064 325 049 797 098 509 573 109 835},
{59 432 144 077 922 655 231 244 055 584 016, 1 935 675 615 272 158 762 085 306 350 557},
{150 909 398 820 252 061 464 316 057 495 013, 6 763 509 150 747 733 238 561 143 446 158},
{555 507 943 499 907 646 800 347 141 718 231, 2 444 805 949 230 530 110 052 413 848 937},
{141 229 165 463 833 008 252 139 076 506 916, 4 499 258 425 205 666 807 688 408 936 883},
{460 816 576 286 279 687 228 979 058 911 809, 14 618 059 430 046 448 818 519 108 217 048},
{1 830 828 599 979 355 515 435 322 260 870 201, -8 859 293 263 338 134 309 070 838 500 047},
{800 862 754 820 869 360 635 764 172 195 864, 33 984 557 402 661 270 360 283 811 308 249},
{3 883 621 807 709 296 666 905 439 690 155 456, 54 934 714 487 772 853 973 162 840 016 721},
{4 403 388 202 637 478 844 739 073 121 346 305, 118 511 292 356 829 119 594 270 473 211 827},
{4 857 711 369 352 773 394 530 256 089 789 678, 101 281 588 510 070 432 000 774 215 067 009},
{1 000 683 211 349 730 816 316 339 391 236 302, -44 757 534 333 813 824 435 953 143 039 661},
{4 212 590 929 532 416 504 772 374 267 668 880, -158 575 925 568 693 750 762 249 455 704 843},
{18 136 232 996 268 783 407 598 952 563 174 703, -290 599 616 223 235 926 820 264 294 011 820},
{31 311 935 882 605 013 467 294 945 958 209 969, -469 466 773 547 556 007 972 187 951 200 066},
{37 434 879 556 365 874 579 353 101 087 141 139, -364 250 777 670 758 055 547 260 643 556 752},
{21 815 992 998 939 952 349 877 987 390 735 371, -424 676 190 348 596 128 174 881 821 581 944},
{41 424 417 575 487 600 808 220 810 884 787 701, -2 064 763 413 242 111 890 519 833 996 917 280},
{33 966 268 699 730 468 427 746 438 914 272 563, 40 073 581 075 978 643 754 288 599 790 065},
{4 241 677 859 947 848 159 147 245 125 772 491, 218 059 327 531 741 111 448 001 292 818 424},
{25 918 817 490 173 731 950 063 007 864 500 405, 190 233 770 883 028 162 396 413 922 233 212},
{12 367 482 971 540 190 271 637 897 926 079 699, -425 967 795 644 293 523 459 733 413 439 073},

```

```

{3 791 644 136 043 338 013 380 410 259 151 066, 18 599 879 880 928 957 438 205 551 159 105},
{718 347 592 202 526 955 556 332 631 571 102, 19 216 271 088 092 810 064 814 841 979 877},
{1 931 882 791 033 454 570 602 254 797 016 739, -58 631 816 224 307 231 049 397 466 986 837},
{780 358 968 963 906 209 327 604 363 355 966, 17 721 249 153 877 307 361 897 885 291 669},
{164 113 628 839 132 261 277 618 967 425 390, -8 125 810 835 924 357 277 681 697 860 513},
{420 119 387 729 665 435 408 057 686 579 190, -6 140 480 907 521 588 234 282 910 331 499},
{675 038 422 785 925 530 403 603 201 798 854, 22 599 200 931 786 128 594 616 798 586 367},
{772 590 159 094 140 115 378 898 773 337 028, 19 748 645 286 652 872 464 316 229 862 159},
{629 357 136 560 337 478 158 807 691 473 501, -10 865 879 035 138 705 365 465 496 650 908},
{227 191 886 637 054 889 044 263 055 419 869, 1 846 424 940 705 886 857 601 812 275 926},
{21 465 778 650 701 862 080 158 261 495 373, 385 219 183 509 193 866 611 744 195 943},
{28 008 349 588 817 540 376 145 744 565 405, 603 668 640 117 701 826 249 974 372 286},
{63 012 733 715 056 424 954 140 864 785 487, -1 043 107 299 016 417 583 754 674 734 865},
{112 115 788 580 770 291 290 280 122 413 381, -2 360 515 783 783 809 914 556 572 760 989},
{308 116 793 390 912 255 509 876 296 134 174, -9 268 251 325 042 397 733 110 854 459 351},
{595 563 411 766 953 273 428 360 030 580 433, -7 741 958 463 561 773 433 134 522 000 170},
{149 223 550 880 762 882 748 516 982 788 791, -4 199 102 665 851 786 187 016 417 789 862},
{511 310 158 644 073 455 811 477 160 961 383, -23 240 151 023 803 823 577 635 556 086 074},
{7 057 899 662 395 658 219 165 818 819 565, 196 077 337 349 113 707 407 263 647 868},
{232 618 811 350 470 091 361 868 468 629, -11 873 891 566 328 525 360 099 707 214},
{1 277 922 253 714 409 365 953 052 696 213, 22 778 737 192 336 863 706 041 931 944},
{608 311 358 152 334 583 067 285 432 787, 21 029 876 294 954 246 336 694 633 503},
{408 979 307 552 041 463 273 900 904 400, 16 021 584 001 679 219 145 146 088 311},
{1 994 033 517 295 595 673 473 014 013 418, -36 062 645 559 987 425 729 958 406 807},
{2 784 647 023 523 548 939 554 331 065 679, 34 146 552 885 552 267 467 112 500 426},
{4 042 392 343 126 829 092 959 113 913 539, -65 761 815 692 790 549 492 085 445 298},
{8 132 377 082 917 265 946 720 160 344 943, -257 563 714 704 243 274 430 607 664 463},
{28 841 050 143 670 453 620 591 933 400 599, 955 228 307 538 010 624 145 300 769 112},
{48 444 841 310 425 477 709 255 416 063 857, 159 194 288 922 930 584 757 326 249 699},
{13 091 476 675 754 525 016 426 108 859 943, 5 239 111 029 011 704 430 197 012 236},
{279 249 651 125 505 269 327 100 786 923, 7 744 197 540 204 535 131 442 538 337},
{120 595 935 351 347 208 529 553 986 033, 2 183 401 157 718 350 802 729 650 964},
{133 833 251 008 371 481 788 297 132 419, -1 299 362 023 754 902 009 721 784 171},
{272 846 294 840 831 031 265 582 022, -11 403 074 943 626 348 975 475 761},
{217 633 501 030 953 510 354 931 646, -692 587 306 142 748 106 252 107},
{42 365 855 260 349 112 835 522 624, 38 824 794 171 493 747 620 147},
{2 105 267 462 601 189 850 810 961, -3 228 495 175 160 534 208 511},
{75 904 008 285 166 824 650 507, -3 760 237 655 609 738 658 412},
{183 904 110 491 649 539 836 221, 4 699 097 367 923 889 139 051},
{168 139 356 508 498 077 680 016, -6 322 828 342 525 768 339 363},
{677 753 298 540 486 547 972 455, 18 772 278 157 165 219 235 639},
{513 187 924 107 666 393 725 613, 14 017 396 689 424 859 088 184},
{1 434 863 144 477 042 237 282 285, -47 587 810 816 125 117 883 327},
{1 901 179 658 234 928 305 790 925, 62 552 543 681 433 358 191 499},
{6 470 680 469 276 948 292 086 165, 40 886 011 001 290 653 712 252},
{2 811 662 272 205 576 459 741 787, -98 071 145 780 938 707 281 959},
{8 521 451 281 152 911 527 411 312, 422 763 229 578 021 741 531 425},
{17 407 099 362 821 371 253 879 556, -139 282 515 526 085 965 925 009},
{845 565 498 055 490 014 347 647, -10 941 691 690 416 412 369 526},
{803 527 565 971 106 878 160 135, -42 404 149 479 945 415 418 778},
{565 785 100 886 131 891 518 161, -14 972 788 294 928 554 255 963},

```

```

{836 564 686 463 283 764 817 879, -28 682 016 911 793 480 597 682},
{1 258 769 553 594 753 628 581 563, -48 187 478 488 437 555 522 200},
{1 550 414 691 484 199 656 147 469, -22 394 568 979 638 082 975 602},
{1 364 820 586 852 217 808 534 853, -20 524 174 991 362 052 800 365},
{2 689 184 842 070 771 135 930 669, -60 388 488 275 966 909 477 709},
{7 442 145 281 455 564 918 920 068, 290 453 594 974 672 590 641 431},
{28 837 473 413 997 601 130 127 294, -74 156 709 736 874 659 728 305},
{2 494 995 169 066 715 600 221 313, -29 846 377 636 821 604 975 494},
{3 182 445 288 116 694 260 408 129, 129 444 870 505 181 203 078 168},
{14 116 912 796 875 819 751 616 673, 201 589 796 326 594 546 835 114},
{1 479 915 205 734 987 440 736 259, -16 867 649 954 518 703 046 543},
{1 167 191 439 079 166 395 555 075, 60 333 539 057 209 524 749 159},
{5 484 653 808 944 766 859 437 202, 143 656 239 938 294 316 954 101},
{6 763 489 809 160 280 392 698 732, -253 395 313 521 578 294 308 793},
{20 562 301 507 573 724 606 972 577, 890 512 825 492 572 793 083 520},
{21 173 215 087 316 746 271 575 271, 735 961 495 350 583 031 276 460},
{44 622 757 074 592 510 121 264 147, -1 663 051 028 670 527 540 728 941},
{73 540 243 971 585 904 823 739 380, -503 594 895 025 883 989 717 677},
{4 047 385 323 199 531 464 095 494, 102 564 618 525 455 572 138 743},
{12 457 047 785 878 971 630 027 971, -497 321 737 728 391 924 530 451},
{6 313 142 121 992 634 909 641 048, 76 059 209 766 937 260 517 979},
{59 888 081 589 521 388 632 033, 1 180 629 141 197 999 778 246},
{85 213 212 844 645 815 388 919, -433 050 856 267 685 681 757},
{25 722 935 943 213 410 226 230, 437 600 696 015 190 338 491},
{25 117 847 002 581 592 866 357, 1 236 255 157 679 390 068 969},
{103 291 632 285 367 161 074 951, -5 162 470 534 099 052 408 810},
{11 104 281 690 547 692 371 513, 159 236 032 726 153 213 881},
{11 109 277 874 437 573 841 291, -229 844 727 908 151 495 901},
{20 180 235 864 577 436 005 309, -368 841 455 189 347 634 294},
{27 889 616 930 047 860 666 443, -1 403 687 821 644 213 619 686},
{48 428 689 245 976 284 273 851, 706 751 916 768 315 696 141},
{88 681 761 902 862 173 847 914, -82 405 028 405 211 392 305},
{3 669 202 118 790 236 394 042, 175 274 175 914 233 455 229},
{3 039 116 332 479 201 596 721, 148 304 520 038 596 674 307},
{19 205 820 039 011 513 082 803, 884 552 418 956 971 619 459},
{66 889 625 825 009 849 412 585, 3 383 903 037 164 906 116 043},
{207 358 383 509 815 774 876 325, 1 753 393 809 666 350 739 716},
{120 431 373 896 019 936 127 131, -3 640 106 781 933 159 139 247},
{80 964 574 255 355 031 910 740, -2 089 247 472 121 750 888 021},
{135 728 292 394 425 465 906 777, -4 278 704 714 939 687 241 244},
{313 037 981 198 510 288 827 153, -13 778 028 818 673 458 623 495},
{1 014 307 268 947 545 251 980 016, 44 621 025 762 366 789 699 889},
{3 149 773 103 352 309 623 884 353, 73 325 281 171 972 670 716 159},
{845 278 592 181 502 047 457 292, 9 015 267 990 034 715 285 635},
{567 185 505 903 192 810 200 674, 5 556 486 321 700 590 300 591},
{111 485 986 599 673 679 123 096, -1 526 758 059 945 764 837 359},
{8 586 482 815 438 496 918 807, -94 811 976 261 786 774 273},
{10 890 047 413 018 179 029 468, -281 328 093 066 698 248 125},
{21 499 780 961 342 846 268 041, 497 641 768 377 309 237 982},
{26 611 634 254 178 396 156 345, -1 166 536 976 474 160 844 309},
{57 522 361 843 280 758 106 406, 2 346 267 832 298 160 288 563},

```

```

{298 329 832 577 564 515 316 947, 7 949 574 365 044 102 433 550},
{987 300 236 351 292 192 541 639, -22 287 752 951 230 125 991 547},
{1 746 085 008 754 828 664 269 173, -85 656 373 638 538 580 970 091},
{8 667 831 963 807 002 800 113 839, 410 818 777 968 056 432 543 755},
{10 687 695 763 666 059 490 780 792, -375 848 837 218 826 383 209 747},
{43 113 148 564 736 160 118 771 388, 984 103 628 651 404 608 733 023},
{49 289 118 228 444 021 021 667 112, 2 056 991 193 175 178 253 635 559},
{20 690 317 240 947 608 249 197 952, -286 971 268 825 068 931 484 625},
{7 465 487 897 715 682 946 202 376, 260 098 926 784 217 409 155 561},
{20 351 197 484 001 564 778 238 859, -1 084 565 991 088 108 809 175 633},
{67 211 319 174 868 182 773 818 184, 3 617 761 623 074 755 913 010 343},
{401 377 887 514 223 227 798 501 579, -22 044 943 765 383 444 934 315 412},
{1 201 620 630 915 480 591 956 754 869, 32 095 854 526 029 401 806 678 632},
{3 701 465 537 979 286 703 836 762 555, -129 864 452 161 436 916 617 620 149},
{16 990 740 146 726 959 933 520 324 458, 431 284 923 813 524 715 690 337 335},
{44 875 195 033 867 453 680 055 287 359, -381 019 742 706 846 178 752 599 026},
{22 390 401 257 123 993 553 617 597 467, -1 016 853 655 629 600 749 478 332 163},
{5 160 279 150 740 368 119 798 238 703, -553 922 633 599 877 630 280 839},
{16 859 319 412 165 465 189 101 723, 678 684 916 926 439 357 974 355},
{28 352 323 391 821 433 947 630 976, -294 929 476 061 040 442 183 109},
{10 281 640 459 888 043 987 810 656, -473 695 599 874 082 134 604 003},
{36 731 299 920 883 662 024 558 830, -974 858 103 361 311 755 338 801},
{82 400 005 800 546 570 397 004 904, 1 981 579 624 923 032 861 830 967},
{217 327 011 356 072 977 372 571 730, 6 048 487 334 119 009 671 918 659},
{110 074 092 791 590 524 739 498 422, -746 547 142 301 811 831 130 111},
{87 227 335 657 960 803 166 863 615, -3 977 431 955 348 884 831 398 293},
{72 632 015 604 956 401 585 392 553, -3 095 195 299 248 497 033 907 910},
{379 383 738 949 375 058 849 293 849, -19 205 792 747 580 357 081 427 057},
{1 244 546 508 587 037 770 942 037 533, -26 436 977 781 390 909 717 027 252},
{528 249 402 617 898 745 582 009 207, -21 409 230 899 845 107 275 833 537},
{1 836 100 277 974 210 250 537 084 334, -38 244 614 462 633 073 285 104 785},
{94 360 130 937 378 740 090 374 002, 3 039 597 380 399 096 186 103 667},
{34 876 994 136 777 438 465 165 475, -502 347 635 803 896 293 815 979},
{56 546 911 039 160 272 459 949 012, -1 178 003 034 490 862 429 081 761},
{727 295 886 504 352 238 439 292, -17 169 639 830 399 777 634 075},
{1 622 976 584 048 694 963 541 346, -41 630 395 412 997 606 858 775},
{160 124 146 309 678 139 081 177, 1 903 686 971 933 567 053 405},
{56 397 895 488 987 234 526 291, -3 051 453 771 703 856 978 278},
{387 064 358 357 583 745 246 481, 8 389 564 714 998 328 138 023},
{300 972 325 994 751 186 022 249, 16 109 390 942 074 482 632 427},
{1 342 904 800 926 627 790 386 232, 57 461 884 056 821 606 511 323},
{5 597 025 983 989 211 084 586 189, 300 574 043 611 417 436 919 061},
{29 950 662 137 090 417 038 380 110, 210 094 391 090 485 035 962 077},
{24 415 812 467 272 036 403 784 963, 1 282 170 552 208 785 997 886 458},
{14 352 429 505 241 942 756 814 643, 119 763 771 292 921 212 792 257},
{5 055 662 125 962 530 681 379 811, 277 829 648 882 113 493 130 050},
{14 393 581 320 220 292 725 233 593, 61 450 579 289 116 771 295 876},
{3 720 336 607 112 647 645 634 167, 162 640 365 796 629 150 388 609},
{5 363 045 033 183 399 898 909 920, -196 324 838 403 432 373 786 247},
{16 378 166 224 460 887 157 169 013, 739 334 780 397 689 113 149 130},
{29 666 677 652 184 113 654 584 239, 1 442 440 921 827 908 001 591 407},

```

```

{164 264 988 731 114 001 633 686 004, 1 008 296 636 250 412 292 162 531},
{22 976 463 135 942 123 056 122 387, 838 251 772 391 623 077 196 052},
{90 383 968 999 862 892 591 022 529, 1 201 766 626 021 487 275 670 522},
{66 137 148 690 104 238 837 878 677, 2 478 978 474 221 549 581 823 673},
{209 156 039 949 808 766 167 809 922, - 6 212 006 251 656 444 474 904 871},
{539 721 395 512 220 992 465 346 996, 26 906 493 288 043 995 377 674 237},
{418 572 324 602 705 331 819 773 328, 14 790 228 055 177 030 395 494 459},
{1 169 281 972 187 850 436 179 189 188, 21 862 998 270 380 745 057 268 597},
{2 772 825 794 567 459 361 859 782 861, - 59 259 640 466 556 477 256 763 386},
{3 255 231 835 862 803 201 729 321 903, 150 783 163 917 602 216 032 708 111},
{16 305 413 595 329 179 910 437 469 757, - 101 394 643 333 121 284 818 561 311},
{5 029 607 082 780 246 627 287 045 582, 46 209 222 351 949 978 826 995 705},
{1 893 114 392 145 180 056 992 887 169, - 45 731 153 132 453 344 571 976 049},
{4 770 060 906 937 940 469 511 589 080, 70 161 573 798 254 381 997 028 833},
{243 567 283 303 024 153 315 721 332, - 1 577 615 229 304 721 837 913 507},
{161 623 491 395 508 442 861 849 802, - 5 015 965 912 449 328 584 735 923},
{292 609 117 845 171 103 528 969 958, 3 661 197 413 311 152 921 468 525},
{75 395 582 786 657 239 578 667 046, 1 480 519 441 048 735 808 287 213},
{29 168 989 895 839 387 366 954 871, - 197 960 735 359 683 850 850 166},
{18 084 352 865 021 519 790 863 347, - 217 277 733 337 438 620 320 032},
{13 229 162 477 712 062 031 081 733, - 253 615 113 783 078 980 086 895},
{10 829 435 540 884 182 506 119 759, 169 960 125 985 256 335 772 047},
{12 627 293 331 294 644 605 598 487, - 143 892 558 299 487 813 769 289},
{9 271 223 152 854 430 604 022 535, 18 562 441 081 629 477 155 022},
{2 252 608 970 907 555 464 304 491, - 85 808 805 897 919 634 832 274},
{5 675 544 618 712 624 128 991 521, - 38 177 616 795 527 114 244 914},
{3 398 034 644 900 879 990 674 895, - 75 869 014 553 513 564 608 313},
{4 226 675 631 901 599 591 886 970, - 86 998 651 442 262 131 903 611},
{9 535 929 946 311 401 175 561 847, - 252 142 905 463 287 256 150 529},
{11 966 621 320 194 328 795 621 065, 337 915 261 248 439 038 119 377},
{36 711 427 419 227 127 359 474 810, - 184 904 897 998 583 375 154 909},
{22 262 235 295 123 609 940 597 303, - 465 435 671 131 864 218 465 913},
{20 692 029 751 144 479 536 595 023, - 798 473 968 716 117 213 836 767},
{17 961 173 529 811 390 091 321 697, 64 633 123 516 724 042 404 715},
{1 797 554 461 366 042 360 726 199, 47 499 262 808 457 637 108 017},
{1 950 809 168 456 484 386 531 561, - 16 028 470 929 275 904 860 617},
{1 226 706 932 691 289 699 956 519, 22 295 715 656 333 167 464 284},
{116 396 328 949 923 717 696 437, - 1 628 103 956 008 252 067 755},
{210 649 343 287 846 892 973 816, - 10 096 446 147 827 791 415 261},
{361 894 789 749 159 134 372 895, - 18 252 824 652 150 926 556 452},
{831 527 966 285 021 346 866 135, 32 644 316 375 723 376 080 216},
{4 055 474 962 579 416 498 373 305, 89 003 859 357 991 290 831 823},
{10 178 775 354 592 097 411 215 439, 161 848 832 751 664 364 577 328},
{4 655 391 604 605 237 532 087 175, 40 325 778 269 712 191 196 311},
{4 714 828 243 732 248 206 500 830, 207 959 603 699 690 468 011 993},
{17 947 814 677 846 362 694 827 367, 719 649 011 815 043 826 153 149},
{11 416 992 410 319 768 217 357 154, - 431 503 853 018 154 622 370 887},
{52 045 656 975 957 733 392 806 196, 1 291 981 127 919 195 030 630 079},
{96 366 318 966 952 160 079 598 468, - 239 168 685 508 758 479 906 631},
{4 907 920 079 384 425 889 515 975, 124 774 376 068 846 404 296 653},
{10 972 205 539 946 440 071 931 604, 149 360 762 463 780 845 903 975},

```



```

{18 112 778 463 785 278 407 595 827, -662 649 924 479 863 673 283 395},
{58 183 622 244 016 277 212 314 606, -1 053 446 423 129 069 810 254 039},
{64 190 139 614 286 101 514 067 243, -1 014 402 044 323 379 821 488 866},
{74 379 246 163 164 435 950 664 155, 3 862 218 913 857 438 525 559 787},
{262 233 828 366 626 342 802 417 126, 3 720 472 473 305 807 718 598 951},
{473 598 626 862 808 057 629 016 228, -13 731 874 126 683 747 778 772 243},
{1 766 020 424 112 446 518 649 871 058, 88 430 616 796 083 200 251 641 357},
{681 672 805 824 198 918 717 449 566, -31 130 494 971 986 188 512 226 089},
{841 095 976 147 771 109 050 915 096, 25 810 933 795 440 315 225 213 023},
{2 804 852 683 762 694 159 233 156 369, 15 891 758 721 626 272 920 129 945},
{2 078 528 122 951 642 951 345 230 887, 54 088 892 910 304 376 464 857 957},
{6 088 500 590 700 157 814 005 301 023, 126 911 688 123 373 790 754 873 402},
{857 495 515 329 229 406 127 657 799, -657 663 043 042 974 125 496 025},
{25 535 406 086 728 475 538 764 663, 1 208 219 227 440 319 613 535 606},
{42 817 007 656 703 841 137 954 431, 1 436 767 550 737 277 633 455 787},
{75 222 961 604 010 308 684 144 077, 3 679 300 619 022 795 270 512 805},
{430 517 645 794 808 061 032 537 951, 18 225 513 141 441 257 289 841 055},
{1 813 298 104 742 695 961 919 258 047, 5 380 085 249 300 623 630 371 359},
{55 065 816 565 465 001 320 946 832, 210 623 863 223 657 655 964 969},
{24 455 913 455 762 869 005 649 749, -1 235 776 803 203 082 961 976 260},
{68 280 745 982 581 831 509 243 613, 1 259 906 693 819 397 357 068 983},
{64 641 327 795 940 421 837 373 653, 3 478 915 684 446 285 399 422 175},
{383 472 464 845 757 197 683 337 736, 15 293 968 038 509 419 503 182 711},
{295 418 401 234 709 757 291 499 743, 15 631 323 389 537 389 189 602 106},
{414 683 452 789 667 612 777 291 273, 4 261 613 118 330 024 688 753 432},
{343 735 821 965 322 325 638 801 047, -16 268 621 019 243 139 199 128 414},
{550 927 287 599 913 846 218 444 839, -26 242 788 791 648 621 448 936 292},
{45 045 857 497 994 707 024 148 059, -2 323 413 743 814 232 478 836 034},
{236 962 044 132 888 250 607 277 619, -10 093 238 818 441 761 116 180 471},
{1 267 015 994 195 396 917 938 344 718, -51 038 141 195 714 300 604 787},
{1 541 439 899 386 373 354 542 491, -4 492 855 999 311 394 389 106},
{102 646 696 734 615 797 811 979, -4 501 594 162 618 221 669 750},
{234 061 848 473 668 055 767 273, -3 299 388 706 210 690 945 264},
{51 219 162 497 533 354 121 873, -2 012 784 388 200 294 735 054},
{236 582 384 434 334 251 072 549, -7 621 674 431 605 782 915 862},
{81 655 465 347 959 919 057 501, 3 354 736 294 739 156 036 503},
{300 291 894 119 905 809 715 827, -11 729 271 197 998 346 458 618},
{1 227 988 298 377 465 128 767 383, -29 529 412 636 584 086 280 213},
{3 220 969 510 434 488 185 411 069, -47 371 121 662 809 119 301 175},
{70 158 573 407 896 819 102 553, 3 457 497 643 123 532 489 635},
{265 267 203 447 082 528 491 339, 2 572 009 803 362 835 216 158},
{92 100 943 286 861 822 718 095, -3 987 782 196 078 222 337 741},
{100 453 580 367 492 453 863 676, 3 493 183 239 190 682 567 377},
{223 216 928 656 820 575 237 591, -8 016 072 330 083 061 874 390},
{324 304 401 987 856 355 521 527, -1 601 234 987 478 773 793 349},
{196 277 023 698 032 550 948 160, 9 913 242 552 484 292 546 467},
{522 798 593 484 817 895 050 340, -13 068 097 395 812 464 280 921},
{19 645 482 559 982 162 950 500, 900 437 593 561 762 828 277},
{43 170 003 073 050 868 429 222, 1 194 435 539 354 319 974 449},
{44 795 121 605 676 878 802 254, -1 984 159 233 982 238 571 561},
{221 062 224 065 541 994 379 687, 9 944 546 005 332 263 038 302},

```

```

{600 221 742 385 070 582 242 309, -31 950 260 546 975 563 896 454},
{1 797 133 705 963 329 660 853 371, 80 071 170 762 042 784 161 296},
{9 354 370 639 176 151 647 177 917, 429 307 375 351 974 837 602 628},
{23 772 995 683 198 527 161 013 437, -189 491 364 152 791 529 857 111},
{22 769 268 158 191 099 294 009 806, 377 366 405 575 666 394 825 767},
{33 475 645 620 243 403 973 975 718, -415 869 252 423 256 455 967 717},
{54 205 727 138 699 411 594 848 154, -1 786 580 815 449 174 716 046 695},
{159 983 603 583 956 739 836 640 952, 6 430 240 237 392 248 508 958 247},
{203 141 818 273 411 369 363 903 649, -11 178 069 336 557 827 945 408 936},
{509 317 966 642 432 649 140 756 663, -19 484 350 736 045 499 056 006 260},
{716 634 893 880 664 179 048 196 489, 11 953 303 815 668 643 729 860 775},
{148 157 120 636 518 967 527 352 893, -7 069 292 478 504 969 423 722 577},
{78 379 631 378 457 667 525 981 912, 1 060 417 494 397 996 368 706 111},
{24 002 223 439 438 768 425 089 426, -993 335 729 748 901 036 637 603},
{42 649 638 397 332 752 541 968 902, 2 110 166 031 432 145 722 323 707},
{117 381 573 165 427 419 115 122 406, -1 584 591 289 573 780 110 833 273},
{32 038 064 822 502 710 240 033 652, 112 786 745 534 136 711 667 289},
{1 743 450 882 473 525 275 700 488, 57 394 527 467 446 114 206 591},
{5 684 760 372 387 306 419 225 354, 50 680 042 639 600 782 413 865},
{2 260 641 945 780 941 473 460 662, 117 419 006 362 127 277 853 957},
{7 806 056 948 837 600 083 930 977, -105 582 522 906 740 706 249 385},
{1 854 083 266 698 802 951 683 919, -35 995 729 748 026 353 147 017},
{4 653 700 892 223 229 345 733 795, 230 253 860 078 741 834 041 741},
{12 788 030 640 527 270 868 430 425, -76 977 037 836 550 776 043 942},
{2 588 540 590 538 457 870 781 939, 20 457 588 601 916 835 576 381},
{2 517 741 581 009 805 071 051 824, -105 533 592 660 011 429 023 355},
{3 962 001 064 413 406 308 787 048, -204 642 223 767 876 710 997 411},
{19 409 087 772 645 934 356 930 857, -316 765 553 733 695 111 045 818},
{22 720 305 656 210 069 364 757 217, -635 072 521 722 132 143 937 371},
{37 426 248 081 898 895 867 880 557, 1 950 127 300 362 886 149 287 333},
{98 317 125 626 067 525 263 783 490, 3 354 041 864 906 597 435 432 089},
{276 126 736 013 140 504 334 515 067, -862 597 845 348 768 570 057 062},
{25 096 906 903 589 783 975 124 701, 58 609 322 462 102 929 922 500},
{3 186 742 019 958 981 661 506 363, -46 899 589 682 368 974 420 976},
{639 110 630 274 561 568 561 315, 1 943 992 761 899 738 691 313},
{121 765 946 688 997 211 614 106, -1 056 890 101 019 385 325 795},
{58 802 873 874 957 475 840 103, 848 487 926 471 896 474 122},
{67 645 427 428 310 830 055 155, -617 720 442 949 866 651 864},
{79 905 000 893 893 933 919 755, 3 865 759 892 725 068 200 262},
{335 576 652 426 447 049 151 461, -17 620 635 627 346 778 929 005},
{206 343 358 303 719 618 596 258, 7 321 528 581 201 185 836 941},
{352 566 761 912 727 187 582 330, -18 247 126 769 390 109 654 017},
{1 544 165 916 404 872 393 029 841, -31 455 465 365 734 264 328 787},
{749 053 846 263 974 961 770 114, -13 258 287 897 132 852 564 781},
{1 733 097 418 452 762 371 445 414, -47 093 776 138 556 354 216 087},
{2 464 914 551 215 379 186 598 715, -116 983 306 439 206 730 608 989},
{2 173 725 505 905 952 922 015 798, -86 499 031 066 893 927 644 555},
{2 958 678 788 438 044 227 205 749, 87 705 173 624 500 760 385 725},
{6 127 141 191 080 167 614 040 963, -95 505 475 391 816 835 269 289},
{3 889 971 459 023 111 240 100 821, 189 060 604 608 230 620 042 030},
{21 119 225 528 179 458 345 615 767, -819 485 222 377 998 574 932 209},

```

```

{49 283 636 709 556 710 489 498 421, - 1 848 080 746 851 713 833 962 753},
{161 624 928 780 605 076 231 424 330, 4 857 710 812 822 887 802 906 509},
{347 284 124 809 291 807 439 007 179, 13 886 280 492 981 242 281 788 786},
{33 430 583 492 077 353 697 620 127, - 993 929 885 138 861 318 845 213},
{95 477 574 495 353 890 639 801 245, - 1 795 077 125 329 551 903 617 356},
{89 022 042 309 449 253 745 402 151, - 931 584 742 077 621 322 087 844},
{107 854 440 590 629 405 033 119 599, - 4 739 807 205 043 035 884 698 685},
{305 375 907 969 790 542 831 891 028, 682 035 414 587 439 734 236 767},
{46 276 892 295 586 481 925 494 644, - 778 182 173 301 672 330 972 901},
{95 769 890 617 195 186 698 586 555, - 4 018 528 574 254 089 696 362 728},
{177 471 128 369 480 061 713 275 171, 143 786 790 780 812 033 173 442},
{10 054 107 586 957 360 416 156 409, 122 579 660 752 966 358 340 648},
{677 331 571 313 305 474 720 799, - 26 225 744 453 083 449 573 720},
{1 193 437 314 785 288 333 527 223, 54 391 815 129 712 230 439 492},
{837 028 551 984 133 605 241 063, 820 838 257 092 350 910 099},
{59 561 675 766 916 964 758 171, 851 567 696 268 878 984 532},
{12 640 561 610 900 373 835 147, 443 711 703 694 885 761 245},
{56 974 717 657 659 572 835 481, - 2 669 104 929 653 503 470 702},
{242 884 217 488 167 987 044 357, - 5 644 938 757 127 449 937 420},
{39 936 795 033 849 250 383 111, - 579 737 741 216 200 483 879},
{17 123 695 948 037 330 194 020, - 470 273 611 240 750 404 283},
{50 981 483 106 393 013 275 816, - 8 247 886 055 978 113 613},
{341 740 725 173 067 905 969, 16 387 335 114 639 077 347},
{629 441 117 634 764 917 634, - 6 693 737 783 889 806 497},
{60 428 444 619 377 118 908, - 1 364 930 676 512 559 815},
{97 703 146 292 840 093 624, - 3 456 193 769 769 126 409},
{244 516 554 437 097 747 236, 7 725 687 505 010 168 025},
{711 532 225 208 866 575 332, 8 050 261 495 958 500 681},
{817 723 167 468 369 551 252, 43 373 325 903 235 904 635},
{1 675 316 494 288 623 481 819, 46 119 685 665 478 070 769},
{3 947 054 117 161 601 677 505, - 56 864 659 086 569 905 373},
{6 152 264 369 517 168 379 984, - 30 900 899 646 389 195 115},
{785 144 389 943 979 202 037, 11 099 921 468 414 706 629},
{775 859 024 441 286 747 586, - 10 545 513 116 608 782 135},
{1 185 852 847 381 703 296 252, 27 521 721 320 363 285 469},
{636 152 449 399 571 545 355, 13 165 686 888 547 097 452},
{1 104 462 911 068 758 194 317, 52 598 907 247 462 090 768},
{30 019 116 649 722 206 293, - 635 169 213 769 785 083},
{43 701 027 468 626 844 096, 1 606 553 358 988 526 051},
{85 234 822 071 336 509 097, - 409 709 183 333 786 882},
{4 027 039 670 024 299 583, 149 711 226 792 906 161},
{3 987 988 240 035 858 932, 202 560 686 140 933 697},
{16 628 301 971 880 347 104, - 100 829 434 718 140 583},
{2 249 900 989 179 310 933, - 27 268 438 799 756 044},
{3 518 790 405 715 909 097, 187 536 317 705 784 254},
{11 677 102 872 519 824 727, - 393 658 531 842 373 444},
{34 887 760 763 612 569 959, - 335 169 919 785 222 547},
{7 913 434 864 698 793 673, - 18 697 577 647 496 902},
{1 146 553 709 399 885 401, 13 153 981 108 582 411},
{567 383 826 695 714 372, 18 519 071 178 221 913},
{1 764 040 895 070 376 853, - 7 665 343 727 788 144},

```

```

{266 113 309 604 281 779, 8 701 795 478 287 861},
{957 938 108 554 822 856, 35 247 231 255 832 413},
{1 647 133 402 252 446 415, 7 245 006 856 668 924},
{661 930 442 401 975 421, 7 735 078 699 024 094},
{864 303 662 807 422 369, -32 953 337 958 468 955},
{1 976 938 358 341 368 757, 52 848 146 108 930 075},
{5 669 478 457 781 423 266, 145 726 852 258 693 209},
{3 647 489 220 901 925 755, -117 672 396 565 570 792},
{93 384 101 892 193 611, 5 035 888 398 303 731}, {604 315 528 676 824 114, 8 272 403 080 939 987},
{113 117 291 037 931 569, 5 338 395 924 468 683},
{265 886 852 135 466 438, -3 281 332 596 938 963},
{26 013 799 036 944 405, 410 484 394 739 846}, {40 313 210 271 870 141, 1 273 006 656 041 026},
{111 249 715 739 427 733, -3 589 619 649 162 785},
{7 493 760 154 692 326, -400 252 222 988 039}, {29 201 437 587 149 145, -991 367 905 102 898},
{118 815 073 200 422 089, 1 295 877 673 697 566}, {106 691 941 075 297 529, 354 979 590 639 845},
{41 268 831 018 799 608, 2 202 033 404 872 709}, {149 858 366 204 629 969, -784 056 592 931 522},
{27 235 479 088 537 221, 1 010 582 432 252 981}, {13 214 851 143 128 958, -581 718 338 676 055},
{43 308 380 008 540 741, 177 563 193 757 569}, {4 481 327 564 502 985, 244 064 225 051 078},
{23 189 108 072 481 803, 264 543 840 337 289}, {23 867 217 703 502 427, -1 149 622 600 186 741},
{72 287 364 810 232 242, -541 560 412 772 785}, {68 335 266 711 833 131, 735 892 650 719 732},
{27 023 198 741 811 535, 143 615 477 876 809}, {6 177 580 955 489 509, 306 073 632 149 182},
{14 756 486 189 043 547, 767 453 184 395 017}, {45 992 305 296 552 912, -1 015 607 728 450 369},
{76 258 826 783 298 741, 1 975 742 531 245 849}, {209 119 698 981 104 310, 10 732 715 120 351 503},
{1 367 103 375 633 973 039, -41 455 466 976 144 614},
{243 810 094 224 195 649, -12 117 316 056 018 120},
{384 972 326 308 144 487, -3 147 621 895 448 985},
{253 125 681 665 867 371, 9 511 346 627 352 735},
{968 018 122 708 652 662, -46 472 422 131 901 147},
{2 078 421 162 114 384 775, 75 732 472 515 821 436},
{8 848 478 301 235 178 789, 403 885 843 081 555 928},
{9 733 694 845 030 577 901, 34 441 140 588 012 053},
{3 457 908 582 107 104 774, 92 947 223 628 666 269},
{4 960 523 963 617 091 923, -168 886 925 281 702 658},
{16 517 223 307 749 003 183, -706 282 557 478 269 718},
{71 726 539 751 934 312 947, -3 845 080 622 335 556 611},
{349 787 915 052 052 080 106, 8 442 181 053 539 341 545},
{962 183 358 374 977 188 143, -7 727 923 795 050 921 114},
{1 001 271 509 680 031 141 141, 45 129 402 763 881 775 128},
{2 215 682 654 028 239 229 475, -102 393 123 951 290 651 161},
{9 722 077 172 740 790 265 621, 128 988 746 576 996 606 768},
{12 603 270 199 569 771 359 523, 570 899 441 382 955 997 368},
{11 435 894 645 066 466 783 301, 88 483 045 221 697 767 207},
{5 676 016 415 940 615 976 274, 113 757 188 727 497 784 787},
{3 114 714 374 213 868 188 988, -38 200 079 660 474 658 233},
{4 653 037 539 549 145 749 034, -214 830 657 426 360 833 161},
{19 261 310 967 498 448 673 604, -844 048 456 377 691 416 421},
{39 924 328 176 563 376 772 777, 1 869 626 704 074 681 604 173},
{174 150 023 831 701 591 392 872, -7 562 389 638 636 304 301 077},
{56 561 343 626 513 819 110 563, 631 410 547 698 891 219 100},
{69 854 290 259 620 730 018 931, 3 395 441 109 708 817 559 506},
{381 342 910 641 547 386 172 785, -9 967 427 896 375 831 156 823},

```

```

{678 711 102 346 905 982 153 393, -2 073 198 792 054 347 530 784},
{203 850 601 770 331 311 387 575, -5 783 530 096 793 048 026 792},
{375 313 724 617 127 808 311 865, 10 154 499 046 006 841 648 119},
{105 920 642 387 962 491 825 494, 3 963 656 217 534 898 305 561},
{288 793 852 681 177 517 683 739, 8 416 654 392 454 386 030 378},
{691 059 677 822 567 267 183 281, 3 765 698 185 925 306 593 447},
{480 971 345 962 245 400 884 321, 17 283 778 718 363 817 966 256},
{782 282 493 960 615 070 932 761, 26 108 376 604 404 711 466 511},
{254 795 497 111 409 815 455 647, -11 244 729 238 530 924 954 149},
{1 008 151 423 572 783 582 812 140, -44 090 828 735 908 734 556 553},
{1 561 598 623 869 853 052 996 277, 59 058 580 437 059 994 564 442},
{6 857 865 049 155 110 106 366 455, -347 592 641 385 776 770 909 819},
{24 718 785 761 391 857 011 270 275, -1 255 084 976 120 066 715 023 653},
{100 706 319 145 492 527 060 332 455, -3 047 623 358 667 695 555 202 211},
{35 438 805 387 604 893 267 446 396, -446 243 598 383 054 687 501 553},
{48 802 573 335 359 687 118 635 467, 1 025 925 214 456 162 364 617 903},
{116 203 120 094 995 978 735 279 651, -739 623 653 481 914 632 967 396},
{21 620 309 062 205 297 521 799 977, 966 032 175 793 324 179 157 914},
{96 679 114 219 819 547 625 703 547, -1 783 969 313 862 984 788 273 442},
{90 674 844 330 431 062 500 609 577, 739 313 124 672 028 016 141 231},
{68 556 211 112 064 856 492 362 868, 2 105 831 399 457 779 265 280 591},
{246 227 193 421 008 985 878 815 005, -10 823 117 433 117 574 868 747 133},
{711 285 483 202 847 094 923 061 202, 22 974 012 424 095 699 607 203 603},
{239 041 211 303 452 932 765 879 133, -6 147 456 638 952 546 131 036 858},
{186 624 172 928 144 348 618 840 527, -8 907 041 515 855 662 920 438 085},
{111 432 811 968 862 622 824 484 854, -4 316 315 153 268 894 604 713 707},
{208 133 470 241 831 504 192 811 864, 10 637 040 390 926 248 880 063 653},
{1 211 729 782 670 383 506 425 294 548, 8 326 961 392 721 850 296 127 625},
{1 053 730 715 422 745 480 856 078 626, 17 635 101 234 810 254 064 059 427},
{1 150 719 329 123 747 665 709 079 422, 56 728 223 723 158 866 725 915 261},
{4 248 726 775 729 997 103 173 615 126, -72 182 285 818 485 396 122 745 813},
{2 637 387 028 448 653 501 986 002 183, 80 996 118 452 868 871 371 068 534},
{9 332 523 570 453 063 607 185 232 457, 308 313 068 971 212 064 297 973 909},
{21 863 584 846 292 541 378 701 994 181, -881 323 158 839 081 840 203 836 315},
{44 576 954 792 024 716 741 599 301 522, 767 498 829 698 718 198 704 585 923},
{16 311 962 078 253 100 000 862 630 844, 402 561 677 812 054 309 489 272 725},
{50 776 545 266 816 318 995 955 881 703, 506 037 070 090 521 801 171 808 756},
{45 456 461 791 968 525 117 826 605 089, -2 244 606 395 513 508 372 644 075 821},
{148 419 810 886 668 065 880 558 319 947, -1 166 909 526 967 299 802 719 370 487},
{58 465 152 958 920 615 957 144 509 774, 2 545 733 262 419 533 680 794 754 335},
{22 805 276 179 637 238 398 462 901 853, -630 888 131 464 137 494 865 162 371},
{24 538 806 542 139 897 412 385 858 711, -869 780 958 925 657 261 664 760 380},
{48 639 139 054 252 944 558 185 402 673, 1 867 404 002 755 265 140 560 404 597},
{22 785 000 428 021 387 650 714 268 713, 1 206 426 030 866 872 025 222 190 106},
{36 055 763 672 134 557 897 431 288 163, 768 401 484 112 179 503 600 460 442},
{15 544 899 339 262 116 980 862 736 693, 171 419 332 317 947 619 665 538 596},
{14 270 354 139 503 615 488 435 467 809, 549 292 905 788 675 745 736 080 915},
{2 961 751 093 513 875 884 793 263 003, -115 267 999 376 621 922 201 276 187},
{9 262 042 143 191 346 311 698 396 917, -323 210 706 064 294 883 792 900 149},
{29 210 971 493 052 998 711 771 047 252, 1 258 892 859 312 744 442 569 356 571},
{67 442 596 690 147 528 093 747 529 297, -3 559 804 162 887 086 746 238 407 122},

```

```

{50 938 472 437 972 582 297 720 183 523, -1 775 391 157 278 756 339 522 686 617},
{144 090 105 378 285 457 239 122 561 310, 6 168 259 827 666 265 058 337 021 101},
{583 894 016 935 837 916 008 592 984 581, 12 658 561 754 241 059 748 606 458 988},
{420 846 351 317 031 071 619 014 107 979, -11 966 249 318 863 177 905 480 211 860},
{533 265 416 243 619 215 855 360 227 177, 28 137 424 718 861 366 864 385 329 334},
{353 906 848 078 396 451 373 750 934 447, 14 407 614 194 078 184 131 934 616 348},
{1 652 562 281 445 793 956 173 606 728 539, 37 453 092 054 352 095 391 410 720 553},
{1 216 698 767 281 362 604 253 711 366 441, 56 432 068 337 777 387 541 373 259 220},
{6 524 171 607 381 599 395 659 588 472 937, 265 668 342 356 159 365 427 537 692 131},
{30 912 218 250 387 186 627 588 557 378 894, -1 699 342 156 686 763 890 707 191 434 413},
{85 227 630 096 689 824 447 946 340 137 980, 4 163 739 386 788 836 787 891 943 517 701},
{513 597 540 920 142 325 498 264 553 181 480, 19 047 317 862 352 206 966 365 294 193 403},
{178 850 878 565 590 062 116 376 580 625 463, -259 915 235 374 167 708 331 335 271 223},
{7 678 713 206 784 520 301 911 388 322 257, 225 172 650 726 357 306 538 866 135 962},
{6 007 730 589 241 804 332 154 140 981 387, 262 412 270 944 150 398 087 429 222 037},
{7 298 681 970 571 218 674 320 285 997 032, 198 169 070 983 576 001 693 541 511 485},
{8 829 871 480 947 561 133 617 231 041 119, 457 879 347 151 757 696 212 969 591 203},
{34 233 101 771 875 370 165 122 716 572 906, -369 817 038 632 758 265 699 571 580 747},
{42 049 181 915 412 067 318 546 834 816 595, -106 756 811 014 039 987 913 900 131 624},
{3 419 427 143 477 922 836 341 882 377 643, 175 555 935 842 241 510 368 359 779 006},
{22 056 327 331 012 878 647 221 249 627 127, -38 052 597 399 593 551 140 041 788 901},
{3 729 119 277 613 206 682 785 827 024 139, 139 137 233 131 918 203 751 387 405 675},
{7 255 122 457 477 807 265 929 460 349 618, 206 654 295 717 660 294 563 439 708 199},
{5 844 414 235 600 299 482 985 557 977 739, 217 026 245 522 872 144 888 752 633 629},
{4 022 425 495 036 336 829 830 703 254 172, 138 423 575 510 998 823 522 927 598 377},
{2 141 294 772 168 559 236 106 163 025 857, 44 098 258 614 038 311 054 201 439 777},
{5 133 733 678 780 635 459 573 078 605 808, -276 300 062 287 632 588 424 615 196 071},
{30 499 453 731 992 918 490 082 461 439 283, -1 320 351 606 989 442 919 887 459 700 485},
{34 549 460 834 997 340 492 443 630 297 664, -575 563 347 128 501 011 927 603 297 763},
{4 118 581 916 554 581 295 094 729 585 492, -144 469 921 534 961 700 724 672 607 881},
{18 685 047 493 298 010 817 164 099 323 991, 909 677 608 936 137 759 943 801 396 949},
{109 981 943 416 912 003 255 456 993 139 694, 3 300 519 579 107 411 295 103 639 526 453},
{280 041 691 574 634 225 980 701 745 653 935, 3 421 236 534 895 590 778 303 516 860 199},
{131 422 227 429 509 291 969 085 500 066 729, -1 316 901 003 556 698 038 251 819 707 703},
{70 450 579 580 214 618 153 371 795 039 173, -3 229 204 704 056 388 145 665 685 034 266},
{155 675 988 073 817 236 484 871 512 960 577, 8 156 962 440 996 268 450 750 373 453 099},
{182 443 545 755 579 747 121 591 763 496 048, -7 275 237 255 867 159 119 188 824 147 651},
{147 967 576 390 902 284 312 115 028 655 299, -4 436 878 542 753 149 977 815 533 237 424},
{407 803 718 252 712 116 625 239 568 740 741, 2 241 641 212 366 179 163 148 351 068 966},
{46 020 370 656 245 150 820 965 688 311 673, -910 852 207 405 167 962 280 302 695 214},
{113 903 175 333 043 212 151 724 024 935 383, 920 481 846 012 368 393 027 830 364 491},
{62 218 849 564 993 237 520 185 288 774 763, -1 964 549 423 427 274 883 475 020 437 618},
{170 090 511 970 723 951 517 041 055 230 419, -8 469 873 198 428 411 470 546 190 865 022},
{182 271 624 566 954 913 908 833 575 584 477, 3 344 867 752 597 242 837 740 699 101 615},
{433 625 438 723 099 576 429 821 737 581 221, 19 044 405 193 690 916 149 503 684 951 371},
{1 156 116 632 461 163 187 304 673 286 982 056, -36 937 458 284 530 092 408 497 706 557 701},
{2 907 576 943 512 074 854 647 272 911 344 475, -96 331 221 396 033 605 552 283 011 482 613},
{4 639 399 328 970 538 964 719 815 085 780 355, 243 326 137 889 859 453 984 289 935 896 031},
{4 261 312 483 624 056 161 814 557 887 766 458, 91 289 719 735 403 309 668 191 127 915 049},
{7 707 042 456 193 540 251 281 807 675 342 235, -214 069 011 212 763 659 309 065 758 091 747},
{146 767 816 454 759 748 880 821 002 347 209, 2 328 263 732 001 040 251 491 735 225 152},

```

```

{22 933 952 076 578 028 689 362 671 772 479, 354 366 560 286 493 587 393 928 856 582},
{26 266 951 957 586 331 196 831 127 107 313, -515 015 938 465 245 611 374 065 115 338},
{299 582 210 865 719 406 251 037 194 725, -10 694 204 443 103 763 818 963 916 394},
{37 999 938 668 087 081 172 501 887 259, -1 013 766 474 287 935 582 512 961 535},
{129 022 308 411 001 194 934 367 652 032, 3 688 512 070 111 947 155 884 181 959},
{19 886 493 287 159 302 175 202 448 179, -857 872 329 906 226 401 551 335 223},
{40 878 010 920 132 969 094 217 107 150, -247 358 756 999 881 301 480 991 149},
{16 783 611 985 121 794 011 488 269 595, -282 097 711 126 117 188 129 593 712},
{36 779 768 543 071 416 814 509 274 381, -1 191 549 054 749 506 496 433 559 842},
{41 620 316 544 943 843 206 874 229 623, 1 304 153 389 123 026 797 935 056 634},
{29 611 671 539 162 768 013 514 240 895, -149 984 545 627 421 997 030 679 817},
{17 020 321 297 446 899 397 693 356 798, -33 860 708 585 514 750 645 771 757},
{3 054 776 840 626 306 585 147 123 899, 147 565 073 457 165 863 940 894 449},
{11 595 591 619 208 434 651 866 456 390, -451 573 601 701 017 094 311 448 987},
{38 219 692 579 736 577 460 810 142 536, 762 372 932 743 538 016 162 658 717},
{26 575 082 893 194 959 654 105 358 418, 1 241 482 583 868 139 171 327 657 779},
{132 538 490 206 541 745 787 055 350 517, 4 990 692 364 264 960 187 914 248 235},
{581 283 554 325 003 152 383 519 530 764, -30 633 987 206 620 543 176 423 225 565},
{200 459 284 007 025 175 721 221 557 373, 10 927 981 431 857 779 683 662 849 719},
{987 727 595 432 892 192 221 339 019 353, 42 322 968 455 399 429 674 471 603 123},
{3 760 721 412 139 496 453 333 434 798 812, -65 427 606 896 207 497 363 319 889 943},
{8 244 476 411 640 974 253 164 881 952 043, 65 187 685 971 104 290 381 659 650 602},
{8 107 758 551 122 253 914 926 451 738 233, 158 144 826 110 078 913 629 435 227 085},
{11 143 946 330 664 311 114 042 106 264 174, -187 116 368 163 355 063 160 119 978 073},
{21 838 404 653 029 073 673 619 306 514 178, 1 050 864 527 506 629 783 357 950 513 719},
{60 424 361 672 469 917 324 083 074 041 223, -3 204 115 872 773 170 291 830 053 416 028},
{119 359 896 387 943 692 040 928 447 050 267, 355 601 170 433 169 154 485 806 113 860},
{32 111 478 809 100 836 837 533 095 360 259, -1 462 062 112 661 012 437 751 974 098 658},
{14 172 457 063 097 876 561 718 055 087 071, 87 701 834 636 189 793 040 651 858 976},
{9 268 158 914 760 786 558 164 615 631 783, 439 596 183 250 314 978 961 787 805 659},
{9 636 074 490 597 235 991 339 860 504 272, -202 293 024 854 852 428 963 491 727 667},
{19 459 554 740 583 997 512 736 257 444 672, -440 193 729 042 245 390 714 932 837 979},
{23 941 064 296 727 684 496 432 906 855 748, 384 174 899 245 072 194 247 907 520 019},
{32 144 002 949 233 823 155 474 481 631 910, -1 749 478 609 974 321 938 481 079 088 373},
{171 841 036 030 055 433 120 360 264 834 548, -5 354 847 514 810 998 901 243 403 569 683},
{127 795 791 255 212 157 790 265 209 033 996, 830 216 304 765 302 629 901 614 780 171},
{15 127 675 483 489 617 435 451 850 544 894, 170 371 016 980 376 538 466 872 587 089},
{9 295 742 301 904 250 370 249 952 685 101, 292 677 960 890 337 198 569 694 486 045},
{18 397 493 452 260 015 786 811 238 373 157, 113 292 424 208 379 122 428 847 079 743},
{11 603 752 122 183 261 727 897 012 610 033, 367 380 321 570 874 322 333 141 626 812},
{40 085 978 206 280 462 318 805 614 811 113, 621 766 664 909 235 581 509 159 941 182},
{77 035 764 499 508 281 883 696 565 347 295, 2 130 312 569 877 766 614 031 469 449 651},
{90 606 651 767 983 833 762 243 937 042 917, 784 744 010 150 163 102 884 245 647 197},
{94 966 827 988 065 232 736 145 842 813 906, -3 044 873 745 251 723 663 742 211 639 149},
{151 420 115 823 853 179 116 105 166 075 481, 630 909 283 221 107 346 894 883 303 317},
{496 504 757 090 371 530 624 572 482 463, -11 054 875 915 563 091 243 777 296 128},
{253 705 345 921 472 315 841 736 787 111, -1 979 509 869 114 244 630 594 502 088},
{86 285 743 485 287 822 043 456 719 761, 2 680 770 807 113 647 550 275 106 821},
{131 783 423 962 239 414 313 818 291 607, -6 988 629 251 324 411 919 988 321 946},
{263 139 866 799 120 399 647 434 071 521, 10 037 870 885 419 307 748 327 726 289},
{566 823 853 671 438 724 210 168 445 841, 14 897 480 995 268 941 277 929 021 481},

```

```

{189 248 448 870 585 335 651 660 575 069, -5 090 039 090 014 641 520 079 727 973},
{241 171 668 031 466 644 490 898 337 884, -9 026 597 610 631 577 150 540 358 299},
{669 720 940 819 101 844 880 821 417 707, 10 873 372 812 353 794 206 554 249 245},
{1 164 609 642 817 183 128 417 555 332 029, -34 522 326 769 341 275 827 948 913 281},
{2 406 309 910 530 525 679 702 130 235 075, 57 997 142 682 389 306 300 752 741 253},
{7 476 316 925 324 363 920 643 442 893 626, -410 061 838 994 443 318 470 610 930 263},
{25 038 605 560 613 041 489 353 337 158 596, -170 739 362 560 075 934 734 080 262 317},
{15 801 233 493 865 801 054 349 348 726 789, -396 422 378 163 200 248 508 788 120 891},
{14 639 009 390 160 937 018 572 316 627 813, -663 092 111 342 084 756 290 689 389 802},
{13 408 513 387 024 035 986 590 463 720 447, 70 397 570 249 394 061 756 169 004 392},
{8 672 435 425 100 198 517 526 809 009 321, 345 314 134 411 134 883 860 007 987 279},
{10 410 083 048 140 348 729 998 253 091 998, 135 106 843 324 143 883 220 131 704 691},
{1 803 157 503 673 936 898 653 411 498 033, -56 978 538 721 285 864 853 875 302 348},
{5 300 958 412 096 434 264 367 320 578 089, -212 068 813 338 743 153 061 821 018 138},
{200 385 320 874 019 852 867 882 219 943, 4 501 152 596 076 059 374 870 846 538},
{569 801 584 692 941 397 343 444 932 221, 9 963 685 352 949 654 128 504 081 623},
{492 209 648 175 322 460 921 329 563 730, 15 293 999 688 691 105 749 080 110 529},
{736 836 090 085 461 238 051 465 048 926, -40 082 380 824 500 766 602 669 793 773},
{4 037 900 869 289 676 510 496 504 146 156, 144 185 573 291 716 069 070 341 902 053},
{185 366 902 987 789 626 582 823 720 736, 5 168 717 819 641 899 252 764 129 699},
{185 924 830 580 830 333 888 141 436 564, -6 292 460 589 738 670 541 974 819 645},
{749 283 610 279 732 763 600 129 182 718, 2 504 610 529 996 577 299 548 950 755},
{106 531 256 228 867 722 203 134 533 899, 892 188 721 110 548 952 893 124 413},
{94 889 983 595 360 360 728 267 661 776, 4 456 243 789 565 210 562 850 776 843},
{344 231 235 811 116 932 909 554 543 199, -4 676 632 371 703 700 623 057 607 918},
{483 804 199 773 668 170 734 320 438 779, 2 967 997 221 812 161 659 619 579 523},
{5 431 638 609 170 716 894 520 827 390, 182 782 170 310 002 056 913 275 439},
{13 630 369 534 017 685 786 765 610 140, 23 281 328 501 445 382 068 963 383},
{2 838 390 856 772 103 698 994 175 355, -136 579 793 959 484 840 640 659 571},
{7 833 406 707 171 502 022 894 692 268, -357 420 535 936 435 443 391 457 475},
{7 849 256 942 110 443 441 668 883 866, -338 707 771 193 188 346 660 151 377},
{15 511 267 827 450 316 211 660 777 285, -141 011 185 804 440 695 633 302 091},
{9 833 296 963 838 995 354 933 325, -316 674 281 326 580 384 492 008},
{4 311 685 834 045 903 584 123 251, -84 554 210 248 205 039 932 329},
{152 247 705 101 557 987 913 864, -6 037 642 088 483 948 710 873},
{343 649 709 927 788 047 356 257, 3 603 350 090 112 522 043 903},
{350 171 709 546 893 187 779 136, -17 621 167 446 785 261 920 711},
{592 181 159 257 569 317 027 092, -1 758 463 059 488 372 490 963},
{110 694 540 773 211 868 416 457, -1 346 967 948 016 129 914 509},
{63 953 456 438 863 657 227 097, -1 657 468 288 879 798 773 317},
{180 893 195 618 954 167 185 958, -2 906 595 936 752 689 403 337},
{179 957 103 095 592 559 093 832, 9 449 236 699 119 433 443 753},
{110 882 328 641 034 123 244 075, 3 155 834 721 004 594 422 364},
{112 593 825 744 682 755 331 105, -1 839 815 987 649 437 292 173},
{96 008 280 991 642 173 749 176, 3 105 759 669 683 390 566 869},
{71 080 686 126 791 595 649 669, -1 684 187 201 243 306 617 339},
{90 688 626 412 624 760 736 353, -2 946 225 172 201 827 814 201},
{169 465 082 441 190 095 519 914, 8 720 402 712 749 827 023 921},
{993 464 326 422 109 483 204 145, -6 989 504 003 315 170 546 512},
{251 101 341 206 434 852 652 983, -10 832 833 977 911 496 402 582},
{511 840 004 905 724 508 516 011, -27 103 750 208 592 233 163 416},

```



```

{823 518 502 129 843 377 878 859, 45 400 936 731 598 687 902 442},
{1 657 331 572 760 619 851 979 489, 61 853 148 799 168 146 550 091},
{3 341 005 986 849 987 581 590 584, -57 782 547 791 168 724 766 765},
{2 730 409 464 940 993 633 909 718, 143 221 764 269 615 035 069 495},
{2 418 533 224 214 995 475 989 319, 65 109 729 847 474 750 576 328},
{2 491 456 822 767 012 326 943 129, 91 009 644 429 250 413 575 230},
{8 993 659 295 617 055 188 334 697, 134 825 953 526 051 123 589 866},
{10 435 732 335 261 334 245 003 475, 212 726 197 553 267 371 371 417},
{3 195 096 304 774 291 572 463 046, -70 458 945 826 264 753 754 991},
{6 428 704 301 795 322 867 462 613, -100 120 837 654 879 507 270 579},
{5 515 291 965 238 047 764 281 491, -181 327 525 089 410 936 652 698},
{19 847 613 902 154 271 816 244 913, 458 304 512 034 069 739 291 964},
{36 956 729 673 278 806 019 591 243, -1 718 213 014 707 191 786 914 538},
{221 960 599 023 485 695 935 019 959, 11 344 651 422 137 701 258 597 948},
{1 297 228 937 267 570 589 314 957 263, 20 206 192 312 197 074 284 591 285},
{1 060 581 502 469 910 631 593 251 049, 51 647 358 627 855 729 892 402 940},
{6 315 426 552 060 700 086 716 411 733, 344 301 335 608 566 803 680 227 560},
{31 034 660 421 008 874 184 219 016 739, 1 577 357 890 753 863 531 773 845 918},
{134 786 814 639 988 266 680 828 126 323, 1 302 758 715 271 809 564 894 639 818},
{158 501 412 318 864 833 626 899 193 147, -6 921 298 738 805 352 507 240 267 886},
{181 064 631 172 126 072 421 892 644 753, 3 459 128 521 622 518 828 621 292 409},
{312 956 336 559 589 546 732 970 584 555, 12 529 973 179 382 078 403 978 531 877},
{77 057 139 265 114 715 387 583 353 310, 1 373 445 499 588 579 529 645 703 589},
{37 922 308 784 570 834 312 499 461 738, 1 603 093 735 067 668 101 482 942 863},
{145 160 445 404 991 632 372 976 914 162, -5 450 246 104 683 817 879 274 074 573},
{525 000 447 846 991 446 632 275 118 267, -13 829 855 034 957 414 132 665 386 326},
{140 453 435 605 646 377 569 514 837 823, -2 254 451 481 029 220 509 169 250 877},
{178 167 714 622 527 678 268 597 547 087, -3 544 649 314 490 773 022 996 380 021},
{245 970 460 171 114 132 238 757 607 731, -10 087 356 293 892 565 932 401 553 041},
{1 018 838 097 953 140 613 474 648 038 461, 43 266 040 620 269 863 118 144 534 129},
{5 140 828 633 467 394 657 895 865 307 005, -41 780 061 796 035 210 795 959 707 627},
{494 711 561 981 760 988 111 993 716 492, -23 617 488 890 778 311 182 226 781 065},
{330 250 342 565 472 785 984 164 384 599, -15 640 150 935 112 317 612 269 824 112},
{475 286 480 094 012 541 268 994 578 961, -25 534 532 540 408 853 888 310 746 742},
{2 595 714 839 697 744 526 143 227 203 031, 132 533 396 232 488 272 483 017 098 767},
{14 452 661 342 381 502 885 001 185 117 267, 203 784 990 244 933 540 885 727 757 421},
{4 227 189 797 308 750 203 882 728 481 112, 7 885 869 858 835 895 148 274 644 317},
{95 614 431 822 836 359 177 530 453 600, -2 994 360 220 699 956 160 542 238 229},
{53 940 048 004 868 583 432 967 638 464, 2 412 160 999 841 560 027 170 935 443},
{229 469 080 197 171 125 659 456 442 834, 1 831 486 901 489 731 620 838 450 959},
{140 236 205 381 079 013 372 969 188 217, 2 318 512 743 548 340 150 097 012 076},
{295 990 922 030 972 948 560 045 941 791, -10 349 011 713 197 546 823 289 299 019},
{1 086 299 842 411 804 149 935 400 926 880, -33 198 493 150 236 698 809 182 107 923},
{2 432 863 496 599 817 531 881 070 894 277, -121 459 291 016 361 817 786 568 908 354},
{967 228 859 688 849 327 369 187 252 811, 51 990 034 153 074 424 459 103 716 798},
{5 413 010 564 745 525 924 045 025 350 313, 54 674 427 191 106 182 229 227 838 243},
{63 717 753 241 651 321 436 442 799 328, -2 667 419 401 231 466 988 948 871 019},
{78 982 158 018 722 096 460 817 648 664, -3 902 496 662 353 096 683 863 867 675},
{245 175 114 946 622 812 071 097 628 132, 955 076 170 634 959 605 208 072 203},
{73 498 218 425 755 100 920 132 074 257, 50 322 122 069 638 002 135 317 672},
{5 891 704 430 323 312 486 132 712 705, -241 605 672 423 078 812 702 717 436},

```

```

{24 503 260 840 557 718 073 350 985 383, 1 302 839 502 647 275 221 361 306 068},
{65 931 393 661 754 427 851 137 266 067, -956 714 819 916 709 601 673 329 917},
{21 547 303 987 114 616 716 817 028 178, -233 479 382 400 932 887 273 717 073},
{17 673 812 038 172 056 048 020 112 506, 957 270 608 872 779 972 345 734 537},
{116 493 503 635 510 351 544 582 290 920, -5 143 655 374 428 463 835 268 503 969},
{476 179 903 778 555 283 314 037 996 521, -12 388 398 688 928 777 935 731 932 871},
{1 425 658 196 605 832 821 887 055 972 249, 43 090 086 762 119 952 443 251 035 534},
{969 242 698 894 964 901 319 983 301 901, 3 977 775 079 668 760 036 510 292 044},
{350 952 603 127 900 015 782 852 647 605, -1 303 559 834 459 127 784 816 605 767},
{77 587 014 157 790 758 469 838 122 166, -627 352 724 966 273 471 359 629 601},
{53 842 343 101 140 970 412 814 418 154, -1 241 908 611 917 483 782 247 481 633},
{115 791 743 425 251 125 133 422 186 905, 5 343 717 737 334 268 503 134 113 511},
{465 522 307 375 031 649 043 945 618 631, -19 451 123 570 434 360 805 604 859 522},
{343 125 136 948 361 706 420 175 602 911, 7 908 194 260 601 604 288 574 307 531},
{808 142 124 275 585 889 019 339 697 514, 30 308 334 295 576 346 237 630 035 627},
{2 678 103 148 408 545 821 324 542 541 145, 2 120 115 259 205 647 096 900 667 044},
{104 562 496 366 960 477 957 016 982 699, 4 164 476 886 640 375 396 785 546 956},
{118 501 014 850 137 468 830 495 214 137, -2 341 332 330 443 909 698 961 384 936},
{238 523 642 658 006 489 748 814 828 537, 10 845 423 237 963 731 197 720 699 635},
{19 900 835 802 441 906 073 668 182 879, 359 048 689 530 554 228 697 420 095},
{40 280 521 982 754 379 266 550 423 002, 1 156 657 485 328 853 503 584 193 699},
{53 254 870 987 694 753 389 741 749 769, 1 154 007 021 795 513 773 062 603 367},
{44 854 120 081 594 514 990 704 655 281, 1 804 461 088 339 145 058 595 730 418},
{67 698 074 370 521 317 711 603 159 447, 3 174 361 263 715 745 683 374 093 730},
{272 596 299 945 043 148 876 511 263 771, -6 771 107 625 173 474 199 332 536 014},
{460 774 668 721 399 577 544 183 504 493, -2 526 443 244 880 097 666 486 412 517},
{253 005 514 297 333 990 081 640 142 937, 5 096 141 238 908 675 298 946 281 733},
{473 807 031 450 240 789 672 247 196 519, 18 081 780 834 248 645 095 281 463 823},
{968 031 926 821 092 522 266 363 062 823, -47 843 977 100 308 779 323 498 957 456},
{2 933 077 206 323 154 114 448 969 303 889, 30 381 248 289 845 423 629 980 587 165},
{3 656 719 859 257 070 124 355 832 243 508, 73 980 819 044 800 627 620 743 222 885},
{8 326 507 954 263 754 557 065 966 723 609, 176 182 237 122 388 162 152 145 433 668},
{12 082 958 901 527 376 145 679 542 739 019, -296 023 290 995 513 307 844 062 276 511},
{14 200 955 702 920 072 168 803 787 256 116, -440 116 936 750 740 131 176 988 279 007},
{30 827 210 173 750 036 409 862 692 235 596, -178 019 645 606 114 955 347 862 077 329},
{7 840 420 263 635 222 421 511 401 569 577, -134 383 019 302 688 343 609 951 212 213},
{12 151 952 892 855 503 431 302 821 701 649, -504 055 440 815 971 300 206 797 849 877},
{14 365 668 390 586 555 527 334 079 110 063, 493 374 196 459 811 409 056 335 490 385},
{15 205 790 325 282 486 816 192 020 780 174, 652 737 637 159 324 305 934 932 062 021},
{50 712 888 372 541 306 058 097 422 020 733, -1 679 380 312 704 681 479 149 302 656 686},
{87 178 974 738 426 622 791 624 030 200 239, 515 952 287 418 256 930 602 056 375 684},
{4 460 962 673 064 000 272 479 787 363 891, 67 077 820 421 462 160 131 485 212 536},
{8 745 090 630 752 652 014 716 853 393 523, -284 290 690 035 101 910 465 791 614 006},
{17 863 159 968 238 396 157 066 586 494 369, -80 226 410 497 142 661 897 483 527 048},
{7 187 677 600 221 788 316 999 129 819 105, -299 509 404 170 340 195 525 781 619 681},
{144 150 264 856 986 787 962 441 001 857, -4 131 898 278 738 132 285 481 745 933},
{122 603 998 396 982 453 737 487 824 874, 5 163 481 981 135 282 827 053 729 019},
{347 046 686 519 519 871 403 839 626 066, -18 633 073 520 280 260 036 434 076 267},
{1 836 189 826 206 733 222 851 257 450 841, 41 227 921 233 380 164 850 317 245 349},
{5 014 523 504 683 413 393 623 889 134 232, 215 701 706 938 049 983 917 346 594 333},
{14 040 056 463 473 369 807 053 293 182 699, -551 746 076 459 872 491 974 285 177 250},

```

```

{64 804 397 169 834 624 524 091 066 631 087, - 2 194 577 962 543 110 925 462 025 776 330},
{271 663 668 798 638 952 059 432 851 267 819, 8 023 123 890 092 688 283 404 410 168 827},
{295 228 931 166 774 238 571 395 846 214 637, 5 912 847 511 590 432 822 363 205 882 114},
{108 735 880 552 566 869 799 049 795 349 569, 3 606 540 509 423 769 020 445 402 311 528},
{141 931 965 971 549 185 835 871 938 980 727, - 6 147 708 392 919 507 104 446 492 664 737},
{140 618 981 747 337 400 037 485 822 937 088, - 4 273 737 185 854 708 723 962 772 429 415},
{108 972 836 483 280 805 414 130 482 438 641, - 5 512 641 996 346 493 654 519 729 876 537},
{336 640 905 679 704 798 857 462 269 222 037, 2 140 950 272 032 289 283 974 788 365 262},
{134 580 511 277 105 274 909 590 415 362 489, - 837 772 095 698 081 624 017 115 181 200},
{79 109 382 265 182 904 534 428 877 216 993, 2 256 866 711 342 213 171 782 904 890 125},
{31 309 457 838 031 646 293 155 194 468 534, - 252 327 525 750 223 692 799 854 235 709},
{5 482 141 636 027 905 510 969 810 282 534, 132 278 290 158 920 048 367 213 579 953},
{15 446 447 491 704 267 841 396 071 673 243, 724 781 394 729 526 530 426 138 940 259},
{59 448 047 227 047 414 743 601 483 012 452, 519 378 608 744 276 744 018 088 004 953},
{62 826 973 342 564 738 416 875 467 774 030, - 1 957 207 416 177 453 136 124 114 427 161},
{51 636 374 545 080 610 017 701 005 582 914, - 2 308 525 501 588 835 841 708 160 611 763},
{223 237 953 163 196 254 531 947 168 645 664, 8 247 587 923 646 761 218 821 049 099 131},
{145 459 836 104 963 527 053 835 700 880 401, 3 810 459 086 656 343 455 765 688 939 248},
{174 208 783 561 911 118 236 494 072 700 951, 3 265 395 260 724 920 879 178 238 044 908},
{300 565 537 537 951 961 332 481 012 377 501, - 2 898 443 021 040 785 371 905 460 092 754},
{229 477 139 026 195 661 915 638 201 724 645, 3 183 628 781 672 462 063 587 580 438 252},
{67 292 954 139 717 447 718 423 874 841 763, - 1 180 956 335 937 443 714 774 473 471 501},
{5 669 493 292 529 978 238 652 727 887 822, - 109 650 284 325 216 906 715 633 068 159},
{8 500 552 496 282 139 477 330 405 645 298, - 218 996 873 257 472 127 400 802 219 137},
{10 605 622 479 688 928 212 131 676 974 835, 293 555 827 787 538 367 859 223 248 086},
{9 892 134 665 774 852 899 505 331 503 357, - 239 324 047 886 618 835 083 135 811 983},
{21 000 208 737 375 413 868 448 724 770 202, - 420 690 596 595 395 988 099 123 513 247},
{9 026 447 299 723 396 101 459 584 634 924, 162 030 487 062 102 852 585 062 159 549},
{12 429 373 623 397 638 188 924 726 852 660, - 127 299 894 160 134 899 668 574 423 207},
{12 102 209 129 738 060 370 634 021 487 638, 118 269 049 818 544 131 049 272 624 591},
{10 195 470 688 845 017 948 960 223 970 628, - 373 271 073 928 804 463 910 888 569 639},
{30 810 895 197 799 222 345 319 171 268 625, 354 281 174 021 559 042 437 914 690 318},
{3 042 105 766 096 973 202 983 985 517 783, 76 738 252 382 435 574 405 969 694 908},
{7 212 598 579 718 290 366 012 999 255 231, - 299 521 706 254 470 459 038 377 821 479},
{6 332 416 587 692 828 811 177 994 950 305, 128 183 490 319 136 247 166 288 662 618},
{13 524 922 820 505 160 107 850 676 772 049, - 588 591 936 854 017 915 176 353 240 807},
{3 337 924 237 097 260 537 032 762 592 656, - 153 617 226 102 238 485 930 879 012 767},
{10 955 195 870 972 358 356 449 406 001 334, 537 747 010 437 972 951 448 246 733 095},
{52 667 239 161 992 523 128 415 962 271 142, 2 049 522 845 008 954 301 696 838 557 921},
{163 153 314 567 195 932 229 583 981 753 452, 684 174 931 696 201 314 332 463 546 257},
{84 076 056 580 505 107 054 363 986 747 218, 3 793 873 287 590 246 099 268 495 564 005},
{160 652 038 675 679 224 930 213 181 185 404, 5 777 606 920 253 502 485 309 366 621 923},
{294 811 189 043 156 145 172 109 152 079 720, 8 351 169 577 214 115 829 738 381 797 971},
{662 826 760 094 129 967 522 902 546 643 305, 3 736 757 431 293 179 019 957 851 726 923},
{373 642 720 627 404 900 465 414 027 196 642, - 6 036 345 215 041 487 043 587 516 461 315},
{160 609 551 458 998 910 334 154 265 485 544, - 6 323 068 930 732 086 137 785 957 431 835},
{666 133 814 153 247 061 939 901 708 382 947, 26 429 274 412 198 191 062 348 098 436 618},
{1 420 713 862 100 871 055 255 402 083 951 711, 58 006 059 987 168 102 987 310 120 304 362},
{7 513 495 093 524 021 476 269 268 718 167 049, 342 877 279 212 514 467 363 860 990 301 200},
{7 838 727 926 791 059 908 482 017 004 809 313, - 284 696 192 580 138 817 905 465 975 812 984},
{34 917 317 414 093 499 125 080 973 621 964 857, 1 721 327 184 068 836 037 199 846 446 029 103},

```

```

{129 073 491 704 512 714 225 103 756 463 675 611, - 2 728 974 551 066 459 862 433 867 577 581 527},
{213 473 892 554 333 481 657 250 823 461 430 446, - 11 551 917 111 961 342 900 684 296 814 799 061},
{1 456 858 133 764 708 384 017 505 449 097 452 524, 14 046 680 559 316 321 278 377 855 778 935 705},
{1 051 117 478 301 714 609 587 178 152 819 389 348, 14 609 019 987 226 354 345 184 104 346 728 273},
{192 505 684 767 303 558 978 345 718 147 179 004, - 110 129 858 871 949 143 356 041 841 465 107},
{344 146 247 111 968 908 055 652 996 772 416, 10 069 195 693 210 145 424 426 892 459 077},
{471 715 101 762 702 433 411 465 782 078 874, - 4 526 382 522 373 954 955 795 312 519 991},
{255 457 011 618 324 036 302 112 639 950 030, - 7 371 530 566 408 418 712 672 152 989 053},
{669 744 808 170 272 702 691 543 957 374 975, 18 607 651 663 567 665 807 589 377 334 889},
{34 361 401 876 939 058 380 163 817 110 627, 1 446 188 622 968 681 151 438 245 718 765},
{91 293 894 543 343 073 895 123 076 749 779, 2 184 224 048 073 615 469 937 689 950 571},
{116 644 570 121 928 046 514 354 008 815 389, 4 336 771 208 791 605 555 558 575 334 742},
{117 890 411 562 114 816 746 339 133 555 635, 3 369 591 504 222 234 464 739 055 152 894},
{11 911 555 529 471 443 635 810 557 257 265, 370 436 250 402 180 530 250 769 735 503},
{15 147 620 866 238 333 627 698 464 667 447, 549 074 931 770 144 240 025 377 431 031},
{59 563 509 734 660 439 462 183 194 573 723, 85 761 426 251 914 215 047 705 745 445},
{10 699 237 240 444 218 940 714 508 275 176, - 139 742 862 866 500 776 810 131 737 883},
{16 033 321 672 677 649 774 062 147 497 345, - 374 216 034 401 887 761 307 397 902 106},
{15 245 533 136 726 802 047 018 083 115 019, - 764 100 050 933 018 025 005 835 433 565},
{9 591 052 948 525 873 164 938 521 301 903, 20 283 941 476 664 003 107 903 919 285},
{855 110 293 220 680 241 308 552 734 226, 39 837 896 176 471 512 975 024 626 051},
{4 869 306 534 386 737 303 088 359 421 765, - 261 027 944 159 504 010 729 163 898 487},
{23 729 018 421 329 630 901 393 472 815 344, 621 148 212 495 023 644 391 099 588 129},
{32 976 609 134 426 625 021 834 066 674 246, - 267 202 320 754 582 488 994 257 028 883},
{29 120 328 264 213 444 267 138 907 990 531, 367 498 510 625 327 989 318 855 008 177},
{23 129 778 225 696 208 179 682 296 616 124, - 264 300 848 950 227 075 338 436 541 345},
{33 847 174 745 952 680 376 331 302 848 068, - 1 400 638 266 090 001 191 156 770 878 301},
{60 978 222 625 467 420 393 594 865 205 972, 1 443 029 887 609 289 493 008 080 313 017},
{97 564 411 965 719 823 748 194 411 584 854, 2 985 004 375 822 524 096 800 682 176 601},
{247 412 630 779 372 990 357 990 363 903 477, 6 099 828 190 815 648 819 252 891 899 276},
{704 925 486 590 044 753 852 467 643 278 657, 28 063 137 653 268 600 445 815 646 295 363},
{880 272 902 940 722 331 961 115 790 275 066, 3 717 453 450 888 990 852 940 064 021 741},
{200 817 573 951 715 548 833 677 696 795 913, - 3 381 419 703 998 357 396 344 285 962 807},
{345 532 402 358 677 624 182 948 972 448 900, - 13 001 167 804 655 541 512 208 939 688 141},
{1 446 270 760 526 785 118 080 100 971 428 541, 70 337 957 108 011 459 875 280 067 258 720},
{8 107 327 089 002 806 836 105 255 984 204 277, 274 357 574 139 409 486 976 630 882 745 251},
{32 454 235 552 202 654 349 935 341 014 305 539, - 583 963 594 567 586 622 525 033 233 114 273},
{65 151 870 562 117 682 515 694 770 544 655 987, 2 717 447 529 717 606 240 973 035 891 960 658},
{17 586 849 740 580 091 394 077 896 811 148 715, 888 786 657 454 189 833 321 878 954 660 251},
{49 676 336 436 474 486 630 596 440 180 808 215, 1 786 719 493 668 548 468 869 640 648 566 322},
{92 525 868 582 400 940 909 169 968 489 834 663, - 593 505 584 171 003 309 549 186 521 842 152},
{16 043 670 196 476 325 072 322 905 313 295 887, 413 465 437 705 499 367 451 057 679 728 928},
{21 429 732 872 033 517 924 574 523 582 796 215, - 44 590 149 653 889 109 657 012 128 213 194},
{4 767 956 321 118 824 777 905 553 078 276 037, 160 836 230 175 078 393 772 353 735 506 860},
{15 025 343 627 117 610 274 710 513 562 527 669, 776 531 900 633 767 027 725 443 706 737 122},
{71 335 466 464 997 664 704 822 864 379 378 313, - 285 196 500 650 979 645 228 988 557 989 568},
{9 557 762 492 474 143 562 415 643 962 400 319, - 179 938 332 788 401 086 806 458 741 437 917},
{5 531 114 783 177 007 920 085 965 208 158 834, 248 011 782 910 559 474 975 317 925 231 945},
{19 687 012 055 055 960 775 419 334 353 739 572, 102 762 449 588 602 471 303 972 177 243 255},
{11 408 483 946 352 707 030 094 127 041 897 044, - 609 160 274 772 797 552 460 563 343 054 773},
{43 542 615 148 907 420 730 679 613 225 778 109, 1 767 012 731 008 487 706 784 471 553 938 948},

```

```

{166 400 922 218 155 019 939 162 188 768 940 433, - 6 014 581 684 272 611 158 488 692 231 639 849},
{527 936 979 608 738 327 111 073 947 564 514 157, 10 068 233 786 350 308 340 431 376 529 589 850},
{1 154 260 374 971 363 166 472 942 790 796 434 691,
- 24 847 549 769 945 592 329 750 100 455 621 263},
{2 964 821 500 666 736 777 067 238 667 356 283 959, 3 484 031 746 542 413 849 862 086 128 431 771},
{23 542 613 545 498 610 499 313 147 997 281 606, 71 266 116 642 783 651 551 561 333 363 621},
{6 521 099 038 941 443 159 349 800 656 395 788, 47 518 428 527 962 935 438 008 260 478 619},
{2 912 548 950 567 024 142 121 939 326 971 055, - 27 721 217 645 003 891 362 433 497 181 238},
{478 948 732 344 889 404 469 018 333 500 095, - 2 646 678 490 596 064 498 673 748 523 464},
{26 319 581 138 544 955 014 629 251 931 807, - 441 749 841 192 781 722 642 896 676 408},
{48 762 654 584 772 414 457 416 295 652 999, - 2 110 946 234 301 450 381 540 214 510 070},
{55 464 384 505 671 644 363 728 185 325 307, 1 363 006 197 986 494 430 127 694 397 161},
{110 162 707 896 726 972 406 415 944 031 322, 5 945 932 173 477 691 087 754 287 262 437},
{739 030 894 028 828 622 620 780 170 160 003, - 15 468 288 583 246 554 314 929 360 826 400},
{906 549 945 322 573 922 403 066 320 392 811, - 30 273 125 376 271 780 714 436 866 714 033},
{432 323 598 947 408 244 900 436 110 411 077, 831 252 657 964 525 414 720 726 319 782},
{18 993 019 939 872 691 608 165 544 726 931, 813 562 585 901 979 165 743 862 800 674},
{73 924 162 065 445 919 362 912 181 905 827, 2 032 290 140 333 740 363 883 881 759 796},
{200 331 574 532 423 027 193 311 339 483 973, 4 337 265 559 612 396 589 123 669 819 332},
{214 965 361 836 482 216 622 724 810 006 363, 2 937 406 146 184 844 616 966 472 260 524},
{140 629 562 391 991 170 637 324 101 873 193, - 2 796 272 786 797 262 787 703 528 243 138},
{214 587 762 709 672 219 314 842 395 385 059, - 1 904 919 064 580 017 485 254 872 997 887},
{175 708 087 609 745 964 486 020 637 933 236, - 2 747 343 269 251 816 672 491 447 189 407},
{32 054 866 683 389 571 552 611 315 657 556, 1 499 601 870 517 878 761 643 981 802 249},
{148 128 806 861 212 917 777 064 524 116 001, 2 389 019 796 376 293 883 329 538 003 895},
{2 519 404 787 149 313 796 523 150 996 393, - 82 908 486 193 212 198 877 737 148 193},
{8 455 502 955 825 279 340 242 612 808 589, - 360 747 566 398 605 567 423 490 722 558},
{41 635 248 236 883 389 139 111 787 905 565, 1 533 527 589 493 671 074 538 589 528 041},
{60 490 873 305 773 043 287 875 980 544 454, 3 111 978 272 405 472 372 074 117 557 863},
{358 544 252 208 164 941 457 017 446 549 991, - 11 790 967 569 423 311 191 364 971 821 744},
{1 266 404 207 997 454 303 325 960 769 087 473, - 28 910 840 711 274 396 477 417 358 404 574},
{1 491 942 007 536 834 261 945 989 187 724 929, 36 058 186 707 231 271 903 162 308 216 440},
{3 565 320 718 112 605 959 995 986 873 783 807, 48 081 735 916 753 224 762 839 668 704 976},
{1 912 604 451 764 107 144 558 915 468 898 329, - 8 236 328 683 051 817 154 585 061 705 732},
{467 139 888 870 503 514 832 643 283 316 815, - 2 746 137 010 410 112 925 226 669 368 426},
{78 005 037 506 275 514 100 796 049 995 885, 276 503 772 737 838 116 105 263 290 182},
{8 146 055 275 958 489 446 403 969 279 543, - 36 480 557 882 004 017 939 039 235 923},
{2 864 298 355 429 076 297 531 772 871 782, - 119 331 326 680 758 699 516 207 266 569},
{91 133 468 898 154 904 555 998 695 138, - 1 306 682 441 837 436 933 104 938 205},
{87 921 434 012 474 040 234 255 532 756, 4 340 921 280 579 940 639 414 847 735},
{290 091 209 430 184 818 287 106 028 728, - 9 878 473 721 213 065 414 650 536 159},
{950 869 008 446 557 291 969 246 270 771, 23 178 259 700 256 711 071 257 075 008},
{147 374 873 576 452 306 546 729 401 509, 1 959 296 818 013 742 935 735 284 479},
{112 462 015 285 877 214 411 346 248 592, - 5 536 627 425 877 802 399 794 063 335},
{454 849 760 068 466 767 267 290 237 596, - 1 651 460 847 761 075 739 788 885 933},
{183 581 083 686 956 911 066 157 383 523, - 9 235 800 051 061 174 928 393 933 590},
{298 483 258 912 112 512 952 698 816 851, - 6 517 185 907 007 772 526 280 108 272},
{343 818 009 094 441 116 376 961 042 843, 8 002 776 173 288 825 088 724 897 931},
{79 259 351 885 309 321 249 116 433 970, 1 519 335 346 814 082 312 023 924 057},
{66 779 342 806 961 789 278 436 730 578, 1 956 105 582 057 404 678 140 239 595},
{71 471 043 473 637 948 298 837 683 524, 2 201 331 017 190 462 505 601 517 505},

```

```

{270 482 592 891 847 955 451 939 444 732, 12 273 598 648 817 025 079 592 130 251},
{121 880 148 500 705 173 340 008 332 230, 2 535 024 239 987 837 581 178 954 413},
{52 333 050 078 998 963 619 070 866 778, -2 674 101 939 291 923 809 837 635 165},
{302 184 029 898 791 807 930 323 005 286, 3 554 687 568 512 802 179 059 606 497},
{9 359 269 278 552 772 797 447 149 783, -118 846 381 116 116 185 370 690 523},
{7 783 440 190 166 737 718 236 603 442, 359 596 109 834 852 654 244 406 053},
{33 578 321 490 605 437 561 906 717 412, 1 692 589 668 249 340 989 529 819 957},
{71 923 102 962 303 526 145 386 294 464, -1 032 758 754 211 940 854 299 522 419},
{97 312 585 956 003 751 417 612 289 758, 3 358 423 771 798 544 385 075 118 347},
{21 488 001 078 511 402 135 895 426 215, 520 508 725 187 529 782 205 187 924},
{38 698 699 951 365 120 221 955 710 053, 344 769 800 872 303 951 999 028 844},
{22 218 832 714 441 408 290 958 115 075, 24 999 444 641 676 652 558 055 647},
{1 492 149 438 402 724 119 332 393 404, 6 489 589 836 606 835 123 290 119},
{119 986 916 431 013 223 399 833 058, -28 079 999 382 927 391 934 491},
{283 794 822 057 625 567 042 945, 99 942 375 226 646 863 527},
{10 920 703 131 551 173 292 305, 207 203 216 265 063 335 329},
{16 060 707 920 759 255 274 716, 405 084 239 256 291 447 141},
{37 520 013 816 501 886 673 012, 1 029 728 792 866 918 038 613},
{118 291 422 876 016 205 414 272, -3 095 686 911 338 461 157 677},
{172 349 224 475 681 214 129 598, 3 018 688 025 872 449 445 811},
{74 693 841 250 269 673 931 573, 3 239 460 155 211 724 303 429},
{48 985 769 945 203 932 561 678, -1 454 670 772 185 021 497 065},
{124 408 549 289 827 963 033 916, -1 527 069 893 819 597 159 889},
{188 278 515 185 875 980 804 541, -7 165 154 441 787 264 369 050},
{521 923 420 944 069 196 030 383, 14 730 594 142 551 070 183 487},
{1 670 740 626 107 597 516 992 894, 5 397 053 028 852 036 779 239},
{616 948 776 008 411 642 224 548, 9 175 070 861 050 030 918 507},
{583 604 447 649 667 090 044 277, 32 026 251 178 238 787 014 074},
{1 875 696 654 080 026 957 018 535, -56 956 478 910 849 402 732 143},
{1 017 060 444 214 876 616 394 392, -48 190 860 967 559 671 973 415},
{1 328 771 704 680 481 802 554 051, 72 917 675 451 409 266 595 926},
{4 274 682 743 995 246 006 601 729, -148 118 210 311 102 436 029 849},
{5 456 028 372 028 579 863 403 596, -149 904 913 556 002 451 586 133},
{15 635 740 295 285 292 457 638 504, 229 147 571 103 256 636 819 957},
{14 124 536 049 390 223 470 815 564, -475 064 358 247 849 556 246 377},
{33 504 805 585 904 225 959 421 198, -669 246 053 445 098 250 888 405},
{11 178 266 289 769 428 145 249 324, 247 870 847 641 892 025 280 841},
{6 332 552 367 567 483 001 818 977, 251 273 479 895 543 120 702 320},
{13 338 142 357 052 010 860 636 951, -98 632 870 943 163 715 864 825},
{5 971 357 067 651 124 566 906 488, -261 339 189 179 730 712 862 519},
{10 373 846 555 945 321 008 971 087, 99 153 494 402 795 142 121 237},
{9 802 103 719 568 424 318 563 874, -137 201 009 609 558 401 761 923},
{15 998 825 807 211 559 681 910 683, -801 283 899 242 739 452 327 969},
{7 062 122 720 169 322 902 607 311, -293 598 597 299 100 811 853 876},
{4 143 929 252 607 598 964 057 481, 5 611 750 754 138 660 551 199},
{646 242 562 009 346 522 698 797, -20 541 948 101 425 934 059 634},
{2 483 290 937 532 495 081 587 609, 73 926 751 107 668 115 399 198},
{7 947 491 833 722 081 442 087 349, -163 268 659 511 817 163 480 600},
{13 852 862 859 880 366 505 519 413, 169 601 777 756 744 404 212 388},
{14 329 006 953 413 430 292 753 989, -365 139 617 811 970 711 978 808},
{23 291 768 850 348 574 227 665 451, -1 004 845 049 475 977 302 574 683},

```

```

{47 427 503 361 488 318 601 756 146, 2 437 833 629 039 350 457 068 789},
{291 578 739 761 793 558 289 127 765, -1 875 113 212 233 581 911 418 393},
{246 218 460 649 739 211 069 811 550, -4 462 620 980 307 068 640 521 659},
{203 642 670 739 664 626 214 640 215, -6 014 764 682 301 804 047 776 377},
{226 003 384 610 935 100 765 986 589, 11 890 017 589 182 718 939 873 470},
{24 472 259 529 884 958 906 743 317, -442 921 797 657 290 731 717 039},
{29 340 453 247 033 758 186 523 236, -19 105 065 604 178 993 937 689},
{1 295 938 019 101 419 964 738 884, 23 198 453 944 926 112 038 187},
{835 130 677 198 327 372 091 644, -23 474 314 672 987 275 231 749},
{2 615 443 220 683 423 034 097 160, 117 452 282 204 000 808 896 107},
{8 282 662 207 391 577 694 677 978, -162 159 805 017 352 305 770 575},
{3 290 695 846 238 456 399 585 739, 168 553 736 056 107 078 089 341},
{21 139 644 094 409 197 658 884 303, -40 872 521 845 637 164 701 052},
{2 248 728 956 488 062 719 830 197, -87 248 877 567 539 291 174 183},
{5 192 109 250 473 177 733 721 543, 45 896 889 430 566 768 479 369},
{1 515 075 887 431 951 530 398 498, 42 446 737 889 574 195 731 599},
{3 420 755 943 885 232 691 974 358, 152 316 570 707 965 389 576 883},
{18 355 135 125 528 453 897 411 116, -419 747 123 601 692 885 380 331},
{29 913 176 304 806 694 602 066 824, 1 545 928 017 891 591 082 487 317},
{142 163 062 759 880 041 154 451 663, -991 080 803 825 427 550 917 583},
{115 327 554 777 946 061 161 408 322, -6 319 719 956 624 649 413 693 809},
{413 592 631 938 723 761 023 896 880, -20 296 585 307 006 725 425 242 327},
{2 014 823 485 028 973 412 510 239 420, -5 997 579 924 649 033 579 695 361},
{95 566 218 765 791 880 326 693 388, -3 294 470 810 439 831 738 280 657},
{6 986 664 178 667 858 053 790 105, 245 883 428 616 530 417 366 584},
{26 807 110 657 516 674 659 273 039, -362 835 458 246 562 714 018 822},
{11 233 585 467 718 104 845 504 507, 47 032 175 064 518 045 461 349},
{1 868 450 020 549 209 196 328 752, -7 853 540 996 291 577 581 827},
{182 189 717 432 988 522 417 462, -3 722 847 147 698 048 302 537},
{60 435 507 508 767 079 001 813, -497 924 527 558 002 838 582},
{49 086 234 327 417 445 281 833, -1 052 937 470 634 815 306 930},
{105 680 446 406 163 899 839 651, -2 748 892 746 579 978 415 802},
{321 523 295 500 801 370 303 025, -13 896 011 398 196 700 634 426},
{503 653 769 018 918 252 052 701, 10 722 819 392 935 164 434 440},
{83 829 264 096 067 284 252 477, -824 538 632 004 789 173 465},
{71 976 884 894 778 608 970 639, 2 565 063 743 450 994 355 096},
{40 791 320 553 651 728 351 113, -73 575 428 225 056 196 602},
{8 030 262 363 266 599 038 115, 129 918 604 050 106 933 664},
{6 493 756 101 928 113 300 939, 201 401 408 144 818 328 144},
{12 863 603 860 302 748 487 053, 487 023 033 703 763 546 709},
{52 864 310 793 287 719 698 797, -154 121 931 034 009 146 455},
{128 461 987 739 188 224 516, 6 190 915 155 002 308 871},
{406 921 625 671 248 846 825, -12 902 027 207 493 939 973},
{1 563 073 426 730 552 097 793, -53 848 926 192 288 527 481},
{382 551 161 550 602 621 972, 11 034 761 804 816 696 433},
{964 026 925 529 201 087 129, -32 054 587 787 078 419 590},
{628 383 774 131 155 349 827, 22 958 213 808 366 627 632},
{2 238 656 343 282 434 189 669, 113 657 323 141 966 048 168},
{9 070 901 443 461 221 480 733, 114 528 028 154 422 442 986},
{6 098 238 665 866 151 512 657, -138 449 732 099 170 209 577},
{1 696 469 271 200 182 603 747, 65 035 015 473 492 007 444},

```

```

{1 461 982 517 909 677 883 389, 16 246 103 542 276 993 750},
{43 868 635 451 158 731 193, -1 454 706 912 303 235 873},
{59 813 585 582 215 265 789, -53 883 908 047 319 553},
{643 731 868 617 795 217, 24 900 388 814 319 761},
{967 377 265 838 383 647, -41 994 717 222 748 582},
{394 176 435 088 726 643, -4 672 907 668 198 540},
{434 526 222 492 961 429, 16 777 267 140 943 362},
{442 556 194 121 853 529, -20 513 780 280 888 576},
{2 300 453 651 173 822 609, 68 218 230 737 353 401},
{4 988 108 994 698 765 575, 209 252 874 732 780 462},
{8 931 479 707 534 929 919, 117 532 139 334 731 606},
{253 237 940 928 772 031, 445 140 655 201 733}, {12 385 164 706 694 098, 375 158 930 974 945},
{1 293 955 929 000 119, -67 450 519 271 549}, {3 260 164 527 100 944, -124 681 271 799 739},
{4 852 734 060 932 990, -150 541 198 956 987}, {9 314 327 603 373 778, 462 814 938 250 605},
{15 261 584 489 121 314, 556 114 260 725 451}, {64 829 355 227 478 031, 3 288 369 840 994 153},
{246 704 938 802 522 627, 5 661 329 570 404 673},
{629 506 883 659 425 055, -31 250 239 189 091 134},
{1 184 052 267 809 424 625, 6 523 569 648 570 883},
{851 438 364 615 209 303, -25 771 721 265 627 947},
{255 521 029 415 094 676, 12 290 062 204 856 367},
{675 982 821 251 815 153, -27 151 081 926 602 864},
{734 881 678 186 445 561, 9 867 464 066 100 488},
{1 233 295 708 587 485 087, 11 318 199 834 221 945},
{102 063 289 131 919 434, -5 597 044 636 207 327},
{346 235 733 889 325 124, 16 922 564 969 589 787},
{2 047 306 272 850 227 992, -64 337 421 564 928 739},
{3 022 190 130 830 305 528, -74 768 407 883 900 867},
{8 272 353 469 733 233 024, 403 442 999 118 873 003},
{52 586 721 593 695 310 257, -1 731 863 627 925 379 431},
{165 903 754 810 622 887 001, 1 859 113 907 722 521 722},
{116 408 277 132 753 334 409, 1 182 998 034 087 188 100},
{124 785 555 350 940 860 167, -5 342 868 438 406 235 903},
{499 589 873 378 125 246 674, 27 109 876 467 625 493 603},
{3 053 981 500 707 853 158 660, 58 130 461 817 890 469 209},
{7 083 372 593 409 869 576 671, 332 814 413 292 998 059 893},
{24 792 987 449 567 413 875 434, 47 710 265 645 713 795 955},
{4 300 230 471 588 885 566 658, -219 382 467 187 672 377 001},
{22 991 163 379 279 798 994 206, -610 798 863 405 001 081 191},
{57 647 872 118 993 669 946 676, 1 724 864 245 589 768 340 533},
{191 293 579 821 735 768 489 881, -10 411 288 680 869 710 837 327},
{1 023 170 877 879 296 008 932 685, -30 461 961 076 376 451 292 481},
{3 296 915 062 703 377 108 068 947, 13 656 181 319 878 952 477 681},
{1 518 920 893 100 534 529 278 238, 74 378 638 085 481 884 404 069},
{8 244 558 555 805 869 234 773 654, -438 526 010 910 449 085 325 257},
{22 995 576 342 570 470 624 838 227, 1 228 815 671 522 390 180 413 746},
{92 555 332 501 349 957 195 035 061, 3 404 552 766 998 303 756 479 618},
{166 323 249 400 083 767 532 453 625, -3 254 095 273 815 061 337 178 341},
{95 834 684 540 613 145 462 215 542, 126 076 012 875 669 427 587 983},
{4 448 580 592 452 070 276 645 506, -197 905 679 537 277 371 527 535},
{24 894 434 012 207 611 099 450 568, 106 065 371 910 476 063 152 831},
{8 134 165 716 371 364 005 220 571, -90 573 120 372 101 032 413 970},

```



```

{4 580 175 801 962 703 865 659 727, 83 926 026 398 064 418 812 483},
{9 403 735 931 810 701 454 058 394, -297 354 134 809 888 210 338 687},
{29 349 848 493 804 695 793 032 170, 533 055 509 418 590 680 480 041},
{8 362 210 130 720 800 423 667 645, 39 141 729 114 868 861 585 463},
{3 713 533 663 478 756 328 437 931, -57 347 357 886 942 771 434 944},
{3 693 729 582 373 763 301 191 827, 12 500 212 147 895 571 120 955},
{1 621 920 669 821 862 794 156 826, 68 382 450 231 088 898 537 921},
{5 064 889 695 483 212 708 112 114, -113 034 458 653 105 056 431 239},
{5 696 828 247 413 400 630 227 583, 204 196 081 186 914 788 183 174},
{5 434 112 790 716 134 431 039 007, 224 318 038 598 486 240 189 528},
{13 276 204 324 698 207 286 958 105, 439 001 502 542 868 041 057 264},
{27 919 882 332 399 672 528 168 655, -1 530 096 581 432 698 076 623 438},
{99 451 836 918 721 180 173 000 773, 3 332 967 956 918 376 667 921 089},
{141 284 070 462 321 524 398 188 911, -4 154 867 609 418 403 501 045 679},
{4 884 368 171 196 810 373 221 975, 49 695 382 243 222 079 565 248},
{3 740 047 087 955 249 442 677 473, -126 934 613 083 815 442 418 464},
{15 502 090 141 970 224 098 550 471, 803 315 703 225 473 918 313 828},
{62 881 138 320 475 768 104 575 357, 3 262 180 751 288 544 505 203 834},
{236 622 164 096 270 118 999 760 393, -3 063 234 426 818 133 088 694 685},
{198 068 779 825 028 117 780 917 424, 2 459 842 903 694 763 372 630 149},
{309 944 283 427 149 150 758 781 635, 2 412 267 538 768 419 568 950 208},
{308 772 116 240 150 280 419 767 893, -12 468 831 403 992 362 534 506 357},
{775 499 910 090 259 913 980 341 416, 29 869 575 906 012 543 509 254 627},
{291 683 691 575 415 139 453 347 018, -7 965 377 396 745 609 200 569 565},
{798 276 563 397 341 454 512 171 281, -17 655 129 159 895 853 788 117 757},
{998 282 566 133 372 954 327 392 808, -20 074 004 982 464 077 184 611 003},
{1 424 850 626 325 527 989 530 380 946, -62 372 117 585 219 934 960 445 423},
{2 553 224 549 381 525 329 244 174 929, 74 879 502 632 517 404 906 263 243},
{1 925 543 947 370 526 919 412 087 421, -52 668 093 040 740 386 665 693 990},
{6 095 155 220 996 122 838 489 224 967, -262 168 068 637 517 123 043 917 911},
{17 171 175 933 639 229 230 006 722 682, -787 815 455 775 918 508 356 423 977},
{42 280 956 572 347 201 858 501 065 556, 2 060 481 651 138 698 604 783 765 839},
{260 148 580 711 718 305 434 958 487 569, 3 119 439 713 095 598 860 736 986 056},
{324 827 230 018 086 798 366 413 614 223, -3 388 733 486 518 695 483 198 829 579},
{129 181 572 867 195 589 437 268 669 943, -6 157 517 488 040 661 690 152 155 270},
{33 215 422 376 134 492 708 693 361 201, 585 715 258 526 999 642 976 897 324},
{44 801 355 654 880 065 480 313 788 221, -900 836 438 467 146 153 106 142 179},
{63 242 628 609 514 692 023 243 351 727, -179 757 401 701 346 276 498 845 717},
{8 409 895 601 468 891 044 139 592 791, -17 474 814 798 742 414 957 408 132},
{1 186 046 701 006 625 251 711 981 637, -18 547 769 172 963 763 122 820 231},
{265 768 354 583 619 683 058 957 661, 13 390 824 939 868 354 359 431 095},
{538 661 928 215 567 286 101 694 857, -17 412 209 463 568 730 674 865 056},
{293 656 635 781 664 947 429 054 177, 13 776 169 864 477 422 100 146 497},
{1 145 909 049 069 078 914 732 145 620, -41 162 041 486 907 064 808 750 629},
{1 743 193 604 415 870 677 085 333 896, 61 562 106 602 664 586 197 300 419},
{5 116 564 939 351 975 316 522 529 132, -170 500 997 700 777 484 845 529 727},
{403 707 190 435 152 814 195 615 686, -14 914 173 716 008 427 094 603 835},
{269 443 527 069 349 334 665 093 083, -641 293 312 234 374 937 932 857},
{26 388 349 829 819 372 856 096 609, 104 894 676 109 144 722 725 135},
{11 863 548 567 180 582 177 639 093, -116 193 058 480 824 258 527 206},
{3 118 286 361 901 553 468 253 303, 43 115 733 869 872 104 537 883},

```

```

{3 669 776 620 210 390 621 266 201, 9 177 111 917 666 974 572 905},
{280 922 623 232 991 676 595 137, 2 567 754 828 593 947 623 323},
{272 822 238 974 114 426 720 590, 13 492 187 351 824 178 364 609},
{783 343 379 596 916 029 671 830, 7 018 359 686 667 049 512 677},
{713 494 096 475 694 641 722 422, -36 320 755 961 159 017 922 053},
{3 398 228 982 588 743 497 001 794, 184 617 325 857 677 092 487 389},
{19 755 801 810 596 183 876 172 296, 629 635 958 514 454 362 214 011},
{62 353 906 418 449 944 302 482 165, 581 637 822 224 838 575 868 213},
{31 207 432 823 152 988 045 427 362, 1 561 301 304 664 055 924 954 795},
{4 890 030 043 698 309 314 825 494, 251 840 164 780 056 904 241 639},
{27 632 598 086 710 999 303 634 839, -798 727 078 516 583 825 966 157},
{84 909 460 940 161 301 162 512 528, 4 087 137 696 162 268 123 840 763},
{242 073 268 641 784 642 231 739 185, -7 217 626 164 934 368 323 666 469},
{874 743 514 053 760 643 278 160 143, -30 856 478 892 911 979 169 760 033},
{2 830 433 628 735 234 576 043 234 597, -626 739 458 029 721 887 957 553},
{20 576 139 801 769 397 081 340 487, 793 712 501 475 210 467 915 694},
{15 881 317 222 137 747 214 967 491, -356 936 429 435 236 564 288 315},
{46 318 067 997 669 995 592 068 953, -1 942 602 254 076 578 768 815 463},
{80 053 544 344 156 348 049 067 817, -1 073 027 660 258 937 484 164 669},
{111 388 436 094 422 338 243 260 154, -288 352 252 962 938 274 024 839},
{22 214 676 541 507 255 523 814 900, 98 696 675 367 092 166 865 043},
{2 084 165 568 729 228 524 399 175, -11 635 856 499 177 888 091 016},
{354 328 163 989 664 256 222 793, -12 738 597 897 394 653 199 726},
{618 727 787 132 526 776 187 705, 7 239 134 789 240 373 418 703},
{894 549 802 385 994 362 260 850, 29 759 593 620 853 594 648 439},
{463 404 358 981 655 498 419 840, 8 806 807 449 493 694 863 297},
{882 742 626 317 216 615 078 963, 19 888 986 474 347 468 043 985},
{2 005 959 240 279 069 560 772 849, -77 742 683 612 518 620 393 553},
{4 037 190 349 007 031 767 856 127, -31 286 094 224 638 495 507 247},
{337 743 029 539 117 871 792 432, 2 156 748 639 491 804 475 015},
{227 891 304 468 098 296 434 749, 10 735 184 164 307 756 614 696},
{644 990 935 638 112 179 372 979, -21 473 505 244 132 740 649 232},
{206 659 696 616 179 452 652 997, 3 785 756 015 760 781 420 632},
{409 460 557 924 507 201 703 669, -2 361 680 221 756 256 261 422},
{234 038 324 457 490 409 625 369, -1 765 724 092 186 936 300 538},
{211 183 688 286 867 125 046 655, -1 342 849 710 664 393 745 806},
{93 702 616 402 571 729 194 719, -1 873 733 323 230 897 405 560},
{4 194 913 390 063 895 097 097, -168 669 895 188 374 795 965},
{5 742 339 276 759 872 933 364, 37 183 454 228 723 221 955},
{4 230 966 616 098 645 853 322, -17 932 789 572 314 772 881},
{308 163 140 489 463 754 222, -6 891 625 040 258 052 711},
{515 476 402 725 086 474 299, -6 369 921 366 049 430 351},
{128 140 944 253 272 026 716, -6 134 249 618 892 457 219},
{178 392 306 532 498 194 229, 315 615 798 067 176 823},
{18 247 104 254 885 068 542, 513 392 309 696 605 223},
{61 809 969 172 685 224 818, 1 288 781 181 570 128 231},
{13 551 743 725 084 661 010, 256 362 715 620 242 657},
{9 331 293 333 296 550 293, 485 713 928 490 619 463},
{27 017 645 989 367 270 448, -359 915 699 518 359 743},
{6 303 722 203 946 197 149, -125 964 439 625 944 897},
{1 446 558 556 674 454 637, 48 695 396 856 759 657},

```

```

{3 761 780 794 452 124 199, 51 821 403 145 440 836},
{5 570 770 048 409 946 027, -115 145 791 944 682 966},
{11 512 045 222 138 042 317, 181 993 123 902 286 606},
{12 223 823 485 318 354 557, -659 275 024 620 151 738},
{79 531 721 388 170 986 295, -2 003 818 354 326 602 606},
{163 326 362 426 890 019 535, 4 732 475 092 784 293 633},
{607 599 910 807 347 754 060, 28 315 517 726 432 723 141},
{3 412 172 139 244 529 410 037, -77 961 198 259 323 311 337},
{4 765 713 635 578 123 952 033, 9 414 450 799 528 259 010},
{526 402 657 424 946 851 899, -19 908 617 704 709 417 701},
{2 308 771 037 958 023 809 999, 110 199 179 085 136 073 494},
{1 423 283 104 246 271 877 625, 51 508 882 667 192 227 953},
{4 987 955 544 434 062 830 517, 203 231 423 983 560 216 136},
{24 414 304 505 749 896 668 229, 391 567 482 190 355 428 372},
{36 062 720 416 287 208 710 395, -406 692 084 623 044 648 574},
{34 946 155 288 070 198 337 733, -934 575 257 116 447 730 130},
{96 487 013 762 309 300 928 749, -1 090 485 855 616 993 634 549},
{137 879 977 087 645 466 258 931, 2 068 635 848 368 133 842 400},
{188 998 310 044 128 810 831 547, -2 208 164 344 115 309 421 974},
{237 705 593 594 191 257 511 071, 4 107 797 737 710 323 636 716},
{143 775 575 760 976 029 054 191, -2 307 324 406 998 655 259 104},
{189 744 644 616 622 986 302 409, -76 333 783 688 418 770 489},
{5 560 249 422 738 286 043 435, -156 757 466 221 679 876 858},
{19 393 121 609 605 962 945 515, -597 517 772 602 622 887 499},
{71 681 409 102 694 033 478 861, 933 499 872 287 897 005 023},
{52 095 319 693 671 443 780 330, 1 496 619 740 405 864 842 721},
{75 315 631 000 396 163 020 015, -3 287 018 139 138 004 220 108},
{75 161 770 541 596 653 169 347, 2 554 592 063 046 037 801 900},
{283 671 987 587 789 468 446 961, 14 989 878 204 819 781 123 277},
{298 688 653 895 816 071 464 426, 9 892 129 308 975 240 229 109},
{506 215 726 784 981 387 474 028, -21 837 807 739 244 257 489 961},
{1 037 837 129 761 591 348 895 275, -21 427 700 994 215 172 718 493},
{2 447 867 776 326 184 361 201 693, 32 771 200 432 612 145 271 440},
{2 622 703 359 488 078 483 108 741, 57 037 110 385 090 509 598 370},
{263 977 893 460 344 063 481 377, -10 228 324 699 950 077 244 445},
{515 098 318 188 139 501 912 759, 20 547 465 704 991 451 763 976},
{371 270 673 161 893 654 913 417, 89 423 896 672 304 387 436},
{4 561 951 058 224 532 584 865, 123 869 898 986 371 629 697},
{5 584 858 723 330 258 762 012, 60 725 531 445 887 690 877},
{497 114 628 840 514 050 736, -19 672 744 469 610 707 643},
{1 392 852 497 364 792 590 843, 47 941 065 335 294 515 637},
{673 701 494 649 180 628 310, -20 200 838 188 114 621 569},
{1 860 418 458 087 704 648 179, 20 850 725 340 034 393 235},
{1 237 126 442 881 280 019 432, 27 213 487 842 411 114 565},
{3 292 625 862 841 104 233 841, -104 156 881 658 197 993 465},
{10 623 714 108 183 899 501 257, 450 228 278 544 623 736 282},
{47 804 083 721 299 454 581 393, -2 444 237 203 285 274 494 148},
{284 213 670 578 787 284 312 121, -15 287 765 279 248 306 693 379},
{1 644 767 738 182 732 772 727 040, 30 713 382 660 618 314 351 637},
{3 617 545 404 042 581 194 737 154, -99 762 855 162 019 362 892 891},
{6 859 728 589 199 526 345 979 514, 236 226 575 421 300 111 143 837},

```

```

{2 408 528 221 219 481 298 567 383, -17 933 512 849 782 145 894 295},
{1 430 062 328 701 195 916 477 339, 14 110 553 853 457 026 512 525},
{1 287 750 439 035 530 781 338 582, 19 197 978 923 873 983 709 319},
{390 778 848 761 128 550 136 967, 7 575 552 619 507 256 939 760},
{828 420 400 204 437 222 135 439, 17 257 856 242 332 670 935 934},
{11 388 050 559 351 526 389 641, -599 323 055 926 817 834 203},
{239 986 643 142 722 963 192, -11 876 445 697 268 743 773},
{646 382 778 902 547 073 516, 12 557 237 434 480 333 733},
{1 568 445 142 685 163 973 979, 16 571 416 296 748 495 496},
{1 535 763 648 063 034 811 083, 44 629 265 436 241 682 866},
{4 830 947 909 705 027 127 057, 18 315 188 469 937 852 076},
{1 120 865 592 302 810 924 841, 3 253 663 944 288 462 929},
{422 166 407 973 455 120 695, 17 801 583 271 274 217 997},
{1 333 828 311 264 167 254 279, 24 619 618 107 911 891 013},
{1 149 029 493 911 311 708 751, 13 307 009 168 545 902 036},
{1 216 823 524 503 767 151 265, 11 207 527 389 015 459 598},
{1 261 600 716 415 419 513 171, -26 230 515 870 037 419 821},
{666 956 073 902 944 143 669, 14 386 711 957 442 753 015},
{1 359 006 175 331 883 809 477, 37 395 445 888 752 933 170},
{3 358 542 437 572 670 638 891, -164 004 303 955 321 200 821},
{20 634 022 276 622 861 709 873, 96 321 574 652 413 165 598},
{5 576 994 164 694 843 509 963, 119 471 236 922 423 261 985},
{10 034 494 283 330 098 276 316, -439 911 135 448 877 596 471},
{21 950 461 814 444 734 381 971, -482 241 512 713 520 111 791},
{61 186 363 609 201 169 989 145, -1 359 403 634 176 319 587 632},
{3 471 618 743 165 387 520 415, 13 974 543 862 497 418 414},
{1 560 080 564 965 299 234 409, 62 799 088 825 919 013 395},
{2 602 820 444 543 814 422 558, 130 014 497 044 500 460 927},
{665 522 460 950 768 656 734, -3 413 654 819 905 875 451},
{36 880 208 820 665 783 493, -936 000 355 808 012 686},
{98 939 270 312 314 938 357, 4 753 934 172 736 252 495},
{234 950 343 883 493 741 994, -6 745 224 745 895 665 289},
{297 853 344 610 744 840 823, 464 307 180 345 443 521},
{60 980 539 980 863 610 317, -1 079 169 153 244 024 025},
{139 942 761 314 034 645 404, 6 064 371 691 292 064 199},
{121 561 864 965 415 401 501, -165 286 998 736 737 640},
{19 967 195 099 181 094 563, 563 637 801 914 939 260},
{63 086 344 457 611 981 769, 2 154 674 319 272 763 413},
{158 007 559 258 584 654 296, -8 275 917 188 926 774 325},
{201 229 891 940 672 777 823, -2 059 175 458 114 139 593},
{149 726 677 036 893 302 533, -3 259 781 984 828 779 528},
{58 726 391 755 636 163 565, 2 552 214 707 401 585 724},
{6 694 266 660 118 973 119, 253 139 425 338 526 819},
{29 624 741 146 443 541 975, 1 243 540 100 012 574 897},
{57 918 189 764 721 210 439, -1 343 811 846 947 235 024},
{35 315 730 995 397 459 041, 943 317 320 762 718 761},
{108 616 403 447 515 464 492, -3 418 532 090 115 680 213},
{204 251 963 716 997 511 212, -1 809 246 275 686 799 821},
{50 723 609 565 658 431 543, 418 471 724 837 350 058},
{23 283 616 269 176 600 075, -339 919 210 602 867 421},
{44 475 916 371 764 862 561, -1 123 359 437 750 868 389},

```

```

{120 575 279 364 976 598 737, 2 945 325 912 299 412 945},
{48 150 839 335 724 318 104, 552 873 458 626 117 337},
{13 373 138 471 304 873 455, -580 137 990 138 333 104},
{7 880 715 606 404 772 569, 363 527 814 492 763 200},
{30 743 730 170 672 689 553, -688 009 513 550 242 828},
{56 991 557 980 206 516 941, -1 296 464 709 494 047 823},
{13 909 869 470 807 452 273, 469 307 368 575 726 751},
{44 539 467 240 124 117 591, -647 937 748 762 199 188},
{44 246 442 634 985 738 203, -353 357 910 182 390 271},
{20 173 115 755 168 988 264, 492 173 765 741 730 231},
{1 580 272 383 633 167 441, 26 470 903 247 606 476},
{2 099 216 351 707 154 297, -17 671 789 918 129 658},
{980 108 568 722 326 315, 550 006 275 168 819}, {687 384 297 904 609, -34 357 701 498 921},
{60 560 464 587 707, -1 052 874 338 430}, {133 142 971 844 279, -2 036 168 712 293},
{208 297 458 396 542, -7 244 672 661 981}, {472 886 834 638 541, -23 957 453 272 208},
{1 646 966 701 877 797, -55 354 057 112 581}, {3 591 268 024 403 479, -93 710 318 497 406},
{7 962 567 355 039 413, -61 765 505 152 366}, {1 363 078 928 955 663, 11 768 138 383 526},
{532 607 489 271 839, 17 594 475 896 223}, {1 255 354 857 294 187, 59 382 908 119 056},
{2 186 525 926 824 893, -53 783 271 399 007}, {4 888 696 740 545 622, 129 497 175 005 765},
{8 467 524 244 116 824, -445 227 327 436 483}, {2 157 921 002 619 161, -25 521 467 999 633},
{2 999 193 442 956 372, 97 955 221 109 959}, {9 841 042 211 969 891, 280 991 218 921 255},
{1 669 931 577 929 058, 61 776 813 031 451}, {514 855 659 008 703, 10 751 120 738 599},
{315 109 884 784 887, -13 122 247 180 436}, {46 275 495 513 249, -1 779 091 946 176},
{5 024 592 032 999, 264 703 207 577}, {1 254 223 583 532, -52 839 360 883},
{3 661 243 424 580, 170 569 339 469}, {20 852 558 777 253, -1 126 895 243 633},
{146 872 574 016 562, 4 862 104 449 451}, {265 482 860 187 416, -9 312 649 943 219},
{1 205 588 887 640 905, 56 385 112 448 527}, {5 654 901 396 343 394, -135 777 676 436 647},
{12 561 146 680 890 140, -302 275 649 979 959}, {35 355 252 604 520 294, 1 528 737 349 209 177},
{51 099 209 622 525 649, 2 007 456 633 723 394},
{240 064 763 992 930 137, -1 459 297 406 410 798},
{189 178 021 055 953 179, 8 316 408 033 539 648}, {552 132 657 165 644 675, 4 520 406 117 981 476},
{169 138 133 010 910 589, -4 746 783 625 814 980},
{459 218 387 346 745 733, -17 502 107 271 461 235},
{1 095 026 349 942 202 849, -14 768 898 187 812 259},
{559 633 503 597 164 629, 3 423 925 168 188 724},
{403 363 410 971 888 271, 10 945 633 440 116 552},
{427 381 920 167 552 239, -4 030 048 072 326 519},
{51 764 843 747 542 175, 1 768 715 055 093 153}, {124 164 180 408 114 094, -325 590 253 468 429},
{30 059 279 037 015 635, 547 316 166 357 503}, {11 337 959 626 168 890, -171 926 074 178 239},
{2 409 413 903 454 492, 51 498 406 098 737}, {2 895 941 177 956 661, -132 459 683 240 785},
{4 779 197 428 580 167, 55 969 398 400 829}, {5 733 022 466 051 626, 180 309 251 446 793},
{9 697 751 604 632 250, -370 644 736 929 559}, {16 039 960 893 957 308, -202 996 892 846 997},
{843 272 428 715 335, -15 130 163 264 141}, {1 056 395 802 135 543, 18 752 858 979 937},
{1 639 988 905 135 673, 49 449 391 870 838}, {2 145 810 003 678 997, -8 372 507 809 911},
{643 825 141 888 403, -1 213 650 745 474}, {155 234 905 029 129, 6 035 833 678 171},
{446 250 668 672 371, -12 821 137 480 797}, {654 644 649 902 812, -20 742 963 529 601},
{2 401 238 140 682 460, -104 882 065 766 717}, {2 905 984 823 384 153, 26 849 648 281 257},
{1 636 598 769 208 411, 23 460 509 473 584}, {1 482 503 106 869 347, 41 743 133 048 246},
{5 325 666 594 154 867, 179 131 268 308 761}, {12 695 392 693 394 269, 484 131 171 247 375},
{28 399 329 373 142 497, -1 064 386 466 375 466}, {89 184 672 595 707 355, 4 580 202 832 738 538},
{568 295 337 476 559 979, 13 982 200 715 237 211},

```

```

{1 308 396 556 067 571 736, -70 522 198 187 274 293},
{8 291 130 096 038 275 553, 262 716 618 682 037 079},
{30 455 847 569 957 586 425, 1 428 765 674 853 031 998},
{118 815 088 685 549 504 821, -4 171 850 268 584 651 273},
{526 862 946 442 147 793 551, 6 611 301 376 014 031 728},
{536 826 037 050 357 853 207, -22 153 641 513 930 061 015},
{1 351 462 508 317 570 266 761, -14 605 068 326 450 260 988},
{1 790 726 509 125 953 347 349, 89 458 800 546 911 817 071},
{407 781 023 369 572 559 327, 11 258 530 733 978 964 530},
{650 640 156 884 746 932 961, 19 506 333 850 292 373 707},
{1 822 889 774 000 931 965 690, -95 913 625 497 450 590 079},
{139 623 951 484 508 351 707, -6 968 131 619 939 704 899},
{68 726 919 542 848 730 201, 1 318 727 498 490 267 649},
{40 262 570 416 315 675 139, 536 608 598 354 623 001},
{4 451 416 946 083 866 832, -234 046 365 405 085 265},
{1 192 968 890 845 907 611, 8 443 870 176 104 189},
{626 780 552 002 061 006, 9 131 954 194 060 971}, {874 287 583 082 396 159, 8 404 403 367 809 552},
{60 393 434 343 323 513, -546 803 458 174 452}, {64 449 187 307 187 559, -1 678 021 902 280 936},
{179 985 370 394 653 633, -4 701 257 213 235 910},
{351 787 824 714 220 939, 4 858 711 606 396 854},
{515 634 921 109 279 613, 26 985 336 255 298 864},
{766 258 984 012 114 811, -221 146 808 914 660},
{3 868 434 698 889 407, 149 799 138 396 564}, {6 928 182 547 790 591, 327 918 928 959 224},
{11 015 765 427 131 281, 1 381 683 335 579}, {104 097 356 742 618, 3 926 587 142 531},
{505 090 475 804 097, 25 500 935 765 516}, {1 296 126 990 136 649, 10 444 340 651 241},
{270 561 087 667 195, 2 158 238 059 363}, {205 489 854 913 660, 1 152 180 667 969},
{105 646 051 991 814, 144 720 231 635}, {74 402 243 432, 2 834 565 821},
{185 028 938 618, -9 399 117 355}, {776 746 430 766, -11 848 668 997},
{1 384 885 158 468, 62 080 585 331}, {5 026 529 951 918, 253 765 464 627},
{12 828 966 583 586, -254 075 929 115}, {32 919 743 620 868, -1 483 162 626 853},
{76 313 613 316 826, -2 990 553 506 271}, {378 924 573 555 860, -7 353 021 117 947},
{902 753 963 851 992, 42 523 511 881 477}, {2 566 936 371 676 425, -138 165 010 702 549},
{15 306 292 729 737 578, -793 456 791 969 441}, {60 651 398 449 686 337, -1 357 435 883 902 082},
{113 935 893 713 633 839, 5 233 980 829 476 930},
{318 673 032 667 817 323, -6 121 749 227 332 239},
{89 965 158 640 255 385, -2 961 813 739 254 147},
{292 126 319 671 946 425, -5 877 475 432 682 061},
{459 579 866 047 192 375, -25 183 275 183 423 832},
{1 651 880 052 083 173 937, -65 928 466 872 279 260},
{964 784 012 638 610 931, 1 246 778 152 204 319}, {58 458 895 060 909 425, 845 276 750 055 128},
{35 452 217 768 770 959, -515 469 381 046 565}, {30 289 584 665 252 838, -1 368 116 157 322 319},
{50 240 680 694 558 660, 275 500 469 260 803}, {26 193 561 031 331 182, 250 038 823 518 539},
{15 915 560 224 353 619, -827 145 487 537 608}, {52 546 337 779 574 621, 2 635 885 952 860 930},
{45 073 276 020 366 477, -2 400 075 419 545 241},
{138 905 278 111 185 826, 3 241 220 609 600 105}, {122 875 730 725 715 207, 1 148 181 332 517 188},
{5 346 302 496 911 933, 139 373 059 821 276}, {13 183 196 834 006 035, 313 602 547 997 963},
{3 127 022 158 087 907, 69 140 930 660 910}, {4 123 913 205 249 691, -5 058 118 650 790},
{406 730 777 086 183, 15 174 019 423 900}, {780 517 555 447 771, -31 792 131 423 622},
{3 757 147 027 550 877, 75 607 081 600 766}, {6 103 454 804 192 249, 305 473 203 056 552},
{1 580 434 574 902 033, -1 696 389 176 297}, {157 836 137 980 773, -6 353 251 339 223},
{261 723 266 447 926, -2 929 628 451 315}, {259 405 915 874 333, 1 807 459 241 808},

```

```

{228 340 530 802 997, 3 024 654 660 965}, {392 246 413 653 586, 16 957 073 449 111},
{587 469 497 220 679, -9 972 055 273 840}, {231 903 915 136 703, -11 178 339 456 627},
{747 239 137 998 032, -26 323 567 279 515}, {2 677 143 847 133 956, -133 535 662 047 241},
{1 691 249 427 742 768, -60 214 175 254 911}, {1 381 412 919 183 380, 5 274 053 422 567},
{102 327 390 172 762, 763 496 428 537}, {4 962 480 935 452, -20 532 815 741},
{1 699 104 627 810, -33 127 984 787}, {2 518 857 165 999, -102 574 096 954},
{11 965 252 814 813, 589 737 945 322}, {44 839 897 902 099, 1 827 055 992 359},
{220 000 001 508 388, 4 655 379 997 663}, {314 848 245 593 701, 9 266 196 884 964},
{53 243 954 204 725, -542 142 517 907}, {29 978 699 307 657, -441 132 260 308},
{4 811 425 434 481, -169 907 304 733}, {14 207 497 214 691, 745 957 401 058},
{9 022 634 376 907, 193 221 591 297}, {15 459 248 895 676, 321 681 714 129},
{4 872 500 398 292, 250 601 411 275}, {29 212 352 609 621, 1 485 492 406 465},
{130 841 321 675 577, -1 145 510 991 638}, {66 557 049 386 235, -370 791 104 089},
{48 746 878 993 455, 765 699 787 637}, {67 829 650 227 319, 562 462 041 548},
{60 031 538 397 107, -2 299 678 534 142}, {63 092 781 976 145, 443 438 774 699},
{32 737 179 817 281, 1 110 698 618 701}, {138 579 927 112 376, 1 780 885 619 811},
{86 566 774 247 966, -649 016 084 971}, {65 127 991 014 449, 1 662 692 641 435},
{74 423 213 601 292, 2 350 981 027 497}, {212 551 150 274 956, -8 940 834 158 263},
{533 592 684 642 628, -2 049 263 469 791}, {206 239 996 702 584, 6 834 725 334 695},
{315 136 242 036 042, -9 408 122 870 087}, {1 227 733 265 993 973, -37 542 532 137 619},
{2 937 787 465 980 402, 155 529 695 908 817}, {4 543 786 903 512 823, 179 816 426 754 867},
{12 722 949 710 621 924, -407 247 119 641 907}, {25 850 007 453 098 241, 1 208 487 432 711 773},
{124 075 869 297 715 104, 3 160 693 580 473 963},
{212 719 570 377 633 861, 10 310 457 545 647 064},
{999 410 015 291 029 029, 43 377 274 186 822 343},
{455 702 465 452 281 820, 1 799 802 874 309 589}, {92 664 960 264 376 189, 3 328 927 834 380 705},
{143 340 022 848 573 913, -6 202 558 679 861 570},
{179 148 554 692 302 189, 8 310 987 897 438 911},
{971 306 090 506 063 339, -43 745 967 241 198 853},
{2 339 335 345 518 094 699, 102 539 231 158 289 426},
{5 014 613 405 233 832 037, 126 348 170 530 623 641},
{10 339 428 405 662 877 589, -166 986 001 027 477 460},
{3 604 062 064 710 656 853, -194 756 962 866 980 909},
{25 332 220 427 400 849 934, 941 921 298 262 200 871},
{26 209 166 553 464 852 329, 813 334 999 403 686 929},
{47 983 448 579 826 968 063, 2 269 080 688 799 765 167},
{87 514 332 253 389 583 228, -1 523 677 673 017 162 767},
{174 817 386 441 173 348 867, 4 078 050 865 971 247 260},
{141 704 609 240 244 511 319, 5 613 014 225 718 879 933},
{362 743 696 082 670 917 422, -3 716 368 509 341 020 183},
{384 089 890 013 002 914 656, 3 306 223 513 064 946 625},
{149 374 136 834 374 919 028, -3 421 574 673 935 199 397},
{309 064 139 337 523 717 720, 13 811 929 889 471 193 651},
{1 368 042 305 288 411 295 674, 12 167 049 597 333 581 205},
{1 402 513 351 794 202 787 782, -47 710 941 614 840 377 911},
{4 969 659 825 487 770 859 469, 55 684 346 172 810 127 528},
{3 617 043 236 317 080 992 451, -112 003 240 080 320 128 957},
{8 663 102 635 418 095 712 501, 155 806 677 282 148 462 782},
{16 324 749 896 523 387 465 533, 424 395 893 734 495 883 431},
{51 996 660 803 099 044 425 765, 2 680 150 080 660 731 111 948},
{282 411 838 153 375 317 572 039, -11 351 312 239 844 967 825 927},

```

```

{360 564 542 642 954 934 023 768, 3 540 061 100 416 722 623 001},
{137 204 364 681 853 436 373 842, 6 961 830 582 692 743 307 269},
{534 480 953 636 376 029 914 494, -3 971 415 418 906 125 199 085},
{436 613 641 895 079 326 001 003, -14 679 355 204 345 384 384 523},
{990 724 743 879 220 055 622 681, 37 150 969 931 397 475 422 244},
{3 248 429 842 618 598 344 589 541, -99 524 229 712 811 686 948 991},
{9 433 741 068 801 266 403 243 606, 169 312 433 933 663 240 392 183},
{12 559 625 880 259 140 443 002 846, -212 315 307 517 377 732 244 353},
{8 684 979 761 003 665 274 122 997, -294 682 690 727 510 914 580 881},
{36 604 794 965 238 221 585 968 824, -812 414 483 212 708 580 897 855},
{12 135 667 035 246 222 183 686 787, 439 534 806 854 110 647 083 495},
{45 053 887 403 914 370 813 232 199, -1 335 513 904 490 851 770 693 494},
{92 992 946 727 717 009 661 155 011, 2 605 002 989 348 876 810 644 280},
{207 023 313 765 592 102 296 275 147, -285 812 905 731 297 025 455 610},
{24 924 514 242 993 692 866 752 341, -963 871 575 148 374 293 049 449},
{35 806 584 957 242 191 916 266 579, 809 928 900 366 514 370 139 039},
{44 634 608 713 392 182 729 150 969, 1 378 764 425 290 420 550 935 096},
{135 220 688 377 964 701 096 936 911, 4 768 659 398 667 935 833 313 936},
{446 633 231 614 036 911 970 582 889, 22 944 140 784 356 245 155 205 493},
{2 812 668 415 063 550 807 701 451 286, 141 608 278 376 884 509 874 179 037},
{5 127 751 100 698 659 512 700 046 402, 74 572 622 382 165 946 086 688 225},
{4 670 838 885 417 971 795 019 015 349, -41 251 961 298 218 276 650 885 629},
{2 463 589 043 177 618 302 331 028 536, 16 754 292 964 172 064 786 635 093},
{186 198 067 857 416 796 961 174 495, -7 860 315 787 742 128 616 578 816},
{644 221 405 727 698 227 056 594 407, 7 224 260 476 582 073 481 156 759},
{331 964 731 028 039 742 448 071 128, -3 452 248 994 595 022 789 199 231},
{144 341 644 839 316 882 140 522 376, -729 550 523 773 099 345 392 097},
{28 761 382 220 035 308 990 674 290, -1 584 049 309 433 281 304 474 759},
{65 354 093 012 132 569 163 829 164, 1 363 033 316 411 964 959 490 679},
{18 806 124 193 779 958 523 261 564, 268 720 978 307 405 430 389 699},
{1 142 547 675 204 881 856 567 258, 3 599 921 533 447 566 036 617},
{360 980 413 826 900 238 392 947, -8 514 811 697 672 512 299 353},
{883 238 823 984 191 838 691 823, 605 647 456 828 719 290 868},
{53 870 797 042 726 615 451 377, -1 098 118 414 711 997 218 173},
{16 567 611 843 591 713 116 700, -163 327 604 094 699 935 699},
{18 810 767 297 106 157 719 563, 602 852 609 548 860 071 672},
{32 174 473 487 063 315 903 253, -1 098 767 113 051 425 689 219},
{81 589 755 854 428 350 882 226, -1 084 901 177 735 946 307 541},
{58 430 058 873 115 365 779 213, -1 843 248 824 039 784 836 607},
{145 676 619 489 487 984 951 493, 2 878 399 065 221 788 804 071},
{295 015 736 084 513 186 761 664, -8 823 151 992 226 670 033 297},
{1 013 002 449 691 698 899 332 969, 25 208 713 733 528 859 926 456},
{1 223 975 792 193 204 098 253 727, 16 699 313 794 352 428 268 019},
{1 295 507 809 040 407 523 033 420, -36 451 271 808 985 750 328 663},
{4 402 087 709 849 905 553 991 824, -121 341 642 422 851 166 661 471},
{8 886 397 230 970 314 749 042 284, 422 821 617 081 364 517 209 803},
{1 878 680 604 816 550 448 378 723, -40 093 638 430 562 135 806 044},
{1 504 465 573 425 792 774 905 735, -72 438 128 040 756 724 930 748},
{4 401 335 358 115 891 992 312 899, 123 812 123 277 673 244 977 261},
{14 701 984 008 530 689 466 414 711, -139 962 091 428 063 845 291 383},
{1 568 639 457 588 241 945 527 448, 32 121 777 698 944 420 393 063},

```



```

{1 401 171 860 589 113 931 684 057, 49 573 672 932 890 140 183 636},
{3 447 671 857 133 971 720 611 487, 112 383 771 714 760 417 638 754},
{9 527 192 364 207 122 487 940 281, -142 178 349 817 794 172 804 058},
{326 889 647 122 095 347 987 885, -14 379 926 403 922 960 624 419},
{1 012 197 624 218 912 296 296 776, -12 858 281 547 149 280 297 275},
{948 540 535 546 662 810 430 587, 34 786 537 442 834 527 766 653},
{2 446 958 467 204 337 472 241 428, -24 908 898 403 252 078 092 877},
{1 548 129 429 321 694 433 683 766, -64 201 378 486 827 846 717 487},
{1 918 938 902 748 267 578 052 514, 42 559 337 720 857 229 961 879},
{991 169 496 449 056 428 973 217, 45 275 514 515 835 826 351 455},
{1 286 549 422 524 250 449 562 559, 9 020 265 107 322 517 987 083},
{880 652 297 414 710 741 251 530, -41 782 198 508 564 907 747 069},
{848 471 857 264 939 462 090 303, -42 463 410 414 397 372 945 314},
{209 440 319 051 103 162 601 951, -9 706 019 953 734 224 435 590},
{1 076 227 541 866 090 820 010 627, -58 089 268 177 655 411 336 332},
{7 224 229 572 962 204 784 856 103, 142 304 547 064 913 727 251 085},
{8 758 512 092 627 965 201 648 016, 238 836 352 962 779 630 546 037},
{20 627 870 319 653 736 810 057 839, 873 608 370 632 433 553 338 905},
{89 086 141 362 987 807 629 956 703, -3 825 707 601 376 154 987 519 388},
{287 949 897 741 431 887 173 834 877, 9 875 041 918 104 665 268 403 868},
{413 878 396 612 304 324 602 271 415, -4 160 513 942 043 561 282 614 081},
{522 716 800 047 832 254 974 555 148, 906 342 088 001 833 208 541 893},
{63 799 783 786 308 171 132 800 719, 820 573 871 867 131 312 955 559},
{53 909 271 683 282 746 043 748 229, -1 813 667 322 549 121 354 182 165},
{131 696 722 209 205 274 991 497 623, -2 221 323 653 267 198 552 992 602},
{167 958 813 273 867 375 977 669 615, 8 437 425 647 566 799 221 795 114},
{207 691 015 174 244 024 515 190 895, 2 382 247 409 127 397 676 371 663},
{114 534 022 582 192 214 435 184 282, -4 930 272 632 113 083 855 762 931},
{299 228 787 464 508 152 943 496 547, -9 864 140 943 996 867 833 352 014},
{869 099 055 030 357 018 992 201 401, -6 799 258 047 717 890 852 592 241},
{317 171 445 391 181 666 716 232 561, 4 567 726 878 483 297 755 303 270},
{525 550 474 044 373 980 880 722 853, -15 646 913 441 872 744 942 160 969},
{1 694 925 323 555 728 301 173 274 459, 3 494 294 419 548 436 333 775 513},
{50 635 409 655 746 653 835 622 002, -2 256 975 273 771 657 157 919 471},
{258 253 805 418 561 643 046 527 320, 4 425 265 355 103 751 555 905 887},
{417 753 098 329 085 887 448 284 862, 12 244 042 047 848 376 313 489 631},
{382 840 868 689 407 403 674 638 304, 11 889 238 844 754 462 086 925 721},
{627 314 347 860 594 242 863 006 016, 14 150 333 440 098 483 476 586 863},
{1 236 014 918 516 635 081 907 403 572, 41 690 998 173 561 727 979 238 517},
{3 870 052 019 527 007 214 544 759 694, 130 397 604 776 700 673 653 231 281},
{11 013 420 552 565 417 698 723 007 568, -291 157 551 773 725 188 430 693 271},
{13 298 967 101 904 678 412 197 559 990, 320 282 543 591 416 399 120 541 433},
{40 212 628 709 855 122 277 542 391 548, 13 441 678 537 990 358 011 891 117},
{1 281 724 138 563 599 131 423 425 708, -1 891 491 770 515 981 150 239 671},
{186 015 125 560 091 259 475 733 490, 5 194 170 665 385 488 919 457 393},
{256 429 837 565 807 847 304 689 054, -8 841 280 845 796 044 189 434 423},
{8 598 268 921 034 808 316 876 981, 427 762 025 804 481 744 061 570},
{11 316 470 500 580 613 574 787 803, 197 275 879 676 031 653 226 500},
{18 869 029 429 310 856 650 730 689, -131 828 954 140 447 337 475 175},
{4 599 603 640 671 384 038 314 632, -182 732 127 515 713 164 501 617},
{8 232 019 080 759 945 478 616 441, 50 246 384 006 358 651 030 888},

```

```

{2 206 016 722 395 675 388 137 233, -79 353 414 692 752 377 690 438},
{4 176 147 807 365 882 232 293 153, 147 997 917 378 376 043 069 739},
{8 470 209 762 865 845 927 541 243, -303 602 828 995 086 755 340 141},
{8 066 065 086 101 387 381 451 415, -199 717 855 374 392 720 402 967},
{20 343 279 106 053 462 682 509 305, -932 764 922 637 682 389 046 076},
{46 695 437 489 569 617 520 648 521, -1 831 300 576 254 959 774 960 876},
{240 098 770 880 448 887 562 801 323, -5 086 202 126 939 138 275 614 226},
{275 432 250 463 369 204 149 300 363, -1 353 472 726 213 501 488 414 962},
{177 836 834 940 681 165 173 545 755, 2 994 399 849 528 959 055 451 036},
{306 985 124 258 288 777 208 807 953, 8 975 533 504 904 769 993 223 591},
{477 867 079 071 495 126 511 140 917, -10 600 232 652 255 149 945 841 562},
{225 288 356 363 518 663 395 174 901, -5 592 816 939 649 611 773 334 310},
{414 403 518 491 492 617 454 057 763, -8 680 949 576 117 291 834 202 602},
{600 182 085 642 133 724 556 455 979, 32 977 432 651 380 632 955 491 188},
{1 732 722 352 245 253 147 052 638 485, 75 336 005 259 664 045 607 135 969},
{1 517 175 206 234 202 721 554 926, -13 029 831 240 266 565 078 617},
{1 502 987 761 542 948 350 498 102, 53 456 843 048 127 397 454 315},
{1 629 589 079 385 261 327 425 166, 43 444 407 705 181 870 272 961},
{5 601 482 727 263 882 395 153 576, -308 107 425 581 666 063 270 999},
{14 609 404 566 793 926 400 481 222, -486 106 076 832 953 040 661 437},
{6 896 454 854 803 152 507 823 456, -91 038 691 473 649 625 076 267},
{5 913 738 362 079 596 466 855 868, -183 977 231 827 133 429 794 807},
{6 960 806 169 778 925 629 997 572, -30 905 992 642 186 613 959 853},
{1 829 908 050 464 559 615 060 161, -57 198 732 047 592 195 890 819},
{118 711 640 356 741 856 310 361, 2 998 207 881 784 043 553 310},
{319 985 502 545 029 971 196 257, -12 290 077 381 716 300 059 648},
{116 638 033 166 822 616 742 567, -4 122 125 454 878 066 755 313},
{320 470 873 152 264 617 170 189, 11 330 872 149 904 530 181 578},
{843 297 127 148 634 058 619 315, 4 431 033 242 638 941 942 374},
{368 413 305 422 828 556 451 065, -12 720 347 910 668 596 058 093},
{125 394 188 465 471 788 445 216, -618 517 177 356 998 350 917},
{43 342 015 493 704 596 015 905, 178 659 177 998 050 429 261},
{18 979 331 833 096 131 458 234, -946 247 047 269 270 993 159},
{14 304 803 467 917 149 499 202, 356 074 058 662 257 336 611},
{16 264 214 935 263 137 142 406, 391 066 316 474 779 107 597},
{42 230 003 806 204 954 063 684, -406 553 672 567 434 983 827},
{13 565 051 032 578 758 887 212, 724 223 960 978 121 093 385},
{51 338 711 439 457 516 308 089, 2 000 465 104 218 453 123 303},
{177 099 274 068 455 668 118 507, 1 135 212 174 580 243 540 098},
{1 623 981 325 608 752 026 597, 50 804 865 539 795 449 657},
{466 659 747 816 721 318 301, 17 082 714 889 609 439 789},
{1 427 155 244 681 074 771 474, -70 886 899 533 796 737 811},
{2 476 737 803 351 824 011 802, -72 429 679 252 431 963 405},
{3 715 850 406 283 098 336 416, -201 308 145 360 506 828 827},
{24 275 896 715 815 534 810 390, 592 155 850 692 446 185 899},
{655 701 757 161 567 416 347, 904 662 770 570 331 117},
{47 011 645 005 655 234 714, 528 194 904 809 315 881},
{604 499 615 669 903 215, 4 466 152 582 887 723},
{412 651 465 755 940 430, -8 440 673 666 228 791},
{247 626 042 878 096 527, 8 210 578 322 169 212},
{344 186 315 024 303 921, -3 887 782 391 833 295},

```

```

{480 321 594 250 004 842, 16 185 634 330 663 551},
{1 380 075 581 184 143 944, 4 095 934 995 656 743}, {66 936 748 622 931 561, 374 395 265 821 189},
{21 041 041 233 114 010, -1 021 132 774 345 847}, {105 922 468 403 128 351, -74 348 122 276 498},
{6 208 336 151 781 637, -298 956 022 453 485}, {18 341 704 092 027 124, -250 867 722 424 233},
{7 458 773 380 284 245, -182 187 262 746 479}, {2 867 855 180 526 622, -151 311 250 380 775},
{1 856 405 674 231 089, 83 306 290 356 347}, {6 224 496 320 952 665, -53 687 407 550 979},
{852 897 154 716 437, 12 934 105 996 827}, {198 260 202 500 135, 8 707 142 266 479},
{527 070 312 395 966, -23 375 665 818 435}, {2 779 910 375 574 257, 17 199 281 985 785},
{1 676 179 510 326 119, -87 590 100 714 007}, {3 147 477 947 876 318, -130 216 289 170 637},
{5 861 483 046 410 890, 8 246 907 565 579}, {543 945 204 249 877, -9 701 734 474 001},
{170 443 384 630 923, 4 446 529 095 761}, {387 998 374 897 315, 14 293 701 445 228},
{543 998 635 429 817, -19 788 865 647 529}, {2 550 906 154 938 442, 139 822 218 240 107},
{8 969 937 600 143 708, 177 262 237 626 473}, {18 524 804 446 087 145, 361 189 548 116 406},
{27 388 160 435 565 457, 1 373 245 711 370 117}, {20 186 247 253 100 229, -574 308 040 664 437},
{22 477 513 249 217 642, 146 038 300 941 315}, {3 257 280 180 900 284, 22 878 948 759 559},
{2 227 467 202 284 278, 122 421 421 901 441}, {6 280 862 919 343 420, 338 768 810 253 423},
{40 960 797 049 035 271, 1 235 598 676 887 611}, {48 928 707 188 700 404, 1 251 613 586 693 773},
{30 449 431 910 176 591, 135 264 978 325 905}, {3 895 499 941 015 058, -77 281 643 341 147},
{8 262 874 550 877 204, -280 532 413 703 957}, {33 515 287 560 624 613, 132 016 204 080 889},
{4 425 836 567 273 759, -70 841 551 537 420}, {8 852 677 823 828 097, -84 463 107 842 291},
{4 194 455 398 076 454, 13 485 901 980 997}, {89 388 962 419 781, -1 575 716 878 069},
{112 274 602 729 976, 5 870 592 876 683}, {192 867 913 198 737, -8 510 773 971 254},
{757 410 580 847 615, -16 618 859 262 413}, {1 855 976 593 749 729, 73 080 344 974 372},
{7 618 575 949 682 827, -101 504 855 156 307}, {1 502 206 808 427 926, -27 322 196 793 203},
{135 185 997 136 857, 833 315 627 647}, {49 671 615 465 309, 78 078 741 281},
{3 559 970 785 959, 122 404 982 659}, {2 689 513 967 024, -132 788 609 211},
{8 874 088 877 452, 303 017 024 883}, {22 774 525 987 235, -666 827 079 931},
{26 932 585 899 803, -160 105 768 762}, {9 156 804 667 981, 298 981 620 160},
{29 357 521 485 477, -940 778 444 696}, {50 861 491 073 963, -659 473 881 372},
{21 566 580 787 897, 157 044 210 487}, {13 550 799 159 814, -534 820 998 455},
{47 412 114 189 457, 496 774 784 072}, {57 468 051 788 271, -2 420 640 682 817},
{164 986 369 625 631, -105 968 746 184}, {1 832 632 091 391, -16 887 547 322},
{2 133 079 043 941, -27 497 309 871}, {3 080 026 137 211, 99 716 763 900},
{2 943 901 990 207, 68 125 219 761}, {3 818 113 147 292, -186 440 186 405},
{23 488 377 247 496, 175 720 950 277}, {15 314 513 570 586, -620 449 748 825},
{51 740 029 460 257, -2 271 772 241 824}, {134 322 542 745 785, 5 026 861 633 512},
{368 915 717 427 257, -20 339 188 425 464}, {739 115 677 222 015, 29 756 965 787 138},
{1 264 626 941 042 405, -17 130 852 766 854}, {803 771 054 360 033, -14 651 841 703 287},
{547 102 941 357 776, -7 489 811 351 231}, {91 185 444 811 119, 894 703 243 739},
{19 537 231 218 117, -488 748 234 658}, {3 339 618 237 389, 22 625 332 491},
{2 348 845 446 377, 6 495 397 960}, {654 505 782 609, 23 786 476 048},
{3 028 588 791 305, 89 223 050 361}, {1 313 664 214 847, 476 467 419},
{11 451 194 632, 305 684 853}, {37 044 883 673, -1 300 824 841},
{163 530 276 875, 488 323 692}, {15 296 065 535, -244 612 216}, {30 114 571 199, 1 241 268 585},
{85 244 916 817, -2 533 398 530}, {234 236 532 389, -5 253 621 672},
{572 404 469 813, -6 868 039 202}, {619 947 820 361, -28 953 410 688},
{3 136 589 525 119, -5 834 018 450}, {555 561 458 003, 2 856 141 125},
{364 534 140 836, 12 554 700 097}, {117 781 400 049, 3 111 248 093},
{117 305 228 555, -3 366 033 364}, {133 062 005 655, 4 932 592 832},
{31 034 212 767, -325 023 097}, {41 295 879 176, 1 036 147 641}, {39 456 960 032, 1 591 520 145},
{87 064 464 959, 3 841 826 533}, {341 254 413 900, 5 577 591 721},

```

```

{268 606 875 697, -14 005 809 927}, {656 576 103 092, 8 776 386 435},
{434 707 317 179, -7 381 322 469}, {207 956 333 396, -7 808 623 433},
{756 519 314 585, -31 794 025 996}, {1 719 312 350 897, 20 222 145 904},
{113 076 601 991, -5 634 800 079}, {100 097 908 093, -2 939 223 631},
{43 212 120 057, -1 112 620 931}, {47 365 314 276, 142 991 605}, {9 229 464 523, -48 019 418},
{2 560 638 221, 76 721 501}, {7 581 944 944, 112 987 915}, {3 091 470 057, 58 867 448},
{7 496 732 681, 223 943 713}, {28 033 209 976, 166 022 767}, {6 479 701 161, -79 990 178},
{130 643 409, -5 318 194}, {607 908 983, -8 982 547}, {763 808 019, 4 188 905},
{375 382 267, -15 900 932}, {1 641 146 563, 19 797 749}, {543 516 852, 7 233 905},
{256 155 951, 10 079 704}, {1 094 961 313, -5 255 786}, {462 307 975, -5 894 743},
{662 239 523, -16 842 620}, {1 414 241 209, -63 206 544}, {6 232 374 383, -130 041 336},
{2 527 362 935, -77 089 047}, {4 359 387 008, 85 319 073}, {2 134 056 955, 84 061 024},
{8 555 746 365, 409 635 527}, {12 255 721 626, 377 165 039}, {49 033 819 414, 1 872 527 941},
{91 548 445 324, -2 165 230 625}, {160 103 636 462, -4 527 233 703},
{434 070 153 391, 5 918 757 436}, {526 226 328 069, -10 040 615 161},
{1 082 071 340 311, -15 733 060 657}, {923 089 240 786, -35 410 778 367},
{633 567 853 172, -21 509 198 413}, {2 577 689 088 285, 27 718 350 481},
{30 904 195 824, -883 700 615}, {6 660 659 363, 328 537 781}, {23 644 684 409, 367 554 352},
{31 877 146 703, -1 752 380 796}, {87 918 894 625, 4 458 836 652},
{330 811 503 145, -5 399 990 356}, {371 380 045 827, 13 075 336 807},
{1 386 171 805 753, 76 161 062 863}, {4 016 713 319 597, 99 519 677 174},
{9 448 599 183 531, 127 156 434 937}, {10 263 048 524 759, -507 866 039 479},
{27 806 394 352 077, 1 339 821 705 427}, {86 753 564 477 070, 1 568 240 080 669},
{131 594 690 592 325, 6 154 788 512 647}, {616 506 670 432 094, -12 806 372 583 487},
{473 606 829 700 834, -25 816 385 180 473}, {2 343 828 766 960 160, -70 139 377 415 119},
{7 687 309 124 704 279, 201 644 962 490 357}, {6 522 544 668 597 519, -189 355 316 786 207},
{22 214 005 138 884 503, -811 387 552 213 461}, {80 620 343 258 837 728, -42 230 763 885 267},
{477 345 489 975 575, -694 501 975 246}, {58 552 474 153 699, -1 876 038 452 422},
{103 959 199 826 271, -481 298 601 587}, {341 404 645 023, 17 767 652 923},
{1 004 459 984 818, 21 059 024 801}, {1 676 153 080 690, 6 165 375 437},
{218 037 039 762, -10 672 567 849}, {1 206 034 571 666, -14 204 530 049},
{355 176 897 237, 15 212 118 142}, {1 393 421 332 373, 5 959 373 212},
{281 935 798 805, -12 916 264 006}, {584 388 453 001, -18 250 902 021},
{94 571 730 527, -3 078 922 663}, {230 091 342 838, -2 124 579 759},
{167 459 691 758, -4 810 363 197}, {237 494 296 031, 8 121 490 107},
{518 394 810 064, 20 979 916 397}, {1 605 115 263 443, -31 031 237 372},
{2 237 888 013 963, 18 025 963 579}, {701 823 433 921, 20 198 555 854},
{1 348 143 514 847, 39 345 702 034}, {2 732 476 816 733, 103 728 983 616},
{9 342 612 834 571, 496 197 682 390}, {22 392 643 410 657, 365 001 630 973},
{33 544 051 302 952, -172 687 717 317}, {11 212 779 728 402, 329 566 271 771},
{1 979 466 393 444, 23 470 967 329}, {2 079 051 243 504, -16 858 496 137},
{1 434 985 505 739, -3 334 937 795}, {253 072 772 807, -12 022 393 874},
{158 457 882 139, 640 537 935}, {64 438 207 022, -2 067 010 119}, {94 914 946 579, 603 484 867},
{44 137 306 980, -1 889 574 199}, {178 077 405 989, -6 060 222 162},
{613 043 345 533, 28 512 021 930}, {3 740 159 011 801, -75 228 291 696},
{5 590 215 698 737, 59 868 972 976}, {5 891 518 747 847, 154 296 362 264},
{7 431 586 217 345, -392 680 356 318}, {7 716 565 359 311, 318 934 297 861},
{16 343 401 400 161, -820 112 774 418}, {15 478 625 196 337, 636 821 392 788},
{51 261 795 358 775, -2 089 213 096 506}, {254 723 930 169 125, -12 285 546 866 422},
{860 681 708 768 831, 4 360 556 492 304}, {434 496 983 440 009, -3 021 172 844 376},
{145 151 317 485 505, -5 695 459 624 862}, {727 149 465 220 165, 25 513 720 700 499},

```

```

{3 352 838 429 802 478, -55 425 425 003 505}, {7 183 300 482 742 814, -319 537 528 804 899},
{40 363 885 296 214 468, 526 271 742 616 399}, {41 827 226 820 291 065, -45 638 142 131 087},
{5 967 109 220 643 099, -159 367 452 051 175}, {18 545 049 119 151 112, -1 015 812 934 677 105},
{68 489 485 575 327 386, -2 836 262 432 408 285},
{110 246 232 950 007 598, -4 394 867 295 381 081},
{98 506 798 721 390 699, -4 481 660 397 942 901}, {23 598 998 771 871 349, -106 763 500 993 888},
{1 121 708 734 412 563, -1 961 983 301 661}, {143 522 818 170 127, -6 246 821 278 410},
{40 520 734 358 689, -1 334 205 587 786}, {130 071 048 703 667, -6 677 628 911 854},
{840 574 136 529 983, 4 834 353 703 389}, {158 696 267 101 889, 5 979 414 999 944},
{722 707 666 805 537, 21 217 835 042 148}, {342 235 422 968 815, -4 783 282 706 536},
{568 325 090 167 351, 4 662 848 788 308}, {142 667 507 637 175, 719 826 755 946},
{37 296 019 445 021, 139 950 351 220}, {18 206 443 391 763, 670 959 669 338},
{23 810 000 064 531, 558 095 981 203}, {49 477 434 453 074, 524 297 539 645},
{50 881 486 054 772, -2 372 398 745 265}, {279 072 562 306 441, -8 495 675 564 635},
{337 884 338 873 182, -1 069 834 635 355}, {48 235 751 436 474, -528 357 661 561},
{40 818 713 653 249, 570 541 755 734}, {68 456 995 774 537, 917 318 809 378},
{89 923 626 277 819, -3 282 056 412 566}, {344 031 125 435 231, 9 323 956 899 321},
{251 238 597 826 898, 13 376 601 604 903}, {767 126 991 226 117, 34 655 965 413 973},
{1 234 982 807 220 993, -9 327 462 780 574}, {988 280 408 714 175, 53 276 652 254 113},
{6 305 683 821 974 636, -105 688 756 727 959}, {9 373 735 987 863 752, -111 215 453 920 615},
{8 320 756 793 940 196, 110 268 336 659 631}, {13 316 096 195 050 073, -365 723 249 882 227},
{39 465 569 413 243 963, -447 445 572 068 863}, {23 764 435 721 396 997, 240 402 441 033 826},
{9 311 762 470 317 351, 434 039 839 398 808}, {51 791 496 693 846 729, -64 511 144 695 636},
{2 880 506 644 981 477, 132 443 551 771 545}, {8 745 142 920 030 919, -118 094 387 732 763},
{1 619 613 913 098 191, 15 593 537 665 353}, {555 983 077 911 023, 6 409 557 438 464},
{433 534 258 895 735, -12 568 082 440 857}, {1 635 716 903 435 011, -58 849 698 701 757},
{3 175 635 636 330 655, 70 204 325 262 031}, {4 323 982 878 825 380, -131 032 934 988 907},
{27 345 637 648 913, -184 059 869 450}, {20 851 402 473 031, 124 460 090 917},
{15 225 806 669 575, -834 070 546 396}, {55 897 187 459 561, 2 527 901 460 520},
{74 522 451 295 823, -763 581 639 469}, {81 148 484 872 557, 3 967 471 755 665},
{473 150 086 684 591, -3 788 629 165}, {116 731 172 932, 5 304 112 383},
{10 704 233 078, -150 387 939}, {7 019 314 567, -78 392 046}, {9 459 997 699, -245 244 242},
{27 490 795 357, 841 842 595}, {76 272 703 114, -2 736 852 873}, {94 463 637 790, 1 078 468 269},
{116 132 878 966, -1 915 570 031}, {188 542 839 275, 4 837 442 353},
{30 879 485 396, 1 208 549 393}, {142 756 090 186, -3 025 173 599},
{150 680 861 679, 1 899 341 399}, {166 450 374 554, 3 973 011 223},
{109 433 461 556, 4 910 305 027}, {369 975 503 006, -14 054 670 635},
{1 197 719 488 448, 1 523 617 747}, {41 012 037 478, -1 767 881 325},
{92 251 721 789, 2 970 393 527}, {44 584 404 876, -454 528 571},
{10 679 093 434, 568 333 271}, {31 359 782 045, -780 972 668}, {31 790 210 475, 1 421 869 391},
{133 889 058 599, 4 865 841 908}, {619 237 398 975, 17 621 246 771},
{655 859 403 370, 5 965 647 333}, {95 154 257 380, 4 878 932 421},
{637 614 843 520, -17 627 103 843}, {799 284 660 236, 35 176 338 655},
{2 569 806 882 027, 99 593 223 088}, {5 159 249 502 643, -24 048 711 970},
{2 951 799 148 541, 140 623 678 353}, {341 399 477 336, -16 824 686 023},
{1 290 214 058 388, -14 616 992 525}, {1 030 622 357 444, 19 585 127 293},
{1 943 409 329 355, -7 873 674 899}, {365 141 493 574, 17 376 236 095},
{63 260 857 277, 976 769 880}, {60 275 634 749, 2 317 669 473}, {4 268 082 613, 87 594 094},
{6 319 362 159, -42 457 421}, {1 786 708 910, -63 469 487}, {2 515 141 062, -52 378 321},
{258 175 002, 2 997 121}, {111 142 748, 3 904 647}, {476 722 216, -24 404 399},
{2 989 195 932, 155 820 973}, {7 521 128 035, 343 946 554}, {12 018 088 239, -345 129 986},

```

```

{16 164 314 273, -132 033 491}, {14 788 061 573, -481 730 194},
{38 286 077 983, 45 277 352}, {4 881 755 767, -65 509 434}, {8 271 818 929, -100 951 291},
{1 627 163 379, -4 126 903}, {306 026 011, -5 557 473}, {95 993 948, -901 407},
{116 983 978, -4 881 309}, {44 036 194, 1 878 939}, {215 817 011, -5 582 616},
{501 018 419, -23 397 171}, {2 545 268 764, 20 998 291}, {1 177 070 439, -58 464 058},
{2 048 580 377, -15 589 066}, {1 686 548 253, -8 601 980}, {147 325 499, -4 263 377},
{497 779 048, 23 504 471}, {1 100 696 291, -8 171 330}, {639 947 117, 32 124 460},
{668 567 829, 29 113 825}, {276 188 398, -12 923 241}, {1 262 488 631, -57 777 831},
{2 268 020 213, -59 669 066}, {156 670 415, -6 860 298}, {293 623 457, -8 838 562},
{513 089 593, -4 908 627}, {609 171 646, 14 719 559}, {1 491 138 201, -74 885 975},
{1 730 881 637, 36 671 312}, {1 927 782 899, 78 940 291}, {8 735 785 645, -430 457 237},
{33 306 558 015, 639 920 264}, {8 075 227 481, 8 832 385}, {638 456 433, -287 332},
{1 243 727, -3625}, {92 576, -4031}, {36 031, -638}, {79 689, -841}, {54 178, 145},
{13 676, -435}, {50 233, 1914}, {123 347, 145}, {12 624, -551}, {12 887, -29},
{2893, 29}, {1841, 87}, {3682, 145}, {14 991, 116}, {7101, -29}, {1052, -29}}

29
264 is a relation number with a list {{264, 261}, {1, 0}}

29
265 is a relation number with a list
{{265, 261}, {1060, 29}, {689, -29}, {1855, -29}, {1, 0}}

29
266 is a relation number with a list
{{266, 261}, {1330, -29}, {532, 29}, {665, -29}, {1, 0}}

29
267 is a relation number with a list
{{267, 261}, {534, 29}, {1068, 29}, {1335, -58}, {1, 0}}

29
268 is a relation number with a list
{{268, 261}, {1876, -87}, {5092, 87}, {2747, 116}, {9916, 29}, {1, 0}}

29
269 is a relation number with a list
{{269, 261}, {2152, -87}, {6187, 58}, {5111, -174}, {17 485, 319},
{16 140, -551}, {43 309, 1189}, {135 845, -2349}, {106 793, -1334},
{19 637, 1044}, {53 531, 1943}, {234 837, 8990}, {295 093, 522}, {43 847, -1392},
{186 955, 8497}, {5649, 116}, {9415, 261}, {5111, 232}, {1883, 87},
{8339, -29}, {3497, -116}, {4573, -145}, {18 023, 145}, {11 567, 348},
{22 327, -261}, {32 011, 1189}, {24 748, 319}, {36 046, -319}, {1, 0}}

29
270 is a relation number with a list {{270, 261}, {1, 0}}

29
271 is a relation number with a list
{{271, 261}, {2710, -29}, {3523, 58}, {4065, -58}, {1355, -58}, {5691, 116}, {1897, -29},
{3252, 145}, {16 802, -261}, {26 558, 319}, {21 951, -464}, {38 753, -1334},
{18 157, -116}, {14 905, -464}, {15 447, -116}, {5149, -29}, {3523, -58}}

29
272 is a relation number with a list
{{272, 261}, {2992, -145}, {7208, -261}, {1700, 87}, {680, -29}, {3536, 29}, {1, 0}}

```

$\frac{29}{273}$  is a relation number with a list  
 $\{\{273, 261\}, \{1092, -29\}, \{910, 29\}, \{3003, -58\}, \{1, 0\}\}$

$\frac{29}{274}$  is a relation number with a list  
 $\{\{274, 261\}, \{1781, -58\}, \{2329, 58\}, \{2466, -29\}, \{1, 0\}\}$

$\frac{29}{275}$  is a relation number with a list  $\{\{275, 261\}, \{3850, -87\}, \{550, 29\}, \{1, 0\}\}$

$\frac{29}{276}$  is a relation number with a list  
 $\{\{276, 290\}, \{1932, -29\}, \{3036, 29\}, \{828, 29\}, \{1196, -29\}, \{644, -29\}, \{1, 0\}\}$

$\frac{29}{277}$  is a relation number with a list  $\{\{277, 290\}, \{3601, -29\},$   
 $\{1385, -58\}, \{1939, 29\}, \{1108, -29\}, \{1662, -29\}, \{2493, 58\}, \{1, 0\}\}$

$\frac{29}{278}$  is a relation number with a list  $\{\{278, 290\}, \{834, 29\}, \{973, 29\},$   
 $\{3614, -145\}, \{1529, 58\}, \{2919, 145\}, \{5282, 87\}, \{6950, -261\}, \{13483, -290\},$   
 $\{39754, -1827\}, \{61160, -1247\}, \{7923, 232\}, \{4865, -232\}, \{973, -29\}\}$

$\frac{29}{279}$  is a relation number with a list  $\{\{279, 290\}, \{3069, 116\}, \{4929, 29\}, \{1, 0\}\}$

$\frac{29}{280}$  is a relation number with a list  $\{\{280, 290\}, \{1, 0\}\}$

$\frac{29}{281}$  is a relation number with a list  $\{\{281, 290\}, \{2529, -58\},$   
 $\{6463, 290\}, \{23323, -348\}, \{1967, 58\}, \{1405, -58\}, \{3653, -87\}, \{1, 0\}\}$

$\frac{29}{282}$  is a relation number with a list  $\{\{282, 290\}, \{564, 29\},$   
 $\{1833, -58\}, \{6486, -319\}, \{7473, -203\}, \{5358, -29\}, \{987, 29\}, \{1, 0\}\}$

$\frac{29}{283}$  is a relation number with a list  $\{\{283, 290\}, \{1981, -58\},$   
 $\{2547, 29\}, \{1415, 58\}, \{6509, -261\}, \{4528, 87\}, \{1132, 29\}, \{1, 0\}\}$

$\frac{29}{284}$  is a relation number with a list  $\{\{284, 290\}, \{852, -29\}, \{1562, 29\}, \{1, 0\}\}$

$\frac{29}{285}$  is a relation number with a list  $\{\{285, 290\}, \{1, 0\}\}$

$\frac{29}{286}$  is a relation number with a list  $\{\{286, 290\}, \{1, 0\}\}$

$\frac{29}{287}$  is a relation number with a list  $\{\{287, 290\}, \{861, 29\},$   
 $\{2583, 29\}, \{574, 29\}, \{1722, 29\}, \{3157, 29\}, \{1148, 29\}, \{3444, 29\}, \{1, 0\}\}$

$\frac{29}{288}$  is a relation number with a list  $\{\{288, 290\}, \{1, 0\}\}$

$\frac{29}{289}$  is a relation number with a list  $\{\{289, 290\}, \{1, 0\}\}$

known cases

```

30
— is a relation number with a list
11
  {{11, 30}, {209, 240}, {341, 150}, {451, 420}, {341, -30}, {1, 0}}

30
— is a relation number with a list
13
  {{13, 30}, {221, 120}, {247, 150}, {689, -360}, {403, 30}, {1, 0}}

30
— is a relation number with a list
17
  {{17, 30}, {221, -120}, {323, -240}, {1411, 900}, {6613, -3630}, {10999, 3480},
  {9503, -7920}, {26911, 7830}, {58157, 30480}, {47651, -13620}, {115447, -27810},
  {71519, 32070}, {125443, 102450}, {390881, -327720}, {1073737, 113250},
  {926279, 290640}, {924103, 48570}, {21641, -14490}, {121567, -31800},
  {95761, 33630}, {87193, 43770}, {5899, -4980}, {15623, -1950}, {391, -30}, {1, 0}}

30
— is a relation number with a list {{19, 30}, {209, 90}, {551, -30}, {209, 90}}
19

30
— is a relation number with a list
23
  {{23, 30}, {161, -60}, {437, 240}, {989, -360}, {2093, 90}, {1, 0}}

30
— is a relation number with a list {{29, 30}, {1, 0}}
29

30
— is a relation number with a list {{31, 30}, {1, 0}}
31

```



30  
 37 is a relation number with a list

```
{ {37, 30}, {259, 60}, {703, -60}, {629, 180}, {3293, 1320}, {24161, 9660},
  {178303, -68280}, {981869, 138030}, {579383, -60360}, {896029, 53790},
  {680837, 217890}, {1005179, -88170}, {1306433, -84480}, {1451621, 405210},
  {6261103, 236940}, {3724531, -292890}, {3072443, 872250}, {15412609, 5216880},
  {8807147, -219450}, {1078439, -249960}, {2908163, 183360}, {947089, 126870},
  {2182963, -615720}, {10356929, -2410890}, {26394653, -3598650},
  {44551811, 11342310}, {30244873, -2776680}, {11048459, 4196850},
  {57057367, -16495260}, {280148719, 71118210}, {159992477, -36901170},
  {458348489, 121192350}, {977573707, 271647030}, {4033533281, -239642940},
  {1494677863, 383481990}, {1452253589, -58798710}, {655423957, 49852950},
  {271417459, 84013470}, {716950813, 201941040}, {3360093839, 701382750},
  {5432336707, 476422230}, {7092610549, 375326580}, {1427995427, 6926100},
  {45096599, 312030}, {5466787, 1752480}, {7745839, 2037660}, {14977637, -2529240},
  {7318711, -1363560}, {18533707, -5369730}, {89707129, 19526520},
  {293242427, -9188850}, {29628601, 3662790}, {12072397, -1514790},
  {1699151, -438060}, {1964293, 281520}, {234839, 56310}, {355163, 67680},
  {620231, -10290}, {104747, -41010}, {676471, -128100}, {1330927, -423180},
  {2271319, 916830}, {16193383, -5466600}, {7637429, -2088630},
  {26532367, -8771610}, {8048869, 1755930}, {27038897, 800880},
  {7067851, -979110}, {7920997, 2307510}, {36943279, -4484160},
  {39589963, -5414070}, {62584501, 2656170}, {43052423, 6443820},
  {76009729, 8096700}, {116158873, 17029290}, {112707809, 9609240},
  {96313627, 34918770}, {312379271, -25592040}, {195167267, 2556900},
  {31186079, -6538740}, {55781977, 15790230}, {273020891, 79866360},
  {1236607007, -52907670}, {730032089, -181830060}, {100338413, 24791790},
  {43336361, 3718890}, {47741803, 17239350}, {147121139, -41418900},
  {686515057, -137402190}, {18348041, -3981150}, {57635233, 7108740},
  {28316581, 10470090}, {114466493, -16150650}, {52241891, -4557990},
  {77848037, 20714460}, {185362711, -14964570}, {214151227, -32780700},
  {566605901, -165344670}, {2611159967, 233717400}, {1489936979, 191144730},
  {1451171857, -12600030}, {80231059, -10835640}, {162118423, -6576570},
  {84945599, -32166150}, {427455487, 150390960}, {877543541, 127708800},
  {607468183, 200192100}, {254999671, -36125940}, {78369367, -2262450},
  {30206171, 10236180}, {18587653, -1961910}, {34427131, 11151000},
  {36042847, 3451980}, {56352739, -9350970}, {9136003, 2169900},
  {16886911, -1866240}, {3357787, -987630}, {14611189, -1001580},
  {15262907, -67530}, {1127, 90}, {1591, 540}, {1073, 30}, {259, -60}}
```

30  
 41 is a relation number with a list {{41, 30}, {451, -90}, {1, 0}}

30  
— is a relation number with a list  
43

```
{ {43, 30}, {559, 120}, {1763, -240}, {3569, -360}, {1333, -330}, {559, -150},
  {1763, 300}, {1591, 420}, {3827, 630}, {2021, 300}, {3397, -1050},
  {10621, -690}, {11653, 2850}, {10879, 1110}, {9503, -1320}, {11309, -1530},
  {25757, 6090}, {60071, 10410}, {102727, -17610}, {126119, -34680},
  {541843, -20880}, {44591, -4350}, {46913, 9330}, {11309, -1200},
  {21887, -5790}, {54739, -18360}, {14663, 1770}, {21629, 660},
  {6493, -1200}, {21199, -7230}, {21113, 1560}, {31261, -1650}, {3827, -1140},
  {17501, -180}, {1763, -360}, {1591, -60}, {1247, -30}, {559, 120} }
```

30  
— is a relation number with a list  
47

```
{ {47, 60}, {611, -90}, {893, 240}, {3149, 780}, {1363, 120}, {2021, 480}, {4747, 1350},
  {30691, -4680}, {97243, -28320}, {577301, 142920}, {264187, -27960},
  {589709, -184890}, {1646833, -280470}, {1691389, 226770}, {4887953, 1298280},
  {14342849, 3065910}, {46374947, 3907380}, {24139811, 1253820},
  {14909857, 1827960}, {13450319, 61020}, {1218193, -242340}, {305171, -92160},
  {1348477, -27870}, {503699, -23850}, {133903, -9840}, {181279, -360}, {7567, -2400},
  {17249, -2700}, {49303, -1020}, {16121, 3510}, {67163, 6510}, {96961, -3480},
  {22513, 5490}, {25991, -7410}, {171503, 19860}, {340139, -64980}, {716233, 146130},
  {677599, 52050}, {44603, -2070}, {44039, 12960}, {242473, -9960}, {161351, 46830},
  {980467, -302310}, {3456239, -971910}, {20275847, -6088350}, {94507459, 15467100},
  {80128373, 10912920}, {175682851, -47782710}, {726055483, -71410980},
  {561447101, -130981650}, {1763463547, -528062400}, {8425988309, 2072519250},
  {6387831523, -447737730}, {5616655241, 466921230}, {639222607, -87481410},
  {1262078639, -83715720}, {298113433, 61349730}, {405855199, -33815700},
  {3139553, -189690}, {4003319, 1249500}, {11976493, -2430060}, {8168929, -499800},
  {8090063, 2328750}, {51879211, 10108080}, {62924117, -6892200},
  {42032899, -1979280}, {21996893, 5257830}, {45381931, -13586700},
  {217226057, 54699750}, {73928321, -22720590}, {271027897, -29888550},
  {95454509, -3408420}, {881203, 108210}, {729581, -36720}, {226493, -9000},
  {70171, -19890}, {441283, 89820}, {367399, -360}, {7567, -2400} }
```

30  
— is a relation number with a list {{49, 60}, {539, 30}, {1, 0}}  
49

30  
— is a relation number with a list  
53

```
{ {53, 60}, {371, -30}, {583, 60}, {901, -120}, {3127, -720},
  {13091, -1110}, {12137, -3000}, {7261, 1290}, {25387, 3480}, {54431, -420},
  {8957, 1980}, {49979, 8220}, {34927, 720}, {18709, 4200},
  {101177, -6480}, {132659, -32010}, {244807, -33690}, {475781, 99600},
  {1177607, 53760}, {270989, 65130}, {554857, -2880}, {52099, 5190},
  {10547, 450}, {10441, 210}, {3127, -510}, {3551, -900}, {2597, 660},
  {2279, -150}, {1537, -120}, {1219, 150}, {1007, -30}, {689, 30}, {1, 0} }
```

30  
— is a relation number with a list {{59, 60}, {1, 0}}  
59

30  
— is a relation number with a list {{61, 60}, {1, 0}}  
61

```

30
— is a relation number with a list
67
{{67, 60}, {469, 30}, {737, -30}, {871, 60}, {1943, 330}, {2479, 90},
{2747, 120}, {871, 150}, {1943, 390}, {469, -90}, {1273, 240}, {4891, 750},
{24053, 3600}, {76849, -330}, {2747, -30}, {871, 60}}

30
— is a relation number with a list {{71, 60}, {781, -30}, {1, 0}}
71

30
— is a relation number with a list
73
{{73, 60}, {949, 90}, {2993, -420}, {3869, -450}, {13213, 270}, {1241, 180},
{1387, -30}, {511, -90}, {2117, -390}, {12191, 1590}, {38617, -4980},
{89279, -3360}, {105193, -14100}, {473989, -55350}, {1763753, -308430},
{6338371, -927900}, {11455817, 1826520}, {36258881, -772230}, {2622817, 323550},
{2512441, -128580}, {4318607, 512490}, {15964151, -1951890}, {25479263, 4105050},
{61974299, -5958030}, {174761927, -4016370}, {142959769, -557940},
{9280417, 1222950}, {36732359, 1297590}, {29188247, -1237290},
{36990049, -886170}, {16723643, 2835840}, {21271981, 2789520},
{76225067, 15642630}, {145130059, -8704680}, {208013573, 37046430},
{1041345511, -136688130}, {3807645617, 589518270}, {19749127781, 2454434160},
{8296778573, -1536962910}, {44673373679, -2044768290},
{22741595173, -265691310}, {7873596551, -18882030}, {209959, -14280},
{309593, 24600}, {745111, 41460}, {85337, -10560}, {62561, 420}, {1387, 120},
{3869, 780}, {2263, -210}, {3431, -180}, {803, 60}, {1679, 240}, {1, 0}}

30
— is a relation number with a list {{77, 90}, {1001, 90}, {1, 0}}
77

30
— is a relation number with a list
79
{{79, 90}, {869, 150}, {2449, 240}, {3871, -150}, {2291, -330}, {1501, -150}, {1, 0}}

30
— is a relation number with a list
83
{{83, 90}, {581, 90}, {3403, 90}, {1411, 180}, {2407, -150}, {581, -60}, {1577, -150},
{6059, -690}, {12533, -1620}, {35441, 6360}, {225677, -38460}, {421889, -10110},
{226673, 19830}, {709069, 108150}, {3982423, -339870}, {7969411, -595890},
{18495803, -2662260}, {11621411, -1659450}, {436663, 51240}, {2033251, 156540},
{146827, 9330}, {203599, 35100}, {581083, 27120}, {959729, 169620},
{4813253, -160620}, {5347, 210}, {8051, -30}, {913, 150}, {1079, -30}, {1, 0}}

30
— is a relation number with a list {{89, 90}, {1, 0}}
89

30
— is a relation number with a list {{91, 90}, {1, 0}}
91

30
— is a relation number with a list {{97, 90}, {679, -90}, {3977, 120},
97
{1649, -90}, {2813, -30}, {679, -30}, {1067, -60}, {1261, -30}, {1, 0}}

30
— is a relation number with a list {{101, 90}, {1111, -150}, {6161, -510},
101
{4141, 150}, {5959, 780}, {28381, -2910}, {72619, -8070}, {1111, -30}, {1, 0}}

```

```

30
103 is a relation number with a list
    {{103, 90}, {1339, -90}, {1133, 30}, {721, 60}, {1, 0}}

30
107 is a relation number with a list
    {{107, 120}, {1391, 30}, {1177, -90}, {749, 30}, {1, 0}}

30
109 is a relation number with a list {{109, 120}, {1199, 120}, {1, 0}}

30
113 is a relation number with a list
    {{113, 120}, {791, 90}, {2147, 90}, {1469, -30}, {1, 0}}

30
119 is a relation number with a list {{119, 120}, {1, 0}}

30
121 is a relation number with a list {{121, 120}, {1, 0}}

30
127 is a relation number with a list
    {{127, 120}, {889, -90}, {1397, -120}, {5461, -240}, {7493, 390}, {10541, -270},
    {1397, 30}, {1651, 90}, {3937, 270}, {14351, -390}, {10033, -240}, {5969, -540},
    {3683, 150}, {8509, -960}, {16637, 90}, {1651, -120}, {3683, -420}, {12319, 960},
    {20447, -1170}, {70739, 1800}, {68453, 2220}, {46609, 4320}, {115697, -2040},
    {74041, -3270}, {148463, -5550}, {176149, -2520}, {31877, -3750}, {237871, 26730},
    {342773, 6030}, {118999, -6840}, {345313, 28590}, {283591, 13470}, {91567, 1920},
    {75311, 5220}, {283337, -6360}, {363601, 34710}, {2095627, -47100},
    {2949829, 289590}, {6848983, -433080}, {10197719, -403770}, {13140563, 1490400},
    {34675699, -885270}, {19071463, 197460}, {10433939, -430320}, {13494893, -458550},
    {25011761, 847050}, {50766853, 354180}, {15127351, -1473210}, {50196877, 2622810},
    {46162849, -4946040}, {209358103, 14763630}, {338744941, 34555740},
    {865182293, -96729810}, {684021619, 4612710}, {170248453, -17428380},
    {512489069, 34316880}, {287544637, -11112240}, {174447581, 10179420},
    {177475007, -6833790}, {25848691, 840750}, {27248993, 2649840},
    {95325311, -1237170}, {8029067, 299700}, {7979791, -362100}, {1726057, 86790},
    {1237361, 84690}, {4189603, 130740}, {752221, 78810}, {4556633, -321540},
    {6994271, 469170}, {5496433, 140430}, {2497201, 137910}, {1882267, 174000},
    {4030091, -202230}, {1842643, 2280}, {51181, -600}, {22987, -180},
    {6731, 600}, {16637, 1530}, {24511, 2550}, {125603, 2520}, {50419, 1530},
    {9017, -480}, {13081, -840}, {45593, -1020}, {38989, 600}, {1397, 30}}

30
131 is a relation number with a list {{131, 120}, {1441, -120}, {1, 0}}

30
133 is a relation number with a list {{133, 120}, {1729, -30}, {1463, 30}, {1, 0}}

30
137 is a relation number with a list
    {{137, 150}, {1781, 120}, {2603, 90}, {959, 60}, {1, 0}}

```

```

30
139 is a relation number with a list
{{139, 150}, {1529, -60}, {4031, 360}, {9869, 1050}, {58241, -4890}, {61021, -5130},
{74921, 1590}, {26549, -2460}, {71029, 4680}, {115231, 3900}, {245891, -11400},
{682351, -35370}, {1434619, 37650}, {544741, -57300}, {3928001, 334770},
{12404221, -1021140}, {20925199, -1935330}, {50516909, -3562380},
{89458871, 6828600}, {95502869, 1017420}, {18710929, -79830},
{4268551, -41130}, {1246691, 66600}, {2600551, -277080}, {14849509, -54960},
{1432951, 92310}, {6117251, 371610}, {23837249, 206490}, {12634961, -1294560},
{43178821, 2879610}, {2130731, -178890}, {2216911, -14730}, {1017341, 71340},
{2582759, -117480}, {250339, 12660}, {397679, 42690}, {1872191, -127140},
{4852351, -131130}, {75199, -780}, {44341, -3150}, {33499, 3180},
{205859, 2280}, {91601, 600}, {27661, 180}, {8201, -240}, {5699, -150}, {1, 0}}

30
143 is a relation number with a list {{143, 150}, {1001, -30}, {1, 0}}

30
149 is a relation number with a list {{149, 150}, {1, 0}}

30
151 is a relation number with a list {{151, 150}, {1, 0}}

30
157 is a relation number with a list {{157, 150}, {1099, 30},
{1727, -90}, {2669, 150}, {4867, -300}, {10519, -870}, {12403, 870},
{35011, 2790}, {197663, 15210}, {10519, -90}, {1727, -60}, {2041, 60}, {1, 0}}

30
161 is a relation number with a list
{{161, 150}, {1771, 60}, {4669, -90}, {1771, -30}, {1, 0}}

30
163 is a relation number with a list
{{163, 150}, {2119, -120}, {6683, -120}, {6031, -420}, {24613, -510}, {21679, 660},
{16463, 1500}, {6031, -300}, {5053, 390}, {2771, 180}, {11573, -480}, {8639, -330},
{9617, -690}, {7009, 240}, {7987, -570}, {1141, -90}, {4727, -120}, {7661, 180},
{12877, -900}, {45151, 2880}, {151427, 4350}, {134149, 6960}, {311167, -10920},
{881341, 4350}, {278567, 8730}, {129259, 4410}, {223147, -20430}, {258029, 5790},
{410923, -36210}, {2055919, 152010}, {11772023, -944700}, {71006549, 2838180},
{8483987, 428220}, {13107319, 159450}, {5284297, -269040}, {15729989, 427170},
{12274063, 401220}, {26692391, -1533630}, {101171003, -7916100},
{283342411, -13398450}, {321918643, 8259360}, {32012711, -2920200},
{17846707, -284550}, {13030709, 814140}, {728447, -24480}, {970339, 61260},
{1600823, 32040}, {191851, 3360}, {53953, 1530}, {65689, -4500}, {295193, -27120},
{509701, 11490}, {674983, 9420}, {530891, 27900}, {128933, -8460}, {331379, 23790},
{274003, 5340}, {271069, 22290}, {585007, -27510}, {1189411, -105930},
{3941503, 143730}, {9909259, -281280}, {10506817, 561840}, {27407309, -782700},
{2087867, -2460}, {109699, -2820}, {45803, -3990}, {311819, -19080},
{1065857, 28680}, {765611, 24810}, {570337, 49800}, {3673531, 4080},
{249553, 22020}, {1195279, 69420}, {2467657, -38790}, {2429189, 63510},
{2576867, -81810}, {6643391, 114780}, {2257387, -12990}, {468299, -37380},
{2875483, -257820}, {6432469, -588510}, {6705983, -342810}, {24485371, 1799910},
{116279147, 6229650}, {339725089, -15015510}, {917957483, 82238910},
{2172704099, -191120130}, {11472375047, 519619860}, {6640314701, 370114290},

```

{3 544 030 597, -319 276 830}, {5 213 631 121, -225 666 750}, {3 797 226 973, 256 754 640},  
 {8 817 098 201, 341 242 740}, {8 999 725 357, 694 733 160}, {5 184 332 849, 304 926 030},  
 {96 225 257, 8 205 870}, {365 964 829, 9 552 990}, {481 047 067, -36 515 490},  
 {1 034 348 611, -50 526 660}, {3 881 911 993, 337 702 380}, {27 251 287 519, -125 830 350},  
 {8 785 444 253, -510 041 040}, {18 703 691 399, -519 156 960}, {2 288 656 757, 43 674 690},  
 {2 864 378 951, -261 633 870}, {2 215 759 897, -173 579 040}, {6 645 122 549, 163 723 650},  
 {11 010 177 463, -343 585 560}, {2 516 645 509, 41 094 810}, {1 607 522 137, -106 394 280},  
 {1 892 093 731, 69 637 860}, {1 935 056 293, -45 679 380}, {2 693 140 279, -10 689 090},  
 {83 195 363, -3 249 750}, {211 596 331, -15 508 290}, {899 715 827, 43 973 220},  
 {3 300 982 601, -122 878 860}, {2 729 698 897, -66 688 620}, {739 127 249, -12 610 140},  
 {793 974 793, 9 628 200}, {727 370 059, -37 064 880}, {2 270 189 183, 192 008 220},  
 {5 527 241 491, 238 455 150}, {6 972 005 683, 372 452 550}, {17 048 621 021, -1 091 888 460},  
 {68 719 877 257, 908 196 600}, {49 399 487 909, -2 565 161 160},  
 {107 812 416 647, -1 422 971 610}, {54 348 391 219, 1 880 630 460},  
 {30 952 415 723, 1 082 471 040}, {71 596 843 231, -5 137 449 090},  
 {53 373 376 727, 2 421 927 720}, {14 827 602 581, -931 740 090}, {13 078 934 017, 222 191 160},  
 {4 946 140 949, 196 148 520}, {6 915 755 687, 151 247 010}, {6 781 903 999, 310 801 170},  
 {9 082 643 783, -511 023 810}, {18 872 921 911, -68 172 810}, {1 784 272 817, -53 220 150},  
 {4 109 602 129, 354 831 060}, {24 184 406 333, 27 067 710}, {2 109 432 389, 141 406 740},  
 {1 901 999 893, 54 749 160}, {2 317 975 241, 34 932 330}, {2 027 958 143, 95 312 340},  
 {4 303 037 489, -303 490 380}, {8 830 063 547, -713 979 840}, {42 755 791 121, 1 658 746 230},  
 {60 572 570 017, -2 815 817 010}, {224 190 885 089, 5 094 785 640}, {3 311 659 427, 300 340 380},  
 {1 290 185 261, 39 255 480}, {855 029 377, 53 418 930}, {53 219 011, -389 400},  
 {20 992 607, 1 653 480}, {81 929 179, 1 904 580}, {5 254 957, -15 030}, {903 509, -44 460},  
 {2 332 367, 50 610}, {702 041, -20 010}, {275 633, -14 910}, {1 182 239, -36 840},  
 {547 517, 41 280}, {1 772 951, -123 870}, {6 319 673, -417 600}, {9 074 699, 408 990},  
 {12 537 797, -254 160}, {13 684 991, -1 128 720}, {22 877 213, 1 281 960},  
 {32 284 921, -989 130}, {58 088 147, 862 140}, {52 937 021, 4 126 680},  
 {115 700 497, 8 777 400}, {259 870 411, -4 151 100}, {268 768 907, -15 904 080},  
 {260 873 839, -368 820}, {19 250 137, 112 830}, {7 138 259, 1 770}, {24 613, 1410},  
 {104 809, -1650}, {128 933, 7920}, {360 719, 29 550}, {997 397, 43 830},  
 {1 742 959, -86 910}, {775 717, -32 100}, {866 671, 31 530}, {2 503 843, 70 260},  
 {4 159 271, 30 270}, {2 001 803, 144 420}, {3 272 551, -50 370}, {244 337, -19 200},  
 {857 869, -28 200}, {1 934 647, 32 310}, {644 339, -48 570}, {2 107 427, -159 510},  
 {5 508 911, 361 530}, {14 011 643, -383 700}, {30 196 891, 1 408 290}, {101 516 563, 5 342 910},  
 {207 499, 9570}, {495 683, -9000}, {111 329, 8280}, {601 307, 21 600},  
 {569 359, 42 060}, {3 175 403, 157 380}, {4 531 889, -203 850}, {7 691 807, -667 140},  
 {51 161 299, -4 250 460}, {25 391 977, -1 166 220}, {43 172 669, -607 500},  
 {6 547 547, -206 760}, {11 209 999, 690 840}, {25 519 117, -115 560}, {3 201 809, -21 000},  
 {1 598 867, 108 240}, {4 031 479, 164 640}, {13 059 397, 397 050}, {7 050 239, 160 350},  
 {841 243, 29 220}, {1 000 331, 24 000}, {1 250 047, -810}, {35 371, -1830},  
 {97 963, 8220}, {110 351, 600}, {7987, 690}, {47 759, 1800}, {137 083, 9360},  
 {540 671, -33 030}, {1 987 133, 102 060}, {7 822 859, -641 700}, {19 960 817, -1 731 540},  
 {133 279 069, -12 117 660}, {2 476 133, 44 760}, {2 336 279, -13 950}, {1 080 527, -86 280},  
 {6 701 419, 496 350}, {40 339 403, 763 680}, {22 108 831, 1 662 570}, {80 753 623, 3 471 570},  
 {147 924 619, -5 867 280}, {202 546 897, 12 876 180}, {565 933 229, -15 627 540},  
 {544 711 607, -40 947 270}, {2 020 726 811, 20 027 370}, {332 122 117, -24 742 500},  
 {1 706 547 571, 50 123 130}, {384 867 613, 24 099 240}, {117 397 001, 4 263 300},  
 {321 990 037, 16 225 740}, {411 536 369, 6 205 530}, {321 336 407, 6 093 000},  
 {259 592 659, 10 174 590}, {806 309 003, -26 053 440}, {219 664 831, 1 654 170},  
 {55 383 977, -4 602 090}, {25 900 211, -1 735 800}, {22 296 607, -217 830},

```

    {12 705 361, -430 140}, {32 410 757, -1469 220}, {14 330 471, 530 550},
    {916 223, -27 540}, {1206 689, -47 220}, {3 428 053, 125 700}, {5 566 939, -2700},
    {75 143, -2460}, {182 071, -1140}, {53 627, -1710}, {100 571, -1080}, {21 353, 810},
    {47 759, 180}, {9617, -750}, {21 679, -1440}, {12 877, -90}, {1141, 30}, {1, 0}}

30
167 is a relation number with a list
    {{167, 180}, {2171, -30}, {1837, -60}, {3841, -330}, {19 873, 1560},
    {67 969, -4110}, {317 467, 2010}, {18 871, -60}, {4843, -420}, {32 899, -780},
    {23 213, -990}, {73 981, -5850}, {345 523, -16 170}, {994 151, -21 540},
    {552 937, -21 300}, {144 121, 10 170}, {290 747, -25 200}, {1946 051, 13 320},
    {222 277, -11 640}, {186 539, -300}, {10 187, 690}, {27 221, 2130},
    {78 323, -3960}, {146 459, 3570}, {14 863, 780}, {7181, -30}, {1837, -60}}

30
169 is a relation number with a list {{169, 180}, {1859, -60}, {1, 0}}

30
173 is a relation number with a list
    {{173, 180}, {1211, -60}, {1903, -150}, {8131, 570}, {26 123, -1050},
    {21 971, -1230}, {29 237, -150}, {2249, -180}, {15 397, 900},
    {16 781, -1440}, {86 327, -5370}, {70 411, -1050}, {10 553, -480}, {1211, 90},
    {7093, -420}, {8131, -660}, {36 503, -240}, {3979, -120}, {3287, -240},
    {12 629, -90}, {5017, 90}, {3979, 300}, {13 667, -240}, {2249, 180}}

30
179 is a relation number with a list {{179, 180}, {1, 0}}

30
181 is a relation number with a list {{181, 180}, {1, 0}}

30
187 is a relation number with a list {{187, 180}, {1309, 60}, {1, 0}}

30
191 is a relation number with a list {{191, 180}, {2101, 60}, {1, 0}}

30
193 is a relation number with a list
    {{193, 180}, {2509, 30}, {2123, 150}, {4439, -30}, {1, 0}}

30
197 is a relation number with a list
    {{197, 210}, {2561, -30}, {2167, 30}, {1379, 30}, {1, 0}}

```

```

30
199 is a relation number with a list
{{199, 210}, {2189, 120}, {5771, 390}, {15721, 600}, {24079, -390}, {20099, -1170},
{41591, -840}, {81391, -4620}, {352031, 17190}, {1637969, -36210},
{1695281, -49830}, {211139, 14790}, {811721, 6330}, {294719, 15630},
{447949, -3990}, {212731, 7740}, {746449, -35160}, {1609711, 40590},
{2763911, -160680}, {6437849, 52170}, {4166861, -297060}, {1596179, 80040},
{919579, 14490}, {1335091, 65730}, {4077709, 170940}, {4945349, 277320},
{9235789, 506520}, {23567371, 1317120}, {28017011, -239340}, {2831969, 187500},
{3874331, -67980}, {105271, 6780}, {638591, -1440}, {133529, -4740},
{160991, 3270}, {151439, -11340}, {799781, 34170}, {2760329, 141750},
{13348721, 35070}, {2576851, 13530}, {1224049, -75480}, {3257431, 202650},
{2991169, 194580}, {14421331, -411840}, {1379269, -31740}, {2875351, 185790},
{17611699, -198210}, {5769209, 305940}, {8686549, -643680}, {63423091, -3795810},
{220030121, -7552320}, {201555359, -14035410}, {1006864181, -60852330},
{5497460371, -321829380}, {5245821289, 12967110}, {1165793939, 55762560},
{1038744379, 21469290}, {1635473341, 80974620}, {3180207259, -186610440},
{1558126021, -22325100}, {921564821, -3044940}, {209347801, 6303630},
{264274189, 19372140}, {1380218429, 98333610}, {706029911, -15958890},
{763911449, 48731730}, {3143449969, -219875670}, {12972927211, -729469590},
{31347556391, -1334181960}, {131612890889, -7567398750},
{590455315661, 7314839640}, {407292340621, 17967440520},
{1185799476461, -245860080}, {3245813579, 5707080}, {301473259, 496830},
{20407649, -420210}, {36345559, 1433340}, {101899741, -6638970},
{460723009, -1496160}, {18759929, 782190}, {2513569, 84420},
{3787169, -242610}, {18823609, 37980}, {2879729, -177810}, {6919031, 80190},
{4515509, 301020}, {41591, -600}, {38009, 930}, {24079, 60}, {3781, -30}, {1, 0}}

```

```

30
203 is a relation number with a list {{203, 210}, {1, 0}}

```

```

30
209 is a relation number with a list {{209, 210}, {1, 0}}

```

```

30
211 is a relation number with a list {{211, 210}, {1, 0}}

```

```

30
217 is a relation number with a list {{217, 210}, {1, 0}}

```

```

30
221 is a relation number with a list {{221, 210}, {2431, -120},
{6851, 450}, {22321, -540}, {40001, 120}, {9061, -540}, {1547, 90}, {1, 0}}

```

```

30
223 is a relation number with a list
{{223, 210}, {2899, 30}, {2453, -90}, {5129, -60}, {6467, -330},
{29659, 1770}, {96113, 6120}, {402961, -9510}, {789643, 3870}, {36349, 2370},
{178177, 1170}, {75151, -1950}, {200477, 3330}, {150971, -8880}, {2453, 90}}

```



30  
 227 is a relation number with a list

```
{ {227, 240}, {2951, 120}, {11123, 690}, {18841, -240}, {27013, 930}, {9761, -450},
  {31553, 2070}, {114181, 2100}, {177287, 8100}, {207251, -3570}, {43357, -2460},
  {209521, 4620}, {367967, -21120}, {2026429, 26340}, {397477, 9240}, {35639, 1530},
  {101923, -2910}, {16571, 810}, {84217, -5340}, {277621, 1410}, {33823, 1770},
  {43811, 2280}, {111457, 2010}, {205889, -6300}, {456497, -17820}, {1548821, -48660},
  {1883873, 91140}, {6825209, 57450}, {2574407, -112410}, {2502221, 53940},
  {4762687, 285210}, {19495441, -330420}, {150047, -8280}, {228589, -6540},
  {70597, 1110}, {100561, 540}, {27467, -840}, {57431, 930}, {51983, 1860},
  {22019, -270}, {27467, -420}, {37909, -150}, {9307, -390}, {12031, -510},
  {47443, 2910}, {200441, -1680}, {118267, -6240}, {66511, 1290}, {129163, -2640},
  {44719, 2370}, {70597, 3150}, {294419, 14670}, {231313, -2040}, {180011, -11070},
  {656257, 2280}, {86941, -510}, {54707, -90}, {2951, 150}, {11123, -240}, {18841, 300},
  {13393, -840}, {10669, 330}, {24743, -300}, {32461, 540}, {13847, -30}, {2951, 180},
  {16117, 390}, {28829, 900}, {6583, -150}, {3859, -120}, {4313, 120}, {1589, 60},
  {6583, -300}, {3859, -240}, {4313, 240}, {1589, -90}, {7037, -30}, {2951, 180}}
```

30  
 229 is a relation number with a list

```
{ {229, 240}, {2519, 150}, {7099, 60}, {4351, 60}, {6641, 180}, {4351, -180},
  {7099, -300}, {23129, -990}, {82211, -540}, {29999, -1830}, {164651, -9240},
  {382201, 13020}, {1058209, -68280}, {7788061, -332070}, {34453279, 685980},
  {35329891, -275160}, {25055119, -647370}, {44039219, -1754850},
  {38464901, 1264950}, {118255829, -4675020}, {316095341, 6077040},
  {20440769, -829440}, {67607899, 3946230}, {119535481, -4574190},
  {138897889, 7891830}, {722506679, -8850000}, {731270509, 14857770},
  {741909391, 661380}, {36403901, 1154220}, {121630831, 6564510},
  {708722711, -17740470}, {205204381, 3284460}, {359040169, -431940},
  {22448641, 1075320}, {30475091, 1278660}, {48719521, 780480},
  {75515269, 658980}, {61241699, 1529250}, {16419071, -409860}, {5649659, 138570},
  {7261819, -338640}, {34436791, -855270}, {51751939, 755340}, {83933309, 2957220},
  {259033121, -1486020}, {106631789, -5037060}, {195458141, -1222590},
  {35783311, -1293090}, {96914861, 4103400}, {358783231, 364800},
  {41212901, -2553150}, {83012729, 2580270}, {101696381, 4684350},
  {311284051, -12447330}, {23083429, 1221720}, {29598479, -591720},
  {2857691, 18060}, {964319, -33150}, {679901, -20400}, {1534529, -47910},
  {322661, 18810}, {662039, -29010}, {1188739, -53100}, {4703431, 163500},
  {8717801, 246810}, {18194279, -685230}, {70287199, 382860}, {36420389, -1792800},
  {129245081, -4191120}, {155637331, 1475490}, {162791749, -3335670},
  {150242549, -3746340}, {89069321, 5554920}, {43647629, 2674020},
  {197697761, -9231900}, {876580169, -47060160}, {4021897459, 239054040},
  {9622859609, -536000070}, {5757438079, -198657360}, {830207669, 30508500},
  {1483500701, -9976020}, {670117891, 2010960}, {107220319, -3019050},
  {335595149, -12068430}, {531484039, -21398730}, {797884319, -12428340},
  {565758011, -29652600}, {540121919, 2354280}, {991799, 15540},
  {632269, 3030}, {229229, -3180}, {61601, -1920}, {36869, -150}, {7099, -60}}
```

30  
 233 is a relation number with a list

```
{ {233, 240}, {1631, -60}, {2563, -120}, {10019, 420}, {14213, -870}, {68269, -540},
  {53357, -2160}, {149819, 1740}, {41707, 2670}, {236029, -14310}, {1647077, 58890},
```

```

{429 419, -9450}, {971 377, 49 410}, {3 919 759, 95 340}, {2 520 827, 143 460},
{14 318 549, -241 560}, {15 496 597, -415 920}, {25 060 781, -108 060}, {2 129 387, -45 660},
{3 875 489, 159 990}, {8 324 857, -237 780}, {595 781, -18 120}, {507 707, -27 090},
{1 631 699, 9270}, {41 707, 1170}, {96 229, -30}, {2563, 60}, {3961, -210}, {6757, 210},
{8621, 90}, {4427, 120}, {3029, 120}, {6757, 120}, {8621, 210}, {2563, 90},
{10 019, 330}, {27 727, -1650}, {75 259, -3150}, {79 453, -2610}, {268 649, 14 490},
{1 552 013, 20 940}, {571 549, 22 080}, {589 723, 18 600}, {1 276 141, -61 740},
{4 752 967, -301 860}, {17 892 769, -1 084 110}, {125 144 533, -5 210 850},
{19 602 989, -88 860}, {8 171 543, -338 220}, {12 643 279, -666 540}, {4 888 573, -165 390},
{17 038 591, -952 710}, {25 674 037, 501 540}, {22 250 801, -602 490}, {9 629 657, 274 860},
{2 226 781, 106 050}, {62 677, 690}, {26 329, -1440}, {95 297, -4230},
{464 369, 28 950}, {272 377, 11 910}, {361 849, 20 370}, {1 120 963, 16 680},
{792 899, 7020}, {84 113, -330}, {8621, 300}, {18 407, -1170}, {72 929, 300},
{6757, 300}, {33 319, -1260}, {130 247, 8280}, {520 289, 13 470}, {1 174 553, 37 320},
{4 108 489, 231 720}, {14 555 743, 359 010}, {38 134 411, -179 160}, {6 213 877, 140 640},
{5 992 061, 365 700}, {32 820 613, 691 500}, {74 586 329, -2 138 130}, {57 835 493, -739 920},
{28 363 789, -757 830}, {75 510 407, -1 571 730}, {15 696 511, -410 280},
{24 667 943, -311 340}, {16 795 339, 982 440}, {21 869 147, 831 150}, {60 404 551, -777 300},
{52 389 817, -1 016 790}, {112 600 279, 4 945 830}, {268 837 963, -10 105 500},
{934 455 121, -51 740 700}, {727 547 393, 28 573 170}, {3 079 827 319, -83 704 320},
{4 015 177 393, -141 967 380}, {9 341 145 449, 597 832 980}, {52 234 459 823, 1 939 721 190},
{32 156 867 531, -654 793 380}, {16 774 115 263, 775 912 890}, {68 960 617 861, -3 206 713 170},
{369 787 747 807, -14 630 333 310}, {938 853 708 281, -24 159 013 350},
{780 040 281 977, 4 725 330 630}, {84 049 630 291, -2 825 725 830},
{168 259 693 897, 8 463 970 290}, {237 592 873 399, -14 258 223 810},
{1 117 685 009 443, 12 283 501 740}, {26 480 193 001, -1 513 167 930},
{176 226 798 503, 10 474 203 990}, {427 477 953 191, -18 726 018 030},
{750 367 529 267, 15 539 177 340}, {1 045 474 948 651, -13 855 406 850},
{1 472 428 331 933, -5 397 996 540}, {285 360 572 471, 8 515 237 080},
{968 694 762 017, 11 544 119 880}, {235 634 741 399, 10 412 168 970},
{895 918 764 263, -3 594 076 080}, {231 560 139 919, -2 610 638 520},
{183 298 388 113, -5 338 146 420}, {419 728 491 089, -815 331 090},
{38 915 720 813, -430 953 570}, {30 266 586 529, 909 438 330}, {59 443 341 887, -2 403 045 870},
{147 443 533 079, 9 369 456 900}, {574 992 115 793, -36 117 188 430},
{671 715 487 271, 26 068 561 020}, {1 413 634 125 017, -67 546 461 150},
{1 128 083 277 989, 51 673 857 030}, {2 036 787 364 343, 23 367 117 990},
{896 607 116 629, 18 718 601 340}, {439 379 212 003, -5 356 946 010},
{25 545 929 639, -1 570 909 620}, {95 850 542 527, 4 216 205 640},
{261 469 615 969, -6 073 056 210}, {76 470 352 787, 2 797 319 550},
{219 654 910 321, 1 295 248 620}, {125 203 733 407, 4 499 466 570},
{182 050 018 849, 6 420 535 740}, {530 079 224 057, -5 527 137 720},
{122 557 315 679, -6 129 686 220}, {8 483 231 993, -461 322 780},
{41 805 315 049, 164 964 060}, {16 172 033 477, 956 376 720}, {20 124 387 779, 792 780},
{77 477 393, 4 819 230}, {86 143 129, 2 650 200}, {306 038 743, 12 969 480},
{1 218 305 041, -41 485 950}, {3 544 510 403, -82 357 020}, {735 940 519, 46 341 210},
{1 285 889 953, -35 761 980}, {359 129 191, 9 375 540}, {666 070 343, 40 497 570},
{4 219 448 959, 200 230 080}, {3 405 826 007, 170 661 420}, {1 724 757 569, -13 260 450},
{209 483 077, 12 103 200}, {868 781 741, 23 537 850}, {493 659 197, -18 049 830},
{1 471 112 371, -38 510 970}, {1 793 054 063, 30 691 860}, {3 011 800 639, 171 064 560},
{15 695 215 753, 558 822 120}, {11 229 759 569, 75 292 860}, {2 591 758 957, -143 015 730},
{4 071 865 361, 230 903 550}, {19 664 859 587, -629 447 580}, {35 412 413 431, -756 063 420},

```

```

{28558182997, -334148100}, {36253517801, 1496686170}, {77600584993, -974329440},
{80564458231, -1189577100}, {76140804577, 2672426340},
{305898024281, -7500850140}, {381381729947, -20079893100},
{31743676049, -1192943250}, {108529466333, -1519243350},
{154522916539, 4138080270}, {329449545917, -11450415900},
{608716037639, 3181418040}, {248189735767, 6287924010},
{689842954841, 43950593370}, {3114403605407, 185412226410},
{8761788750179, -332211091710}, {28961985212527, 904046034540},
{7575320988551, -35728912740}, {184416627343, 9528507210},
{786372752249, -7351453050}, {54224715533, 2366418300},
{47276950511, 2556188010}, {294876955123, -11880032550},
{494859060091, 28269955320}, {3262031610877, 133165531560},
{15391712850821, -680680796280}, {61499293023227, 231347361840},
{9111517707629, 61276865220}, {4365303965183, -226101983010},
{16162345102369, -657046046580}, {61466812476523, 2722273438470},
{266896049730871, -15732342688530}, {129029801974387, -5898862114080},
{173623336741909, 10783772848050}, {252332283334397, 10955663713860},
{82020174338761, -2980422050040}, {333572833529647, 7249667727000},
{20531514421751, -51159801990}, {3829080936313, -87880755750},
{8777649788071, 133165078770}, {2620180704517, 9870313830},
{1059576719111, -19462056780}, {2009777146903, 123193385400},
{9013134457199, -308176579050}, {17711183886517, -1112434702080},
{20450723795779, 1149526101420}, {56093824938973, -611488573950},
{38007860411491, 559075678860}, {2163579980437, 107310711180},
{4046221343021, -3294140340}, {236962281733, -4780573470},
{481469281711, -1977935670}, {193602938933, -12165504570},
{243516265571, 12700259910}, {515239256473, -26131270320},
{1720972932991, 105804543690}, {6547354510583, 205255142400},
{4848740768561, 246758582070}, {20138393371487, -450373548570},
{29921001199979, 919822344780}, {100920729418313, -6413241008460},
{394032525071951, 23004911140290}, {687125315075893, -36591011560860},
{1888209767244151, 16605884211030}, {1132620645491677, 68265557577900},
{6499263166501159, -6389916055590}, {167419346108057, -1476851065440},
{124695941207521, -6945598845210}, {75687255458347, 631259764110},
{14892482720749, 562977472800}, {59430943712117, 1088852908410},
{106240136350889, 6198035087280}, {203534789041057, 2801394573390},
{225314452224229, -14495156767290}, {1539677060211763, 7262940048960},
{15431629087381, 578056461240}, {40983620301067, 2511230088300},
{187317760966211, 6280611021660}, {256432736276237, -10630385709300},
{303710665957621, -13304082026970}, {531990414406537, 17503217653860},
{1606275156241721, -58081161092820}, {4659383565236687, -265263971867850},
{26880727313614829, -492175882481970}, {44024469934190393, 1309246882186410},
{114152306014378451, 3597634343521080}, {226474363942993397, 7385089077203190},
{573971605921179869, -20981514277553100}, {1740677859548357377,
41982655312599240}, {4517635073506729121, -106427095376530950},
{11113416772336008493, -472008699592808640}, {50046540168695936011,
434097880510990950}, {29191151014150585313, -335160885840285060},
{7491869428667926669, 41602490471357010}, {797126510913914477,
45754697091252750}, {4496121864489930391, 240647826448318170},
{17751533260550757487, 1069184958627995640}, {98934371417164235569,
5646526314778051680}, {629822823979881858343, -18151551899752599360},

```

```

{1 277 187 755 169 974 786 881, -46 252 566 295 757 369 580},
{4 166 995 558 916 953 796 647, 46 387 280 172 530 296 740},
{1 831 299 990 310 088 019 049, 38 089 842 667 056 594 720},
{696 097 353 889 553 089 937, 1 932 736 050 913 277 430},
{72 783 505 660 159 126 921, 506 692 349 363 843 910},
{41 984 887 038 614 295 727, 867 830 432 925 807 510},
{76 663 118 154 899 712 551, 4 788 735 966 392 001 630},
{10 098 847 382 250 947 743, 134 571 932 686 616 250},
{1 386 916 365 851 855 369, -73 574 068 987 496 790},
{2 560 890 164 165 988 353, -3 115 986 423 727 890}, {105 007 540 232 573 891,
-4 070 507 377 709 370}, {192 376 819 973 646 857, 7 185 408 834 792 150},
{379 607 925 817 697 969, -12 397 321 450 554 090}, {1 097 206 121 828 565 293,
63 152 408 291 810 370}, {5 502 337 142 194 837 699, -163 052 814 715 255 680},
{9 659 844 042 858 313 093, -565 153 226 530 968 090}, {12 171 731 696 822 346 179,
-37 938 365 439 546 210}, {1 510 680 960 373 024 823, 86 766 630 231 505 080},
{8 306 041 419 923 161 879, -102 875 625 399 240 270}, {6 264 027 317 764 897 903,
-225 792 955 747 008 990}, {13 554 878 254 265 439 361, 251 859 852 834 659 370},
{10 614 035 121 836 822 227, 81 054 749 479 305 300}, {963 934 968 856 093 009,
-20 763 246 773 482 020}, {2 056 368 825 289 380 737, -72 003 169 224 462 600},
{7 391 478 157 268 076 479, -353 725 969 518 932 220}, {8 566 758 212 673 532 853,
-308 055 018 464 109 990}, {13 696 276 906 920 420 011, -525 415 013 365 018 740},
{8 268 368 347 174 335 643, 6 931 919 218 693 530}, {328 828 409 401 635 751,
-6 277 149 123 554 910}, {563 080 609 589 840 423, -12 582 759 720 035 430},
{732 453 630 138 664 991, 8 255 649 837 103 080}, {535 714 849 697 627 057, 7 766 093 302 650 720},
{33 922 047 168 521 159, -1 294 478 431 640 100}, {61 886 651 389 704 247, 1 179 583 729 413 960},
{127 753 308 221 550 191, -4 788 695 737 494 090},
{359 164 068 954 125 687, 5 902 889 467 150 890},
{212 539 930 304 314 499, -7 090 432 728 252 870},
{40 321 009 582 283 033, 1 159 102 871 845 170}, {57 688 687 225 414 661, -2 672 762 258 174 250},
{259 115 211 879 589 487, -11 133 392 864 137 980},
{709 992 009 028 915 651, -34 452 693 634 753 860},
{3 148 891 851 113 290 297, -81 256 763 651 596 020},
{4 688 409 992 656 394 539, 219 429 822 794 203 470},
{18 729 405 356 902 348 877, 485 408 904 832 757 040},
{46 959 270 057 015 934 139, 1 778 626 171 817 748 990},
{166 592 574 412 789 272 967, 6 875 831 873 493 087 240},
{366 418 001 606 556 755 231, -1 992 811 410 393 464 220},
{60 416 412 060 874 071 017, -2 411 171 891 513 084 940},
{31 947 742 119 938 771 461, 1 738 666 500 405 503 850},
{151 856 611 245 050 603 513, -5 490 126 368 529 964 380},
{434 994 008 192 696 996 591, -8 980 237 046 513 697 090},
{918 632 780 689 211 951 143, 36 624 946 583 658 164 370},
{701 124 050 777 577 161 069, -42 368 324 617 497 096 840},
{4 459 029 978 730 522 054 163, 111 711 098 741 346 106 110},
{2 193 455 225 134 070 325 221, -46 126 258 364 397 669 510},
{4 801 006 091 185 150 023 347, 238 778 256 825 573 253 740},
{5 927 742 438 968 593 011 451, -80 356 895 011 469 196 510},
{4 349 595 508 069 714 557 337, 242 042 576 346 067 800 720},
{1 670 811 815 164 864 360 159, -32 912 274 917 772 370 980},
{1 797 409 914 475 688 438 293, 31 496 470 729 668 215 550},
{491 882 312 111 835 402 719, -7 890 758 395 834 538 490},

```

```

{618 682 935 831 905 806 987, -6 395 522 864 576 194 260},
{392 088 213 452 513 442 289, -24 347 001 340 279 347 120},
{590 932 737 874 225 989 977, 33 580 705 813 660 951 290},
{3 150 152 257 799 374 045 619, -117 923 394 730 455 702 060},
{7 870 600 182 042 669 030 233, 114 837 034 622 951 479 170},
{12 385 163 217 249 046 571 801, 352 126 472 753 651 926 860},
{14 151 644 312 996 387 686 333, 50 962 475 441 571 162 030},
{3 710 259 324 172 118 415 631, 68 638 042 410 437 752 260},
{886 572 923 975 791 906 703, 11 521 046 016 863 194 380},
{127 595 302 183 056 109 781, -6 545 234 052 968 166 810},
{753 954 256 161 999 111 103, 28 170 950 455 668 520 950},
{1 552 107 630 864 872 409 451, 30 960 623 469 679 620 180},
{949 814 569 747 696 305 083, -1 504 295 742 427 296 330},
{140 721 812 324 850 758 749, -6 245 830 624 337 158 680},
{683 224 044 132 606 577 603, -40 190 402 330 426 381 970},
{2 981 347 921 566 401 671, -11 692 196 794 901 940},
{37 806 844 127 175 757, -1 705 191 150 735 180},
{68 184 842 963 418 701, -2 247 143 268 870 990},
{179 536 961 068 337 233, 8 091 597 482 470 020},
{354 583 233 781 252 769, 13 507 974 999 459 270},
{786 580 924 307 637 517, 7 786 245 234 083 340}, {39 646 269 996 301 241, 2 037 304 946 533 170},
{218 431 910 835 845 563, -3 420 713 664 987 000},
{115 046 947 534 127 821, -2 870 947 840 376 940},
{48 704 903 138 701 493, 2 068 033 343 382 390},
{216 200 024 876 877 011, -8 624 246 745 404 700},
{138 368 504 329 966 063, 3 723 167 885 447 190}, {142 431 168 441 867 689, 5 575 595 836 948 740},
{590 497 333 280 295 383, -6 608 937 421 285 410},
{536 343 349 113 277 069, -20 626 580 469 531 150}, {12 175 858 973 850 377, 596 915 469 446 670},
{55 349 053 285 655 641, -3 448 446 569 112 090}, {40 520 605 907 892 833, -32 259 639 748 350},
{582 123 463 899 289, -21 344 165 666 550}, {1 358 620 880 268 287, -75 158 242 257 390},
{1 344 997 075 017 211, -21 135 951 112 860}, {1 794 984 515 958 157, 71 284 999 624 110},
{2 996 269 407 809 831, 20 617 203 942 600}, {1 578 536 818 949 623, -74 073 497 012 520},
{5 357 457 933 001 799, -14 088 538 889 910}, {888 465 076 787 767, 34 815 145 970 100},
{3 897 791 395 316 089, -82 144 162 313 460}, {8 624 673 613 948 277, -261 548 861 466 990},
{1 500 243 769 737 569, 94 088 052 194 820}, {1 203 460 233 435 383, -74 289 605 892 330},
{3 454 583 623 837 999, 37 572 642 067 620}, {489 171 007 248 553, 265 815 525 510},
{16 412 592 265 649, 651 947 610 720}, {26 539 165 452 217, 1 553 156 401 080},
{31 573 045 688 681, 82 729 053 450}, {6 862 485 908 027, 162 931 830 690},
{4 508 321 437 951, 232 529 409 120}, {21 031 200 868 343, 21 753 522 360},
{1 038 074 130 041, 10 418 595 900}, {882 012 170 447, -42 693 070 530},
{3 388 358 389 139, -86 708 937 780}, {1 563 387 062 527, -73 735 345 740},
{3 482 138 862 971, -143 261 292 240}, {10 221 208 866 163, -478 994 183 670},
{37 823 125 118 669, 402 751 479 060}, {8 274 741 722 243, -84 364 377 540},
{1 638 624 534 259, -35 601 895 650}, {218 398 905 647, 167 390 700},
{10 708 179 749, -397 436 580}, {5 267 643 263, -315 791 070}, {23 487 547 991, 999 771 870},
{114 821 230 573, -3 594 745 170}, {49 073 264 011, -2 777 694 720},
{215 581 141 117, 8 786 614 950}, {951 626 203 489, 35 677 359 480},
{2 717 363 075 743, 84 177 020 280}, {5 521 733 440 439, -293 432 772 480},
{12 462 992 146 673, -631 279 330 650}, {37 884 510 654 191, 753 064 347 150},
{53 891 338 129 003, 1 994 020 367 700}, {12 299 650 856 999, 598 457 978 730},
{62 436 240 245 123, -2 777 693 915 280}, {309 184 967 388 379, -10 255 109 958 000},

```

```

{356878795072307, -37528742760}, {4189379019811, -113716678920},
{4226177353357, -167021148270}, {11801134659431, 590016806550},
{186057124423, -8724039120}, {664586576399, 20956975200},
{1406534790233, 6695079210}, {132380378989, -8157471150},
{433575857237, -2633377170}, {217010564429, -1131155970},
{39931961963, 1345170180}, {98592420821, 3932925810},
{62741208043, 3527528040}, {175751125741, -7273622160},
{275917178933, 10485254160}, {769032990109, -32363860470},
{1794021052843, -81885069780}, {1735962379861, 80491350390},
{8119427591527, 63072867390}, {3954546315439, 69924449340},
{7257320187253, -407275256310}, {17156821334191, -93275241600},
{1356787008697, 71124115320}, {1264914504761, -40263038460},
{3905152812733, 172090164390}, {12330585599221, -406282125120},
{33114390029693, -863317043100}, {71843777311069, 2353107607080},
{256896132459763, 14030766839970}, {1011762736290599, 12421668485760},
{1306568223961087, 34378395722190}, {44080458663011, 1900901960160},
{83813263984123, 462454140150}, {25412055754709, -222156148320},
{20097379171357, -9474821160}, {299053402301, -12863725410},
{742738263943, -32670400500}, {2022660780781, 59778941910},
{228815889047, -77719200840}, {8145462072071, -279450805350},
{9643571042593, -545639249790}, {41458960695091, -979581410370},
{73754160075383, -332617739490}, {20265895295501, -780348956130},
{5400372383807, 340981605720}, {12892660697129, 231248973960},
{13346669799023, -608895425850}, {11423889734741, 667473553290},
{17903563612963, 1074287006460}, {83720510767681, -2381179673850},
{88358768622923, 2641744901520}, {275216541353779, 13121256945030},
{76856096601283, 498271266780}, {28500913498979, -1331451316740},
{125921552453287, -2179723760190}, {117065173591789, -4598514363390},
{489839280140087, 726551920020}, {33385648859431, 1641922834470},
{127495775617223, 5005423110120}, {549926102363959, 33368609830920},
{3734604401132687, 81280457369640}, {1001116623885449, 9826442894610},
{275068467991643, 12513966859320}, {55641078821501, 29294355810},
{2585633226463, -165612232200}, {14949859875721, 90156860400},
{3769695508207, -135702097290}, {6981429307729, 157211959920},
{14936015601017, 91636049430}, {153886265009, 7949883630},
{661364917087, -21071299950}, {1900026142421, -16841706150},
{719190039257, 34935346410}, {3367370837249, 97838437680},
{9521301778057, -496099014090}, {22232978910851, -1086457866570},
{117390428012083, 3804322609200}, {126652479436261, -5819113494060},
{318748061902747, 1516185387570}, {81347409539951, -2841928004130},
{248961101097827, -10987400323680}, {873541778807429, -26819103883530},
{2676855298331213, 44980556369550}, {5120893535136371, 69010609952610},
{3287256883872823, -4102334325210}, {299891825449829, 9473136935820},
{756913663663763, 34263076477530}, {728353609837999, 12044866101840},
{1319162988530567, -80984499346770}, {5454762762863551, 93520827822660},
{7119256551780143, -209066504795340}, {2561925576089839, 107030381994300},
{1585236883193113, -36933114170640}, {672677091646831, 30947952870330},
{1905444059599957, -96124813413660}, {3973164620865619, -111833923297980},
{12315591961767013, 686127554832060}, {8086037873945611, 464876194639560},
{42672217662030203, -1569385692837120}, {69621321614715379, 1861998745345530},
{169476752604869177, -2575114492952910},

```

```

{112 027 315 695 331 739, -5 811 274 970 804 550}, {375 850 261 260 552 337, 969 581 840 582 610},
{80 965 842 321 579 919, 3 432 735 574 478 250}, {330 816 071 554 252 873, 9 465 146 708 473 920},
{108 126 735 463 898 191, -5 719 414 409 713 380},
{126 318 228 712 854 757, -1 036 711 350 613 800},
{37 409 562 452 720 419, 719 651 649 750 900}, {2 871 336 898 046 773, 164 979 133 349 520},
{15 539 150 047 449 389, 425 908 340 626 350}, {48 102 799 881 883 837, 140 746 613 560 830},
{7 582 275 729 365 359, 398 834 078 750 070}, {1 031 778 315 568 757, -64 555 045 842 690},
{256 863 374 027 939, -6 678 848 616 180}, {714 640 500 852 067, 8 062 845 110 550},
{687 982 358 943 739, -18 433 099 021 860}, {1 388 142 966 436 127, -5 371 574 951 700},
{530 454 533 123 791, -22 197 359 081 520}, {531 725 766 016 537, -31 168 752 536 760},
{432 674 683 746 761, -20 125 063 758 780}, {2 341 264 341 284 773, 134 065 654 147 140},
{14 480 535 442 530 569, -458 295 183 246 810}, {43 084 128 178 592 783, 1 383 837 517 116 660},
{43 143 479 478 483 259, 246 784 009 379 760}, {10 187 263 973 114 653, 212 580 941 174 040},
{3 872 740 354 749 211, -166 385 672 928 330}, {10 687 681 433 645 693, -237 164 778 299 250},
{3 557 073 571 810 219, 157 675 607 652 840}, {16 185 439 179 788 533, 772 901 687 642 820},
{10 600 628 745 590 071, 79 099 193 543 460}, {311 476 908 578 423, -17 876 481 121 620},
{1 765 377 976 035 739, -73 786 165 460 640}, {1 279 168 839 571 693, 63 392 091 111 600},
{2 639 195 040 148 469, 158 504 860 798 830}, {12 905 309 269 572 353, -375 820 901 244 330},
{29 683 880 152 775 989, 338 782 823 012 880}, {30 058 927 459 286 083, -1 531 434 347 530 440},
{132 753 961 478 193 061, -2 124 276 558 719 190},
{244 373 857 161 564 473, 8 474 683 868 003 610},
{324 330 177 455 870 561, -11 916 576 383 135 160},
{601 749 320 914 549 153, 12 662 022 848 448 000},
{1 404 471 763 952 479 351, -56 918 934 430 057 440},
{4 310 872 054 156 899 217, -59 037 973 045 403 760},
{256 305 089 284 963 721, 5 425 529 154 383 790},
{304 116 033 739 662 703, 11 138 025 202 855 710},
{789 719 310 176 138 189, -48 535 672 530 275 310},
{3 063 612 078 173 842 357, 130 426 532 253 762 000},
{14 865 827 866 594 711 181, -235 499 426 785 305 360},
{6 841 807 135 070 325 733, -254 365 276 895 437 020},
{6 070 894 477 808 397 031, -139 068 206 123 454 300},
{11 208 835 848 296 975 377, 652 541 555 194 020 360},
{26 941 652 529 680 616 881, -588 638 837 983 875 360},
{31 626 026 095 592 375 207, -1 295 848 678 959 713 700},
{122 478 267 530 304 412 831, -2 307 795 878 842 840 110},
{38 465 026 730 695 671 233, 2 114 622 072 428 747 640},
{93 626 256 485 923 795 129, -1 543 252 307 304 666 870},
{119 327 282 500 985 958 253, 6 205 148 435 977 461 420},
{333 064 696 657 506 566 609, -12 251 876 179 726 587 600},
{527 521 274 539 067 428 297, -1 996 995 716 531 135 460},
{73 256 452 339 506 377 681, -3 124 100 925 684 282 390},
{326 696 534 362 916 671 663, -12 828 680 812 817 614 260},
{1 393 226 771 896 981 432 979, 60 469 532 276 416 610 550},
{565 614 382 680 057 946 657, 34 004 987 282 600 253 240},
{2 905 603 461 926 101 512 559, -66 809 328 633 653 198 430},
{7 642 943 048 210 257 356 077, 178 545 154 285 515 198 930},
{8 038 170 553 586 814 113 729, -202 717 668 249 603 855 090},
{16 434 929 100 580 240 939 943, 679 340 279 913 238 921 110},
{30 467 635 160 364 092 159 599, 1 371 426 024 776 468 655 030},
{69 029 189 360 655 147 502 787, -421 360 731 407 092 232 130},

```

```

{17 235 147 495 159 006 002 189, 535 871 475 320 782 262 730},
{20 331 646 380 295 847 595 157, -796 756 497 579 709 337 670},
{89 477 255 728 946 677 933 279, 1 313 436 683 306 587 230 870},
{38 109 774 535 007 872 549 727, 1 806 795 986 766 829 331 370},
{38 924 703 406 738 385 692 981, -4 743 602 559 375 002 430},
{302 712 549 842 029 690 567, 13 935 182 311 607 583 030},
{899 720 416 107 552 709 669, -3 270 227 401 372 527 870},
{95 036 210 115 058 082 627, -3 304 826 519 764 514 370},
{187 275 837 240 290 345 999, -1 584 020 683 188 890 670},
{84 205 413 392 290 536 787, -452 262 701 739 648 330},
{19 700 352 410 815 745 831, 1 156 885 076 755 671 930},
{7 760 322 690 852 263 893, -225 235 467 444 910 410},
{23 839 813 869 997 219 049, -298 297 074 756 049 500},
{5 580 841 743 410 641 583, -197 423 098 256 633 910},
{12 347 833 188 399 859 999, 106 061 341 860 428 580},
{10 419 185 093 503 719 527, 564 825 054 801 710 880},
{58 793 846 947 991 219 071, 2 913 843 161 607 554 670},
{120 457 205 790 749 281 343, -3 493 048 254 405 647 610},
{394 600 677 843 042 186 499, -968 975 617 029 843 690},
{53 031 198 871 722 487 877, -445 623 991 106 957 460},
{452 935 688 730 181 921, -24 528 218 943 772 380},
{2 662 665 223 951 025 873, 113 076 334 663 366 770},
{11 921 866 256 957 949 431, -251 713 911 978 387 840},
{21 275 787 795 876 981 583, -1 122 533 287 520 167 590},
{12 196 307 412 445 212 091, -696 525 708 876 112 800},
{79 489 195 926 682 665 997, -1 464 076 547 778 505 920},
{99 971 526 767 899 691 861, 6 410 665 148 718 637 410},
{605 593 937 502 452 060 867, -12 189 081 040 293 698 100},
{899 406 681 350 252 682 989, -55 030 001 786 201 442 450},
{4 409 910 095 649 897 682 837, 237 399 995 825 490 523 560},
{23 460 729 233 020 387 699 099, -941 693 508 751 268 995 860},
{19 014 777 182 391 566 994 433, -928 324 016 564 756 947 320},
{104 453 166 305 467 735 191 689, -1 117 007 333 302 905 669 720},
{127 106 864 826 257 678 543 903, -1 588 343 343 013 904 710 920},
{9 179 590 738 855 289 180 599, -142 552 407 857 113 499 190},
{13 103 136 188 005 879 158 287, 527 270 569 307 694 152 130},
{18 320 334 411 948 592 276 379, -194 292 937 792 291 304 010},
{13 233 994 457 257 859 969 287, 736 335 667 695 982 711 260},
{4 671 081 775 870 118 180 569, -159 561 716 127 446 213 430},
{10 203 537 904 583 471 926 067, -392 592 991 385 455 206 030},
{904 010 045 138 679 356 129, -13 201 523 798 633 207 550},
{1 469 397 451 767 749 555 857, -48 870 165 903 340 849 230},
{767 146 597 533 110 396 981, -27 711 052 520 345 468 940},
{2 041 749 417 519 116 867 987, -115 479 540 181 555 741 230},
{8 593 577 239 490 548 477 649, 351 472 723 104 226 316 430},
{36 868 029 202 464 233 815 657, 1 194 883 138 835 121 230 400},
{40 390 107 631 914 168 131 119, 2 416 152 959 146 162 640 460},
{159 486 792 941 949 044 311 333, -8 524 573 888 872 522 299 370},
{577 865 850 564 528 894 770 401, -22 664 150 662 094 599 371 360},
{2 624 065 574 834 191 143 331 433, 125 053 221 570 635 379 945 600},
{478 134 208 752 377 677 596 911, -18 411 689 493 497 411 015 070},

```



```

{132 744 312 303 317 049 213 797, -53 479 534 319 459 153 460},
{1 889 192 523 727 265 975 941, -55 304 194 705 583 858 370},
{2 062 027 570 817 646 387 113, 123 481 127 598 704 300 460},
{8 656 322 417 956 125 924 731, 207 143 990 556 740 144 280},
{10 187 968 204 481 711 461 757, 270 406 024 205 296 264 950},
{20 378 346 669 454 359 277 919, -32 888 609 760 473 166 390},
{2 933 792 015 087 904 944 273, 108 216 850 787 917 440 270},
{2 781 331 208 693 235 277 039, 146 734 223 903 243 918 610},
{1 542 237 594 137 008 136 383, -34 799 552 516 082 032 970},
{2 576 347 039 049 893 768 799, -147 051 667 080 059 975 850},
{16 445 831 635 146 290 584 733, 383 213 601 884 792 052 570},
{7 538 306 294 645 868 456 041, 6 189 444 202 236 895 710},
{101 761 277 130 230 866 187, -886 359 508 484 861 730},
{39 625 458 508 078 233 779, 2 442 150 843 093 467 490},
{128 393 489 329 781 667 787, 6 955 227 486 368 907 390},
{745 458 936 007 931 000 711, -11 123 228 998 125 309 300},
{47 204 200 113 719 683 363, -2 572 109 982 349 198 320},
{211 149 360 524 148 469 499, -1 196 141 140 848 230 580},
{132 255 787 595 283 956 513, 6 242 610 943 233 007 860},
{270 503 164 462 054 408 549, -8 278 462 339 106 399 400},
{625 859 605 730 427 794 683, -5 105 039 477 084 528 520},
{480 038 238 575 826 693 541, 15 131 726 108 243 577 270},
{973 240 274 896 492 530 067, -17 014 797 327 819 060 750},
{791 460 740 117 813 684 861, 9 840 059 261 257 606 140},
{991 647 817 608 810 123 013, -5 505 769 417 782 346 320},
{141 972 121 061 154 001 229, -3 267 217 568 937 325 260},
{345 251 384 065 820 506 417, -5 561 239 169 399 110 590},
{105 911 446 196 626 412 021, -285 371 704 390 732 020},
{8 980 721 165 905 996 033, 574 722 613 768 165 080},
{50 057 872 471 622 342 551, 1 439 243 254 344 041 970},
{73 544 453 287 656 450 967, -3 920 176 322 079 060 060},
{218 762 961 820 045 810 309, 12 060 124 472 558 427 900},
{391 608 066 160 627 189 397, -13 602 805 403 987 922 420},
{669 476 699 320 256 662 439, -19 898 856 945 856 545 270},
{1 650 673 783 455 749 280 653, -39 294 645 266 903 601 150},
{69 592 963 270 941 538 249, 1 945 308 979 132 875 030},
{102 091 274 837 177 339 623, -6 333 814 739 157 794 370},
{174 805 689 482 062 720 799, 9 694 406 868 440 723 730},
{71 383 243 080 218 622 547, -2 183 173 610 450 574 330},
{154 126 253 063 526 969 919, -7 279 679 192 273 848 650},
{291 946 676 005 842 546 677, -4 628 717 002 006 572 300},
{78 638 636 906 838 584 041, 4 899 601 497 927 258 270},
{57 088 015 020 571 250 993, 2 296 978 005 650 674 260},
{78 389 383 122 076 083 131, -264 033 410 594 346 450},
{6 649 779 095 641 316 927, -126 236 132 312 318 190},
{9 491 468 640 390 484 319, 83 158 652 456 195 310},
{2 652 066 669 523 022 107, -87 699 234 720 946 860},
{4 913 883 299 445 599 531, -187 878 911 148 963 660},
{6 764 365 030 402 838 443, -228 371 938 891 976 280},
{20 222 800 771 052 839 981, 1 134 779 947 960 499 040},
{47 354 522 091 021 258 187, -2 226 330 890 172 143 010},

```

```

{140 166 601 595 657 409 641, 4 633 758 333 332 508 660},
{268 847 421 793 940 912 953, 6 583 707 682 075 165 650},
{252 710 208 875 824 736 401, -4 727 518 614 874 633 680},
{501 351 292 980 312 267 113, -4 133 470 656 522 453 330},
{279 913 045 075 231 504 639, 9 989 605 317 553 862 340},
{47 554 410 807 542 674 727, 881 544 543 755 968 620},
{11 415 731 380 153 965 449, 377 253 479 308 474 140},
{22 863 591 209 639 711 017, -414 240 130 892 649 480},
{18 729 474 456 749 580 761, -57 137 845 199 788 440},
{2 735 133 125 979 421 247, -69 078 478 820 710 740},
{6 525 404 255 818 946 249, 131 850 261 290 841 210},
{15 084 758 448 280 381 447, -354 786 351 742 938 390},
{39 855 739 663 170 852 259, 558 975 156 439 369 830},
{39 261 328 542 313 478 657, -1 191 562 210 590 406 230},
{14 032 286 870 592 975 389, -602 766 057 497 778 870},
{39 299 538 717 566 301 307, 1 236 249 044 029 081 650},
{60 680 351 087 884 577 869, 1 032 040 155 609 732 780},
{48 934 215 689 889 883 183, -1 044 730 134 859 725 600},
{39 167 451 104 512 263 961, 1 357 187 557 519 240 320},
{44 500 218 806 149 339 327, -1 094 396 051 569 218 210},
{86 214 498 807 945 496 939, -319 042 634 511 182 340},
{17 006 085 152 819 777 387, 110 305 883 684 956 560},
{4 422 122 223 396 845 251, 79 532 694 364 230 030},
{7 388 118 013 008 487 957, -457 181 016 844 832 460},
{17 060 666 233 442 283 101, -1 083 866 297 563 183 500},
{65 518 324 923 496 125 467, -534 227 479 565 853 600},
{44 655 629 703 201 088 589, -2 017 338 909 708 550 980},
{63 882 469 679 821 317 757, -1 202 956 723 918 758 750},
{29 302 851 725 615 233 631, -1 094 363 750 899 893 210},
{57 077 904 842 878 748 087, -2 231 272 156 302 073 020},
{217 894 894 487 210 050 889, -13 161 183 537 452 733 150},
{1 361 937 576 330 334 150 013, 85 490 682 988 416 366 840},
{1 377 810 895 848 358 626 491, -50 468 148 959 876 199 000},
{3 534 813 626 086 392 063 403, 74 202 959 075 823 355 980},
{6 274 319 425 879 062 507 421, -324 391 446 195 557 052 030},
{25 835 493 922 090 494 892 283, 925 337 269 235 384 884 200},
{17 230 260 644 565 674 618 861, -410 199 716 024 449 946 130},
{436 309 168 535 013 366 433, -19 208 209 912 579 555 260},
{1 276 760 652 855 722 259 451, 36 988 751 634 748 692 510},
{4 158 037 465 992 300 966 967, -52 465 037 865 095 723 310},
{3 098 777 593 389 146 336 141, 144 157 601 689 804 162 380},
{16 652 034 191 459 329 795 513, -715 898 599 839 914 722 740},
{43 423 370 067 920 843 190 869, 925 381 864 461 924 845 280},
{16 211 571 896 982 517 188 803, -619 308 489 688 668 721 050},
{25 525 421 462 971 392 870 199, 308 659 804 352 370 779 310},
{21 748 755 498 163 962 319 723, 889 258 240 695 422 194 950},
{94 727 949 103 402 306 335 059, -147 267 869 619 745 447 380},
{8 087 182 532 094 195 044 527, 48 434 905 523 143 782 270},
{337 078 833 100 266 533 179, -1 148 874 523 063 677 510},
{106 853 297 327 902 300 517, -6 286 993 586 693 892 900},
{5 963 319 493 273 756 439, -110 785 265 944 493 220},

```

```

{4 446 774 180 828 443 753, 48 395 531 082 374 910},
{1 308 220 148 761 176 311, 9 345 545 403 059 640},
{36 396 386 451 376 337, 1 584 878 154 485 430}, {13 003 986 716 732 849, 750 994 863 001 200},
{55 238 252 651 000 617, -2 823 731 205 057 150},
{288 074 547 883 175 239, -9 711 212 298 570 870},
{760 004 310 230 550 613, 12 055 924 540 918 620},
{112 087 947 573 869 849, -5 194 875 129 646 590},
{512 438 129 856 745 523, 22 781 054 895 884 730},
{2 622 396 860 316 580 879, -94 376 839 953 960 150},
{4 696 035 405 872 673 793, 222 772 643 425 128 270},
{4 149 705 289 180 368 659, 79 234 538 162 728 980},
{6 875 667 999 401 575 867, -129 214 580 715 018 030},
{6 359 786 610 809 524 541, 190 698 564 639 306 480},
{15 549 016 806 991 693 333, 388 340 270 767 347 180},
{3 589 592 477 388 828 989, -103 857 542 308 169 100},
{10 583 210 291 521 856 063, -328 804 476 624 935 640},
{14 321 820 209 072 330 839, 837 026 746 523 630 460},
{21 521 165 733 752 833 427, 1 059 643 781 718 557 280},
{76 491 593 155 933 263 691, 679 426 604 157 975 990},
{66 081 855 542 899 400 707, 3 353 076 164 464 806 360},
{228 262 584 910 437 272 869, 12 264 128 261 048 577 450},
{1 108 113 527 530 167 792 673, -4 030 655 132 899 337 250},
{73 775 725 995 938 600 941, -1 260 384 969 809 119 440},
{136 768 022 912 270 922 427, -5 693 785 662 192 640 170},
{27 299 915 577 881 094 851, -1 493 067 077 000 255 040},
{98 957 008 707 225 462 523, -3 870 993 521 091 078 210},
{393 495 721 986 219 028 321, -10 022 843 802 767 083 050},
{606 921 587 044 549 923 443, 9 009 704 427 780 083 250},
{762 233 959 305 252 546 469, 38 285 190 203 621 610 660},
{808 473 830 752 862 348 323, 31 750 181 879 704 882 200},
{3 429 593 116 135 988 344 259, -109 042 339 751 312 042 130},
{11 482 376 035 958 403 907 357, -273 767 400 945 036 319 500},
{3 694 169 269 817 312 212 819, 51 493 413 044 985 638 640},
{3 112 057 375 245 328 237 813, 22 857 240 006 738 531 780},
{809 147 098 630 884 365 789, 12 453 398 371 566 833 250},
{75 444 356 383 632 342 413, 2 804 002 434 293 137 920},
{61 444 276 751 794 872 491, 3 303 695 092 828 617 870},
{308 941 692 784 086 020 087, -13 980 849 818 213 751 480},
{317 578 250 528 352 593 791, 13 654 272 476 565 969 960},
{822 486 171 189 121 337 663, 4 460 276 438 114 760 780},
{418 306 432 209 247 515 319, 15 919 661 757 687 400 230},
{1 024 087 776 684 400 475 987, 17 290 921 666 072 408 830},
{914 151 823 967 906 718 961, 26 918 394 343 949 140 050},
{250 145 008 242 821 958 187, 8 478 917 089 500 391 500},
{983 843 535 030 220 327 429, 51 214 450 397 506 450 740},
{2 509 171 752 280 278 864 977, -20 598 057 514 514 317 170},
{883 364 626 279 004 334 779, 22 354 142 892 370 399 230},
{2 516 653 833 884 110 820 093, -23 992 374 332 718 498 510},
{593 094 754 960 244 965 481, 15 641 617 107 373 782 000},
{299 799 962 950 388 870 927, -16 016 547 734 414 742 420},
{1 051 865 452 813 457 767 349, -60 277 340 814 002 460 660},

```

```

{6 326 103 541 271 913 118 057, -197 784 332 200 445 907 990},
{697 855 770 168 933 466 159, -10 672 498 153 983 456 300},
{965 409 907 282 051 951 547, -657 973 872 861 322 500},
{37 800 940 116 599 662 951, -2 428 623 499 273 178 790},
{246 289 358 122 689 061 537, -4 930 095 425 796 093 990},
{50 191 267 937 943 645 379, -1 594 078 187 016 822 750},
{180 538 684 718 358 650 057, 504 969 827 707 561 170},
{56 039 669 020 941 971 099, -2 211 441 400 702 327 170},
{175 596 722 788 423 500 817, 4 741 615 971 174 145 200},
{36 565 122 210 369 921 161, -1 573 056 326 329 508 250},
{89 664 622 216 356 918 763, 2 911 512 564 806 732 310},
{137 998 279 187 865 403 351, -3 197 713 976 936 182 650},
{115 702 715 849 025 010 433, -200 087 211 806 455 950},
{12 187 630 000 178 820 589, 456 362 053 219 963 350},
{31 255 886 765 124 237 613, -1 698 917 727 303 368 970},
{157 360 667 963 617 903 649, 9 372 773 736 472 721 790},
{460 521 134 645 479 459 973, 10 042 687 026 242 949 840},
{336 095 174 875 222 211 411, -3 147 007 166 710 392 180},
{147 859 927 330 012 180 817, -9 219 926 620 488 285 390},
{79 476 626 712 510 196 441, 695 931 283 801 339 230},
{32 727 263 683 703 143 493, 2 027 179 686 134 428 650},
{68 126 568 393 682 426 669, -1 336 836 125 379 975 210},
{12 133 242 162 240 006 553, 601 033 056 569 249 160},
{26 231 380 189 220 441 249, 1 566 034 228 956 330 090},
{91 149 996 807 660 675 473, -1 068 391 522 256 549 640},
{78 455 157 893 971 765 009, 3 602 837 204 690 988 630},
{188 091 721 950 586 470 283, 8 162 570 998 483 742 760},
{82 153 233 612 270 125 099, -2 101 478 839 376 673 120},
{45 565 218 243 110 506 627, -2 702 966 890 880 023 650},
{89 756 004 131 025 633 559, 5 736 664 578 214 925 190},
{473 136 585 056 268 489 073, 3 572 372 748 614 288 190},
{368 928 061 729 510 382 369, -22 663 558 731 392 767 950},
{1 470 491 432 343 680 174 377, 20 733 318 455 405 009 610},
{366 783 471 687 593 348 389, -13 878 550 478 312 964 150},
{1 384 290 105 589 313 353 937, -25 476 265 660 529 182 890},
{1 997 220 061 531 832 345 341, -21 455 553 594 439 878 240},
{431 883 498 999 214 881 893, 5 514 584 589 414 726 780},
{406 794 938 793 822 981 349, -24 527 559 316 013 450 010},
{2 370 441 711 768 520 835 293, -84 013 339 060 097 375 640},
{4 209 894 813 990 075 947 909, -61 432 468 344 825 761 280},
{6 744 301 920 076 068 235 763, 419 924 258 951 643 780 960},
{5 944 710 005 995 883 513 899, -130 550 767 375 122 183 840},
{14 125 693 329 518 707 658 653, -500 570 764 062 371 963 190},
{25 562 881 034 944 196 614 589, -1 435 455 465 625 343 623 620},
{64 148 941 690 693 346 263 043, 4 080 307 916 318 731 618 260},
{264 684 498 104 681 793 584 261, 3 515 630 639 077 621 403 700},
{235 842 640 509 423 875 475 313, -740 201 921 666 741 414 310},
{65 652 993 028 126 115 671 441, 3 403 546 388 369 335 788 030},
{229 647 514 242 335 417 836 943, -5 319 127 288 020 677 474 520},
{215 534 519 784 984 738 791 839, 9 448 499 443 668 832 423 890},
{414 965 408 719 828 821 128 023, -10 910 444 514 797 396 880 240},

```

```

{85 864 497 703 963 345 184 399, 634 814 993 610 311 334 780},
{38 322 341 011 116 392 460 067, -114 316 402 980 949 185 360},
{6 138 620 912 130 779 920 811, 237 210 853 822 511 567 460},
{6 724 679 930 303 354 123 717, 143 542 588 034 804 427 900},
{5 084 457 808 461 779 106 839, -58 210 793 454 830 698 710},
{4 687 675 248 721 438 343 077, -284 721 466 580 062 213 890},
{30 786 705 541 623 200 555 021, 1 047 107 841 471 393 790 500},
{97 994 706 375 997 886 911 393, 4 246 587 859 749 793 789 530},
{75 302 245 208 362 732 263 299, 507 029 958 654 911 219 310},
{57 135 941 074 036 183 436 603, -433 037 381 455 395 431 550},
{5 823 433 791 711 152 023 301, -325 066 328 747 652 836 700},
{6 468 109 298 957 575 690 667, -44 688 690 012 260 875 170},
{2 737 925 407 118 531 693 039, -163 212 765 369 304 170 090},
{8 549 143 769 195 933 248 403, -497 610 036 573 286 784 580},
{20 917 143 355 863 493 156 519, -135 778 311 001 116 206 670},
{1 697 046 574 142 177 735 987, 46 711 895 188 306 470 540},
{3 592 474 935 612 737 595 451, -217 338 522 588 845 878 020},
{23 831 227 976 650 663 097 137, -1 522 897 919 596 499 174 730},
{124 687 325 696 144 421 760 519, 1 643 648 916 390 666 673 710},
{53 588 124 244 275 187 855 753, 3 416 277 718 667 006 646 450},
{249 850 386 274 482 007 575 151, 8 246 732 348 276 316 962 400},
{570 480 887 502 852 197 834 183, 11 724 292 718 232 863 781 420},
{934 203 175 900 043 697 107 501, 34 764 223 136 850 683 153 070},
{1 032 387 769 217 466 289 915 637, 8 389 303 826 079 711 796 560},
{117 291 876 051 185 172 730 381, 6 555 172 085 643 155 608 890},
{163 384 607 261 249 377 505 887, 8 319 968 002 810 566 038 040},
{702 437 401 226 132 778 394 729, -39 258 283 828 837 636 268 130},
{981 327 892 456 109 142 565 363, 49 891 515 358 672 478 194 530},
{3 845 062 629 140 318 168 780 221, -238 056 923 605 796 704 911 960},
{8 423 381 387 284 017 414 004 613, -154 930 485 367 170 255 529 350},
{13 312 496 347 439 902 392 793 129, -103 641 292 751 791 823 919 360},
{10 813 733 924 057 900 949 806 417, -478 874 853 787 540 104 535 890},
{46 690 337 141 936 498 902 939 349, -2 643 155 509 150 384 718 997 840},
{206 545 651 305 509 267 092 072 643, 4 196 437 920 445 672 601 474 730},
{214 405 016 455 415 141 415 933 409, 11 567 171 608 966 615 342 195 440},
{1 251 499 878 783 478 169 986 728 583, 44 183 513 735 559 169 016 237 490},
{3 346 228 145 762 394 944 974 375 079, -45 517 114 846 148 642 313 446 190},
{5 134 936 214 656 868 589 409 814 573, 27 078 389 902 432 273 124 331 390},
{2 320 182 965 626 349 881 663 839 791, -35 808 759 950 837 983 685 011 860},
{1 721 038 464 501 740 481 829 948 397, -77 090 474 510 475 763 993 700 880},
{5 836 189 888 206 766 034 667 265 621, 72 497 634 376 192 246 808 601 600},
{8 415 609 629 699 787 941 265 107 107, 444 929 397 454 065 771 738 537 120},
{8 865 398 809 098 581 171 733 874 309, 205 007 255 173 175 609 098 863 330},
{11 670 232 939 922 985 452 481 010 727, -316 672 730 598 864 343 405 918 350},
{10 871 335 490 753 894 074 346 595 959, -401 620 424 107 061 111 790 499 020},
{6 427 081 288 135 865 048 727 523 627, -67 663 680 547 889 196 601 271 250},
{225 628 791 870 810 415 626 113 659, -9 010 585 026 373 717 866 852 420},
{84 850 727 271 920 266 469 136 047, -1 868 933 092 455 083 310 418 020},
{174 455 979 965 873 577 575 759 251, -8 680 687 020 369 436 142 064 870},
{196 241 817 126 971 153 129 611 283, -1 225 135 382 427 258 392 672 310},
{51 296 333 696 085 800 375 712 139, -1 455 383 298 895 915 858 877 160},

```

```

{83 394 948 691 797 658 397 688 587, 4 497 196 696 847 107 292 699 160},
{478 066 731 753 289 578 117 740 549, -1 434 670 733 712 115 765 223 250},
{74 880 940 527 121 593 526 803 667, 3 168 017 557 856 740 021 196 700},
{268 295 040 715 558 906 786 691 989, -12 715 148 273 315 226 331 037 310},
{297 523 985 393 822 843 533 675 607, -12 928 233 263 002 376 493 106 740},
{40 686 540 330 986 916 787 396 771, -77 403 028 376 407 088 744 670},
{6 396 454 635 748 370 905 818 217, -83 807 090 416 997 240 260 230},
{6 317 973 025 183 290 527 491 721, -3 701 946 422 291 831 302 950},
{291 137 616 845 663 048 035 457, 386 324 876 797 109 276 340},
{35 262 280 430 261 693 702 399, 790 459 320 681 333 554 580},
{71 854 637 092 807 687 112 333, 856 378 520 239 034 003 460},
{18 909 955 494 182 418 545 531, 113 978 671 381 255 829 040},
{2 447 421 539 709 434 500 397, -87 063 564 588 938 891 640},
{2 246 523 374 060 909 533 141, -38 174 989 017 139 350 420},
{1 351 627 862 422 729 001 887, 19 276 177 015 891 940 190},
{534 844 815 298 312 940 771, 15 180 189 631 104 319 620},
{824 395 522 851 188 698 543, 34 187 756 482 169 941 170},
{906 222 576 032 655 737 879, 31 438 010 960 970 948 090},
{1 276 779 847 671 909 318 323, 72 594 924 021 140 681 880},
{6 973 406 837 109 148 635 461, 144 789 986 989 305 766 650},
{5 472 578 558 035 937 848 813, -85 877 767 851 200 586 390},
{5 498 470 174 729 625 474 251, 186 708 978 974 005 305 390},
{19 550 979 784 648 886 980 253, 709 202 014 372 711 005 960},
{71 455 651 944 375 936 484 091, 361 304 256 149 776 389 900},
{19 243 650 174 190 770 853 397, 58 697 062 486 591 584 480},
{2 093 812 888 825 643 458 019, 72 656 199 865 510 561 950},
{3 079 539 394 879 941 377 723, 120 915 815 006 100 770 640},
{13 198 056 596 489 352 031 459, -715 065 164 563 797 419 610},
{76 163 886 801 452 645 485 607, 100 470 170 544 425 255 160},
{1 746 924 205 344 383 318 191, 17 259 948 548 612 552 040},
{854 970 650 742 125 981 183, -51 468 135 485 549 362 290},
{4 657 123 035 345 670 415 051, -515 939 194 905 234 630},
{59 615 876 528 276 208 343, 2 599 990 477 949 773 290},
{42 849 740 244 478 517 191, 1 086 951 714 008 002 530},
{106 859 251 772 775 515 393, 5 603 114 353 998 588 150},
{93 218 417 904 945 346 519, -2 732 838 561 982 536 660},
{70 344 283 826 610 318 407, -2 747 110 109 820 875 880},
{251 774 913 694 661 892 209, -8 270 761 651 208 603 760},
{850 930 948 908 080 602 297, 45 027 180 806 436 204 780},
{1 068 418 334 510 298 225 859, -36 424 103 507 017 881 300},
{2 823 804 543 979 662 681 047, -124 476 480 457 195 313 190},
{9 123 000 022 848 278 701 259, -362 859 955 345 633 768 980},
{11 999 765 435 332 233 084 847, 430 510 096 734 218 480 010},
{12 702 524 661 631 054 815 889, -542 242 535 704 535 399 940},
{53 810 497 319 430 563 823 677, -1 631 486 988 716 814 860 760},
{6 657 580 816 268 093 466 899, 397 202 069 717 595 711 210},
{22 101 067 960 930 834 315 343, 1 357 742 997 523 486 722 360},
{87 882 940 129 325 894 516 839, -477 082 043 266 870 059 840},
{23 263 691 195 680 216 963 007, -333 089 354 978 831 973 030},
{12 247 331 111 258 927 738 669, 341 250 038 176 760 549 280},
{8 777 171 303 337 324 250 763, -403 706 375 835 933 619 140},

```

```

{24 317 968 857 399 181 283 861, 131 517 021 878 699 974 320},
{2 954 484 307 353 153 923 987, 169 395 991 825 841 757 210},
{17 417 319 991 125 663 980 161, -897 054 914 054 658 335 250},
{86 973 453 412 307 257 225 763, 3 753 880 754 943 305 821 020},
{147 767 679 326 415 038 756 599, -536 331 181 697 956 080 480},
{60 516 349 577 455 593 220 273, 296 290 669 620 827 928 960},
{17 021 343 129 960 100 996 889, -1 095 129 792 774 976 488 000},
{116 670 918 184 408 814 988 863, -208 871 047 587 111 962 610},
{20 503 398 111 317 901 659 591, 1 148 349 022 940 147 819 550},
{38 884 042 273 908 868 507 997, -2 219 282 793 487 485 183 840},
{247 690 186 065 746 498 661 659, 6 829 846 626 968 943 295 680},
{423 059 846 303 437 824 002 707, 11 688 743 551 613 972 947 710},
{527 763 277 763 007 907 239 251, 5 383 113 124 298 234 640 030},
{50 838 638 554 952 616 300 463, -2 518 153 096 567 422 824 370},
{110 809 353 299 769 236 443 679, -1 770 424 467 092 948 010 720},
{169 481 433 611 151 757 981 673, -2 102 331 606 641 405 560 410},
{188 130 380 744 887 531 888 121, 5 387 348 266 192 048 653 330},
{99 446 397 237 361 837 973 957, -434 944 830 284 659 644 630},
{36 340 753 193 276 410 590 929, -1 597 327 108 319 929 367 790},
{92 680 479 453 097 814 300 153, 2 250 839 022 316 215 230 940},
{92 286 532 384 986 630 765 829, 1 620 501 864 131 571 079 860},
{19 123 211 829 510 543 182 503, -857 868 688 349 652 990 690},
{58 273 459 795 635 331 246 259, 2 698 151 127 254 536 900 860},
{253 006 545 923 723 973 430 013, -9 726 160 390 553 171 483 610},
{29 445 554 256 572 961 483 649, 985 930 987 887 563 703 690},
{30 843 463 552 570 263 102 883, 611 241 116 070 008 108 970},
{65 568 005 533 276 833 471 239, -1 098 771 981 315 514 345 320},
{83 487 009 537 388 348 774 913, -1 971 737 224 384 776 072 360},
{157 052 744 382 066 620 439 769, 5 677 044 845 497 252 837 290},
{443 751 131 002 554 948 013 783, -8 638 657 619 903 198 086 380},
{740 845 026 285 600 026 757 899, -9 664 021 317 582 420 832 650},
{765 315 334 201 405 923 983 183, -14 667 499 093 296 321 736 740},
{607 053 854 549 346 125 739 799, 21 576 093 258 252 683 307 540},
{681 115 693 157 141 398 982 207, 28 483 654 929 476 960 615 730},
{580 641 860 021 217 800 307 929, 17 015 552 747 969 150 020 620},
{492 344 515 532 141 008 395 817, -29 072 065 327 250 302 140 150},
{438 178 642 249 591 820 908 789, 3 649 109 238 459 646 416 150},
{66 529 336 823 180 476 193 837, 2 207 558 291 372 231 719 620},
{70 503 023 109 151 233 020 221, -3 064 538 353 397 084 283 810},
{4 343 348 577 262 616 773 703, 98 546 469 341 373 033 480},
{1 701 814 814 433 369 035 839, -46 040 306 400 480 035 610},
{390 629 715 563 401 643 323, 14 413 355 045 168 036 040},
{342 307 137 120 468 166 619, 8 696 821 512 704 243 280},
{729 545 863 125 624 136 867, -40 165 350 041 679 257 100},
{1 530 708 033 467 619 612 611, -95 443 610 400 779 119 830},
{841 192 223 850 811 012 123, -35 218 834 186 308 634 740},
{945 932 612 598 919 641 421, 45 797 158 011 506 404 050},
{3 683 195 414 752 558 565 557, 236 579 076 792 249 960 360},
{23 782 266 644 161 706 447 299, -5 225 373 936 208 654 260},
{370 437 490 936 172 039 087, 22 579 044 237 693 387 840},
{2 137 258 470 007 135 239 751, 32 430 921 528 194 187 930},

```

```

{741 487 748 907 711 125 557, -14 233 192 844 887 986 960},
{317 280 986 833 842 247 421, -7 351 967 166 898 123 770},
{267 110 887 132 941 597 463, 6 589 635 947 125 128 090},
{713 955 500 910 956 434 891, 27 350 040 906 058 810 800},
{665 083 903 348 573 503 203, 35 708 606 502 976 834 380},
{3 117 451 508 460 819 553 961, 109 055 415 837 798 100 170},
{10 521 243 344 630 806 775 777, 328 752 085 928 492 712 720},
{274 146 616 136 312 715 721, 2 906 791 836 837 285 060},
{211 606 749 350 645 378 873, -3 855 107 222 852 641 770},
{98 826 462 156 231 005 141, -5 195 057 387 660 823 600},
{28 046 627 227 358 120 653, -711 875 037 636 651 750},
{66 055 676 970 187 659 899, 4 233 571 947 881 584 050},
{391 783 487 648 820 581 933, 22 462 253 694 201 856 950},
{2 312 565 739 441 640 211 439, -125 889 306 841 034 773 470},
{10 848 064 398 602 329 332 107, -532 223 062 100 161 740},
{55 518 351 167 307 534 929, 2 487 118 982 956 385 790},
{186 803 915 348 222 078 917, 2 250 572 596 563 653 790},
{1 488 831 191 243 742 851, -94 113 658 550 268 690},
{3 958 051 515 609 592 037, 14 806 669 095 120 960},
{1 088 312 060 464 902 061, -53 196 510 058 604 070},
{5 680 973 215 227 214 013, 39 961 395 683 788 800},
{1 504 021 554 104 628 229, 15 764 688 268 435 680},
{1 485 647 284 554 600 557, 38 756 262 699 494 910},
{3 007 867 359 893 996 641, 122 790 847 064 469 900},
{14 186 678 070 785 536 553, -615 507 200 403 652 980},
{6 992 903 529 853 697 029, -253 736 331 810 222 330},
{26 029 306 273 979 073 163, -1 204 865 537 783 431 050},
{111 312 384 840 743 515 321, -5 907 664 050 306 527 550},
{217 443 082 813 758 394 057, 4 634 514 553 073 969 520},
{88 330 575 107 334 398 239, 596 474 180 559 243 390},
{12 208 357 603 965 728 927, 652 028 815 069 699 710},
{41 984 242 589 545 776 179, -563 212 730 044 959 510},
{59 813 934 171 501 587 543, 305 362 549 120 159 620},
{8 650 231 259 579 628 641, 131 401 670 422 924 380},
{5 191 004 281 677 642 287, 128 414 691 523 625 280},
{12 679 072 630 703 043 271, 535 647 929 383 903 260},
{41 119 298 160 977 947 777, 2 257 958 101 207 718 100},
{110 920 195 042 692 120 641, -2 313 858 973 916 077 170},
{33 793 319 330 142 959 927, -403 682 717 604 710 070},
{27 034 745 036 075 827 049, 74 624 793 221 824 380},
{4 792 784 317 668 546 937, 108 869 409 347 829 780},
{589 561 382 820 531 761, 12 902 610 397 436 400},
{922 376 042 539 434 887, -37 286 626 445 701 950},
{2 280 981 134 525 530 079, -122 872 780 953 922 350},
{12 489 196 938 565 735 043, -315 561 981 193 160 790},
{31 054 778 034 442 297 781, 1 553 494 671 230 323 290},
{3 521 885 908 251 148 427, -101 817 866 482 951 710},
{9 725 284 545 953 611 559, -67 905 741 204 262 680},
{3 439 908 022 363 258 327, 122 600 342 978 980 080},
{1 653 931 615 773 148 271, 30 235 727 801 688 900},
{2 104 785 303 499 706 357, 1 137 811 604 644 920},

```



```

{38 716 466 761 184 819, -907 605 383 193 990}, {72 361 578 864 522 983, -2 817 599 863 958 520},
{208 772 100 426 859 121, 11 368 097 455 388 520},
{966 098 671 558 722 313, 36 568 582 290 095 730},
{3 568 518 959 782 366 589, -209 373 575 660 694 720},
{2 136 184 437 279 629 317, -101 041 575 487 656 570},
{3 334 545 025 050 033 851, 71 043 775 464 241 740},
{1 051 394 272 253 407 457, -37 736 007 428 105 280},
{1 214 847 025 914 909 239, 33 077 698 400 686 800},
{2 103 480 874 147 050 113, -123 739 202 538 041 160},
{19 937 576 918 358 431, 471 139 421 503 770}, {34 885 043 141 621 203, 1 976 210 266 312 890},
{160 010 804 918 520 361, -7 207 501 723 764 150},
{336 863 710 000 211 213, 12 199 483 342 554 420},
{1 100 184 896 775 823 451, -9 385 464 027 651 660},
{485 946 090 954 960 823, 3 072 699 165 355 770},
{107 092 119 098 554 979, -1 072 707 320 799 870},
{41 616 824 673 660 893, -1 903 498 072 779 900},
{60 610 972 106 779 331, -1 312 255 061 994 270},
{57 606 746 424 998 263, -1 651 145 741 884 380}, {42 721 608 042 523 621, -327 578 146 517 160},
{31 792 615 903 227 293, 1 450 219 178 409 690}, {26 144 003 076 111 671, -1 283 003 211 796 770},
{112 757 749 761 071 143, 5 941 720 962 403 320}, {31 443 006 229 921 321, 150 878 073 300 060},
{14 065 507 157 559 953, 745 410 478 874 610}, {22 669 022 266 429 421, 1 444 852 325 962 470},
{104 527 283 110 033 067, -189 380 221 681 260}, {2 469 627 119 231 549, -73 314 301 895 430},
{5 372 780 834 645 543, -212 126 568 168 060}, {16 220 674 893 462 019, 698 483 536 552 980},
{36 243 977 789 230 607, -584 566 363 808 610}, {201 133 311 551 371, -11 677 087 321 140},
{611 118 712 433 903, 33 207 100 764 930}, {3 120 079 388 982 979, 104 442 239 085 780},
{3 072 753 576 568 093, 194 235 771 196 320}, {8 159 371 679 515 291, -82 730 969 537 730},
{7 221 672 999 755 107, -250 096 071 295 680}, {7 249 344 801 969 829, 402 078 467 413 260},
{2 780 246 527 757 717, -104 290 947 541 560}, {8 296 910 016 405 899, -270 457 769 254 590},
{20 336 433 503 329 103, 174 462 286 117 950}, {17 627 375 585 753 951, 203 432 468 883 030},
{16 601 065 247 230 547, -375 288 583 771 050}, {20 589 641 783 912 851, 41 645 672 648 880},
{3 886 322 420 308 523, 196 129 368 494 370}, {8 449 733 251 878 341, -4 306 389 803 190},
{138 974 718 557 713, -1 339 351 280 790}, {74 050 812 156 151, -2 567 649 578 460},
{95 768 969 271 037, -5 945 308 426 650}, {150 060 025 600 421, 5 857 537 006 470},
{520 973 220 297 167, -23 244 181 828 110}, {2 237 084 278 348 051, 56 801 078 936 160},
{5 089 232 562 209 963, 129 331 489 438 680}, {10 555 942 465 636 219, 233 284 132 260 060},
{13 550 467 746 509 927, 269 644 858 421 310}, {15 896 384 328 551 491, -621 835 651 151 880},
{63 222 826 125 591 637, -1 637 298 036 202 020},
{147 208 767 704 904 319, 2 412 070 662 784 860}, {16 882 545 081 491 147, -980 562 537 592 050},
{49 624 792 585 327 201, 1 549 426 561 453 110}, {10 052 230 186 849 673, -87 330 769 115 340},
{2 141 675 090 438 509, 57 590 456 097 840}, {2 522 974 052 693 957, 99 872 044 129 050},
{6 098 297 225 975 731, -285 468 238 867 650}, {24 107 160 872 933 873, -1 331 647 510 461 420},
{32 038 824 518 396 929, -886 079 523 806 610}, {32 611 067 096 639 777, -712 886 849 255 700},
{42 342 616 805 524 559, 2 547 463 666 397 400}, {224 673 866 912 879 153, 13 928 245 365 087 630},
{424 512 269 654 158 009, 20 445 473 550 998 580},
{1 128 343 255 617 235 843, 30 452 830 261 380 150},
{370 128 875 457 678 269, -5 246 228 479 634 760},
{548 329 756 958 798 003, 22 164 471 596 156 670},
{1 347 213 676 212 668 051, 39 507 768 702 368 190},
{920 242 897 390 854 703, -36 614 269 578 254 670},
{1 138 474 798 735 693 049, -29 210 005 724 299 890},
{166 693 911 296 620 013, 2 244 224 616 568 260},

```

```

{144 760 493 242 524 109, 1 021 012 382 635 260}, {52 020 766 362 094 963, 3 230 413 863 420 300},
{77 855 679 537 247 979, 861 198 594 063 150}, {81 038 814 674 523 607, 2 409 811 624 960 920},
{208 483 873 776 407 809, 2 225 653 097 139 630}, {169 511 543 649 156 763, 5 235 323 763 002 130},
{461 615 693 309 644 499, -28 315 000 066 323 600},
{1 998 136 293 892 787 467, 91 644 938 350 782 420},
{4 206 197 509 091 205 109, -232 021 341 154 149 450},
{6 946 514 817 747 997 097, -396 909 519 189 805 650},
{46 100 570 946 761 572 499, -2 491 215 309 657 492 990},
{287 177 145 258 275 074 463, -11 156 402 480 585 402 610},
{673 211 382 208 276 661 501, -945 535 274 455 249 170},
{2 267 836 499 554 176 587, 144 647 617 963 724 430},
{10 840 415 372 641 530 269, -204 615 722 449 501 230},
{982 774 703 414 136 593, -29 179 998 081 169 920},
{2 177 438 903 534 280 071, 70 372 984 051 296 720},
{960 799 279 028 952 017, 56 266 919 161 677 750},
{992 965 214 340 252 211, -58 316 471 858 609 280},
{369 349 909 327 407 083, 13 215 799 558 427 340},
{161 347 445 894 115 821, -4 677 607 114 109 940},
{537 951 335 350 041 613, 18 343 469 313 757 260},
{1 395 838 983 501 890 009, -39 293 830 672 930 980},
{4 366 168 528 604 688 143, 160 780 599 452 788 260},
{5 846 516 007 401 393 659, -176 635 396 608 019 920},
{4 088 665 205 459 557 667, -93 916 161 705 701 700},
{10 169 496 934 776 891 989, -376 948 214 143 241 730},
{1 888 429 372 117 889 993, 53 439 903 801 294 660},
{4 201 628 203 910 416 069, 8 907 625 623 599 610},
{645 664 069 863 765 283, 2 841 051 151 179 120},
{173 691 841 242 475 019, -8 947 773 269 803 740},
{858 406 744 075 522 447, 15 133 824 371 985 210},
{983 550 114 738 843 859, 19 664 828 540 445 390},
{71 924 237 961 825 647, -2 107 541 205 455 280}, {62 406 015 488 647 591, -915 434 157 667 830},
{36 462 814 765 790 183, -2 030 922 969 150 540}, {21 855 092 188 252 121, 459 710 057 609 340},
{49 160 804 440 114 367, 492 750 845 085 270}, {26 627 255 940 143 489, -1 673 679 176 361 240},
{35 325 335 421 269 783, -1 188 826 529 616 660}, {79 094 288 864 593 961, 2 033 602 944 368 010},
{50 380 650 021 713 957, -294 621 026 786 820}, {105 884 792 082 721, -3 360 854 655 210},
{387 375 753 971 767, -14 948 169 655 590}, {297 461 098 142 509, -2 350 281 101 820},
{238 732 216 751 023, -5 669 469 136 680}, {143 181 531 437 879, 6 361 793 753 640},
{731 555 900 730 953, 24 770 005 405 560}, {2 689 812 914 552 351, 116 162 072 786 490},
{4 213 861 027 897 873, -62 097 735 369 330}, {2 046 899 691 460 111, -26 440 066 281 660},
{2 566 398 950 943 803, 117 779 586 579 090}, {5 767 205 234 509 241, 32 025 040 828 500},
{628 607 293 363 153, 15 670 866 335 340}, {413 025 108 245 849, -18 052 839 440 490},
{510 316 340 303 093, 1 129 729 625 850}, {74 897 985 397 931, -2 852 032 126 380},
{173 619 976 107 883, 6 111 615 399 360}, {581 275 567 712 099, 2 001 780 343 170},
{176 909 488 922 167, 10 853 904 279 210}, {756 555 765 970 031, -3 716 257 693 530},
{363 667 217 850 737, 23 054 147 144 430}, {1 211 398 795 213 319, -68 497 095 306 330},
{5 020 898 430 044 693, -201 867 019 090 860}, {6 006 052 003 846 031, -136 980 976 886 430},
{4 918 858 143 555 137, 250 098 879 204 690}, {19 366 829 645 508 479, -920 624 883 015 300},
{7 853 754 809 612 707, -128 427 832 106 460}, {4 580 092 910 644 751, 151 603 330 724 730},
{7 454 366 414 364 283, -188 641 623 302 520}, {21 272 554 632 608 461, 130 209 715 959 000},
{11 270 426 990 910 413, -134 822 895 173 430}, {12 744 215 452 245 731, 236 898 490 516 200},
{11 254 607 301 573 077, -131 887 673 135 940}, {10 288 134 809 235 241, -262 819 178 131 890},

```

```

{8 897 538 867 326 723, -519 757 779 196 080}, {14 365 992 691 453 579, -873 151 615 628 790},
{92 167 074 044 554 787, -1 705 237 331 109 180},
{19 632 152 365 562 611, -464 342 604 233 370}, {30 234 776 148 329 543, 809 082 932 924 430},
{69 598 877 819 272 489, 330 516 392 243 400}, {32 638 859 971 784 263, -1 366 609 586 860 260},
{37 226 436 296 840 641, 2 075 210 271 726 120}, {29 672 222 455 477 927, 1 674 150 702 281 430},
{107 760 213 241 960 429, -1 585 357 737 810 270}, {10 278 312 489 137 923, 163 136 025 310 440},
{173 094 437 187 299, -10 650 717 457 020}, {625 129 184 870 107, 13 533 656 244 810},
{601 372 442 861 351, -21 285 153 841 080}, {1 255 435 527 488 863, 51 524 994 361 590},
{4 388 709 434 893 799, 138 856 115 507 580}, {12 741 898 894 261 313, 458 281 895 990 460},
{20 968 647 078 875 111, 1 213 350 400 103 220}, {79 613 834 569 046 443, -4 309 189 557 061 380},
{477 282 452 272 393 499, -20 798 346 663 332 100},
{251 528 389 329 038 633, -11 829 656 545 225 200},
{723 605 237 879 097 889, 38 731 716 341 018 100},
{2 865 287 815 857 320 563, -170 381 635 280 089 380},
{7 269 596 249 678 343 001, 386 941 300 970 215 320},
{19 173 213 220 089 302 407, 1 182 877 192 820 198 130},
{57 592 505 447 108 832 191, 1 242 656 114 699 281 320},
{100 265 531 829 460 712 743, 5 524 921 903 284 176 700},
{190 346 453 890 508 989 319, -11 623 933 384 182 936 270},
{1 016 700 100 254 608 096 767, 40 640 959 942 041 518 460},
{157 531 696 931 841 517 211, -2 841 200 521 921 289 490},
{294 900 696 697 748 695 813, -16 508 926 260 656 868 060},
{526 574 406 619 458 519 211, -17 979 131 135 078 788 590},
{1 206 847 662 606 460 473 533, 6 341 444 287 298 840 340},
{459 766 788 585 628 481 389, -2 379 495 819 976 900 530},
{122 114 211 910 196 230 067, -4 122 429 463 604 769 540},
{363 170 575 521 617 478 989, -21 437 293 686 608 060 970},
{294 376 196 117 656 897 733, -8 242 487 869 769 497 950},
{548 334 556 212 491 632 811, 14 272 246 479 819 964 080},
{1 395 481 265 184 588 480 643, -88 404 858 421 757 098 830},
{4 426 177 408 301 348 448 421, 82 144 883 662 295 339 430},
{2 247 590 104 785 772 226 167, -40 065 157 367 050 105 170},
{918 321 089 815 156 438 751, 5 680 920 867 543 348 780},
{463 225 139 359 792 820 897, -11 514 682 405 998 283 800},
{614 617 446 927 722 253 001, 7 678 981 661 098 149 540},
{69 646 971 289 777 523 633, -4 281 512 185 869 963 180},
{266 266 881 594 940 271 449, -3 376 944 511 143 325 830},
{119 234 204 994 115 305 193, 3 873 849 461 217 163 260},
{199 244 894 742 704 117 011, -4 722 205 666 005 379 230},
{212 555 827 521 418 118 783, -5 565 795 605 426 139 390},
{245 953 522 047 383 517 379, 1 550 877 662 240 536 620},
{148 194 115 984 800 611 833, 1 180 466 549 183 932 110},
{126 907 926 483 336 328 291, 2 732 592 351 309 172 140},
{281 622 049 285 657 495 283, -15 992 276 626 744 210 920},
{1 453 670 689 007 024 197 541, -17 157 543 411 579 621 840},
{1 099 876 727 697 772 514 147, 32 486 794 013 378 447 160},
{1 089 104 620 403 062 605 269, 2 892 381 376 218 466 380},
{308 295 914 492 718 257 903, 885 939 303 699 528 870},
{2 554 424 369 244 803 681, 122 730 721 151 839 170},
{5 340 540 561 909 801 137, 283 918 400 833 273 530},
{12 560 809 563 918 252 389, 155 148 930 394 265 100},

```

```

{1 457 134 938 012 425 663, 59 789 737 844 148 390},
{5 168 226 532 417 382 599, -43 165 826 617 936 020},
{2 719 730 184 240 973 633, -97 578 107 418 534 210},
{2 902 439 870 370 329 551, -60 287 936 192 701 080},
{2 008 211 417 117 906 663, -84 417 477 401 459 820},
{4 149 273 440 491 060 961, -97 652 739 473 070 810},
{11 151 003 150 946 257 253, 218 935 361 376 232 950},
{3 425 165 063 298 204 901, 145 032 560 186 448 210},
{12 958 616 814 136 648 387, -422 757 817 511 149 530},
{34 221 998 189 193 981 019, 1 564 722 532 166 392 110},
{47 042 121 802 728 378 433, -1 164 816 754 807 639 830},
{104 722 225 228 508 959 289, -1 731 337 616 508 940 590},
{196 178 599 447 598 066 137, 743 089 580 228 309 250},
{687 412 286 590 823 921, 18 185 595 987 696 090},
{848 204 099 399 207 267, 21 978 436 570 984 860},
{2 086 497 960 524 129 609, -16 667 405 594 176 770},
{715 836 871 723 772 647, -12 456 325 881 155 070},
{1 357 527 084 018 542 081, 69 087 283 637 033 760},
{5 642 931 172 257 016 727, -113 068 530 821 007 540},
{2 445 420 928 852 943 609, -103 361 677 973 131 140},
{8 215 426 803 013 473 983, -245 675 358 781 032 570},
{25 196 611 434 780 007 309, 1 153 221 553 294 964 610},
{40 603 217 886 246 887 863, -2 078 633 222 629 164 300},
{225 881 049 956 380 765 921, -10 096 207 958 967 767 970},
{877 122 642 167 939 845 373, 19 202 706 787 128 529 020},
{1 445 035 719 313 590 064 451, -8 884 252 620 754 787 820},
{721 707 683 579 601 598 697, 25 708 666 805 234 424 120},
{434 548 036 697 789 537 521, 3 427 529 568 528 908 190},
{174 334 911 753 960 007 897, 9 461 596 345 111 209 450},
{938 099 367 276 269 406 701, 30 416 075 753 463 391 470},
{1 118 162 591 895 304 826 477, -32 443 461 346 248 775 080},
{3 514 783 126 623 228 385 381, 133 975 628 975 737 022 430},
{7 320 108 168 197 331 912 833, 113 716 029 821 582 047 200},
{9 851 766 490 546 847 843 689, -141 988 609 702 344 983 190},
{12 710 714 112 815 252 833 907, -351 893 409 619 978 935 870},
{9 914 468 393 570 596 222 771, -292 540 769 113 698 290 670},
{7 436 837 216 768 938 782 097, 177 178 294 831 445 906 940},
{1 083 721 713 366 909 086 239, 19 812 732 162 171 004 020},
{1 393 003 443 731 599 422 613, 46 906 737 161 141 254 920},
{3 308 290 366 914 706 421 971, 145 693 701 511 903 093 500},
{9 940 890 911 162 081 747 257, 611 829 513 569 009 322 990},
{35 327 155 715 498 291 004 161, 1 550 891 187 701 873 398 860},
{79 998 593 183 237 740 521 227, -848 965 007 499 473 834 430},
{45 640 617 440 917 619 760 031, 1 991 281 105 566 683 080 950},
{37 011 580 998 049 226 723 827, -1 720 855 089 212 051 568 060},
{197 404 814 755 506 511 223 869, -5 711 627 229 227 715 918 660},
{582 998 216 319 006 201 510 823, -20 345 520 020 256 992 736 960},
{1 636 094 374 548 054 971 616 961, -104 580 180 508 266 316 390 050},
{8 664 923 665 120 019 115 354 487, -177 236 907 149 968 092 852 090},
{4 586 554 958 221 262 214 716 059, -41 849 613 734 046 601 101 330},
{3 938 294 738 060 290 198 246 153, 116 505 061 430 431 391 372 520},

```

```

{5 330 422 683 829 866 261 749 791, 307 141 375 962 015 913 635 240},
{25 401 495 146 813 805 078 515 663, -388 792 434 743 473 890 458 340},
{30 286 945 017 704 512 302 590 179, -897 684 238 507 899 357 534 750},
{54 596 348 334 427 343 886 777 793, -1 726 754 835 318 717 926 592 150},
{153 734 890 214 789 735 051 844 631, 6 450 039 166 283 418 393 366 750},
{248 389 597 810 867 388 627 066 977, 271 058 433 315 522 775 437 540},
{23 316 984 266 706 634 023 318 521, 110 691 837 945 221 120 334 510},
{9 085 494 758 260 211 572 299 737, -55 462 016 121 758 644 302 090},
{2 394 281 370 012 019 725 624 359, -24 966 235 969 913 363 822 010},
{577 206 962 221 525 900 244 033, 20 290 527 777 922 755 201 990},
{2 113 818 974 447 479 819 076 929, 100 878 908 014 737 122 024 040},
{1 080 675 869 845 940 218 703 263, 10 350 312 904 949 747 907 450},
{988 695 361 361 779 664 531 879, -7 073 899 911 577 444 788 060},
{384 595 918 361 587 150 589 393, 14 098 682 925 564 897 062 190},
{916 034 693 521 038 669 091 279, -17 449 550 264 720 109 130 650},
{2 017 332 583 053 167 671 312 607, 90 133 071 004 851 835 348 470},
{8 016 369 880 517 559 419 580 211, 357 992 976 274 101 448 433 310},
{32 742 185 779 547 320 093 042 103, -902 278 020 530 894 943 473 370},
{60 621 250 421 378 795 824 182 439, 512 623 968 734 201 851 339 020},
{30 667 951 803 113 726 319 492 407, 981 485 046 389 401 801 720 560},
{56 366 280 054 849 018 614 125 951, -3 552 734 631 849 027 707 954 640},
{111 251 454 753 353 958 163 551 337, -3 017 686 018 815 544 924 591 740},
{93 882 210 677 340 542 797 929 019, 2 026 221 875 126 926 792 980 600},
{157 509 030 209 945 104 751 390 627, 5 666 646 068 255 821 397 700 690},
{269 594 910 383 769 391 525 285 469, -1 280 474 515 206 787 643 550 750},
{136 354 471 693 032 694 494 007 973, -107 723 636 847 123 653 293 560},
{5 511 045 414 223 184 123 883 971, 264 424 188 236 706 796 463 130},
{9 753 971 528 204 454 229 129 847, -72 903 900 094 538 868 523 560},
{3 530 202 680 054 717 655 335 969, 168 904 967 260 446 505 805 250},
{3 914 780 352 615 539 211 807 473, -39 037 521 382 054 068 805 710},
{2 569 573 957 560 833 178 098 209, -162 888 809 811 409 730 187 300},
{8 538 750 865 261 343 641 371 703, -526 256 706 750 163 009 879 650},
{27 643 948 841 285 367 608 271 599, -1 601 384 268 877 788 338 709 390},
{97 956 990 994 571 043 099 388 777, 5 252 108 678 144 582 271 484 230},
{427 106 216 411 012 673 703 101 169, -13 912 554 491 514 430 440 174 210},
{974 632 668 442 778 096 555 746 453, -21 093 607 706 180 262 432 895 050},
{1 008 124 352 327 243 741 719 777 649, 17 643 317 134 066 945 669 987 770},
{572 079 234 704 686 377 600 618 847, -13 970 259 281 170 390 090 444 710},
{163 425 226 828 810 553 074 123 279, -6 420 165 830 514 009 332 705 520},
{680 611 888 368 754 503 261 070 007, -6 147 294 870 001 098 712 893 870},
{404 917 232 918 616 751 744 848 179, 24 667 521 602 618 365 283 125 680},
{2 385 194 735 476 437 381 057 090 667, -87 493 214 321 978 001 488 976 990},
{5 330 562 066 446 302 419 147 881 321, 204 234 967 707 332 422 309 104 630},
{4 765 527 110 968 649 312 900 499 253, -273 052 694 434 633 122 095 223 150},
{28 806 094 200 113 493 286 637 428 799, -569 311 957 527 536 434 517 085 420},
{53 314 042 673 271 515 580 005 135 693, 2 224 774 843 123 011 214 142 158 890},
{18 768 979 871 615 579 341 755 896 411, 1 197 934 393 198 845 277 947 930 780},
{92 727 107 758 865 209 560 762 084 077, -4 519 124 114 828 827 028 280 584 130},
{506 658 186 041 856 821 719 332 558 149, 9 196 565 535 840 841 686 888 428 850},
{197 370 005 952 253 243 129 270 335 967, 8 154 211 912 383 183 063 195 996 570},
{388 858 372 828 245 959 727 975 460 871, -2 637 487 179 526 904 601 049 646 370},

```

```

{267 427 483 005 299 126 066 844 564 073, 5 254 503 577 362 249 741 252 415 530},
{128 662 469 560 917 301 727 670 313 981, 1 583 423 664 451 646 491 741 246 050},
{94 400 588 497 807 063 914 646 455 923, 4 300 247 516 691 325 609 264 791 750},
{47 731 650 570 689 180 978 698 280 441, -207 580 012 812 364 873 569 476 220},
{2 738 303 644 054 406 551 531 287 047, 63 876 989 299 852 765 749 805 770},
{1 958 806 730 548 133 540 514 127 679, -3 132 871 371 289 412 365 662 900},
{177 574 773 694 439 190 131 936 707, 1 679 523 050 346 414 623 116 140},
{105 938 026 651 417 060 981 172 989, 4 233 718 053 546 521 799 435 090},
{22 152 547 871 685 726 903 907 187, -425 439 910 346 451 901 394 850},
{6 913 700 345 163 131 310 371 971, -317 961 988 863 948 546 293 340},
{18 980 974 493 590 652 982 991 597, 768 074 545 936 974 012 990 120},
{51 467 173 076 251 480 630 406 899, -41 153 788 020 098 199 961 530},
{3 778 266 695 688 632 501 841 523, -140 609 526 137 632 289 242 110},
{4 238 388 836 393 358 693 039 151, 19 101 540 677 569 541 607 030},
{501 694 208 309 533 687 111 597, 6 452 658 180 952 309 085 640},
{375 859 244 505 916 225 419 259, -3 258 637 747 715 958 413 730},
{260 005 519 829 374 826 791 997, 10 710 832 603 077 099 414 120},
{686 310 203 837 194 718 776 261, 21 372 617 876 433 846 871 680},
{556 038 607 375 607 199 622 733, -31 686 796 545 313 332 150 660},
{3 337 429 192 527 637 527 771 251, 77 921 070 641 289 055 638 810},
{3 070 204 896 135 504 474 535 907, 28 436 706 532 423 318 816 290},
{223 542 382 327 852 126 255 229, -5 827 995 178 325 682 645 870},
{484 305 773 493 951 270 935 377, 13 930 387 424 398 513 543 830},
{759 064 221 879 231 821 990 809, -20 571 773 488 117 588 026 120},
{487 295 543 200 711 849 322 023, 24 837 649 780 226 265 647 280},
{2 203 586 410 088 537 024 293 441, -112 700 956 504 641 721 670 040},
{11 750 823 761 001 296 322 014 647, 538 635 663 389 842 504 366 230},
{23 104 474 223 030 634 351 882 229, -559 459 265 032 448 223 891 210},
{38 828 135 111 159 921 155 830 227, -371 410 526 359 841 739 409 110},
{39 603 046 493 266 525 335 433 259, -146 127 236 122 230 602 102 100},
{597 762 465 093 494 623 049 047, -29 061 093 133 212 257 040 960},
{2 917 274 334 023 326 530 989 329, 10 169 719 898 557 492 542 660},
{334 419 509 003 002 099 703 203, -1 337 912 952 078 318 189 630},
{13 683 860 862 545 315 101 201, -117 360 191 999 171 633 280},
{11 016 613 116 359 476 266 247, 394 411 961 880 374 795 610},
{6 272 783 195 807 196 524 089, 174 624 597 154 269 671 730},
{3 192 636 306 937 216 358 503, 8 305 050 194 791 314 180},
{814 808 488 002 949 218 239, 46 679 341 216 450 977 120},
{4 953 507 146 324 847 477 367, 33 845 968 558 947 997 470},
{2 795 006 655 396 484 292 051, -31 075 559 935 415 442 510},
{417 941 138 280 989 386 817, -24 036 638 215 613 983 620},
{2 171 161 247 423 538 009 541, -9 563 534 907 059 017 260},
{55 645 880 425 874 324 393, -80 181 098 367 130 650},
{46 171 066 957 217 269, 2 224 266 707 555 520},
{125 478 399 037 535 683, -1 261 597 469 731 200},
{135 198 141 456 223 739, 1 975 051 967 540 730}, {208 443 585 584 805 067, 3 937 200 075 399 600},
{53 128 289 850 079 789, -733 603 845 700 140}, {71 953 419 603 042 197, -4 170 697 826 489 760},
{245 012 676 782 892 541, 6 175 000 454 023 530},
{463 050 541 085 337 547, -7 889 313 592 448 010},
{563 617 882 499 145 019, 23 989 415 219 104 080},
{2 763 690 463 122 024 707, -103 905 834 629 315 280},

```

```

{9 731 727 745 590 669 749, 402 828 503 022 384 030},
{14 875 575 821 454 555 757, 8 841 815 639 526 360},
{848 566 374 693 849 221, -15 748 945 584 753 210},
{437 268 043 698 019 727, 9 964 899 740 465 880},
{276 697 957 617 605 369, -6 109 118 694 513 690},
{416 514 612 926 011 327, 24 544 599 414 658 620},
{173 253 469 702 154 629, -8 219 357 553 022 620},
{150 741 933 662 348 897, 6 364 123 524 168 270},
{465 308 203 821 672 839, 14 932 407 135 980 340},
{560 034 747 263 775 667, 18 091 909 636 908 660},
{189 767 194 931 520 769, 11 588 237 838 877 890},
{1 014 805 755 707 565 257, -43 835 974 510 404 900},
{1 532 753 678 602 845 781, 48 431 409 549 647 220},
{3 972 982 487 706 605 347, -30 576 614 396 731 320},
{460 730 441 352 636 949, 5 769 227 959 886 760},
{188 216 337 124 797 283, -11 367 641 452 260 930},
{1 172 821 242 327 776 791, -69 466 025 988 007 890},
{1 887 579 476 127 259 987, -97 826 876 192 413 020},
{6 726 437 033 839 137 431, -275 975 945 130 400 200},
{24 002 343 715 321 103 023, 596 645 731 622 310 930},
{31 807 866 949 879 136 759, -226 283 969 240 692 770},
{22 874 242 142 640 707 963, -289 100 218 532 242 530},
{8 230 696 712 296 705 669, 463 415 981 599 829 070},
{25 814 292 864 550 698 703, -1 616 605 472 551 285 950},
{11 974 964 230 881 223 801, 459 898 408 953 668 310},
{4 102 104 354 002 523 653, -61 763 056 608 026 460},
{5 998 029 964 357 109 269, 282 499 997 812 891 830},
{15 268 492 396 726 735 487, 947 789 306 886 765 780},
{24 200 192 363 466 540 631, -394 317 822 352 378 170},
{34 205 611 593 353 036 813, 611 223 373 923 410 820},
{5 335 081 701 406 801 931, -222 525 241 166 566 590},
{1 287 112 175 655 521 357, -22 791 895 766 574 840},
{2 508 480 965 467 963 861, -142 825 604 493 385 560},
{14 534 520 291 223 459 027, -406 788 476 048 322 780},
{25 598 509 238 265 525 349, -800 701 549 800 908 370},
{5 578 102 799 705 400 403, -171 310 732 019 779 590},
{17 510 266 168 726 973 611, -666 332 190 947 431 710},
{43 251 604 553 843 552 183, 673 130 947 997 698 410},
{39 895 164 503 868 968 719, -2 398 699 368 030 437 460},
{205 674 867 367 093 067 533, 2 780 358 582 557 024 550},
{16 698 583 915 532 555 911, -663 838 331 241 742 140},
{23 911 772 835 937 561 763, -735 879 445 822 302 120},
{84 725 922 722 367 284 059, 3 082 762 542 872 689 080},
{347 480 837 099 490 183 467, 2 443 321 383 090 684 120},
{123 303 763 242 837 953 491, -2 242 874 401 952 101 200},
{12 658 625 434 933 714 597, -597 229 746 068 882 070},
{27 214 578 824 515 532 591, 1 006 390 150 579 830 090},
{9 796 428 814 407 997 513, -120 849 354 370 087 410},
{1 778 048 730 403 731 599, 897 921 854 481 540},
{38 085 837 555 798 967, -1 645 711 970 095 890},
{54 629 702 757 284 801, 3 411 812 896 927 680}, {9 482 262 700 967 593, 151 587 173 432 310},

```

```

{15 780 909 487 429 321, - 777 906 523 080 360}, {51 907 513 016 554 193, - 801 208 961 805 870},
{39 859 193 692 774 181, 1 926 627 207 222 150}, {139 794 794 521 595 777, 1 079 104 885 465 800},
{113 899 857 227 265 959, - 2 122 737 944 837 670},
{169 622 087 994 595 493, - 7 716 396 690 895 380},
{32 302 934 788 968 011, 1 156 330 845 467 220}, {17 318 629 998 596 717, 388 762 340 498 610},
{40 932 350 454 890 789, - 987 210 177 402 300}, {106 418 831 265 381 937, 2 913 951 177 473 490},
{325 585 416 164 965 969, - 8 216 719 805 470 530},
{718 426 620 548 268 823, - 28 031 199 254 162 040},
{2 419 602 493 967 002 561, - 11 003 411 545 101 390},
{267 494 707 585 654 687, 15 132 869 235 433 290},
{1 140 986 705 949 676 189, - 162 702 311 892 810}, {10 393 513 621 879 453, 439 460 806 738 290},
{35 776 157 382 605 131, - 1 054 179 675 946 950}, {15 366 722 704 742 377, 283 914 016 490 670},
{8 240 234 719 363 901, 371 551 344 399 690}, {15 402 498 218 977 993, - 687 324 948 223 950},
{65 554 400 425 904 669, 222 421 152 942 660}, {13 942 648 277 947 223, 236 403 560 987 190},
{1 202 704 129 197 971, 46 211 061 805 890}, {283 449 683 045 623, 955 534 018 020},
{80 133 431 371 861, 4 347 975 970 560}, {435 678 289 114 973, 3 351 894 178 740},
{15 833 310 245 891, - 198 490 748 190}, {10 706 258 968 997, - 620 257 166 910},
{37 719 701 645 791, 1 178 498 484 270}, {1 805 784 752 183, 2 362 414 980},
{209 631 838 879, 10 618 212 540}, {636 651 977 593, - 14 872 792 920},
{670 601 486 311, 11 619 189 960}, {771 586 808 977, - 24 930 851 790},
{295 815 987 529, - 18 559 527 600}, {264 793 798 543, - 5 520 079 710},
{39 616 416 121, 770 392 710}, {76 048 383 263, 3 252 029 490}, {291 647 263 369, 6 699 875 370},
{733 309 928 263, 44 028 023 400}, {3 533 787 402 121, 206 334 528 330},
{6 081 397 979 063, 312 175 565 760}, {34 964 499 502 159, 707 036 603 040},
{74 491 487 095 367, 1 689 492 376 830}, {35 840 645 959 351, 1 404 310 941 540},
{156 445 175 320 537, - 4 913 959 448 100}, {186 755 795 348 479, - 9 246 355 467 420},
{426 083 838 018 407, - 14 838 203 816 430}, {984 208 929 328 679, 35 802 636 197 160},
{4 086 296 217 248 647, - 76 106 728 634 040}, {5 467 841 054 556 529, 132 521 029 596 570},
{8 033 569 975 638 047, - 153 557 091 442 290}, {11 324 084 408 879 311, 672 113 173 171 680},
{23 728 611 664 145 017, - 787 880 738 950 470}, {21 480 152 482 003 661, - 1 041 010 826 243 850},
{88 790 444 504 305 037, 2 478 354 970 987 980}, {100 267 927 144 102 619, 3 494 800 963 828 710},
{251 943 088 014 683 243, - 3 313 019 374 611 180},
{35 792 421 806 420 179, 2 288 828 652 752 580},
{193 118 936 565 716 533, - 11 129 994 390 057 510},
{910 804 440 794 155 079, - 13 327 615 955 750 250},
{1 054 687 502 131 172 407, 17 988 986 475 466 260},
{1 552 409 081 671 505 389, 6 067 101 658 629 210},
{179 163 704 454 362 443, - 6 469 110 703 167 000},
{459 335 089 595 058 781, 28 756 368 102 743 250},
{178 664 411 378 140 027, - 6 069 341 625 175 380},
{618 266 489 796 583 631, 18 735 695 283 300 240}, {2 668 910 691 559 337, 141 980 824 067 760},
{6 692 917 014 647 999, - 335 071 077 750 660}, {1 981 557 905 091 833, - 119 436 641 400},
{3 591 083 507 111, 86 461 425 600}, {9 389 053 764 737, 405 635 560 590},
{13 848 557 981 911, 10 050 461 940}, {228 007 138 297, 6 813 749 580},
{734 742 702 581, - 20 631 447 930}, {1 861 535 535 467, 13 473 628 290},
{506 735 727 151, 7 598 107 890}, {544 637 844 607, - 17 233 029 120},
{1 588 847 325 289, - 76 156 554 840}, {2 432 596 039 783, - 108 480 782 490},
{10 722 386 225 699, - 425 856 818 550}, {17 700 022 534 117, 1 050 167 050 530},
{35 606 436 700 069, - 1 709 376 193 620}, {67 677 964 266 583, - 2 554 791 898 920},
{292 036 350 456 479, 6 353 436 989 880}, {51 668 001 174 233, 3 163 893 184 650},
{243 650 481 221 089, 15 647 060 338 680}, {1 561 678 818 085 303, - 26 423 592 105 300},

```



```

{626 043 942 316 499, -30 601 731 000 060}, {3 264 172 099 464 667, 14 551 057 788 510},
{1 103 291 077 353 491, -18 915 018 944 610}, {1 449 255 005 903 863, 71 185 153 505 790},
{5 953 601 038 618 679, -278 136 853 272 510}, {26 265 418 935 760 777, -551 428 471 792 500},
{47 333 416 495 058 959, 499 776 451 742 010}, {33 865 715 960 653 903, 1 282 687 294 024 380},
{120 192 191 632 665 359, 4 833 739 376 267 430}, {151 751 216 346 751 103, 6 988 152 125 169 150},
{463 234 384 824 055 901, -17 853 815 518 552 380},
{224 802 747 385 293 107, -8 077 588 059 124 740},
{319 144 356 956 509 829, -8 133 195 099 401 520},
{454 291 302 605 177 917, -23 276 301 504 027 120},
{2 617 691 501 759 924 539, 30 709 062 263 367 120},
{1 729 141 784 076 605 987, 30 850 508 593 973 520},
{352 599 555 682 706 011, 15 113 163 614 600 580},
{1 164 252 663 425 992 343, 73 580 264 845 992 150},
{3 036 356 767 602 519 281, 57 476 115 928 144 290},
{2 301 428 745 266 844 737, -57 476 615 934 699 420},
{550 837 135 776 229 321, 12 440 160 396 237 930},
{808 528 253 630 173 433, -16 308 434 755 299 150},
{1 606 181 803 404 687 611, 77 383 865 201 305 770},
{4 398 892 236 696 919 247, 93 750 597 919 972 230},
{1 720 906 671 233 706 179, 92 131 343 719 892 520},
{6 894 204 250 510 646 333, -162 624 286 873 732 440},
{14 908 319 022 634 937 749, 499 062 246 750 653 280},
{14 806 772 513 125 931 683, 12 031 696 026 777 090},
{989 153 929 943 202 931, -1 489 922 039 431 350}, {35 952 887 736 738 277, -32 703 042 800 700},
{2 852 781 813 171 641, 93 721 251 892 410}, {9 586 611 741 046 453, -380 846 764 712 610},
{15 248 131 212 870 299, -389 754 815 914 080}, {11 112 560 387 534 707, -672 360 809 952 330},
{73 994 597 925 592 399, 4 224 845 524 539 450}, {478 260 813 255 424 333, 869 320 518 804 630},
{31 345 003 700 535 089, 759 811 564 729 290}, {44 905 984 365 768 367, -2 202 383 787 880 500},
{199 985 905 700 899 511, 1 829 742 318 863 700}, {126 750 356 128 197 163, 2 015 463 385 397 520},
{52 154 056 380 257 101, 455 050 080 231 540}, {41 171 763 204 209 767, -4 960 871 949 420},
{346 446 761 752 571, 3 895 694 871 000}, {62 929 051 577 957, -222 169 741 560},
{12 818 428 939 141, -601 863 459 870}, {41 776 033 675 943, -383 086 290 330},
{4 573 330 983 709, 244 711 029 990}, {17 749 610 561 533, 116 269 588 080},
{9 235 284 626 731, 258 312 125 190}, {14 900 788 065 397, -711 476 667 900},
{9 371 716 797 199, 461 805 953 370}, {31 594 271 043 167, 1 834 557 891 990},
{94 781 342 885 521, 325 765 529 820}, {3 827 326 059 067, -13 898 950 680},
{1 191 706 941 611, -16 243 606 230}, {1 380 219 029 293, -52 837 554 360},
{1 501 129 512 389, 58 672 425 480}, {5 674 377 171 203, 210 848 415 030},
{4 317 498 063 431, -208 389 339 510}, {13 671 989 443 007, -734 859 568 530},
{67 649 769 661 679, -2 983 135 970 310}, {224 229 333 720 083, 2 173 169 157 510},
{91 548 145 696 849, -506 126 853 540}, {14 169 846 976 603, -661 291 212 630},
{65 876 442 149 909, -1 405 836 401 370}, {46 103 410 474 073, 1 076 502 625 560},
{43 385 165 026 631, 548 162 003 970}, {18 725 444 129 233, -61 326 746 580},
{4 843 236 403 589, 53 499 456 630}, {5 874 896 889 653, -362 581 519 110},
{17 147 072 047 069, -585 948 314 610}, {36 015 025 147 307, -2 049 253 964 400},
{203 070 267 371 069, 6 841 219 282 980}, {504 750 490 571 123, 30 729 245 813 910},
{3 048 235 908 815 179, 95 333 198 417 010}, {565 360 643 289 853, -10 704 389 523 180},
{459 476 335 214 071, 9 400 946 155 320}, {272 616 150 409 897, -14 171 356 496 820},
{782 967 834 083 861, 24 847 136 854 770}, {2 828 747 047 625 507, 38 078 841 852 510},
{2 542 670 875 765 711, 33 042 214 423 560}, {368 054 919 679 297, -21 810 597 421 740},
{634 980 102 235 939, 12 929 327 339 040}, {336 233 591 154 107, -17 898 238 259 580},

```

```

{893 074 036 253 729, 30 718 874 336 100}, {518 816 558 091 157, 9 853 293 390 210},
{794 062 040 463 709, -46 542 910 536 750}, {659 986 791 977 447, 32 537 386 539 810},
{2 152 701 255 230 551, 97 571 506 965 660}, {1 427 847 762 745 223, -62 378 265 036 540},
{1 596 593 611 180 901, -61 333 739 255 790}, {446 518 993 574 113, 24 676 015 197 600},
{547 717 764 033 929, -33 259 701 549 180}, {3 626 071 644 562 417, 187 384 555 036 050},
{15 323 268 038 449 811, 255 636 064 271 430}, {3 470 725 555 785 437, -128 889 809 647 080},
{2 166 737 991 773 459, -98 421 533 972 880}, {341 168 938 233 067, -2 150 579 930 700},
{180 172 084 338 289, -9 273 569 980 680}, {926 001 346 350 977, -14 644 264 599 180},
{795 153 648 414 421, -33 563 814 998 310}, {2 418 053 389 989 427, 36 935 235 841 980},
{4 022 293 040 749 391, -198 250 781 789 430}, {13 345 635 355 864 303, 202 265 861 303 520},
{911 377 209 147 961, 44 625 742 564 860}, {4 394 929 379 227 313, 212 124 778 201 440},
{13 907 994 379 681 991, 715 335 601 523 160}, {73 771 982 522 874 583, -4 300 498 245 757 260},
{154 598 376 385 270 979, -6 747 573 759 697 080},
{138 826 080 448 513 613, -780 345 681 893 400}, {17 580 066 343 199 771, 738 315 453 353 400},
{32 504 557 186 666 157, -436 919 774 692 530}, {40 191 069 244 612 321, 1 694 008 148 002 710},
{108 374 429 636 483 527, -3 997 800 224 347 470},
{101 080 893 930 728 021, 5 571 478 587 007 410},
{185 067 091 950 551 353, 11 421 940 129 408 110},
{539 639 622 045 031 169, 21 015 186 927 473 610},
{1 573 970 470 142 867 003, -32 767 144 217 813 610},
{267 378 611 260 597 459, 7 922 998 088 824 050},
{466 774 435 944 916 153, 17 032 541 564 820 480},
{1 606 724 590 879 823 969, 37 968 378 588 151 830},
{2 808 276 811 345 176 397, 168 695 283 277 457 910},
{13 873 520 018 584 681 009, -7 618 118 386 364 850},
{215 859 824 329 374 047, 3 737 483 412 175 230}, {213 011 763 391 905 269, 6 811 398 680 892 690},
{433 008 198 226 027 807, 25 996 293 893 218 410},
{2 080 409 924 373 642 979, 103 734 114 372 872 940},
{1 334 539 401 470 913 707, -57 855 506 579 682 150},
{900 020 782 206 251 881, -37 962 552 045 526 590},
{2 581 748 784 528 003 007, -129 903 551 365 190 520},
{3 803 082 566 763 122 569, -91 844 094 912 359 820},
{8 731 599 358 034 198 117, -39 109 161 448 967 130},
{2 389 730 695 085 053 591, 118 284 805 465 973 010},
{5 600 058 483 383 260 103, 160 931 900 795 245 590},
{7 586 024 356 928 182 451, -380 962 211 909 698 890},
{7 740 232 334 930 316 317, 67 112 395 286 259 540},
{5 197 502 343 439 327 561, 245 442 964 474 713 090},
{10 065 620 846 592 172 343, 164 092 621 742 624 250},
{13 041 224 428 057 690 669, -386 354 135 512 783 920},
{22 092 169 794 832 288 363, -1 003 018 627 405 453 200},
{6 002 078 115 570 085 379, -317 813 459 869 850 820},
{8 475 985 915 999 686 833, -159 812 642 768 368 980},
{1 378 392 881 338 498 069, 33 504 674 594 653 560},
{1 095 384 949 144 591 397, 49 571 300 345 799 630},
{1 122 207 578 120 892 121, -9 106 708 227 575 010},
{485 214 608 095 652 603, 2 252 434 724 231 490},
{219 286 175 910 564 949, -11 633 869 206 947 040},
{409 459 991 992 912 963, 21 962 822 432 579 490},
{1 825 236 774 680 681 851, 52 860 962 433 227 850},
{5 800 980 142 374 245 467, -366 087 215 441 497 530},

```

```

{13 144 765 992 703 598 029, 675 364 163 296 404 990},
{72 893 325 386 753 450 027, -2 192 063 888 608 279 020},
{129 365 575 604 496 471 511, 5 600 982 246 896 389 650},
{126 515 254 729 925 727 713, 1 867 441 416 035 842 050},
{109 687 443 599 186 883 071, 2 694 401 339 373 271 260},
{182 441 636 422 316 591 237, 6 443 653 170 991 053 510},
{470 507 998 854 132 658 981, -13 139 537 084 404 249 920},
{586 073 330 969 938 786 387, -32 351 366 170 825 679 610},
{873 456 395 552 836 943 831, -2 901 128 698 511 001 060},
{50 481 151 138 970 571 643, 7 792 446 886 038 540},
{391 489 212 607 918 859, 1 012 014 504 694 980}, {37 373 365 205 947 433, -10 337 307 480 870},
{931 688 386 355 239, -9 395 081 612 910}, {367 046 455 775 717, -15 130 801 342 410},
{910 383 088 985 341, -8 975 510 692 230}, {898 566 613 335 863, -8 779 093 429 650},
{722 086 458 194 179, -133 651 476 870}, {7 565 820 922 423, -31 686 943 050},
{1 714 522 700 791, 98 175 868 920}, {10 609 172 492 183, -346 816 408 650},
{33 117 729 000 311, -209 397 085 740}, {7 686 542 640 103, -295 024 492 650},
{3 706 058 670 299, -27 515 990 490}, {2 003 810 683 283, -38 808 604 080},
{3 317 157 828 341, 73 265 558 130}, {4 708 397 010 403, 96 396 551 850},
{3 502 929 047 551, 90 648 789 450}, {7 543 081 652 767, 245 501 117 490},
{15 716 546 535 559, -541 249 259 850}, {4 734 093 978 797, 63 701 889 840},
{4 695 912 438 421, -273 057 645 030}, {12 566 266 188 263, -521 437 986 120},
{12 058 803 482 239, -389 470 729 740}, {3 445 869 550 333, -206 529 131 730},
{15 174 285 554 941, -722 979 114 660}, {1 928 273 730 127, 123 285 343 320},
{10 319 980 777 369, 507 078 581 820}, {41 569 329 845 777, 399 276 524 520},
{10 385 111 897 401, -568 290 750 540}, {36 319 664 329 673, -1 473 899 223 780},
{122 981 189 704 691, -4 940 215 645 080}, {122 138 931 397 997, 3 069 130 446 930},
{145 924 749 654 299, -1 140 807 843 270}, {22 986 448 232 813, -558 340 022 790},
{22 020 200 532 559, 326 846 513 670}, {28 305 799 183 877, -379 755 816 360},
{40 981 681 047 659, -1 219 286 780 850}, {110 458 193 789 153, -347 880 806 550},
{39 121 327 643 051, 462 934 927 590}, {53 156 900 089 067, 1 643 938 879 050},
{128 349 438 555 811, 2 947 146 786 420}, {308 729 670 873 877, -10 924 977 434 670},
{659 460 529 826 261, 1 752 690 527 190}, {104 591 743 457 293, 4 374 450 296 370},
{92 049 831 751 771, 17 312 360 250}, {2 866 487 393, 152 377 980},
{6 685 754 891, -210 170 130}, {9 247 599 677, 151 839 420}, {3 402 951 719, 111 426 630},
{11 946 797 963, 187 238 820}, {8 501 358 461, 157 175 340}, {3 236 393 533, -48 012 420},
{4 557 804 569, -36 899 850}, {4 142 001 623, 64 786 170}, {1 004 988 881, 44 354 460},
{3 533 141 867, 128 363 130}, {14 219 005 109, -616 238 250}, {10 607 408 647, -178 631 400},
{15 880 358 951, -727 488 000}, {28 979 852 417, 1 595 687 850}, {59 990 770 261, 1 036 860 570},
{34 284 272 167, 1 197 105 540}, {100 606 718 869, 6 054 814 560},
{541 754 975 683, -15 694 601 880}, {1 760 568 997 261, 29 918 981 880},
{1 083 667 542 547, 5 277 710 460}, {404 697 291 551, -20 860 200 660},
{1 946 360 609 563, -98 943 717 510}, {7 575 701 568 421, -356 007 078 810},
{23 195 828 824 763, 674 797 902 510}, {58 879 132 485 559, -1 973 176 551 660},
{73 666 226 968 153, 4 473 884 029 740}, {485 591 220 708 929, -20 467 092 150 210},
{1 309 224 878 793 863, 48 880 118 265 690}, {2 455 427 250 485 711, -7 688 025 757 410},
{686 658 892 157 593, -23 089 678 323 930}, {1 405 329 611 551 531, -48 416 754 800 610},
{289 787 303 784 953, -12 979 523 942 670}, {987 402 051 767 629, 26 970 394 631 250},
{2 447 094 054 148 693, 17 427 804 091 350}, {1 677 945 156 808 469, -44 166 021 740 460},
{84 734 953 659 563, 2 477 747 805 990}, {114 526 083 625 399, 2 227 179 389 160},
{219 004 803 329 687, 11 368 017 425 220}, {701 906 034 368 131, 27 897 202 135 170},
{1 042 903 570 409 273, 54 635 473 505 970}, {1 125 290 694 431 419, -20 009 494 134 510},

```

```

{1 108 852 335 434 147, 49 220 536 529 580}, {5 410 261 105 862 969, -322 782 733 219 500},
{17 951 568 616 367 723, -1 066 528 439 702 190}, {41 803 662 046 695 131, 908 621 624 690 610},
{1 646 683 446 007 543, -98 469 931 405 740}, {6 362 155 378 378 621, 6 968 189 906 340},
{46 132 576 416 833, 2 018 287 431 030}, {67 112 037 767 681, -3 645 086 521 650},
{349 611 928 069 573, 5 968 655 904 720}, {591 533 481 975 331, -19 760 858 989 980},
{301 103 039 708 077, -9 187 030 260 990}, {482 067 424 770 169, 30 239 968 125 810},
{412 891 201 570 303, 24 627 745 422 360}, {1 346 849 652 087 361, -15 598 779 691 050},
{1 247 621 487 095 213, 60 157 405 357 440}, {3 654 377 920 769 291, 98 947 421 640 780},
{1 555 666 425 919 577, -20 203 450 788 690}, {166 639 374 151, 944 102 640},
{108 762 799 057, 4 084 786 800}, {355 661 578 519, 9 904 737 690},
{211 791 948 793, 10 090 836 780}, {26 940 295 771, 618 789 840},
{66 744 525 037, 1 915 133 670}, {66 440 745 229, -1 386 820 830},
{29 510 524 363, 159 995 340}, {16 631 960 099, 874 194 690}, {5 186 810 437, -686 580},
{70 240 879, -2 816 880}, {42 201 193, -1 136 190}, {37 783 979, -2 028 210},
{175 218 563, -1 194 000}, {69 768 821, -274 410}, {16 002 673, -64 200},
{3 931 409, 227 100}, {16 475 197, -117 450}, {7 501 901, -320 370},
{31 080 103, 1 386 660}, {133 644 839, -3 850 530}, {261 824 663, -13 032 420},
{274 069 279, -1 795 320}, {143 220 673, -5 820 330}, {533 005 441, -16 409 310},
{1 842 452 393, -27 759 150}, {2 411 198 869, 51 668 640}, {4 013 940 163, -152 017 530},
{14 325 861 239, -373 986 180}, {26 652 030 967, -1 348 980 690},
{76 326 800 089, -167 018 910}, {196 134 973, -129 600}, {11 690 309, -93 000},
{6 452 003, 70 020}, {2 367 979, -149 400}, {5 224 093, -166 560}, {14 150 789, -546 690},
{14 714 183, 445 260}, {4 800 499, -93 540}, {6 980 447, -224 340}, {6 036 331, -198 150},
{21 396 623, 664 860}, {28 216 999, -1 310 490}, {143 010 973, -7 684 140},
{696 131 071, -2 207 580}, {173 205 443, -1 440 150}, {90 274 219, 1 520 460},
{132 129 407, -2 992 590}, {106 119 151, -439 560}, {43 149 503, -2 414 340},
{71 907 761, -2 227 890}, {143 360 473, -2 262 330}, {194 248 139, -1 902 600},
{42 624 787, 1 235 970}, {140 221 031, -886 350}, {41 411 323, 1 425 720},
{15 248 219, 396 750}, {40 010 527, -285 510}, {9 116 591, 383 340},
{19 471 577, 936 300}, {44 438 459, -733 680}, {73 632 893, 296 100},
{22 369 631, 133 740}, {8 166 883, -384 480}, {21 623 099, -492 960},
{15 643 853, 48 570}, {1 004 929, 59 880}, {3 036 223, 121 440}, {51 959, -3 180},
{251 407, 3570}, {351 131, 18 030}, {1 994 713, 91 710}, {5 337 331, -64 920},
{3 236 603, -124 080}, {2 451 859, 132 840}, {14 152 187, -25 170}, {1 548 751, -81 720},
{915 457, -54 180}, {1 305 499, 17 190}, {219 253, 3390}, {255 601, -30}, {1, 0}

30
--- is a relation number with a list {{239, 240}, {1, 0}}
239

30
--- is a relation number with a list {{241, 240}, {1, 0}}
241

30
--- is a relation number with a list {{247, 240}, {1729, 60}, {2717, 30}, {1, 0}}
247

30
--- is a relation number with a list
251
{{251, 240}, {2761, -150}, {15 311, 780}, {72 539, 3630}, {15 311, 210},
{4769, -270}, {22 841, -480}, {49 949, 1080}, {67 519, -3300}, {381 269, -8040},
{850 639, 15 360}, {1 465 589, 1620}, {128 261, 7290}, {742 709, 34 380},
{3 426 401, -29 250}, {1 041 901, 5520}, {346 129, -20 310}, {215 609, 4650},
{428 959, -12 060}, {1 305 451, 62 490}, {1 716 589, -92 070}, {8 217 991, -463 950},
{33 410 359, 646 620}, {53 684 131, -1 890 870}, {185 682 521, -8 552 640},
{621 365 309, -7 023 690}, {823 427 839, 8 571 870}, {132 608 069, -4 002 150},

```

```

{134816869, -5498310}, {662861131, 33226500}, {418886119, 21182190},
{1194177931, -35703780}, {4004250941, 131670090}, {13591208491, 560247990},
{36459439481, 1175783730}, {2546106601, -64347870}, {6979857949, 300641940},
{16338425579, -698067990}, {70998314059, 2987874180},
{178377231511, -3756845130}, {453183110651, -22157823120},
{2516688711001, -147223547580}, {3485988937391, 128923273890},
{1270196132611, 22876059600}, {2726664452239, 124239734460},
{1659036176131, -52458649950}, {4929796189519, 204310439910},
{6612753551429, -92061356640}, {3931695789401, 81134339670},
{9349118795491, 251077227030}, {14874610240631, 795918834480},
{62209751236739, 980940281610}, {103038887322559, -92086501290},
{1482812858701, 73990114890}, {755650786151, -33747530790},
{3314482301521, -151411702560}, {4160363854549, 212984400840},
{24930364725001, 175963004700}, {14151867542149, -188799108480},
{2024464056601, -37115615400}, {4240592390149, 192832649940},
{433203041281, 10739159610}, {912800877131, -31963598640},
{3550014340679, -38922295890}, {2029439086939, -66998641590},
{4889439648989, 130801098840}, {12499546969159, -36258851100},
{2448921745591, 27277508970}, {1519569488959, 54975596790},
{4956552511411, -173292193200}, {17299193938639, 76052918130},
{8830562305379, 91259960970}, {5435131086461, -169646056920},
{1620773520271, 36788851680}, {518075634101, 7714582710},
{300846725281, -5359640010}, {177428064971, -9257519820},
{385332286141, -20854888320}, {2496018391631, 135343077420},
{15020592515821, -139396468050}, {8590734428329, 77959229970},
{3820002038879, -64913078940}, {2477274263831, 8312155290},
{63248840161, -104785290}, {10410224749, 171858420}, {18357856621, 746859180},
{78719342629, 712073220}, {80516982541, 4116952650}, {457339685209, 5225046480},
{618565662781, 19292050260}, {306233669711, 10888949700},
{337112605861, -6752971740}, {134531265889, 6655318890},
{357646910339, 3365977260}, {214183515529, 72721050}, {5025843029, 232032450},
{19796588621, 913008300}, {72688088729, -3281779680},
{122722878019, -2314607760}, {12215351489, 114315900}, {4128902561, -70619760},
{8272076731, 70939980}, {7003133179, -228349710}, {19002665581, 534903960},
{63723121729, 2832674700}, {352473860579, -5180598090},
{48490805209, -2090236110}, {104259044429, -1277168070},
{117653065061, -2859559020}, {103197455491, -2356594680},
{123670317679, 252749880}, {18982216109, -85921680}, {1625267921, 4022250},
{70009171, -2898480}, {111858401, -5563860}, {145881451, -1646460},
{164025739, 1563390}, {32682961, -1777890}, {170916191, 3170670},
{75297239, -3867210}, {456882499, 12264750}, {774773999, 22570740},
{1849578589, -82438680}, {9017834879, -213360150}, {14233853329, -814419180},
{97570544519, 5493511080}, {329476385171, -583614030},
{66650986529, 3094560870}, {358767505361, -4884368430},
{554361102721, 32931207540}, {1372825790209, -61594904040},
{4452213233579, -28346757810}, {444836609659, 9438573870},
{307133080019, -17011608180}, {231957327529, -420214200}, {228628621, -5097600},
{191608129, -2979120}, {237056699, -11088900}, {1051639549, -18046560},
{1239706319, 63647610}, {7630833979, -441383550}, {31955720879, -24413820},
{494344751, -16974300}, {524602801, 3154740}, {229906211, -5046330},
{558467219, -1603500}, {112753969, 1818600}, {193019, 5580}, {572531, -31980},

```

```

{780359, 5760}, {692509, 38670}, {891301, -11940}, {1053949, -26340},
{87599, -4770}, {436489, 2640}, {223139, -4110}, {300949, 11520}, {358679, 19230},
{1679441, -9210}, {808471, 7410}, {196031, 8940}, {162899, -4890},
{383779, 11100}, {1184971, 46500}, {5640221, 211290}, {16216859, -700500},
{26445109, 1177620}, {134904719, 5349360}, {293850469, 8069700},
{838658519, 20733300}, {2340956269, -112057530}, {3075217111, -175358880},
{20391924979, 144005220}, {14260881511, -351065790}, {33336785629, 459033150},
{43331214571, -1278668790}, {36024596539, -1983783960},
{79437800009, -4212769920}, {151811946221, 5003710380},
{426859340071, -19544810370}, {784748505319, 28426015230},
{2806160201371, -91579516500}, {8234007342379, 351139652490},
{39606629112359, -1807288237140}, {38581738284971, 1715759642400},
{209591564194921, 4792332635190}, {319039010113189, 17353391868750},
{1676167075397939, -51749914898490}, {5062619460211009, -282255492377820},
{4512830050027501, 187076409111390}, {5772054069889391, 43866724511250},
{4606744964497859, 1591505041650}, {166194900801641, -2189118119550},
{44697147323909, -787070044260}, {41627144926661, -1459657583940},
{176434176907349, 7882299693450}, {758919496513699, -17107986900390},
{1548186297031289, -38134413385980}, {3846487600266641, -82792870270350},
{9541907525465791, -252603809365710}, {14316344838228439, 92230372173420},
{5179924988433089, 242585418872130}, {21493429221708109, -765518188313850},
{14788907178997559, 523167702634080}, {35193087816073069, 918393484867410},
{73827983168983739, 1091159634758490}, {93088870642988831, 4272927620804760},
{229799790693688139, -1326525604404630},
{78026144053474399, 2772095516558790}, {102274867046898029, -977023950100800},
{78474576135178721, 1367794800243420}, {128078402847249031, 6536630800602960},
{666207504367352419, 31459962879063510},
{1392619260661695959, 73370373748561320},
{355877980803249371, 1785076099990470}, {162607063191606091, 1046636546977680},
{94978000926488441, 1610870346070890}, {15900722415211319, 474795061307520},
{58353833407852909, 606010435976430}, {44384720083022879, -1734832650513300},
{180953136411053171, 2885697085085700},
{212290767285828179, 11518587574447530}, {1244003927388932389,
66136642095925800}, {3160660380848110561, 21502446350934720},
{50007417562613029, 100873370313390}, {6469302319931161, 197155751466000},
{9246207090156589, 244502285266650}, {11264817244003861, 563981365104030},
{3717324577261489, 172933153280700}, {21517817950064039, -315241293606690},
{20433906187088869, -971979278524950}, {5607675854294669, 612759153030},
{74274473208641, -2886287106120}, {193016879170229, 9295921690650},
{551566559688671, -25926194261100}, {1786236531598321, -102642574522200},
{10369503944951171, 263755569108030}, {20842224184238251, -1057119441665280},
{75341326915904599, 4193735169391650}, {36622439419420351, -2103368872576950},
{217157314988662451, -8844435649493850},
{992347638419633549, -33585113726809080}, {3816649119544351601,
218745917724099540}, {24590098076899514671, -936830045006885430},
{58361743586843866241, 2022903558175117890}, {75917359658872694819,
383335292093725530}, {4259927903075009629, -13085550751005900},
{1496372079981356521, 65186691929044560}, {733380431053758109,
29631235019309430}, {1857511551673387891, -111000005158802340},
{7401622542589224139, 436662790445130570}, {5432868639476883301,
137257136709670500}, {14411624056394111449, -1443968165276100},

```

```

{156 172 507 887 305 401, 7 781 310 297 990 030}, {137 121 783 803 705 051, 2 811 003 603 357 960},
{154 965 582 969 582 239, -1 734 157 090 960 500}, {157 026 070 398 532 489,
-3 608 136 703 645 590}, {434 718 085 030 241 221, 22 350 586 059 572 880},
{2 524 294 424 487 481 751, -122 464 341 110 412 690}, {11 911 641 446 627 369 489,
-582 898 009 868 342 550}, {63 673 993 564 390 140 739, -1 709 088 398 458 441 320},
{109 868 428 178 380 786 649, 4 364 405 200 465 008 690}, {190 332 839 855 647 919 149,
3 516 345 188 697 246 630}, {113 000 116 165 146 883 379, 4 713 293 669 636 702 580},
{29 851 908 439 628 613 791, 1 525 074 015 613 920 780}, {163 042 540 035 100 254 059,
6 949 545 670 786 969 620}, {803 950 391 356 988 152 549, 14 721 575 587 554 863 160},
{1 439 802 755 590 859 634 001, -81 267 918 602 798 265 030},
{5 777 964 594 136 793 271 289, -319 553 764 255 858 362 570},
{6 525 206 220 367 029 002 279, 122 233 143 628 633 134 540},
{11 759 251 620 417 690 786 409, -240 222 261 865 178 525 400},
{2 921 441 954 990 296 505 941, -111 717 237 575 803 135 890},
{4 215 238 282 873 158 173 051, 172 520 441 090 567 197 290},
{18 761 671 871 585 904 960 841, 696 443 594 991 466 807 920},
{10 618 603 489 108 412 102 749, 336 157 437 655 082 627 940},
{34 747 063 479 412 229 824 081, -1 314 807 338 886 544 814 340},
{141 080 239 758 878 227 461 491, 7 226 958 956 716 042 345 260},
{868 193 783 236 097 480 370 959, -49 907 616 659 990 712 368 670},
{4 960 839 304 080 097 895 995 819, -75 302 771 416 785 639 287 700},
{2 295 045 966 366 328 545 087 631, -26 275 889 838 199 313 015 970},
{2 269 931 161 190 066 487 258 491, -83 892 030 436 442 424 274 950},
{1 216 431 190 936 378 990 545 091, 24 676 777 079 439 988 545 900},
{1 824 547 624 998 707 500 793 741, 87 815 250 131 013 616 388 460},
{4 912 729 565 897 189 284 343 669, 271 167 855 055 007 721 364 200},
{7 958 751 901 669 625 246 805 319, -426 526 180 421 709 479 814 840},
{36 456 627 112 056 572 288 836 891, -1 876 073 471 292 072 823 955 910},
{203 619 020 534 304 347 052 324 851, -8 492 681 515 212 757 618 410 840},
{51 539 293 531 260 783 173 362 559, 277 136 595 346 666 844 613 420},
{2 036 414 008 031 731 108 123 811, 49 998 189 150 976 215 984 960},
{3 391 448 536 731 730 562 146 799, 16 379 380 318 154 739 155 610},
{230 119 529 298 588 790 817 779, 13 079 854 419 820 026 243 480},
{1 334 780 414 801 092 072 780 111, 67 202 203 273 332 798 748 950},
{2 325 176 317 056 539 451 921 139, 84 727 696 375 408 537 980 420},
{9 419 657 245 047 740 538 899 549, -124 601 714 462 545 043 300 010},
{12 568 336 580 526 370 727 203 961, -270 993 756 481 327 829 460 420},
{25 758 569 378 707 933 578 184 891, -287 736 502 521 507 658 302 360},
{34 566 677 905 166 672 925 904 759, 1 986 779 536 743 031 029 862 770},
{198 647 870 914 321 499 977 654 919, 83 421 985 359 175 005 823 800},
{5 051 067 305 578 588 907 966 869, -191 044 506 948 740 284 701 150},
{21 061 441 352 746 717 939 979 219, -123 400 044 669 153 189 916 320},
{10 031 537 705 297 861 463 586 751, -200 291 617 255 027 185 974 460},
{4 256 167 479 172 043 380 801 501, 88 626 432 099 605 965 751 010},
{526 783 336 130 213 213 008 271, 19 594 896 766 205 269 011 120},
{571 998 015 889 591 623 284 219, 4 054 275 513 226 108 861 920},
{86 637 299 702 278 712 128 249, 2 827 691 171 548 489 054 860},
{256 302 780 546 836 591 675 161, -5 173 119 208 801 237 806 270},
{590 648 153 199 549 958 223 089, 27 735 779 067 449 424 670 710},
{2 057 394 988 561 122 074 682 929, 76 374 608 115 691 876 277 850},
{1 184 577 071 202 204 789 574 271, -56 332 858 676 392 428 705 300},

```

```

{398346788488910477505721, 969944082840453041310},
{75357619187446340644939, -270022395218510490720},
{5364101291960347248809, 183909112639541136900},
{7714993378827223955959, 55649152043407298400},
{5079927556804020931891, -3196070485771966110},
{344260283004062558351, -20427391879697126040},
{754350116647934666579, -11922644044500566550},
{809109002944142456179, 5310260121403549920},
{489315587191519953089, -12255208181688123990},
{224077759077256634261, -3896008613553341460},
{474575867718129775169, 13620502494931792770},
{537571620725225917031, -13411955099954853480},
{274447598484976235581, 12256956439525274310},
{1203433760670470391011, 55925272606117372380},
{6757481402692062138599, -306902725438441779390},
{1410982204632090996769, 37400080313533953600},
{2565432667832009247781, 117967813748270875230},
{7494667892117451827029, -49278967165482476520},
{1070485623992964393239, 41788667039700721470},
{4020949478852845610231, 84059138942999798490},
{3486186793197324039539, 151617454358468031180},
{254678918907610077851, -6341764950065788680},
{253088547149611193401, 11447236449350776410},
{313585661237422207631, -12731210808354721200},
{1178346851832901414619, -43746277400582413410},
{703462133688760610201, -34051644951141716520},
{2917224981589074616469, -169844831175006692730},
{7495575755104170854809, 371453699176929809730},
{16691944662959239712459, -532619414050888652460},
{45366449672804563035949, 1869647609495562881790},
{124221668272674522120239, -5829213131225434740150},
{453856321752038536849339, 1503442784133867664440},
{46033163153763950696791, 2271907908659686115430},
{149346250123127325435941, -955896273838037690430},
{56834282502754877944111, -2176990120229444993880},
{58367383574116333910981, -2282378490609731903340},
{244588752615910589540609, -1179730789897463777060},
{791833028901757748190401, 27240948464806568826630},
{463226379014180306750881, 27496636131288090580740},
{1058325239647025513546449, 55462440280123915037610},
{1139257455492453085796609, 32117076817451508951570},
{3805101487294218395406409, -124887834910818398651790},
{14675076432386275399029959, 225031021004457298863570},
{12063076841234294197375159, 252507769154143724202540},
{14381315619315745651037011, 219196705020991650067170},
{21502394929495516602448459, -1048218356355854527248000},
{128057829048334545909644791, 2905624916830966761882090},
{52793509650774105095040581, -2645968922016528945847290},
{31593066178674929298209969, -449009432033014251886530},
{40763890027346848204370119, -641271349173727578039420},
{69646556262700914328343011, 2797606372727051700820650},

```



```

{73 694 366 924 319 926 235 482 989, 2 448 133 586 417 684 309 790 450},
{62 840 192 279 138 632 384 141 739, -1 402 426 011 077 714 995 539 990},
{67 513 533 058 994 146 204 610 561, -3 042 320 772 769 524 127 773 030},
{146 201 490 574 218 463 794 579 151, 5 245 882 680 141 763 486 118 790},
{171 489 341 907 479 368 003 489 219, -4 925 570 793 828 106 861 635 810},
{227 314 605 002 597 410 594 796 881, -13 459 240 325 178 749 923 912 470},
{374 612 611 885 775 866 040 492 359, 20 188 139 376 855 479 543 034 720},
{2 249 471 104 894 039 564 568 997 571, 41 137 692 861 874 442 683 658 250},
{3 288 602 629 772 750 541 083 750 929, -105 998 951 267 754 348 477 401 130},
{661 420 258 563 800 309 363 290 649, 35 533 407 411 272 586 606 055 260},
{3 442 335 044 845 087 874 091 582 041, 132 673 025 020 612 622 041 261 800},
{1 798 065 028 400 915 044 287 414 509, 9 837 182 233 622 130 338 417 550},
{536 969 408 335 636 718 392 282 391, -30 307 539 433 474 001 926 064 310},
{2 150 141 668 190 724 385 495 672 439, -102 478 922 403 810 165 745 528 290},
{480 841 274 611 562 885 265 834 401, -24 829 244 689 087 353 939 388 650},
{2 280 492 005 244 693 264 779 962 801, 36 941 191 082 254 849 253 984 040},
{2 475 322 305 631 954 630 728 967 429, -100 726 036 396 095 423 395 652 570},
{10 749 979 671 878 169 494 749 052 071, -414 927 426 838 621 225 099 297 530},
{9 571 489 907 421 571 816 003 610 959, 42 531 358 562 090 616 697 154 460},
{485 491 968 746 947 845 108 222 209, -1 583 851 445 741 683 107 404 220},
{188 356 699 032 966 085 083 206 081, -7 682 838 823 226 727 073 139 520},
{932 282 158 473 225 028 065 761 669, 34 114 055 301 841 705 264 240 830},
{2 811 868 996 198 245 468 746 074 009, 160 628 888 138 028 572 880 004 080},
{19 942 198 561 853 479 616 593 857 181, 202 154 123 351 938 185 058 685 730},
{17 835 972 147 088 576 758 223 552 339, 422 263 030 312 022 585 811 545 850},
{25 332 143 369 890 666 688 795 286 389, 16 902 925 508 107 193 140 037 400},
{1 340 833 657 265 972 858 314 828 961, -75 900 228 162 559 543 943 942 820},
{6 367 982 864 684 832 101 711 591 549, 23 120 023 728 246 022 823 298 570},
{2 504 061 193 711 132 151 425 684 549, 116 612 487 999 531 305 091 605 640},
{13 854 935 375 964 660 869 993 493 359, -537 696 201 444 004 453 068 683 220},
{31 416 631 256 443 182 357 859 860 611, -217 383 943 366 184 855 412 501 660},
{26 114 173 445 059 040 915 172 902 339, 1 502 698 641 565 343 462 569 071 270},
{142 642 431 150 498 714 926 171 377 999, 2 101 643 657 087 855 115 700 994 430},
{67 603 720 400 333 668 315 557 053 491, -2 304 371 551 957 398 123 275 281 980},
{195 013 293 785 849 807 884 042 893 821, 4 311 785 635 535 126 488 311 276 270},
{246 717 986 879 048 093 418 900 879 421, -8 805 412 794 401 911 573 232 111 040},
{41 773 587 584 436 911 468 844 345 551, 1 677 958 314 947 101 178 267 429 250},
{44 017 942 599 395 114 948 187 810 449, -278 842 874 239 224 925 799 064 150},
{9 847 114 131 008 255 344 145 638 001, 549 752 621 756 165 701 709 407 380},
{12 156 698 211 284 548 942 547 404 589, 46 314 656 975 175 748 469 038 770},
{5 586 779 030 914 213 758 470 959 099, 273 356 168 632 662 599 512 838 280},
{30 033 570 223 501 403 821 762 568 249, 408 673 118 050 104 595 632 113 850},
{50 308 584 066 785 853 495 182 556 949, 356 323 650 254 399 788 349 404 860},
{16 804 294 609 786 317 817 034 393 939, -944 428 022 048 159 311 536 160 290},
{49 047 856 557 217 997 444 739 311 531, 2 559 689 037 428 238 455 786 695 590},
{103 854 976 366 448 162 982 815 925 571, -2 991 211 492 600 331 873 208 107 670},
{210 193 894 515 426 597 446 428 562 629, -2 889 202 464 424 021 345 823 565 930},
{180 189 232 269 267 160 471 629 315 511, -7 053 276 707 070 656 863 870 217 790},
{802 186 490 757 049 415 238 083 104 279, 44 552 911 606 979 158 773 397 269 630},
{58 754 539 687 563 886 549 994 985 689, 3 032 544 514 911 395 438 409 830 490},
{285 184 669 966 090 678 272 259 801 129, 11 280 696 439 493 929 703 451 242 850},

```

```

{794982003664351357180661199629, -19078274555215761814594935750},
{1582687441332370397113851569621, 59501172326176941218752470000},
{5984897080076160963908745215129, 87058975006007703346155868770},
{5565221029931012310978442230251, 98670658478927766364509639720},
{9955702932875406036041503888681, -222082441755289219026596166810},
{9539743474264813858986228060019, -127517904957371652650080251120},
{6048948782053082532217484269231, 195789394060966319046321376200},
{5151130893055212912838076635219, 110703299193513643721477699400},
{13032966429022013859915184381831, 252523183989380144451725204340},
{24658023744864166545206087206099, 1454512179662993781804294651000},
{17239510661088664112197387086151, -374184145687110803522876016690},
{6787029829873354686417669921161, 178838428388870820672427881090},
{2216442674837861282781979625009, -118069583662525376410327640460},
{6746733102280338122575631476481, -200684873340295126820315785950},
{19214700413713743518091416700569, -152807042785408116070199967090},
{9785731289167455795198567345521, -242539736064878552621169503700},
{21119603489650736278298586577771, -295344220218659654626763213580},
{36440271889282472561919564797239, 89412567576557348851518614190},
{10053976170184368144507477862531, 389184251451794053285809438480},
{16268406258131587471815452025199, -463695770984445989386862134980},
{9802622692670438662094602525649, -396445699441748808528812209950},
{27238468136693669332551383498351, -1415537277272891606171667786480},
{86158226995690932637713584362981, 5123005338669462905091718586070},
{234148804184174123960253531652459, 1477651126077524228950243184850},
{170661492245249242314892219985909, 3730250125798856964352478471490},
{233433398916042689375769215360381, 12321030752628508175753400339630},
{167212531358640456849893164239839, 5183316220436178371965095291720},
{337949488475369985699538841104549, 8456558834041782233528609614680},
{78529086461627214042991414145401, -1372338221648650530096200910900},
{76757764741187590704498518249351, 4164029891901280304930506839240},
{453111898428100849153098180900781, 16192291297430583560401985121570},
{68336732888828125077508028297929, 3267909679952166410695131980190},
{72631967932009756319525564801311, -4220829396011646291402060335670},
{220344918152754110788325312825171, -5986338624799980313270230347970},
{288552352176135361470975722479469, -14915478770817200897809448288610},
{1294722138182744647561647453965629, -29841189436965448280903923408230},
{2899299090700823242177465600346489, 133516430853717660127088516282010},
{9553659408322285435238921222290481, -398346513843338553820088250558540},
{1670887903377803967242394569734229, -68591510455065332405619560425830},
{619760476651523336638804998091559, -179228929418565673618177202010120},
{1892734854677586772096665137922891, -258196596679142070275765653044480},
{198282442882265713340888884638601, -819784515682379646941481716725170},
{38507394023831947310145248491864771, 1345568365209277815680461468585680},
{129036230376514445491621658377107199, 1560794708963435692372675484160660},
{127942347330129960802912108865122831, 5830292661736881956575763893187520},
{81346898248442002680428893035654859, 4729805112975984048259698871751250},
{235993043290418738863517066186785859, 2514810265626932495529024796216410},
{100179541306741844769027429046726931, 3386092163175932398125581664803880},
{352209120722567920859745245244756719, -7974979835482727085508459432092480},
{328811998293310203440630588404587349, 2592242125567020518112938556813990},
{101090665079051992287864686008134631, 1804905478949672688077885718485730},

```

```

{4 005 522 725 450 760 631 274 529 006 371 501, 135 916 856 636 423 529 975 079 480 064 850},
{16 047 404 631 614 043 761 303 245 207 203 601, -409 165 801 275 955 454 756 056 128 782 190},
{22 574 533 844 797 037 480 081 102 359 245 941, -170 860 809 234 449 712 326 037 768 391 950},
{5 247 663 488 268 538 714 073 349 808 643 791, -235 730 384 508 953 583 836 939 588 955 810},
{15 460 352 296 961 527 284 830 391 755 608 721, -37 098 603 049 874 668 820 139 276 576 150},
{2 451 058 883 888 612 905 089 330 738 103 079, -62 818 477 242 686 767 124 155 159 382 190},
{285 706 127 381 075 799 067 160 071 614 919, 9 004 146 355 384 699 131 232 654 762 650},
{609 065 553 799 877 856 203 505 078 260 131, -3 343 663 353 406 468 914 457 210 835 820},
{130 224 693 455 028 956 845 469 241 363 641, 1 234 535 733 808 613 585 424 028 452 600},
{150 208 792 686 257 124 362 509 714 000 891, 4 663 352 572 451 518 208 841 682 875 690},
{246 359 102 319 943 961 573 541 356 681 561, -7 310 945 684 918 945 071 771 972 775 010},
{555 475 792 792 342 887 543 135 134 863 529, -23 915 445 617 488 315 018 037 675 246 850},
{1 360 556 441 118 022 174 195 419 650 680 729, 14 026 535 034 355 692 850 694 159 477 340},
{4 381 760 834 488 112 800 368 473 934 001, -238 421 579 960 868 383 570 867 335 680},
{22 633 271 193 312 955 919 308 334 832 011, -330 035 743 139 912 854 998 852 693 420},
{34 937 965 918 598 799 978 737 754 506 219, -678 078 476 500 518 762 788 582 332 980},
{80 850 829 716 472 097 253 400 228 993 991, -3 744 326 489 584 661 125 070 311 142 160},
{382 612 616 652 002 322 034 800 649 515 779, -20 516 475 380 231 981 439 720 067 441 110},
{1 807 304 308 673 736 655 290 038 598 193 061, -34 663 891 693 606 888 944 318 015 305 310},
{1 200 267 092 150 785 976 560 952 381 552 191, 50 314 494 211 198 114 444 476 398 369 220},
{1 827 472 998 410 161 296 726 776 006 581 339, 39 599 870 254 933 259 713 676 007 140 640},
{1 475 620 637 491 068 824 317 599 206 086 649, 62 903 406 159 580 360 030 818 564 310 320},
{7 239 416 251 000 856 445 801 828 964 271 539, 213 915 202 865 576 818 998 457 089 274 260},
{8 458 862 253 617 605 436 573 729 834 378 551, -108 688 097 538 695 336 930 536 433 090 670},
{4 721 147 954 558 341 846 036 098 620 120 959, 195 242 145 304 114 197 883 441 466 817 210},
{8 869 453 282 159 875 305 209 357 543 487 669, 241 453 653 083 150 038 509 093 390 191 490},
{16 147 302 361 085 706 026 401 571 292 962 711, -776 216 741 361 868 412 581 399 892 425 260},
{38 465 551 085 896 190 089 764 438 439 904 999, 1 736 400 614 780 367 920 070 048 559 376 520},
{66 449 127 742 752 057 904 065 903 539 011 309, -980 420 891 485 801 630 978 532 072 065 830},
{55 092 712 448 895 703 621 043 617 727 747 881, 2 448 548 869 413 376 629 163 678 862 227 920},
{307 201 798 450 601 671 279 970 021 977 064 029, 9 609 123 059 341 479 437 624 618 362 874 370},
{72 825 001 529 743 351 728 459 174 363 868 561, -831 072 308 387 622 256 146 782 931 077 460},
{77 649 763 700 219 109 926 888 616 307 927 669, 4 420 487 882 804 690 070 744 958 874 815 920},
{481 673 565 756 593 147 976 681 503 128 481 641, -15 702 090 132 749 740 240 217 917 486 228 050},
{1 277 898 318 020 848 666 988 558 675 091 565 159,
-29 933 496 425 878 786 362 975 087 735 328 470},
{2 319 749 101 276 725 801 461 894 479 417 321 801, 27 264 686 424 866 615 416 968 024 244 614 660},
{564 939 545 928 936 245 922 717 074 894 000 951, 23 648 148 559 142 680 233 345 651 418 905 630},
{656 620 892 112 507 999 072 218 349 093 276 419, 28 839 149 968 008 926 309 356 378 048 592 190},
{1 676 568 845 076 023 816 787 564 852 110 331 701,
-24 704 918 137 149 977 231 837 183 905 172 610},
{844 762 650 793 833 379 318 277 013 792 850 529, 41 907 954 605 062 276 615 647 362 425 749 540},
{1 657 493 231 839 549 598 337 771 084 742 791 979, 19 238 284 655 954 692 053 161 177 066 165 430},
{753 188 608 288 966 523 243 374 120 193 814 749, -32 407 863 818 024 755 430 512 981 547 775 450},
{1 959 742 859 073 684 233 735 461 693 339 829 149, 63 753 679 792 792 145 595 563 456 236 731 000},
{4 171 924 840 220 942 211 478 367 949 706 794 601,
-45 807 705 233 440 006 561 195 516 540 904 040},
{859 339 658 453 305 216 803 562 065 616 267 211, 5 776 952 155 982 769 315 098 816 243 674 920},
{357 979 409 819 980 197 686 550 227 515 263 119, 4 722 052 738 284 270 994 982 907 959 381 460},
{225 046 170 695 723 880 969 845 126 829 688 091, -1 725 495 005 146 749 301 683 732 803 996 340},
{183 686 826 688 264 409 490 925 439 851 136 641, 5 992 769 696 048 975 853 300 452 295 253 260},

```

```

{524 347 506 202 714 332 308 533 906 730 319 169, - 80 793 445 526 726 978 634 988 874 186 580},
{490 771 701 683 517 168 515 571 886 842 781, - 16 503 593 010 286 168 162 159 851 790 200},
{1 088 358 244 892 036 963 655 140 382 667 969, - 20 243 234 483 333 086 552 597 389 350 040},
{1 198 880 719 195 377 256 464 779 200 781 941, 65 813 786 969 409 030 327 370 380 959 490},
{3 572 370 990 249 692 353 600 198 221 291 371, - 132 827 353 515 544 757 201 476 287 179 580},
{3 505 856 222 174 038 800 755 044 671 879 539, - 182 465 475 636 883 957 617 130 055 419 020},
{9 792 058 453 384 145 113 422 978 348 457 909, - 154 577 849 162 854 307 298 509 775 927 990},
{13 467 142 987 205 262 157 832 478 713 629 289, - 168 191 730 363 328 527 784 978 961 857 410},
{2 962 944 092 883 963 693 574 603 024 158 739, - 73 851 765 037 092 402 072 218 245 944 180},
{2 227 246 341 467 170 282 154 169 784 276 289, 97 538 916 251 789 520 206 911 690 242 720},
{4 053 331 813 321 159 333 804 571 917 874 021, 225 292 476 503 514 813 407 775 447 671 910},
{485 123 699 268 934 191 381 921 195 310 109, - 15 072 145 743 472 755 307 035 920 148 660},
{706 573 904 929 311 410 749 709 388 800 239, 17 189 313 426 467 519 575 847 289 221 490},
{454 825 665 479 920 143 132 603 210 506 399, 19 948 637 424 181 121 807 511 790 210 860},
{1 002 241 814 337 660 268 482 159 050 188 631, 24 066 054 600 068 060 926 175 729 734 200},
{2 141 652 195 164 770 894 722 621 260 590 019, 102 805 078 325 685 807 929 442 863 109 480},
{4 330 866 868 332 399 020 715 395 041 974 311, 77 599 852 199 469 903 228 138 423 112 020},
{3 695 938 564 316 805 575 149 519 727 001 059, - 40 754 516 018 406 430 591 963 166 689 140},
{3 193 320 732 903 081 788 501 238 869 380 931, - 75 755 099 505 468 983 911 282 946 677 470},
{2 913 244 972 019 500 521 066 132 340 724 941, 136 283 585 211 651 013 403 910 113 820 180},
{12 873 710 326 282 139 135 589 007 575 791 411, 355 989 388 737 106 238 928 271 238 098 920},
{14 581 175 268 324 948 076 981 994 061 803 041, 472 069 001 152 428 688 994 284 290 483 690},
{13 293 905 617 485 661 742 045 554 741 028 599, 679 157 361 508 283 204 277 265 269 129 060},
{72 599 644 782 680 588 218 437 411 029 702 851, 3 076 469 869 422 321 826 256 802 380 166 540},
{310 143 652 947 239 038 543 187 369 667 821 359, 6 254 275 351 732 656 996 825 641 983 487 130},
{645 098 774 487 846 635 821 777 106 140 320 391, - 27 754 329 648 610 127 346 398 433 934 185 030},
{1 694 047 335 023 240 420 507 894 539 170 239 951,
- 82 160 320 591 160 972 240 618 750 334 447 510},
{7 861 168 745 176 139 132 819 903 681 142 597 509,
- 48 561 809 770 993 687 370 177 449 137 795 930},
{1 466 953 868 934 393 508 359 612 874 266 130 901,
- 84 304 969 640 848 882 655 926 545 133 838 670},
{8 476 115 645 030 588 305 424 263 354 709 251 261,
114 165 195 323 307 474 945 249 575 656 805 760},
{7 000 688 967 564 625 028 424 483 782 511 880 271,
206 449 098 198 313 545 946 992 262 120 724 340},
{4 663 673 165 686 918 977 086 535 527 779 569 539, 20 511 938 942 439 194 681 173 771 463 126 970},
{1 873 219 464 058 667 899 482 440 818 086 584 599, - 991 095 170 793 412 487 073 261 080 801 340},
{12 447 406 038 693 027 408 321 218 385 051 749, - 312 679 686 468 975 228 737 917 300 621 350},
{15 005 136 436 561 417 040 063 883 590 365 001, - 428 873 183 383 115 964 807 962 083 012 470},
{1 361 670 443 758 073 781 912 118 082 933 699, 69 778 990 426 636 667 526 364 969 296 300},
{8 511 250 558 439 551 722 410 507 051 067 551, - 220 750 562 009 423 555 375 142 767 297 790},
{24 603 361 341 919 701 242 235 279 260 111 009, - 463 784 094 575 841 816 273 863 329 622 340},
{5 723 886 679 421 329 909 851 220 321 874 239, - 107 727 798 102 899 310 073 466 087 563 440},
{3 592 658 371 884 285 465 336 937 933 991 669, 12 610 815 061 912 731 268 429 134 103 470},
{357 404 110 971 579 487 506 686 659 817 531, - 4 210 491 468 755 061 264 778 856 007 150},
{122 403 632 022 780 719 878 541 298 344 969, 3 479 393 839 965 178 504 715 150 921 610},
{156 836 753 623 867 525 591 265 038 243 369, - 7 707 296 007 996 016 367 029 803 628 680},
{675 399 199 450 746 760 917 910 383 112 019, 2 868 796 034 982 632 357 174 571 435 000},
{309 264 938 686 867 402 453 410 067 641 769, 17 753 003 778 591 241 975 742 774 584 170},
{1 873 432 487 154 888 505 311 507 827 430 629, - 22 320 722 063 371 583 558 303 405 900 730},

```

```

{378 549 708 249 452 910 080 545 325 903 441, - 7 876 908 260 923 066 705 002 937 087 290},
{114 986 043 011 572 768 341 490 774 093 771, 1 938 679 137 769 855 591 036 273 500 930},
{151 597 444 670 973 406 058 010 022 264 151, - 2 610 381 772 309 907 633 911 757 776 380},
{49 020 771 126 689 586 073 145 879 761 861, 1 008 481 866 057 842 078 468 144 741 580},
{99 104 917 846 313 618 720 096 356 465 309, - 4 379 552 989 372 625 465 780 407 534 410},
{407 825 028 223 448 515 206 107 223 356 371, - 21 844 827 054 640 233 157 699 318 886 580},
{1 813 898 139 493 694 612 335 138 707 650 899, 63 037 229 677 762 429 947 652 424 044 830},
{3 559 561 811 515 379 892 842 179 001 941 921, - 80 856 159 946 769 593 933 193 924 672 520},
{474 584 238 236 957 705 193 225 404 111 291, 12 015 083 101 571 977 649 762 517 377 820},
{1 504 995 316 188 294 789 974 293 820 454 061, - 42 172 752 087 227 804 678 093 590 085 790},
{3 319 163 496 928 450 787 705 931 081 229 129, - 125 883 977 149 825 559 829 601 222 313 700},
{11 591 202 849 279 544 266 211 124 569 305 179, 267 384 548 154 284 656 816 610 939 582 310},
{23 510 486 939 971 309 797 310 395 983 728 099, - 326 919 037 893 447 768 765 654 596 251 470},
{6 948 630 877 589 318 008 000 471 540 812 991, - 164 172 908 825 384 875 523 487 082 771 800},
{13 395 545 437 711 462 239 517 530 163 745 141, 420 191 284 887 920 334 535 712 454 243 180},
{12 694 495 354 199 104 871 942 361 381 191 369, 740 912 767 307 773 844 599 755 261 861 720},
{24 843 555 801 704 327 950 377 004 315 074 379, - 1 099 901 243 283 345 986 387 876 107 332 090},
{113 997 371 246 970 063 872 580 684 544 486 441, 3 571 535 776 542 000 656 869 210 802 139 990},
{73 235 174 195 863 243 955 749 342 122 302 989, - 3 628 256 647 733 294 337 944 871 917 826 150},
{168 180 351 540 536 656 409 827 845 210 777 239, - 6 136 742 964 624 663 074 092 767 571 378 500},
{624 561 165 413 359 105 740 103 316 672 992 489, 27 301 158 151 784 216 276 281 433 225 372 070},
{844 733 491 497 145 022 206 781 525 151 845 371, 12 972 342 365 013 687 967 441 181 984 457 270},
{384 340 680 585 081 385 099 278 736 692 828 071, - 5 478 519 155 362 528 385 266 147 222 833 960},
{211 929 267 135 803 930 792 756 204 707 168 621, - 7 277 978 274 869 653 051 344 579 920 912 940},
{217 842 188 310 582 068 244 610 137 174 033 611, - 4 188 501 365 899 077 984 376 858 693 089 840},
{10 069 438 241 333 277 310 384 768 473 844 681, 561 339 182 273 780 814 988 664 784 280 980},
{8 701 426 938 289 117 212 210 608 446 452 709, - 494 624 391 870 678 946 804 405 842 042 030},
{50 654 840 961 159 061 397 442 874 286 261 581, - 2 990 910 331 814 997 421 373 061 138 864 000},
{47 849 304 603 669 586 240 690 433 681 031 169, 1 524 202 080 697 922 780 919 603 359 037 330},
{150 359 065 610 528 988 077 865 117 269 358 689, 5 179 457 973 771 197 735 700 826 067 788 260},
{38 850 877 162 227 689 377 831 487 178 286 399, - 144 766 363 160 805 684 847 606 377 998 340},
{13 426 450 618 073 225 506 917 446 557 551 029, 573 009 087 556 201 787 605 532 686 999 170},
{62 057 642 674 426 682 389 538 883 899 099 869, 2 897 566 536 673 545 254 577 693 191 823 840},
{303 395 096 474 840 242 895 239 044 570 606 479, 2 041 958 135 720 632 854 604 868 668 246 440},
{215 023 102 631 047 162 662 483 136 526 383 331, 1 467 956 454 552 618 026 010 163 137 992 160},
{176 066 526 857 597 647 114 828 913 261 520 721, - 10 331 473 744 355 542 571 080 977 309 072 180},
{108 299 774 091 909 275 019 527 050 830 708 911, - 4 360 688 512 700 746 627 531 260 815 151 180},
{180 077 120 127 957 057 857 371 856 565 717 839, - 3 148 433 494 480 319 683 991 943 945 054 990},
{154 719 146 587 287 803 327 593 976 093 435 659, 4 913 308 812 138 031 400 078 759 673 795 120},
{604 049 926 163 216 311 213 258 977 652 521 689, 5 888 072 232 142 619 592 031 313 171 236 230},
{607 799 950 615 850 198 257 536 025 187 310 251, - 24 997 881 783 693 458 020 092 215 094 293 130},
{1 970 547 739 609 008 649 606 038 593 993 057 881, 84 669 796 130 778 714 968 372 979 995 280 480},
{5 808 749 578 875 649 538 698 473 579 503 317 091,
- 270 339 770 195 873 503 056 232 335 678 961 650},
{33 035 215 595 338 799 603 916 227 091 525 732 691,
- 731 935 890 388 202 263 141 105 830 406 929 240},
{24 623 232 495 294 138 404 182 645 526 693 139 641,
- 1 248 926 649 800 929 674 793 178 254 253 821 980},
{89 180 425 681 838 228 011 910 809 154 208 289 709,
4 369 153 469 757 418 610 687 726 024 238 352 650},
{451 136 427 959 153 805 337 228 456 029 750 413 959,

```

```

18 243 748 895 198 592 388 846 030 419 084 489 750},
{1 244 280 899 623 562 100 364 498 416 287 819 277 541,
 31 102 838 659 387 387 447 389 500 856 294 778 380},
{42 005 665 264 717 219 698 513 891 043 063 727 591,
 -216 518 800 770 925 747 757 265 782 850 834 270},
{255 496 704 563 783 034 686 621 670 471 681 961, 10 450 423 653 071 784 103 966 604 790 465 630},
{1 176 320 759 405 114 264 047 212 030 627 217 091,
 -48 269 690 413 305 419 015 580 832 882 026 240},
{4 479 895 560 931 836 125 991 282 406 105 420 081,
 199 558 451 451 443 121 646 919 553 036 672 150},
{22 492 016 879 021 949 889 522 112 063 956 828 031,
 -988 317 215 737 622 829 282 968 588 015 975 520},
{60 059 049 818 787 171 180 527 530 563 062 841 179,
 -3 175 415 940 400 613 035 448 617 839 129 519 930},
{68 737 115 254 943 599 742 048 303 479 907 410 241,
 117 028 961 327 277 278 636 690 663 220 403 620},
{10 319 853 913 791 132 760 031 926 552 151 810 551,
 -228 498 905 776 174 326 027 245 593 628 108 100},
{9 388 191 619 685 310 290 274 584 560 623 458 801,
 -126 399 938 988 979 959 850 140 503 627 675 070},
{8 683 629 759 699 108 602 411 010 336 051 408 871,
 448 020 399 503 763 146 308 915 312 671 924 960},
{42 981 784 451 029 814 457 946 468 216 493 492 381,
 -566 711 348 777 273 153 931 057 407 337 691 500},
{22 157 792 066 779 255 444 287 580 033 936 466 369,
 -765 902 246 475 728 481 814 071 455 359 256 280},
{13 396 643 335 234 502 608 443 535 041 973 403 501,
 98 372 204 673 946 981 560 117 960 096 622 680},
{4 523 898 394 005 992 183 140 609 677 012 474 271,
 -181 006 044 083 408 077 549 999 004 899 956 300},
{314 429 727 881 648 657 950 726 817 094 740 479, -3 204 968 002 408 486 634 957 563 044 184 530},
{86 058 775 049 858 898 946 295 329 928 791 289, -2 146 037 860 825 669 141 953 614 794 015 770},
{54 532 414 824 865 450 305 835 280 208 282 739, 2 323 432 844 768 883 064 980 725 421 659 340},
{274 458 308 190 466 092 630 927 473 039 597 669, -7 286 429 360 825 848 780 279 494 627 181 920},
{608 927 887 749 956 415 943 024 021 122 138 041, 9 388 128 880 167 279 080 161 056 436 193 670},
{326 422 854 690 097 791 128 606 454 843 077 759, -15 539 319 271 883 367 720 060 150 673 694 970},
{24 384 645 117 314 320 843 165 964 566 330 639, -768 918 083 375 342 975 409 302 394 203 010},
{55 404 121 224 860 246 852 859 724 089 585 931, 960 249 821 121 784 987 145 419 040 813 040},
{72 882 468 451 023 882 795 219 649 670 167 639, 2 886 751 069 189 185 549 147 253 915 053 720},
{179 136 622 044 855 260 701 113 750 249 984 389, -3 391 037 353 643 375 033 107 097 022 648 060},
{147 677 782 259 147 629 444 160 379 541 060 541, 3 915 290 293 680 016 180 036 944 162 244 020},
{276 915 474 073 939 334 708 118 154 677 266 969, 10 186 146 910 002 796 329 875 777 067 748 080},
{474 266 383 469 822 284 169 515 635 865 271 059, 5 887 744 194 526 246 811 385 349 111 875 930},
{662 864 967 987 730 595 727 108 191 366 497 021, 27 487 090 652 025 355 379 933 425 026 326 040},
{796 872 877 119 638 718 785 203 674 402 687 311, 41 708 301 154 700 325 558 349 694 716 184 280},
{1 108 203 950 263 465 827 316 428 173 591 683 741, 4 865 812 441 678 086 699 818 109 171 455 610},
{301 522 896 223 623 000 767 280 092 549 030 089, 3 993 245 059 499 285 288 386 448 163 887 670},
{492 895 802 878 992 968 672 581 944 514 640 581, -803 077 789 753 220 839 114 856 855 061 360},
{48 683 967 400 641 262 528 981 287 751 649 209, -2 085 505 730 799 440 519 343 647 065 780 590},
{180 051 233 655 786 776 603 428 714 912 605 389, -6 980 312 007 685 549 819 523 641 650 068 010},
{360 656 514 553 417 194 750 677 965 279 880 621, -15 302 295 237 075 001 448 306 572 503 260 820},

```

```

{1 656 241 355 232 092 842 178 623 474 393 143 809, 79 690 556 767 606 558 577 478 063 242 402 190},
{4 332 344 558 798 866 875 052 379 278 022 847 431,
 192 264 409 875 272 696 699 554 952 000 602 080},
{22 523 953 951 433 692 408 383 539 115 741 102 659,
 199 542 020 805 333 608 599 400 762 989 098 780},
{6 097 894 291 820 346 200 535 522 608 791 929 731,
 204 359 885 702 366 373 456 909 685 749 331 890},
{8 258 472 091 911 895 796 113 758 885 694 769 219, 33 224 319 712 245 210 273 692 230 239 767 250},
{3 610 262 625 727 552 070 937 217 445 826 283 781,
 -140 699 878 591 457 418 401 076 706 034 242 080},
{12 031 488 630 235 542 680 185 004 677 066 585 049,
 -634 993 711 299 793 599 412 430 083 412 962 170},
{8 381 362 999 594 462 871 442 893 852 703 741 431,
 104 132 659 492 863 186 453 800 827 502 721 300},
{12 738 310 281 517 396 739 845 740 773 995 395 181,
 254 675 048 350 602 679 101 904 935 303 956 490},
{1 144 023 860 802 958 972 373 996 208 190 240 931, 67 762 674 449 658 100 157 075 507 327 838 180},
{1 993 342 815 148 411 304 368 141 512 135 040 379,
 -92 812 975 046 987 608 333 755 443 480 068 410},
{11 111 855 129 579 553 869 178 576 962 454 546 019,
 609 926 410 508 736 162 237 071 175 448 864 350},
{33 428 114 845 998 040 176 735 246 898 121 917 469,
 1 266 624 956 267 414 962 627 648 050 178 952 190},
{124 462 361 744 358 038 252 515 795 960 759 292 779,
 5 527 294 704 612 932 117 209 176 709 345 866 420},
{669 019 531 896 589 511 267 112 356 903 104 355 131,
 -27 988 575 370 751 735 338 916 493 406 038 682 110},
{679 275 527 364 486 353 587 754 695 297 827 892 759,
 -38 250 555 731 391 652 497 855 592 244 971 268 880},
{2 317 853 425 941 411 234 785 137 243 025 391 717 331,
 -95 310 102 012 256 165 366 509 713 749 905 946 170},
{7 633 155 389 463 079 763 214 932 369 939 901 322 001,
 -202 273 040 210 950 035 648 729 989 660 165 272 890},
{13 358 254 776 808 419 450 638 616 523 741 141 002 569,
 -320 799 917 952 268 831 503 720 255 822 402 410 850},
{28 950 786 073 904 739 601 926 189 420 739 823 535 881,
 934 953 147 078 160 670 266 171 859 588 430 462 960},
{8 223 132 865 078 535 257 609 694 851 881 724 785 629,
 226 611 249 170 906 014 431 947 259 208 203 649 470},
{16 347 101 626 405 603 252 957 973 616 984 744 581 959,
 218 154 956 348 107 510 572 399 325 096 853 920 140},
{3 644 545 025 317 470 032 965 917 085 104 156 563 791,
 129 082 831 923 965 940 396 162 156 441 505 929 840},
{7 586 658 593 052 349 170 217 552 890 239 622 596 021,
 -243 999 149 222 146 983 810 139 854 531 782 142 840},
{5 693 926 758 613 960 697 907 567 338 348 418 163 231,
 5 624 892 881 321 742 341 875 849 338 335 695 860},
{385 325 841 805 719 430 231 159 796 126 182 180 661,
 -15 853 213 000 669 246 352 423 212 083 116 546 370},
{1 217 031 177 204 036 961 023 679 238 977 652 013 031,
 -51 685 333 545 391 438 326 034 266 440 348 236 260},

```

```

{5 877 623 799 224 747 259 086 932 053 267 119 959 459,
 327 931 661 800 169 267 217 296 857 546 352 408 400},
{6 311 674 407 753 187 256 927 257 024 373 071 326 991,
 -83 057 018 802 954 875 716 290 249 313 963 515 330},
{165 414 339 117 207 675 211 282 795 527 115 360 339,
 9 059 118 401 806 513 232 031 882 317 241 973 650},
{589 902 179 057 299 695 711 937 368 006 718 494 389,
 17 639 149 550 615 267 919 445 197 538 294 132 710},
{1 960 371 215 635 959 446 931 708 159 996 040 854 709,
 -24 412 478 383 204 743 259 389 486 405 078 216 420},
{1 850 609 189 874 576 531 317 861 145 035 668 818 359,
 65 741 708 662 797 833 554 606 887 743 542 210 140},
{2 470 178 176 375 535 139 005 940 342 338 220 544 189,
 -32 294 616 916 225 983 092 395 380 068 955 112 380},
{3 962 609 976 332 466 419 956 755 731 505 632 830 559,
 -54 430 567 368 905 524 406 597 277 515 411 519 790},
{2 716 181 841 006 852 292 936 227 306 971 436 641 861,
 27 055 996 572 840 852 750 552 485 914 067 687 430},
{2 656 128 114 414 521 488 125 657 606 731 642 614 111,
 124 279 394 439 832 775 372 083 158 690 213 262 500},
{11 611 468 625 686 334 533 289 729 833 528 189 504 361,
 661 979 426 896 111 112 531 431 834 715 221 824 240},
{76 344 425 669 360 038 561 286 841 027 796 636 321 709,
 -1 909 864 591 344 523 416 326 067 186 786 878 626 380},
{12 589 654 089 645 421 030 717 457 363 305 692 106 241,
 -635 898 480 519 360 605 607 602 119 822 044 287 490},
{32 207 195 706 189 561 440 080 843 316 933 604 533 309,
 1 782 428 097 956 481 842 968 541 319 044 934 582 420},
{30 995 975 686 194 954 928 421 993 105 320 294 486 999,
 -879 040 404 507 465 343 867 582 992 680 260 401 450},
{57 619 943 636 850 641 157 203 678 739 306 289 498 499,
 -260 074 235 052 623 976 438 504 112 012 141 964 910},
{29 250 672 752 802 284 648 202 765 974 695 904 591 771,
 -1 147 197 555 963 900 836 148 920 496 811 592 374 560},
{143 254 197 279 895 699 864 418 142 155 929 902 170 521,
 3 127 678 842 490 399 811 295 268 047 398 880 148 650},
{155 376 398 140 335 555 246 211 194 129 064 751 512 129,
 -5 070 251 390 099 119 128 235 369 129 702 236 413 610},
{452 150 133 137 021 570 000 397 471 817 848 904 755 031,
 -24 371 267 055 860 263 754 301 550 472 034 323 226 210},
{2 736 889 172 005 183 774 164 328 774 851 612 372 282 709,
 -98 058 295 843 435 356 529 543 507 477 229 699 707 920},
{2 194 521 014 362 558 374 385 248 062 215 624 104 301 801,
 -42 942 486 335 233 940 432 784 943 725 544 473 435 900},
{1 118 007 027 672 480 490 617 198 985 426 845 726 796 151,
 45 169 305 330 892 872 485 694 402 128 317 709 878 530},
{2 817 627 005 560 171 702 815 428 013 055 352 061 941 849,
 112 622 073 784 036 961 754 994 202 511 215 390 929 950},
{520 865 400 771 162 394 083 810 519 016 789 461 967 849,
 4 448 254 840 162 629 899 962 085 260 591 123 409 070},
{105 315 702 505 808 642 849 882 425 434 633 799 771 409,

```



```

- 3 778 575 718 817 649 727 787 818 358 449 719 102 960},
{121 588 822 892 472 931 572 298 639 091 542 112 979 221,
 3 808 144 306 408 501 730 589 634 152 126 027 474 510},
{68 220 523 062 380 075 448 983 097 899 182 317 479 849,
 -1 844 077 685 609 373 318 513 416 701 043 516 204 520},
{2 598 177 596 851 071 339 343 329 896 373 303 935 141,
 -150 381 020 208 336 928 937 771 642 770 201 664 910},
{10 466 763 580 645 230 397 704 204 289 248 783 549 421,
 -215 408 093 883 376 502 289 909 983 432 549 388 510},
{22 146 487 929 694 771 839 847 609 635 480 258 379 819,
 1 127 619 780 596 573 373 936 466 473 888 003 974 610},
{101 882 828 241 410 605 359 311 680 412 235 099 207 631,
 -2 956 264 186 419 926 029 666 393 772 812 430 084 220},
{343 831 321 686 413 208 014 227 326 289 731 562 381 901,
 -2 305 523 099 516 444 092 947 083 205 182 725 297 680},
{77 403 344 474 222 579 443 094 108 093 878 749 922 831,
 4 151 634 516 514 664 731 827 391 584 517 772 410 410},
{370 905 546 228 568 665 868 209 335 001 690 394 614 709,
 21 891 900 835 175 484 682 283 760 896 465 754 957 570},
{315 448 760 323 058 006 384 264 659 795 087 355 659 231,
 9 776 596 406 786 284 838 725 058 423 281 233 886 710},
{652 016 501 780 119 777 810 760 352 772 055 692 412 261,
 38 087 663 619 248 357 611 594 731 661 869 410 968 980},
{1 136 081 283 477 322 301 826 128 544 589 202 190 839 851,
 54 941 037 346 171 091 845 457 154 550 239 680 051 880},
{4 437 805 698 859 927 359 046 396 942 423 603 652 656 879,
 590 244 082 144 950 998 180 961 238 090 701 688 740},
{60 128 251 777 758 265 338 902 301 875 968 589 774 431,
 2 768 251 795 910 953 494 461 000 880 111 213 010 290},
{194 095 220 802 960 596 349 169 089 106 002 209 439 199,
 1 127 758 280 791 058 206 034 516 922 372 341 171 310},
{30 319 923 231 544 812 719 276 792 947 841 521 443 629,
 403 502 335 866 917 431 366 155 890 162 175 121 950},
{14 369 258 423 027 347 070 590 397 605 275 211 642 129,
 -49 947 198 433 223 989 823 970 220 039 560 751 380},
{3 899 216 161 031 661 676 969 467 295 689 473 583 061,
 -46 381 043 601 997 511 734 345 325 880 903 205 530},
{805 333 114 431 543 512 399 440 345 094 683 953 791,
 5 207 479 749 233 917 268 838 951 676 971 715 800},
{458 387 921 628 129 731 919 888 373 818 930 797 459,
 7 820 206 736 125 040 351 381 810 951 135 884 680},
{754 073 226 615 159 851 721 256 546 819 686 063 911,
 19 950 139 376 063 087 484 557 168 001 916 061 580},
{1 012 049 488 484 605 645 670 875 150 534 193 308 379,
 -48 039 282 849 743 547 567 369 347 138 071 817 910},
{809 361 708 637 777 835 785 834 019 305 968 199 519,
 34 197 404 681 169 896 036 021 248 413 219 713 340},
{2 855 376 931 285 216 938 747 661 595 437 535 080 891,
 -51 545 792 248 892 096 034 376 393 239 457 567 590},
{5 109 947 756 634 065 871 096 951 784 109 584 723 691,
 -112 228 568 896 372 284 743 695 324 661 465 497 260},

```

```

{13 194 169 562 363 866 005 371 320 729 774 865 717 519,
 -216 492 010 502 539 170 370 374 681 599 361 333 000},
{2 972 612 651 046 870 192 605 246 794 330 074 465 731,
 -20 234 719 660 015 583 880 906 257 106 288 674 790},
{474 675 882 830 580 109 881 223 073 884 542 828 149,
 -27 160 598 971 810 743 419 630 261 095 509 305 010},
{3 249 370 777 759 165 408 624 667 450 482 045 387 729,
 173 367 825 366 138 145 327 467 505 904 871 651 150},
{11 199 093 953 562 297 501 901 005 589 339 512 014 371,
 656 400 988 584 084 594 048 666 111 288 039 841 140},
{10 109 564 055 847 710 171 494 106 058 151 513 462 741,
 425 885 792 538 868 565 593 868 366 532 362 962 860},
{28 035 436 236 368 986 092 442 419 394 924 609 120 649,
 329 832 554 473 976 684 324 389 080 566 636 385 180},
{83 054 373 677 050 857 793 765 763 110 388 532 401,
 1 687 368 857 049 923 822 141 296 575 904 000 020},
{93 698 220 082 752 217 719 399 953 664 225 386 671,
 -2 032 053 909 702 300 722 677 775 293 581 814 920},
{56 158 799 348 042 503 531 794 830 024 936 988 101,
 82 207 762 479 124 394 699 964 884 097 255 360},
{2 735 291 274 936 029 881 422 360 814 405 882 471, 37 732 009 235 934 321 132 373 401 530 147 670},
{4 665 239 097 138 448 732 760 451 963 047 807 981, -8 436 755 647 452 940 426 987 375 910 552 640},
{71 980 751 659 858 164 255 295 787 438 286 689, 1 219 503 169 041 624 049 995 053 570 402 820},
{7 546 236 286 988 671 702 494 322 914 597 559, 337 434 717 595 878 722 594 047 599 565 290},
{30 790 797 469 714 291 161 744 206 764 455 929, 52 089 199 821 093 627 665 697 819 674 280},
{1 526 174 237 437 260 040 515 629 576 068 699, -59 221 812 493 075 900 187 775 087 685 560},
{3 411 814 733 061 054 455 997 198 642 721 111, 184 356 562 431 617 431 287 026 952 745 680},
{22 830 948 238 058 861 352 534 678 321 149 059, 116 078 930 899 161 359 676 099 178 706 910},
{9 186 888 418 057 552 417 871 830 912 164 961, 511 119 095 810 966 683 355 612 275 456 500},
{3 327 081 941 501 818 514 826 701 559 061 789, 153 027 322 573 344 185 592 865 104 676 410},
{9 919 307 933 050 145 622 299 016 698 626 981, -471 469 058 625 965 096 131 627 207 317 150},
{4 632 883 178 124 529 487 246 181 586 674 581, 159 712 514 203 395 564 668 685 650 450 370},
{306 286 822 740 586 075 428 728 627 076 601, 2 095 539 043 312 318 159 877 548 037 520},
{84 868 726 663 893 645 738 260 013 268 931, -1 490 670 629 301 716 977 052 656 524 840},
{24 974 300 782 359 710 389 093 570 384 199, 1 036 304 313 898 634 709 934 361 676 090},
{25 852 309 446 911 815 017 891 429 667 789, 559 315 831 514 388 507 921 582 440 310},
{31 069 080 509 735 857 028 157 990 795 779, -722 291 154 824 249 500 129 458 905 250},
{2 650 773 925 575 259 170 405 725 377 279, -70 854 510 801 176 866 509 135 520 110},
{7 318 413 508 860 492 501 495 494 435 459, -290 266 652 066 327 753 166 335 622 210},
{15 498 549 007 776 966 756 613 073 932 459, -612 697 241 958 819 410 338 701 330 180},
{45 460 607 660 426 856 034 530 710 167 709, -1 647 922 334 219 213 552 759 864 389 620},
{170 985 642 125 491 984 129 118 678 154 401, 4 897 887 262 348 536 095 430 316 804 020},
{110 543 426 233 401 581 946 544 906 561 049, -620 064 637 568 561 423 685 656 034 810},
{43 152 107 295 609 781 155 031 223 582 119, -907 552 451 825 239 896 780 536 355 210},
{103 013 008 392 435 206 499 064 888 458 211, -6 138 258 032 853 103 455 762 611 580 060},
{335 681 919 682 955 614 473 776 609 105 059, 16 091 656 929 119 403 650 975 927 392 800},
{562 961 832 966 517 411 376 184 402 078 991, -1 829 397 815 618 362 302 798 716 859 000},
{123 666 255 228 482 649 340 918 013 745 259, 973 204 857 703 504 189 514 773 110 630},
{17 378 813 334 541 935 407 999 002 507 499, -829 163 203 585 593 229 865 530 413 330},
{8 437 099 129 636 127 213 461 179 280 181, 385 810 230 855 350 181 546 588 122 250},
{12 732 213 244 575 771 921 503 611 739 069, 555 454 483 934 523 114 224 447 207 730},

```

```

{10 853 211 365 483 186 120 327 183 718 971, - 619 041 669 951 646 505 992 584 845 820},
{72 674 212 105 259 197 872 375 219 953 039, - 971 435 411 220 260 267 106 696 825 240},
{46 044 377 801 340 862 317 387 526 930 211, 1 684 556 352 660 075 016 085 542 386 720},
{140 900 426 159 228 057 652 548 504 681 521, 1 806 434 878 551 166 729 059 272 488 470},
{375 086 308 499 750 732 762 104 203 889, 5 912 117 100 845 566 591 360 549 410},
{658 355 717 766 489 414 103 787 355 809, - 11 129 361 181 384 164 210 569 001 720},
{432 575 424 270 755 145 734 279 836 579, - 1 548 591 512 989 614 902 487 418 740},
{130 116 428 809 799 573 012 792 037 869, 97 640 229 047 614 693 163 985 510},
{9 537 124 178 374 056 674 962 387 211, - 569 895 768 339 113 859 752 777 580},
{37 927 074 731 110 614 149 542 743 899, - 2 015 890 202 126 204 403 491 210 460},
{94 084 616 431 104 648 714 353 965 091, - 44 356 804 136 542 390 550 209 890},
{962 549 232 057 827 697 055 888 651, 25 877 481 601 479 885 971 564 520},
{1 275 685 613 571 050 943 108 354 161, - 61 064 633 991 320 400 459 125 670},
{1 674 596 761 916 044 099 854 512 159, - 84 404 438 003 527 176 647 596 620},
{3 386 491 536 779 357 707 452 480 491, 137 996 817 866 205 706 571 175 660},
{15 920 656 378 822 024 163 554 663 259, - 385 589 951 493 755 662 833 145 800},
{27 978 560 262 088 538 836 317 050 209, 194 401 967 963 857 663 126 753 530},
{3 846 104 301 448 128 137 799 985 861, - 67 357 390 780 673 930 058 343 050},
{1 689 989 764 378 245 243 082 434 761, 60 522 827 330 437 230 924 562 170},
{1 166 999 619 373 302 924 131 805 749, 12 311 198 031 173 611 285 512 060},
{643 612 590 635 727 145 951 827 701, - 13 078 399 996 398 842 455 585 860},
{695 518 693 858 150 272 658 260 811, - 40 619 148 840 986 671 450 994 490},
{1 253 284 053 905 591 355 829 974 731, - 9 352 693 878 864 231 836 475 750},
{5 791 608 583 856 725 298 281 981, - 194 126 799 126 714 484 393 620},
{8 081 042 876 122 017 615 181 369, 432 741 663 741 485 292 870 120},
{35 403 232 476 516 940 287 078 661, 1 399 855 674 525 491 983 310 460},
{102 116 993 958 289 816 783 607 411, - 2 587 559 334 388 924 945 004 610},
{301 747 159 197 557 726 035 332 871, - 300 237 685 878 439 845 241 770},
{2 079 507 321 146 073 405 859 271, - 50 011 549 042 953 907 633 380},
{5 265 412 403 155 669 400 414 939, - 33 744 385 012 998 029 635 020},
{323 373 623 122 171 115 306 569, - 5 439 427 455 078 236 939 190},
{614 298 221 411 339 109 484 109, 29 723 574 131 789 988 047 940},
{2 484 105 674 418 910 520 180 381, - 37 990 589 891 307 358 059 690},
{3 694 050 202 466 993 821 433 281, 177 800 716 677 135 685 368 270},
{9 980 976 785 966 748 396 397 639, - 488 998 880 291 372 884 003 980},
{50 450 794 214 961 969 795 827 789, - 2 139 210 869 560 164 094 175 580},
{223 456 930 274 974 084 560 918 881, 2 781 935 570 420 109 006 391 980},
{226 423 244 982 706 376 439 680 731, - 5 360 192 089 536 598 052 788 200},
{325 089 482 764 483 813 866 659 081, 14 527 868 804 035 022 455 309 350},
{1 374 568 638 004 043 282 313 198 631, 32 091 479 841 999 535 379 415 390},
{1 346 613 795 686 121 489 417 447 889, - 7 468 637 436 774 877 738 554 390},
{567 023 323 727 517 615 892 079 939, 22 979 939 350 042 728 855 306 870},
{1 876 265 165 911 201 978 138 544 561, 62 660 041 508 747 339 979 588 210},
{887 555 917 155 773 533 524 536 489, - 27 478 099 286 679 988 864 919 550},
{2 072 441 735 485 486 351 624 833 139, 38 658 663 934 990 266 478 339 710},
{3 796 655 368 000 997 589 583 311 451, - 173 870 935 170 092 816 591 210 580},
{7 154 806 641 002 138 231 253 648 559, 28 639 943 895 402 566 712 252 810},
{1 300 012 544 974 365 149 198 039 191, - 41 146 586 811 287 647 591 016 730},
{4 186 236 479 696 733 002 338 538 419, - 179 493 492 075 731 894 787 387 240},
{14 529 426 650 679 754 979 386 606 649, 98 339 813 812 843 746 698 683 980},
{6 241 314 198 901 002 536 674 220 141, - 66 157 582 115 443 722 933 511 890},

```

```

{5 647 871 492 372 437 811 949 722 731, 270 556 925 993 061 236 765 376 360},
{8 489 812 323 943 888 190 918 388 079, 76 358 074 256 431 419 483 999 930},
{3 530 586 451 480 157 676 793 358 099, 176 666 640 363 438 228 049 586 280},
{689 335 302 940 327 933 790 242 751, -17 144 303 107 884 278 794 690 140},
{894 357 834 864 152 282 661 924 901, -27 405 730 130 815 574 302 643 940},
{2 517 846 122 643 179 000 656 604 869, -42 730 759 570 842 684 510 703 170},
{820 441 701 171 385 754 195 422 411, 36 797 692 797 723 309 321 829 200},
{2 734 007 364 989 710 227 910 182 761, 86 554 810 191 273 383 027 919 960},
{8 972 386 843 890 545 274 797 245 709, -277 320 679 386 801 750 054 334 560},
{24 629 400 981 735 207 537 693 487 039, 1 042 584 003 193 037 338 510 673 520},
{98 546 388 819 319 835 227 232 037 691, -2 562 622 168 977 904 834 811 942 460},
{292 853 345 938 022 327 598 934 276 961, -13 175 109 407 350 301 173 556 483 520},
{753 235 683 055 241 146 953 601 519 771, 24 089 802 465 503 382 005 042 504 790},
{1 619 403 462 783 712 504 118 251 691 531, 46 360 257 929 585 421 791 668 410 960},
{804 596 752 696 091 906 125 815 709 319, -224 691 374 492 187 490 798 940 490},
{5 787 899 468 306 104 722 736 528 121, -328 491 663 947 065 777 321 949 670},
{31 362 571 168 010 896 533 700 050 689, -15 910 958 398 807 470 844 152 570},
{520 113 154 304 246 468 709 139 969, -15 095 752 267 395 421 238 674 590},
{1 721 251 880 413 338 795 145 181 159, -85 942 124 203 091 570 037 211 230},
{604 758 484 228 355 994 640 096 309, -31 469 792 499 878 134 788 381 270},
{1 714 939 109 398 529 848 873 896 929, 95 021 357 416 165 551 313 350 660},
{1 143 223 652 795 031 233 629 847 299, -61 687 803 179 554 096 670 491 590},
{7 239 996 511 740 647 380 482 720 661, -92 449 514 840 087 414 832 782 850},
{7 262 522 907 671 084 904 940 248 611, 231 998 688 339 567 932 754 777 060},
{17 711 455 855 264 226 375 082 097 501, -1 041 727 308 130 800 093 965 148 780},
{524 995 877 196 819 196 316 628 491, -508 092 327 366 487 476 536 370},
{34 262 259 836 645 896 694 128 531, -583 358 837 989 615 871 427 540},
{39 133 812 790 101 369 744 178 579, 1 425 275 925 854 644 038 726 570},
{163 492 060 798 521 155 338 858 439, 6 008 349 695 486 076 497 327 010},
{317 921 374 119 669 567 668 321 419, -11 847 050 909 502 692 405 923 290},
{489 199 109 662 684 950 193 460 161, -8 360 890 176 608 962 272 593 040},
{1 027 446 100 068 199 796 271 828 949, 10 943 948 134 499 346 760 961 550},
{322 541 168 259 438 613 897 744 501, -9 828 637 565 693 616 275 469 420},
{452 771 723 521 131 521 379 336 109, -22 354 514 672 900 320 847 151 000},
{1 426 038 945 844 401 213 515 343 359, 13 632 579 595 872 859 318 046 910},
{1 350 859 842 284 502 734 775 129 941, -31 173 093 547 208 314 692 994 080},
{2 614 621 758 390 845 947 072 509 751, -11 831 664 440 384 755 653 138 330},
{44 196 816 480 448 120 036 355 929, 989 504 176 592 378 846 242 890},
{83 048 738 018 440 939 188 104 371, -211 948 667 991 056 976 374 640},
{8 820 098 347 402 283 239 381 759, 489 364 585 661 974 938 271 140},
{2 895 487 177 170 321 975 810 989, -25 817 432 565 123 332 139 210},
{987 617 199 003 702 831 086 719, 12 128 722 393 524 395 182 140},
{1 302 861 967 184 932 154 678 129, -70 101 756 161 469 609 310 260},
{7 296 921 370 630 595 976 419 561, 152 700 866 734 618 606 788 660},
{8 212 778 390 405 384 508 465 869, -45 245 372 005 605 463 694 430},
{5 491 707 968 317 280 864 018 141, 198 137 919 853 930 587 902 520},
{14 094 600 685 786 674 910 357 169, 805 790 950 161 459 963 644 580},
{99 434 787 793 505 737 628 226 559, 214 716 639 180 131 391 141 990},
{5 266 947 129 330 785 900 782 439, -244 464 576 438 126 895 148 130},
{27 929 661 629 309 453 911 581 671, 1 272 890 439 646 722 744 913 290},
{18 555 938 772 530 065 604 187 959, -126 354 943 638 630 446 972 910},

```

```

{4 577 723 529 501 135 308 282 561, -18 928 833 285 333 253 670 730},
{766 585 512 927 532 088 558 849, -13 298 702 620 198 181 841 210},
{1 189 549 000 034 577 016 064 081, 67 899 417 335 647 462 525 320},
{8 192 768 513 776 404 657 311 429, -396 092 627 638 085 304 099 030},
{31 419 343 322 470 068 920 818 451, 1 781 449 570 917 762 889 659 750},
{162 333 987 466 465 436 357 319 299, -887 064 006 090 951 095 233 440},
{319 862 307 167 868 329 544 529, 1 684 703 720 894 769 793 440},
{58 081 350 336 620 733 476 821, 601 003 967 826 894 446 490},
{54 224 670 189 594 986 009 959, -1 788 161 538 811 301 499 780},
{145 535 830 339 241 195 156 309, 3 434 193 457 997 316 471 240},
{326 225 980 941 829 744 421 479, 4 177 189 743 750 213 890 100},
{101 700 413 257 578 309 413 429, 3 107 828 053 606 322 723 280},
{215 336 040 369 015 454 157 561, -7 943 581 167 880 594 213 380},
{215 696 557 896 092 009 471 551, -8 743 061 424 991 132 103 070},
{722 874 409 900 259 569 404 949, 34 525 121 158 054 328 971 320},
{540 436 739 139 216 087 185 521, -10 205 046 768 653 820 861 900},
{108 115 639 458 541 042 289 929, 2 873 518 279 783 174 973 640},
{270 591 848 478 121 283 806 141, -9 736 673 900 636 490 845 580},
{510 790 205 664 815 427 394 849, 1 880 261 419 207 358 121 780},
{160 865 990 256 081 414 057 061, 8 729 653 468 439 408 416 470},
{936 789 183 867 187 702 710 851, -48 193 673 924 946 023 826 630},
{5 298 454 202 596 525 751 225 131, -64 265 958 029 899 477 701 960},
{7 190 056 680 336 913 495 767 161, 197 261 697 013 321 505 522 310},
{22 247 532 552 192 163 537 964 251, -1 009 599 128 339 701 383 380 760},
{9 124 283 908 402 009 000 470 281, -401 349 330 882 646 259 355 000},
{26 794 426 176 612 596 138 374 469, 1 460 529 285 609 093 932 016 330},
{126 729 657 947 875 245 882 212 779, 3 065 545 020 670 716 238 117 950},
{261 620 337 194 345 909 963 584 079, -12 282 275 093 560 313 765 016 300},
{926 832 617 624 409 545 458 686 529, 18 899 544 362 990 799 504 003 060},
{189 490 903 302 952 810 396 683 839, 10 287 771 726 172 264 400 355 030},
{1 082 064 070 194 864 848 763 618 049, -4 376 635 841 992 349 686 866 870},
{259 789 322 911 373 502 982 790 909, -11 767 512 447 879 858 527 367 420},
{226 916 313 562 170 460 557 624 919, 2 594 795 296 487 804 544 855 210},
{293 449 814 700 597 753 960 633 899, -15 106 358 188 496 197 717 682 220},
{1 613 681 288 911 669 328 492 601 469, 65 709 566 189 452 767 664 794 180},
{7 293 524 321 987 115 644 940 510 781, 69 882 406 497 777 298 670 888 490},
{6 464 265 600 787 422 375 195 063 071, -229 807 859 668 740 419 601 385 500},
{7 441 028 045 735 347 215 423 536 821, 127 010 845 392 876 074 776 927 950},
{13 205 569 943 529 640 300 218 269 479, -312 622 727 007 176 919 881 578 050},
{18 929 267 716 280 625 963 189 836 129, 717 875 210 818 741 561 314 857 400},
{66 392 570 983 329 687 619 889 475 979, -2 326 764 229 904 172 722 415 965 610},
{271 981 512 656 721 653 873 555 204 461, -1 121 687 595 366 164 967 297 055 830},
{133 811 759 105 542 678 704 591 093 851, 6 338 285 742 347 758 548 993 531 210},
{177 647 387 576 177 043 107 461 548 691, -1 546 940 210 148 249 588 235 158 540},
{62 934 884 308 786 544 435 002 535 659, -2 867 089 012 578 235 100 401 324 500},
{35 409 565 951 591 571 230 477 438 591, 162 105 690 535 363 685 055 410 400},
{17 701 879 135 454 259 987 890 819 141, 489 041 841 472 188 562 064 317 530},
{24 189 583 456 323 410 147 422 403 311, 1 319 720 715 624 919 573 154 743 170},
{109 087 254 343 789 315 489 893 589 001, 5 291 968 315 711 439 884 070 847 420},
{513 064 151 823 881 440 974 145 911 569, 20 808 941 616 037 158 990 393 798 120},
{1 797 006 532 838 930 980 210 459 399 181, -68 284 570 151 102 580 885 533 497 800},

```

```

{5 423 534 936 476 233 173 833 702 551 631, -285 414 157 920 923 596 729 911 970 620},
{167 149 930 649 893 827 309 152 572 601, 2 438 948 762 830 375 846 413 144 960},
{285 521 030 335 928 629 431 961 839 389, 2 092 212 646 712 952 961 692 620 100},
{246 007 706 124 723 687 083 141 953 039, -4 114 232 477 243 193 168 525 480 960},
{212 406 869 976 843 660 125 113 044 811, -8 205 935 349 479 239 615 996 889 070},
{237 809 726 513 759 042 592 323 823 259, 13 199 695 947 498 179 474 105 777 130},
{54 015 064 156 744 826 663 378 564 669, 1 204 012 016 055 468 919 290 656 220},
{41 534 618 003 569 950 879 942 272 981, 615 099 294 910 010 860 811 661 510},
{73 325 646 628 007 701 467 928 134 449, 3 362 464 145 412 607 771 656 198 450},
{162 789 707 338 487 046 635 566 094 201, -7 330 203 818 690 884 710 087 239 160},
{382 831 055 149 183 336 425 355 002 931, -9 613 165 746 312 445 855 697 811 960},
{425 589 250 531 938 948 441 926 342 719, 22 144 270 650 982 008 174 110 390 670},
{1 216 875 148 983 479 076 591 058 917 239, 31 368 627 256 379 879 136 739 270 710},
{1 631 829 817 849 388 645 184 932 753 201, -71 948 622 947 897 973 194 388 407 010},
{5 770 115 998 018 449 309 786 152 615 279, 128 066 597 155 895 408 711 015 896 890},
{1 786 900 626 792 135 365 399 751 062 479, -104 924 908 166 560 004 215 776 067 980},
{797 474 178 114 438 726 621 034 611 569, -29 035 635 911 928 960 860 324 601 660},
{3 391 514 131 581 552 631 459 862 053 999, 8 539 971 978 493 855 884 523 027 800},
{287 459 285 992 453 171 359 224 367 149, 13 356 584 347 125 561 166 047 615 660},
{1 602 777 980 721 602 747 749 617 520 121, 95 704 936 798 438 265 986 564 249 680},
{6 075 692 157 813 791 279 515 655 834 189, -58 053 733 078 708 480 872 649 475 070},
{5 007 403 678 100 402 240 247 301 088 411, 207 619 878 324 395 978 006 903 566 650},
{6 156 176 177 039 590 788 485 487 691 561, -129 064 951 310 985 534 108 195 938 280},
{9 774 312 957 816 427 025 687 253 815 629, -315 545 366 623 103 853 493 390 030 080},
{1 905 945 282 447 900 584 567 116 329 601, -73 287 275 433 929 198 978 602 374 360},
{119 506 412 601 094 191 987 103 656 491, 2 215 710 331 896 866 656 402 787 880},
{35 628 275 655 488 472 120 369 146 279, 1 701 819 546 753 781 725 174 126 090},
{27 593 641 411 576 971 180 162 904 361, 1 589 116 494 482 809 302 550 634 310},
{145 243 912 347 672 472 237 332 393 841, -407 853 589 571 860 453 254 340 980},
{12 056 649 482 627 870 575 538 245 211, -57 850 990 515 601 950 519 019 050},
{5 934 507 301 048 881 763 152 985 561, -334 525 389 817 169 030 904 094 950},
{21 824 378 630 700 359 073 301 608 289, 494 145 810 355 065 361 033 235 010},
{20 572 706 744 448 280 147 656 230 099, 1 086 135 782 896 623 860 440 214 010},
{16 032 155 777 480 873 377 666 858 841, -520 545 203 990 753 955 111 968 850},
{26 291 132 104 357 306 931 848 052 759, -1 322 542 051 269 788 080 156 959 990},
{40 086 939 180 652 122 494 077 907 291, 1 360 588 319 115 638 546 722 582 620},
{158 099 359 500 949 764 419 875 839 061, 1 373 587 896 778 770 100 942 129 680},
{34 324 594 219 191 905 694 262 391 111, 157 106 185 640 210 278 541 379 960},
{18 936 883 156 142 308 032 631 517 581, 956 320 286 399 644 070 690 856 150},
{47 570 165 534 493 918 677 586 960 169, -1 237 951 354 588 201 449 542 065 710},
{132 531 529 095 708 162 342 104 260 439, 6 082 646 083 719 593 158 019 420 190},
{322 957 871 276 844 670 715 068 918 991, 17 277 528 333 846 678 524 706 021 510},
{1 334 106 933 626 797 534 840 717 914 449, -31 374 288 139 317 093 681 364 742 820},
{3 761 851 547 323 210 857 949 472 729 561, -218 280 113 503 655 953 279 104 030 120},
{12 823 494 058 025 972 703 380 758 597 771, 388 478 692 526 780 108 025 443 362 560},
{927 998 365 199 513 773 823 035 956 041, 12 865 408 639 423 784 850 594 118 890},
{423 924 733 411 317 409 645 108 386 211, -13 553 300 627 057 996 598 916 403 730},
{946 875 907 102 398 284 753 667 515 831, -6 705 882 123 993 575 498 133 813 330},
{337 978 432 445 339 018 716 758 911 551, 13 448 387 200 828 341 136 206 593 430},
{443 956 858 582 253 068 210 113 026 051, -20 459 467 882 627 773 072 770 586 990},
{1 544 010 143 725 042 787 100 811 819 979, -31 878 823 329 098 047 040 088 357 870},

```

```

{3 470 482 606 012 468 823 319 231 196 969, -120 409 016 451 788 176 416 911 760 540},
{5 366 096 643 436 461 485 573 674 531 441, 78 454 893 361 339 473 238 951 141 230},
{7 822 137 611 209 703 636 574 228 878 051, 58 924 468 508 505 428 228 671 934 100},
{3 718 991 805 801 097 777 623 727 669 499, -121 508 178 331 727 824 649 681 782 590},
{11 988 192 343 098 661 415 618 305 288 541, 408 667 597 310 868 481 733 345 231 760},
{34 344 837 291 952 336 783 174 685 442 751, -48 448 887 578 595 098 400 522 453 990},
{1 361 424 319 168 583 681 729 343 475 909, -43 332 078 845 591 591 871 345 406 260},
{4 550 598 613 766 327 763 126 606 344 099, 1 573 182 903 110 670 873 832 138 140},
{155 500 758 143 611 792 312 093 025 171, -4 568 200 989 641 221 377 210 872 910},
{45 663 048 448 376 637 217 759 903 981, -494 124 795 273 998 062 847 845 110},
{51 095 388 075 372 674 375 296 619 111, -1 884 953 712 484 252 319 916 806 010},
{50 611 097 412 763 296 123 257 067 091, -1 290 840 216 550 866 448 833 300 570},
{67 350 570 787 155 659 308 344 560 111, -2 006 133 618 861 936 147 144 609 870},
{215 351 035 791 692 593 337 616 042 719, -11 243 814 155 755 843 810 008 204 030},
{431 360 274 915 221 797 812 501 703 399, 13 437 920 252 358 766 997 214 934 320},
{338 053 536 775 054 729 307 575 094 909, 19 319 152 386 328 301 257 673 668 410},
{2 416 614 498 075 875 589 707 805 716 689, -61 145 316 843 136 427 156 502 517 980},
{7 328 742 088 044 955 634 626 045 630 261, -419 540 323 146 764 921 957 169 342 960},
{49 335 705 232 037 942 299 895 866 785 191, 835 939 947 136 063 720 000 566 885 180},
{3 827 336 103 555 887 785 467 560 452 321, -148 866 679 065 435 785 388 817 112 490},
{10 842 585 588 506 101 295 062 802 577 169, -216 333 921 110 710 005 672 395 769 540},
{6 498 272 775 620 853 872 196 539 142 419, 68 205 039 473 912 606 558 272 200 360},
{4 717 300 425 388 218 539 330 707 162 969, 204 841 868 711 440 001 514 224 893 260},
{1 490 298 701 299 724 630 387 189 115 239, -62 339 321 032 593 665 574 689 756 370},
{1 467 095 874 113 359 194 746 624 447 891, 41 010 280 843 683 166 922 478 347 400},
{2 327 833 301 067 938 430 111 610 685 759, 821 755 986 169 155 939 559 747 590},
{50 553 345 069 367 011 949 713 414 461, -824 848 262 504 546 452 175 199 870},
{59 637 865 204 009 270 123 581 820 141, -323 994 655 620 980 183 161 687 200},
{5 734 991 006 978 021 879 675 210 591, 246 735 442 765 599 964 426 480 170},
{15 079 031 665 674 897 164 407 836 931, 653 256 297 558 439 247 556 508 050},
{13 588 342 279 529 412 122 646 097 031, -67 239 460 138 994 806 016 375 880},
{1 498 804 194 567 788 141 880 487 021, -37 949 798 946 809 616 473 001 660},
{4 709 270 946 195 487 957 788 992 531, 43 238 641 879 466 976 321 946 650},
{938 995 685 269 527 787 101 272 069, 33 465 207 514 051 335 481 039 140},
{494 438 593 898 688 801 676 213 399, 8 100 113 881 808 332 670 429 400},
{83 243 424 203 507 703 785 019 749, 3 448 281 045 177 766 555 385 520},
{121 654 458 929 567 920 397 584 519, -6 903 872 294 732 214 979 318 680},
{656 425 836 278 599 256 768 081 971, 6 811 978 073 899 467 908 852 820},
{621 461 237 246 834 717 071 024 001, 1 407 079 416 033 557 556 294 630},
{117 434 024 639 428 425 611 817 209, -2 278 453 426 130 838 228 107 880},
{262 433 933 363 165 724 697 930 301, 7 292 909 496 252 780 367 100 340},
{27 812 933 985 526 497 938 166 689, 1 144 253 415 663 725 140 266 330},
{88 063 854 408 870 737 515 467 019, 3 017 479 557 948 407 069 285 940},
{139 793 754 320 100 059 049 864 509, 5 508 610 749 691 291 054 846 290},
{521 699 880 032 263 452 355 522 009, 10 860 816 812 777 486 819 627 850},
{95 548 927 754 965 338 359 687 459, -3 360 525 821 940 354 245 358 180},
{365 005 389 899 490 291 904 263 169, -14 595 279 144 839 806 479 604 350},
{30 976 230 902 277 608 452 759 169, -1 802 432 404 286 873 419 080 120},
{84 054 887 379 590 842 427 679 379, -322 493 784 978 784 852 985 970},
{29 113 615 467 873 054 616 356 541, 912 495 117 992 098 954 912 680},
{21 643 305 276 402 097 153 153 969, 1 193 307 407 862 044 384 332 050},

```

```

{41 106 755 656 209 857 029 444 319, - 182 481 466 722 629 906 691 720},
{12 154 836 548 150 133 975 637 069, 685 769 726 022 796 275 404 520},
{47 443 648 585 309 944 392 717 041, - 2 011 532 997 542 781 646 672 620},
{209 118 982 284 920 596 983 885 589, 5 008 768 953 149 116 859 324 220},
{313 577 750 582 920 088 040 644 401, 17 099 015 048 728 998 195 904 800},
{1 454 665 406 155 328 249 103 858 251, - 54 757 002 117 611 838 596 395 950},
{5 967 186 406 068 039 642 706 932 149, 193 026 450 011 477 478 360 916 020},
{4 175 019 616 228 308 806 847 582 221, - 46 025 075 492 884 407 528 310 410},
{3 328 825 659 667 241 835 394 937 339, 14 133 295 684 104 230 667 285 480},
{1 664 662 567 120 507 123 193 421 191, 33 888 545 222 403 228 106 752 660},
{1 035 086 656 909 985 436 597 753 601, - 30 347 180 267 107 887 664 643 910},
{823 914 484 907 631 255 965 025 911, - 34 502 963 631 218 444 147 494 500},
{1 043 317 202 644 462 297 285 364 339, 55 994 431 300 224 081 097 995 270},
{5 164 825 007 008 606 137 712 993 541, 143 522 264 902 473 712 219 783 020},
{496 108 899 592 323 051 997 989 929, 27 809 232 841 538 346 154 526 940},
{1 118 780 180 397 161 874 657 242 741, - 26 742 616 853 325 982 534 075 980},
{1 106 841 588 074 877 335 261 053 169, - 34 486 156 885 147 798 088 010 090},
{824 426 505 287 096 907 627 302 539, 15 233 482 218 085 293 997 430 370},
{456 434 843 133 248 973 281 702 309, 4 826 464 708 242 084 623 648 970},
{521 905 341 587 015 557 202 410 091, - 26 239 276 411 795 640 514 482 100},
{722 926 848 873 210 524 895 209 159, 19 232 819 874 968 730 246 254 580},
{1 987 996 900 275 907 340 078 685 131, - 75 253 963 256 416 614 330 970 980},
{7 879 857 757 877 917 235 833 352 401, - 52 431 411 915 349 713 009 925 380},
{3 801 638 614 440 531 370 480 895 651, 16 710 009 897 669 414 263 228 490},
{2 069 154 199 251 865 465 335 217 319, 10 045 052 013 468 602 881 684 200},
{31 755 396 189 348 801 223 698 131, - 1 118 843 859 391 752 083 344 680},
{107 369 799 721 315 465 401 819 841, 1 497 154 703 300 534 511 565 380},
{106 760 067 997 077 877 152 767 269, - 5 740 973 327 407 257 530 768 850},
{581 924 731 138 663 998 892 061 131, - 19 623 585 726 588 396 836 773 680},
{1 702 493 005 405 964 458 998 466 519, 41 874 742 902 395 134 002 720 000},
{3 607 234 851 651 244 813 376 423 731, - 163 113 882 091 233 353 284 213 680},
{4 701 090 856 671 871 322 054 415 521, 75 901 555 703 608 386 615 234 810},
{1 206 204 834 914 010 670 625 817 449, - 21 126 552 285 058 603 458 849 270},
{499 830 021 083 238 641 323 673 809, 14 152 333 789 920 700 491 020 760},
{1 129 082 947 439 545 158 624 749 459, 43 531 801 179 078 995 647 387 740},
{688 714 687 343 690 780 040 277 031, 21 611 937 920 997 639 759 483 450},
{719 698 858 186 656 758 061 535 619, - 5 350 035 808 729 202 194 878 540},
{641 549 973 938 170 100 013 887 531, - 37 368 047 573 160 902 501 818 200},
{1 579 584 463 803 124 128 227 510 881, 60 367 850 788 749 696 510 828 300},
{2 515 106 167 203 636 755 439 745 331, 121 815 604 528 145 405 255 281 800},
{10 798 403 499 741 605 485 214 289 719, 399 783 342 375 566 824 168 445 880},
{1 067 567 155 926 609 399 228 990 709, 53 851 857 584 206 596 082 302 660},
{2 376 968 935 138 153 126 682 685 241, 119 977 637 196 576 663 912 019 380},
{5 668 536 007 138 418 040 983 292 109, - 303 759 329 078 942 585 749 750 500},
{25 825 702 585 734 263 153 753 815 141, - 924 842 422 303 727 173 288 167 750},
{17 541 194 931 294 522 277 035 346 609, - 582 397 106 189 814 893 226 485 220},
{17 389 718 145 618 945 540 438 292 259, - 690 007 893 485 029 694 188 771 320},
{35 019 722 931 793 999 615 471 324 009, - 1 581 386 818 102 534 807 000 212 750},
{57 532 446 318 096 699 228 127 520 759, 1 902 413 012 790 682 394 906 305 410},
{115 474 039 528 433 072 615 527 973 209, - 5 553 064 884 577 468 863 793 724 040},
{286 221 084 971 137 154 559 198 139 381, - 8 778 062 634 396 749 880 260 172 090},

```



```

{867 200 472 952 853 463 836 272 436 839, 26 655 083 941 561 581 631 153 253 520},
{3 116 741 576 788 361 227 938 017 259 571, 14 914 374 754 557 206 144 395 199 820},
{91 049 475 437 808 916 385 455 205 059, 40 090 065 057 660 537 273 834 060},
{1 239 360 657 320 895 381 091 754 549, -10 285 068 673 127 763 499 440 900},
{1 288 295 684 018 564 587 489 182 101, -36 100 348 102 572 555 343 453 110},
{2 840 528 766 185 898 623 657 594 609, -105 459 242 232 686 557 648 455 180},
{1 724 564 298 256 246 645 524 508 001, 86 497 269 312 743 823 092 486 340},
{1 350 653 087 656 083 897 629 918 549, -78 840 843 006 837 968 834 499 360},
{2 600 047 891 499 445 288 300 786 679, 99 760 961 773 450 513 925 164 320},
{1 571 984 232 822 713 487 875 104 109, 51 088 700 105 693 271 623 951 910},
{2 953 133 083 898 261 049 318 680 351, -116 555 636 448 844 112 814 420 330},
{9 849 785 341 966 715 468 501 197 351, 176 164 759 208 799 402 209 572 920},
{3 875 734 605 238 814 863 956 428 419, -210 009 442 163 142 535 177 221 270},
{23 986 726 221 864 556 922 377 835 309, -1 107 460 979 734 191 715 601 936 910},
{94 731 248 404 202 866 037 058 954 461, -5 088 793 302 463 495 032 496 368 840},
{490 911 909 993 488 434 673 385 428 249, -13 556 947 199 998 869 888 966 730 500},
{718 314 509 175 808 786 316 365 692 499, 31 379 205 035 226 062 569 106 943 300},
{855 208 865 232 053 846 046 594 853 651, -5 533 138 399 333 798 998 694 911 990},
{609 324 252 835 934 686 530 242 704 549, 5 093 339 362 334 260 536 015 174 060},
{470 994 131 688 321 025 686 123 845 401, 16 336 564 535 939 281 649 137 340 130},
{694 326 203 333 453 676 853 613 610 619, -34 105 113 261 090 749 810 715 370 200},
{3 068 208 466 021 308 840 465 857 861 369, -125 866 131 503 088 561 368 275 353 090},
{11 902 748 796 743 025 274 439 596 189 459, -294 334 442 134 206 269 452 518 067 650},
{32 472 148 955 068 398 581 057 244 348 209, -136 411 492 064 310 719 424 149 408 520},
{1 559 674 784 374 286 885 530 965 232 699, 61 133 060 567 426 190 000 363 339 960},
{7 475 982 385 077 307 674 098 883 171 511, -154 155 109 239 005 906 065 579 136 850},
{19 210 822 542 861 069 920 722 235 280 461, 341 009 799 571 850 882 592 784 033 260},
{28 682 715 476 192 544 377 108 683 893 151, -111 865 435 530 800 113 958 271 077 490},
{11 336 159 057 236 516 151 613 301 983 461, 375 083 275 629 749 784 985 434 647 940},
{20 998 857 874 349 673 114 615 898 860 511, -1 227 396 529 118 570 305 955 204 964 600},
{33 412 336 712 828 456 257 731 030 040 061, -576 537 547 272 166 892 929 038 176 190},
{6 737 098 268 263 106 570 449 228 918 709, -230 632 003 693 183 502 005 984 154 910},
{12 241 310 451 357 038 081 197 795 006 069, 635 560 465 952 955 727 324 088 700 390},
{41 581 061 160 970 694 772 067 534 363 409, 490 542 633 347 795 999 840 953 085 250},
{28 880 731 071 583 268 817 782 948 593 091, 1 141 486 509 025 635 606 476 889 070 530},
{86 235 654 831 537 042 621 041 179 290 091, -2 084 296 826 163 533 697 307 180 363 410},
{195 650 724 666 872 418 893 142 881 960 531, -8 698 430 537 820 677 269 224 573 630 450},
{1 075 598 461 539 197 261 520 767 784 748 381, 2 172 880 763 944 680 227 785 684 978 860},
{5 643 330 031 717 740 480 283 773 382 931, -278 720 559 803 834 365 582 632 074 010},
{17 298 627 745 904 345 326 414 107 585 481, 338 351 843 111 806 242 513 890 209 110},
{10 713 620 547 758 966 509 632 437 138 621, 412 493 160 653 989 623 686 739 162 030},
{2 811 608 940 435 690 261 918 049 613 909, -32 729 102 534 750 046 874 404 440 370},
{776 563 265 756 256 089 463 796 735 661, -45 648 329 790 502 214 079 614 089 500},
{135 956 488 747 330 977 699 660 754 411, -1 636 207 670 835 899 928 056 959 350},
{37 964 269 055 772 201 404 215 218 611, 2 230 020 127 193 539 705 143 628 680},
{13 535 650 263 988 630 610 156 293 801, -26 102 417 855 740 118 201 510 700},
{2 887 655 388 263 174 843 367 634 249, -5 916 908 288 950 095 243 728 730},
{51 239 957 137 619 471 431 516 259, 3 060 352 275 302 774 046 214 380},
{197 293 917 174 449 525 886 178 451, 10 022 806 001 414 194 987 109 610},
{793 712 916 312 427 837 859 450 999, 45 660 005 250 879 881 606 624 580},
{4 390 699 588 914 932 487 255 117 889, -84 604 533 359 251 077 647 102 160},

```

```

{2 192 772 587 297 011 148 942 802 181, 6 903 661 491 793 031 530 174 830},
{650 533 540 386 392 290 851 233 509, -22 252 752 945 951 663 230 001 390},
{1 306 129 943 402 308 352 479 492 949, 34 560 360 663 714 284 958 306 030},
{1 798 104 216 527 453 459 970 183 941, -78 136 343 990 914 401 171 384 330},
{243 044 488 841 980 490 114 432 101, -4 051 429 169 295 870 044 359 080},
{10 356 590 258 699 849 325 287 449, -595 325 437 168 030 665 028 260},
{59 250 514 537 675 332 971 564 279, -710 253 817 879 044 443 664 990},
{75 161 361 082 375 680 989 897 359, 1 394 883 941 146 333 062 152 910},
{40 755 306 621 102 395 956 305 031, 607 088 149 087 832 736 746 550},
{20 180 558 686 618 251 165 831 431, 421 930 529 777 113 722 501 960},
{18 098 792 413 485 086 079 924 899, 92 348 770 259 501 618 102 070},
{393 205 901 684 998 088 286 071, -10 157 725 887 409 228 276 980},
{739 297 388 914 415 443 553 399, -12 915 696 107 062 331 527 650},
{778 780 413 777 499 165 814 599, 16 006 629 583 028 587 776 300},
{1 391 653 383 516 310 441 249 351, -25 670 255 890 998 170 498 580},
{1 370 350 916 004 717 815 833 781, -55 542 707 821 736 633 687 310},
{4 572 411 664 213 204 613 591 219, -267 868 376 928 565 496 681 010},
{4 680 963 363 325 383 673 526 299, -97 639 469 741 727 616 357 110},
{1 438 527 253 663 019 815 360 231, -79 273 645 481 169 122 633 880},
{2 912 010 385 495 877 595 548 141, -58 889 162 395 160 185 935 270},
{6 636 798 461 390 149 664 697 661, 290 434 274 641 029 620 596 500},
{10 840 653 693 736 433 864 481 589, -340 045 940 965 331 613 031 980},
{10 244 920 705 698 615 887 984 521, -362 944 841 475 045 466 692 120},
{20 698 751 243 733 047 971 895 411, 437 155 070 814 118 732 006 590},
{38 268 191 782 836 359 464 005 931, -47 376 363 672 846 928 036 230},
{2 989 426 270 813 555 706 245 159, 100 503 106 165 773 561 863 820},
{6 442 395 454 072 438 567 029 691, 183 965 370 445 474 144 927 770},
{905 479 608 691 717 133 992 991, -36 619 457 791 154 907 791 940},
{2 511 715 857 876 045 762 182 759, -114 873 655 474 789 693 346 430},
{3 891 645 204 901 200 351 113 951, -5 198 854 776 921 046 029 930},
{576 552 776 178 444 451 208 369, -4 390 568 210 798 869 550 400},
{348 473 481 511 927 566 598 219, -19 126 981 152 334 974 494 580},
{1 051 143 013 244 404 449 640 529, -26 756 591 552 329 304 951 520},
{1 916 621 618 593 950 689 343 499, -72 634 327 536 101 360 644 890},
{7 060 404 766 484 143 456 666 109, 333 991 540 946 664 778 529 550},
{11 692 184 057 649 959 993 935 309, -16 455 109 916 734 171 089 150},
{1 857 172 380 156 948 263 035 591, -87 250 505 280 043 813 317 720},
{6 252 854 088 283 074 024 231 221, -226 637 555 146 477 616 527 950},
{23 342 361 410 393 108 876 396 129, 1 087 552 850 786 338 617 688 050},
{126 441 637 513 879 474 141 716 829, 949 931 852 172 124 368 277 890},
{25 275 994 921 720 223 350 122 209, -228 889 823 828 374 557 427 440},
{24 626 689 450 354 530 309 056 059, 1 417 234 578 491 205 947 997 960},
{133 959 105 617 011 327 465 775 489, 3 482 812 638 633 425 507 600 220},
{404 668 562 584 230 702 418 749 379, 3 584 283 868 764 386 845 405 560},
{89 234 161 122 397 789 131 804 151, -3 758 493 974 433 095 757 965 040},
{243 393 260 263 123 773 898 559 059, 12 475 494 146 058 338 266 688 400},
{1 535 272 287 168 790 850 237 444 191, -11 871 475 058 717 272 982 228 490},
{966 853 153 159 921 518 022 214 231, 24 823 343 786 820 194 836 454 190},
{315 570 886 042 586 230 474 293 929, -7 249 386 464 769 936 429 065 640},
{853 931 720 230 034 073 553 151 981, -17 547 937 279 871 054 785 409 100},
{1 485 218 827 395 550 343 905 373 669, -33 372 605 488 073 447 782 755 150},

```

```

{4 153 653 311 506 456 385 970 628 331, -63 170 002 048 515 829 018 578 660},
{3 907 272 747 592 670 643 146 370 479, -22 489 655 322 622 757 011 249 920},
{1 487 746 914 465 958 279 590 015 851, -45 283 915 963 201 728 847 247 040},
{1 662 200 392 244 391 864 653 253 719, 42 108 840 078 733 189 435 645 050},
{5 008 862 922 623 166 642 437 289 019, -206 720 894 088 606 849 725 347 710},
{11 937 927 588 647 164 506 264 938 729, -520 562 759 909 890 329 802 777 890},
{8 788 988 209 358 582 878 937 137 991, 402 144 614 617 818 160 393 053 870},
{14 606 521 370 587 579 077 221 834 399, 318 065 017 072 612 236 825 517 890},
{6 141 823 102 898 538 004 749 123 791, 180 666 955 723 409 335 797 538 680},
{214 201 316 042 232 504 165 023 579, -6 705 004 807 564 216 306 898 910},
{90 068 287 755 426 831 591 126 791, 3 595 303 529 703 664 161 214 530},
{46 610 577 721 642 117 751 648 791, -78 446 423 586 240 845 962 230},
{3 363 929 965 178 867 771 126 921, 11 051 459 984 765 287 211 640},
{1 075 818 582 365 335 155 878 611, -54 929 218 569 415 710 196 620},
{5 714 213 044 767 741 061 501 039, 127 760 447 135 914 427 078 220},
{8 786 776 163 450 447 411 734 111, 488 708 772 905 064 830 907 510},
{2 505 418 959 020 605 694 868 319, 109 608 741 679 126 035 363 690},
{3 911 106 999 422 572 742 634 301, 68 522 129 288 184 862 609 080},
{1 341 753 129 004 929 053 101 991, 39 582 164 060 208 242 140 470},
{1 014 152 709 579 946 098 171 239, 4 381 464 579 633 220 754 970},
{510 632 312 852 698 047 065 419, 1 176 099 765 002 371 986 210},
{51 458 725 258 819 867 620 029, -20 330 987 195 903 863 050},
{250 163 162 784 750 360 229, 9 818 728 114 064 031 720},
{1 178 434 943 220 541 374 479, 70 071 190 723 792 674 930},
{3 206 600 070 067 458 932 081, 42 043 864 157 095 669 350},
{2 827 864 926 175 203 431 731, 75 263 364 216 115 829 520},
{8 067 871 423 336 720 597 279, 394 644 004 073 780 807 880},
{43 922 826 807 137 214 359 429, -689 419 838 310 547 839 150},
{50 210 754 029 199 683 888 921, -992 895 505 979 683 542 120},
{107 156 110 716 808 366 558 949, 5 874 209 815 319 816 328 690},
{356 503 844 303 969 833 274 779, -16 924 079 458 982 376 154 260},
{275 642 092 000 323 442 865 069, 1 995 880 660 968 301 965 270},
{52 850 757 461 140 686 110 059, 1 936 981 429 324 964 275 440},
{138 616 976 211 029 318 967 929, 5 717 122 411 579 947 469 710},
{352 915 621 610 755 503 417 139, 838 625 533 775 526 110 430},
{36 577 755 293 988 257 546 641, -646 532 390 632 787 314 890},
{68 922 333 992 235 469 924 339, -2 474 953 199 542 025 216 010},
{94 465 254 330 250 267 109 191, 226 521 432 008 724 715 860},
{1 460 112 835 627 209 488 321, -35 166 511 762 721 003 520},
{4 237 045 260 175 237 539 269, 217 658 664 835 915 528 830},
{25 484 187 701 503 465 366 249, -194 214 404 320 147 673 130},
{10 567 284 626 594 166 740 969, 510 045 125 663 551 920 600},
{36 059 416 097 446 321 499 381, 1 275 384 564 829 700 397 300},
{87 510 718 835 892 304 120 231, -4 121 376 687 425 849 010 030},
{241 413 908 387 318 202 309 851, 4 287 523 401 544 800 851 550},
{329 462 073 103 148 010 385 801, 12 964 074 132 167 769 067 740},
{1 345 415 169 537 399 706 767 551, 37 850 727 801 839 820 622 140},
{4 319 968 863 537 292 743 001 739, -206 575 760 691 523 736 233 080},
{4 548 649 857 161 135 191 128 191, 202 499 627 161 161 799 621 230},
{23 508 172 963 509 475 464 743 881, 252 054 225 040 787 995 917 990},
{16 849 638 713 764 152 937 073 561, 834 678 199 179 371 710 561 260},

```

```

{39 174 757 274 356 400 187 938 611, - 1 196 657 744 547 980 544 411 090},
{79 052 022 227 466 402 184 467 109, - 1 989 270 016 336 349 875 081 050},
{130 213 384 922 885 797 512 497 641, 1 279 485 152 334 712 621 448 190},
{73 819 254 428 977 358 679 652 489, - 3 522 108 760 731 802 748 337 570},
{36 402 416 144 015 257 894 556 731, 819 361 425 543 364 024 560 780},
{87 978 868 446 917 444 284 485 161, - 4 648 334 252 960 118 164 690 820},
{85 210 072 190 525 012 004 745 169, - 4 482 242 177 573 254 672 049 730},
{11 915 174 974 926 482 185 875 049, 15 567 635 318 765 782 604 070},
{1 489 422 973 735 281 934 136 249, - 8 934 541 624 394 448 967 770},
{664 014 862 186 351 913 816 591, 20 368 815 306 530 166 583 830},
{2 047 166 775 215 039 445 899 549, 25 734 403 421 385 760 832 040},
{2 907 960 122 451 176 586 576 401, 144 398 883 850 383 809 439 030},
{5 015 593 806 318 599 846 746 051, 275 718 048 145 620 136 754 730},
{13 219 903 864 056 783 675 388 661, - 317 770 316 066 694 086 965 290},
{31 738 802 096 836 362 265 533 269, 97 220 563 788 390 221 570 820},
{11 269 473 757 108 658 394 933 199, 157 278 527 464 927 553 463 360},
{13 699 635 311 897 489 061 608 971, - 179 151 730 086 488 730 624 240},
{21 110 060 156 410 729 075 849 481, 448 981 423 437 917 063 350 500},
{1 991 246 961 985 401 692 371 231, - 116 546 380 160 156 005 474 320},
{2 499 583 314 950 149 426 255 541, 24 846 412 284 664 590 851 220},
{2 485 985 776 044 536 679 137 429, 3 275 771 162 965 018 481 550},
{81 458 698 123 999 438 114 271, - 4 386 214 205 101 774 136 130},
{471 722 315 006 501 888 521 949, - 26 683 298 280 016 975 150 770},
{2 152 840 562 484 719 712 169 661, 7 405 721 917 402 693 152 690},
{558 353 385 345 462 811 045 379, 9 756 801 481 680 039 703 170},
{556 140 923 314 837 539 136 939, - 10 470 815 665 918 275 309 120},
{298 110 948 313 405 886 148 329, 8 503 774 849 576 910 356 260},
{120 185 973 131 719 943 486 479, - 5 916 257 372 881 346 732 370},
{467 067 244 197 345 218 608 829, 22 288 195 422 119 129 829 120},
{247 199 776 456 283 458 475 441, - 10 182 738 174 502 345 851 150},
{706 329 127 325 016 670 008 091, - 23 213 040 395 646 565 581 750},
{2 494 416 779 360 545 341 453 341, 136 276 134 064 533 572 335 350},
{10 403 037 915 934 200 893 677 291, - 609 637 956 912 546 454 141 590},
{9 837 354 753 648 704 490 835 511, - 167 798 343 495 584 235 521 190},
{15 749 625 660 282 116 633 589 449, 704 025 907 486 475 872 117 350},
{65 524 979 590 491 509 198 944 999, - 3 417 927 170 851 294 533 891 960},
{146 675 199 423 545 176 804 437 509, 1 114 396 262 187 262 839 823 770},
{106 701 903 478 553 031 127 332 881, 857 280 405 518 941 722 320 190},
{100 182 431 745 268 647 466 959 571, - 354 543 085 044 709 897 465 650},
{38 468 591 918 447 632 470 664 129, 1 631 360 587 197 680 246 832 120},
{171 699 605 748 470 056 779 994 501, 965 797 191 398 330 029 188 480},
{53 285 874 428 604 792 304 289 689, - 399 569 747 716 043 593 678 020},
{35 917 593 575 119 580 623 370 279, - 1 554 398 840 740 843 885 193 010},
{41 771 479 758 122 987 246 693 299, - 730 751 918 351 057 584 790 850},
{29 773 723 440 288 933 317 327 099, 1 629 111 389 704 211 456 661 090},
{112 879 324 828 894 901 454 297 229, 4 160 375 763 942 687 937 202 490},
{137 843 979 813 024 114 607 329 749, 6 305 624 133 616 359 059 126 880},
{220 817 532 760 481 958 058 864 361, 840 370 226 706 324 390 052 920},
{50 159 052 683 620 487 788 453 349, - 1 104 220 457 863 070 597 003 970},
{117 752 152 025 360 041 741 949 449, 4 319 912 945 755 834 116 822 930},
{279 740 124 978 082 667 520 315 089, 14 375 759 030 294 599 101 429 990},

```

```

{1 656 776 554 023 806 432 879 465 029, 43 935 679 261 890 694 160 476 830},
{3 207 593 739 938 026 249 882 282 261, 90 098 902 660 188 105 949 740 240},
{9 027 655 713 015 136 641 399 961 129, 44 231 604 402 490 920 886 018 530},
{1 106 512 141 654 183 943 697 433 259, - 7 072 860 586 506 101 105 491 650},
{789 618 429 967 274 981 424 700 609, 17 869 383 549 306 229 741 035 480},
{844 754 003 248 019 077 604 011 739, 42 684 257 778 711 543 735 780 000},
{2 241 719 233 879 161 075 008 653 511, 3 634 088 997 559 056 225 133 200},
{128 933 081 308 930 590 531 253 139, - 2 946 960 232 712 972 108 759 670},
{184 025 401 540 485 745 797 257 591, - 8 145 290 638 029 899 957 110 650},
{832 387 066 684 690 257 288 127 109, - 44 790 424 401 725 637 026 263 020},
{4 676 380 233 972 308 398 928 438 021, 63 798 355 975 027 167 069 855 420},
{4 794 162 196 626 625 910 077 082 611, - 30 820 798 341 351 441 819 872 820},
{3 484 468 500 673 952 469 592 404 559, - 176 916 052 114 225 982 365 988 310},
{13 516 987 944 252 361 609 567 771 891, 785 370 376 111 307 614 700 136 600},
{41 588 579 140 393 172 076 027 872 441, - 1 701 896 028 220 380 308 805 342 600},
{186 511 690 239 115 210 839 612 160 291, - 3 623 459 114 009 998 631 340 469 230},
{430 534 131 575 925 440 953 305 619 811, 16 760 491 670 341 889 807 586 186 210},
{1 314 901 615 093 887 205 027 740 633 899, 36 424 591 644 777 833 883 396 796 980},
{907 695 286 353 181 491 589 441 597 369, 29 456 480 488 569 536 583 620 642 100},
{1 369 357 806 911 009 768 202 375 240 481, - 28 504 732 790 861 303 711 065 730 250},
{283 788 870 366 464 707 876 267 308 731, 2 218 640 887 125 919 346 294 791 980},
{49 487 959 598 895 080 815 982 241 959, - 878 679 127 234 728 425 690 307 600},
{70 764 046 911 322 533 308 579 106 109, - 644 251 410 691 432 534 754 447 580},
{26 005 674 448 496 424 116 942 050 441, 78 211 096 878 563 743 567 144 620},
{9 693 823 828 390 925 220 194 112 769, 65 628 836 784 770 732 371 790 070},
{4 830 247 954 540 935 878 535 215 341, 269 455 673 997 104 797 491 996 600},
{5 008 498 529 144 569 556 501 588 209, 11 287 236 288 810 556 761 379 410},
{761 630 154 916 729 033 268 327 581, - 11 120 037 286 039 384 797 289 080},
{1 372 372 485 978 767 630 220 205 391, - 2 643 431 109 943 387 257 787 170},
{108 366 719 455 560 500 594 704 411, - 2 939 133 826 835 755 848 413 340},
{95 689 266 477 978 914 943 881 419, - 5 680 077 321 033 585 397 131 210},
{218 884 042 877 601 238 644 636 901, 12 981 680 640 330 306 774 309 090},
{452 936 530 011 508 106 173 024 879, - 10 251 426 297 749 266 839 849 390},
{470 317 000 545 631 670 132 581 469, 12 698 615 810 638 026 317 175 330},
{117 522 103 558 198 795 670 659 009, - 1 195 340 818 037 858 600 895 960},
{95 054 551 012 651 848 496 587 179, - 4 641 900 746 353 338 198 041 340},
{556 350 557 481 856 218 475 855 129, 31 812 398 881 257 761 602 228 320},
{3 900 483 901 619 042 080 731 395 939, 59 626 103 953 819 830 792 726 930},
{6 221 573 299 809 022 880 240 517 739, 93 865 319 956 930 006 487 166 030},
{6 642 007 845 562 255 473 977 499 509, - 255 769 077 288 775 250 525 109 570},
{2 005 029 150 421 160 958 512 677 061, - 26 799 725 561 771 108 005 958 370},
{1 242 516 944 629 707 625 484 372 939, 43 871 055 247 156 498 324 620 720},
{3 545 976 825 040 743 771 143 187 529, - 7 735 346 237 743 388 614 566 900},
{800 250 286 722 218 203 558 379 579, - 28 623 013 110 519 139 327 894 500},
{299 714 173 451 742 103 289 271 671, - 15 928 354 335 412 693 376 999 130},
{734 064 289 195 866 789 301 661 549, - 37 874 372 928 131 768 095 500 990},
{3 627 252 093 902 162 067 272 827 489, 31 326 745 538 635 229 543 459 250},
{1 669 247 533 460 664 501 879 823 261, - 82 058 492 153 707 686 327 023 880},
{7 047 500 287 014 204 610 175 760 911, - 380 744 452 292 871 023 754 117 960},
{46 847 720 944 136 555 129 272 562 579, 378 261 184 834 757 974 518 640 170},
{14 223 159 818 731 861 470 743 443 751, 255 281 233 844 382 941 036 399 010},

```

```

{18 219 908 414 949 390 051 020 103 059, -922 919 093 322 710 453 572 447 680},
{59 856 836 327 709 574 127 641 485 791, 2 718 178 979 374 064 234 987 848 320},
{14 281 594 151 520 400 435 114 510 501, -522 453 939 041 371 923 923 083 680},
{44 009 787 148 242 980 787 004 036 391, 367 409 353 134 513 988 744 352 070},
{19 913 142 202 573 163 441 871 214 259, 602 469 004 713 487 737 475 680 960},
{7 947 926 804 045 094 398 609 387 329, 177 445 859 200 560 427 643 819 130},
{9 321 351 855 011 336 185 980 853 771, 25 321 316 809 147 096 369 623 570},
{779 924 580 546 385 211 804 382 761, 16 821 258 878 288 391 640 293 630},
{1 542 814 708 424 918 284 069 821 031, -19 067 801 681 859 180 390 587 760},
{420 984 179 224 507 219 514 669 779, 5 918 975 971 970 709 843 070 110},
{184 958 188 861 291 984 829 684 219, 4 523 687 645 138 650 659 739 920},
{128 764 151 937 565 747 132 777 751, 3 424 589 521 975 412 033 832 300},
{343 932 724 272 477 448 365 261 899, 3 685 465 409 114 975 803 371 570},
{297 294 747 420 959 361 578 178 139, 1 187 662 355 793 978 315 670 650},
{95 168 776 588 660 447 789 425 389, 2 359 642 781 758 082 031 134 730},
{196 549 394 902 628 802 553 083 439, 4 971 349 468 403 681 787 675 480},
{578 450 542 213 135 707 437 876 011, -3 333 446 469 350 893 581 234 540},
{393 855 006 933 863 699 930 421 199, -10 642 401 309 604 587 454 462 920},
{21 625 778 101 984 992 938 582 909, -1 191 480 182 803 518 135 195 510},
{44 962 837 691 938 292 770 995 979, 1 884 957 472 716 676 572 991 710},
{69 311 554 968 748 190 182 070 311, -922 098 573 959 902 644 264 900},
{38 694 642 360 628 457 412 905 561, -203 859 430 697 770 406 273 400},
{9 701 017 458 927 864 539 150 189, 151 414 133 886 263 641 243 920},
{2 638 735 441 954 866 384 366 559, -156 843 845 926 969 375 467 750},
{6 930 094 639 706 862 644 882 941, -390 506 549 533 404 720 269 790},
{24 854 836 225 500 002 313 293 029, -15 875 442 593 511 985 828 920},
{1 532 825 860 881 641 193 718 441, -45 802 029 275 038 122 097 140},
{5 361 082 596 151 174 292 718 071, 37 493 846 872 340 190 541 200},
{134 914 154 961 711 623 055 779, 6 159 952 688 778 054 386 880},
{151 805 852 042 798 937 350 831, -3 897 436 799 079 339 375 330},
{48 739 963 445 119 870 046 789, -426 294 759 389 183 468 730},
{35 732 579 562 991 607 503 819, -229 328 541 969 091 974 480},
{10 710 919 030 871 869 280 311, -47 064 617 857 609 737 870},
{4 973 274 006 450 889 466 299, -75 085 315 630 528 224 030},
{4 428 436 883 842 696 760 069, 208 214 599 646 230 512 990},
{14 038 503 109 235 852 807 029, 246 693 628 377 790 591 020},
{5 781 460 782 850 931 158 861, 270 911 682 343 940 653 680},
{23 171 178 860 672 535 326 831, -1 237 757 952 803 969 612 070},
{86 901 782 893 324 712 927 249, -922 772 188 802 199 619 530},
{40 460 483 625 405 121 548 679, 508 070 732 494 011 155 730},
{46 478 918 503 058 498 339 971, 244 978 283 885 127 619 260},
{16 805 814 214 053 079 176 679, 779 005 402 479 834 634 710},
{83 408 464 766 323 979 522 191, 3 852 428 279 531 178 852 390},
{337 584 303 223 850 762 827 639, 1 409 817 858 281 873 930 190},
{160 096 608 715 206 271 569 479, 9 433 331 407 987 859 874 030},
{67 776 330 367 423 918 546 781, -2 345 251 059 799 336 469 970},
{59 223 542 055 966 609 669 599, 1 141 602 785 104 138 913 460},
{35 090 495 131 602 071 410 571, -1 344 649 385 966 653 423 620},
{32 532 385 213 739 681 509 201, 777 965 906 675 045 408 490},
{35 687 899 519 668 637 492 129, 942 913 349 434 995 852 030},
{35 844 747 474 162 426 137 761, -1 038 448 587 195 898 591 380},

```

```

{125 739 222 501 200 164 695 289, 5 164 525 762 218 020 561 490},
{449 441 656 199 885 476 101 779, 7 060 936 579 999 882 873 110},
{617 029 514 946 863 972 092 511, -2 329 939 102 910 601 522 690},
{101 491 178 435 803 286 505 089, 2 554 567 629 139 736 907 030},
{173 573 209 176 333 633 803 861, 1 923 383 787 082 528 118 700},
{117 635 753 065 431 883 336 111, 4 727 624 873 489 374 515 480},
{139 272 061 722 422 367 273 139, -4 763 359 306 551 559 991 910},
{284 795 099 939 209 004 444 999, -4 229 261 895 957 674 832 960},
{360 072 780 421 242 449 806 429, 14 369 946 648 216 594 436 290},
{206 852 668 172 724 813 693 929, -2 763 656 622 474 174 895 230},
{105 816 206 722 414 165 528 571, -1 926 733 942 182 791 026 920},
{38 694 184 507 474 578 959 279, -1 994 088 076 043 451 134 430},
{202 434 276 724 900 858 682 359, 7 585 862 381 968 430 476 740},
{598 385 904 649 937 811 594 871, 26 994 688 605 802 943 931 270},
{1 130 191 585 890 534 321 839 681, 21 533 856 646 971 266 352 270},
{2 618 191 102 255 146 351 931 891, 85 167 491 895 267 378 382 860},
{5 522 287 771 033 736 862 129 019, -255 939 827 495 429 154 799 620},
{27 205 496 900 291 840 409 117 871, -792 163 618 070 008 222 867 980},
{68 255 405 363 801 768 733 244 301, -3 040 670 279 248 265 183 146 260},
{341 525 464 305 323 610 710 671 831, 12 367 515 502 448 220 325 439 910},
{1 196 007 410 569 866 158 813 057 899, 40 633 652 615 025 243 400 710 930},
{4 425 502 668 267 659 148 302 673 179, 149 100 507 914 898 983 887 113 900},
{11 925 654 864 006 902 445 996 699 071, -364 423 526 777 557 673 285 408 520},
{25 180 701 432 777 693 877 867 304 339, 1 180 937 533 916 280 815 033 658 420},
{95 634 318 354 484 987 302 279 857 269, -774 991 004 934 989 911 724 201 400},
{77 916 611 617 788 268 210 974 352 319, 1 044 848 674 491 273 085 169 042 070},
{112 206 781 233 360 507 352 654 535 681, 5 966 364 137 018 361 644 852 199 030},
{289 688 479 867 079 338 783 848 718 139, -8 720 191 106 619 342 454 854 759 720},
{482 465 510 508 900 481 184 053 492 129, 2 509 649 689 328 105 782 933 322 340},
{153 805 309 633 946 886 074 756 315 099, 4 896 510 959 100 273 443 549 001 360},
{505 380 945 361 440 740 509 055 507 689, 20 942 309 631 123 039 488 435 577 960},
{694 144 067 836 435 989 437 010 798 899, 29 697 852 029 954 544 920 236 801 350},
{2 784 461 258 017 845 524 162 656 330 099, 132 469 902 180 829 635 746 954 358 510},
{650 921 367 326 216 542 630 315 148 639, 29 615 903 767 386 337 049 938 192 920},
{157 757 404 627 000 989 549 598 995 851, -4 537 970 350 418 023 931 856 419 100},
{268 960 967 045 091 864 409 293 834 899, 13 895 038 443 583 538 251 504 912 650},
{1 243 764 390 868 164 045 305 824 131 799, 68 541 383 606 268 135 944 391 836 340},
{2 514 890 974 789 737 174 999 540 497 429, 70 566 301 546 009 017 463 808 090 250},
{6 399 466 097 513 450 878 085 238 644 321, -119 983 890 102 920 332 105 812 068 760},
{10 120 300 436 726 992 395 776 949 010 291, 123 985 128 171 953 999 340 420 771 990},
{11 666 498 416 682 123 084 526 127 515 139, -443 418 744 824 990 743 659 780 462 750},
{34 540 373 859 323 301 092 330 706 393 389, 166 846 547 141 960 332 581 845 597 340},
{787 788 835 315 574 220 055 603 746 259, -21 839 183 156 465 835 671 137 587 810},
{396 138 662 383 838 109 557 296 859 849, 10 646 083 885 468 159 928 501 604 210},
{560 623 214 000 564 242 887 113 523 829, -8 103 290 566 922 501 231 102 238 090},
{375 537 385 610 826 143 205 833 000 369, -14 103 340 366 809 588 576 882 674 940},
{1 318 453 877 551 219 840 869 804 975 761, 73 087 598 667 592 808 598 064 222 680},
{722 152 485 171 870 812 266 890 847 771, -39 691 540 204 143 250 592 782 566 510},
{1 933 895 135 820 367 700 797 967 298 341, -23 434 259 732 886 838 910 424 931 620},
{2 798 253 924 319 222 120 592 808 555 869, -138 148 692 034 964 967 826 436 267 640},
{8 855 300 988 600 613 780 084 883 970 319, 251 961 082 947 329 499 006 867 860 670},

```

```

{9 202 434 446 464 410 025 971 720 564 119, 548 355 710 400 655 866 613 704 882 180},
{30 022 770 217 031 666 321 776 870 668 191, -1 278 884 715 281 357 154 200 751 874 440},
{152 713 863 155 673 395 565 053 966 573 821, 7 547 689 867 023 312 881 783 159 793 900},
{441 776 519 616 991 620 277 083 444 651 071, -6 400 923 800 857 430 414 459 243 217 780},
{28 307 116 815 059 341 528 311 318 687 001, 445 475 046 918 897 358 922 347 913 970},
{51 024 833 125 272 450 122 455 899 576 829, -2 039 695 391 594 938 021 277 510 583 810},
{8 144 532 185 148 897 220 051 880 376 329, 71 189 305 884 095 035 514 852 780 310},
{7 266 779 904 877 856 011 024 518 668 239, -370 812 271 191 944 041 729 907 365 260},
{37 515 845 259 217 230 716 980 787 877 211, -1 089 396 876 267 684 377 179 292 605 170},
{119 564 217 995 106 435 114 094 664 659 181, -1 918 280 257 090 499 727 644 042 082 000},
{158 341 355 929 358 452 041 177 949 370 431, -8 356 802 908 126 431 515 612 881 196 250},
{109 912 730 585 980 435 622 165 132 938 069, -4 359 230 270 250 115 821 774 939 672 450},
{233 925 431 261 612 559 525 701 922 831 569, -3 757 417 051 557 180 249 289 739 406 720},
{242 359 090 331 913 401 504 257 983 347 179, 12 806 644 475 857 986 468 974 227 692 990},
{242 755 832 056 473 692 969 338 047 727 381, 6 157 418 822 822 279 107 770 438 430 740},
{656 740 989 567 606 749 339 028 181 058 771, -24 386 655 314 492 603 724 189 310 996 860},
{426 374 684 847 081 354 734 887 179 968 699, 5 716 358 640 859 164 071 939 976 995 460},
{590 405 517 556 343 615 813 384 767 391 051, -23 478 088 442 079 785 690 277 411 379 860},
{866 779 932 591 592 362 668 820 206 532 301, 12 153 923 474 718 573 268 985 493 337 350},
{966 692 837 529 988 803 283 395 074 693 201, 46 569 400 626 906 645 252 218 754 923 070},
{2 827 408 484 397 737 500 312 893 451 508 519, 138 884 859 449 716 405 551 810 140 141 880},
{12 477 535 146 255 756 708 449 352 816 400 669, 559 305 893 526 339 192 587 797 592 677 770},
{43 374 177 657 749 912 350 969 250 149 921 979, 413 333 447 312 615 410 114 515 995 439 780},
{6 484 411 828 751 133 474 787 272 184 985 171, 107 231 224 850 490 502 072 557 589 397 640},
{12 685 122 768 147 540 958 888 022 102 819 521, -375 664 932 246 693 214 049 128 469 648 700},
{21 958 716 988 247 108 014 368 812 174 306 029, -191 824 505 310 587 558 602 288 573 357 620},
{22 771 569 092 871 709 760 686 617 695 874 599, 842 675 900 710 742 993 099 566 317 405 840},
{4 849 263 194 093 885 696 580 108 605 146 669, -39 870 735 659 478 363 690 883 121 397 210},
{3 756 605 646 981 143 100 615 683 533 550 701, 129 627 451 295 784 639 374 407 964 152 050},
{650 200 589 749 471 751 779 004 141 545 999, 25 348 024 163 871 930 816 756 612 310 380},
{2 220 857 666 310 810 813 623 612 409 494 131, 8 233 662 931 028 973 794 890 847 288 940},
{560 062 591 820 039 860 226 005 988 436 919, 8 482 916 632 990 804 614 610 753 768 230},
{47 713 604 704 335 671 085 756 173 168 489, 2 059 737 663 496 103 886 376 575 286 320},
{85 249 249 425 245 706 472 830 337 365 379, -2 652 665 668 158 924 134 740 225 321 050},
{91 350 959 084 193 674 446 924 900 036 529, 205 838 105 155 557 072 126 022 372 020},
{10 331 060 823 290 059 834 287 318 228 101, 195 737 746 773 801 952 950 141 465 240},
{10 802 978 686 082 361 689 615 036 834 369, -64 852 917 778 504 030 480 958 009 580},
{6 892 104 314 880 661 576 942 642 138 241, -197 067 394 282 328 772 249 998 890 020},
{1 318 875 735 212 208 403 637 072 127 209, -33 332 743 099 634 190 195 375 968 760},
{3 622 931 182 062 960 248 669 622 420 941, 139 144 917 307 435 357 598 392 939 890},
{1 295 996 349 479 878 728 962 901 934 051, 72 882 774 089 854 755 206 237 255 640},
{3 989 289 618 514 223 052 091 535 534 719, -174 890 379 795 717 742 485 270 250 980},
{8 330 468 313 608 541 292 489 739 693 071, 87 851 169 508 920 271 824 919 072 260},
{3 863 590 224 460 017 250 270 615 078 879, 114 973 677 254 736 235 649 240 008 500},
{11 424 215 352 454 705 212 689 847 740 371, -184 067 604 299 495 211 725 759 757 270},
{3 017 995 357 386 523 508 878 440 197 381, -29 246 876 925 289 083 033 386 891 730},
{1 397 325 554 518 737 066 337 177 646 941, 7 518 879 659 742 658 879 151 107 890},
{297 701 610 542 768 781 417 033 570 349, -1 399 907 093 405 934 630 739 327 980},
{120 128 688 526 519 027 541 265 637 141, 6 784 426 504 277 242 396 402 961 460},
{499 738 126 168 305 234 090 904 953 889, 29 268 986 336 474 125 272 128 824 470},
{543 504 970 509 521 220 643 449 412 649, 5 950 430 904 101 307 920 695 464 360},

```



```

{505 955 317 311 852 164 900 701 128 139, -18 260 520 297 221 607 027 055 362 390},
{1 340 152 003 598 560 796 069 103 714 031, -61 757 784 404 340 351 667 750 379 580},
{4 648 332 577 528 662 095 972 563 818 979, -54 968 883 929 201 853 374 549 577 780},
{6 029 661 669 827 355 656 901 723 372 571, 104 332 687 737 263 904 446 277 399 810},
{5 430 188 952 421 651 046 573 819 918 659, -226 441 901 312 278 837 176 647 661 510},
{1 108 586 447 333 302 462 096 713 352 831, -5 742 440 656 269 586 528 771 028 460},
{74 145 568 991 337 773 020 119 872 801, 3 156 687 577 695 175 973 237 505 930},
{386 980 430 791 530 134 549 966 339 161, 6 033 682 783 639 095 097 423 418 820},
{207 007 892 295 640 127 031 751 204 931, 5 193 650 004 084 453 245 689 657 590},
{185 265 074 802 238 701 754 609 765 919, 2 844 774 871 067 183 960 020 589 040},
{89 031 753 900 807 832 671 141 058 069, 1 075 045 065 657 023 889 496 427 850},
{49 443 623 730 012 689 422 675 823 731, 2 005 125 760 794 220 482 582 413 430},
{171 814 592 750 548 483 113 012 516 769, 10 103 651 422 767 640 285 198 243 320},
{13 182 159 438 148 164 425 237 462 579, -630 109 867 618 470 642 210 817 380},
{12 587 093 241 769 484 358 615 302 651, 192 063 977 121 088 447 352 599 230},
{22 371 441 303 810 644 830 717 878 779, -78 264 217 322 490 291 129 281 070},
{3 043 337 455 816 186 496 383 317 491, 2 060 864 988 002 817 907 818 150},
{140 592 997 457 863 919 486 604 809, 3 645 149 508 557 426 741 399 220},
{393 526 177 344 806 580 419 157 521, -21 267 502 398 751 758 151 284 750},
{2 649 648 426 100 682 938 268 434 979, -45 604 695 966 489 176 206 419 540},
{1 148 591 071 121 990 292 321 516 409, -52 389 177 255 094 670 518 173 630},
{996 677 951 013 207 228 654 166 201, 45 949 473 723 647 341 660 192 830},
{3 566 828 197 665 606 255 389 090 809, -22 836 469 937 709 581 946 792 540},
{1 089 060 733 110 779 394 053 096 819, -4 622 608 921 962 438 564 896 460},
{470 618 090 561 382 922 879 402 991, -20 957 818 171 775 495 565 665 370},
{2 396 068 786 362 827 129 125 977 601, -105 523 338 661 758 352 208 988 330},
{7 772 968 717 261 357 891 869 251 239, -455 804 482 023 678 957 799 899 600},
{6 097 423 237 562 717 927 010 467 789, 10 857 677 078 101 258 437 564 090},
{1 152 411 362 877 518 040 038 248 541, 29 491 251 510 173 072 501 888 010},
{565 391 049 172 821 328 618 653 901, -31 124 007 481 659 935 259 407 790},
{1 294 887 540 238 565 981 277 733 931, -73 754 123 482 902 826 140 833 790},
{8 204 357 295 874 907 203 575 846 539, -119 124 004 391 777 515 297 063 440},
{3 814 950 796 593 079 332 304 236 071, -193 909 069 991 720 465 068 102 140},
{15 870 881 413 573 822 233 509 488 979, -648 693 960 315 539 132 995 611 480},
{75 858 817 866 221 643 445 318 178 209, 380 053 601 276 520 090 100 786 380},
{38 127 499 659 676 018 284 613 545 541, 305 051 201 489 439 533 334 226 950},
{979 032 152 484 768 923 370 625 459, -39 521 566 872 564 793 059 603 870},
{2 260 761 851 667 076 682 987 294 041, -77 878 170 565 739 404 652 561 640},
{576 021 220 419 120 963 814 626 731, 5 172 008 600 646 929 022 246 480},
{483 994 702 575 272 428 662 130 201, 25 518 765 536 563 236 707 348 820},
{216 322 497 476 696 263 151 842 129, 6 898 938 874 899 291 035 945 940},
{616 303 481 059 378 500 417 015 239, -36 248 837 869 411 496 990 521 140},
{18 382 557 125 145 946 117 120 609, -191 087 465 788 190 318 442 570},
{9 578 262 779 398 562 205 106 139, 119 162 031 555 418 829 615 070},
{11 370 363 996 229 014 811 035 289, 11 501 643 473 274 539 026 830},
{1 195 111 108 715 575 911 394 831, -30 073 208 089 337 395 985 730},
{1 962 120 929 337 901 936 626 619, 43 848 966 820 555 479 423 990},
{2 781 726 974 360 754 000 685 681, -34 338 860 735 734 257 019 800},
{70 092 946 336 074 702 552 131, 1 540 590 369 052 355 696 670},
{192 361 311 908 392 746 697 231, -4 165 479 014 393 783 146 140},
{188 068 588 815 959 215 672 541, 10 945 684 640 158 414 774 170},

```

```

{499 979 433 249 807 292 424 401, -1 524 063 227 544 917 761 710},
{21 760 348 383 640 912 463 771, -216 617 636 258 724 861 600},
{24 744 774 199 875 002 246 521, -1 135 257 505 989 736 225 260},
{57 953 623 906 697 872 008 949, 953 787 767 414 300 225 490},
{57 084 906 299 184 878 231 191, -599 328 767 825 523 359 940},
{37 317 012 295 799 918 259 641, 1 215 302 151 155 854 283 880},
{89 695 951 897 922 699 700 389, -4 863 152 313 605 211 117 120},
{541 961 773 510 253 797 649 479, 10 098 613 511 564 777 173 410},
{844 202 384 675 286 598 379 911, -12 234 905 719 631 784 530 160},
{1 533 604 805 940 084 483 379, -36 463 422 642 254 387 820},
{537 404 796 315 448 929 689, -31 424 930 601 020 902 680},
{798 425 000 621 489 616 379, 32 972 903 396 777 908 530},
{1 775 905 093 803 772 726 409, -1 924 593 027 924 600 000},
{124 062 013 628 901 471 341, -6 255 410 917 668 255 090},
{262 597 385 840 371 245 209, 801 053 639 286 339 090},
{37 200 169 232 542 054 061, -983 871 971 103 091 740},
{46 928 383 013 233 446 809, 157 181 171 305 708 860},
{17 265 589 000 549 085 081, -243 765 908 836 595 190},
{10 489 422 239 142 525 659, -246 831 350 299 518 540},
{30 748 887 167 249 491 729, 523 149 621 821 805 750},
{29 352 070 579 498 927 771, -1 506 577 614 150 494 940},
{182 501 073 570 520 501 661, -7 332 066 725 617 035 330},
{200 949 237 046 250 778 839, -9 024 708 351 555 602 760},
{603 818 981 318 907 047 869, -27 944 216 054 864 442 090},
{2 749 396 743 915 780 205 861, 113 121 940 261 247 754 660},
{8 652 014 589 104 357 599 271, 472 763 112 447 570 262 650},
{35 711 919 827 071 310 764 321, -850 453 416 057 876 194 490},
{1 788 035 487 231 840 469 009, -31 903 933 370 520 825 240},
{355 219 839 151 238 147 819, 16 401 520 762 301 940 990},
{1 409 018 022 470 543 044 211, -74 977 025 366 508 336 570},
{3 901 910 332 771 953 005 369, 164 681 975 255 171 736 270},
{12 664 725 411 394 334 942 861, -464 946 373 791 487 063 860},
{27 904 503 075 070 238 878 891, 30 445 153 730 176 544 190},
{3 439 426 770 914 687 978 089, 168 916 849 667 409 111 540},
{15 333 534 169 192 942 569 539, 246 182 745 630 721 367 130},
{17 621 188 962 142 669 677 229, 714 441 276 561 570 642 900},
{60 200 580 926 045 695 213 021, 557 453 505 493 065 085 350},
{1 103 814 468 538 835 199 529, 56 917 267 022 035 692 720},
{5 618 985 175 159 416 500 099, 182 805 096 832 025 027 850},
{12 041 179 484 973 200 176 001, 169 834 263 186 706 730 610},
{4 280 353 522 027 402 024 559, -165 928 865 248 923 083 700},
{8 483 040 585 594 136 061 891, 77 866 610 623 967 490 270},
{1 109 413 076 998 414 762 289, -52 440 901 822 975 110 780},
{2 046 688 817 700 296 413 159, 47 038 362 251 893 366 800},
{5 772 779 467 135 943 236 291, -77 077 019 889 254 785 890},
{2 007 253 164 099 592 070 209, -86 437 684 139 713 006 980},
{4 815 793 650 434 420 326 919, 176 670 211 191 952 270 680},
{11 470 185 011 178 963 658 309, 474 192 687 539 362 124 040},
{22 479 688 068 802 443 018 599, 802 491 063 139 953 753 360},
{2 494 513 521 818 219 054 269, -123 485 074 076 717 151 960},
{6 227 822 111 252 879 782 319, 268 417 164 427 773 844 980},

```

```

{13 611 059 682 934 418 292 529, 673 093 092 051 177 321 810},
{37 448 658 319 628 835 938 579, -1 139 173 673 548 408 440 750},
{36 162 299 774 629 294 148 921, 668 235 272 738 158 409 670},
{19 476 356 738 953 746 711 991, 121 752 436 799 303 066 610},
{1 012 320 382 620 730 347 859, 51 738 778 081 477 453 200},
{5 636 249 931 213 497 751 391, -186 981 263 424 172 552 830},
{6 729 819 150 568 612 789 241, -279 367 549 788 481 065 990},
{6 274 486 866 911 868 575 731, 372 979 922 180 771 892 930},
{16 609 124 350 474 654 623 829, -315 708 140 006 163 374 040},
{30 975 174 532 853 054 273 041, 1 496 289 134 784 360 700 710},
{112 171 221 702 248 630 909 119, -174 842 831 317 364 708 250},
{19 546 876 878 377 458 632 631, -503 771 334 063 177 036 420},
{25 151 492 671 697 892 724 999, 188 115 740 935 743 577 680},
{14 060 170 036 628 417 714 371, -163 095 473 804 423 336 040},
{8 523 781 651 450 714 547 681, -185 816 587 297 279 428 840},
{5 969 122 420 258 933 918 709, 266 303 174 545 737 668 790},
{27 723 597 643 429 006 537 579, 570 548 659 357 031 668 890},
{58 554 952 931 451 854 745 781, -3 235 714 459 287 806 072 790},
{78 335 258 732 107 704 325 811, 2 397 524 466 972 262 543 920},
{196 545 218 172 216 865 510 799, 8 999 327 611 990 607 844 300},
{361 437 312 185 703 273 014 051, -12 447 935 750 291 549 389 740},
{112 241 032 239 333 518 609 341, 1 324 363 142 722 677 196 350},
{82 788 557 915 604 813 182 659, 4 016 441 112 531 965 733 330},
{390 733 067 339 183 271 535 021, 19 298 876 148 344 964 333 030},
{1 193 641 637 443 280 203 479 671, -6 637 346 495 078 524 318 890},
{271 263 649 384 397 654 052 779, 12 454 513 857 823 505 632 020},
{686 649 527 417 586 932 766 911, -7 435 722 313 504 282 743 480},
{643 331 718 373 423 012 054 501, -20 952 606 550 672 304 552 760},
{1 555 970 259 052 025 699 345 809, 51 873 098 387 268 014 653 200},
{55 895 834 069 699 802 797 941, 686 639 677 590 750 714 570},
{69 783 066 397 097 724 360 521, -2 806 157 379 588 368 838 660},
{93 087 891 245 485 648 100 729, 3 404 807 240 951 993 203 350},
{290 682 030 685 239 734 180 029, -13 965 187 357 423 413 668 400},
{649 312 858 983 640 166 949 121, 12 941 868 833 140 474 667 550},
{557 073 748 980 724 826 476 871, -14 134 393 007 898 208 727 820},
{1 463 937 839 846 366 209 064 641, -48 279 641 365 638 735 548 220},
{3 902 698 318 178 239 797 128 291, 9 717 141 443 908 619 468 760},
{901 728 110 529 332 557 620 479, 39 851 665 966 344 739 469 250},
{3 729 911 880 845 708 993 240 021, -195 031 737 798 872 493 082 890},
{6 101 524 529 450 037 790 942 861, -92 152 226 582 430 186 932 280},
{4 888 871 327 421 008 806 507 631, 242 881 139 384 567 174 854 920},
{7 843 383 472 145 992 661 716 981, 28 513 512 679 007 540 584 470},
{544 038 840 148 669 247 920 481, 4 189 799 998 189 427 189 670},
{159 425 063 605 027 970 891 369, -3 626 433 217 673 109 185 820},
{34 637 491 119 797 154 462 461, -551 881 450 349 273 451 780},
{32 891 103 303 975 322 919 429, 929 979 220 240 986 733 830},
{85 799 479 480 737 596 080 129, -2 438 326 642 655 522 220 180},
{114 969 793 936 373 911 831 079, 6 343 446 215 793 727 403 970},
{197 728 275 073 791 458 464 369, 8 803 275 469 720 273 562 280},
{1 018 109 899 726 305 463 646 459, 19 266 183 329 251 013 259 420},
{752 451 997 723 558 014 803 051, 20 651 077 235 143 018 423 200},

```

```

{2 262 317 531 860 747 243 530 601, 45 886 548 727 567 230 548 130},
{3 483 037 696 698 189 614 729 981, -138 857 405 741 100 337 093 410},
{2 912 240 845 840 978 036 077 481, -45 549 328 972 622 426 252 910},
{731 968 310 121 168 271 298 509, -27 817 466 820 740 357 942 460},
{2 187 257 368 261 660 163 431 799, 76 295 781 348 531 640 027 230},
{6 355 393 002 285 106 736 825 621, -160 022 984 163 393 628 431 480},
{11 427 117 426 910 238 508 828 329, 557 832 126 956 392 359 087 750},
{67 889 196 833 380 223 095 405 579, 2 073 671 097 034 905 323 627 460},
{136 029 291 561 684 798 659 450 851, -220 051 334 974 755 301 915 500},
{9 429 203 368 791 540 993 634 601, -10 060 568 211 129 543 169 530},
{615 189 695 752 919 990 032 741, -25 228 558 571 290 674 861 210},
{2 435 776 800 527 892 134 288 951, 72 463 226 288 944 229 878 950},
{7 021 196 217 349 132 080 432 599, 273 839 776 974 708 153 313 890},
{24 758 133 982 313 256 337 863 791, -673 575 065 288 611 529 093 100},
{41 200 001 774 707 929 883 808 159, 1 641 039 354 763 850 449 840 920},
{43 678 494 308 528 828 084 074 909, -521 558 253 928 208 640 755 910},
{33 232 154 381 615 132 594 804 281, -163 909 490 310 393 197 582 280},
{10 409 510 000 066 315 114 038 309, 83 852 187 169 043 338 578 870},
{2 971 536 567 340 223 694 865 679, 92 238 723 684 077 425 877 040},
{4 994 249 771 886 262 766 900 149, -128 049 411 499 464 261 329 790},
{81 003 575 196 300 334 623 089, 2 849 066 429 344 224 787 110},
{308 658 508 840 172 186 586 259, 14 178 024 208 037 288 679 480},
{817 763 957 898 689 254 937 551, -40 018 440 637 341 947 264 400},
{4 366 181 433 114 427 722 037 301, -129 395 863 418 152 263 120 330},
{8 352 758 698 790 055 237 533 669, -466 782 153 765 513 770 176 980},
{12 379 337 316 287 349 038 644 721, 273 757 090 757 433 519 250 710},
{15 127 326 282 913 008 763 055 521, 7 245 068 877 446 838 369 270},
{94 760 832 193 427 747 039 989, 4 973 048 391 345 633 867 600},
{68 501 102 223 036 592 452 839, 3 752 970 382 945 887 281 760},
{237 856 467 832 665 966 670 909, 3 836 589 408 902 540 374 350},
{3 030 955 342 175 671 236 541, -82 033 327 414 030 767 510},
{1 073 720 808 010 257 493 579, 57 058 892 279 348 265 810},
{2 609 934 469 637 248 759 561, 27 658 548 239 773 680 870},
{2 517 764 709 729 212 203 031, 20 950 390 202 491 029 480},
{933 189 243 002 455 023 181, 16 329 484 118 230 141 770},
{604 570 714 097 572 515 041, -20 088 016 630 405 733 340},
{484 484 011 535 529 225 091, -4 230 540 336 495 333 330},
{509 059 917 519 961 072 609, 27 520 772 128 933 657 740},
{3 435 190 818 987 963 555 539, -72 155 987 206 820 884 650},
{7 102 438 301 799 165 822 911, 284 315 617 065 530 220 720},
{1 368 483 334 611 513 467 339, -49 426 988 154 873 636 600},
{3 883 555 764 962 037 722 711, -126 416 290 334 886 756 810},
{8 872 658 090 282 386 338 149, -83 823 003 449 988 599 790},
{3 157 649 129 517 715 137 341, -95 288 833 613 663 965 590},
{3 292 522 686 967 872 490 621, 87 747 851 222 163 990 840},
{10 515 810 528 064 149 486 049, 598 945 459 390 785 400 620},
{66 567 142 983 466 919 002 861, 833 102 045 805 867 757 650},
{20 336 190 931 627 903 893 889, -75 256 510 818 655 591 530},
{4 250 185 658 314 439 378 039, -93 742 459 590 012 798 240},
{7 975 519 167 729 727 766 989, 301 875 215 804 380 571 010},
{31 817 652 760 774 063 102 979, -287 454 922 600 229 113 890},

```

```

{22 550 755 610 693 503 241 561, -622 169 186 951 008 850 520},
{38 318 884 994 753 340 333 091, -446 287 858 374 906 182 700},
{15 529 577 197 636 436 156 359, 650 766 572 636 969 461 500},
{22 293 956 958 358 560 829 891, -800 811 190 858 751 893 470},
{32 317 852 807 309 539 004 519, 143 647 234 618 913 121 330},
{696 520 468 424 236 977 481, -8 440 411 933 494 898 140},
{1 012 464 236 015 731 602 889, -59 666 514 846 147 361 920},
{468 495 608 562 160 987 501, 25 499 112 506 854 336 410},
{2 387 407 443 134 515 962 371, 122 632 169 623 703 239 050},
{14 406 451 291 322 759 525 671, -213 284 377 893 874 025 790},
{24 318 487 770 629 231 240 299, 1 215 719 902 598 297 326 830},
{1 026 519 384 484 460 628 449, 11 786 084 500 886 051 940},
{283 638 259 750 901 526 919, 8 921 321 475 972 800 850},
{462 850 897 537 253 170 531, -26 418 714 195 452 676 150},
{3 184 175 453 204 645 042 419, 161 258 692 802 171 627 460},
{10 290 599 112 535 664 202 031, 112 486 917 054 553 220 730},
{13 626 704 803 401 600 015 851, 546 489 289 319 089 446 720},
{8 917 384 823 484 674 189 399, 322 340 838 620 457 689 910},
{27 147 823 129 923 423 148 331, 211 442 922 370 965 893 340},
{20 865 395 676 386 989 003 561, 700 861 658 045 494 717 410},
{40 273 970 309 440 982 203 489, 2 187 735 955 997 121 730 380},
{224 575 498 474 690 555 218 899, 12 287 864 059 602 920 335 980},
{851 880 295 861 335 281 986 009, 29 703 017 306 142 750 197 880},
{2 386 308 710 217 922 911 880 261, -39 836 650 734 340 772 709 300},
{976 473 794 473 386 120 112 489, -38 061 979 390 968 798 532 320},
{3 297 555 092 642 463 073 685 581, 94 434 649 035 266 387 574 000},
{1 922 063 521 556 983 342 509 169, -41 040 009 002 944 841 419 290},
{1 711 042 296 937 475 253 562 711, 75 689 887 602 848 900 050 290},
{7 486 104 599 940 411 346 083 709, -208 337 493 643 921 928 428 620},
{3 525 337 981 435 297 413 999 361, 44 673 888 929 956 306 190 700},
{978 710 251 843 944 541 550 689, 16 676 688 583 199 336 038 620},
{1 308 808 015 768 887 466 700 641, 37 794 563 118 157 283 898 090},
{3 514 425 035 020 984 902 859 759, 174 733 080 308 575 857 010 620},
{4 960 620 641 216 408 424 487 109, -16 808 888 365 892 967 471 360},
{501 641 892 773 738 129 413 159, -22 027 096 074 791 919 902 460},
{1 250 310 553 565 483 114 198 671, -460 695 815 619 565 679 850},
{4 490 396 530 553 369 471 479, 243 981 903 502 088 865 300},
{24 779 289 146 458 243 915 829, -955 570 755 910 729 339 470},
{16 453 177 312 400 446 508 141, -66 596 694 238 147 824 090},
{952 252 730 061 423 435 661, 15 044 644 913 650 540 920},
{1 114 465 225 861 278 782 951, 46 521 452 117 225 302 080},
{514 455 862 984 245 209 219, 5 977 745 708 710 901 220},
{92 802 740 812 033 779 049, 2 999 430 700 233 795 270},
{45 082 334 698 682 454 571, 1 508 654 139 589 535 430},
{44 499 661 739 905 690 579, -1 045 577 459 287 652 160},
{115 502 421 375 301 427 551, 143 606 887 089 880 590},
{10 663 522 914 395 730 941, 358 638 428 116 147 650},
{24 003 112 201 263 338 309, -1 082 411 404 663 400 280},
{47 705 385 965 801 569 399, 2 003 007 512 172 824 280},
{92 065 375 912 899 543 571, 3 421 284 802 395 488 700},
{77 637 751 696 441 483 579, 4 242 882 061 169 544 210},

```

```

{317 734 523 442 811 637 549, 1 628 737 226 217 845 550},
{32 821 846 913 270 580 049, 828 333 145 602 700 170},
{78 181 206 620 194 114 501, -2 335 538 393 576 087 010},
{278 218 347 677 994 035 921, 12 337 264 591 353 472 830},
{1 390 223 218 707 095 631 419, 60 427 203 757 706 646 000},
{99 780 602 240 536 128 169, -2 603 655 615 865 523 040},
{211 263 898 249 209 414 899, 2 999 733 781 830 783 180},
{321 915 913 784 702 667 049, -16 586 933 393 228 801 220},
{1 697 809 007 652 216 411 119, 98 112 685 713 500 531 250},
{7 503 230 981 199 552 347 119, 412 670 190 695 655 649 860},
{18 867 054 718 115 413 059 389, -150 999 310 686 328 386 960},
{1 972 638 536 584 462 963 361, -58 711 391 050 125 124 170},
{5 910 738 539 067 605 863 169, -99 159 091 887 086 637 300},
{9 740 550 513 555 686 082 581, 440 538 344 375 549 818 770},
{12 225 441 260 691 107 479 891, -476 692 591 122 354 270 210},
{42 310 093 231 015 989 937 819, -1 717 757 741 163 630 986 970},
{159 096 424 816 770 968 844 181, -6 199 512 639 530 090 407 920},
{524 816 856 563 856 822 196 489, -12 100 185 736 483 628 916 330},
{1 131 726 343 660 255 477 369 049, -61 292 489 117 276 853 761 490},
{7 143 846 426 867 299 525 219 479, -15 183 411 829 551 076 530 330},
{1 892 676 757 665 637 662 053 701, -34 641 504 924 015 279 522 180},
{3 164 109 301 955 880 628 215 949, -3 131 341 162 035 889 610 130},
{365 136 803 207 662 618 146 899, -413 349 869 662 420 432 170},
{37 365 942 232 089 511 738 039, -1 031 693 220 957 715 330 260},
{56 471 555 680 551 722 018 429, -2 470 641 982 980 320 401 200},
{88 655 691 926 907 449 501 921, -5 050 434 824 235 139 531 470},
{565 285 862 240 590 578 199 289, -16 057 757 432 265 354 388 260},
{819 352 379 937 096 827 157 439, -15 344 018 595 699 180 920 790},
{1 535 967 985 625 099 827 247 819, 3 869 782 454 855 752 890 180},
{84 247 887 111 151 608 563 891, -4 646 412 582 671 932 949 100},
{153 727 616 387 260 685 502 841, -8 698 980 673 273 912 852 110},
{716 362 968 649 106 204 619 889, -42 703 721 710 649 625 528 810},
{2 409 675 408 416 294 771 840 131, 62 300 669 922 509 407 163 400},
{5 032 730 358 954 598 990 649 719, 2 092 327 476 382 677 312 420},
{171 377 341 819 273 624 184 369, -7 392 841 750 790 332 685 400},
{336 837 369 325 089 077 462 419, -3 668 738 935 931 564 202 180},
{172 339 807 934 322 113 673 391, -6 073 780 911 196 721 743 170},
{570 759 547 624 290 121 022 381, -23 717 010 973 199 946 879 210},
{389 372 351 140 340 376 256 591, 3 961 832 893 773 671 267 730},
{279 294 615 180 668 596 781 801, -7 034 739 131 341 328 945 670},
{525 832 468 319 124 822 294 749, 5 961 460 659 642 287 564 010},
{307 206 497 921 482 682 129 119, -9 107 607 272 111 315 532 360},
{615 489 481 905 813 538 751 371, 5 510 548 119 037 445 479 830},
{424 668 764 021 469 102 386 839, -12 702 562 510 311 273 870 240},
{1 376 534 496 480 463 231 898 669, -62 348 516 805 802 880 146 410},
{1 221 648 814 952 767 038 089 899, -26 000 841 768 944 461 495 620},
{98 077 795 093 285 703 264 491, -3 190 931 169 458 497 466 490},
{211 108 861 141 857 267 371 449, -6 504 589 996 526 604 742 050},
{743 457 294 504 484 822 088 099, -33 182 212 504 983 352 296 090},
{3 375 603 468 107 618 965 103 869, 143 894 880 005 353 665 376 380},
{16 571 328 224 105 650 023 229 379, 466 151 769 722 052 828 021 720},

```

```

{52 744 006 957 951 198 173 687 791, 2 773 132 756 068 257 931 496 650},
{13 675 632 756 228 666 288 111 691, -256 772 348 788 992 907 756 830},
{16 741 265 873 422 586 426 924 951, -419 519 950 476 729 927 251 370},
{9 922 568 557 299 276 445 592 099, -251 321 306 791 258 816 602 960},
{30 380 435 702 485 832 117 241 409, -1 352 475 860 112 837 948 246 870},
{157 117 661 780 852 711 208 377 519, -1 449 379 686 487 806 872 419 110},
{146 748 565 682 561 815 765 523 389, 4 538 751 998 388 936 904 395 960},
{378 633 935 263 074 541 038 019 919, 7 850 451 008 747 044 363 884 210},
{454 883 997 647 319 304 466 037 589, 13 193 412 521 783 638 030 870 590},
{1 583 300 948 575 578 465 525 819 779, 94 480 870 563 131 323 365 378 300},
{5 741 336 600 411 161 953 088 441 571, 302 845 036 190 771 105 181 933 750},
{3 192 490 890 585 750 387 443 219 429, -81 153 419 353 946 551 916 287 620},
{6 904 391 481 240 550 539 708 564 499, 261 143 578 535 562 500 013 494 130},
{28 779 268 268 297 310 378 786 996 869, 191 727 802 348 630 069 488 268 800},
{5 044 576 916 702 788 842 215 894 119, -111 320 017 213 745 870 469 016 800},
{8 829 211 663 140 392 448 644 667 869, -503 933 494 954 970 021 815 483 980},
{60 639 402 758 316 053 952 544 986 521, 3 275 771 748 672 824 018 324 155 770},
{401 665 377 083 368 201 299 107 250 359, -6 085 871 018 401 606 836 236 812 680},
{529 642 915 600 323 023 119 016 771, 29 694 929 266 118 939 837 430 780},
{1 221 318 608 644 291 382 639 054 519, -8 736 125 374 476 148 447 104 210},
{436 474 889 374 719 388 839 255 131, 1 698 303 208 069 316 249 206 650},
{2 752 190 127 183 311 079 666 331, -41 241 965 387 018 968 760 130},
{2 766 409 990 486 916 642 857 129, 101 688 327 469 121 804 780 160},
{5 227 112 353 977 606 361 995 059, -91 162 854 622 760 965 334 910},
{7 738 239 760 538 065 814 202 439, 240 353 849 860 501 129 829 340},
{11 776 057 815 509 444 575 553 309, -193 552 537 632 477 378 826 770},
{7 692 391 997 990 558 752 794 911, -147 011 368 212 275 193 141 720},
{11 998 013 589 014 426 065 793 221, 384 810 321 472 919 873 295 660},
{17 292 299 461 831 408 400 568 011, -552 618 239 310 202 817 932 350},
{40 444 644 846 995 382 210 955 411, 1 479 439 530 294 401 557 670 220},
{125 444 159 790 681 578 618 727 221, -3 493 824 681 010 324 419 378 030},
{83 715 710 148 215 220 199 346 609, -3 565 840 888 273 834 984 222 230},
{427 043 799 197 170 906 121 065 069, 23 713 584 718 455 822 567 292 530},
{50 017 840 506 491 077 359 681 779, -2 205 272 854 653 840 419 501 490},
{176 562 222 787 360 324 501 975 241, 4 844 069 091 257 159 989 931 010},
{546 109 611 027 743 780 979 179 131, -24 307 894 292 914 815 268 878 660},
{2 845 320 082 488 079 111 026 001 361, 20 124 287 632 017 701 989 706 280},
{1 956 677 119 769 365 749 831 386 131, -93 851 210 928 422 915 678 205 180},
{3 563 775 741 606 385 332 141 584 899, 129 442 892 633 610 807 207 129 330},
{15 216 938 285 814 034 684 167 121 591, 247 470 101 711 013 006 350 162 310},
{30 436 782 442 002 565 498 612 390 931, 271 333 993 921 203 222 208 192 500},
{11 891 155 829 778 957 435 002 563 681, -115 344 397 816 631 490 300 223 140},
{2 681 396 521 144 397 453 974 645 511, -107 736 254 006 882 050 489 303 440},
{3 014 467 085 941 105 872 743 062 739, 19 684 443 506 326 092 449 063 190},
{689 554 597 776 645 737 135 061 919, -4 217 731 696 861 260 795 543 510},
{518 147 128 253 317 092 828 917 039, -5 841 749 899 460 454 331 828 620},
{443 921 812 464 499 018 661 365 391, -19 355 526 112 633 833 928 334 820},
{315 077 319 645 869 584 274 202 719, 272 006 344 736 574 413 774 790},
{23 587 082 670 019 693 871 970 649, 613 435 069 062 729 300 425 010},
{69 414 061 454 631 094 410 887 519, -3 661 323 677 763 805 410 875 820},
{37 923 194 143 183 307 334 018 311, -1 136 252 227 843 972 006 310 670},

```

```

{107 144 526 707 390 012 567 316 451, - 3 464 697 129 564 430 578 285 510},
{65 532 161 585 941 175 243 124 109, 228 230 193 245 327 900 247 540},
{7 554 127 257 549 035 892 112 379, 404 103 138 969 024 730 688 730},
{31 081 928 098 470 931 734 346 241, - 1 125 657 762 653 674 714 343 520},
{109 558 803 213 822 027 085 352 069, - 5 542 810 423 021 423 099 507 020},
{325 648 716 898 215 161 101 871 081, - 9 952 250 156 572 499 195 135 460},
{696 660 105 438 005 396 737 373 849, 30 347 490 116 194 139 811 360},
{783 704 993 833 530 176 215 939, 29 956 533 047 285 553 987 090},
{1 213 618 785 630 548 910 451 349, - 23 720 187 536 331 129 734 850},
{976 194 540 692 984 787 473 749, - 3 258 516 797 333 783 228 880},
{341 485 125 294 695 478 753 001, 1 588 611 840 670 876 298 280},
{16 671 532 835 274 269 676 949, - 218 874 750 837 687 674 280},
{9 299 994 674 111 614 348 919, - 471 458 193 550 151 690 850},
{32 421 468 419 746 286 488 331, - 1 791 346 527 932 030 911 980},
{44 484 960 159 402 248 245 441, 2 310 859 761 871 926 455 070},
{145 234 795 642 747 045 376 861, 7 187 363 232 564 397 102 680},
{373 370 278 856 234 934 138 511, 18 990 981 622 739 684 859 480},
{1 618 787 753 238 249 525 823 339, 70 278 811 611 411 388 587 270},
{596 146 630 122 684 667 348 379, - 30 659 433 395 398 536 594 990},
{3 417 966 298 138 230 482 935 819, 66 397 715 519 076 379 491 840},
{7 952 384 472 999 117 341 846 729, - 442 889 003 992 798 327 616 820},
{4 924 017 316 684 391 369 263 781, - 66 645 597 809 608 069 873 950},
{1 946 987 227 878 056 153 538 269, - 26 904 799 256 905 504 039 590},
{2 470 262 026 595 825 534 635 039, 37 655 539 310 023 740 637 320},
{3 765 895 534 301 078 204 448 331, 707 388 601 089 979 723 710},
{60 585 853 395 434 990 510 959, 3 478 887 606 798 527 130 540},
{362 635 784 044 867 352 236 529, 6 342 341 390 412 734 698 140},
{281 703 522 626 710 085 079 799, 9 449 733 202 117 445 239 050},
{448 906 832 640 131 295 016 951, - 11 098 097 137 959 593 956 230},
{1 250 719 727 558 631 728 705 501, 54 657 477 768 237 874 604 340},
{1 606 967 538 820 686 185 774 069, - 82 210 753 739 811 801 789 870},
{9 349 131 529 863 012 355 856 081, 521 229 761 895 843 236 658 630},
{8 284 050 249 803 641 903 814 009, - 132 100 557 679 672 564 250 490},
{9 609 505 887 948 140 635 682 111, - 150 609 116 086 976 624 296 080},
{7 398 862 946 209 193 136 019 259, - 223 140 549 857 549 156 125 530},
{8 841 425 028 427 816 953 069 019, - 844 567 231 973 823 445 320},
{87 680 099 641 314 692 501 311, 2 392 511 541 012 093 138 720},
{211 549 671 409 321 161 463 579, 6 315 314 021 547 236 738 160},
{789 221 483 263 849 625 179 049, - 18 453 616 705 441 621 914 330},
{1 075 292 802 605 169 401 422 391, 5 099 917 314 520 592 384 550},
{198 227 440 427 573 521 132 409, - 683 016 890 210 105 914 470},
{38 288 108 927 344 289 963 359, - 2 115 323 469 221 995 450 980},
{53 283 906 818 441 333 275 469, - 2 352 852 217 274 962 355 670},
{208 755 238 899 583 027 140 191, - 8 253 902 259 601 100 284 350},
{604 328 284 798 435 527 891 691, 22 954 229 153 426 255 981 820},
{1 887 100 029 147 570 963 457 121, - 102 783 393 785 250 192 772 560},
{9 286 734 194 279 940 881 311 291, - 269 362 541 081 227 835 694 270},
{32 230 357 177 066 811 394 233 861, 1 730 212 848 436 825 802 038 170},
{161 565 422 751 452 589 967 333 619, - 9 450 042 423 943 238 947 277 130},
{229 590 087 648 799 493 769 224 659, - 12 030 663 812 531 087 620 744 410},
{252 876 277 887 916 072 745 298 119, 2 729 015 181 183 932 435 760 090},

```



```

{231 455 624 509 600 588 877 953 001, 6 617 661 165 065 793 916 905 660},
{40 791 583 193 251 751 650 019 849, 1 508 466 161 973 453 469 042 110},
{15 812 201 812 095 504 456 602 629, 644 086 844 288 905 432 295 610},
{72 782 293 076 909 969 047 692 871, 3 616 700 305 949 606 442 745 860},
{112 520 026 437 377 888 386 693 421, - 6 713 617 359 042 776 133 157 980},
{404 478 635 253 675 775 125 051 989, - 6 924 142 547 034 361 419 197 970},
{722 470 248 946 386 015 704 001 979, - 10 939 263 895 937 029 276 853 070},
{120 186 785 450 062 941 356 539 109, - 2 048 940 554 056 284 852 793 500},
{175 877 517 053 724 104 527 625 141, 9 774 866 802 464 728 091 446 980},
{17 591 433 050 891 280 723 545 249, 197 958 922 802 404 948 478 010},
{6 754 680 709 212 682 440 407 891, 366 916 428 929 383 187 631 750},
{37 696 432 109 430 050 822 134 141, 1 985 030 571 004 142 273 734 650},
{4 806 333 651 811 747 084 876 459, - 183 955 060 591 337 489 721 060},
{5 899 021 185 680 060 384 353 649, - 343 671 156 329 623 268 633 010},
{14 209 493 547 192 669 215 712 229, 354 177 718 255 730 489 607 360},
{10 638 589 057 825 857 485 875 079, - 109 508 341 055 873 085 993 540},
{4 086 273 826 948 204 269 926 449, - 136 234 922 661 661 821 524 220},
{194 237 078 314 244 325 837 901, - 1 594 135 852 989 406 093 470},
{62 121 433 366 267 608 925 189, - 815 016 650 071 526 550 210},
{45 222 158 168 729 368 416 479, 822 296 180 060 700 418 350},
{1 037 065 386 897 802 785 521, - 16 197 467 963 896 094 400},
{107 286 739 321 638 724 171, - 636 606 552 325 005 690},
{75 241 773 343 096 597 189, - 2 086 486 861 531 788 870},
{32 189 828 316 001 665 119, - 463 184 199 511 700 850},
{57 759 755 973 270 923 719, 1 101 226 266 659 385 840},
{124 493 516 852 697 869 789, - 6 306 568 048 724 376 390},
{411 098 874 569 204 160 761, 10 618 223 311 746 783 330},
{755 970 481 819 017 666 359, - 44 877 958 887 704 091 000},
{1 745 659 637 259 922 040 891, - 2 439 539 748 319 797 420},
{263 756 456 800 280 869 079, 13 355 630 708 109 409 890},
{842 395 497 838 739 508 971, - 29 667 519 447 206 448 600},
{2 937 943 282 556 695 990 921, - 72 426 791 564 681 250 870},
{7 920 348 070 404 058 981 999, 192 676 873 450 875 961 440},
{5 169 660 988 454 285 302 709, 166 649 367 711 588 997 380},
{886 177 938 151 622 366 179, - 8 493 035 453 811 216 270},
{728 464 989 769 224 398 849, - 42 131 211 122 385 932 490},
{3 070 834 572 854 550 176 269, 68 994 607 418 416 416 540},
{8 514 613 004 521 330 575 781, - 17 038 365 186 350 855 730},
{1 146 966 752 178 419 593 969, 26 912 213 463 585 814 560},
{2 574 865 115 698 378 459 861, 15 596 079 448 445 738 700},
{379 513 682 912 725 164 611, 13 638 643 094 418 562 320},
{594 449 256 479 639 667 599, - 12 913 244 066 863 439 760},
{110 447 380 384 281 098 389, 6 192 740 157 493 776 060},
{256 507 555 102 324 543 441, 9 194 169 897 574 366 170},
{233 229 709 469 185 039 069, 5 976 409 805 530 295 640},
{37 581 490 429 380 786 359, - 186 214 917 057 066 540},
{8 514 626 852 810 334 971, - 73 542 101 059 813 440},
{4 080 474 402 134 041 319, - 73 764 579 934 265 220},
{5 879 048 943 113 008 969, - 245 355 078 926 279 400},
{2 377 710 730 541 854 381, - 84 786 965 708 938 410},
{922 598 363 586 304 151, 720 711 298 295 880}, {22 063 343 662 015 501, - 1 058 123 013 678 690},

```

```

{39 467 145 934 484 239, 1 426 306 035 209 670},
{117 825 185 898 016 771, - 5 935 526 297 736 420},
{222 220 354 234 618 879, 2 445 805 456 304 700}, {87 333 514 566 314 071, 1 960 682 190 133 470},
{225 193 181 412 711 829, - 7 651 875 289 778 310},
{825 488 300 294 350 589, - 46 005 832 524 077 580},
{656 787 969 900 508 601, 7 882 500 351 269 670},
{637 650 627 026 623 741, - 3 036 193 029 585 810},
{12 572 794 214 513 891, - 203 175 514 658 700}, {6 046 011 275 702 759, - 309 734 734 000 470},
{37 319 534 480 966 891, 1 914 882 037 731 060}, {235 130 716 783 264 501, 2 879 751 791 353 050},
{253 241 457 029 085 349, 3 611 977 904 015 730}, {101 153 940 744 046 499, - 151 979 056 612 020},
{16 091 850 849 264 071, - 319 832 525 675 580}, {25 156 365 936 752 821, 903 934 098 336 930},
{38 600 992 986 985 969, - 817 898 161 177 500}, {40 104 632 322 510 719, 823 002 564 522 510},
{55 845 828 112 160 021, 345 161 660 662 020}, {17 660 589 686 891 969, - 91 651 268 887 650},
{7 054 407 314 544 731, 239 249 666 970 540}, {29 157 910 072 166 821, 806 510 486 079 330},
{31 006 675 901 046 191, - 1 394 613 957 140 820},
{81 617 379 830 985 901, 1 134 248 221 657 260}, {12 171 524 212 541 569, 437 410 984 523 460},
{19 071 821 882 943 061, - 374 127 189 340 620}, {2 174 858 130 568 309, 66 428 293 201 650},
{4 336 161 816 621 391, - 88 978 310 918 790}, {5 967 630 018 229 069, 222 416 929 249 620},
{9 444 394 949 178 421, - 514 854 120 968 250}, {44 432 213 709 230 171, - 1 773 428 703 087 630},
{24 220 529 141 894 671, 681 525 547 129 890}, {78 912 029 250 123 619, - 1 292 012 747 663 130},
{24 912 162 310 844 939, 257 671 876 247 400}, {20 584 430 973 368 111, - 708 086 518 865 820},
{12 530 403 491 092 081, 491 560 510 490 850}, {60 589 072 934 028 581, 272 416 434 579 540},
{28 268 738 800 045 951, 801 850 657 043 940}, {51 195 416 680 520 801, - 661 630 554 941 550},
{62 715 851 455 384 201, - 1 159 062 276 171 390}, {31 748 624 074 414 391, 1 263 900 999 296 820},
{37 925 872 090 466 641, - 68 942 363 669 280}, {1 900 590 163 022 891, - 40 208 294 167 800},
{2 710 884 621 209 041, - 47 968 299 367 170}, {5 850 419 122 631 899, 152 737 354 138 680},
{11 646 316 005 876 809, - 638 643 015 320 880}, {37 836 174 255 343 219, - 2 020 580 239 523 430},
{139 267 424 196 089 701, 7 800 374 078 625 030},
{285 966 614 009 370 589, - 9 675 128 969 847 840},
{1 076 101 026 602 217 361, - 15 278 027 625 020 430},
{1 666 412 305 547 602 511, - 50 502 008 931 389 160},
{38 651 286 248 182 019, - 385 734 119 104 920}, {19 546 458 760 194 769, - 1 033 828 536 611 550},
{24 167 142 291 594 931, - 474 312 957 139 650}, {5 727 449 154 331 969, - 60 135 350 031 030},
{3 662 316 247 413 869, - 211 253 445 987 150}, {17 822 924 073 712 069, 231 134 281 464 600},
{6 421 684 635 405 119, - 317 729 490 726 720}, {16 840 800 038 550 469, 763 682 872 456 080},
{9 983 987 973 693 959, - 437 758 029 228 390}, {21 196 121 338 311 761, 941 024 195 201 700},
{112 306 222 983 162 089, 5 417 908 721 136 360}, {368 934 900 336 069 221, 7 074 860 447 141 670},
{261 581 428 260 297 631, - 6 298 642 608 512 340},
{743 351 885 602 382 899, - 18 283 805 762 553 120},
{1 577 321 816 236 050 271, 64 646 769 548 418 000},
{6 475 636 115 578 586 021, - 27 249 499 978 592 730},
{2 445 964 710 947 413 469, 115 657 759 353 009 120},
{4 305 092 898 089 709 199, 215 133 180 112 414 800},
{609 753 256 194 712 949, - 4 818 346 399 298 970},
{546 360 865 580 316 491, - 31 334 868 042 015 900},
{3 430 695 325 377 593 941, - 74 229 824 899 662 030},
{4 046 968 378 278 280 811, 232 668 542 159 286 840},
{22 992 393 554 171 537 281, 689 812 292 626 142 310},
{57 375 562 274 719 103 801, 1 701 962 317 530 931 560},
{123 280 286 854 474 878 989, 113 631 859 071 416 370},
{2 580 339 740 982 497 711, - 148 139 714 129 916 510},

```

```

{15 553 114 794 253 177 291, -4 307 782 258 819 410},
{507 230 818 691 904 941, 10 000 207 194 211 230},
{697 716 801 429 815 039, -8 278 614 166 008 630},
{580 616 082 757 619 869, 3 958 180 912 940 970}, {310 364 372 620 382 971, 8 070 861 061 020 540},
{921 584 727 702 215 201, 43 093 883 450 832 000},
{4 169 906 983 920 543 451, -148 130 908 771 680 660},
{5 582 626 116 684 727 721, 184 926 264 962 905 620},
{8 744 380 117 187 339 371, 430 111 012 911 270 900},
{35 682 124 599 442 264 121, 1 337 970 019 287 967 650},
{111 209 546 254 548 469 679, -3 531 033 841 633 058 400},
{438 621 788 144 838 479 029, 4 934 059 351 168 573 890},
{127 883 021 400 313 892 431, -378 211 873 340 896 560},
{11 899 460 983 804 642 901, 359 324 084 053 816 950},
{10 483 318 717 199 571 301, -24 668 564 448 415 710}, {821 173 377 105 449, 33 363 135 252 240},
{3 239 156 054 338 301, 143 155 824 051 420}, {13 410 402 609 934 109, -669 698 599 629 480},
{4 124 084 953 471 759, -9 133 072 672 410}, {1 020 037 508 847 811, -24 018 600 034 860},
{2 825 333 153 306 441, 49 737 378 443 280}, {2 434 051 908 090 269, 25 587 179 806 230},
{820 726 451 103 169, 46 220 459 446 680}, {2 821 696 553 204 821, -134 680 005 304 260},
{1 652 473 104 344 389, 31 027 844 171 190}, {2 007 338 181 101 069, 110 520 146 502 450},
{4 511 861 558 299 219, 237 974 364 952 380}, {2 422 495 324 796 251, -86 063 183 761 200},
{3 194 271 050 145 401, 159 907 791 272 010}, {975 078 598 994 549, -45 974 566 948 830},
{2 412 785 960 348 869, -4 384 621 213 530}, {312 317 519 749 619, -18 005 095 185 000},
{1 563 956 302 759 369, -33 029 736 109 320}, {2 901 235 110 953 579, 31 804 283 917 560},
{1 768 363 888 360 369, -48 737 616 098 100}, {3 466 236 916 021 019, 195 596 305 269 000},
{13 678 641 284 066 231, -47 751 683 636 100}, {5 436 600 799 549 381, -289 399 956 180 360},
{15 561 590 337 242 209, 101 298 584 643 330}, {9 636 316 155 483 361, -87 424 177 272 570},
{4 933 820 530 665 911, -124 580 889 681 360}, {12 403 179 203 710 739, 138 317 659 273 290},
{11 397 942 852 225 611, -660 134 313 575 040}, {44 090 539 883 932 681, -2 330 357 758 899 210},
{46 750 641 323 229 559, -1 791 438 246 071 640}, {43 484 978 267 096 669, 2 523 475 443 676 950},
{147 059 826 871 718 269, 624 953 807 313 930}, {49 116 220 389 124 469, -1 639 138 249 425 960},
{14 539 700 507 237 081, -437 935 276 377 450}, {22 046 933 082 088 981, 752 092 973 611 110},
{59 295 448 689 064 541, -2 576 509 990 712 100}, {8 965 444 574 246 491, 522 509 005 949 820},
{20 780 659 747 987 301, -488 681 734 881 270}, {58 396 367 828 734 559, -2 974 504 574 748 090},
{274 524 640 223 037 491, -8 068 681 435 025 700},
{47 557 329 473 086 441, -1 684 144 683 230 820},
{100 720 863 998 493 731, -1 378 055 736 280 770}, {30 821 607 749 377 771, 390 615 186 535 950},
{9 284 988 727 532 029, -385 566 240 106 890}, {7 881 140 206 633 919, 245 675 480 177 820},
{4 900 735 076 863 429, 161 296 552 043 970}, {15 521 467 401 626 579, -327 985 696 220 670},
{26 641 059 493 027 339, 464 540 067 581 250}, {40 731 185 864 918 339, -238 904 482 290 330},
{29 473 392 766 121 989, -78 848 518 130 940}, {4 004 206 727 242 321, 168 769 785 893 610},
{11 613 301 685 284 069, 668 148 550 720 560}, {63 948 857 081 671 799, -447 086 971 941 780},
{3 870 443 593 312 009, 193 655 282 631 330}, {668 176 887 962 341, 28 347 737 113 740},
{3 054 369 494 622 169, -179 064 438 119 910}, {2 578 785 692 508 449, 55 150 068 504 210},
{3 330 149 324 544 671, 88 236 354 335 340}, {5 730 867 189 760 499, -228 470 347 851 300},
{4 796 231 862 977 749, -20 576 876 679 300}, {456 718 771 913 099, 21 054 550 915 350},
{1 626 818 404 374 851, -34 800 217 826 040}, {2 206 750 195 706 279, 30 939 559 797 330},
{2 520 403 974 058 099, -66 501 565 632 390}, {1 670 535 513 152 971, -80 017 357 527 030},
{2 467 077 723 579 409, 33 207 113 380 170}, {2 447 584 695 154 079, 143 865 363 086 310},
{470 254 194 389 059, 26 159 186 722 470}, {153 402 820 465 651, -2 026 417 933 230},
{151 840 557 417 079, 479 234 984 370}, {19 310 089 680 961, -273 081 067 710},
{19 745 197 738 699, 103 817 984 580}, {4 964 947 793 249, -52 168 289 100},

```

```

{2 249 042 515 999, 77 442 696 930}, {804 280 562 279, 20 028 453 690},
{788 746 084 429, 30 702 536 580}, {2 389 486 529 401, 4 755 305 730},
{2 323 052 941, 35 158 320}, {653 559 071, -2 214 870}, {43 277 671, -2 460 960},
{255 921 859, 5 935 560}, {173 887 529, -6 577 080}, {723 745 699, -7 281 150},
{730 874 099, 6 896 220}, {31 430 471, 855 210}, {53 287 049, 1 887 270},
{111 315 739, -5 263 350}, {197 132 639, -1 647 330}, {137 287 211, 3 259 080},
{101 868 601, 2 268 570}, {54 479 299, -2 913 180}, {218 651 371, -533 460},
{16 874 479, 785 040}, {97 548 389, -1 160 850}, {9 284 239, 469 860},
{28 353 211, 674 190}, {9 344 981, -551 670}, {8 385 659, 155 910}, {8 403 731, 39 360},
{4 846 559, -31 770}, {3 577 001, -148 800}, {1 456 051, 67 650}, {8 094 499, 434 310},
{39 505 141, -412 020}, {12 243 529, -482 250}, {47 007 029, 2 559 390},
{235 440 259, -4 819 320}, {177 311 671, 1 669 410}, {88 906 961, 4 595 040},
{401 901 451, 490 320}, {40 398 199, -2 358 570}, {75 929 759, -2 108 520},
{5 782 789, 197 700}, {12 421 739, 628 590}, {37 665 311, -212 040},
{19 530 059, -466 170}, {12 319 331, 686 700}, {10 358 519, -269 970},
{25 014 409, 1 002 240}, {10 439 341, 479 220}, {25 978 249, 809 610},
{17 752 979, -487 410}, {51 760 969, 1 391 490}, {69 235 589, 1 706 850},
{187 060 511, -3 620 580}, {303 621 899, 1 528 830}, {154 433 021, 3 884 400},
{236 687 729, -13 145 820}, {15 805 219, 604 470}, {22 338 749, -466 320},
{11 197 361, 611 610}, {47 283 631, 925 500}, {20 865 881, 365 010},
{15 138 061, -658 320}, {828 049, -41 580}, {891 301, -3360}, {226 151, -5430},
{479 159, -11 550}, {1 407 859, -38 460}, {3 805 411, 102 030}, {7 605 551, 156 690},
{18 137 009, -309 330}, {28 478 711, -646 260}, {10 861 021, 54 990}, {6 776 749, -33 000},
{2 948 999, -176 190}, {11 603 981, -158 070}, {16 282 621, -752 970},
{70 962 469, 2 400 930}, {267 423 181, 4 662 240}, {420 550 751, 14 126 550},
{814 682 999, -40 355 130}, {1 902 680 149, 104 401 020}, {5 888 909 039, 162 070 230},
{13 649 570 509, -105 941 520}, {4 238 278 321, 249 830 760}, {2 219 994 349, -87 759 840},
{6 525 585 599, -189 106 680}, {23 380 198 451, -39 805 830}, {3 558 236 491, -209 657 040},
{1 489 230 439, -62 801 280}, {4 518 070 531, 102 876 810}, {2 135 786 359, -39 479 040},
{983 467 949, -35 377 560}, {1 783 036 481, -70 933 500}, {2 434 444 231, -55 173 270},
{1 711 908 101, 65 025 270}, {5 334 021 331, -254 500 410}, {2 632 307 029, 12 073 800},
{54 875 879, 325 860}, {32 981 149, -990 510}, {73 874 069, -1 390 050},
{50 556 169, 1 566 510}, {107 390 099, -4 705 560}, {210 283 031, -175 650},
{7 525 231, -16 080}, {52 459, -1800}, {65 009, -1140}, {7279, 90}, {2761, -150}

```

30  
253 is a relation number with a list {{253, 240}, {3289, -120}, {12 397, 510},  
{39 721, 1860}, {167 233, -5340}, {428 329, 20 310}, {460 207, 8850}, {1771, 30}, {1, 0}}

30  
257 is a relation number with a list

```

{{257, 270}, {3341, 30}, {2827, 120}, {13 621, -630}, {61 423, -3000},
{365 711, -2580}, {166 793, 1080}, {121 561, -6240}, {771 257, 16 860},
{1 105 871, 56 040}, {3 836 753, -70 440}, {8 479 201, -286 860}, {32 535 943, 1 561 590},
{66 163 879, 288 690}, {13 844 333, -145 890}, {3 910 769, 59 910}, {4 271 083, -58 800},
{5 478 469, -236 640}, {9 187 493, 314 310}, {18 633 271, 299 340}, {19 067 087, -970 170},
{86 432 441, -2 901 060}, {154 035 263, 8 360 850}, {909 770 491, 24 760 650},
{1 638 004 663, -53 663 640}, {6 571 021 489, -15 260 100}, {1 562 974 027, 90 430 770},
{6 592 290 809, 154 864 590}, {17 189 846 177, 331 736 970}, {15 542 399 591, 15 129 540},
{1 121 036 827, -37 518 120}, {1 158 240 661, 42 730 350}, {1 161 951 227, -4 842 780},
{81 205 061, 2 820 570}, {152 007 533, 2 620 380}, {6 551 701, -342 330},
{12 189 767, 242 850}, {12 147 619, 20 010}, {398 093, -15 600}, {1 929 299, -44 580},

```

```

{3176263, 36810}, {2724971, -82530}, {380617, -17100}, {1135169, -21870},
{532247, 28890}, {3142339, 88530}, {11253773, 419820}, {20911319, -489300},
{33045317, -1545090}, {153795739, -2126310}, {180264683, 645150},
{68833081, -2931240}, {363542177, 10534260}, {1325329211, -77274090},
{2999108017, 95713380}, {8222261909, -356386200}, {6522482413, -225741000},
{6169692859, -320569410}, {20270635733, 431434080}, {1738868939, -51036300},
{934127923, -31268700}, {1010800789, 12578820}, {1155263573, -3779340},
{312118019, -12427890}, {365137633, 2762520}, {124643201, -2972070},
{47220923, -2369640}, {44172389, 552900}, {15320027, -817230},
{53287151, -1461750}, {170686807, 2896320}, {50390761, 2683890},
{155009293, -2169870}, {243770411, 11457210}, {814433257, -2667960},
{181302449, -8427000}, {1051528607, -43698540}, {710257279, -37754430},
{1818760987, -63221070}, {3765061051, -13732740}, {588604787, -25168950},
{2497766809, -53921730}, {4463377853, 209570880}, {16034068861, -419038350},
{28427171177, -1505757390}, {46830342881, -1147317060},
{53881740803, -755291970}, {65794809781, -2101836540},
{163934399537, -4355276340}, {402488055431, -8286976380},
{918463307573, -14519383740}, {961727911921, -26770987710},
{521104929223, 6425125260}, {172134272891, 3590610840},
{55267189253, -233515470}, {19526124209, 751308930}, {2032348547, 26256810},
{2717563489, 86268660}, {11059643167, -223893810}, {22833544589, 1097965650},
{57499653677, -272255190}, {13828806859, -556506600}, {21551542237, -375224910},
{42076648319, 1800618330}, {170243669353, 5684467800},
{74623714279, 2529596280}, {324892749097, -5377442250},
{577277022929, 3311222860}, {3692893217413, -111699310380},
{1751705542361, -79628301060}, {30089806463, 1063358400},
{81153214591, -1437890010}, {162263125967, 9286686030},
{1128092108449, 16368042930}, {334833406297, 14659023030},
{597299712001, -2289022050}, {34706063593, 841403700},
{53587556501, -2696736750}, {89224874243, -4767438240},
{348608245469, 4424542380}, {239164855607, 7533746070},
{492159788681, 17146265670}, {1306052347493, 14676424440},
{38402910419, -1781042670}, {200467278497, -10289026410},
{1278774613699, 42639634410}, {106505580457, -5302418940},
{117500825849, -4832746290}, {389333126473, -14934736440},
{264704611481, -6705262320}, {822240917257, 4413324300},
{350187546449, -10357518780}, {505799662247, 4958030610},
{20698786939, 876039900}, {83825859877, -84498210}, {934338149, -11764680},
{1266606253, -66465360}, {967454141, -28806630}, {3076618703, -138601860},
{7036090231, -303337950}, {15244566917, 341089770}, {26849492381, 97024830},
{6781080953, 394726530}, {18177595351, -406399710}, {28370640943, -1531209570},
{185641607959, 3456780510}, {263306672317, 2956844400},
{37912824269, -1297888920}, {70429716373, 3518622030}, {14719873661, 474163770},
{5344775287, 198861540}, {6292977301, 313799520}, {4365633557, 128565900},
{1441010051, -72023460}, {138998707, 3300510}, {96962759, -664680},
{20693897, -686970}, {21792829, -1021500}, {87721553, 3711120},
{345749039, 14877600}, {916009423, -25834920}, {3029316311, 79142670},
{5626976707, -22545240}, {2398656301, -85847910}, {1306891003, -57615780},
{4695887809, 6986490}, {248397953, -2216010}, {52642081, 1969500},
{137345683, 6880740}, {69163069, -251490}, {852983, -12000},
{252631, 12450}, {933167, 40680}, {635561, 6030}, {619627, 30780},

```

```

{1034939, 57810}, {1449737, 35070}, {3049819, 112740}, {1500623, 71130},
{1771501, 82890}, {7918427, 43140}, {4968581, -67170}, {513743, -8670},
{568741, 29070}, {3253363, 124410}, {4806671, -8760}, {660233, 16290},
{1967849, -51750}, {346693, 14880}, {1144421, -49950}, {1138253, -51240},
{2820061, -1080}, {46517, -630}, {26471, 1230}, {151373, 1950}, {186839, 480},
{30583, -1590}, {95861, 5400}, {344123, 18150}, {186839, 2790}, {23387, 960},
{89179, -3120}, {334357, -17790}, {938821, -30750}, {3708253, 111090},
{10866731, -625140}, {61513207, -2689320}, {87676321, -4796880},
{342447617, 6409170}, {709732999, -9807510}, {923215703, -41857560},
{603791431, 26275050}, {137422783, 813120}, {1414271, -32100},
{480847, 1410}, {9509, 510}, {46517, -750}, {4369, 30}, {2827, -120}

30
259 is a relation number with a list {{259, 270}, {2849, 30}, {1, 0}}

30
263 is a relation number with a list
{{263, 270}, {1841, -30}, {2893, 30}, {3419, 90}, {1, 0}}

30
269 is a relation number with a list {{269, 270}, {1, 0}}

30
271 is a relation number with a list {{271, 270}, {1, 0}}

30
277 is a relation number with a list
{{277, 270}, {1939, 30}, {3047, -60}, {3601, -150}, {1, 0}}

30
281 is a relation number with a list {{281, 270}, {3091, -30}, {1, 0}}

30
283 is a relation number with a list
{{283, 270}, {3679, -30}, {3113, -90}, {10471, -60}, {8207, -420}, {54619, -2730},
{5377, -240}, {27451, -990}, {76127, -2280}, {251021, -6600}, {62543, 1860},
{197251, -3630}, {348373, 6750}, {743441, -18810}, {2535397, -52170},
{5924039, -307650}, {22268987, 279840}, {33454279, -1174140},
{163675597, -2616990}, {338120759, -12098820}, {182874883, -7361250},
{327251861, 1773150}, {220991587, -9841380}, {1268187241, 38062470},
{3431581873, -141478890}, {10213049179, 19723560}, {1062636983, 50584020},
{105435329, -2318430}, {312992057, 7471710}, {231992929, 494610},
{5897437, -63450}, {965879, 38100}, {3786257, -54690}, {3579101, 78540},
{9548137, 40920}, {3898891, 7680}, {721367, -32280}, {3171581, -57570},
{1480373, 28410}, {863999, -19890}, {2470307, -129600}, {2237681, 90750},
{8792527, 415710}, {17720611, -700200}, {61017913, 2361630},
{108804161, 631290}, {62905523, -1392540}, {68266109, -3307560},
{337520233, 5771700}, {781542139, -23588700}, {881556037, -40569030},
{3102422309, -29718660}, {3305912327, 420900}, {46334741, 1231260},
{128238337, 5001840}, {512089349, -4108380}, {412656733, -18430770},
{2031881419, -46456950}, {3459499823, -55014630}, {1817388361, -35996520},
{4970148163, -176469390}, {8208483769, -341871840}, {1007369347, 441900},
{46030799, 1811640}, {209363117, 2232810}, {147449509, -6657630},
{277806667, 656790}, {4387349, 164430}, {14789863, 501210},
{69741671, -1373340}, {84523327, 3372210}, {61715791, -841830},
{74202883, -2256990}, {78613721, -2959800}, {368148757, 18069630},

```

```

{1911992 431, 46 587 540}, {538 631 353, -5 532 810}, {551 505 589, 12 729 000},
{1 176 880 687, -15 665 430}, {558 482 671, 6 916 560}, {497 708 987, -5 241 690},
{71 192 329, -3 339 060}, {303 395 527, -12 253 950}, {835 762 109, 12 596 940},
{1 235 031 527, 30 038 130}, {981 499 751, -30 973 830}, {2 734 574 947, 69 065 790},
{7 940 032 799, -186 528 000}, {22 829 949 883, -455 568 660}, {14 579 277 889, -648 892 110},
{85 933 365 727, -1 445 585 730}, {182 197 566 931, -3 501 937 680},
{27 396 542 593, -706 912 110}, {48 967 404 251, -2 388 618 360},
{337 783 510 447, -4 362 350 250}, {532 759 158 751, 7 932 069 270},
{370 876 498 063, 3 790 403 100}, {164 990 623 571, -5 783 578 590},
{773 483 017 537, -3 140 582 430}, {254 626 351 231, 1 957 531 740},
{41 664 683 773, 1 887 616 170}, {38 807 233 339, -603 952 590}, {43 657 724 857, 318 429 720},
{9 297 460 411, 426 328 350}, {23 139 010 787, -458 888 220}, {55 071 739 721, -1 429 506 840},
{192 164 652 037, -2 865 787 680}, {44 396 325 991, -1 530 132 120},
{6 365 946 613, 216 891 900}, {21 531 068 179, -245 617 830}, {23 574 143 663, -462 877 350},
{9 226 135 921, -62 481 690}, {5 986 638 317, -87 208 890}, {8 709 351 319, -247 709 460},
{11 184 221 977, -150 989 550}, {3 111 663 391, 151 537 650}, {19 987 514 297, -508 799 550},
{40 845 912 701, -1 101 744 120}, {23 030 613 863, 706 616 280},
{81 425 715 691, -1 443 277 110}, {170 421 901 273, 7 068 874 260},
{217 604 086 339, -6 387 260 550}, {123 735 421 837, 2 527 689 810},
{34 350 215 399, -1 628 560 590}, {42 575 371 547, -527 039 430},
{32 494 706 089, 1 031 413 620}, {144 479 919 533, -888 096 390},
{79 181 146 471, -481 554 930}, {58 337 040 133, -228 997 530}, {16 224 394 811, -549 918 390},
{77 303 399 587, -72 522 360}, {1538 436 959, -24 906 060}, {1 624 069 363, -10 261 050},
{799 040 029, -23 944 890}, {2 507 000 497, -132 409 620}, {2 485 386 089, 59 396 880},
{2 627 052 493, -100 149 240}, {6 557 747 599, 159 636 270}, {3 582 929 707, -21 024 120},
{2 498 693 881, -122 483 340}, {13 874 663 923, 636 713 100}, {37 645 870 391, -607 033 350},
{2 774 161 553, -47 291 730}, {4 542 296 311, -98 874 690}, {1 680 858 407, 6 826 680},
{423 120 941, 3 236 610}, {247 616 227, 2 756 820}, {140 813 159, -3 966 180},
{557 317 843, -84 030}, {8 739 889, 308 250}, {30 815 587, -965 340}, {21 307 919, -122 370},
{4 397 537, -134 130}, {8 137 099, 4830}, {410 633, -17 460}, {2 379 181, -103 020},
{2 751 043, 8340}, {327 431, 60}, {3113, 150}, {10 471, -270}, {16 697, 300},
{29 149, -1470}, {71 033, 1860}, {99 899, -3120}, {16 697, 270}, {12 169, -300},
{37 073, -1560}, {103 861, 1080}, {51 223, 1560}, {72 731, -2010}, {104 993, -1200},
{167 819, -1590}, {204 043, -4260}, {123 671, -540}, {3113, -30}, {1981, 90}, {1, 0}}

30
--- is a relation number with a list {{287, 300}, {3731, 90}, {1, 0}}
287

30
--- is a relation number with a list
289
{{289, 300}, {3179, 90}, {8381, -90}, {3179, 60}, {1, 0}}

30
--- is a relation number with a list
293
{{293, 300}, {2051, 90}, {5567, -150}, {4981, -90}, {9083, -330}, {46001, -2220},
{181367, 510}, {56549, 1110}, {17873, 510}, {6739, -300}, {40727, -330},
{40141, 1950}, {237037, 11130}, {968951, -12840}, {1743643, -12990},
{874019, 42000}, {2338433, -95070}, {11226881, 267270}, {451513, -3510},
{374161, -5940}, {17287, 510}, {15529, 30}, {3223, 120}, {4981, 30}, {1, 0}}

30
--- is a relation number with a list {{299, 300}, {1, 0}}
299

Unresolved cases are :{{28, 17}, {29, 17}}: END

```

```

ln[14]:= RelNumMin[28, 17, 10];
RelNumMin[29, 17, 10];

28
— is a relation number with a list
17
  {{11, -28}, {19, -168}, {13, -336}, {3, -112}, {5, -28}, {1, 84}}

29
— is a relation number with a list {{12, -29}, {1, 203}}
17

ln[6]:= listgood = {};
excp = {};
excp2 = {};
T = {2, 2, 2, 2, 2, 3, 6, 2, 4, 6, 12, 12, 1680, 6, 60, 60};
For[s = 12, s ≤ 27, s++,
  l0 = VerifyList[s, T[[s - 11]]]; l = l0[[2]]; flag = l0[[1]];
  If[flag, listgood = Append[listgood, s];
  Print[s, "/r is a relation number for almost all r;"];
  Print["this is certified by the list of s--good coset ", l];
  excp = Union[excp, l0[[3]]];];];
Print["The list of s such that s/r is a relation number
for almost all r:"];
Print[listgood];
Print["Pairs of (s,r) that require individual verifications:", excp];
For[i = 1, i ≤ Length[excp], i++, s = excp[[i, 1]]; r = excp[[i, 2]];
  If[! RelNum[s, Abs[r], 5000], Print["No answer found for s/r = ", s / r];
  excp2 = Append[excp2, {s, r}]]];
If[excp2 == {}, Print["Individual verification is complete."]];

12/r is a relation number for almost all r;
this is certified by the list of s--good coset
  {{5, 2, 1}, {7, 2, 2}, {17, 2, 2}, {19, 2, 1}}

13/r is a relation number for almost all r;
this is certified by the list of s--good coset
  {{5, 2, 1}, {8, 2, 1}, {18, 2, 1}, {21, 2, 1}}

14/r is a relation number for almost all r;
this is certified by the list of s--good coset {}

15/r is a relation number for almost all r;
this is certified by the list of s--good coset {}

16/r is a relation number for almost all r;
this is certified by the list of s--good coset
  {{7, 2, 2}, {9, 2, 2}, {23, 2, 2}, {25, 2, 2}}

17/r is a relation number for almost all r;
this is certified by the list of s--good coset
  {{5, 3, 1}, {7, 3, 3}, {10, 3, 1}, {12, 3, 1}, {22, 3, 3}, {24, 3, 1},
  {27, 3, 1}, {29, 3, 3}, {39, 3, 1}, {41, 3, 1}, {44, 3, 3}, {46, 3, 1}}

18/r is a relation number for almost all r;

```



this is certified by the list of s--good coset

```
{ {5, 2, 1}, {7, 2, 1}, {11, 3, 1}, {13, 6, 3}, {23, 3, 3}, {25, 6, 3},
  {29, 2, 1}, {31, 2, 1}, {41, 2, 1}, {43, 2, 1}, {47, 3, 3}, {49, 3, 1},
  {59, 3, 1}, {61, 3, 3}, {65, 2, 1}, {67, 2, 1}, {77, 2, 1}, {79, 2, 1},
  {83, 6, 3}, {85, 3, 3}, {95, 6, 3}, {97, 3, 1}, {101, 2, 1}, {103, 2, 1} }
```

19/r is a relation number for almost all r;

this is certified by the list of s--good coset

```
{ {7, 2, 2}, {8, 2, 1}, {11, 2, 2}, {12, 2, 1}, {26, 2, 1}, {27, 2, 2}, {30, 2, 1}, {31, 2, 2} }
```

20/r is a relation number for almost all r;

this is certified by the list of s--good coset { {9, 2, 2}, {11, 4, 4},

```
{29, 4, 4}, {31, 2, 2}, {49, 2, 2}, {51, 4, 4}, {69, 4, 4}, {71, 2, 2} }
```

21/r is a relation number for almost all r;

this is certified by the list of s--good coset

```
{ {8, 2, 1}, {13, 6, 3}, {29, 6, 3}, {34, 2, 1}, {50, 2, 1}, {55, 3, 1},
  {71, 3, 1}, {76, 2, 1}, {92, 2, 1}, {97, 6, 3}, {113, 6, 3}, {118, 2, 1} }
```

22/r is a relation number for almost all r;

this is certified by the list of s--good coset

```
{ {5, 2, 1}, {9, 2, 1}, {13, 3, 1}, {17, 12, 2}, {27, 4, 4}, {31, 12, 2}, {35, 2, 1},
  {39, 2, 1}, {49, 2, 1}, {53, 2, 1}, {57, 3, 1}, {61, 3, 1}, {71, 3, 1}, {75, 3, 1},
  {79, 2, 1}, {83, 2, 1}, {93, 2, 1}, {97, 2, 1}, {101, 4, 4}, {105, 6, 1}, {115, 4, 4},
  {119, 3, 1}, {123, 2, 1}, {127, 2, 1}, {137, 2, 1}, {141, 2, 1}, {145, 3, 1}, {149, 4, 4},
  {159, 6, 1}, {163, 4, 4}, {167, 2, 1}, {171, 2, 1}, {181, 2, 1}, {185, 2, 1}, {189, 3, 1},
  {193, 3, 1}, {203, 3, 1}, {207, 3, 1}, {211, 2, 1}, {215, 2, 1}, {225, 2, 1}, {229, 2, 1},
  {233, 12, 2}, {237, 4, 4}, {247, 12, 2}, {251, 3, 1}, {255, 2, 1}, {259, 2, 1} }
```

23/r is a relation number for almost all r;

this is certified by the list of s--good coset

```
{ {5, 2, 1}, {7, 2, 2}, {9, 2, 1}, {10, 3, 1}, {13, 2, 2}, {14, 3, 1}, {16, 2, 1}, {18, 3, 1},
  {28, 6, 1}, {30, 2, 1}, {32, 4, 1}, {33, 2, 2}, {36, 3, 1}, {37, 2, 1}, {39, 2, 2},
  {41, 2, 1}, {51, 2, 1}, {53, 2, 2}, {55, 2, 1}, {56, 3, 3}, {59, 2, 2}, {60, 3, 1},
  {62, 2, 1}, {64, 3, 1}, {74, 3, 1}, {76, 2, 1}, {78, 3, 1}, {79, 2, 2}, {82, 3, 3},
  {83, 2, 1}, {85, 2, 2}, {87, 2, 1}, {97, 2, 1}, {99, 2, 2}, {101, 2, 1}, {102, 3, 1},
  {105, 2, 2}, {106, 4, 2}, {108, 2, 1}, {110, 4, 1}, {120, 3, 1}, {122, 2, 1},
  {124, 3, 1}, {125, 2, 2}, {128, 3, 1}, {129, 2, 1}, {131, 2, 2}, {133, 2, 1},
  {143, 2, 1}, {145, 2, 2}, {147, 2, 1}, {148, 3, 1}, {151, 2, 2}, {152, 3, 1},
  {154, 2, 1}, {156, 3, 1}, {166, 4, 1}, {168, 2, 1}, {170, 4, 2}, {171, 2, 2},
  {174, 3, 1}, {175, 2, 1}, {177, 2, 2}, {179, 2, 1}, {189, 2, 1}, {191, 2, 2},
  {193, 2, 1}, {194, 3, 3}, {197, 2, 2}, {198, 3, 1}, {200, 2, 1}, {202, 3, 1},
  {212, 3, 1}, {214, 2, 1}, {216, 3, 1}, {217, 2, 2}, {220, 3, 3}, {221, 2, 1},
  {223, 2, 2}, {225, 2, 1}, {235, 2, 1}, {237, 2, 2}, {239, 2, 1}, {240, 3, 1},
  {243, 2, 2}, {244, 4, 1}, {246, 2, 1}, {248, 6, 1}, {258, 3, 1}, {260, 2, 1},
  {262, 3, 1}, {263, 2, 2}, {266, 3, 1}, {267, 2, 1}, {269, 2, 2}, {271, 2, 1} }
```

For s = 24, the following remainders are not eliminated:

```
{1261, 6299, 34021, 39059} modulo 1680 * s
```

25/r is a relation number for almost all r;

this is certified by the list of s--good coset

```
{ {7, 2, 1}, {9, 2, 2}, {11, 2, 2}, {14, 3, 3}, {16, 2, 1}, {18, 3, 1}, {32, 3, 3}, {34, 2, 1},
  {36, 3, 1}, {39, 2, 2}, {41, 2, 2}, {43, 2, 1}, {57, 2, 1}, {59, 2, 2}, {61, 2, 2},
  {64, 6, 3}, {66, 2, 1}, {68, 3, 3}, {82, 3, 3}, {84, 2, 1}, {86, 6, 3}, {89, 2, 2},
  {91, 2, 2}, {93, 2, 1}, {107, 2, 1}, {109, 2, 2}, {111, 2, 2}, {114, 3, 1}, {116, 2, 1},
  {118, 3, 3}, {132, 3, 1}, {134, 2, 1}, {136, 3, 3}, {139, 2, 2}, {141, 2, 2}, {143, 2, 1} }
```

26/r is a relation number for almost all r;

this is certified by the list of s--good coset

```
{ {7, 2, 2}, {11, 3, 1}, {15, 2, 2}, {19, 4, 2}, {33, 12, 2}, {37, 2, 2}, {41, 30, 1},
  {45, 2, 2}, {59, 2, 2}, {63, 3, 1}, {67, 2, 2}, {71, 3, 1}, {85, 3, 1}, {89, 2, 2},
  {93, 3, 1}, {97, 2, 2}, {111, 2, 2}, {115, 4, 2}, {119, 2, 2}, {123, 4, 2}, {137, 5, 5},
  {141, 2, 2}, {145, 3, 1}, {149, 2, 2}, {163, 2, 2}, {167, 3, 1}, {171, 2, 2}, {175, 5, 1},
  {189, 4, 2}, {193, 2, 2}, {197, 4, 2}, {201, 2, 2}, {215, 2, 2}, {219, 3, 1}, {223, 2, 2},
  {227, 3, 1}, {241, 3, 1}, {245, 2, 2}, {249, 3, 1}, {253, 2, 2}, {267, 2, 2}, {271, 5, 5},
  {275, 2, 2}, {279, 12, 2}, {293, 4, 2}, {297, 2, 2}, {301, 3, 1}, {305, 2, 2},
  {319, 2, 2}, {323, 3, 1}, {327, 2, 2}, {331, 4, 2}, {345, 5, 1}, {349, 2, 2}, {353, 5, 5},
  {357, 2, 2}, {371, 2, 2}, {375, 3, 1}, {379, 2, 2}, {383, 3, 1}, {397, 3, 1}, {401, 2, 2},
  {405, 3, 1}, {409, 2, 2}, {423, 2, 2}, {427, 4, 2}, {431, 2, 2}, {435, 4, 2}, {449, 5, 5},
  {453, 2, 2}, {457, 3, 1}, {461, 2, 2}, {475, 2, 2}, {479, 3, 1}, {483, 2, 2},
  {487, 20, 4}, {501, 4, 2}, {505, 2, 2}, {509, 4, 2}, {513, 2, 2}, {527, 2, 2},
  {531, 3, 1}, {535, 2, 2}, {539, 3, 1}, {553, 3, 1}, {557, 2, 2}, {561, 3, 1},
  {565, 2, 2}, {579, 2, 2}, {583, 20, 4}, {587, 2, 2}, {591, 5, 5}, {605, 4, 2},
  {609, 2, 2}, {613, 3, 1}, {617, 2, 2}, {631, 2, 2}, {635, 3, 1}, {639, 2, 2},
  {643, 4, 2}, {657, 5, 5}, {661, 2, 2}, {665, 5, 1}, {669, 2, 2}, {683, 2, 2},
  {687, 3, 1}, {691, 2, 2}, {695, 3, 1}, {709, 3, 1}, {713, 2, 2}, {717, 3, 1}, {721, 2, 2},
  {735, 2, 2}, {739, 4, 2}, {743, 2, 2}, {747, 4, 2}, {761, 30, 1}, {765, 2, 2},
  {769, 3, 1}, {773, 2, 2}, {787, 2, 2}, {791, 3, 1}, {795, 2, 2}, {799, 30, 1},
  {813, 4, 2}, {817, 2, 2}, {821, 4, 2}, {825, 2, 2}, {839, 2, 2}, {843, 3, 1}, {847, 2, 2},
  {851, 3, 1}, {865, 3, 1}, {869, 2, 2}, {873, 3, 1}, {877, 2, 2}, {891, 2, 2}, {895, 5, 1},
  {899, 2, 2}, {903, 5, 5}, {917, 4, 2}, {921, 2, 2}, {925, 3, 1}, {929, 2, 2},
  {943, 2, 2}, {947, 3, 1}, {951, 2, 2}, {955, 4, 2}, {969, 5, 5}, {973, 2, 2},
  {977, 20, 4}, {981, 2, 2}, {995, 2, 2}, {999, 3, 1}, {1003, 2, 2}, {1007, 3, 1},
  {1021, 3, 1}, {1025, 2, 2}, {1029, 3, 1}, {1033, 2, 2}, {1047, 2, 2}, {1051, 4, 2},
  {1055, 2, 2}, {1059, 4, 2}, {1073, 20, 4}, {1077, 2, 2}, {1081, 3, 1}, {1085, 2, 2},
  {1099, 2, 2}, {1103, 3, 1}, {1107, 2, 2}, {1111, 5, 5}, {1125, 4, 2}, {1129, 2, 2},
  {1133, 4, 2}, {1137, 2, 2}, {1151, 2, 2}, {1155, 3, 1}, {1159, 2, 2}, {1163, 3, 1},
  {1177, 3, 1}, {1181, 2, 2}, {1185, 3, 1}, {1189, 2, 2}, {1203, 2, 2}, {1207, 5, 5},
  {1211, 2, 2}, {1215, 5, 1}, {1229, 4, 2}, {1233, 2, 2}, {1237, 3, 1}, {1241, 2, 2},
  {1255, 2, 2}, {1259, 3, 1}, {1263, 2, 2}, {1267, 4, 2}, {1281, 12, 2}, {1285, 2, 2},
  {1289, 5, 5}, {1293, 2, 2}, {1307, 2, 2}, {1311, 3, 1}, {1315, 2, 2}, {1319, 3, 1},
  {1333, 3, 1}, {1337, 2, 2}, {1341, 3, 1}, {1345, 2, 2}, {1359, 2, 2}, {1363, 4, 2},
  {1367, 2, 2}, {1371, 4, 2}, {1385, 5, 1}, {1389, 2, 2}, {1393, 3, 1}, {1397, 2, 2},
  {1411, 2, 2}, {1415, 3, 1}, {1419, 2, 2}, {1423, 5, 5}, {1437, 4, 2}, {1441, 2, 2},
  {1445, 4, 2}, {1449, 2, 2}, {1463, 2, 2}, {1467, 3, 1}, {1471, 2, 2}, {1475, 3, 1},
  {1489, 3, 1}, {1493, 2, 2}, {1497, 3, 1}, {1501, 2, 2}, {1515, 2, 2}, {1519, 30, 1},
  {1523, 2, 2}, {1527, 12, 2}, {1541, 4, 2}, {1545, 2, 2}, {1549, 3, 1}, {1553, 2, 2} }
```

27/r is a relation number for almost all r;

this is certified by the list of s--good coset

```
{ {5, 2, 1}, {8, 2, 1}, {10, 3, 1}, {11, 2, 1}, {16, 3, 1}, {17, 5, 1}, {19, 6, 2},
  {22, 3, 3}, {32, 6, 1}, {35, 5, 1}, {37, 10, 10}, {38, 12, 2}, {43, 2, 1}, {44, 6, 3},
```

```

{46, 2, 1}, {49, 2, 1}, {59, 2, 1}, {62, 2, 1}, {64, 12, 1}, {65, 2, 1}, {70, 3, 3},
{71, 3, 1}, {73, 3, 1}, {76, 3, 1}, {86, 3, 1}, {89, 3, 1}, {91, 3, 1}, {92, 3, 3},
{97, 2, 1}, {98, 4, 1}, {100, 2, 1}, {103, 2, 1}, {113, 2, 1}, {116, 2, 1}, {118, 4, 1},
{119, 2, 1}, {124, 4, 1}, {125, 5, 1}, {127, 5, 1}, {130, 4, 1}, {140, 3, 3}, {143, 5, 1},
{145, 5, 1}, {146, 3, 1}, {151, 2, 1}, {152, 3, 1}, {154, 2, 1}, {157, 2, 1}, {167, 2, 1},
{170, 2, 1}, {172, 3, 1}, {173, 2, 1}, {178, 3, 1}, {179, 6, 2}, {181, 6, 2}, {184, 3, 3},
{194, 4, 1}, {197, 10, 10}, {199, 10, 5}, {200, 4, 1}, {205, 2, 1}, {206, 4, 1},
{208, 2, 1}, {211, 2, 1}, {221, 2, 1}, {224, 2, 1}, {226, 4, 1}, {227, 2, 1}, {232, 3, 3},
{233, 3, 1}, {235, 3, 1}, {238, 3, 1}, {248, 3, 1}, {251, 3, 1}, {253, 3, 1}, {254, 3, 3},
{259, 2, 1}, {260, 5, 1}, {262, 2, 1}, {265, 2, 1}, {275, 2, 1}, {278, 2, 1},
{280, 5, 1}, {281, 2, 1}, {286, 10, 1}, {287, 5, 1}, {289, 10, 5}, {292, 6, 1},
{302, 3, 3}, {305, 5, 1}, {307, 6, 2}, {308, 3, 1}, {313, 2, 1}, {314, 3, 1},
{316, 2, 1}, {319, 2, 1}, {329, 2, 1}, {332, 2, 1}, {334, 3, 1}, {335, 2, 1},
{340, 3, 1}, {341, 6, 2}, {343, 6, 2}, {346, 3, 3}, {356, 6, 1}, {359, 12, 4},
{361, 12, 4}, {362, 12, 2}, {367, 2, 1}, {368, 6, 3}, {370, 2, 1}, {373, 2, 1},
{383, 2, 1}, {386, 2, 1}, {388, 5, 1}, {389, 2, 1}, {394, 3, 3}, {395, 3, 1}, {397, 3, 1},
{400, 3, 1}, {410, 3, 1}, {413, 3, 1}, {415, 3, 1}, {416, 3, 3}, {421, 2, 1}, {422, 4, 1},
{424, 2, 1}, {427, 2, 1}, {437, 2, 1}, {440, 2, 1}, {442, 4, 1}, {443, 2, 1},
{448, 4, 1}, {449, 15, 5}, {451, 15, 5}, {454, 4, 1}, {464, 3, 3}, {467, 6, 2},
{469, 6, 2}, {470, 3, 1}, {475, 2, 1}, {476, 3, 1}, {478, 2, 1}, {481, 2, 1}, {491, 2, 1},
{494, 2, 1}, {496, 3, 1}, {497, 2, 1}, {502, 3, 1}, {503, 6, 2}, {505, 5, 1}, {508, 3, 3},
{518, 4, 1}, {521, 10, 5}, {523, 5, 1}, {524, 4, 1}, {529, 2, 1}, {530, 4, 1},
{532, 2, 1}, {535, 2, 1}, {545, 2, 1}, {548, 2, 1}, {550, 4, 1}, {551, 2, 1}, {556, 3, 3},
{557, 3, 1}, {559, 3, 1}, {562, 3, 1}, {572, 3, 1}, {575, 3, 1}, {577, 3, 1}, {578, 3, 3},
{583, 2, 1}, {584, 12, 1}, {586, 2, 1}, {589, 2, 1}, {599, 2, 1}, {602, 2, 1},
{604, 6, 3}, {605, 2, 1}, {610, 5, 1}, {611, 10, 5}, {613, 10, 10}, {616, 6, 1},
{626, 3, 3}, {629, 6, 2}, {631, 6, 2}, {632, 3, 1}, {637, 2, 1}, {638, 3, 1}, {640, 2, 1},
{643, 2, 1}, {653, 2, 1}, {656, 2, 1}, {658, 3, 1}, {659, 2, 1}, {664, 3, 1}, {665, 5, 1},
{667, 5, 1}, {670, 3, 3}, {680, 5, 1}, {683, 5, 1}, {685, 5, 1}, {686, 12, 2},
{691, 2, 1}, {692, 5, 1}, {694, 2, 1}, {697, 2, 1}, {707, 2, 1}, {710, 2, 1},
{712, 12, 1}, {713, 2, 1}, {718, 3, 3}, {719, 3, 1}, {721, 3, 1}, {724, 3, 1},
{734, 3, 1}, {737, 3, 1}, {739, 3, 1}, {740, 3, 3}, {745, 2, 1}, {746, 4, 1}, {748, 2, 1},
{751, 2, 1}, {761, 2, 1}, {764, 2, 1}, {766, 4, 1}, {767, 2, 1}, {772, 4, 1},
{773, 10, 10}, {775, 5, 1}, {778, 4, 1}, {788, 3, 3}, {791, 6, 2}, {793, 5, 1},
{794, 3, 1}, {799, 2, 1}, {800, 3, 1}, {802, 2, 1}, {805, 2, 1}, {815, 2, 1}, {818, 2, 1},
{820, 3, 1}, {821, 2, 1}, {826, 3, 1}, {827, 5, 1}, {829, 6, 2}, {832, 3, 3}, {842, 4, 1},
{845, 5, 1}, {847, 10, 10}, {848, 4, 1}, {853, 2, 1}, {854, 4, 1}, {856, 2, 1},
{859, 2, 1}, {869, 2, 1}, {872, 2, 1}, {874, 4, 1}, {875, 2, 1}, {880, 3, 3}, {881, 3, 1},
{883, 3, 1}, {886, 3, 1}, {896, 3, 1}, {899, 3, 1}, {901, 3, 1}, {902, 3, 3}, {907, 2, 1},
{908, 12, 1}, {910, 2, 1}, {913, 2, 1}, {923, 2, 1}, {926, 2, 1}, {928, 5, 1},
{929, 2, 1}, {934, 12, 2}, {935, 5, 1}, {937, 5, 1}, {940, 5, 1}, {950, 3, 3},
{953, 5, 1}, {955, 5, 1}, {956, 3, 1}, {961, 2, 1}, {962, 3, 1}, {964, 2, 1}, {967, 2, 1},
{977, 2, 1}, {980, 2, 1}, {982, 3, 1}, {983, 2, 1}, {988, 3, 1}, {989, 6, 2},
{991, 6, 2}, {994, 3, 3}, {1004, 6, 1}, {1007, 10, 10}, {1009, 10, 5}, {1010, 5, 1},
{1015, 2, 1}, {1016, 6, 3}, {1018, 2, 1}, {1021, 2, 1}, {1031, 2, 1}, {1034, 2, 1},
{1036, 12, 1}, {1037, 2, 1}, {1042, 3, 3}, {1043, 3, 1}, {1045, 3, 1}, {1048, 3, 1},
{1058, 3, 1}, {1061, 3, 1}, {1063, 3, 1}, {1064, 3, 3}, {1069, 2, 1}, {1070, 4, 1},
{1072, 2, 1}, {1075, 2, 1}, {1085, 2, 1}, {1088, 2, 1}, {1090, 4, 1}, {1091, 2, 1},
{1096, 4, 1}, {1097, 5, 1}, {1099, 10, 5}, {1102, 4, 1}, {1112, 3, 3}, {1115, 5, 1},
{1117, 6, 2}, {1118, 3, 1}, {1123, 2, 1}, {1124, 3, 1}, {1126, 2, 1}, {1129, 2, 1},
{1139, 2, 1}, {1142, 2, 1}, {1144, 3, 1}, {1145, 2, 1}, {1150, 3, 1}, {1151, 6, 2},

```

```

{1153, 6, 2}, {1156, 3, 3}, {1166, 4, 1}, {1169, 15, 5}, {1171, 15, 5}, {1172, 4, 1},
{1177, 2, 1}, {1178, 4, 1}, {1180, 2, 1}, {1183, 2, 1}, {1193, 2, 1}, {1196, 2, 1},
{1198, 4, 1}, {1199, 2, 1}, {1204, 3, 3}, {1205, 3, 1}, {1207, 3, 1}, {1210, 3, 1},
{1220, 3, 1}, {1223, 3, 1}, {1225, 3, 1}, {1226, 3, 3}, {1231, 2, 1}, {1232, 5, 1},
{1234, 2, 1}, {1237, 2, 1}, {1247, 2, 1}, {1250, 2, 1}, {1252, 6, 3}, {1253, 2, 1},
{1258, 12, 2}, {1259, 12, 4}, {1261, 12, 4}, {1264, 6, 1}, {1274, 3, 3}, {1277, 6, 2},
{1279, 6, 2}, {1280, 3, 1}, {1285, 2, 1}, {1286, 3, 1}, {1288, 2, 1}, {1291, 2, 1},
{1301, 2, 1}, {1304, 2, 1}, {1306, 3, 1}, {1307, 2, 1}, {1312, 3, 1}, {1313, 6, 2},
{1315, 5, 1}, {1318, 3, 3}, {1328, 6, 1}, {1331, 10, 5}, {1333, 5, 1}, {1334, 10, 1},
{1339, 2, 1}, {1340, 5, 1}, {1342, 2, 1}, {1345, 2, 1}, {1355, 2, 1}, {1358, 2, 1},
{1360, 5, 1}, {1361, 2, 1}, {1366, 3, 3}, {1367, 3, 1}, {1369, 3, 1}, {1372, 3, 1},
{1382, 3, 1}, {1385, 3, 1}, {1387, 3, 1}, {1388, 3, 3}, {1393, 2, 1}, {1394, 4, 1},
{1396, 2, 1}, {1399, 2, 1}, {1409, 2, 1}, {1412, 2, 1}, {1414, 4, 1}, {1415, 2, 1},
{1420, 4, 1}, {1421, 10, 5}, {1423, 10, 10}, {1426, 4, 1}, {1436, 3, 3}, {1439, 6, 2},
{1441, 6, 2}, {1442, 3, 1}, {1447, 2, 1}, {1448, 3, 1}, {1450, 2, 1}, {1453, 2, 1},
{1463, 2, 1}, {1466, 2, 1}, {1468, 3, 1}, {1469, 2, 1}, {1474, 3, 1}, {1475, 5, 1},
{1477, 5, 1}, {1480, 3, 3}, {1490, 4, 1}, {1493, 5, 1}, {1495, 5, 1}, {1496, 4, 1},
{1501, 2, 1}, {1502, 4, 1}, {1504, 2, 1}, {1507, 2, 1}, {1517, 2, 1}, {1520, 2, 1},
{1522, 4, 1}, {1523, 2, 1}, {1528, 3, 3}, {1529, 3, 1}, {1531, 3, 1}, {1534, 3, 1},
{1544, 3, 1}, {1547, 3, 1}, {1549, 3, 1}, {1550, 3, 3}, {1555, 2, 1}, {1556, 12, 1},
{1558, 2, 1}, {1561, 2, 1}, {1571, 2, 1}, {1574, 2, 1}, {1576, 6, 3}, {1577, 2, 1},
{1582, 12, 2}, {1583, 10, 10}, {1585, 5, 1}, {1588, 6, 1}, {1598, 3, 3}, {1601, 6, 2},
{1603, 5, 1}, {1604, 3, 1}, {1609, 2, 1}, {1610, 3, 1}, {1612, 2, 1}, {1615, 2, 1}

```

The list of  $s$  such that  $s/r$  is a relation number  
for almost all  $r$ :

```
{12, 13, 14, 15, 16, 17, 18, 19, 20, 21, 22, 23, 25, 26, 27}
```

Pairs of (s,r) that require individual verifications:

```
{ {12, -1}, {12, 1}, {12, 5}, {12, 7}, {12, 17}, {12, 19}, {13, -2}, {13, -1}, {13, 1},
  {13, 2}, {13, 5}, {13, 8}, {13, 18}, {13, 21}, {16, -1}, {16, 1}, {16, 7}, {16, 9},
  {16, 23}, {16, 25}, {17, -3}, {17, -1}, {17, 1}, {17, 3}, {17, 5}, {17, 7}, {17, 10},
  {17, 12}, {17, 22}, {17, 24}, {17, 27}, {17, 29}, {17, 39}, {17, 41}, {17, 44},
  {17, 46}, {18, -1}, {18, 1}, {18, 5}, {18, 7}, {18, 11}, {18, 13}, {18, 23}, {18, 25},
  {18, 29}, {18, 31}, {18, 43}, {18, 47}, {18, 49}, {18, 83}, {18, 95}, {19, -2},
  {19, -1}, {19, 1}, {19, 2}, {19, 7}, {19, 8}, {19, 11}, {19, 12}, {19, 26}, {19, 27},
  {19, 30}, {19, 31}, {20, -1}, {20, 1}, {20, 9}, {20, 11}, {20, 29}, {20, 31}, {20, 51},
  {20, 69}, {21, -2}, {21, -1}, {21, 1}, {21, 2}, {21, 8}, {21, 13}, {21, 29}, {21, 34},
  {21, 55}, {21, 97}, {21, 113}, {22, -3}, {22, -1}, {22, 1}, {22, 3}, {22, 5}, {22, 9},
  {22, 13}, {22, 17}, {22, 27}, {22, 31}, {22, 35}, {22, 39}, {22, 53}, {22, 57},
  {22, 61}, {22, 75}, {22, 105}, {22, 233}, {22, 247}, {23, -4}, {23, -3}, {23, -2},
  {23, -1}, {23, 1}, {23, 2}, {23, 3}, {23, 4}, {23, 5}, {23, 7}, {23, 9}, {23, 10},
  {23, 13}, {23, 14}, {23, 16}, {23, 18}, {23, 28}, {23, 30}, {23, 32}, {23, 33},
  {23, 36}, {23, 37}, {23, 39}, {23, 41}, {23, 51}, {23, 55}, {23, 56}, {23, 59},
  {23, 60}, {23, 64}, {23, 74}, {23, 78}, {23, 110}, {25, -3}, {25, -2}, {25, -1},
  {25, 1}, {25, 2}, {25, 3}, {25, 7}, {25, 9}, {25, 11}, {25, 14}, {25, 16}, {25, 18},
  {25, 32}, {25, 34}, {25, 36}, {25, 39}, {25, 41}, {25, 43}, {25, 57}, {25, 61},
  {25, 64}, {25, 68}, {25, 86}, {26, -5}, {26, -3}, {26, -1}, {26, 1}, {26, 3}, {26, 5},
  {26, 7}, {26, 11}, {26, 15}, {26, 19}, {26, 33}, {26, 37}, {26, 41}, {26, 45},
  {26, 59}, {26, 63}, {26, 67}, {26, 71}, {26, 85}, {26, 93}, {26, 115}, {26, 119},
  {26, 123}, {26, 279}, {26, 457}, {26, 487}, {26, 739}, {26, 761}, {27, -5}, {27, -4},
  {27, -2}, {27, -1}, {27, 1}, {27, 2}, {27, 4}, {27, 5}, {27, 8}, {27, 10}, {27, 11},
  {27, 16}, {27, 17}, {27, 19}, {27, 22}, {27, 32}, {27, 35}, {27, 37}, {27, 38},
  {27, 43}, {27, 44}, {27, 46}, {27, 49}, {27, 59}, {27, 64}, {27, 65}, {27, 70},
  {27, 71}, {27, 73}, {27, 76}, {27, 86}, {27, 92}, {27, 98}, {27, 100}, {27, 118},
  {27, 125}, {27, 127}, {27, 130}, {27, 143}, {27, 145}, {27, 197}, {27, 199}, {27, 233},
  {27, 251}, {27, 254}, {27, 260}, {27, 286}, {27, 287}, {27, 289}, {27, 359}, {27, 361}}
```

known cases

known cases

$\frac{12}{5}$  is a relation number with a list  $\{\{5, 12\}, \{35, 24\}, \{55, -12\}, \{1, 0\}\}$

$\frac{12}{7}$  is a relation number with a list  $\{\{7, 12\}, \{35, -24\}, \{77, -36\}, \{35, -12\}, \{1, 0\}\}$

$\frac{12}{17}$  is a relation number with a list  $\{\{17, 12\}, \{85, 24\}, \{187, -12\}, \{85, 24\}\}$

$\frac{12}{19}$  is a relation number with a list  $\{\{19, 24\}, \{95, 24\}, \{1, 0\}\}$

known cases

known cases

known cases

known cases

$\frac{13}{5}$  is a relation number with a list  $\{\{5, 13\}, \{40, 39\}, \{1, 0\}\}$

$\frac{13}{8}$  is a relation number with a list  $\{\{8, 13\}, \{20, 13\}, \{24, -13\}, \{1, 0\}\}$

$\frac{13}{18}$  is a relation number with a list  $\{\{18, 13\}, \{45, -13\}, \{1, 0\}\}$

$\frac{13}{21}$  is a relation number with a list  $\{\{21, 26\}, \{105, -26\}, \{1, 0\}\}$

known cases

known cases

$\frac{16}{7}$  is a relation number with a list  $\{\{7, 16\}, \{63, 32\}, \{1, 0\}\}$

$\frac{16}{9}$  is a relation number with a list  $\{\{9, 16\}, \{63, -32\}, \{1, 0\}\}$

$\frac{16}{23}$  is a relation number with a list  $\{\{23, 16\}, \{161, 32\}, \{1, 0\}\}$

$\frac{16}{25}$  is a relation number with a list  $\{\{25, 32\}, \{175, -16\}, \{1, 0\}\}$

known cases

known cases

known cases

known cases

$\frac{17}{5}$  is a relation number with a list  $\{\{5, 17\}, \{60, 119\}, \{295, 408\}, \{565, -119\}, \{30, 17\}, \{20, -17\}, \{15, 17\}, \{10, 17\}, \{35, 34\}, \{1, 0\}\}$

$\frac{17}{7}$  is a relation number with a list  $\{\{7, 17\}, \{70, 51\}, \{133, 34\}, \{21, 17\}, \{28, -17\}, \{42, 17\}, \{56, -17\}, \{35, -34\}, \{1, 0\}\}$

$\frac{17}{10}$  is a relation number with a list  $\{\{10, 17\}, \{70, -51\}, \{95, 68\}, \{270, 221\}, \{490, -289\}, \{440, -51\}, \{95, -68\}\}$

$\frac{17}{12}$  is a relation number with a list  $\{\{12, 17\}, \{30, -17\}, \{1, 0\}\}$

$\frac{17}{22}$  is a relation number with a list  $\{\{22, 17\}, \{55, 17\}, \{44, 17\}, \{154, -17\}, \{1, 0\}\}$

$\frac{17}{24}$  is a relation number with a list  $\{\{24, 17\}, \{56, 17\}, \{120, -17\}, \{1, 0\}\}$

$\frac{17}{27}$  is a relation number with a list  $\{\{27, 34\}, \{189, 34\}, \{135, 34\}, \{1, 0\}\}$

$\frac{17}{29}$  is a relation number with a list  $\{\{29, 34\}, \{145, 34\}, \{261, 68\}, \{319, 85\}, \{609, 34\}, \{87, -17\}, \{58, 17\}, \{203, 17\}, \{1, 0\}\}$

$\frac{17}{39}$  is a relation number with a list  $\{\{39, 34\}, \{195, -34\}, \{117, -17\}, \{78, 17\}, \{91, 17\}, \{78, 17\}\}$

$\frac{17}{41}$  is a relation number with a list  $\{\{41, 34\}, \{287, -34\}, \{615, -119\}, \{820, -119\}, \{533, 17\}, \{246, -17\}, \{328, -17\}, \{205, -17\}, \{1, 0\}\}$

```

17
— is a relation number with a list {{44, 51}, {308, 17}, {1, 0}}
44

17
— is a relation number with a list
46
  {{46, 51}, {115, 17}, {92, 17}, {322, -51}, {368, 51}, {506, -85}, {92, 17}}

known cases

known cases

18
— is a relation number with a list {{5, 18}, {65, 144}, {395, 702}, {1535, 2016},
5
  {2405, -1422}, {2195, -792}, {905, 702}, {1015, -144}, {35, 36}, {1, 0}}

18
— is a relation number with a list {{7, 18}, {77, 72}, {35, -36}, {1, 0}}
7

18
— is a relation number with a list {{11, 18}, {77, 54}, {253, 180},
11
  {803, -648}, {1705, 1242}, {5093, -3006}, {10109, -18}, {77, -54}}

18
— is a relation number with a list
13
  {{13, 18}, {65, 36}, {91, 36}, {221, 144}, {871, 540}, {2717, 504},
  {2561, -540}, {1807, -486}, {1781, -1080}, {4927, 396}, {2275, -1152},
  {377, -162}, {689, -198}, {1235, 846}, {5057, -3006}, {12415, 4698},
  {21827, -630}, {2899, 162}, {221, 36}, {65, 18}, {91, 18}, {1, 0}}

18
— is a relation number with a list {{23, 18}, {115, -36}, {161, 54}, {1, 0}}
23

18
— is a relation number with a list {{25, 18}, {175, -54}, {325, 54}, {1, 0}}
25

18
— is a relation number with a list
29
  {{29, 36}, {203, -36}, {377, 108}, {1537, 270}, {2407, -360}, {3277, 270},
  {1073, -162}, {1769, 306}, {1943, -432}, {6235, -918}, {5539, -882},
  {7163, 1098}, {15167, -3600}, {22243, 6048}, {56521, 18}, {1, 0}}

18
— is a relation number with a list
31
  {{31, 36}, {155, -36}, {341, 72}, {589, 162}, {1829, 288}, {3131, -162},
  {1643, -252}, {3751, -900}, {4681, -720}, {11129, 2934}, {18817, -3546},
  {33697, 7470}, {113243, 31446}, {388771, -71874}, {911431, -111222},
  {671305, 60228}, {272707, -33084}, {249085, -13194}, {49631, 5562},
  {13237, -3330}, {2573, 144}, {589, -18}, {155, 18}, {217, -54}, {1, 0}}

18
— is a relation number with a list
43
  {{43, 36}, {301, 36}, {559, -90}, {817, -108}, {2021, 414}, {2107, -162}, {1, 0}}

18
— is a relation number with a list {{47, 54}, {329, -18}, {235, -36}, {799, -144},
47
  {3055, -252}, {1457, -126}, {2585, -18}, {329, -36}, {235, 18}, {1, 0}}

18
— is a relation number with a list {{49, 54}, {245, -36}, {1, 0}}
49

```

```

18
— is a relation number with a list {{83, 90}, {581, -36}, {415, -18}, {1, 0}}
83

18
— is a relation number with a list {{95, 90}, {1, 0}}
95

known cases

known cases

known cases

known cases

19
— is a relation number with a list {{7, 19}, {84, 95}, {77, -38}, {1, 0}}
7

19
— is a relation number with a list {{8, 19}, {88, 57}, {104, 19}, {72, -19}, {1, 0}}
8

19
— is a relation number with a list
11
  {{11, 19}, {88, -57}, {286, 133}, {220, -57}, {88, 19}, {77, 57},
  {220, -133}, {506, -285}, {704, -513}, {2101, 1615}, {5346, -703},
  {3058, 2451}, {6677, 3895}, {12243, -551}, {121, 76}, {341, -247},
  {1034, 855}, {1969, -798}, {4103, -1691}, {7931, -4902}, {20603, -17252},
  {36861, 1235}, {2079, 779}, {2838, 1235}, {4048, -399}, {638, 19}, {88, -57}}

19
— is a relation number with a list {{12, 19}, {42, 19}, {1, 0}}
12

19
— is a relation number with a list
26
  {{26, 19}, {91, -19}, {52, 19}, {130, -19}, {78, -19}, {1, 0}}

19
— is a relation number with a list {{27, 19}, {72, 19}, {108, 19}, {54, 19}, {1, 0}}
27

19
— is a relation number with a list {{30, 38}, {60, 19}, {1, 0}}
30

19
— is a relation number with a list {{31, 38}, {217, 19}, {248, -19}, {1, 0}}
31

known cases

known cases

20
— is a relation number with a list {{9, 20}, {99, 40}, {171, -20}, {1, 0}}
9

20
— is a relation number with a list
11
  {{11, 20}, {99, -40}, {209, -60}, {319, -80}, {1, 0}}

20
— is a relation number with a list {{29, 20}, {261, 40}, {551, -20}, {261, 40}}
29

20
— is a relation number with a list {{31, 40}, {279, 20}, {1, 0}}
31

20
— is a relation number with a list {{51, 60}, {1, 0}}
51

20
— is a relation number with a list {{69, 60}, {1, 0}}
69

```



known cases

known cases

known cases

known cases

$\frac{21}{8}$  is a relation number with a list  $\{\{8, 21\}, \{104, 105\}, \{1, 0\}\}$

$\frac{21}{13}$  is a relation number with a list  $\{\{13, 21\}, \{104, 63\}, \{286, 105\}, \{377, -147\}, \{832, 567\}, \{3445, 1806\}, \{2171, 1071\}, \{377, -84\}, \{533, -231\}, \{923, -21\}, \{1, 0\}\}$

$\frac{21}{29}$  is a relation number with a list  $\{\{29, 21\}, \{232, -63\}, \{580, 147\}, \{232, -63\}\}$

$\frac{21}{34}$  is a relation number with a list  $\{\{34, 42\}, \{68, 21\}, \{170, -21\}, \{1, 0\}\}$

$\frac{21}{55}$  is a relation number with a list  $\{\{55, 63\}, \{440, 63\}, \{1, 0\}\}$

$\frac{21}{97}$  is a relation number with a list  $\{\{97, 105\}, \{776, 63\}, \{1940, -189\}, \{4850, -483\}, \{1940, 189\}\}$

$\frac{21}{113}$  is a relation number with a list  $\{\{113, 105\}, \{904, -63\}, \{2486, -189\}, \{3277, -42\}, \{1, 0\}\}$

known cases

known cases

known cases

known cases

known cases

$\frac{22}{9}$  is a relation number with a list  $\{\{9, 22\}, \{117, 88\}, \{261, 154\}, \{423, -352\}, \{639, -44\}, \{63, -22\}, \{1, 0\}\}$

$\frac{22}{13}$  is a relation number with a list  $\{\{13, 22\}, \{117, -88\}, \{377, 132\}, \{247, -44\}, \{221, -176\}, \{585, -308\}, \{403, -88\}, \{481, 330\}, \{1963, 968\}, \{351, 110\}, \{273, 44\}, \{117, -22\}, \{91, 22\}, \{39, 22\}, \{65, 44\}, \{273, 110\}, \{689, 264\}, \{1339, 1100\}, \{3107, -1474\}, \{2067, -1672\}, \{5135, 4334\}, \{10413, 3476\}, \{195, 22\}, \{39, -22\}\}$

$\frac{22}{17}$  is a relation number with a list  $\{\{17, 22\}, \{85, -44\}, \{51, 22\}, \{119, 66\}, \{221, 22\}, \{1, 0\}\}$

$\frac{22}{27}$  is a relation number with a list  $\{\{27, 22\}, \{135, 44\}, \{1, 0\}\}$

$\frac{22}{31}$  is a relation number with a list  $\{\{31, 22\}, \{279, 88\}, \{465, 88\}, \{775, -22\}, \{155, -22\}, \{1, 0\}\}$

```

 $\frac{22}{35}$  is a relation number with a list  $\{\{35, 44\}, \{315, 44\}, \{1, 0\}\}$ 
 $\frac{22}{39}$  is a relation number with a list
 $\{\{39, 44\}, \{195, 44\}, \{741, 44\}, \{273, -22\}, \{117, -22\}, \{91, 22\}, \{1, 0\}\}$ 
 $\frac{22}{53}$  is a relation number with a list
 $\{\{53, 44\}, \{477, -44\}, \{371, 22\}, \{159, 22\}, \{265, -44\}, \{1, 0\}\}$ 
 $\frac{22}{57}$  is a relation number with a list  $\{\{57, 66\}, \{1, 0\}\}$ 
 $\frac{22}{61}$  is a relation number with a list
 $\{\{61, 66\}, \{305, 44\}, \{183, 22\}, \{427, -44\}, \{793, 110\}, \{1403, 132\}, \{2989, -506\},$   

 $\{2867, -154\}, \{3599, 308\}, \{5917, 418\}, \{3965, -242\}, \{5673, -440\},$   

 $\{2867, -44\}, \{427, -66\}, \{1891, 66\}, \{1403, 22\}, \{305, -22\}, \{183, 22\}\}$ 
 $\frac{22}{75}$  is a relation number with a list  $\{\{75, 66\}, \{1, 0\}\}$ 
 $\frac{22}{105}$  is a relation number with a list  $\{\{105, 110\}, \{1, 0\}\}$ 
 $\frac{22}{233}$  is a relation number with a list
 $\{\{233, 242\}, \{2097, 44\}, \{3495, -22\}, \{699, -22\}, \{1165, -44\},$   

 $\{4893, -88\}, \{8155, -286\}, \{32387, -638\}, \{35183, -836\}, \{16543, 462\},$   

 $\{20737, 44\}, \{3029, -44\}, \{1631, -66\}, \{4427, -88\}, \{6291, 286\}, \{1, 0\}\}$ 
 $\frac{22}{247}$  is a relation number with a list
 $\{\{247, 242\}, \{1235, 44\}, \{741, -22\}, \{1729, 44\}, \{1, 0\}\}$ 
known cases
known cases
known cases
known cases
known cases
known cases
known cases
known cases
known cases
known cases
 $\frac{23}{7}$  is a relation number with a list
 $\{\{7, 23\}, \{112, 207\}, \{665, 736\}, \{497, -253\}, \{63, -92\}, \{203, -23\}, \{28, -23\},$   

 $\{35, -46\}, \{77, 69\}, \{56, -69\}, \{91, -115\}, \{168, 253\}, \{595, 184\}, \{301, 299\}, \{14, 23\},$   

 $\{63, 46\}, \{119, -69\}, \{133, 46\}, \{35, 23\}, \{77, 92\}, \{105, 46\}, \{91, 23\}, \{1, 0\}\}$ 
 $\frac{23}{9}$  is a relation number with a list
 $\{\{9, 23\}, \{126, 115\}, \{99, 23\}, \{63, 46\}, \{153, 23\}, \{72, -23\}, \{1, 0\}\}$ 

```

```

23
— is a relation number with a list
10
  {{10, 23}, {130, 69}, {40, 23}, {30, 23}, {70, 69}, {1, 0}}

23
— is a relation number with a list {{13, 23}, {130, -69}, {104, -23}, {143, 46},
13
  {65, 23}, {52, -23}, {78, -23}, {117, -92}, {325, -46}, {39, 23}, {91, 23}, {1, 0}}

23
— is a relation number with a list
14
  {{14, 23}, {63, 46}, {119, -69}, {133, 46}, {35, 23}, {154, -69}, {112, 69},
  {182, 115}, {336, -253}, {581, 138}, {406, -69}, {56, 23}, {35, 23}}

23
— is a relation number with a list {{16, 23}, {56, -23}, {40, 23}, {48, 23}, {1, 0}}
16

23
— is a relation number with a list {{18, 23}, {45, 23}, {1, 0}}
18

23
— is a relation number with a list {{28, 23}, {70, -23}, {1, 0}}
28

23
— is a relation number with a list {{30, 23}, {105, 23}, {1, 0}}
30

23
— is a relation number with a list {{32, 23}, {72, -23}, {96, 23}, {1, 0}}
32

23
— is a relation number with a list
33
  {{33, 23}, {110, 23}, {165, 46}, {209, -69}, {66, 23}, {1, 0}}

23
— is a relation number with a list {{36, 46}, {180, -23}, {1, 0}}
36

23
— is a relation number with a list
37
  {{37, 46}, {333, -46}, {407, 69}, {259, 23}, {222, 23}, {296, 69}, {740, -207},
  {3256, -437}, {7289, 1955}, {19647, 943}, {5772, 989}, {5994, 667}, {333, -46}}

23
— is a relation number with a list {{39, 46}, {273, -23}, {1, 0}}
39

23
— is a relation number with a list {{41, 46}, {205, -46}, {861, 46},
41
  {533, -92}, {779, -161}, {1066, 23}, {328, 23}, {246, -23}, {287, -23},
  {451, 69}, {1312, 115}, {1927, 391}, {1148, 69}, {1025, 46}, {533, 92}}

23
— is a relation number with a list {{51, 46}, {255, 46}, {357, 23},
51
  {561, 92}, {153, -23}, {136, 23}, {102, 23}, {510, 23}, {204, -23}, {1, 0}}

23
— is a relation number with a list {{55, 46}, {495, 46}, {1, 0}}
55

23
— is a relation number with a list {{56, 46}, {280, 23}, {1, 0}}
56

23
— is a relation number with a list
59
  {{59, 69}, {590, 69}, {1829, 207}, {2006, 299}, {5133, 368}, {1121, 138},
  {1003, -69}, {1888, -345}, {9617, -1610}, {2537, 46}, {413, -23}, {1, 0}}

```

$\frac{23}{60}$  is a relation number with a list  $\{\{60, 69\}, \{1, 0\}\}$

$\frac{23}{64}$  is a relation number with a list  $\{\{64, 69\}, \{160, -23\}, \{1, 0\}\}$

$\frac{23}{74}$  is a relation number with a list  $\{\{74, 69\}, \{185, 23\}, \{1, 0\}\}$

$\frac{23}{78}$  is a relation number with a list  $\{\{78, 69\}, \{1, 0\}\}$

$\frac{23}{110}$  is a relation number with a list  $\{\{110, 115\}, \{1, 0\}\}$

known cases

known cases

known cases

known cases

known cases

known cases

$\frac{25}{7}$  is a relation number with a list

$\{\{7, 25\}, \{126, 275\}, \{1043, 1800\}, \{5299, 6325\}, \{7182, 7025\}, \{1099, -1850\},$   
 $\{5257, -5825\}, \{3976, -1825\}, \{2282, 3525\}, \{8701, 6400\}, \{16107, -12725\},$   
 $\{23674, -4525\}, \{7343, -5450\}, \{13251, 9175\}, \{28532, -37675\},$   
 $\{64001, 35150\}, \{44093, 68900\}, \{173649, 137875\}, \{250418, 70775\},$   
 $\{228774, 321625\}, \{649957, 69900\}, \{145999, -32125\}, \{102382, -140775\},$   
 $\{268751, 25600\}, \{89257, -139575\}, \{352226, -280925\}, \{499107, -183950\},$   
 $\{369201, -30925\}, \{13293, -20900\}, \{53249, -43875\}, \{65618, -72775\},$   
 $\{50099, -27350\}, \{32207, -38600\}, \{44751, -49450\}, \{32893, -6275\},$   
 $\{10626, -5975\}, \{9268, 8725\}, \{3801, 6775\}, \{20818, 26925\}, \{42749, -35800\},$   
 $\{48643, -76875\}, \{197624, -167675\}, \{209643, 323725\}, \{798574, 585975\},$   
 $\{1488193, -1213150\}, \{1925301, -1615975\}, \{2165282, -3578675\},$   
 $\{9893751, -10284100\}, \{390349, 525375\}, \{945182, -301975\}, \{274799, -150975\},$   
 $\{190057, -300725\}, \{774676, -661625\}, \{791357, 1021175\}, \{1608726, -1402775\},$   
 $\{1441657, 478125\}, \{50974, 69975\}, \{133007, -14800\}, \{193, 325\}, \{924, 1025\},$   
 $\{707, 400\}, \{651, -475\}, \{1232, 1075\}, \{1099, -325\}, \{868, 825\}, \{301, 400\},$   
 $\{693, -325\}, \{301, -125\}, \{357, 400\}, \{301, 425\}, \{868, 125\}, \{1, 0\}\}$

$\frac{25}{9}$  is a relation number with a list

$\{\{9, 25\}, \{144, 175\}, \{279, -25\}, \{36, -25\}, \{99, 50\}, \{1, 0\}\}$

$\frac{25}{11}$  is a relation number with a list

$\{\{11, 25\}, \{154, 75\}, \{44, 25\}, \{66, 25\}, \{99, -50\}, \{1, 0\}\}$

$\frac{25}{14}$  is a relation number with a list

$\{\{14, 25\}, \{154, -75\}, \{28, 25\}, \{42, -25\}, \{56, -25\}, \{42, -25\}\}$

$\frac{25}{16}$  is a relation number with a list  $\{\{16, 25\}, \{72, 25\}, \{48, -25\}, \{1, 0\}\}$

```

25
— is a relation number with a list {{18, 25}, {42, 25}, {72, -25}, {1, 0}}
18
25
— is a relation number with a list {{32, 25}, {224, -75}, {1, 0}}
32
25
— is a relation number with a list {{34, 25}, {153, -25}, {102, -25}, {1, 0}}
34
25
— is a relation number with a list {{36, 25}, {132, 25}, {252, 25}, {1, 0}}
36
25
— is a relation number with a list {{39, 50}, {429, -25}, {156, 25}, {78, 25}, {1, 0}}
39
25
— is a relation number with a list
41
  {{41, 50}, {369, -25}, {246, -25}, {164, 25}, {451, 75}, {1, 0}}
25
— is a relation number with a list {{43, 50}, {301, -50}, {1, 0}}
43
25
— is a relation number with a list {{57, 50}, {399, 50}, {1, 0}}
57
25
— is a relation number with a list
61
  {{61, 50}, {671, 25}, {244, -25}, {366, 25}, {549, 50}, {1, 0}}
25
— is a relation number with a list
64
  {{64, 75}, {704, -125}, {1472, -25}, {192, 25}, {1, 0}}
25
— is a relation number with a list {{68, 75}, {476, -25}, {1, 0}}
68
25
— is a relation number with a list
86
  {{86, 75}, {946, 125}, {2322, 25}, {258, 25}, {344, -25}, {258, 25}}
known cases
known cases
known cases
known cases
known cases
known cases
26
— is a relation number with a list
7
  {{7, 26}, {133, 312}, {1253, 2470}, {8519, 14352}, {40831, 51194},
  {72541, -88920}, {114653, 196586}, {573531, 754156}, {1264375, -582842},
  {690837, 1052038}, {2528407, 2026960}, {3510129, 1151098}, {397845, 669136},
  {1899037, 2369614}, {3294039, -4352296}, {7407799, 2951390},
  {10124597, 16945916}, {47749233, 58732882}, {76885543, -125555300},
  {340688299, -386526582}, {320867981, 322095358}, {8591639, 11070436},
  {17351579, -13044330}, {30150743, 20678164}, {66308053, -101539906},
  {246622971, -205248836}, {289618945, -361014342}, {499767779, 670820072},
  {1197366051, -248380886}, {311768653, -577329506}, {1858925971, -2863275636},
  {7030447655, -6070161838}, {6722000719, 7443729618}, {5052102293, 4188746796},

```

```

{6043488479, 6873984650}, {5813473197, -4932091658}, {6169670773, 11307198422},
{35962693543, 54425329920}, {129238454639, 99051236362},
{211310527939, -91509020668}, {198047406221, 95041507002},
{55750745519, 44067956088}, {81779526017, 4723167410},
{10399760329, -5565509352}, {5118808625, 933129964}, {3172111635, -5250219182},
{14546752829, -17279261948}, {19127563833, -21135640552},
{14056537033, -8680500218}, {23131243821, -25152546952},
{14149121917, 18406184446}, {29799437703, -18159665368},
{45639251231, -42399561282}, {22677829643, 40130825722},
{122170972553, 172862118000}, {354838018129, 107934955622},
{217232058841, -51317243484}, {83741594335, -48180496858},
{88335795667, 9159094100}, {22786017331, 20520119958},
{15861281611, 25814176310}, {69670262893, 78076028004},
{58840355777, 109117482630}, {351939887971, 543382919768},
{1340101222579, 1173838388346}, {1163839839631, -428798661694},
{857893018157, -184869149868}, {465169118281, -433686961682},
{220375096193, 238335554522}, {125723208303, 199538784562},
{516709033813, 522433490800}, {40071198909, 63862605950},
{166539849287, 171538341416}, {34989444903, -31121231726},
{27077492239, -16701536878}, {44279070619, -47554361296},
{22927034739, -7749701336}, {2254484883, 4005103388},
{12254329535, 17480357414}, {36582195153, 13514222956},
{27723316005, 8372755898}, {18235338177, -9121964800}, {60139961, -32067828},
{27969865, 16698656}, {37992129, 24223030}, {73177517, 102240996},
{203444353, 39963482}, {25388601, -3157180}, {918127, -1639144},
{5047119, -7272434}, {15577205, -6951152}, {11724307, -5110638},
{10521217, 3304340}, {4257379, 7317258}, {21419153, 28336048},
{48418265, -18513066}, {49846531, -55552796}, {39943855, -56219098},
{113926701, -29622632}, {31946789, -29960580}, {13903463, -3158324},
{8891169, 10916074}, {14174335, -23764988}, {67134571, -83002062},
{111072437, 168459668}, {401710617, 312850330}, {622022009, -120415152},
{139623743, 194298884}, {382725987, 61461478}, {97699833, 67345252},
{212482067, -317802342}, {737241925, -513710756}, {1564718183, 2215835102},
{4557818433, 1418194180}, {2122651251, 2043226042}, {79425209, -21829392},
{55246513, -52395590}, {19956461, 3850860}, {4915127, 8699834},
{26492949, 37503544}, {77074165, 23750662}, {40755253, 14877980},
{27150809, -3299998}, {5255775, -3578536}, {11740673, 18558462},
{47724523, 47353280}, {2598701, 3294148}, {4868129, -4977414}, {764995, 744978},
{140119, 10426}, {32067, -46124}, {98399, -42614}, {92197, 44148}, {27307, 4758},
{8687, -1040}, {2569, 2262}, {2149, -130}, {427, -676}, {1743, -1742}, {1, 0}

```

26  
11 is a relation number with a list

```
{11, 26}, {165, 104}, {473, -26}, {55, -26}, {33, 26}, {77, -78}, {1, 0}
```

26  
15 is a relation number with a list

```
{15, 26}, {165, -104}, {645, 442}, {3045, 1352}, {5115, 2548}, {285, 182},
{1185, -676}, {2505, 1456}, {6105, -676}, {35, 26}, {45, -26}, {105, 26}, {1, 0}
```

```

26
19 is a relation number with a list
  {{19, 26}, {133, 52}, {437, 208}, {399, 130}, {171, -104}, {703, 52},
  {475, 312}, {2831, 1820}, {15371, 7488}, {7505, -1508}, {665, 442},
  {4161, -2704}, {23693, -13468}, {61617, 2938}, {1539, 1040},
  {9481, -6188}, {55005, -32968}, {207689, 57980}, {460389, 158392},
  {280953, 66248}, {303259, 13754}, {12749, -364}, {171, 104}}

26
33 is a relation number with a list {{33, 26}, {231, -52}, {253, 26}, {231, 52}}

26
37 is a relation number with a list
  {{37, 26}, {407, 104}, {333, -104}, {777, -26}, {111, 26}, {259, 52}, {1, 0}}

26
41 is a relation number with a list
  {{41, 52}, {451, -130}, {2501, -572}, {8733, -1300}, {15047, -3952},
  {31201, 3744}, {51209, -8866}, {81467, 1872}, {36941, -6474}, {78023, 18044},
  {239727, -20306}, {161745, 11986}, {243007, 29120}, {411927, -112190},
  {1510153, -188500}, {88273, -3536}, {5207, -312}, {3977, 182}, {1107, 260},
  {2747, 208}, {1763, -416}, {4059, 962}, {8651, 1040}, {13571, -390}, {3239, -442},
  {5945, 728}, {4961, 1534}, {14719, -2444}, {2255, -104}, {1353, -26}, {1, 0}}

26
45 is a relation number with a list {{45, 52}, {315, 26}, {1, 0}}

26
59 is a relation number with a list
  {{59, 52}, {413, -26}, {177, -26}, {295, -26}, {531, 104}, {649, 130}, {1, 0}}

26
63 is a relation number with a list
  {{63, 52}, {693, 130}, {387, 52}, {1449, 286}, {133, 26}, {1, 0}}

26
67 is a relation number with a list
  {{67, 78}, {737, -78}, {2345, 234}, {335, -52}, {1541, 104}, {1273, -52}, {1675, -234},
  {2479, -286}, {6365, -598}, {14271, 1300}, {1943, 364}, {8241, -1196}, {8777, -1612},
  {48039, 3848}, {124821, 15626}, {12529, -1612}, {24589, 3042}, {16951, -104}, {1, 0}}

26
71 is a relation number with a list
  {{71, 78}, {497, -78}, {2059, -260}, {1491, -104}, {2485, -104}, {781, -52}, {1, 0}}

26
85 is a relation number with a list
  {{85, 78}, {595, 78}, {2465, 156}, {2635, -364}, {7395, 728}, {1955, -182}, {3995, -416},
  {2805, 208}, {8585, -702}, {13685, -1066}, {2941, 130}, {4165, 416}, {1, 0}}

26
93 is a relation number with a list
  {{93, 104}, {1023, 52}, {1581, 26}, {465, 52}, {1, 0}}

26
115 is a relation number with a list
  {{115, 104}, {1265, -52}, {1955, 208}, {9545, 182}, {1863, -26}, {1035, -52}, {1, 0}}

```

```

26
119 is a relation number with a list
    {{119, 130}, {1309, -26}, {1071, -52}, {357, 26}, {1, 0}}

26
123 is a relation number with a list {{123, 130}, {861, 26}, {1, 0}}

26
279 is a relation number with a list {{279, 286}, {651, -26}, {1, 0}}

26
457 is a relation number with a list
    {{457, 468}, {5027, 52}, {7769, 104}, {14167, 26}, {1371, -26}, {3199, 52},
    {11425, 286}, {6855, -52}, {4113, -104}, {21479, -130}, {13253, 156}, {3199, 52}}

26
487 is a relation number with a list
    {{487, 494}, {3409, 26}, {1461, 26}, {2435, 52}, {4383, -52}, {7305, 26}, {1, 0}}

26
739 is a relation number with a list
    {{739, 728}, {8129, 26}, {6651, -26}, {3695, -26}, {2217, -26},
    {5173, 78}, {18475, -208}, {27343, -208}, {70205, -572}, {111589, -1300},
    {155929, 650}, {52469, -390}, {133759, 1144}, {65771, -806}, {237219, 3068},
    {726437, -7410}, {189923, 3250}, {1051597, -3120}, {116023, 650},
    {238697, 1664}, {550555, 9386}, {2378841, 10348}, {886061, -9542},
    {993955, -12402}, {1326505, -17758}, {3949955, 59982}, {6545323, -112554},
    {12704149, -41730}, {13471231, -31460}, {4693389, 33826}, {6226075, -25714},
    {2429093, -30082}, {5578711, 51636}, {1494997, 25454}, {5017071, 76492},
    {23205339, -194194}, {71130967, -862420}, {304857453, -4511962},
    {1445456657, -22092590}, {6974908873, 115106784}, {34441058789, -242902556},
    {37765976457, 129376754}, {8894390429, 146695510}, {39932368259, -228548528},
    {47018240199, 166140260}, {403951441, -627926}, {144121997, 2457702},
    {652109119, -3749044}, {165932843, -2488434}, {585461665, 5720936},
    {1423456627, 20966192}, {1658633031, 28455076}, {6088342397, 36289760},
    {6161252137, 61267752}, {19798412285, -391378}, {121770203, 2097394},
    {89678389, 807300}, {50317771, -1118}, {40645, -338}, {62815, -52}, {1, 0}}

26
761 is a relation number with a list {{761, 754}, {5327, -52},
    {17503, -104}, {23591, -156}, {26635, -416}, {8371, 26}, {1, 0}}

```

known cases

known cases

known cases

known cases

known cases

known cases

known cases

known cases



```

27
— is a relation number with a list
8
  {{8, 27}, {152, 297}, {1160, 1539}, {3032, -2079}, {7624, 9099}, {5900, 3429},
  {3832, -783}, {664, -459}, {1640, 1863}, {892, -1431}, {4312, -3105},
  {9656, 7749}, {15256, 10503}, {38024, -44307}, {25132, 7587},
  {18968, -3321}, {3832, 351}, {58, 81}, {184, -27}, {20, -27}, {56, 27}, {1, 0}}

27
— is a relation number with a list
10
  {{10, 27}, {170, 189}, {95, 81}, {70, 27}, {110, 27}, {1, 0}}

27
— is a relation number with a list {{11, 27}, {176, 135}, {451, 378}, {803, 216},
11
  {671, -729}, {638, 189}, {781, 162}, {319, -216}, {1133, 405}, {902, -27}, {1, 0}}

27
— is a relation number with a list {{16, 27}, {176, -135}, {328, 27}, {1, 0}}
16

27
— is a relation number with a list
17
  {{17, 27}, {170, 81}, {136, 81}, {442, 27}, {170, -81}}

27
— is a relation number with a list
19
  {{19, 27}, {152, -81}, {190, -81}, {532, -27}, {152, 81}}

27
— is a relation number with a list {{22, 27}, {55, -27}, {1, 0}}
22

27
— is a relation number with a list {{32, 27}, {80, 27}, {1, 0}}
32

27
— is a relation number with a list {{35, 27}, {280, 81}, {1295, -162}, {1, 0}}
35

27
— is a relation number with a list {{37, 27}, {370, -81}, {1295, 162}, {1, 0}}
37

27
— is a relation number with a list
38
  {{38, 27}, {418, 135}, {494, -135}, {874, 81}, {646, 135}, {1102, 351}, {931, 54},
  {247, -27}, {76, 27}, {95, 27}, {494, 27}, {152, -27}, {190, -27}, {1, 0}}

27
— is a relation number with a list {{43, 54}, {473, 54}, {559, 135},
43
  {817, 162}, {301, -27}, {172, 27}, {430, 81}, {1075, 108}, {215, -54}, {1, 0}}

27
— is a relation number with a list {{44, 54}, {220, 27}, {1, 0}}
44

27
— is a relation number with a list
46
  {{46, 54}, {92, 27}, {253, 27}, {115, -27}, {322, 81}, {1, 0}}

27
— is a relation number with a list {{49, 54}, {245, 54}, {1225, 54}, {833, 108},
49
  {1519, -270}, {4949, -405}, {4361, -621}, {98, 27}, {490, 27}, {196, 27}, {1, 0}}

```

```

27
— is a relation number with a list
59
{{59, 54}, {295, -54}, {1475, 189}, {2183, -162}, {4543, 837}, {21122, 1053},
{3658, 189}, {3953, 297}, {5428, 135}, {1652, -351}, {6077, 1242}, {7847, -1458},
{32863, 4212}, {49147, -1107}, {25901, 5805}, {158179, -19440}, {156881, 1728},
{21653, -2862}, {73337, 1053}, {22007, -1701}, {6254, 189}, {1003, 135}, {3422, 135},
{2773, 351}, {2065, 81}, {2360, 459}, {3835, 756}, {3245, 54}, {295, -54}}

27
— is a relation number with a list {{64, 54}, {320, -27}, {1, 0}}
64

27
— is a relation number with a list {{65, 54}, {715, -54}, {1, 0}}
65

27
— is a relation number with a list {{70, 81}, {770, -27}, {182, 27}, {1, 0}}
70

27
— is a relation number with a list
71
{{71, 81}, {710, -81}, {1349, 108}, {3763, 513}, {12212, -729}, {12851, -1998},
{61273, -2052}, {20377, -1539}, {26270, 621}, {13348, -1593}, {42884, 1053},
{20519, 3267}, {65107, 9126}, {86975, -13554}, {401221, -46872},
{1464517, -13662}, {190493, -28269}, {524690, 11799}, {392914, -58779},
{1316269, 168885}, {2471581, 227826}, {2449855, -337851}, {6027758, -1064961},
{25702568, -2581497}, {7980542, 1195047}, {27319877, -1734345},
{30504653, -4465476}, {53511209, -8540532}, {161029207, 5986818},
{43656409, 6580980}, {171142021, -11674341}, {282089674, -29310093},
{781799176, -110781}, {1253789, -236763}, {4968154, 193509}, {4478680, -113859},
{2710709, 162675}, {3888386, 279531}, {1778408, -234117}, {6711488, -1243485},
{35078473, 5090472}, {39393001, -1893024}, {25595713, -1865430},
{36941797, 6010929}, {62211833, 931581}, {14490674, -15795},
{472789, -42687}, {229472, 23463}, {366218, 5319}, {56303, 7749},
{146260, -6021}, {124676, -783}, {12709, 2403}, {49274, 1971}, {1, 0}}

27
— is a relation number with a list {{73, 81}, {584, -81}, {1241, 54}, {1, 0}}
73

27
— is a relation number with a list {{76, 81}, {190, 27}, {1, 0}}
76

27
— is a relation number with a list {{86, 81}, {215, -27}, {1, 0}}
86

27
— is a relation number with a list
92
{{92, 81}, {1012, 27}, {1196, 27}, {184, 27}, {230, -27}, {1196, 27}}

27
— is a relation number with a list {{98, 108}, {490, -27}, {196, 27}, {1, 0}}
98

27
— is a relation number with a list {{100, 108}, {1, 0}}
100

27
— is a relation number with a list
118
{{118, 108}, {590, 27}, {236, 27}, {826, 27}, {1298, 81}, {1, 0}}

```

```

27
125 is a relation number with a list
    {{125, 135}, {250, 27}, {875, -27}, {1375, -108}, {3625, 189},
    {4250, -243}, {14875, -1458}, {7375, 189}, {500, -27}, {325, -27}, {1, 0}}

27
127 is a relation number with a list
    {{127, 135}, {1016, -81}, {4699, 297}, {6731, -513}, {7874, 135}, {5588, 513},
    {6985, 189}, {1016, -27}, {1270, -81}, {3302, -243}, {12700, 1161}, {9017, 162},
    {6985, 216}, {9271, -162}, {4699, 405}, {20447, 729}, {4445, -27}, {1270, -81}}

27
130 is a relation number with a list {{130, 135}, {1, 0}}

27
143 is a relation number with a list {{143, 135}, {1144, 81}, {1430, -27}, {1, 0}}

27
145 is a relation number with a list {{145, 135}, {290, 27},
    {1015, 54}, {1595, -108}, {725, 27}, {580, -27}, {1885, -54}, {1, 0}}

27
197 is a relation number with a list {{197, 189}, {1576, 81}, {7289, -27}, {1, 0}}

27
199 is a relation number with a list {{199, 189}, {1990, 81}, {6965, -54}, {1, 0}}

27
233 is a relation number with a list {{233, 243}, {2330, 81}, {4427, 108}, {1, 0}}

27
251 is a relation number with a list
    {{251, 243}, {2008, 81}, {4267, -135}, {13303, -459}, {2008, 81}}

27
254 is a relation number with a list {{254, 243}, {1397, -27}, {889, 27}, {1, 0}}

27
260 is a relation number with a list {{260, 270}, {1, 0}}

27
286 is a relation number with a list {{286, 297}, {1, 0}}

27
287 is a relation number with a list
    {{287, 297}, {2870, 81}, {1435, -54}, {6601, -27}, {3731, -27}, {1435, -54}}

27
289 is a relation number with a list
    {{289, 297}, {2312, -81}, {10693, 432}, {30923, -621}, {36703, 1161},
    {129761, 3915}, {163574, 567}, {80342, -1269}, {6715, -243}, {25721, 540},
    {57511, -243}, {23120, -1053}, {13294, 27}, {2890, -27}, {1, 0}}

27
359 is a relation number with a list {{359, 351}, {2872, 81}, {13283, 108}, {1, 0}}

27
361 is a relation number with a list {{361, 351}, {3610, 81}, {12635, 54}, {1, 0}}

```

Individual verification is complete.

SCHOOL OF MATHEMATICS, KOREA INSTITUTE FOR ADVANCED STUDY (KIAS), SEOUL, 02455, KOREA

*Email address:* skim.math@gmail.com

*URL:* <http://cayley.kr>

DEPARTMENT OF MATHEMATICS, UNIVERSITY OF VIRGINIA, CHARLOTTESVILLE, VA 22904-4137, USA

*Email address:* thomas.koberda@gmail.com

*URL:* <http://faculty.virginia.edu/Koberda>
